# Supplementary material for: A deeper look at depth pruning of LLMs
Source: arXiv:2407.16286 source file (2024-07-23)
Supplement: Supplementary file 1 [file appendix.tex]

\clearpage
\appendix

\section{Remaining results}
\label{appendix:remaining_results}

We divide the remaining results into different sub-sections and add a reference to the figure in the text to make the identification clear.

\subsection{Results on other datasets}

\begin{figure}[t]
    \centering
    \includegraphics[width=\textwidth]{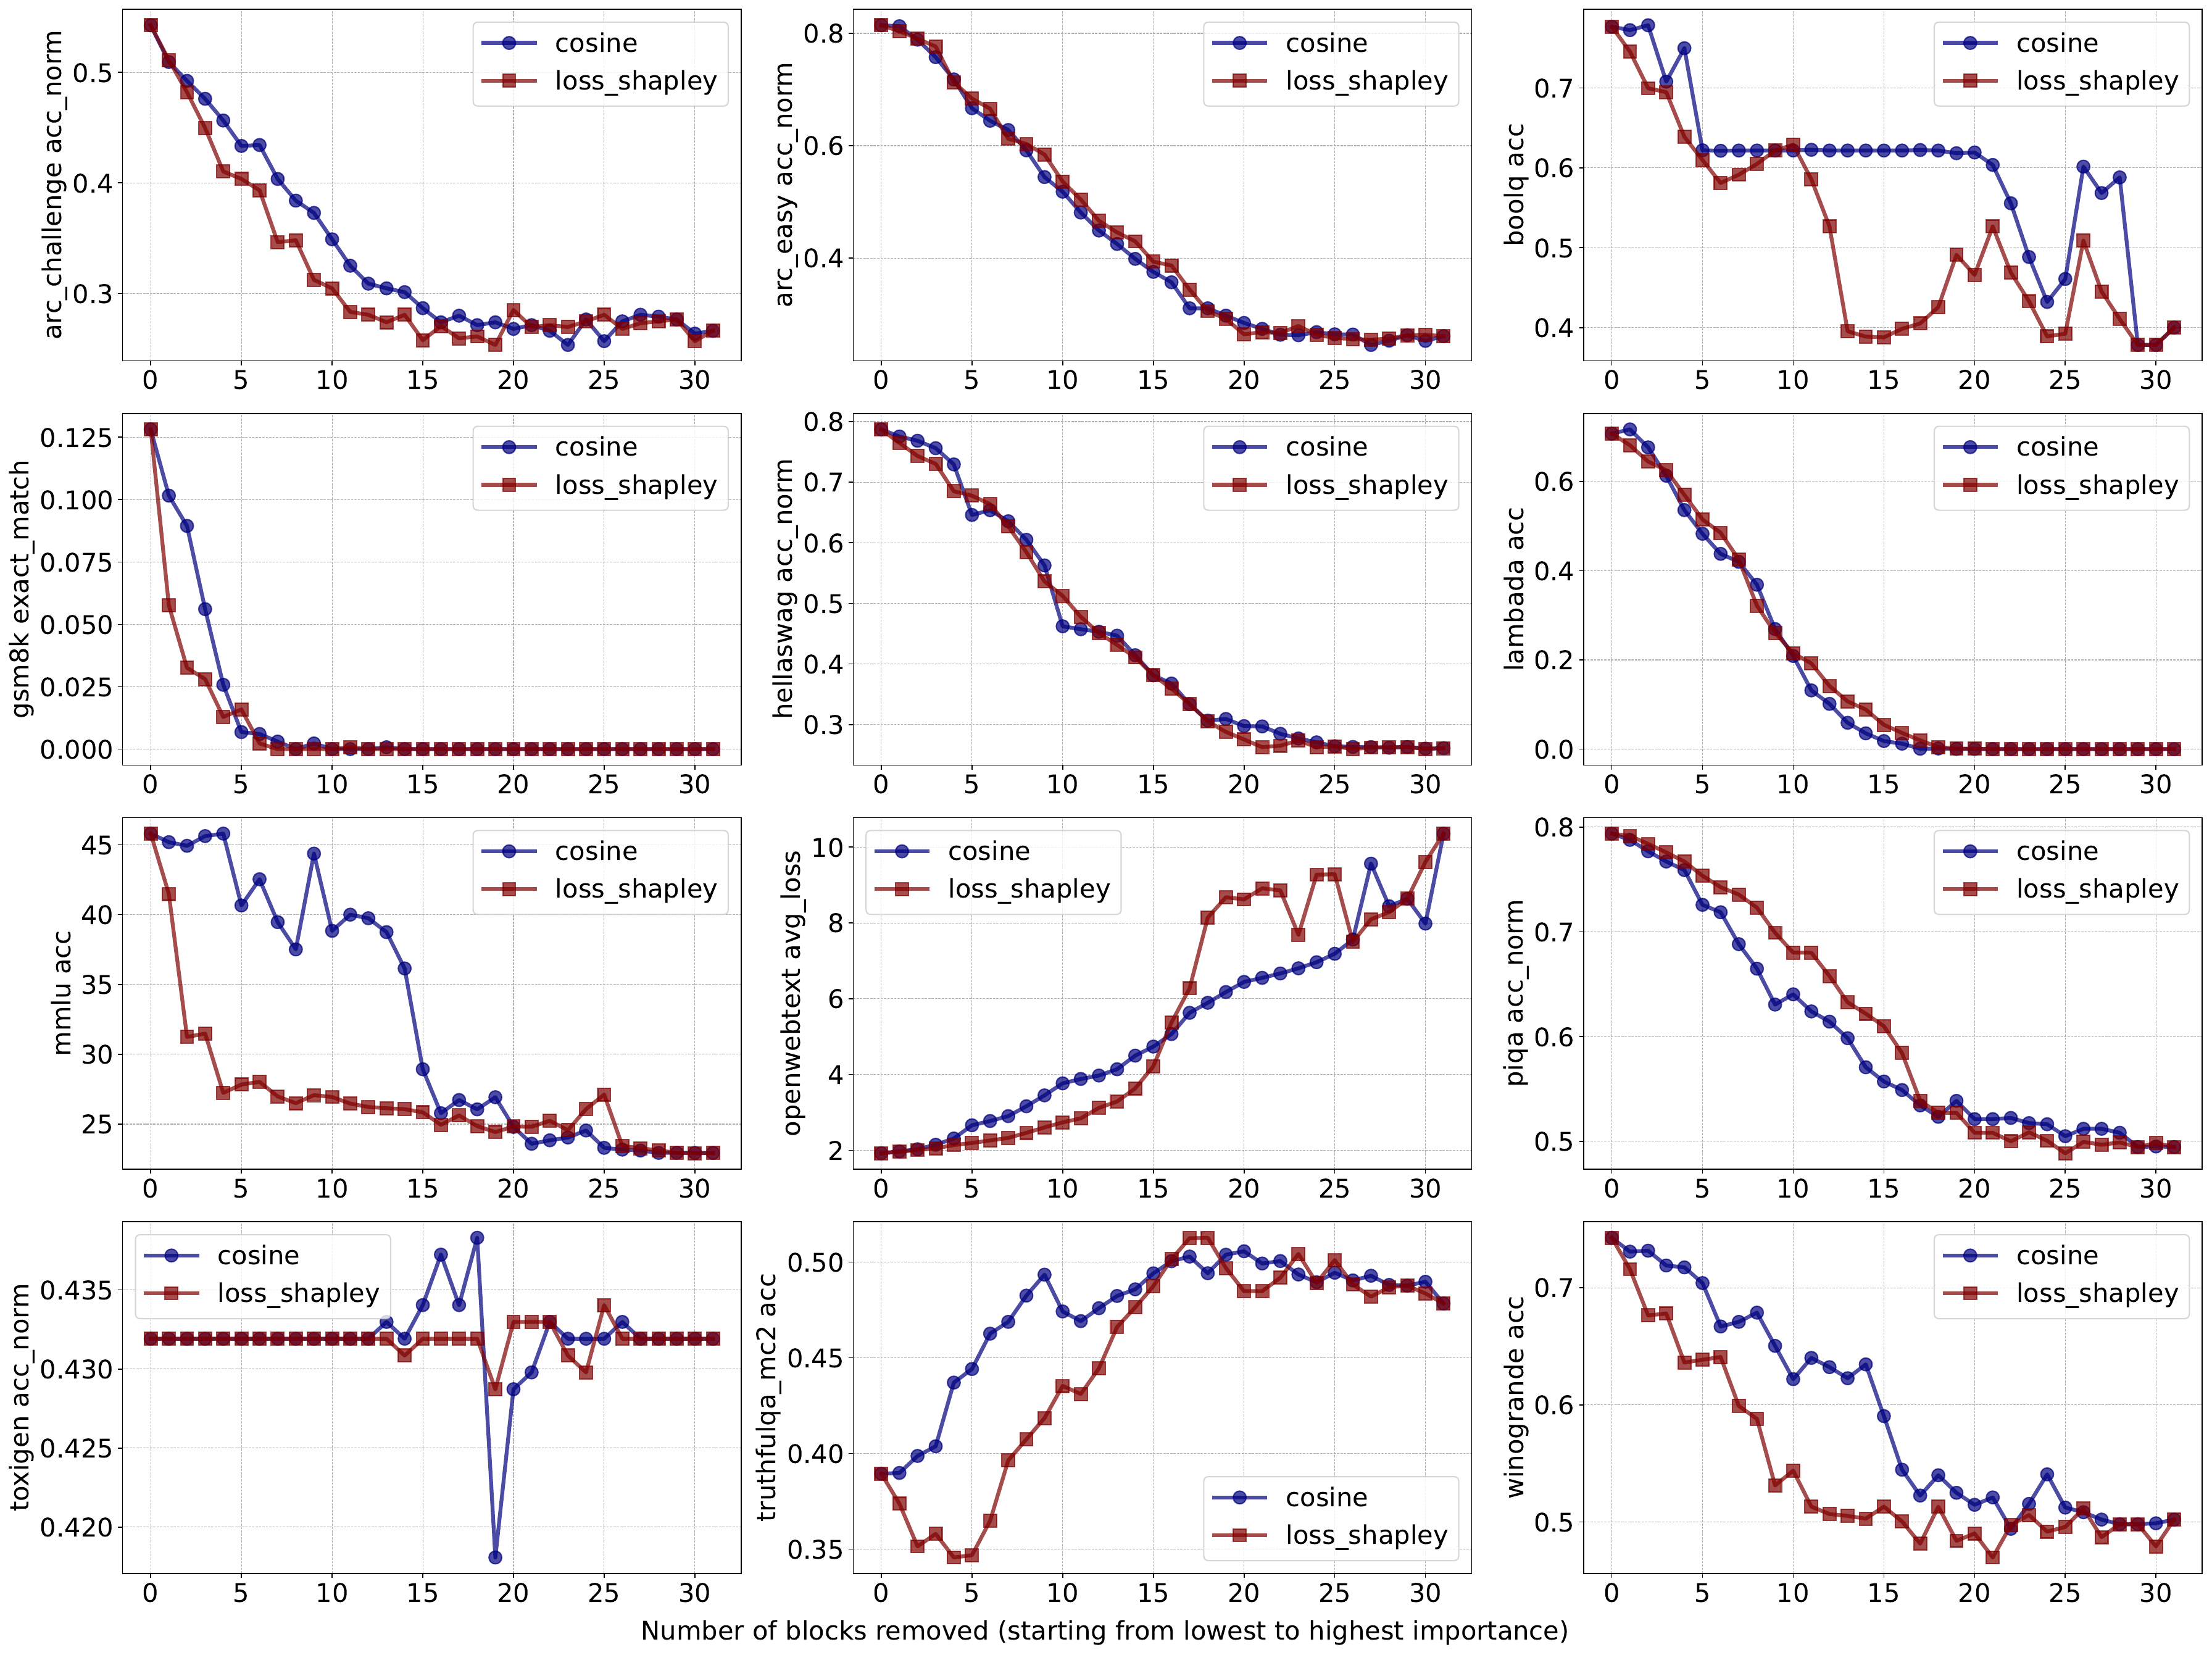}
    \caption{\textbf{LLaMa-2 7b evaluation on multiple datasets from eval-harness~\citep{eval-harness}}, highlighting the impact of pruning on some tasks is more significant (such as GSM-8k~\citep{cobbe2021gsm8k}) as compared to others.}
    \label{fig:llama2_harness}
\end{figure}

\begin{figure}[t]
    \centering
    \includegraphics[width=\textwidth]{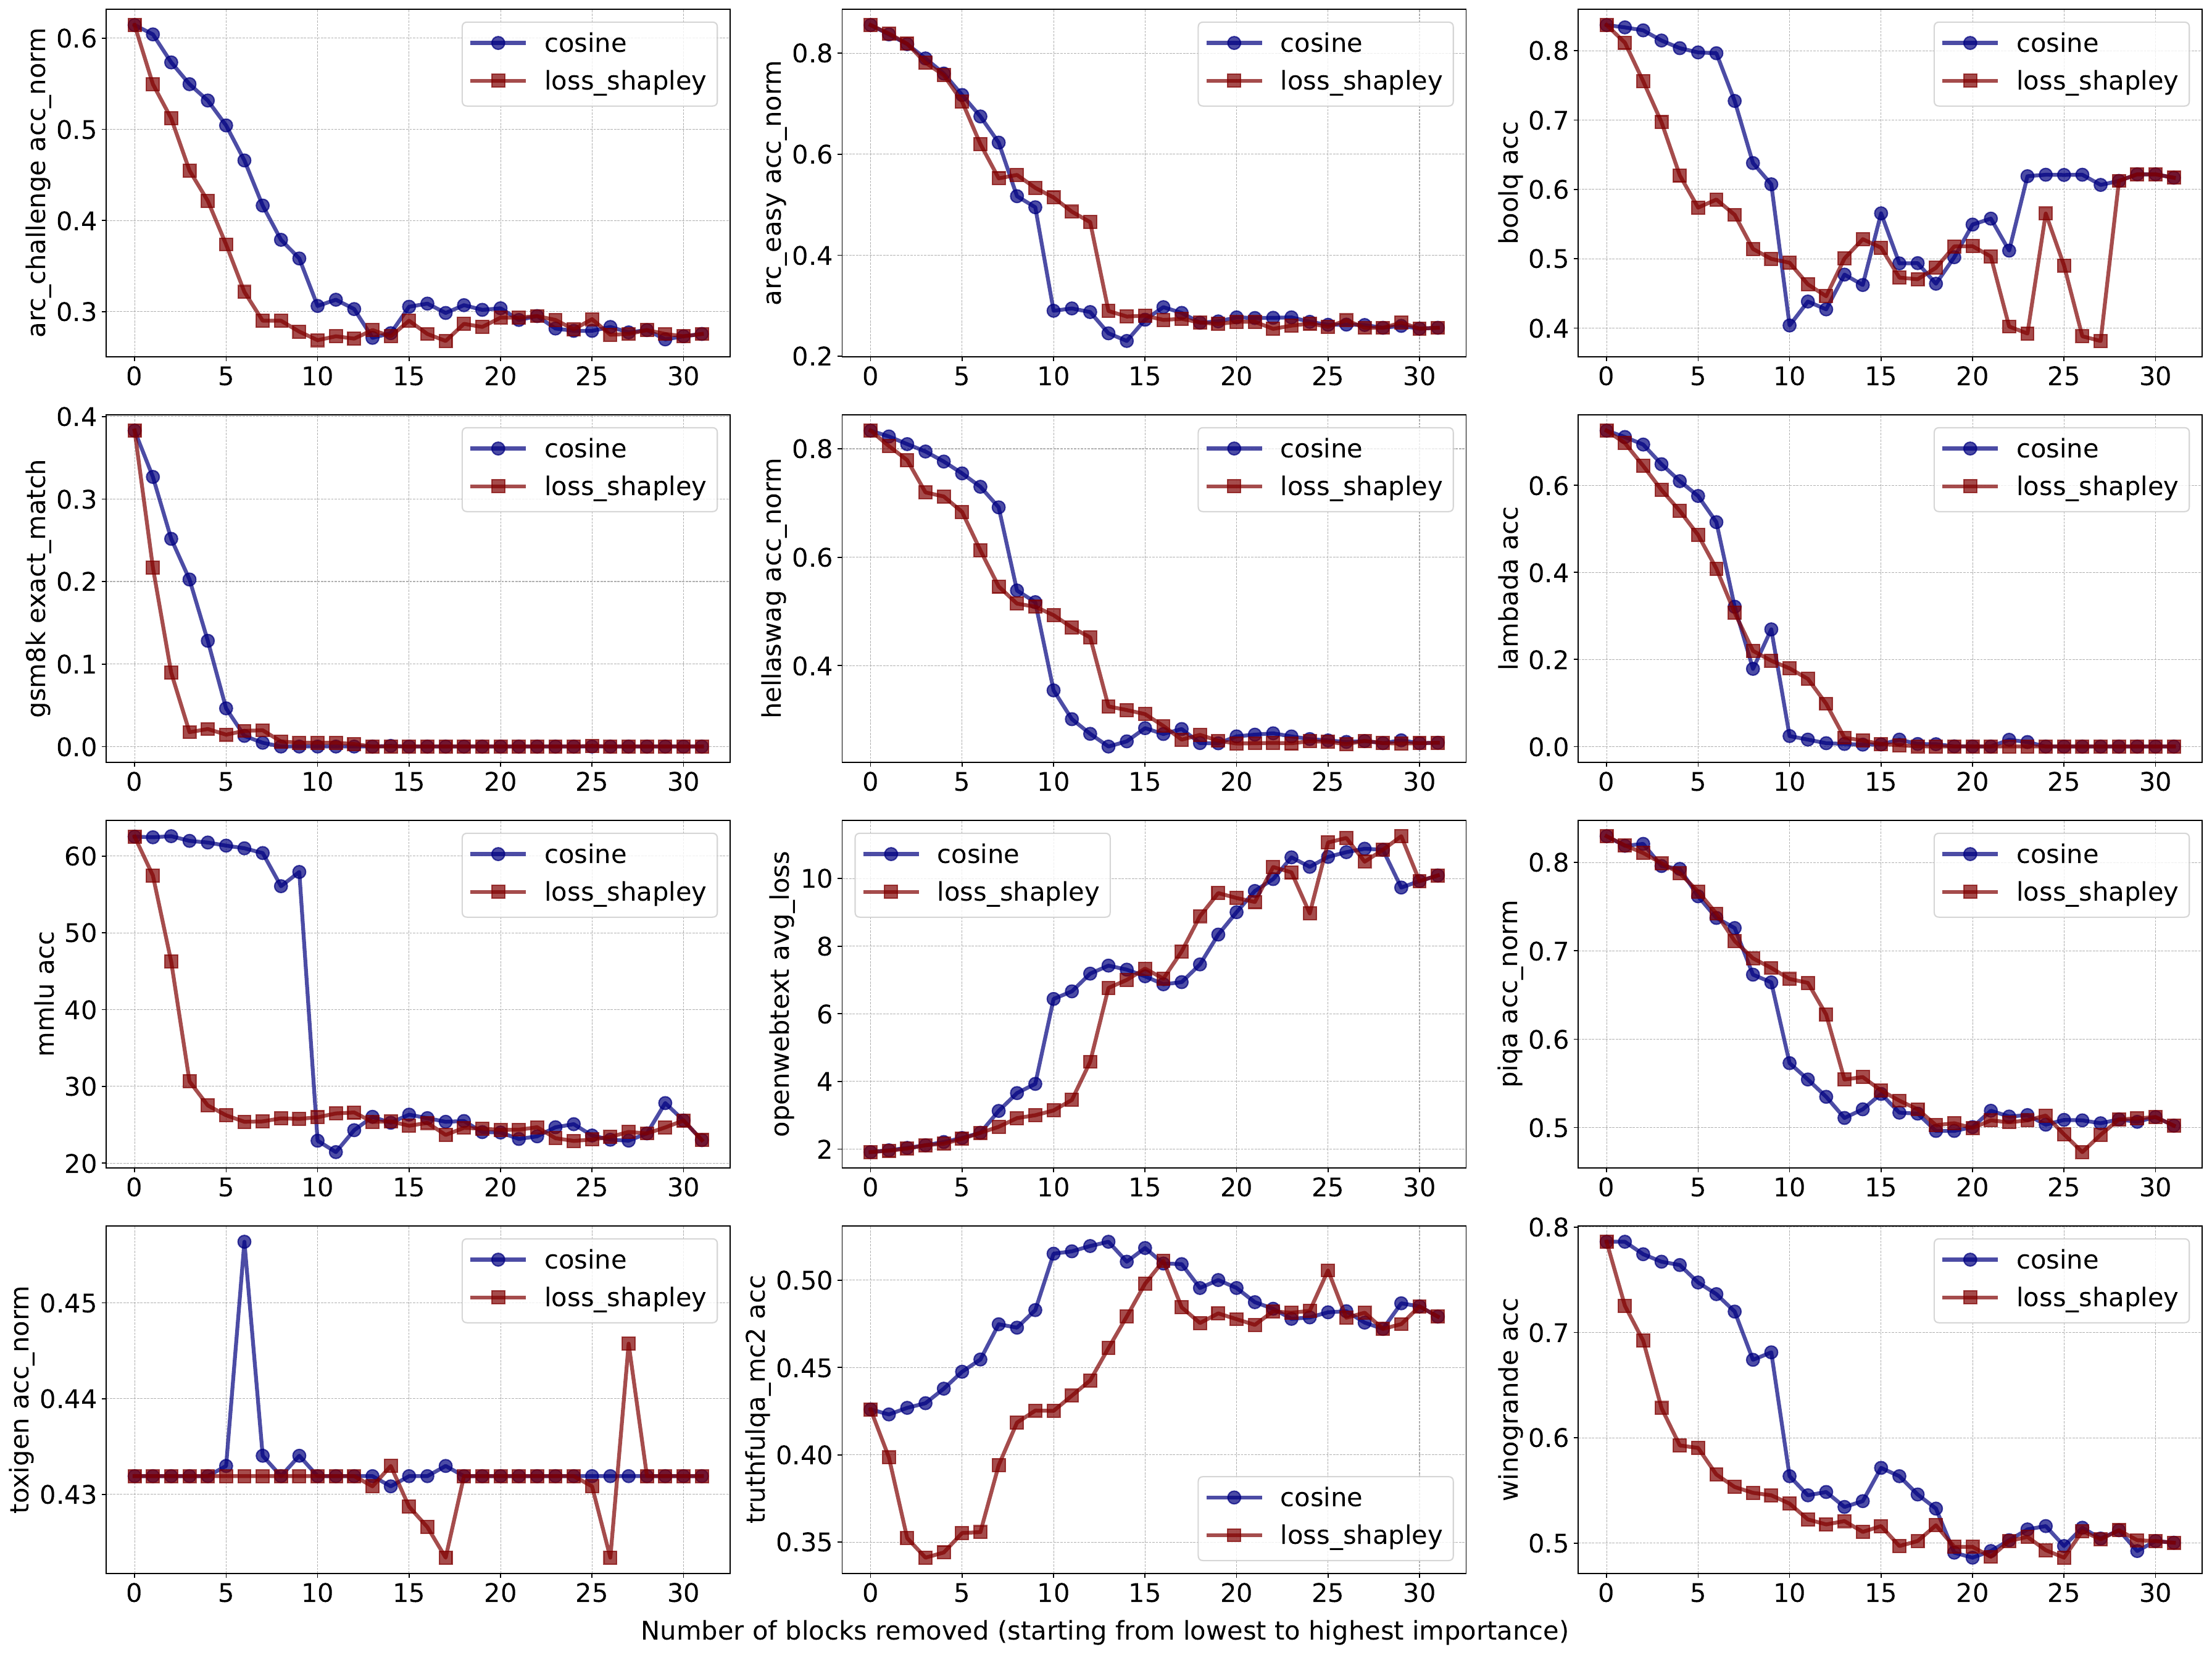}
    \caption{\textbf{Mistral-7b evaluation on multiple datasets from eval-harness~\citep{eval-harness}}, highlighting the impact of pruning on some tasks is more significant (such as GSM-8k~\citep{cobbe2021gsm8k}) as compared to others.}
    \label{fig:mistral_harness}
    \vspace{-5mm}
\end{figure}

We include tasks from OpenLLM leaderboard~\citep{open-llm-leaderboard} evaluated using lm-eval-harness package for reproducibility~\citep{eval-harness}.
In particular, we evaluate performance on MMLU~\citep{hendrycks2020mmlu}, GSM-8k~\citep{cobbe2021gsm8k}, ARC (easy as well as challenging)~\citep{clark2018arc}, BoolQ~\citep{clark2019boolq}, HellaSwag~\citep{zellers2019hellaswag}, Lambada~\citep{paperno2016lambada}, PiQA~\citep{bisk2020piqa}, Toxigen~\citep{hartvigsen2022toxigen}, TruthfulQA (MC2)~\citep{lin22truthfulqa}, and Winogrande~\citep{sakaguchi2019winogrande}.

Fig.~\ref{fig:llama2_harness} presents our results on LLaMa-2 7b~\citep{touvron2023llama2} while Fig.~\ref{fig:mistral_harness} presents the results on Mistral 7b~\citep{jiang2023mistral}.
We only plot the results for cosine block influence and loss shapley (computed on OpenWebText language modeling task).
The results highlight that the model suffers from performance degradation on some tasks such as GSM-8k~\citep{cobbe2021gsm8k} and ARC challenge~\citep{clark2018arc} even after pruning just a single block from the model.
This indicates that just looking at MMLU provides only a partial picture of the true impact of depth pruning on model performance.

\subsection{LLaMa-2 7b remaining results}
\label{appendix:llama_remaining_results}

\begin{figure}[t]
    \centering
    \subfloat{
        \includegraphics[width=\textwidth]{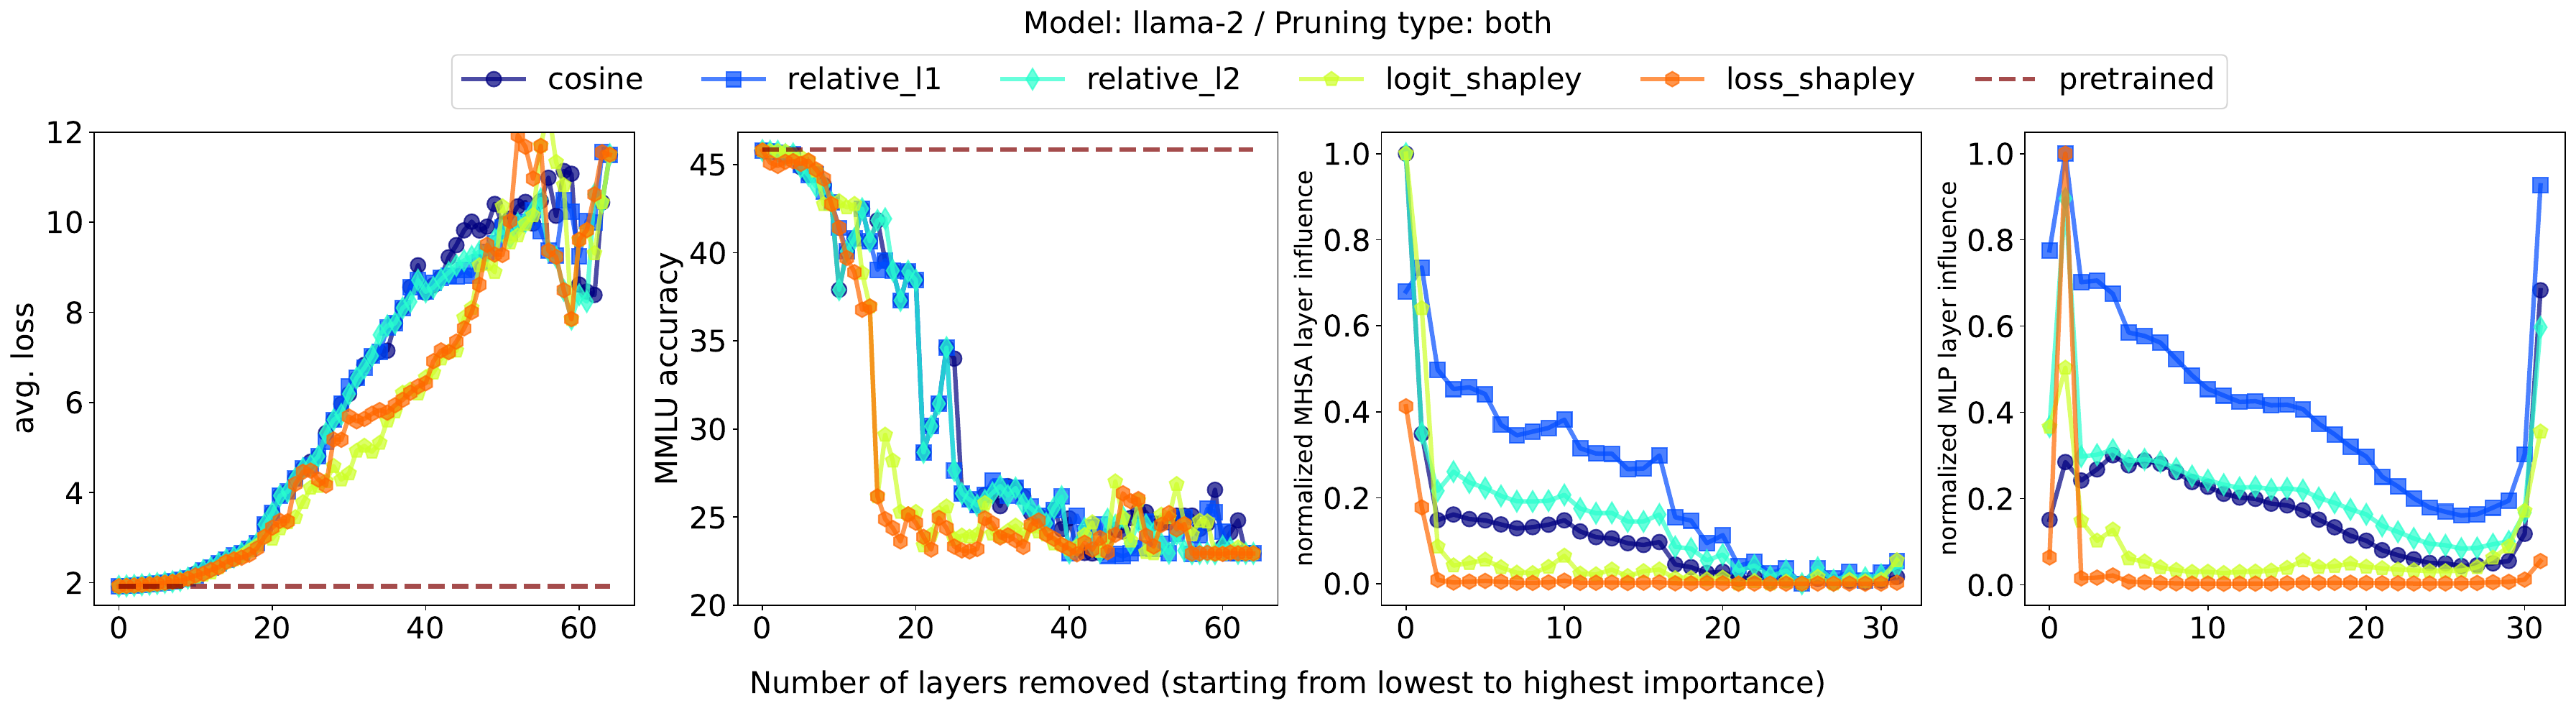}
    }

    \vspace{-3mm}
    \subfloat{
        \includegraphics[width=\textwidth]{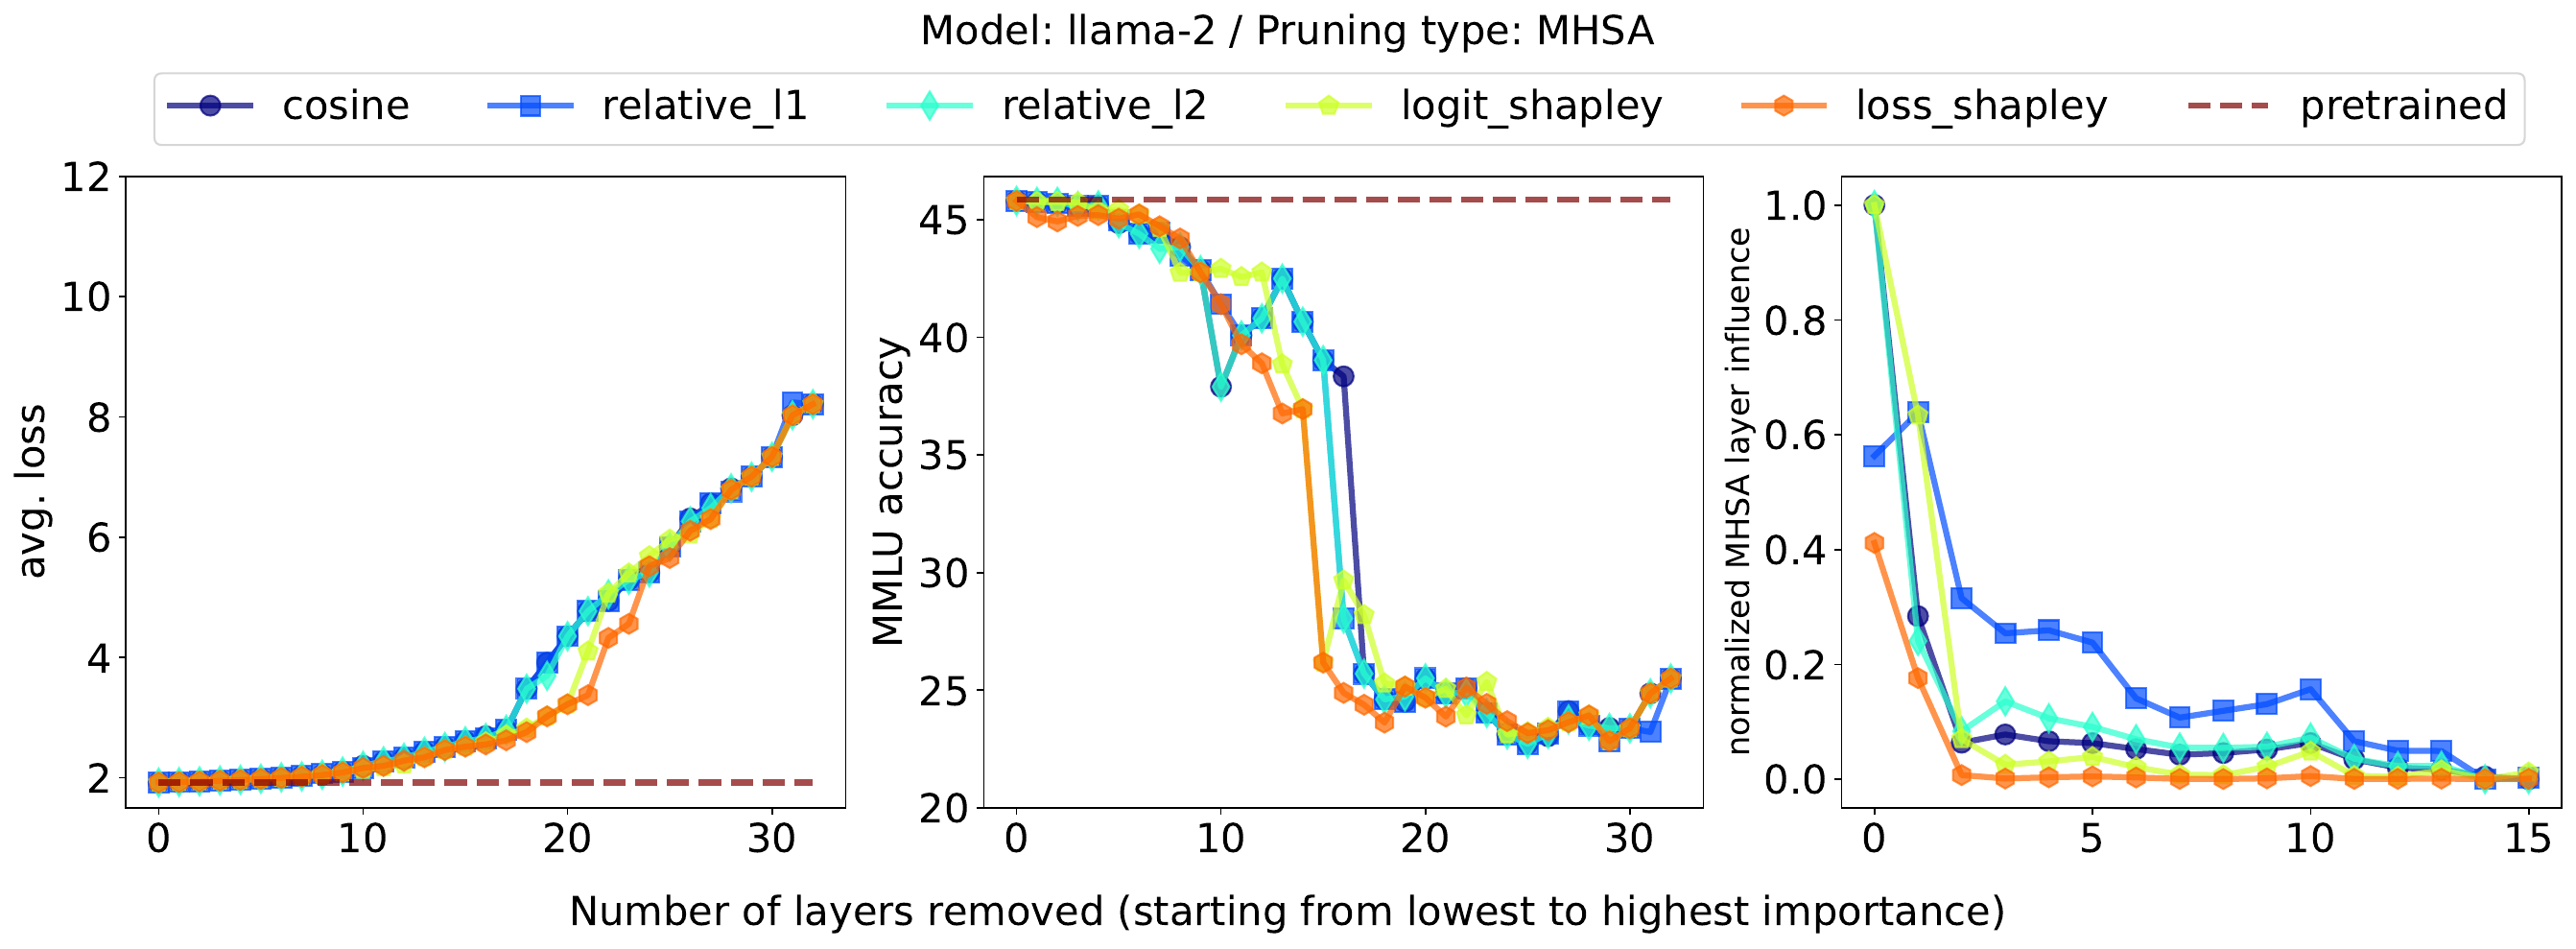}
    }

    \vspace{-3mm}
    \subfloat{
        \includegraphics[width=\textwidth]{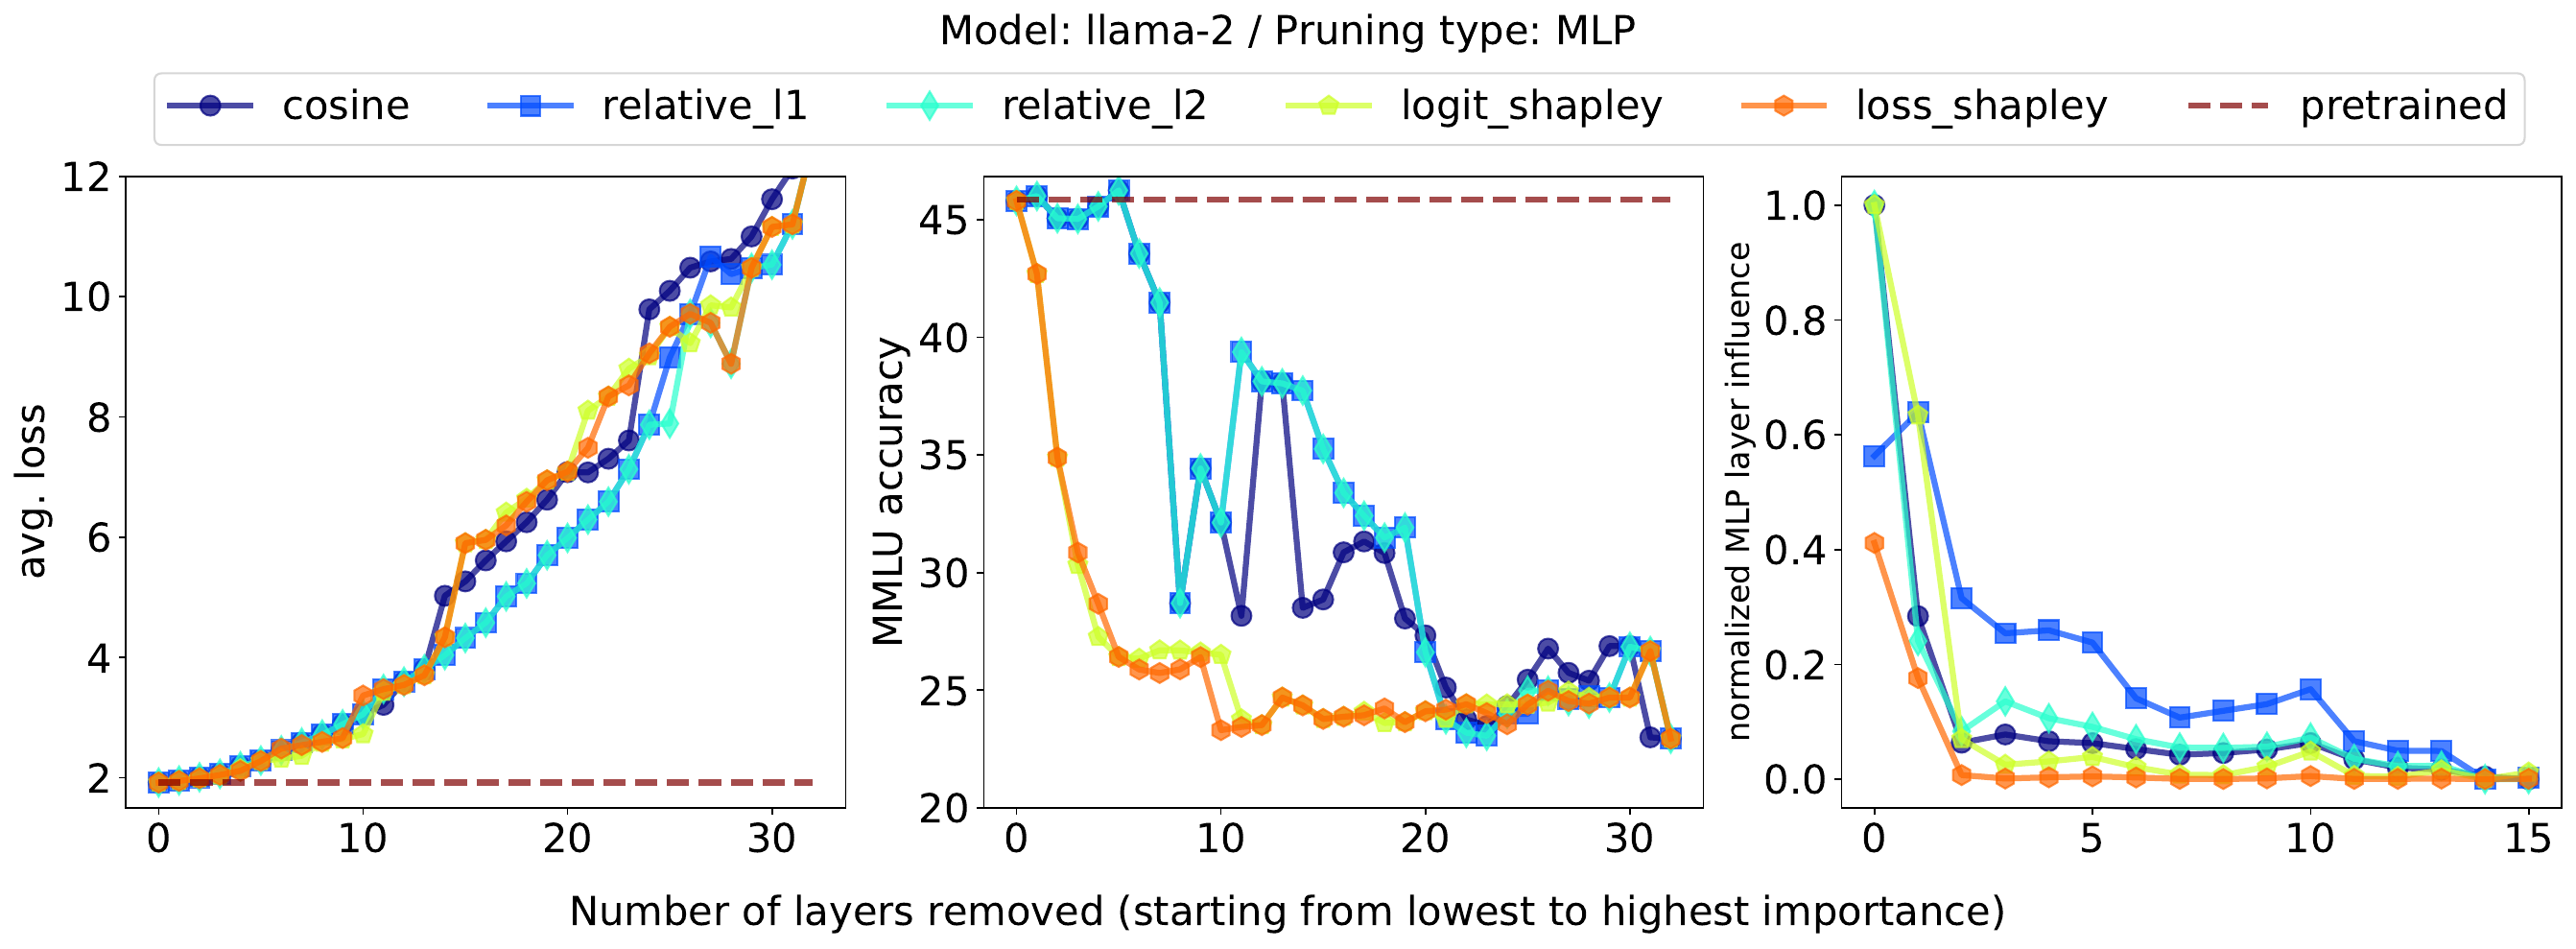}
    }
    \caption{\textbf{Comparison of different layer influence metrics on LLaMa-2 7b} (detailed in Section~\ref{subsec:block_inf_metrics}) and their impact on downstream performance in terms of average loss on a small curated validation set from OpenWebText and accuracy on MMLU. The first row highlights joint pruning, while the second and third row highlights pruning of just self-attention or feed-forward layer respectively.}
    \label{fig:layer_influence_llama2}
\end{figure}

The results for layer pruning of LLaMa-2 are visualized in Fig.~\ref{fig:layer_influence_llama2}, where we again see a higher propensity for the self-attention layers to be pruned in contrast to the feed-forward layers, albeit to a lesser extent.

\begin{figure}
    \centering
    \subfloat{
        \includegraphics[width=\textwidth]{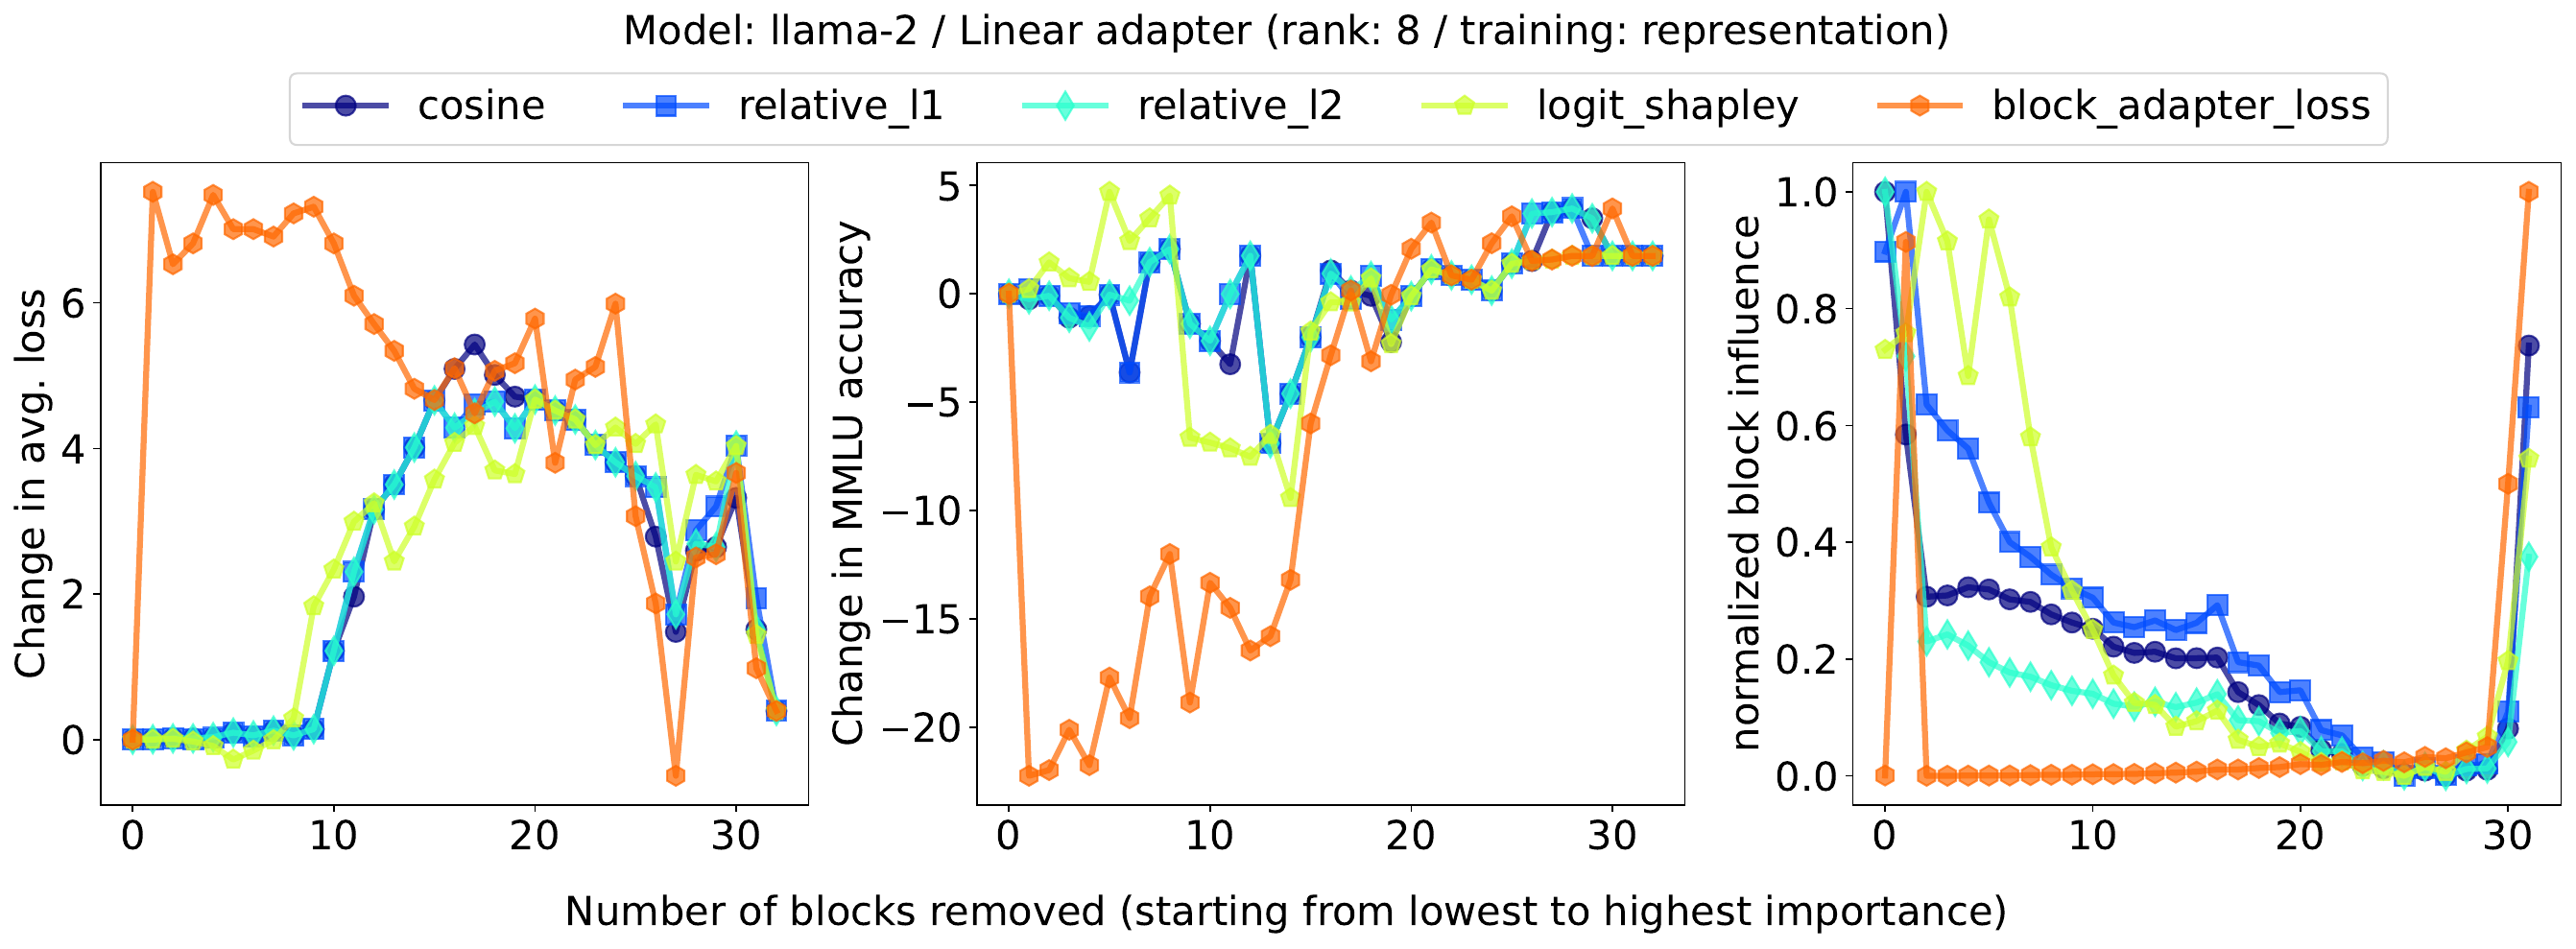}
    }

    \vspace{-3mm}
    \subfloat{
        \includegraphics[width=\textwidth]{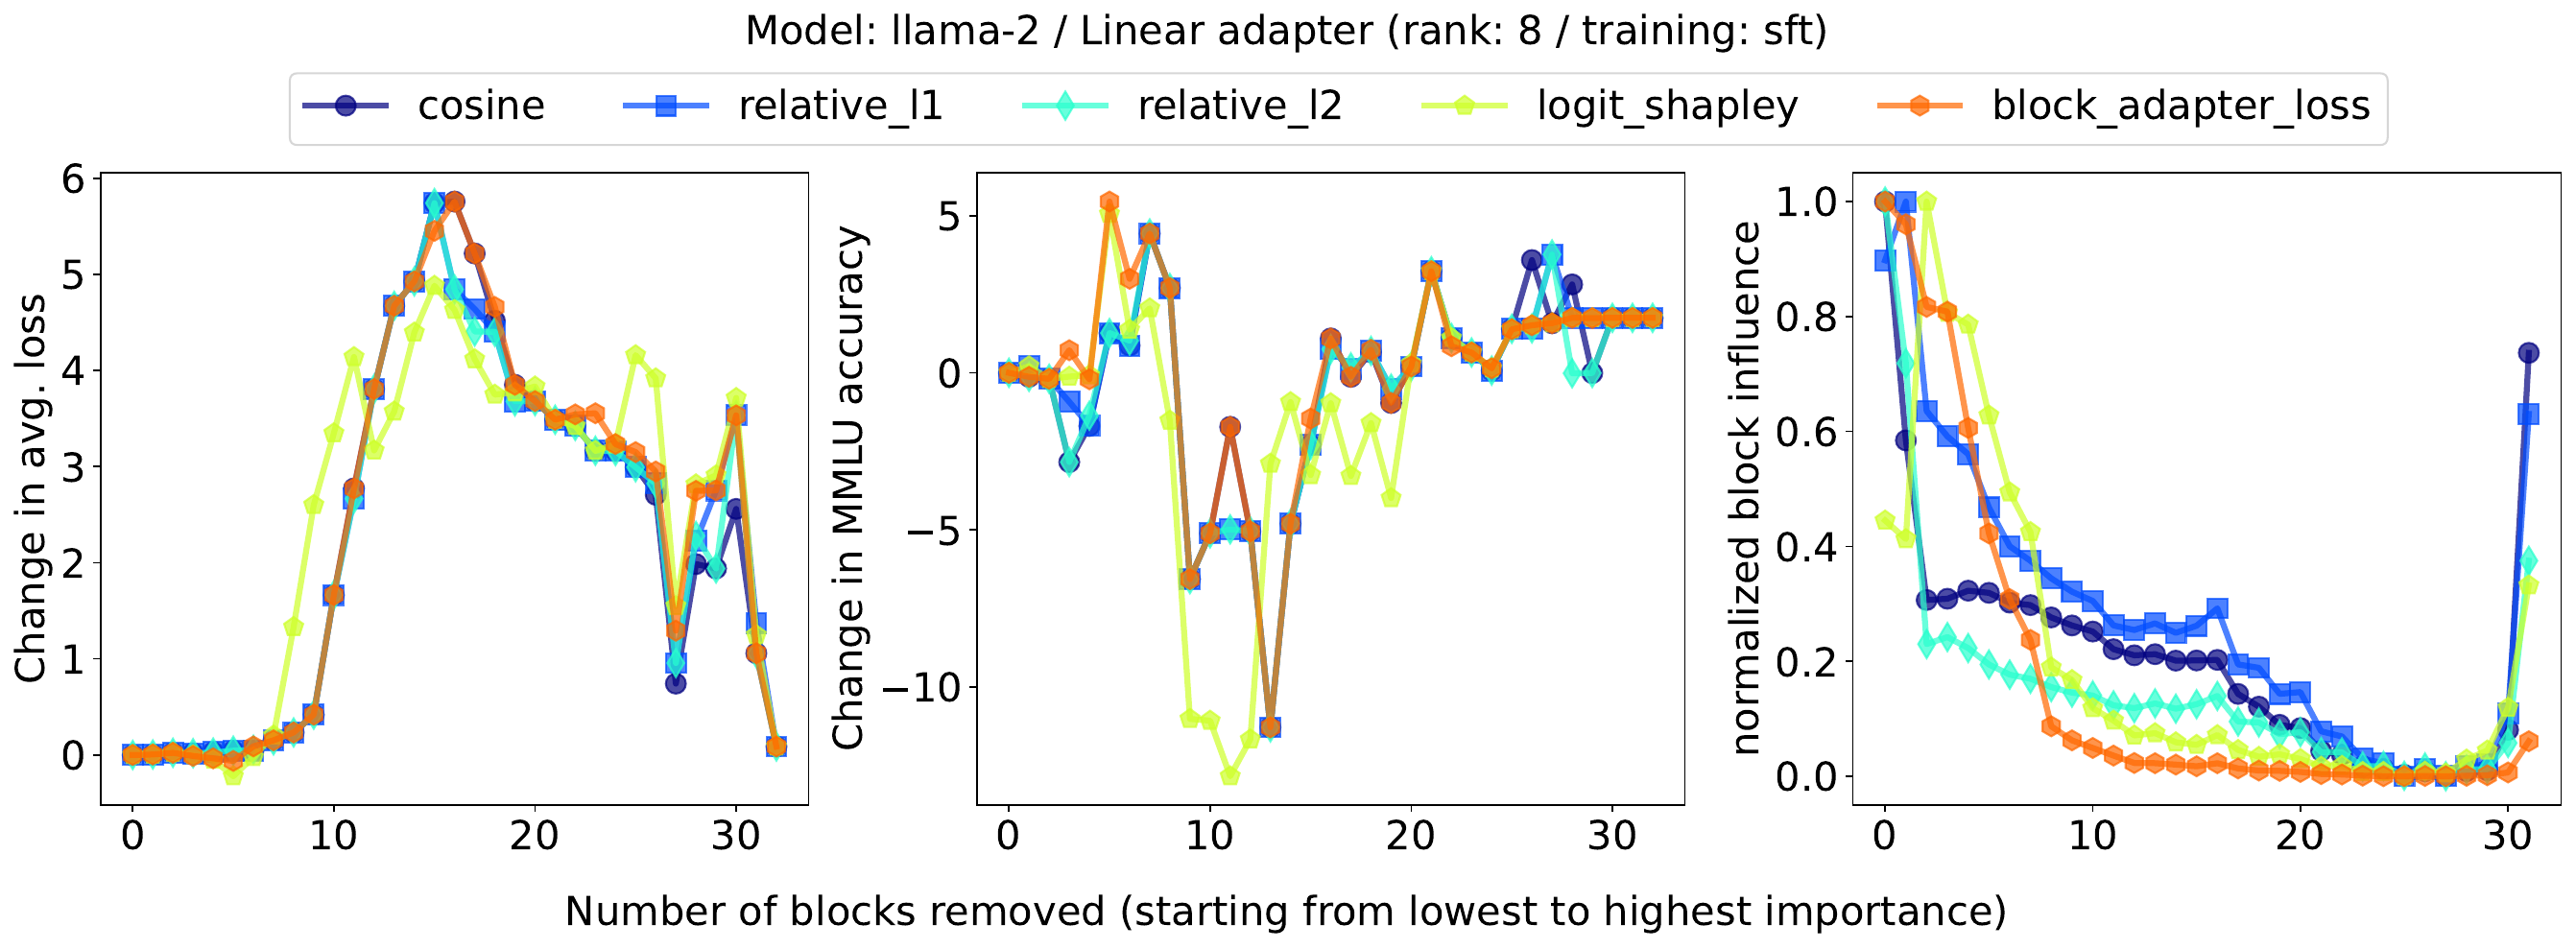}
    }

    \vspace{-3mm}
    \subfloat{
        \includegraphics[width=\textwidth]{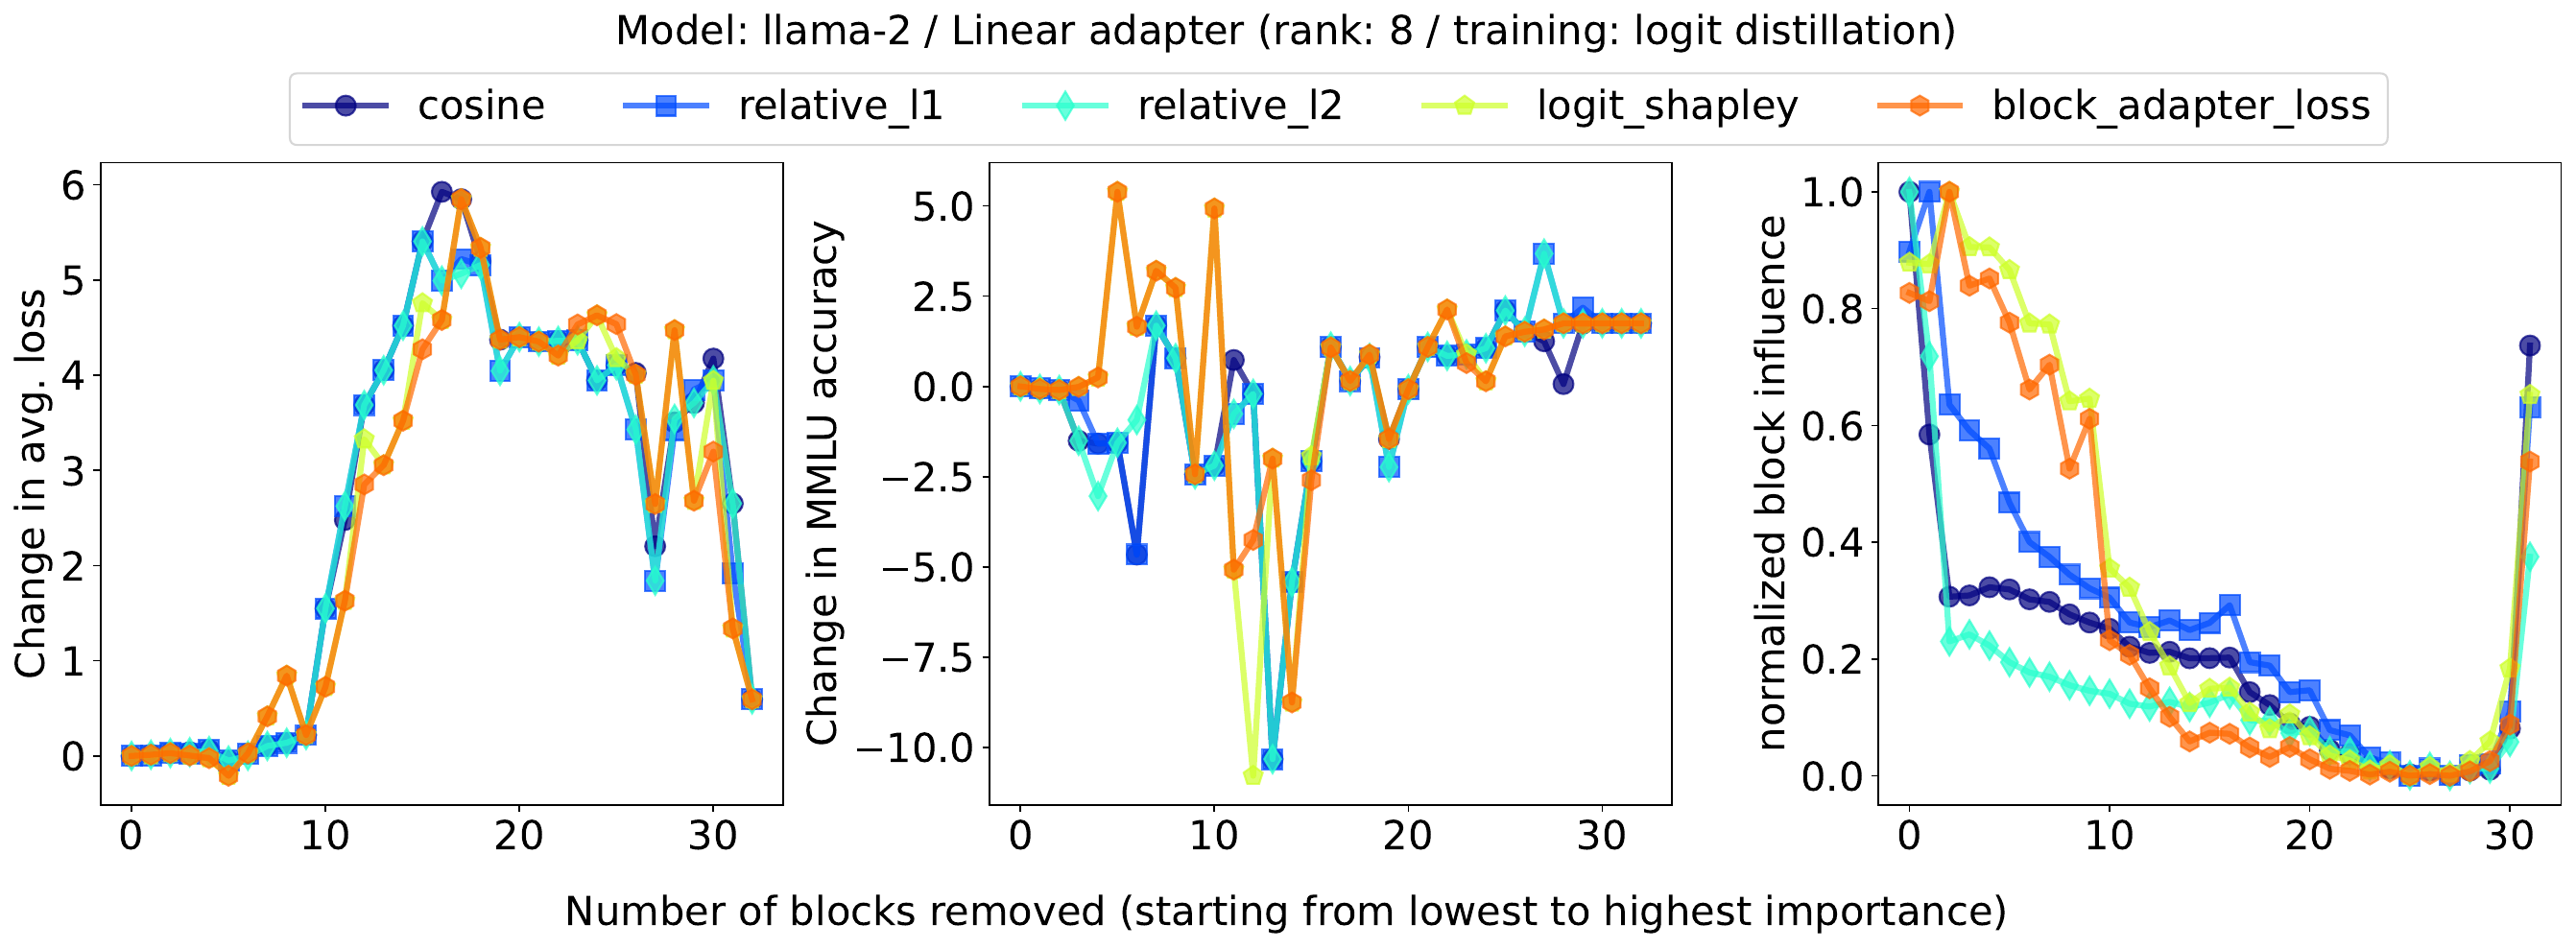}
    }
    \caption{\textbf{Evaluating the relative impact of linear adapters for LLaMa-2 7b with a rank of 8} trained using three different metrics including (a) MSE loss defined on the representation, (b) supervised fine-tuning (SFT), and (c) logit distillation where logits are distilled from the full model. The plot with the original values is presented in Fig.~\ref{fig:linear_adapters_rank_8_llama2}.}
    \label{fig:linear_adapters_rank_8_llama2_relative}
\end{figure}

Fig.~\ref{fig:linear_adapters_rank_8_llama2_relative} presents the results for training a linear adapter on top of LLaMa-2 7b model.
In contrast to the results on Mistral 7b (Fig.~\ref{fig:linear_adapters_rank_8_mistral_relative}), we see a positive impact of training these linear adapters as a performance recovery technique.
This difference in the utility of parameter efficient fine-tuning between the two architectures was similarly observed in~\citep{gromov2024unreasonable}.

\subsection{Update norms}
\label{appendix:update_norms}

\begin{figure}
    \centering
    \subfloat[LLaMa-2 7b]{
         \includegraphics[width=0.49\textwidth]{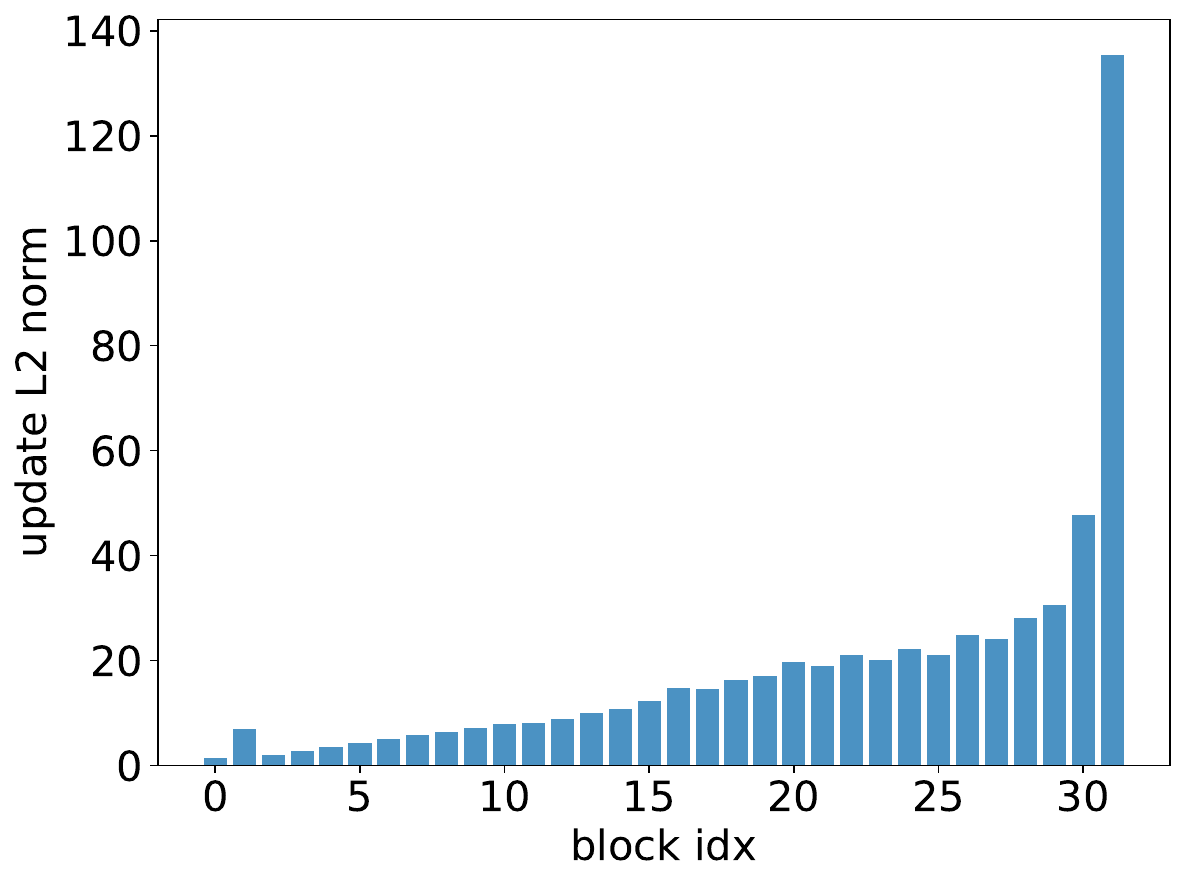}
    }
    \subfloat[Mistral 7b]{
         \includegraphics[width=0.49\textwidth]{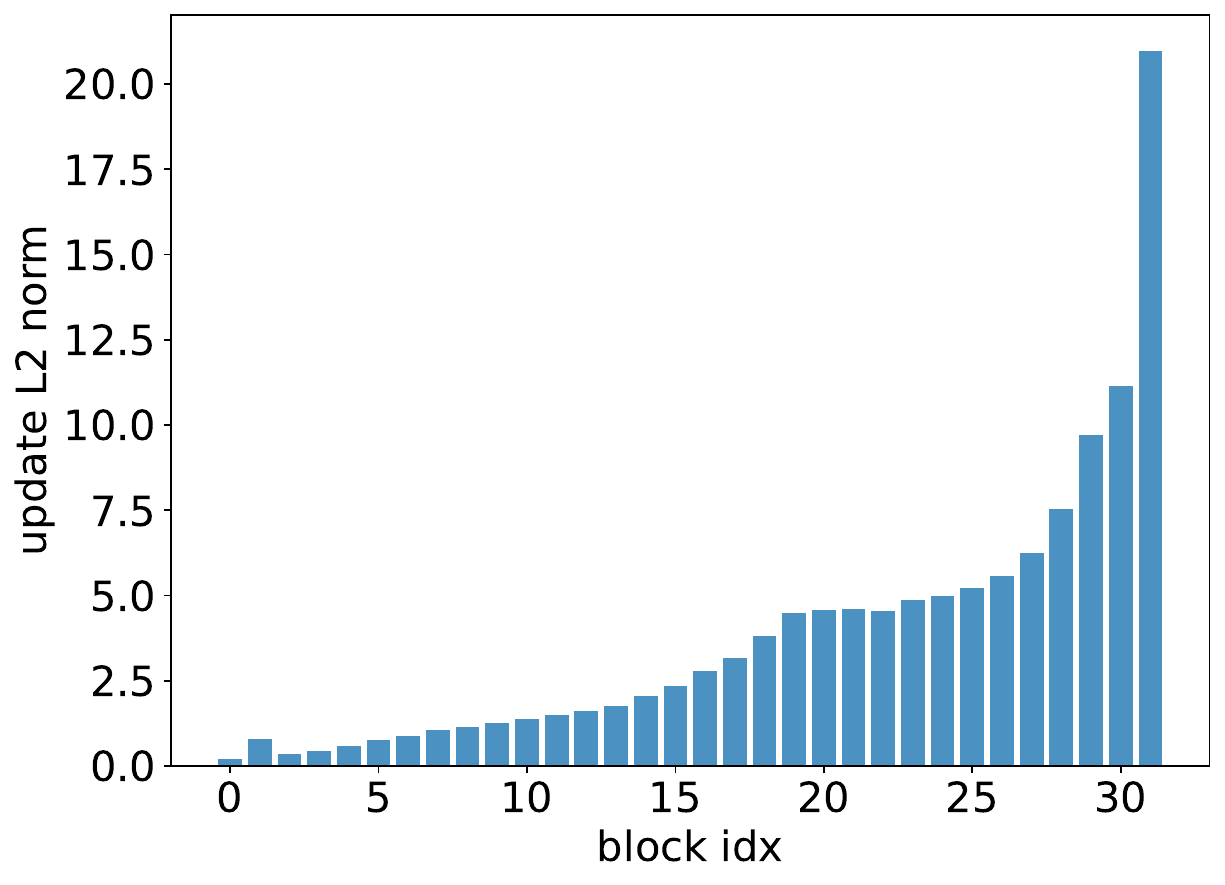}
    }
    \caption{\textbf{Block update L2 norm} that highlights the increasing trend.}
    \label{fig:block_update_norm}
\end{figure}

\begin{figure}
    \centering
    \subfloat[MHSA]{
         \includegraphics[width=0.49\textwidth]{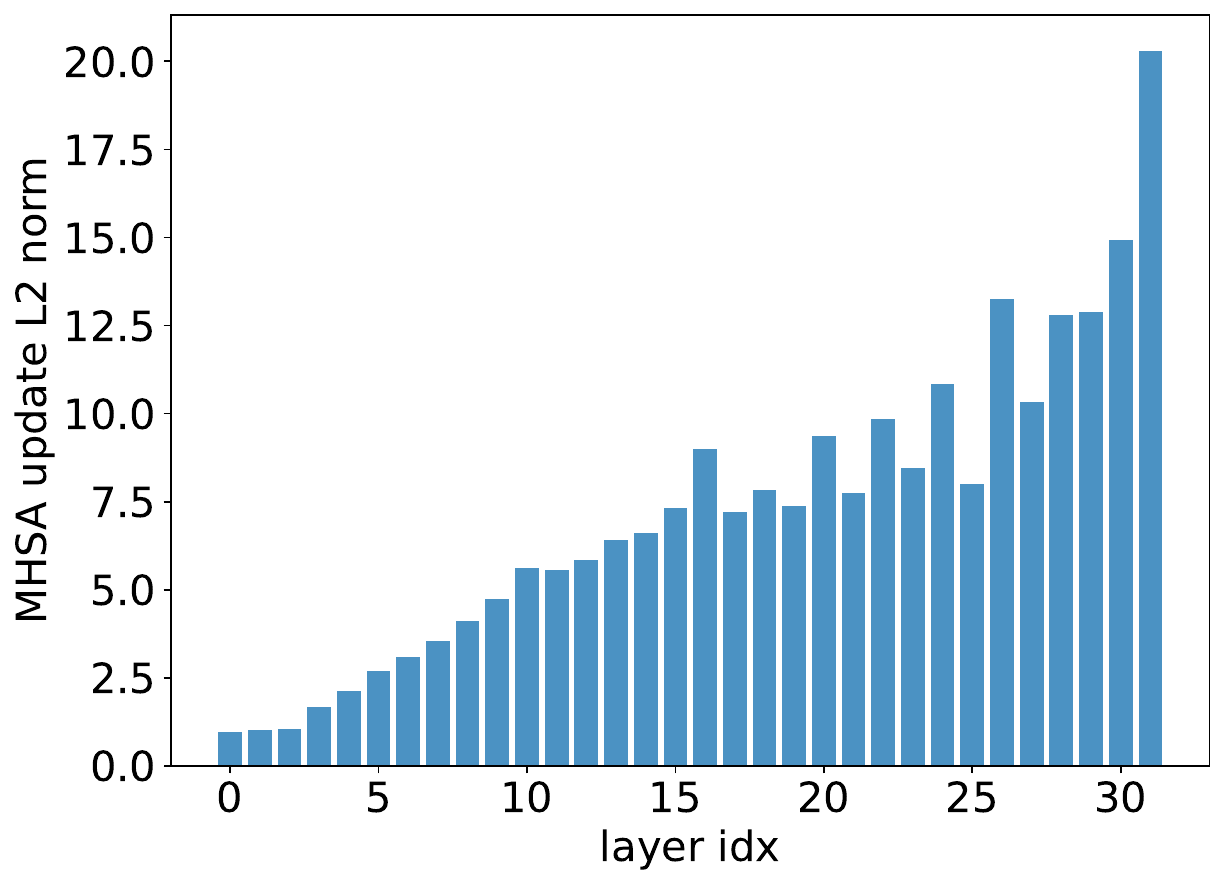}
    }
    \subfloat[MLP]{
         \includegraphics[width=0.49\textwidth]{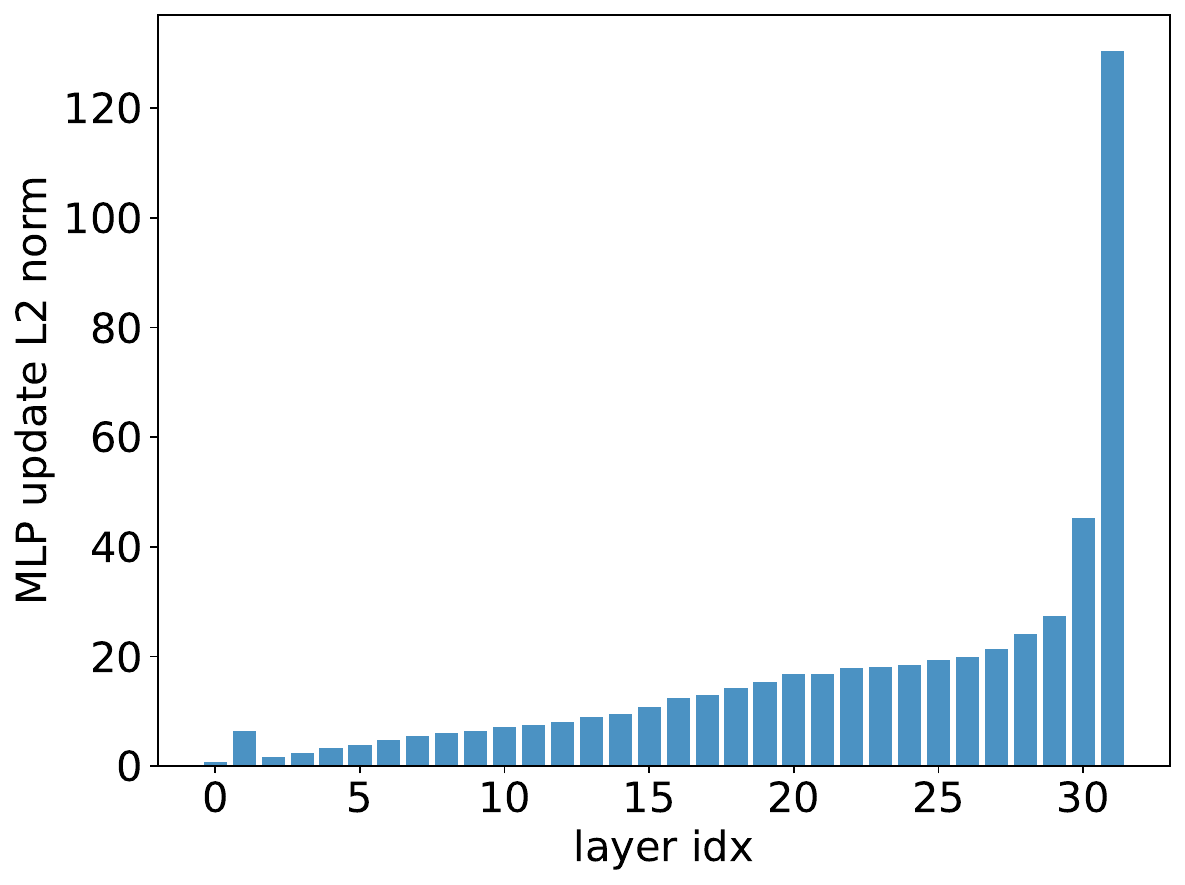}
    }

    \subfloat[MHSA]{
         \includegraphics[width=0.49\textwidth]{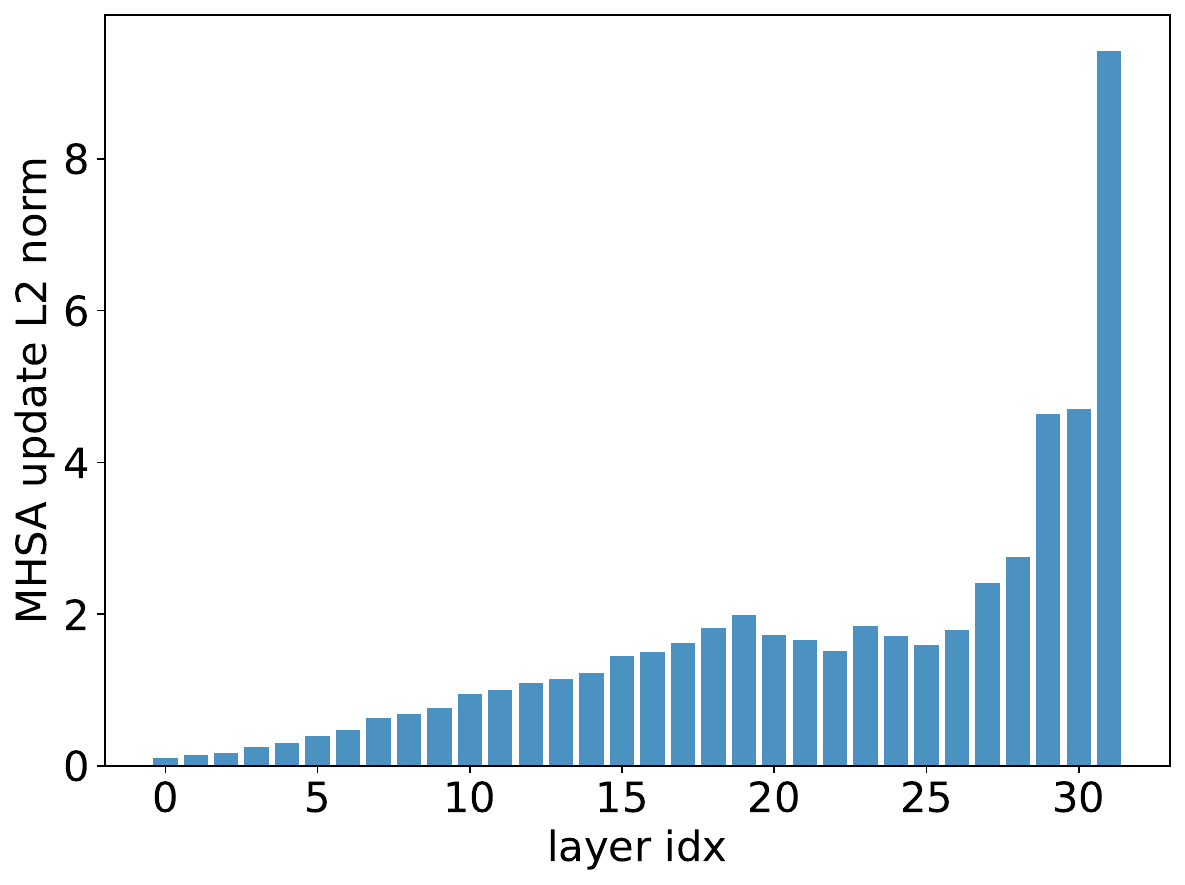}
    }
    \subfloat[MLP]{
         \includegraphics[width=0.49\textwidth]{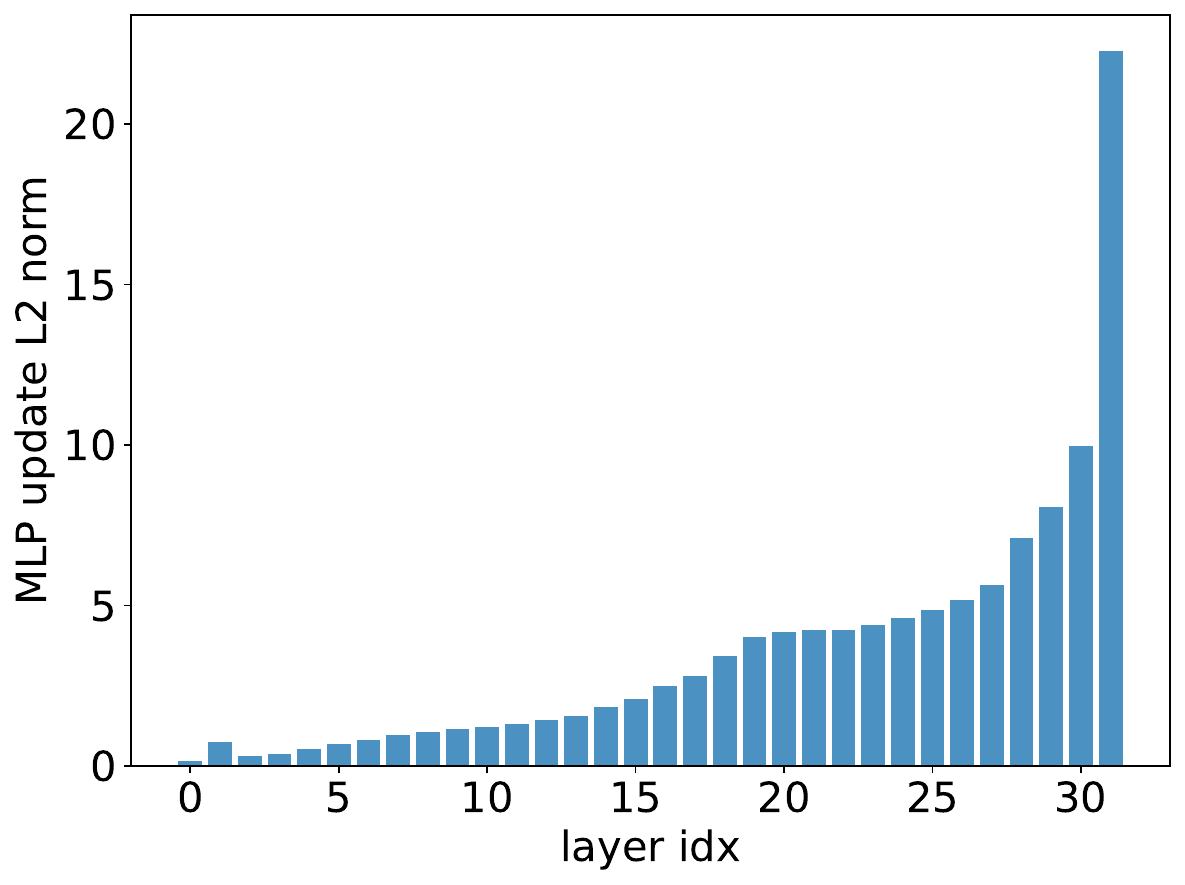}
    }
    \caption{\textbf{Layer update L2 norm} for LLaMa-2 7b (first row) and Mistral 7b (second row).}
    \label{fig:layer_update_norm}
\end{figure}

We visualize the block and layer update norms for both architectures in Fig.~\ref{fig:block_update_norm} and Fig.~\ref{fig:layer_update_norm} respectively.

\subsection{Emulated update}

\begin{figure}
    \centering
    \subfloat{
        \includegraphics[width=\textwidth]{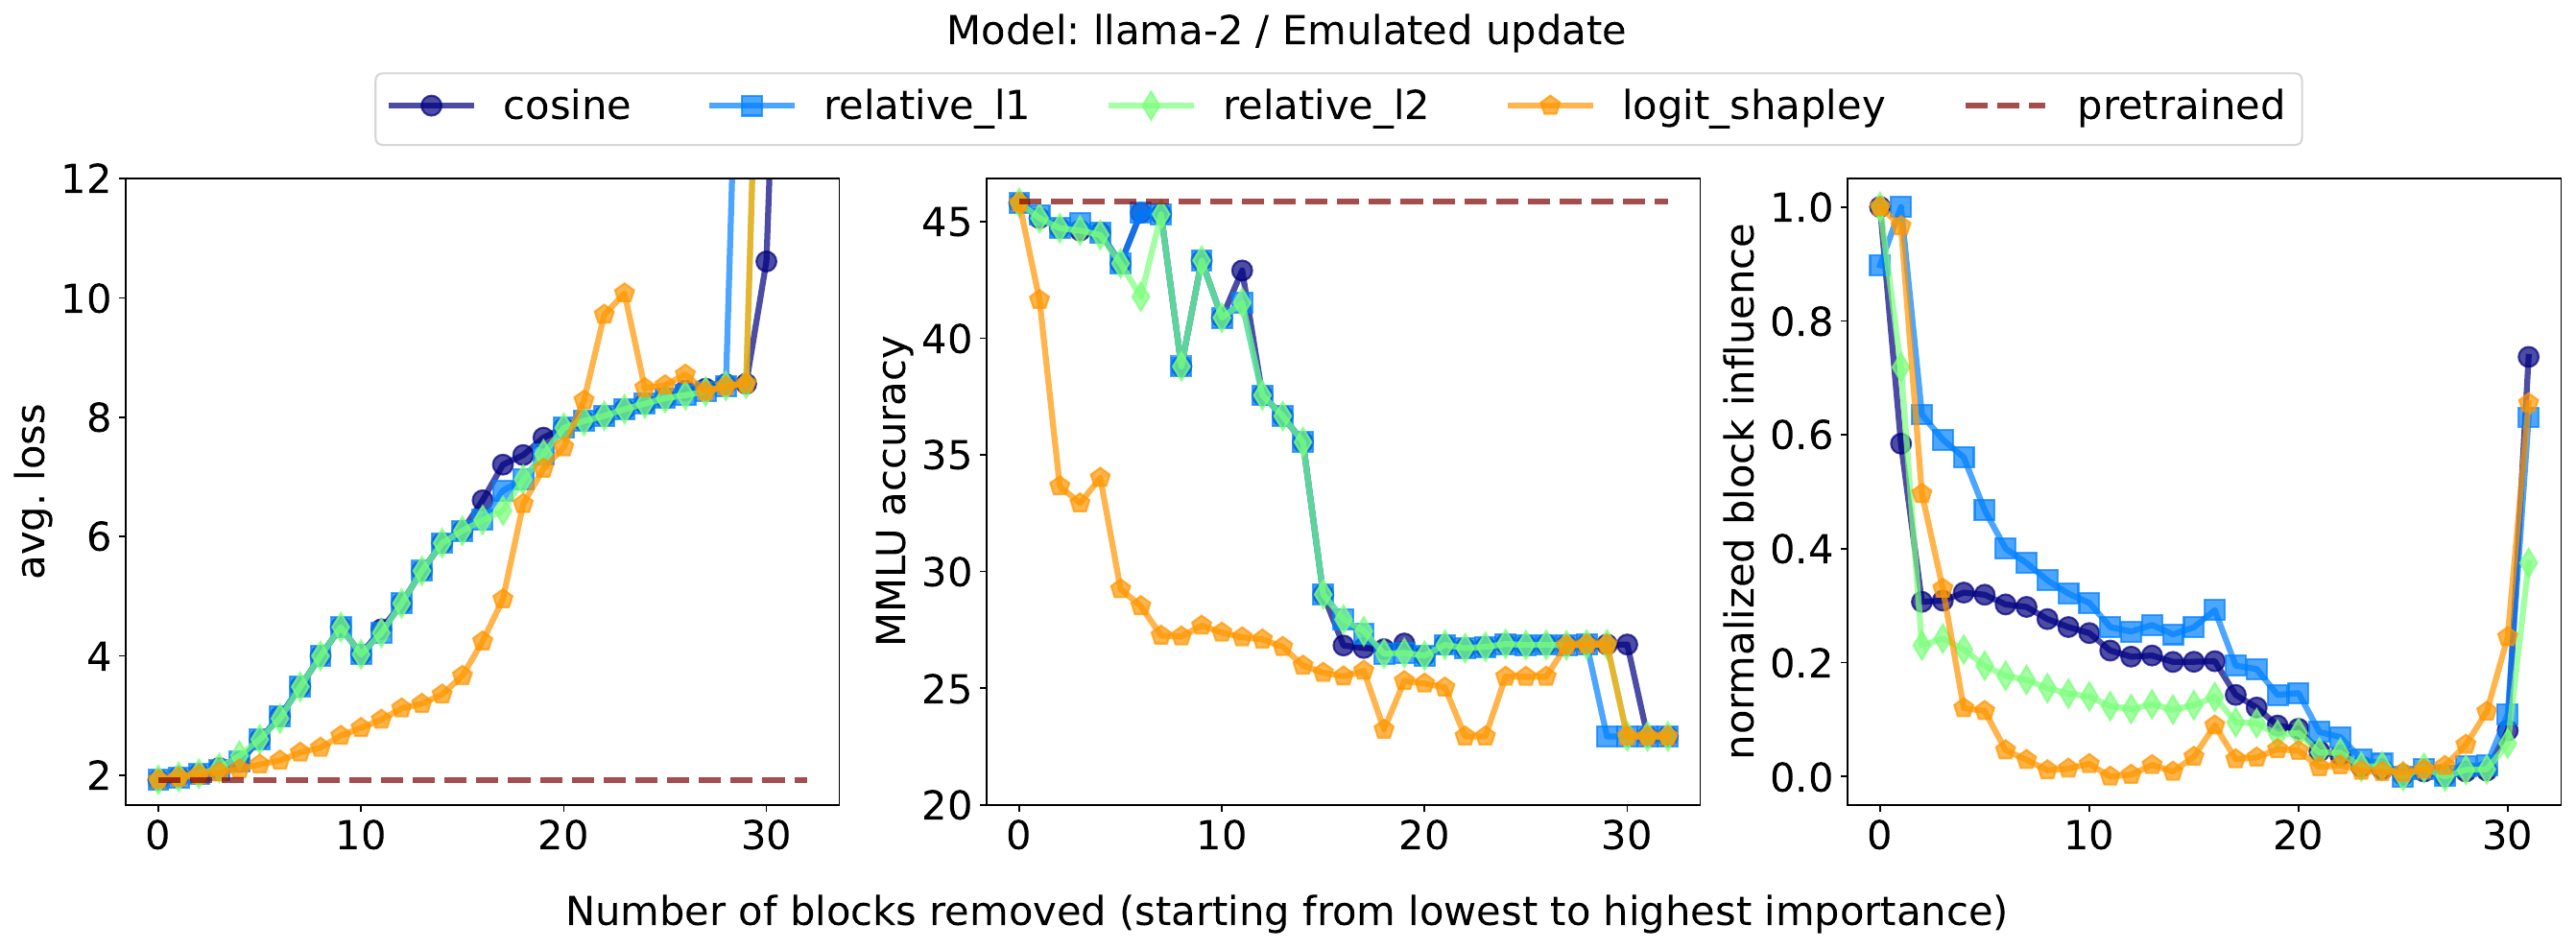}
    }
    
    \subfloat{
        \includegraphics[width=\textwidth]{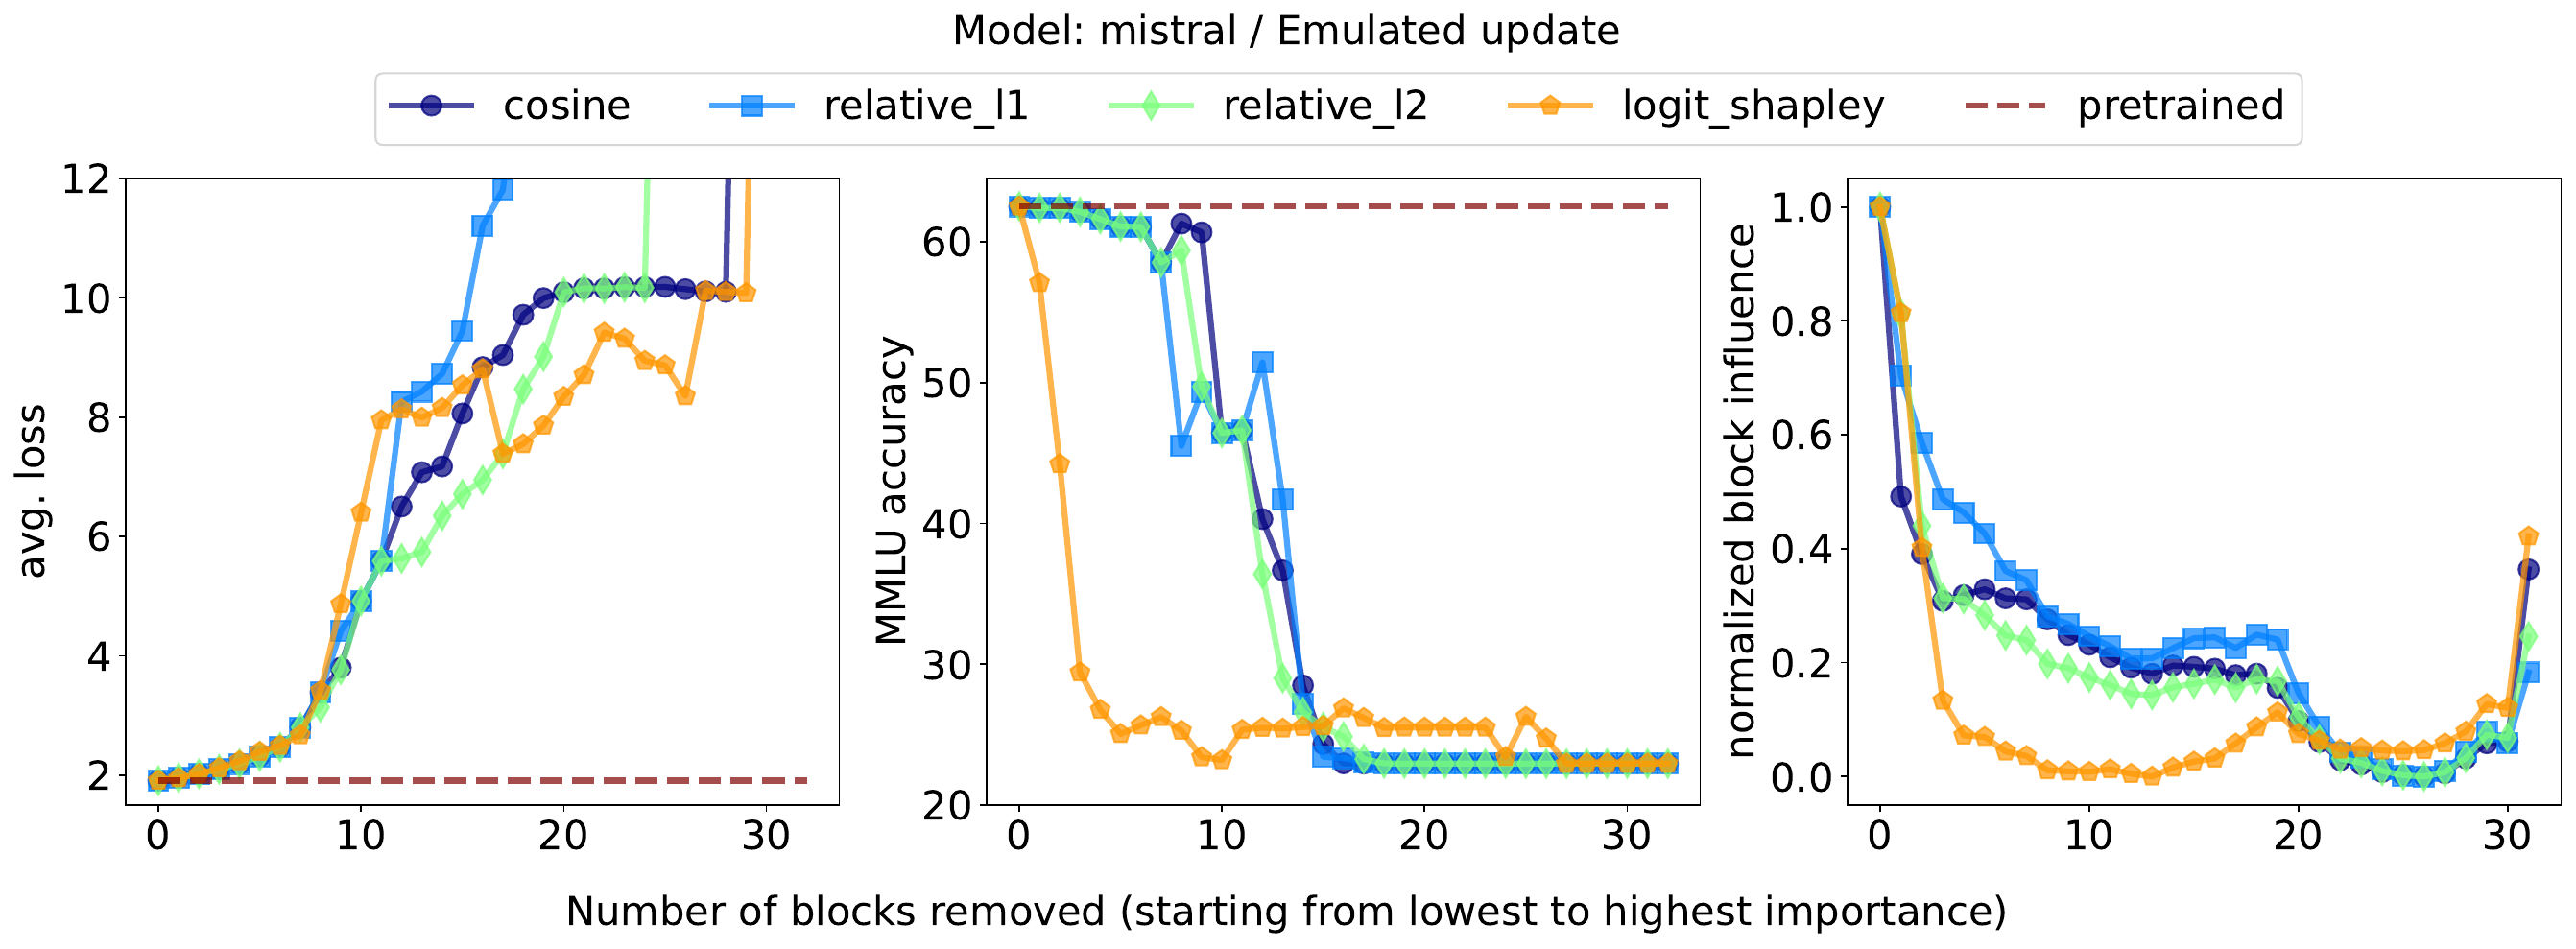}
    }
    \caption{\textbf{Impact on performance with emulated update as a performance recovery method.}}
    \label{fig:emulated_update}
\end{figure}

The non-relative results for emulated update are visualized in Fig.~\ref{fig:emulated_update}.

\subsubsection{Emulated update statistics}
\label{appendix_subsec:emulated_update_stats}

\begin{figure}
    \centering
    \subfloat{
        \includegraphics[width=0.48\textwidth]{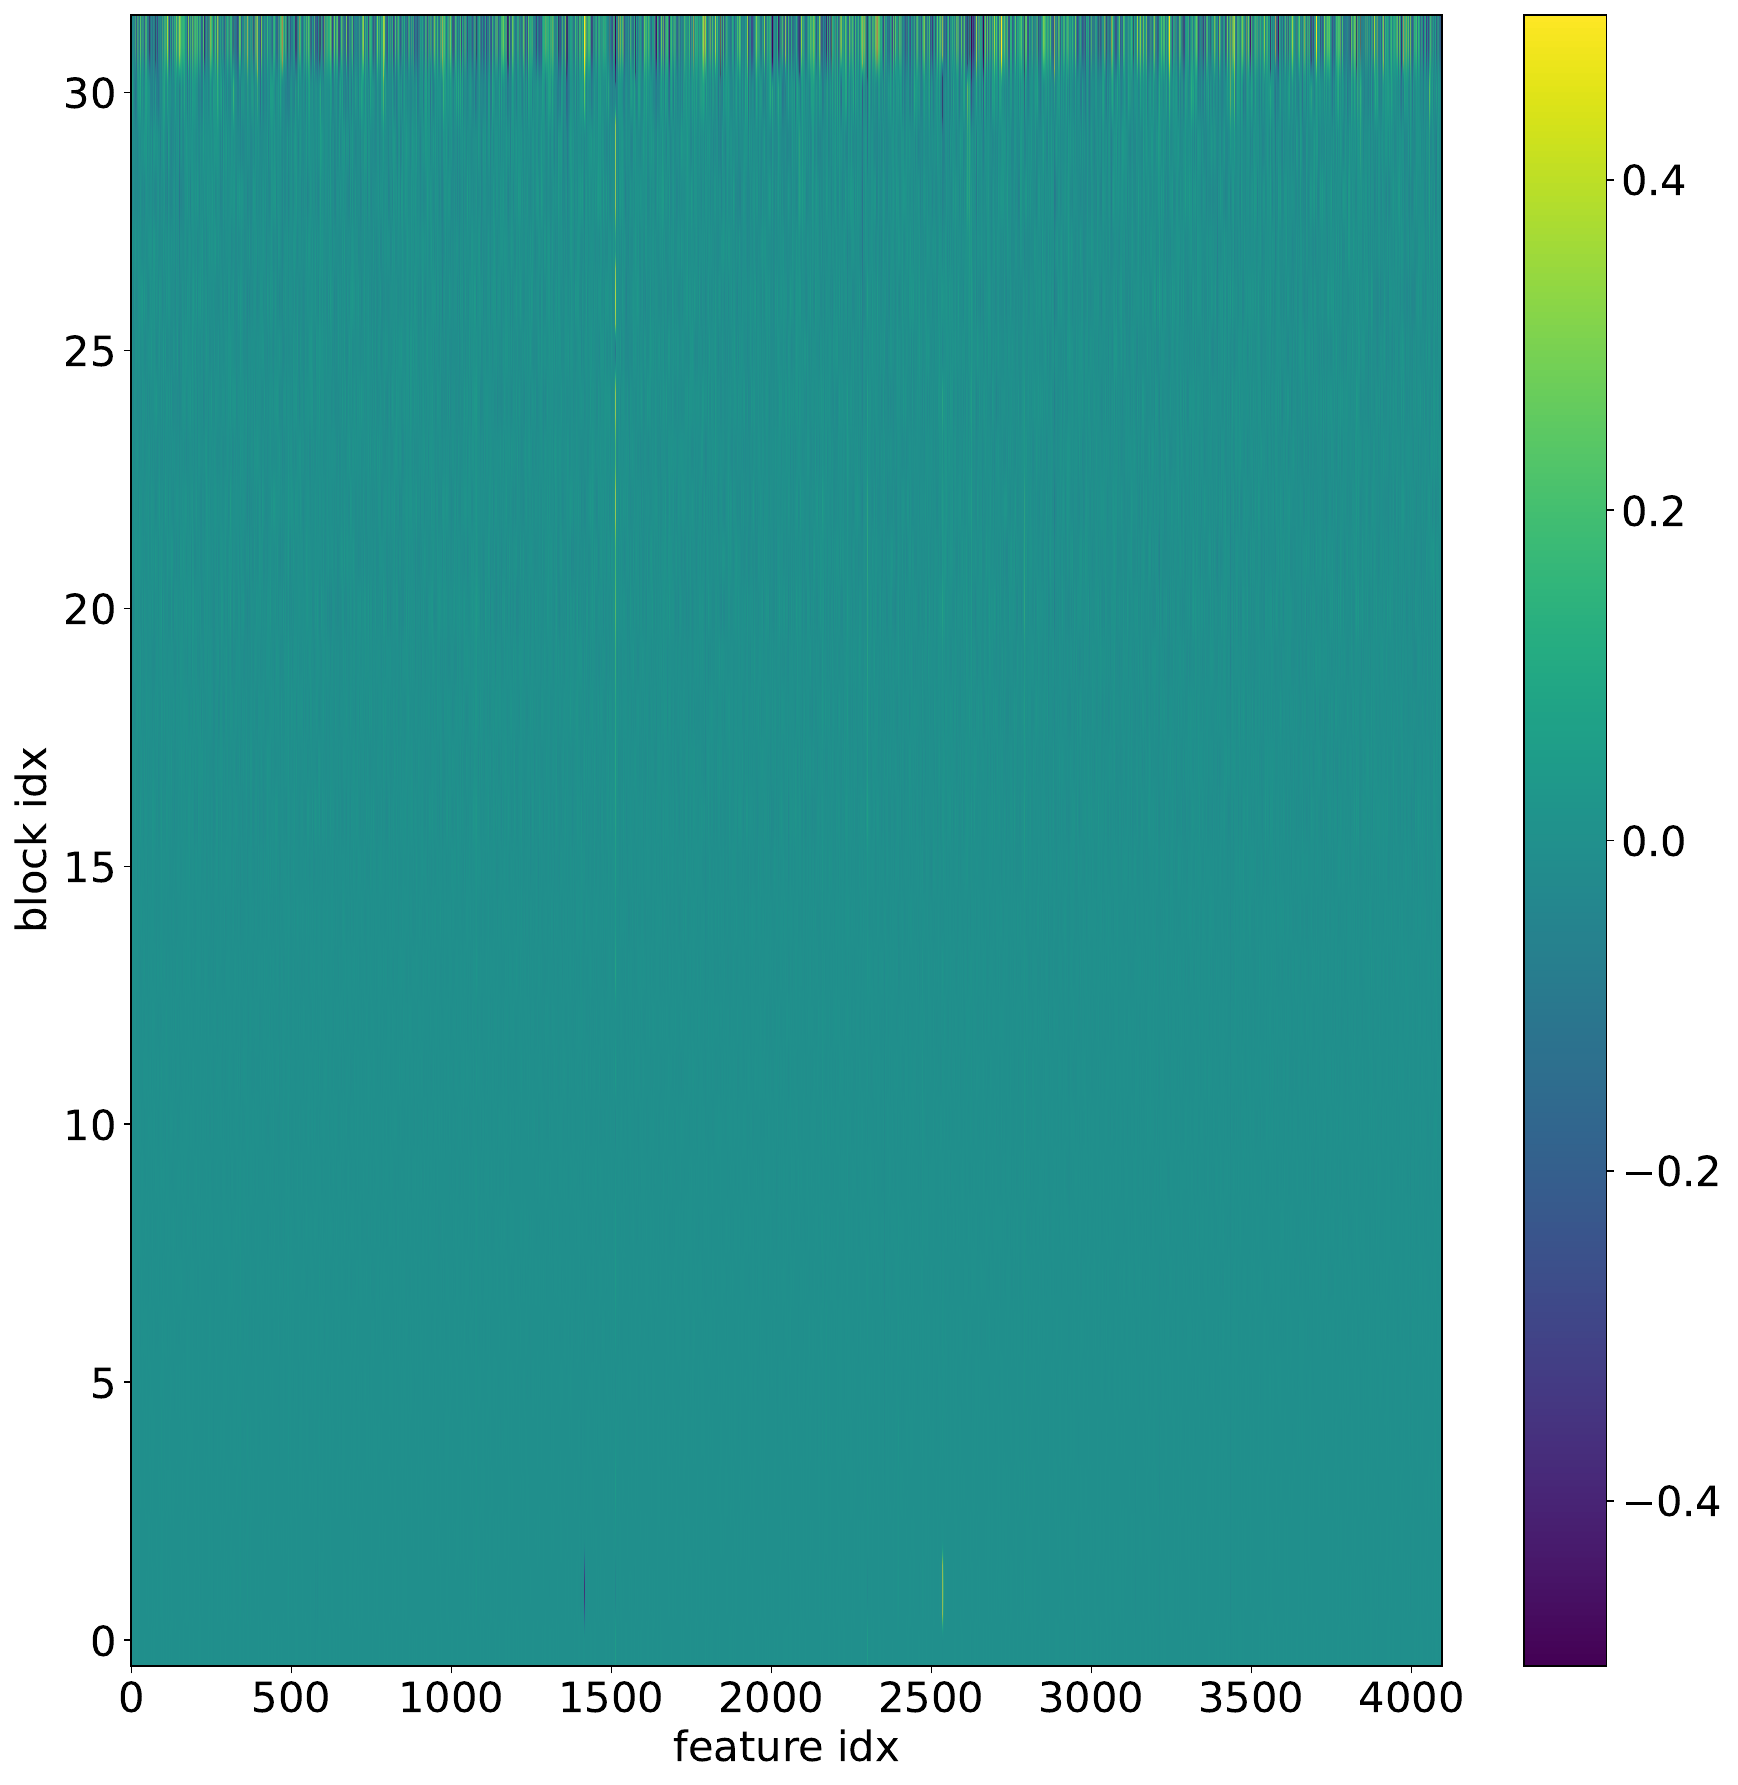}
    }
    \subfloat{
        \includegraphics[width=0.48\textwidth]{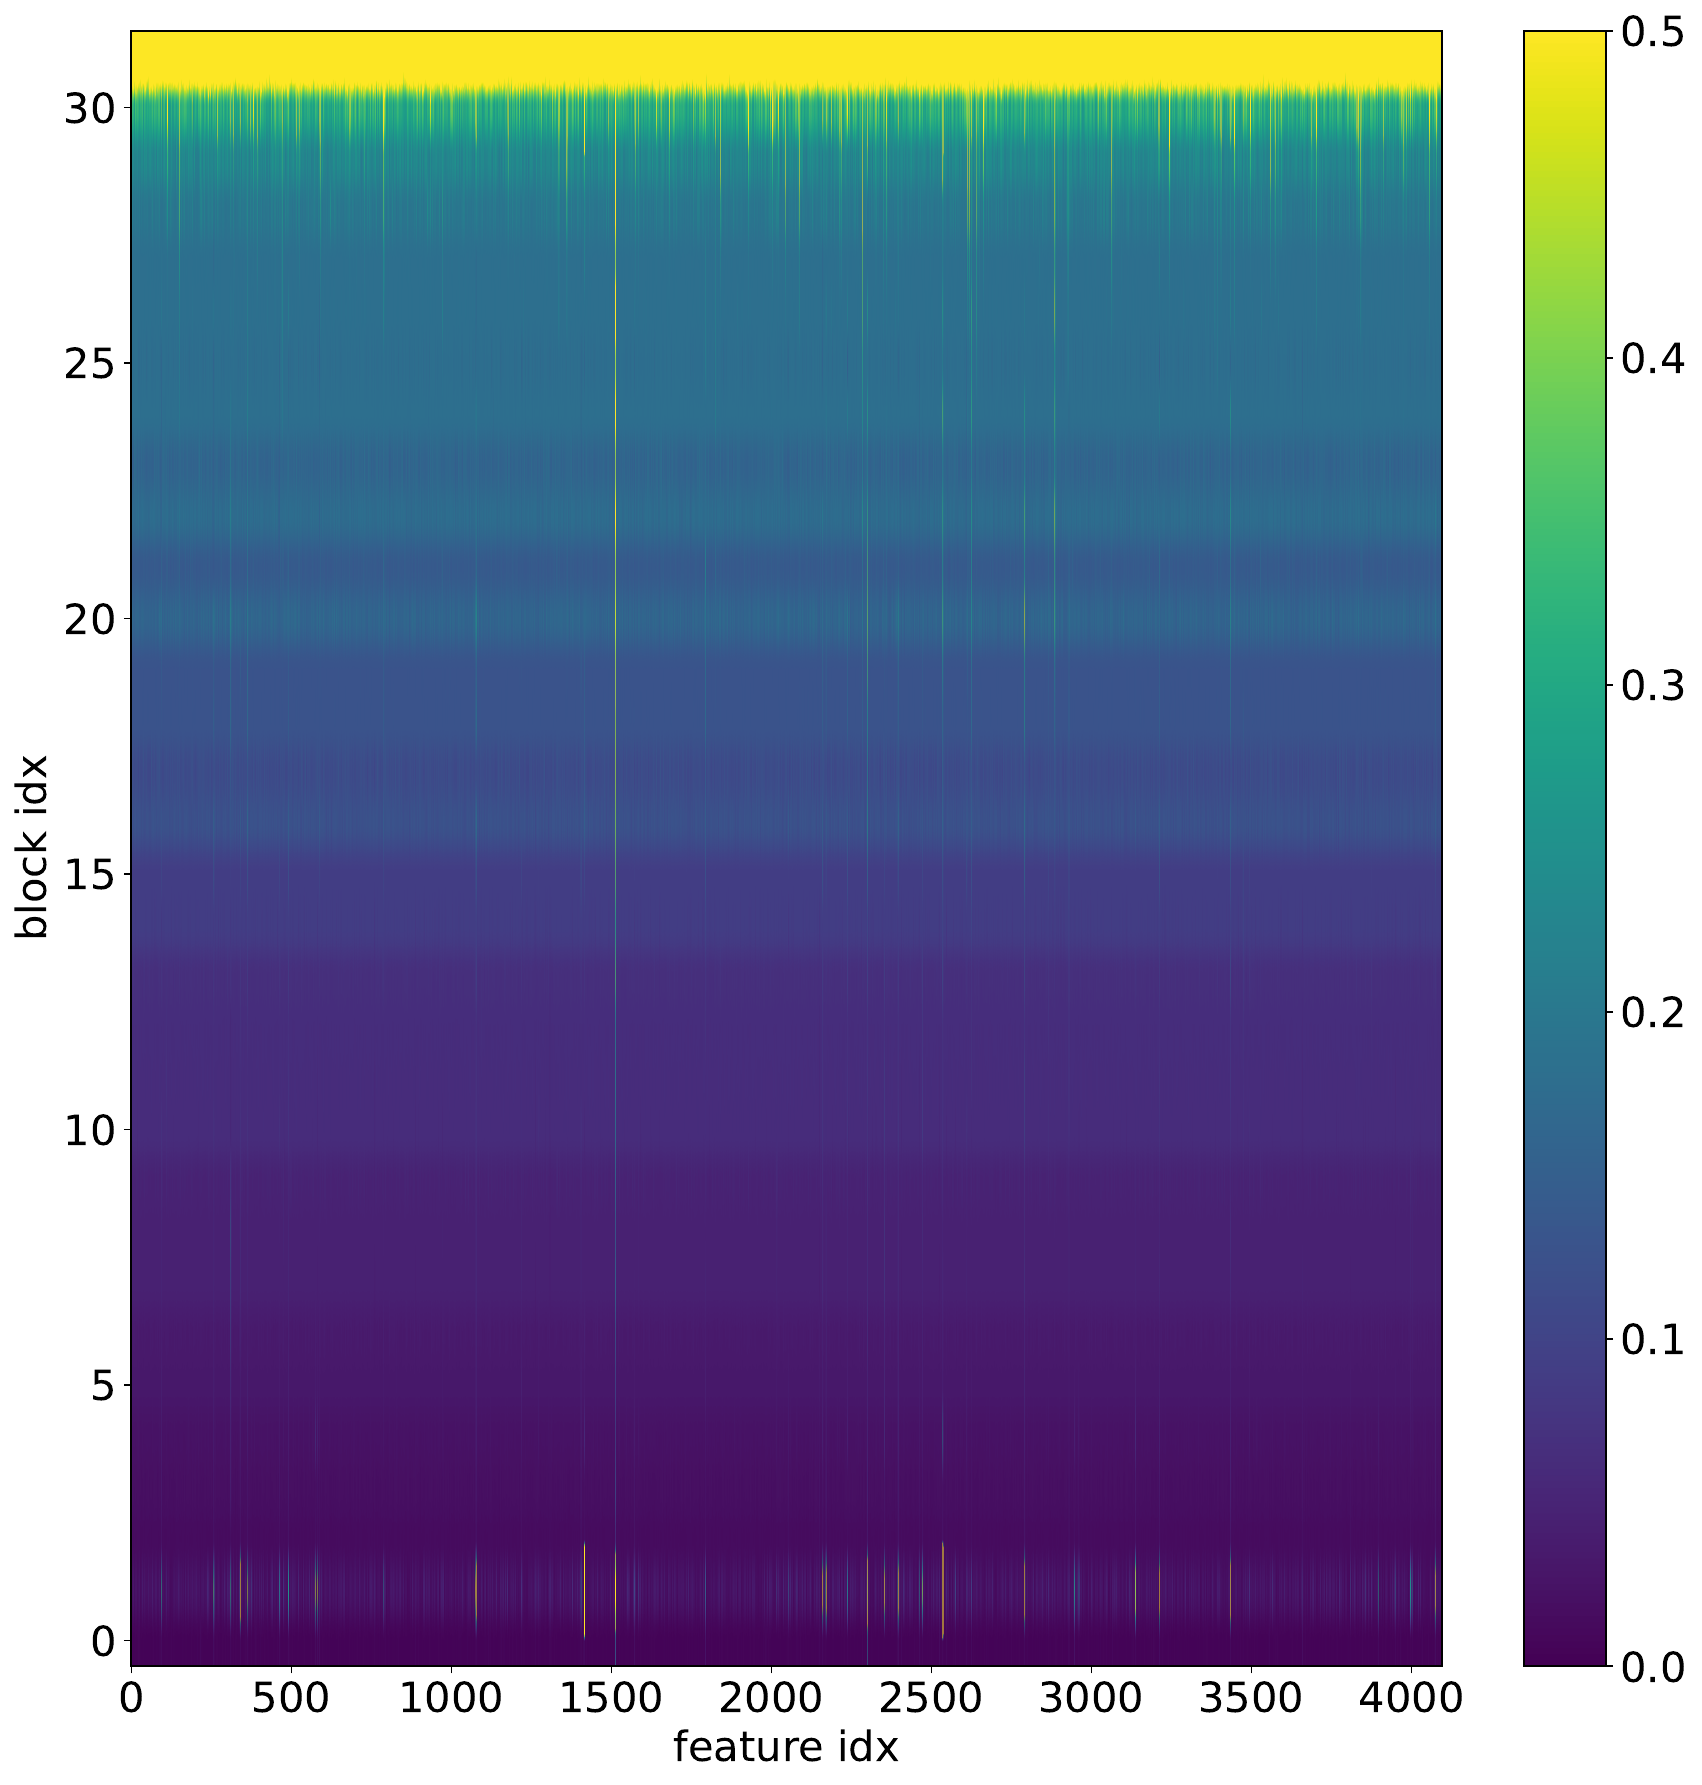}
    }
    \caption{\textbf{Computed emulated update statistics for LLaMa-2 7b model with mean visualized on the left and standard deviation visualized on the right.} Note that we adjust the visualization range to focus on the values in the middle.}
    \label{fig:llama2_emulated_update_stats}
\end{figure}

Statistics for the emulated update for LLaMa-2 7b are presented in Fig.~\ref{fig:llama2_emulated_update_stats}.

\begin{figure}
    \centering
    \subfloat{
        \includegraphics[width=0.48\textwidth]{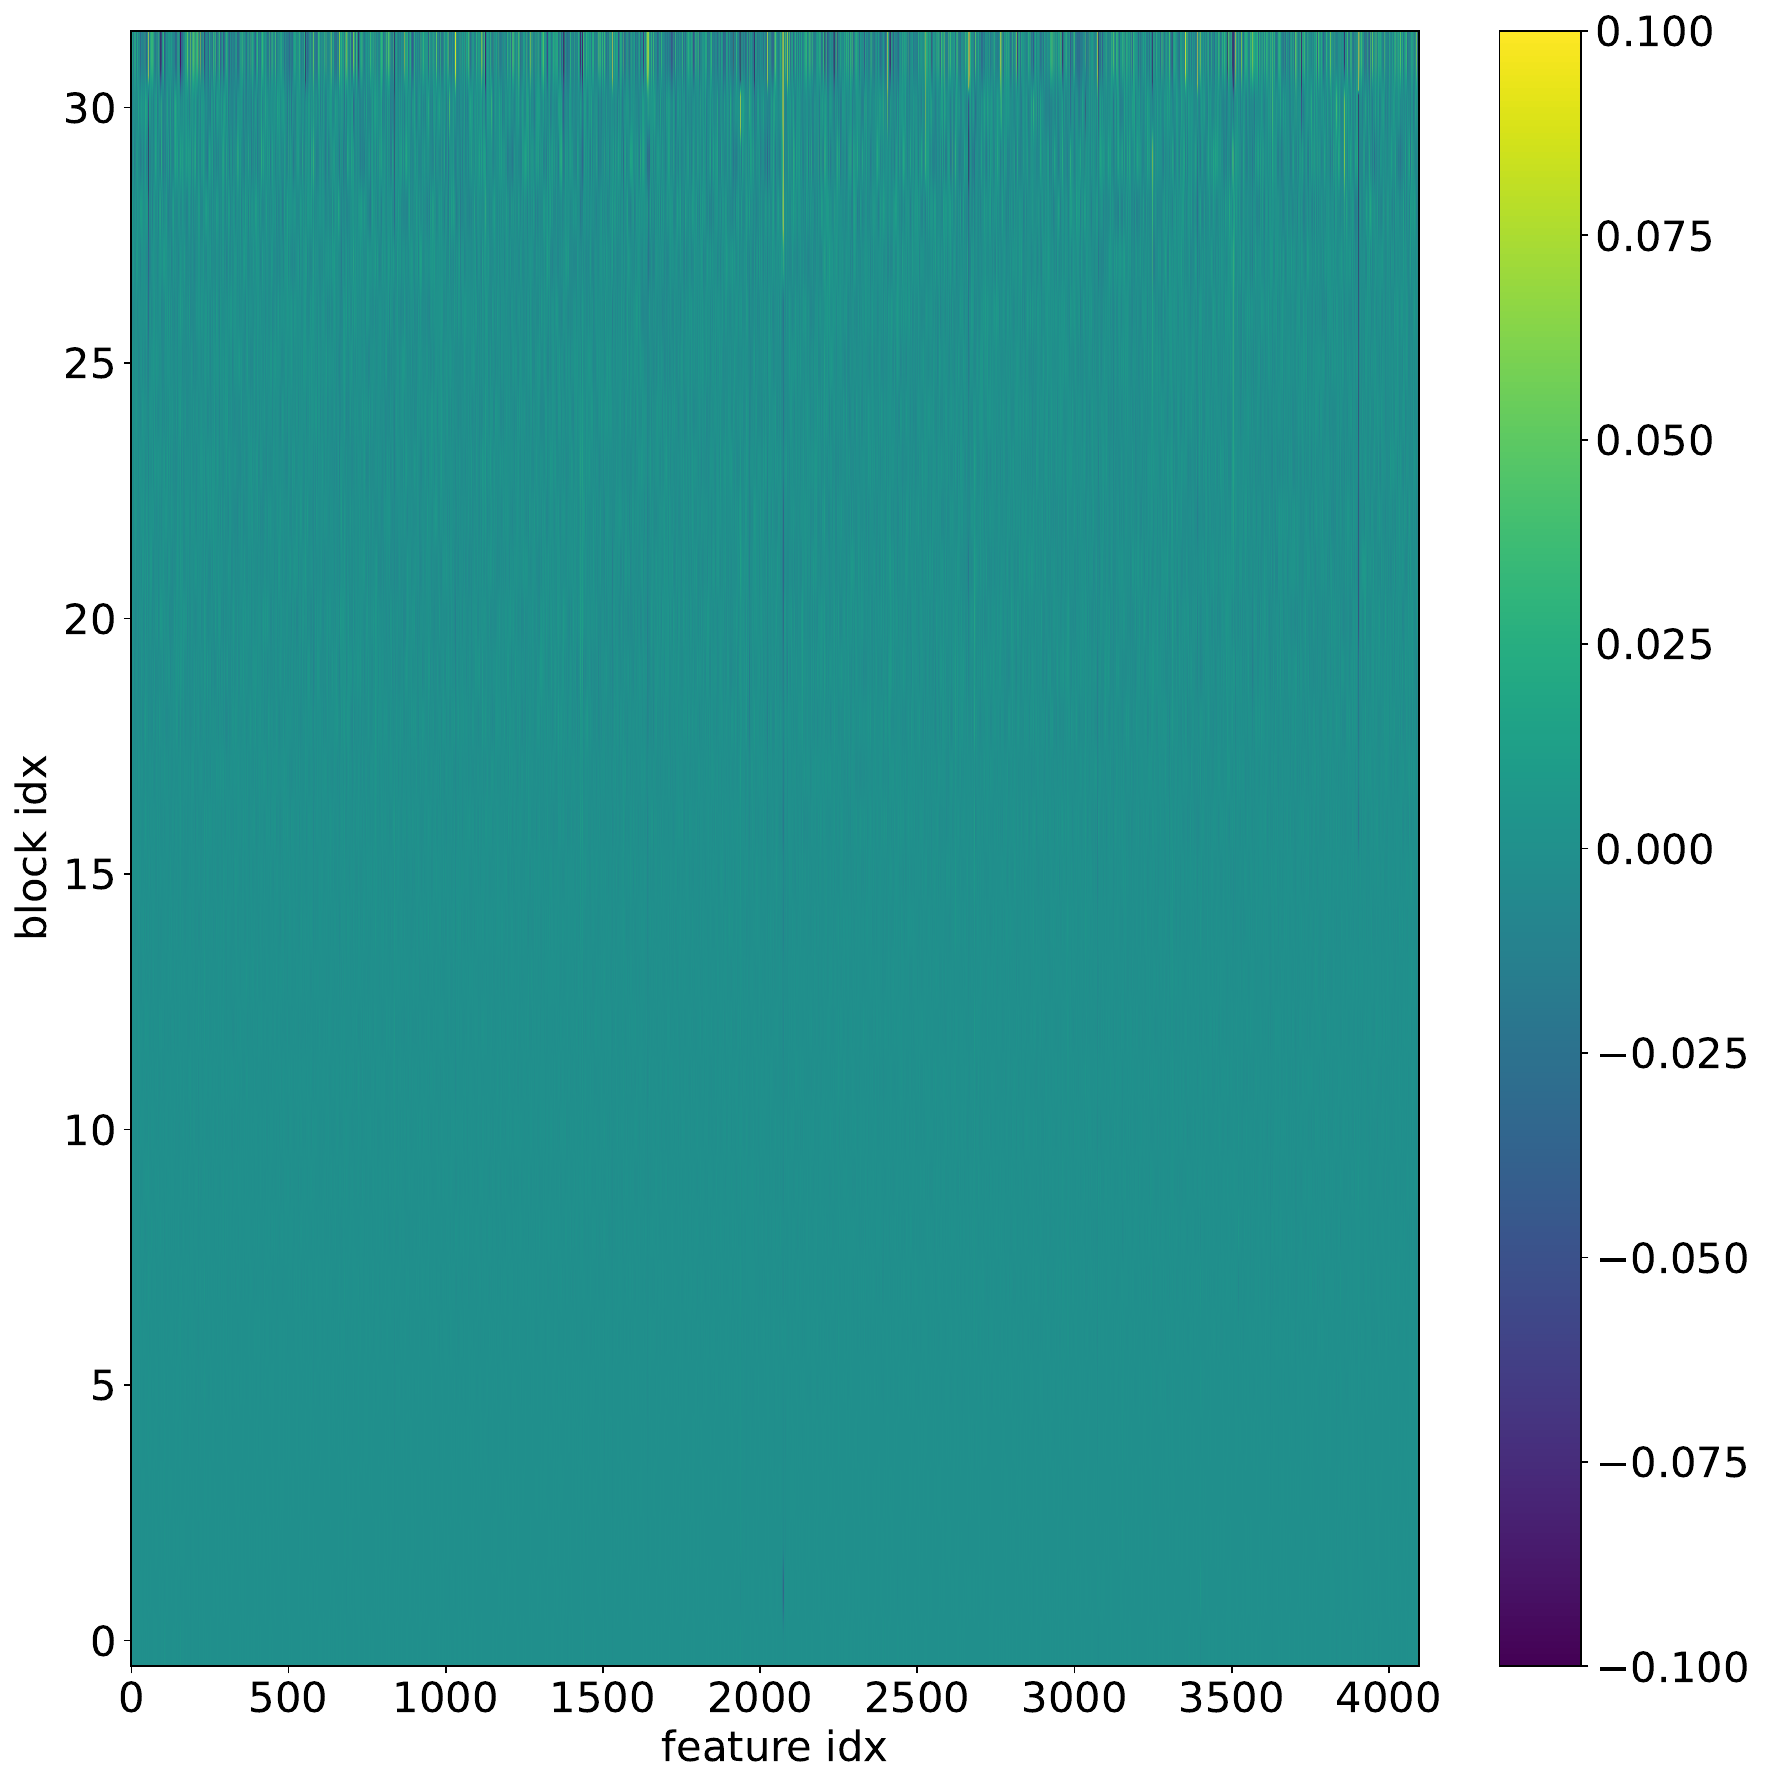}
    }
    \subfloat{
        \includegraphics[width=0.48\textwidth]{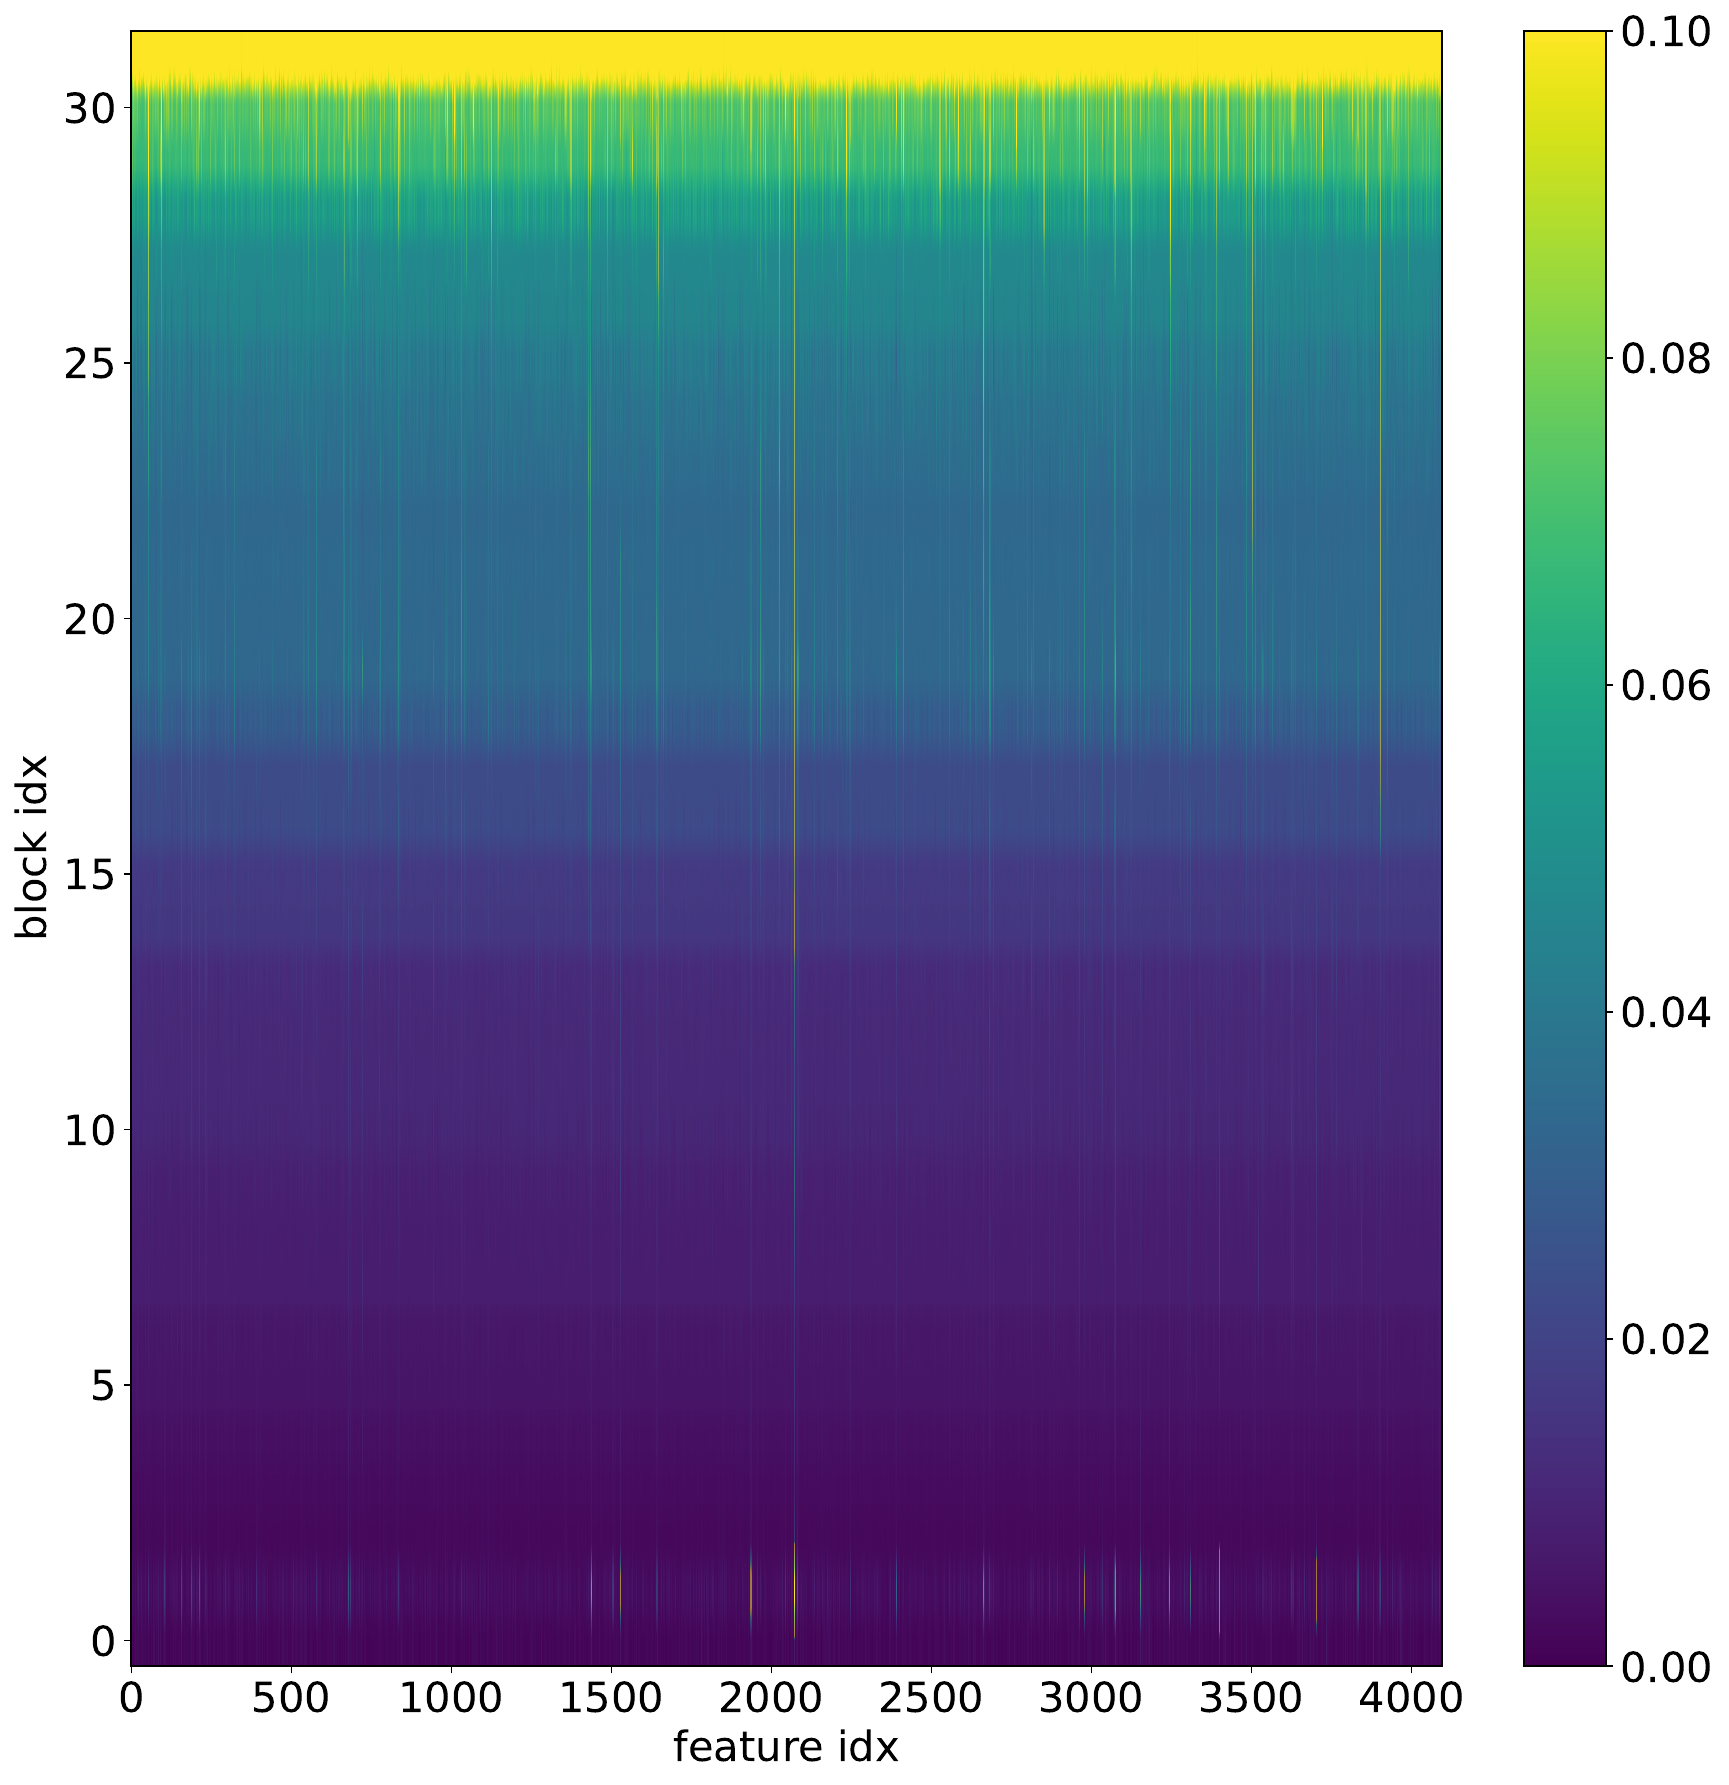}
    }
    \caption{\textbf{Computed emulated update statistics for Mistral 7b model with mean visualized on the left and standard deviation visualized on the right.} Note that we adjust the visualization range to focus on the values in the middle.}
    \label{fig:mistral_emulated_update_stats}
\end{figure}

Statistics for the emulated update for Mistral 7b are presented in Fig.~\ref{fig:mistral_emulated_update_stats}.
We further reduce the visualization range for Mistral as the values are significantly smaller as compared to LLaMa-2 (also see Appendix~\ref{appendix:update_norms} to understand the differences in value range).

\subsection{Low-rank linear adapters (remaining relative results).}
\label{appendix:low_rank_remaining_relative_results}

\begin{figure}
    \centering
    \subfloat{
        \includegraphics[width=\textwidth]{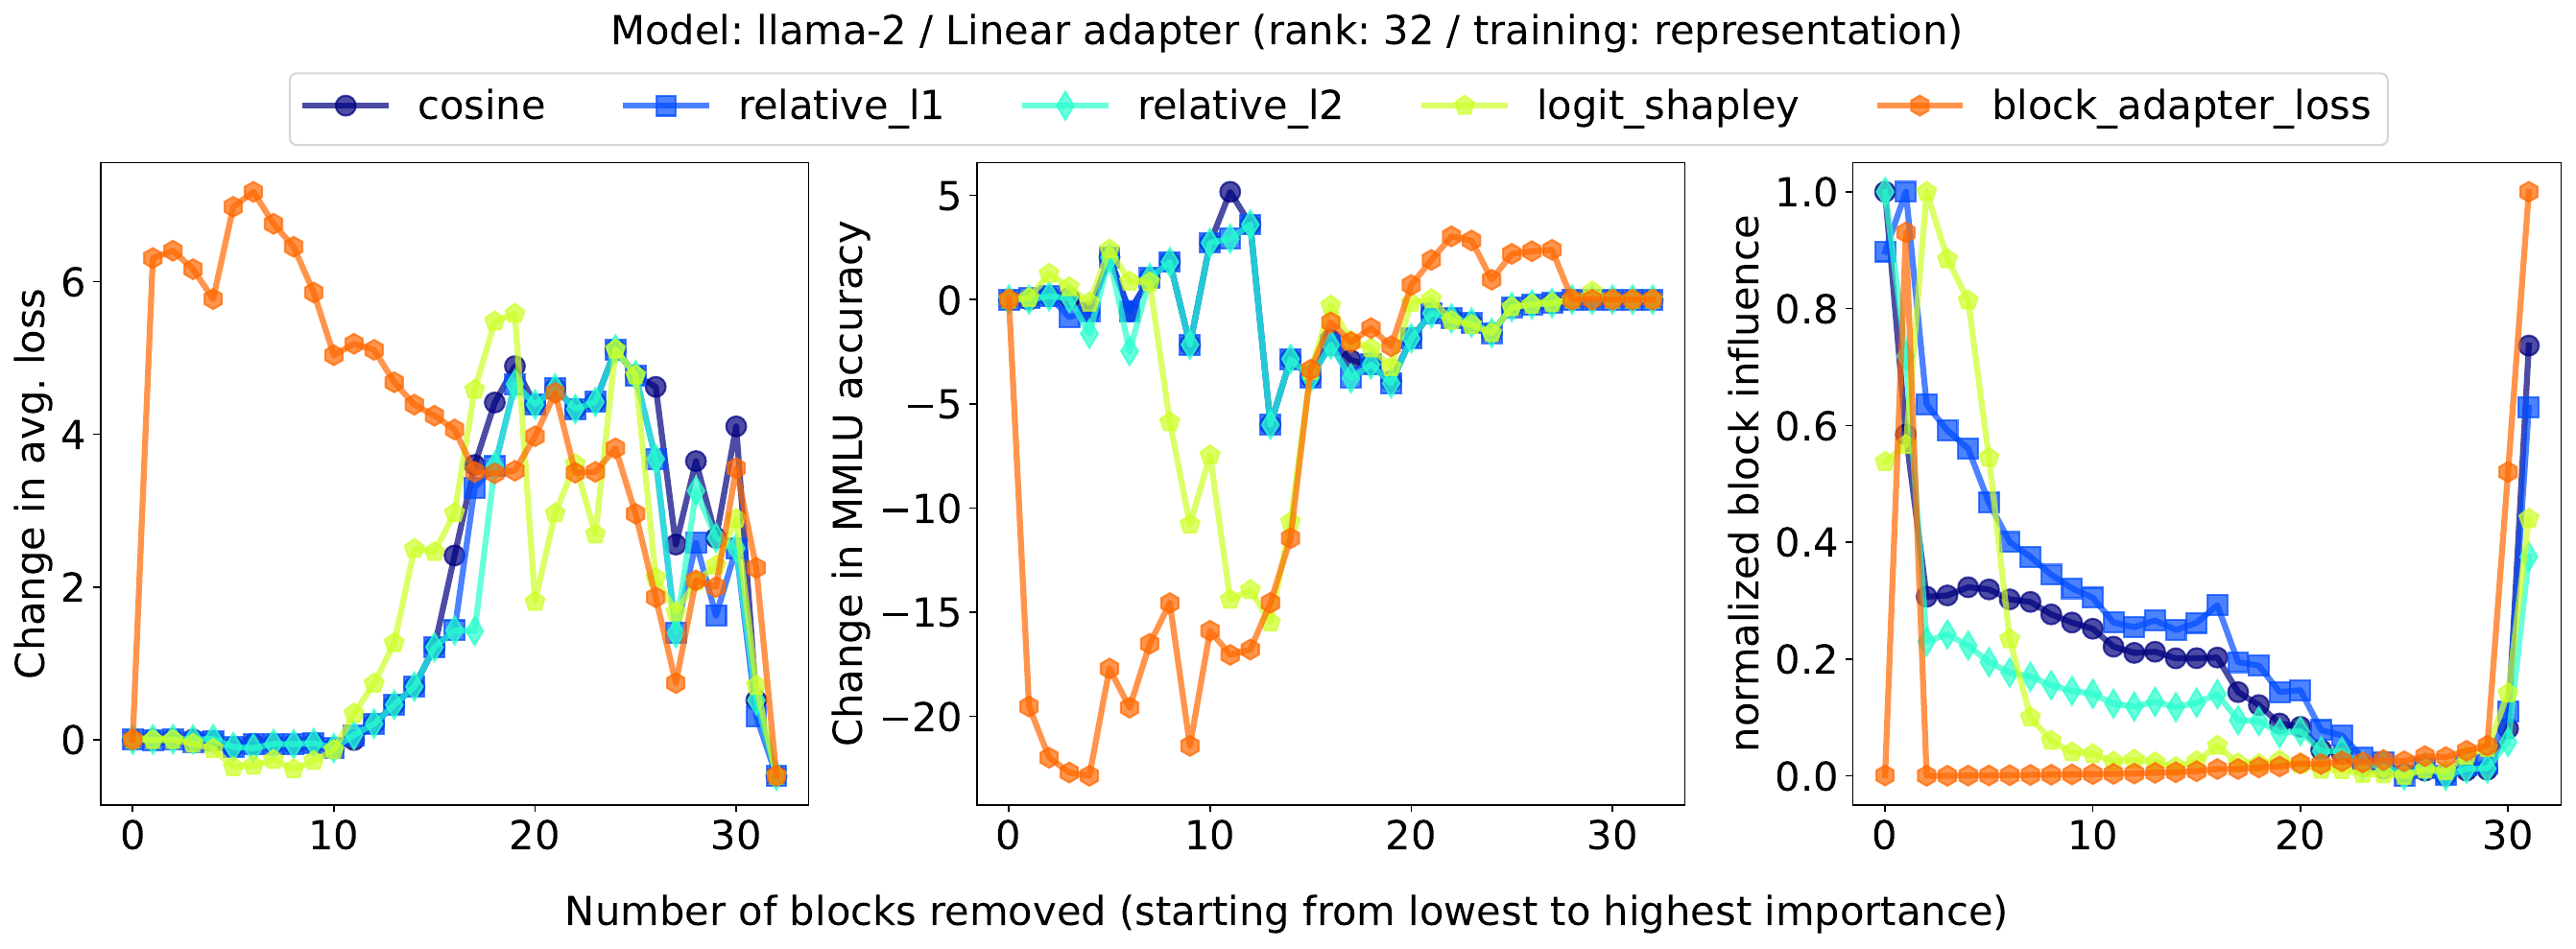}
    }

    \subfloat{
        \includegraphics[width=\textwidth]{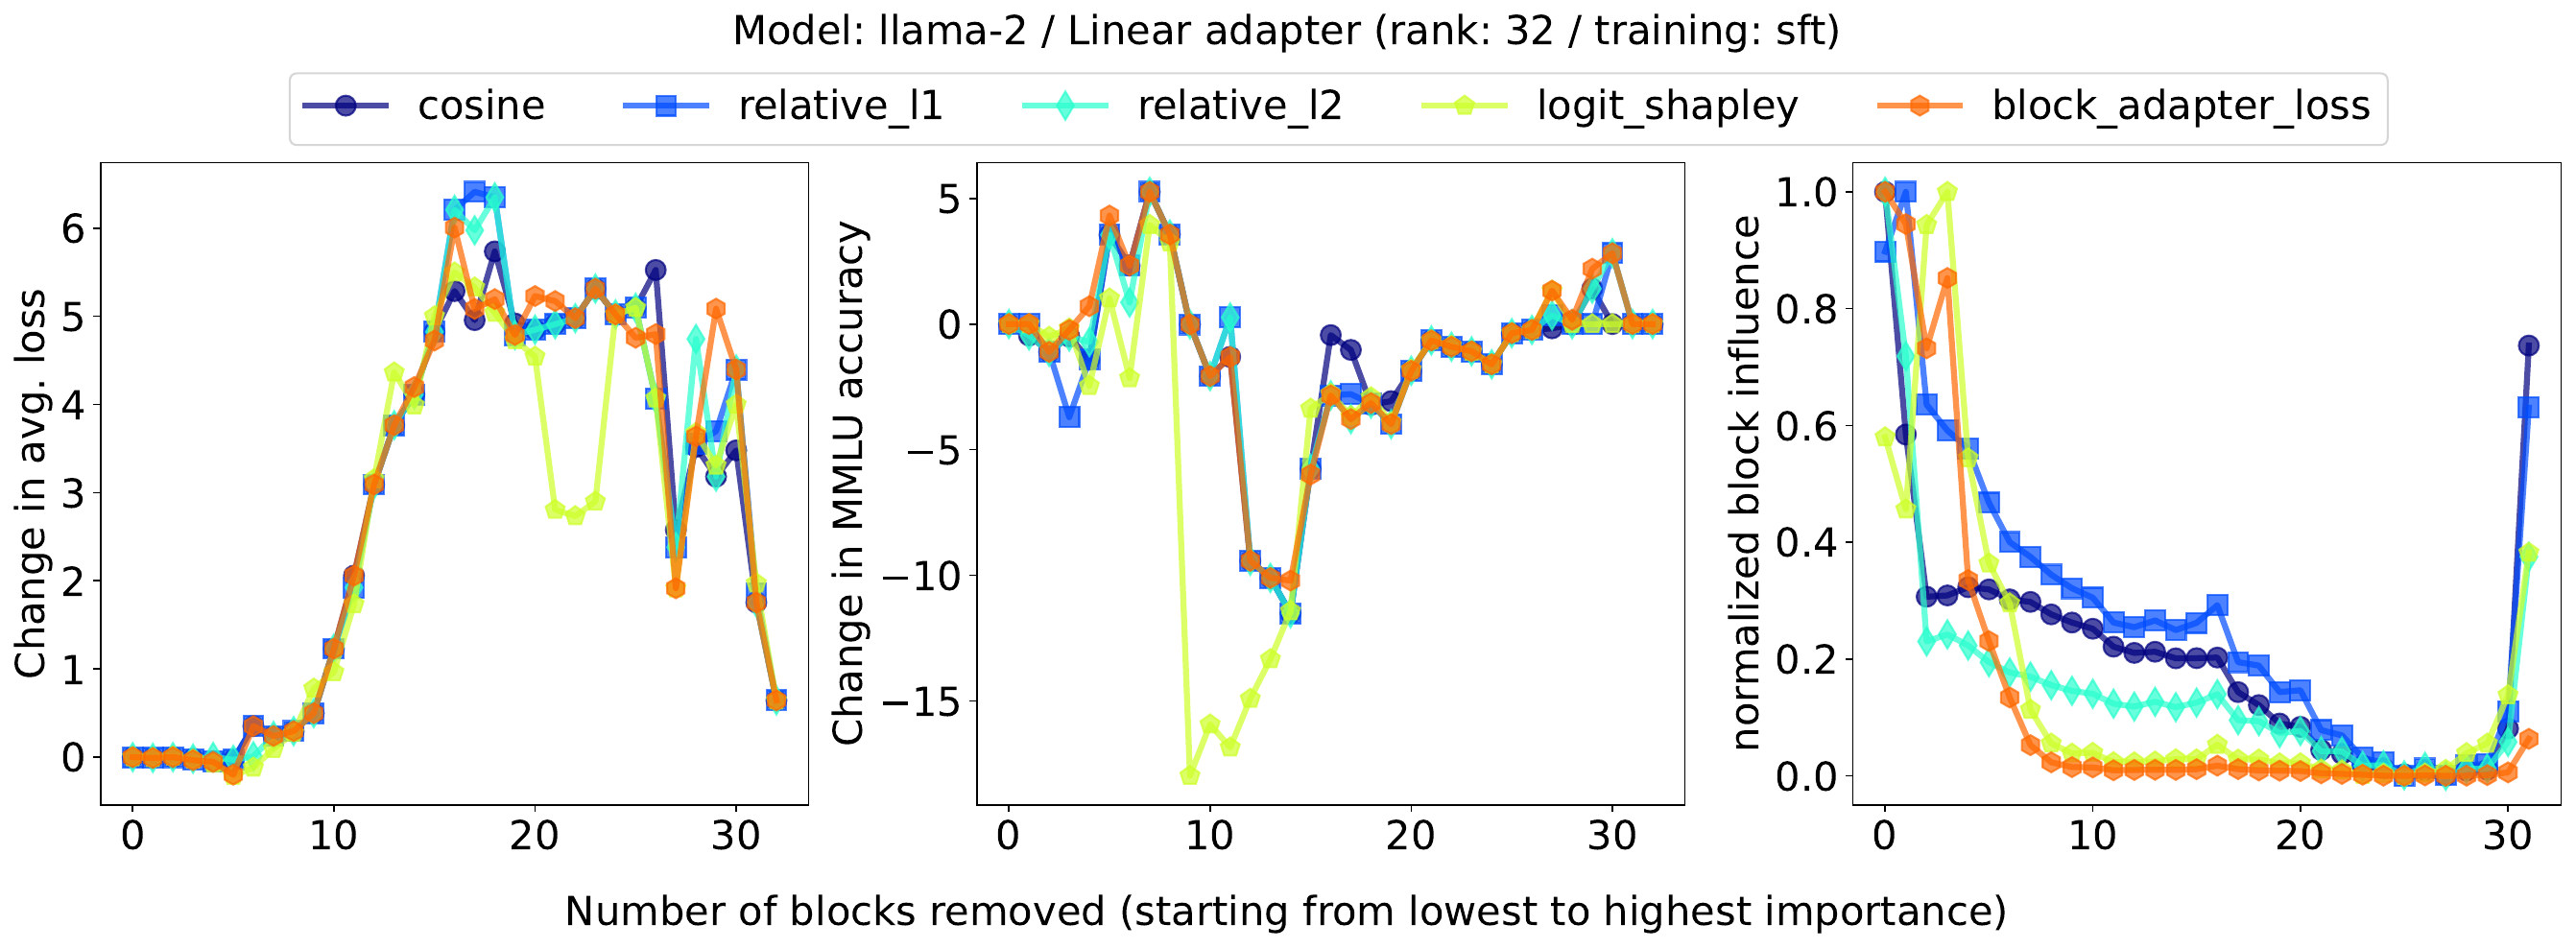}
    }

    \subfloat{
        \includegraphics[width=\textwidth]{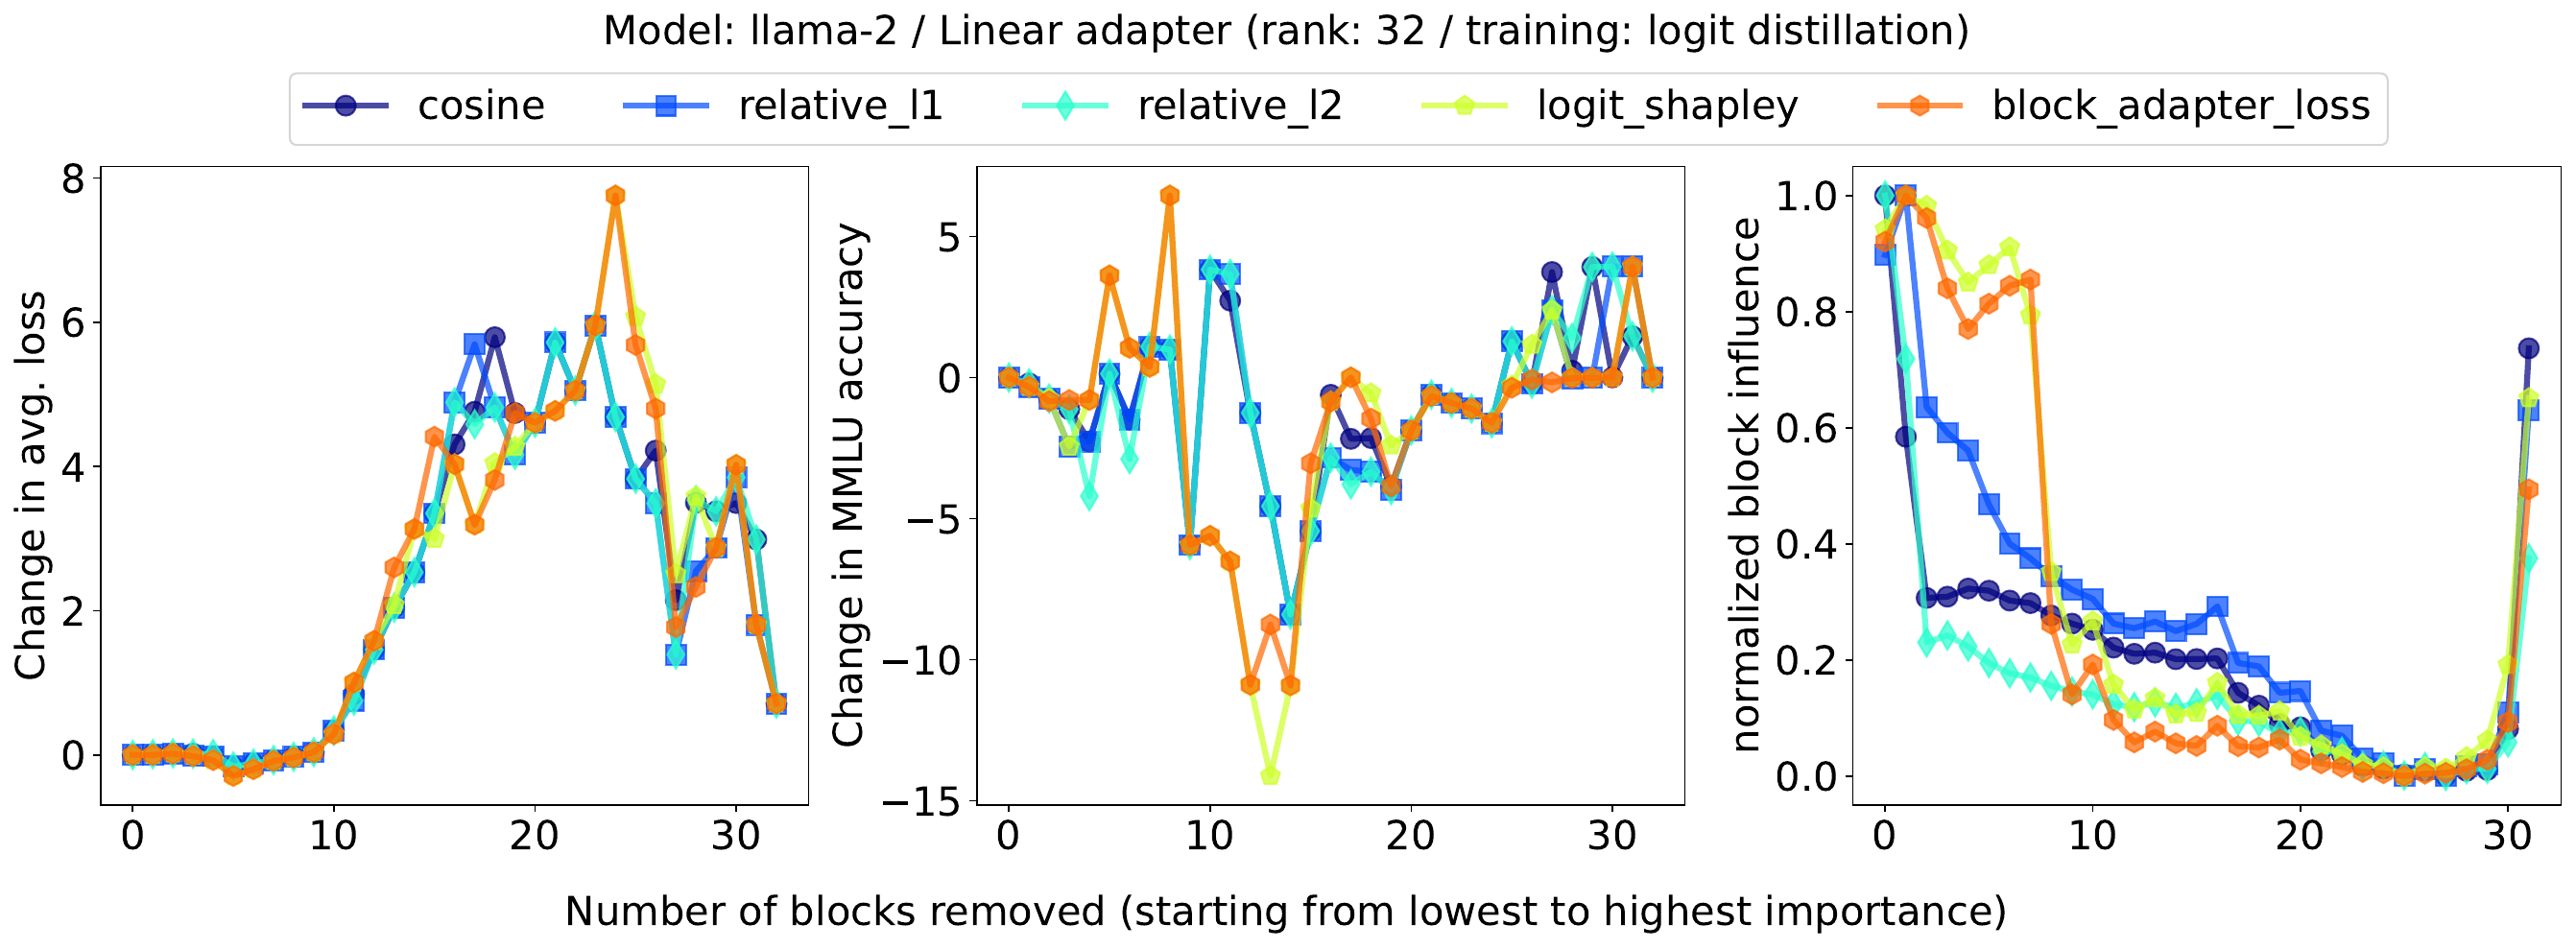}
    }
    \caption{\textbf{Evaluating the relative impact of linear adapters for LLaMa-2 7b with a rank of 32} trained using three different metrics including (a) MSE loss defined on the representation, (b) supervised fine-tuning (SFT), and (c) logit distillation where logits are distilled from the full model. The plot with the original values is presented in Fig.~\ref{fig:linear_adapters_rank_32_llama2}.}
    \label{fig:linear_adapters_rank_32_llama2_relative}
\end{figure}

\begin{figure}
    \centering
    \subfloat{
        \includegraphics[width=\textwidth]{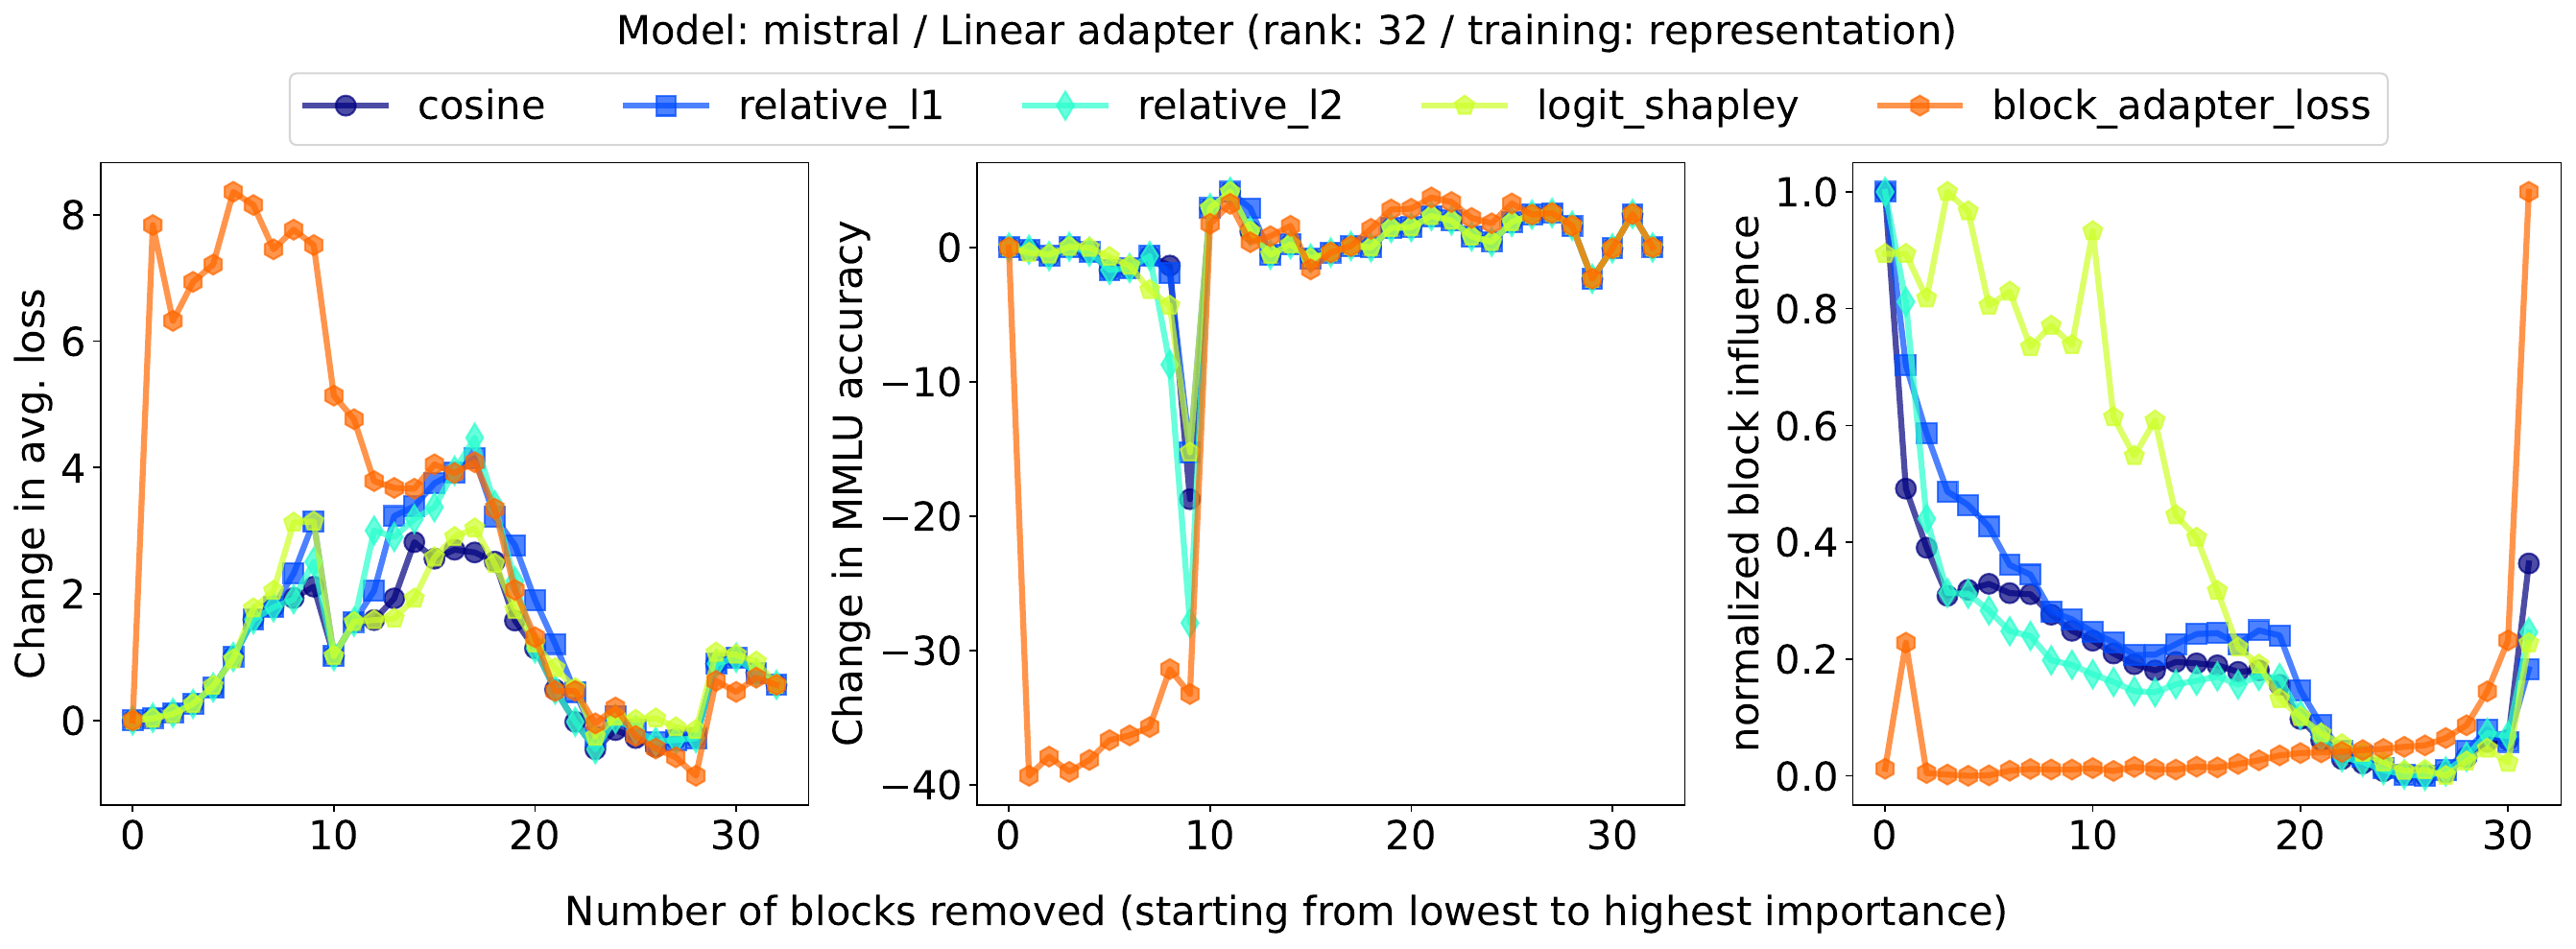}
    }

    \subfloat{
        \includegraphics[width=\textwidth]{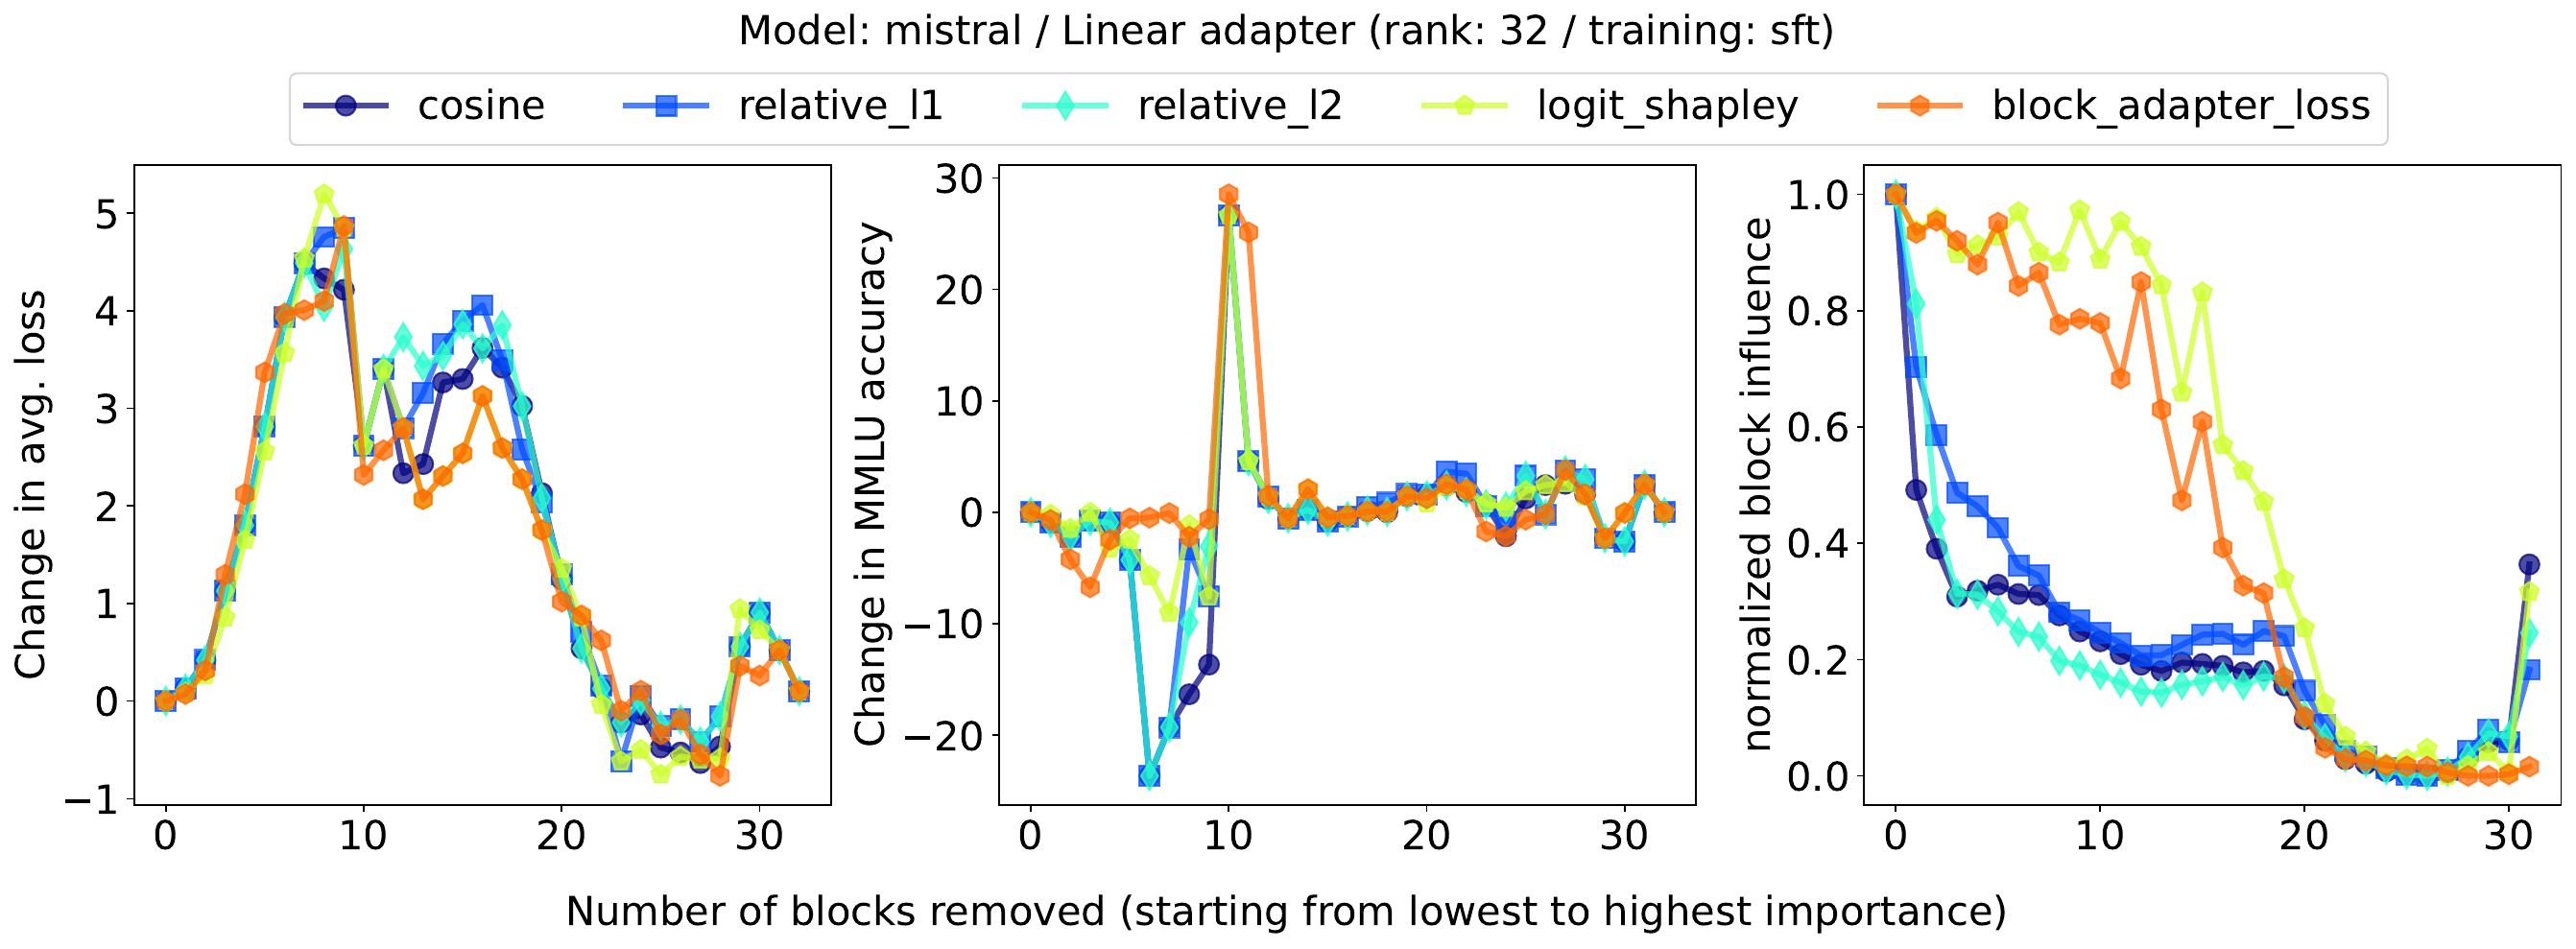}
    }

    \subfloat{
        \includegraphics[width=\textwidth]{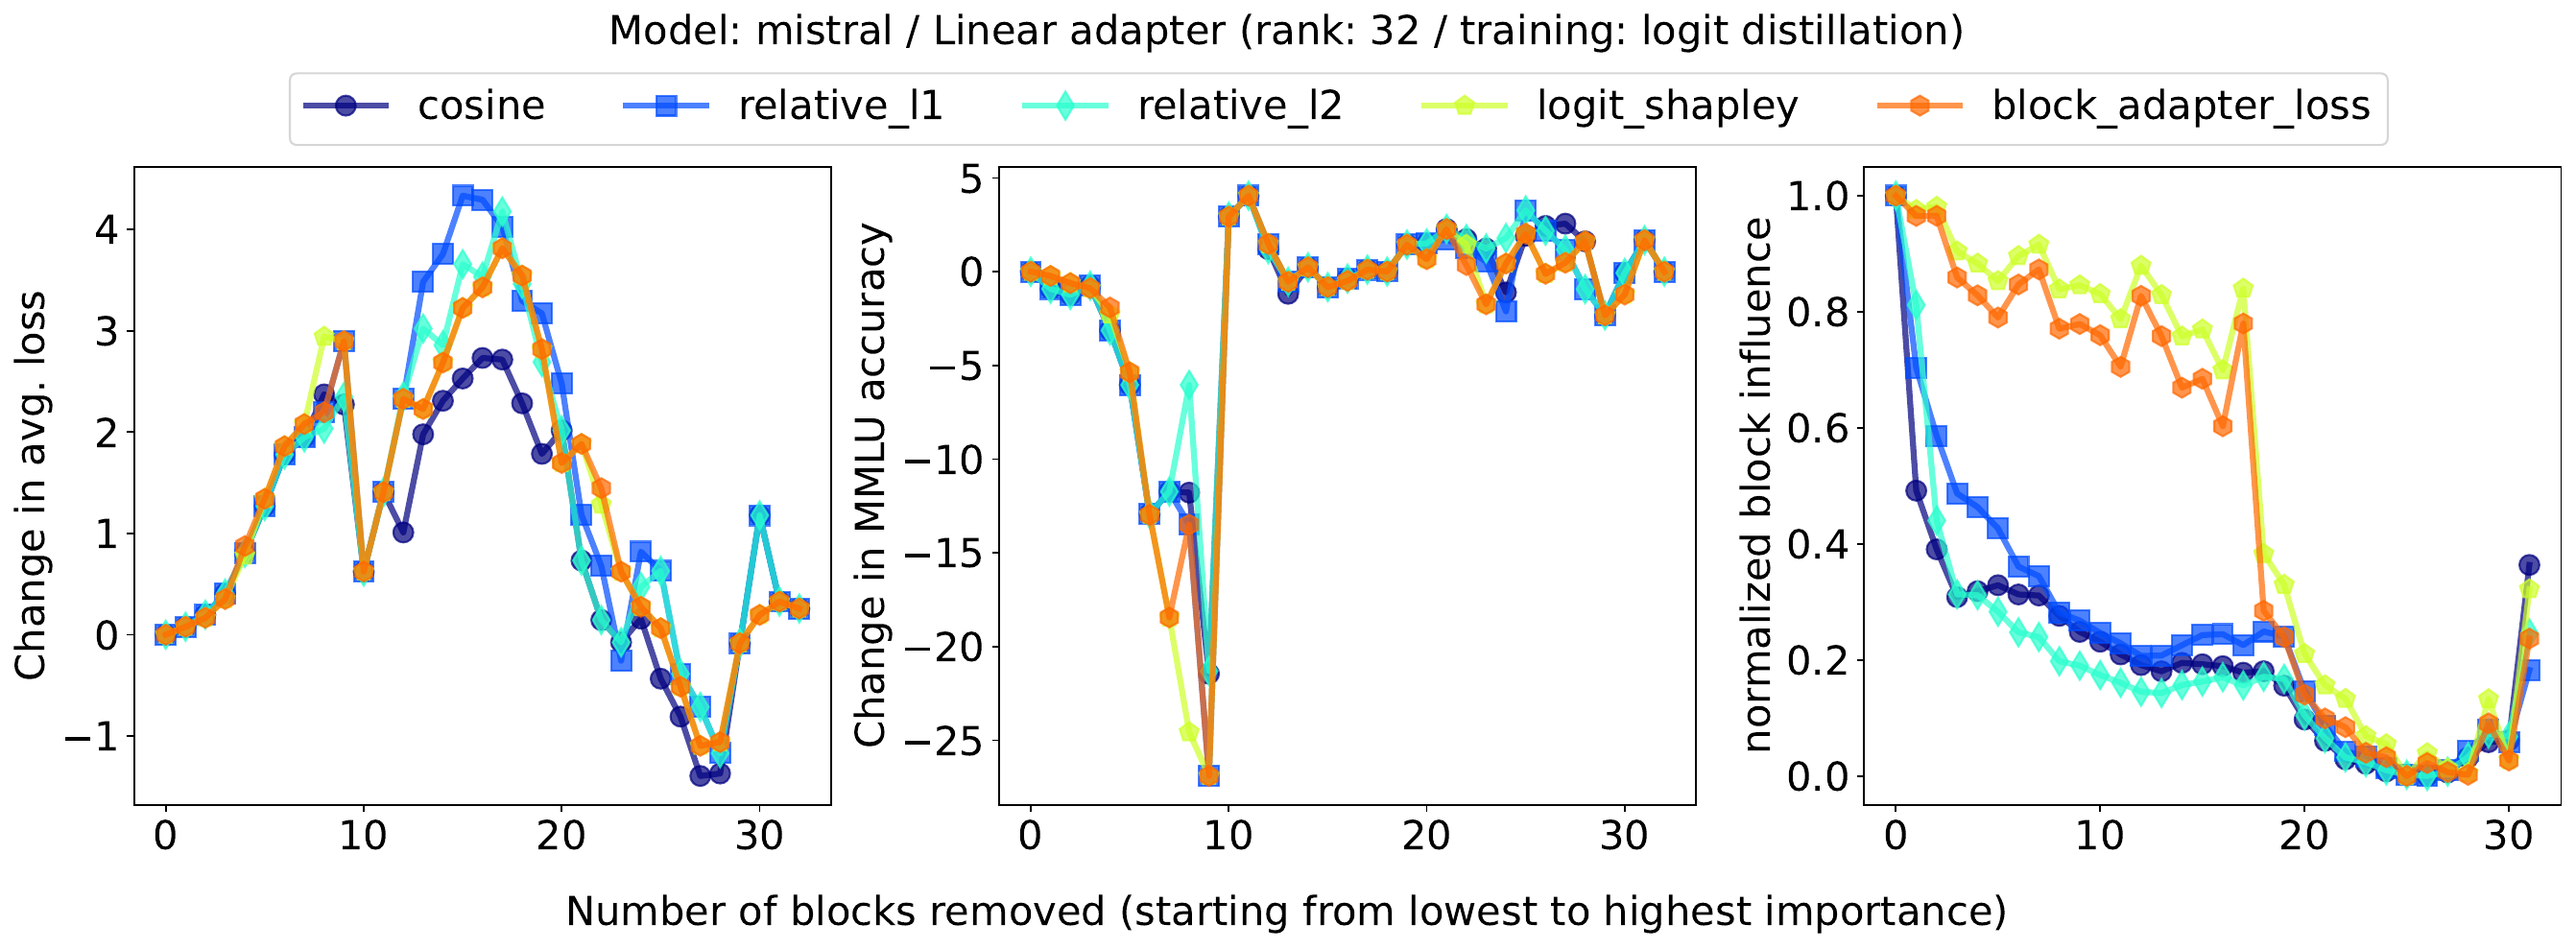}
    }
    \caption{\textbf{Evaluating the relative impact of linear adapters for Mistral 7b with a rank of 32} trained using three different metrics including (a) MSE loss defined on the representation, (b) supervised fine-tuning (SFT), and (c) logit distillation where logits are distilled from the full model. The plot with the original values is presented in Fig.~\ref{fig:linear_adapters_rank_32_mistral}.}
    \label{fig:linear_adapters_rank_32_mistral_relative}
\end{figure}

Results for LLaMa-2 7b and Mistral 7b with an adapter rank of 32 on a relative scale are visualized in Fig.~\ref{fig:linear_adapters_rank_32_llama2_relative} and Fig.~\ref{fig:linear_adapters_rank_32_mistral_relative} respectively.

\begin{figure}
    \centering
    \subfloat{
        \includegraphics[width=\textwidth]{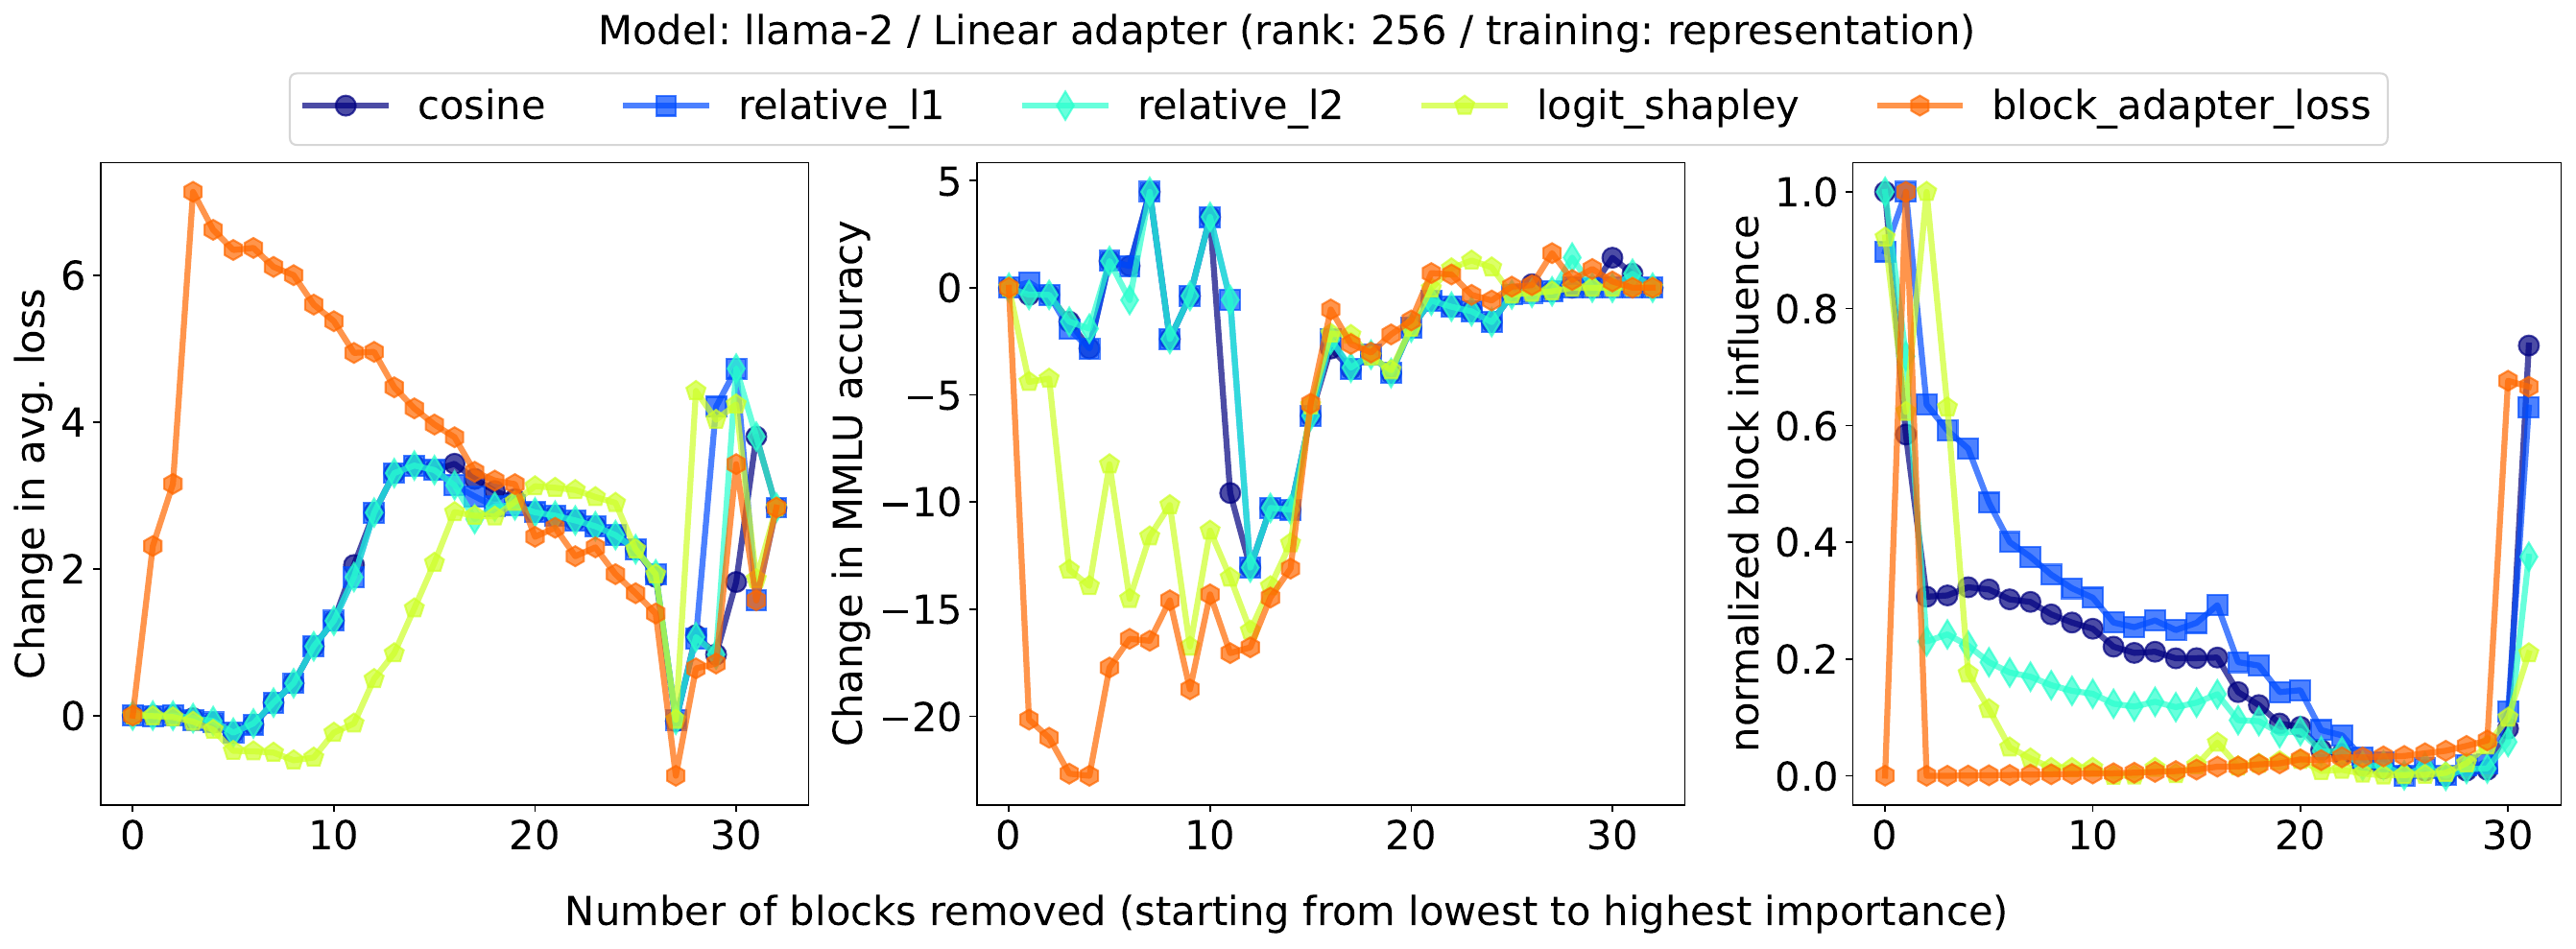}
    }

    \subfloat{
        \includegraphics[width=\textwidth]{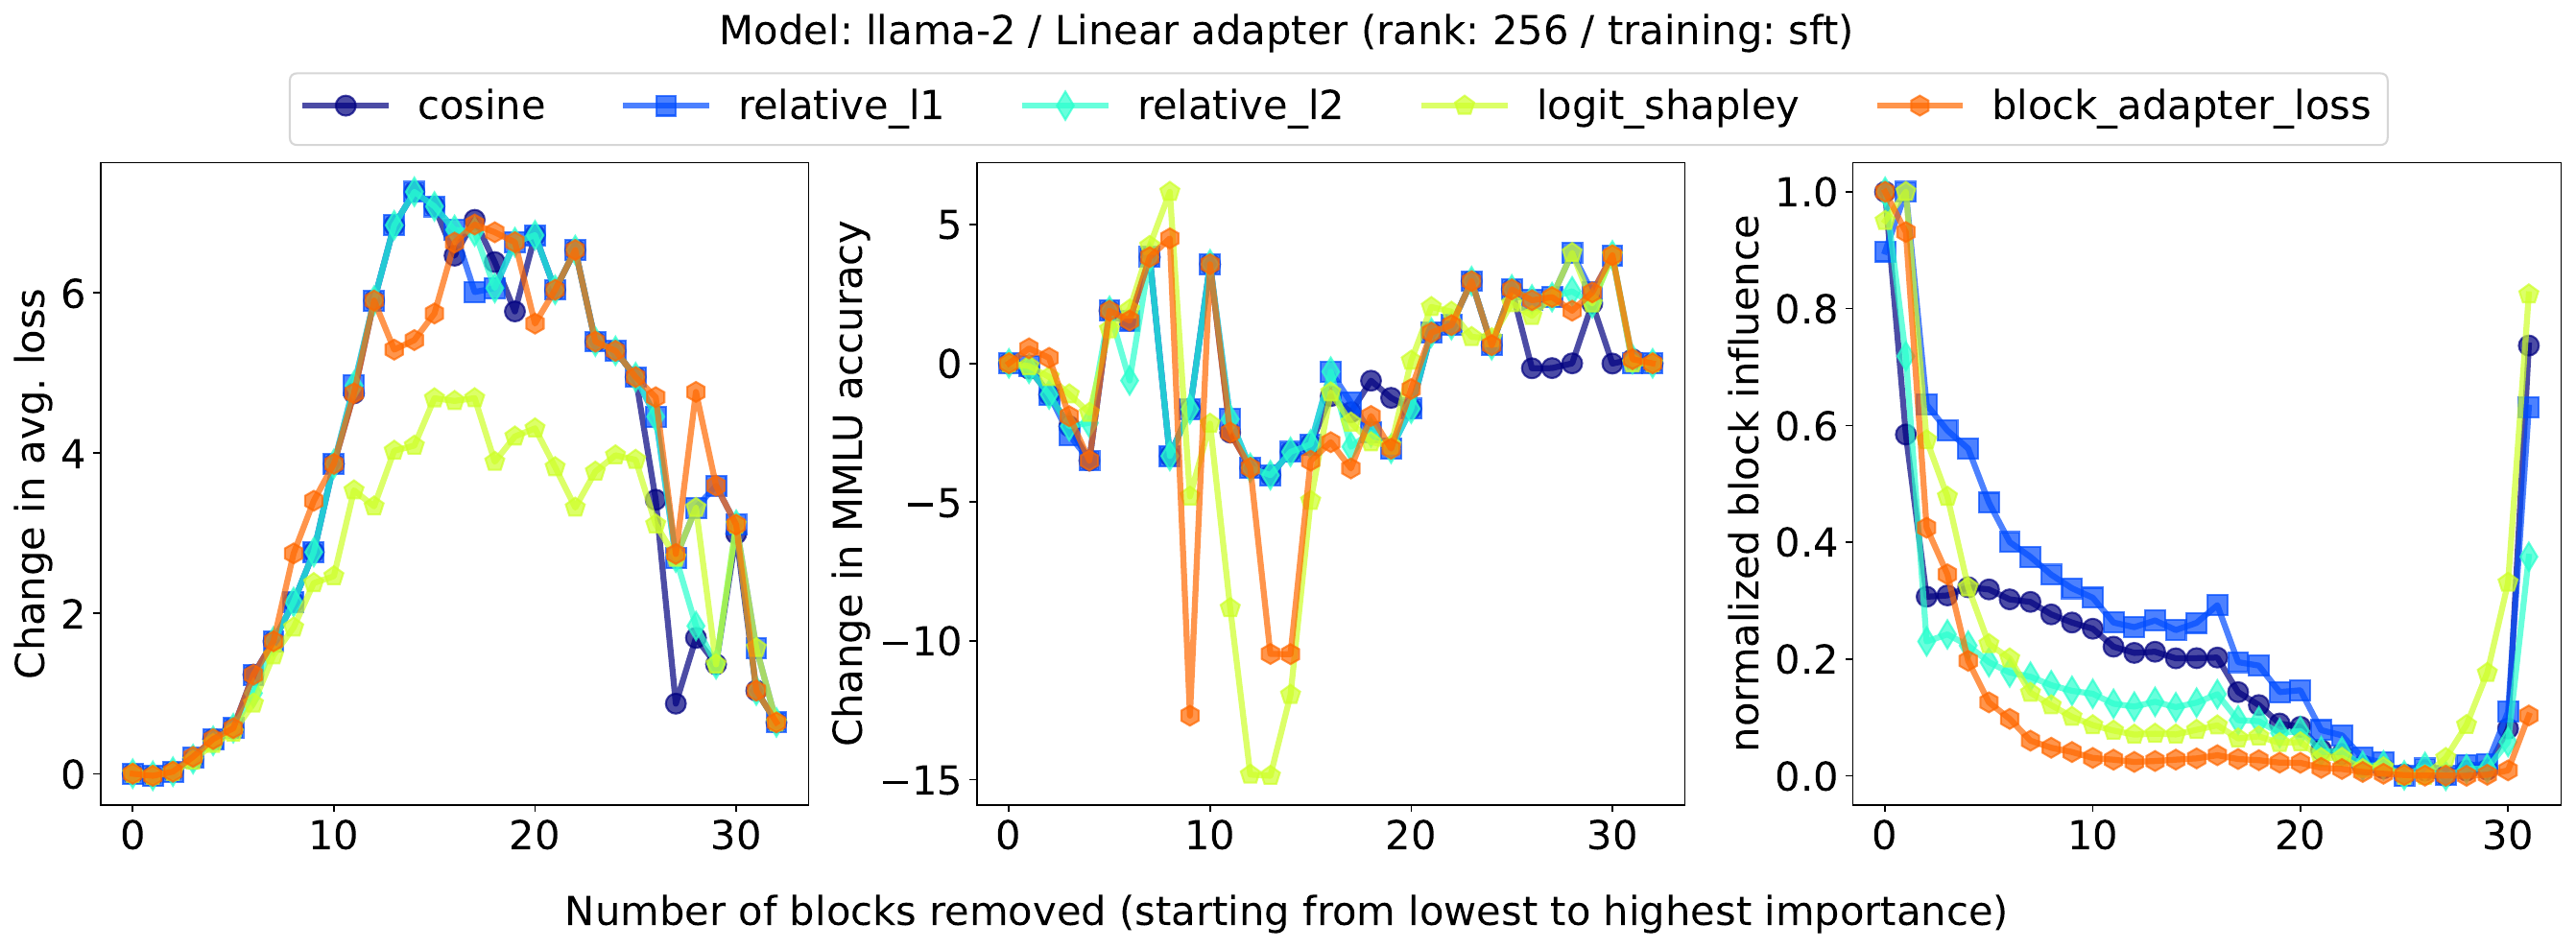}
    }

    \subfloat{
        \includegraphics[width=\textwidth]{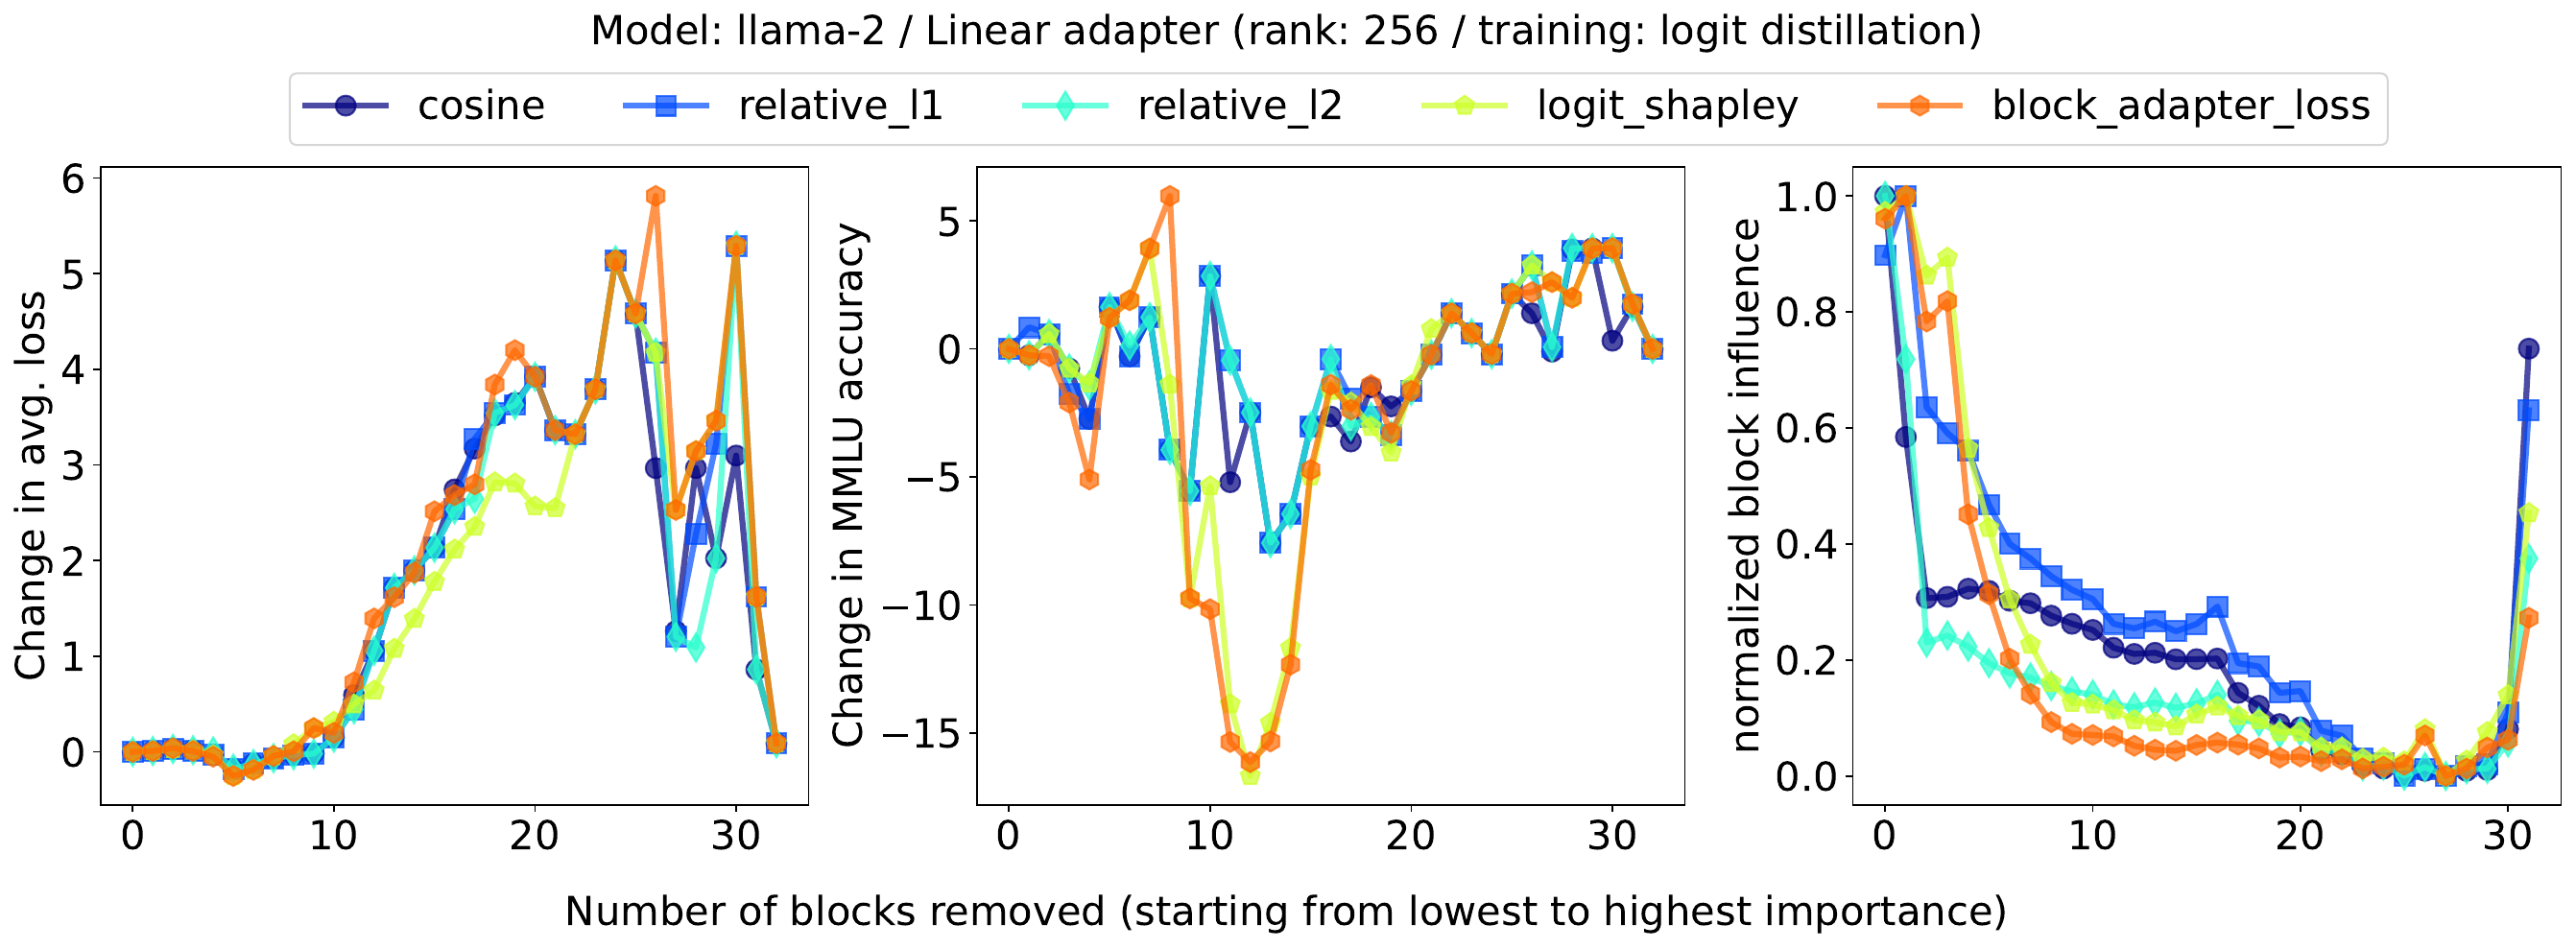}
    }
    \caption{\textbf{Evaluating the relative impact of linear adapters for LLaMa-2 7b with a rank of 256} trained using three different metrics including (a) MSE loss defined on the representation, (b) supervised fine-tuning (SFT), and (c) logit distillation where logits are distilled from the full model. The plot with the original values is presented in Fig.~\ref{fig:linear_adapters_rank_256_llama2}.}
    \label{fig:linear_adapters_rank_256_llama2_relative}
\end{figure}

\begin{figure}
    \centering
    \subfloat{
        \includegraphics[width=\textwidth]{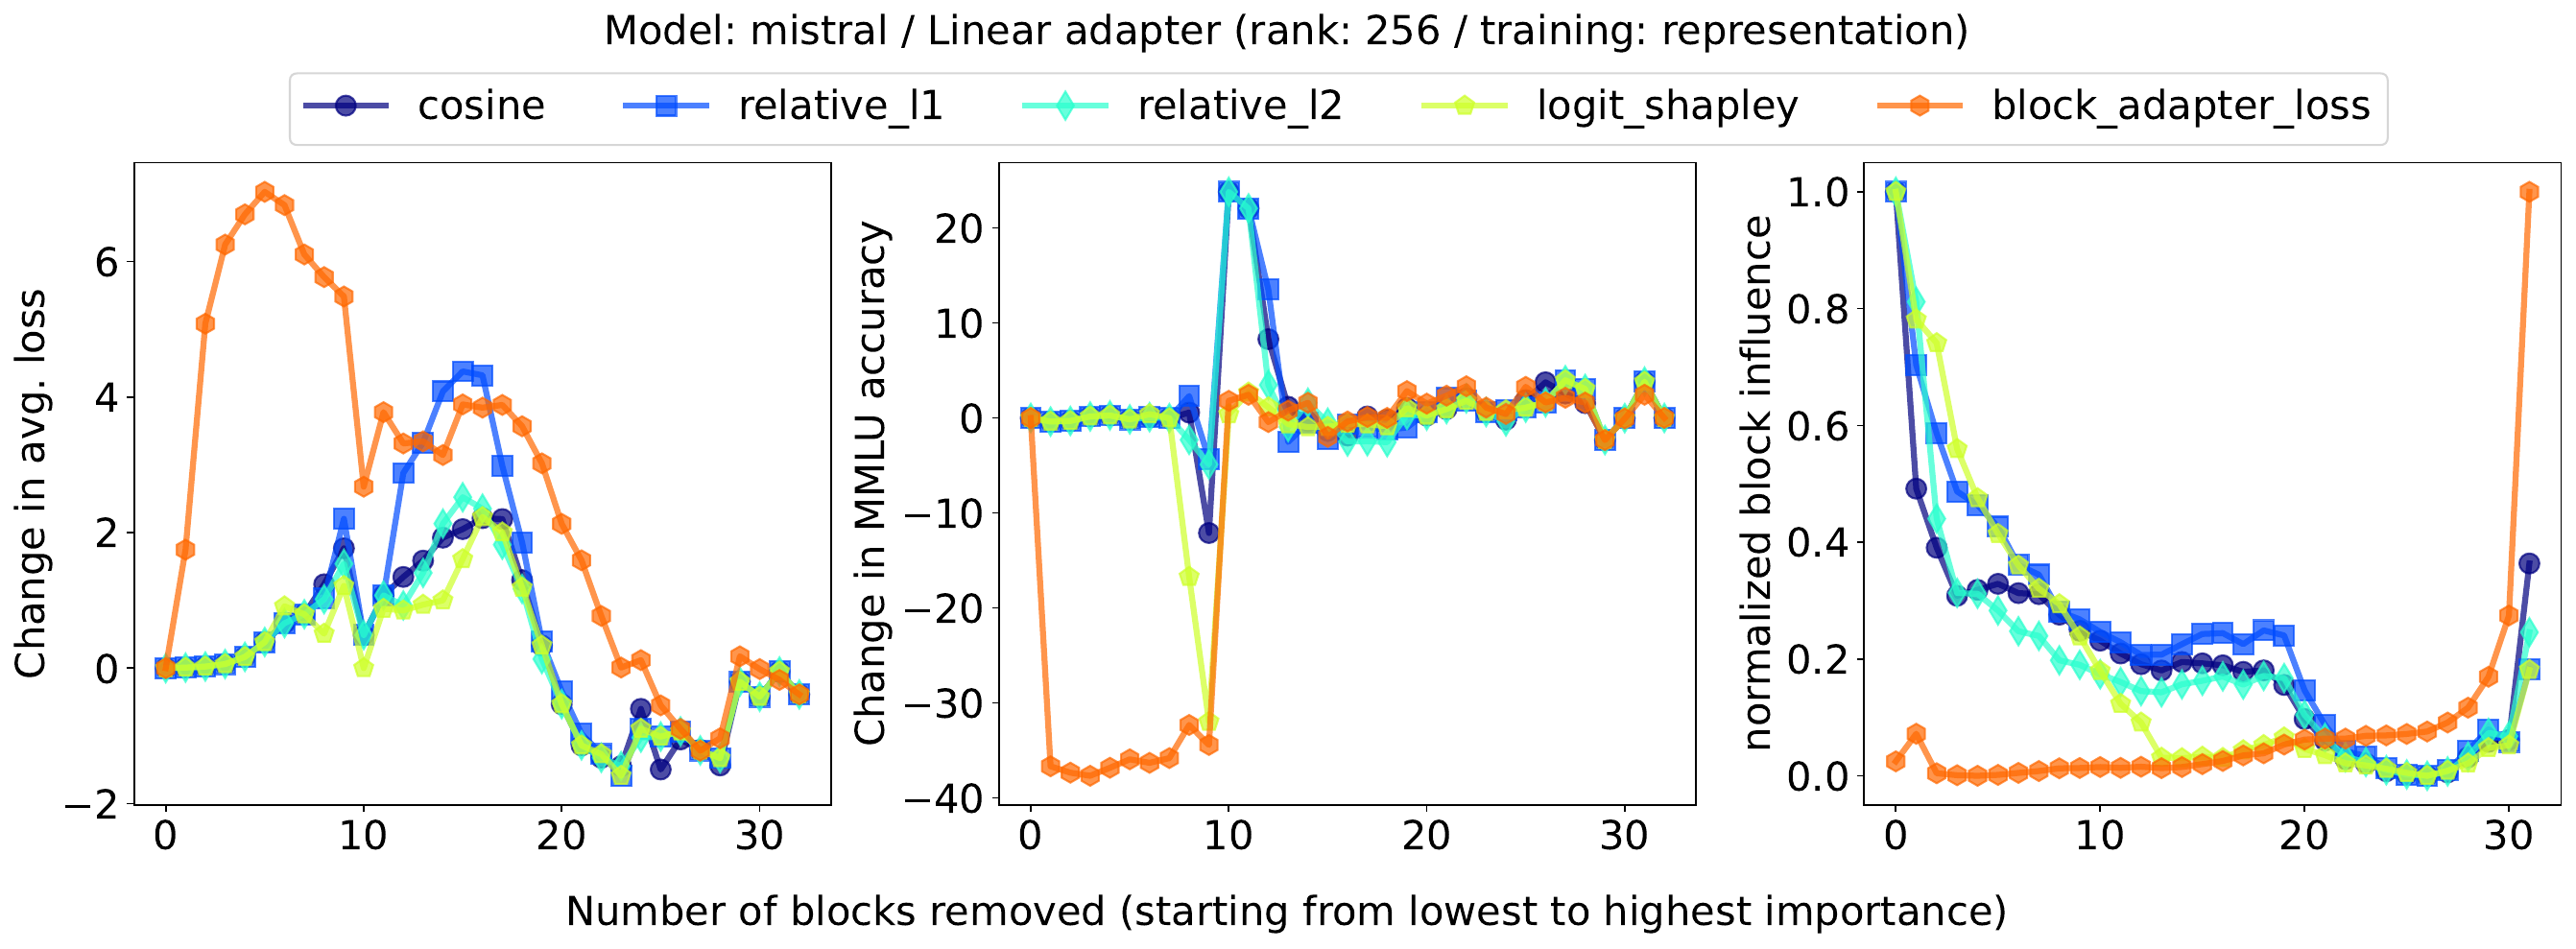}
    }

    \subfloat{
        \includegraphics[width=\textwidth]{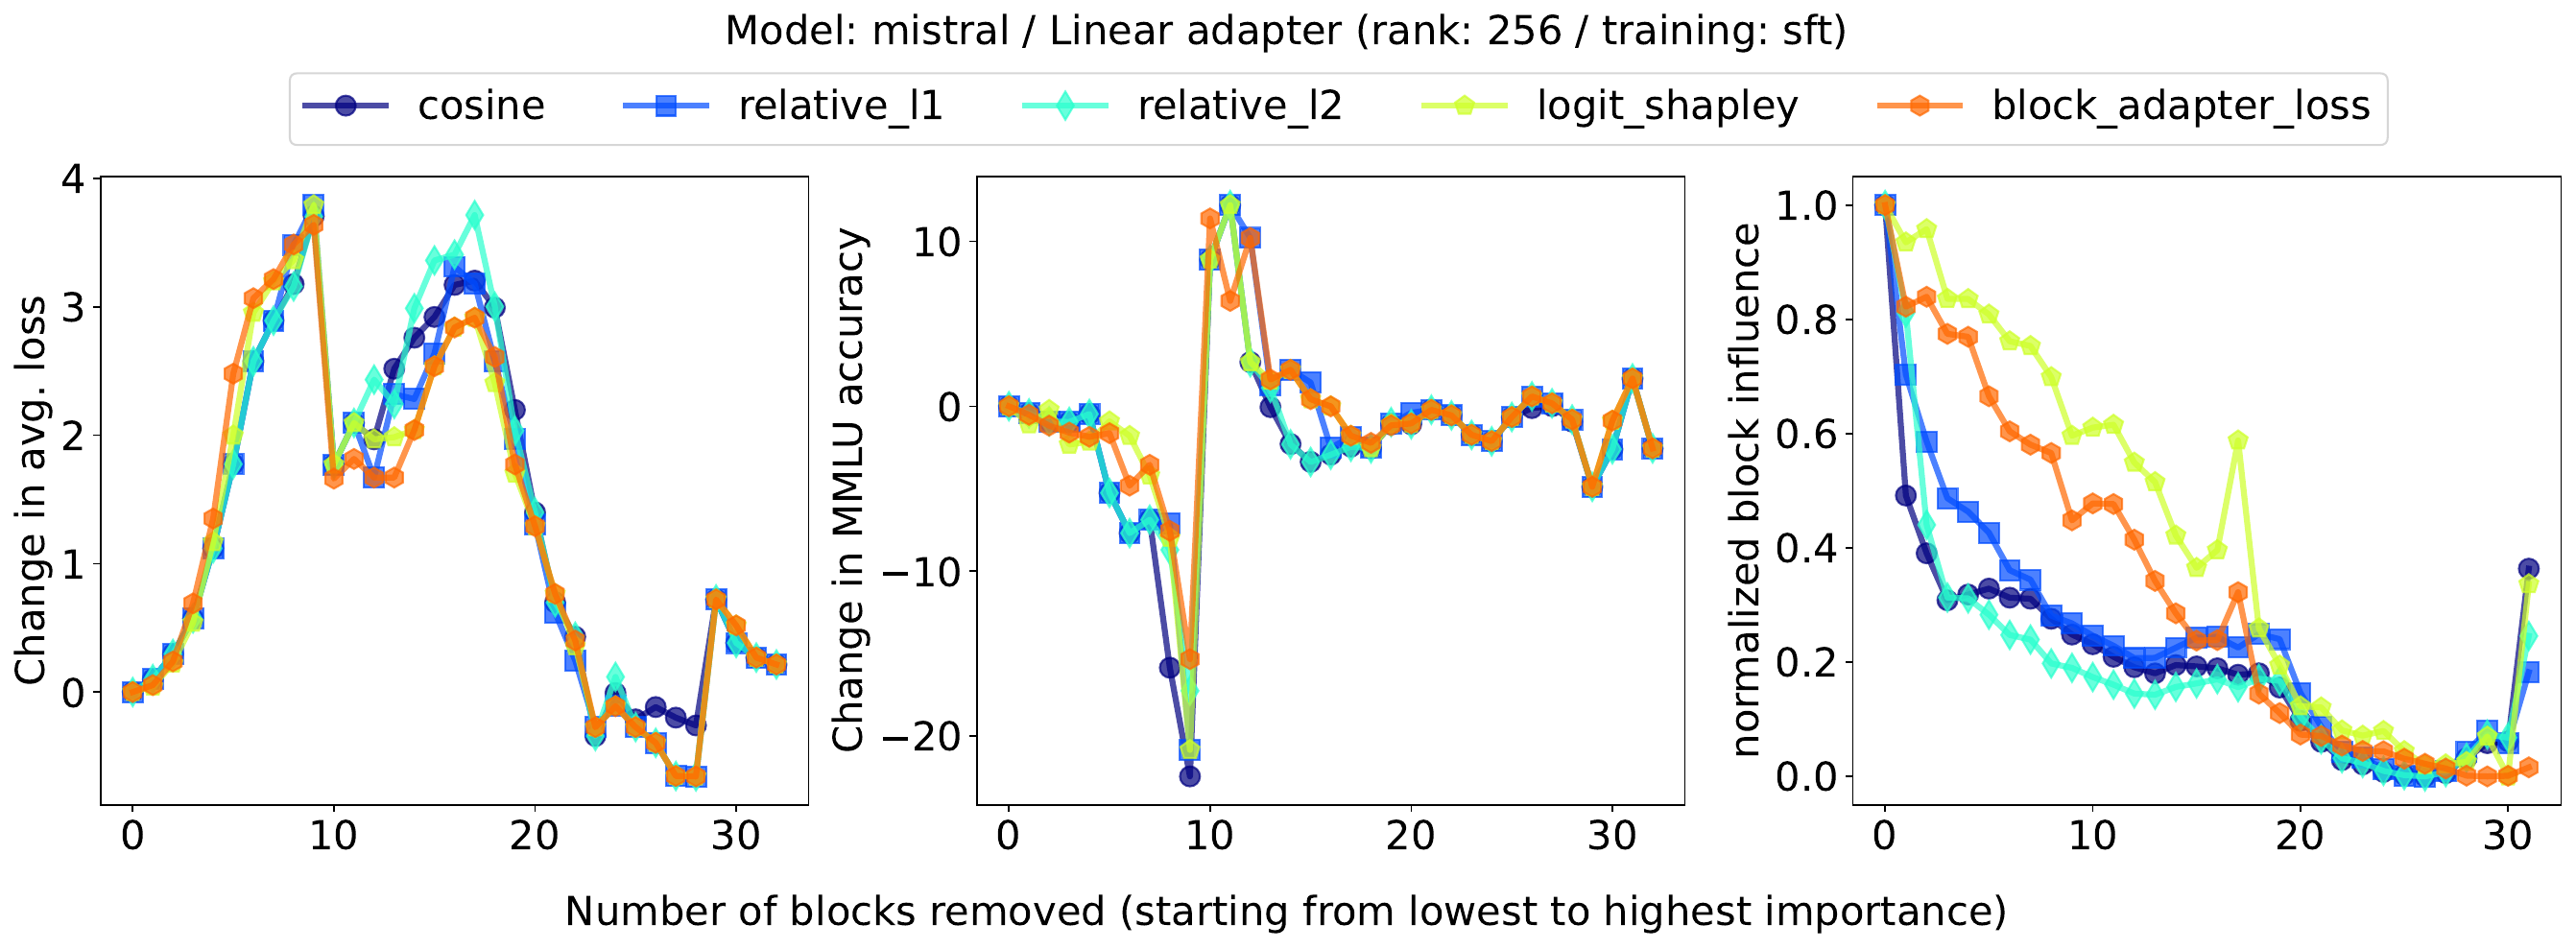}
    }

    \subfloat{
        \includegraphics[width=\textwidth]{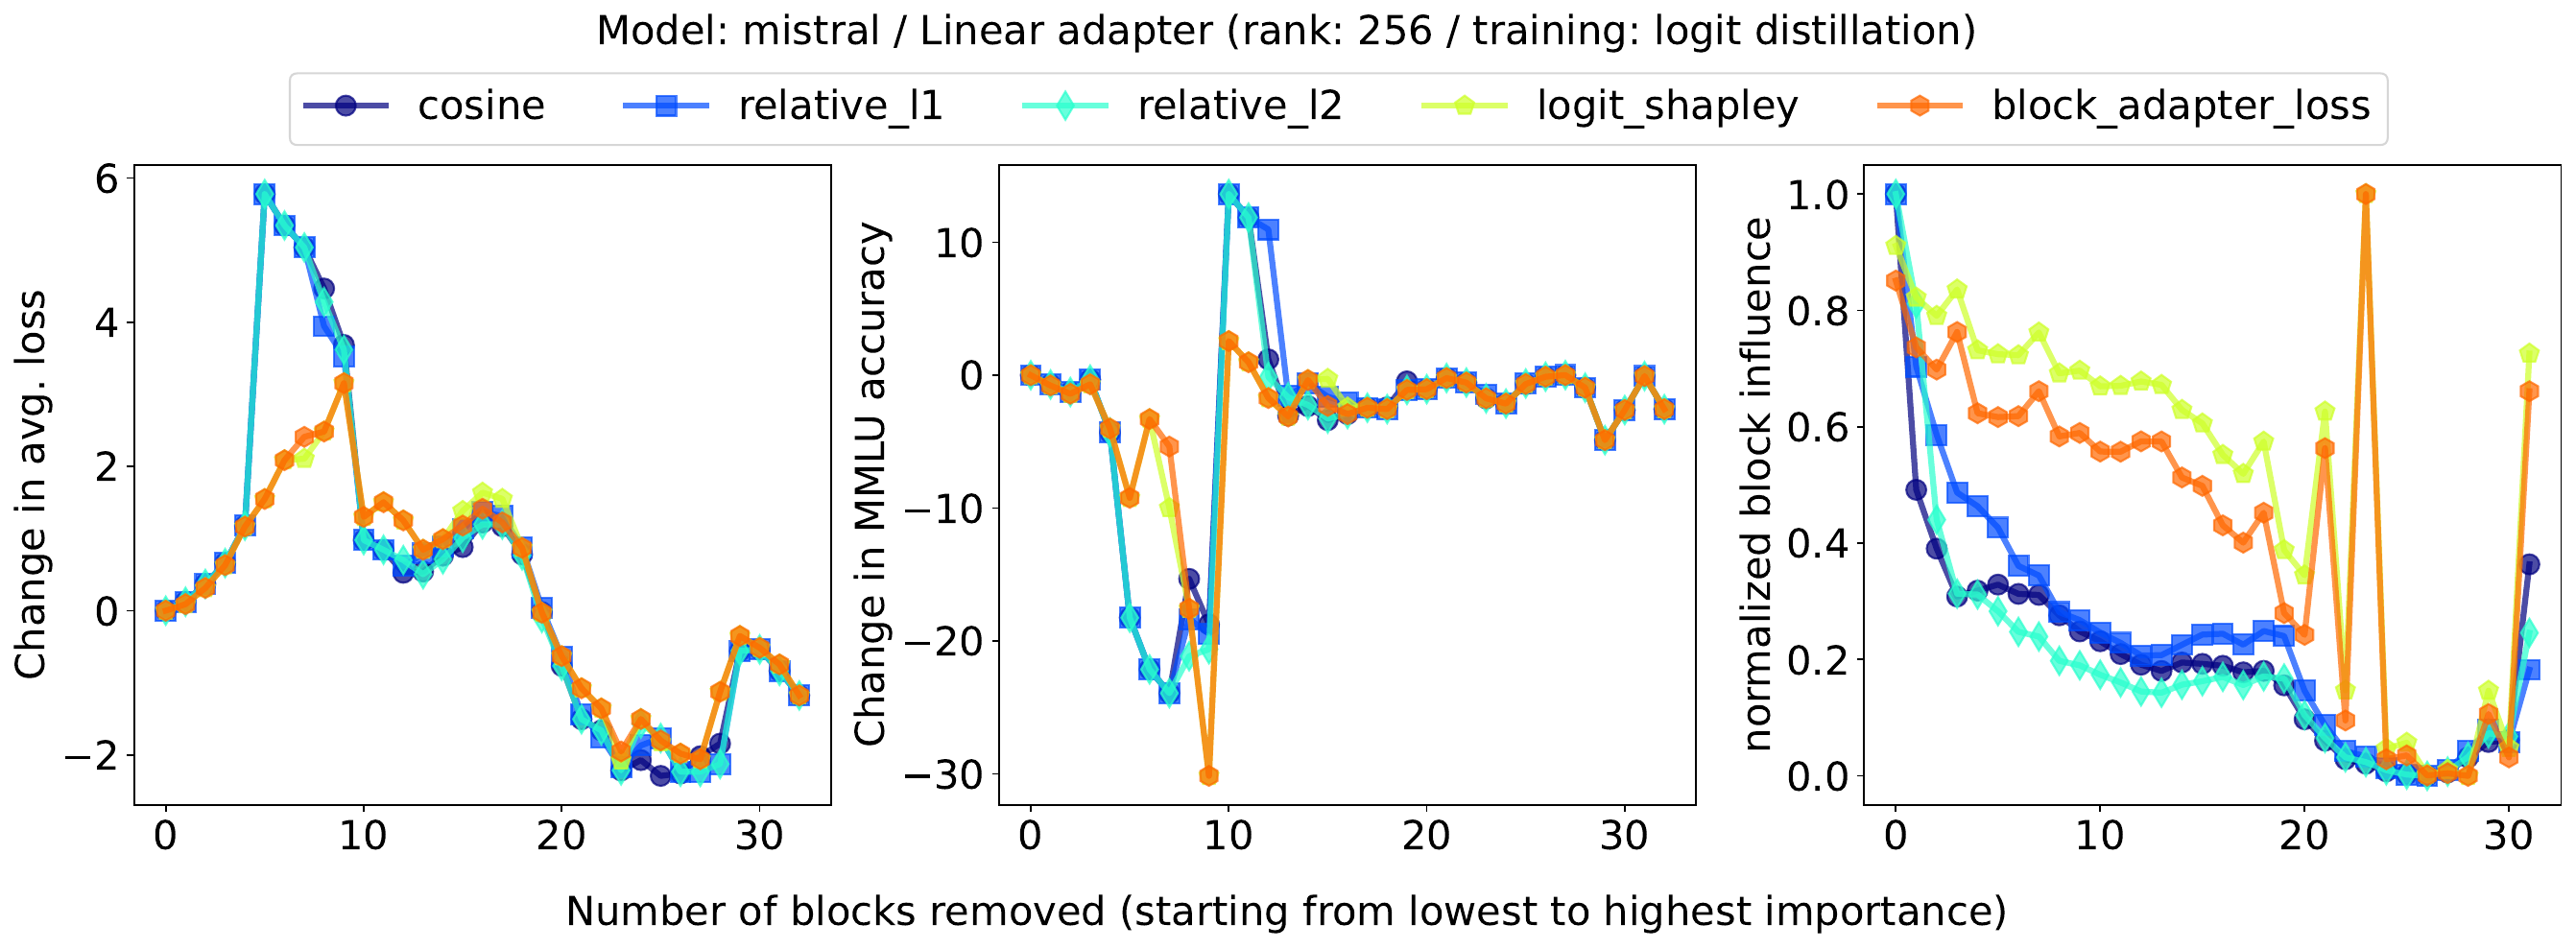}
    }
    \caption{\textbf{Evaluating the relative impact of linear adapters for Mistral 7b with a rank of 256} trained using three different metrics including (a) MSE loss defined on the representation, (b) supervised fine-tuning (SFT), and (c) logit distillation where logits are distilled from the full model. The plot with the original values is presented in Fig.~\ref{fig:linear_adapters_rank_256_mistral}.}
    \label{fig:linear_adapters_rank_256_mistral_relative}
\end{figure}

Results for LLaMa-2 7b and Mistral 7b with an adapter rank of 256 on a relative scale are visualized in Fig.~\ref{fig:linear_adapters_rank_256_llama2_relative} and Fig.~\ref{fig:linear_adapters_rank_256_mistral_relative} respectively.

\subsection{Low-rank linear adapters (original results).}
\label{appendix:low_rank_original_results}

\begin{figure}
    \centering
    \subfloat{
        \includegraphics[width=\textwidth]{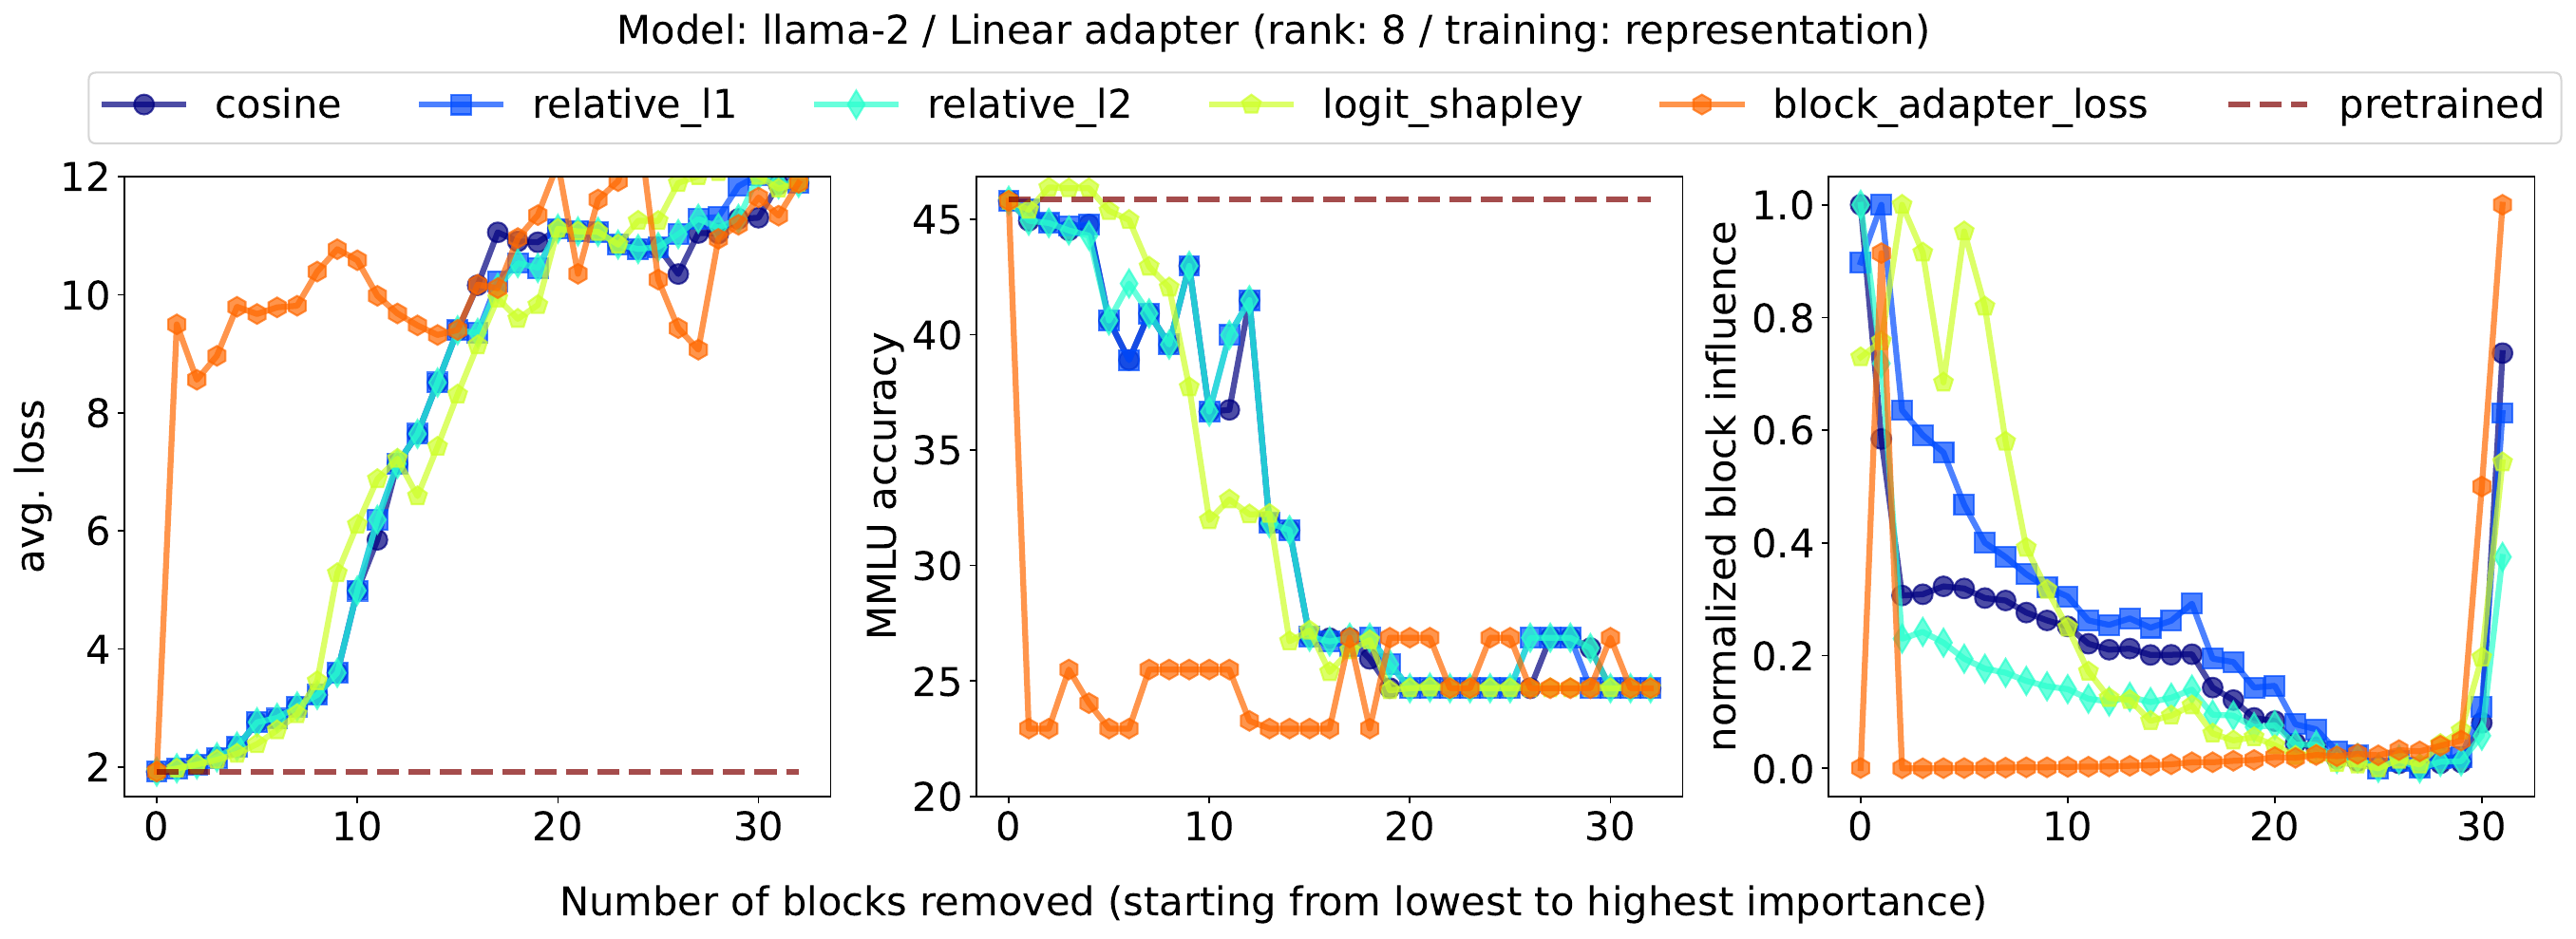}
    }

    \subfloat{
        \includegraphics[width=\textwidth]{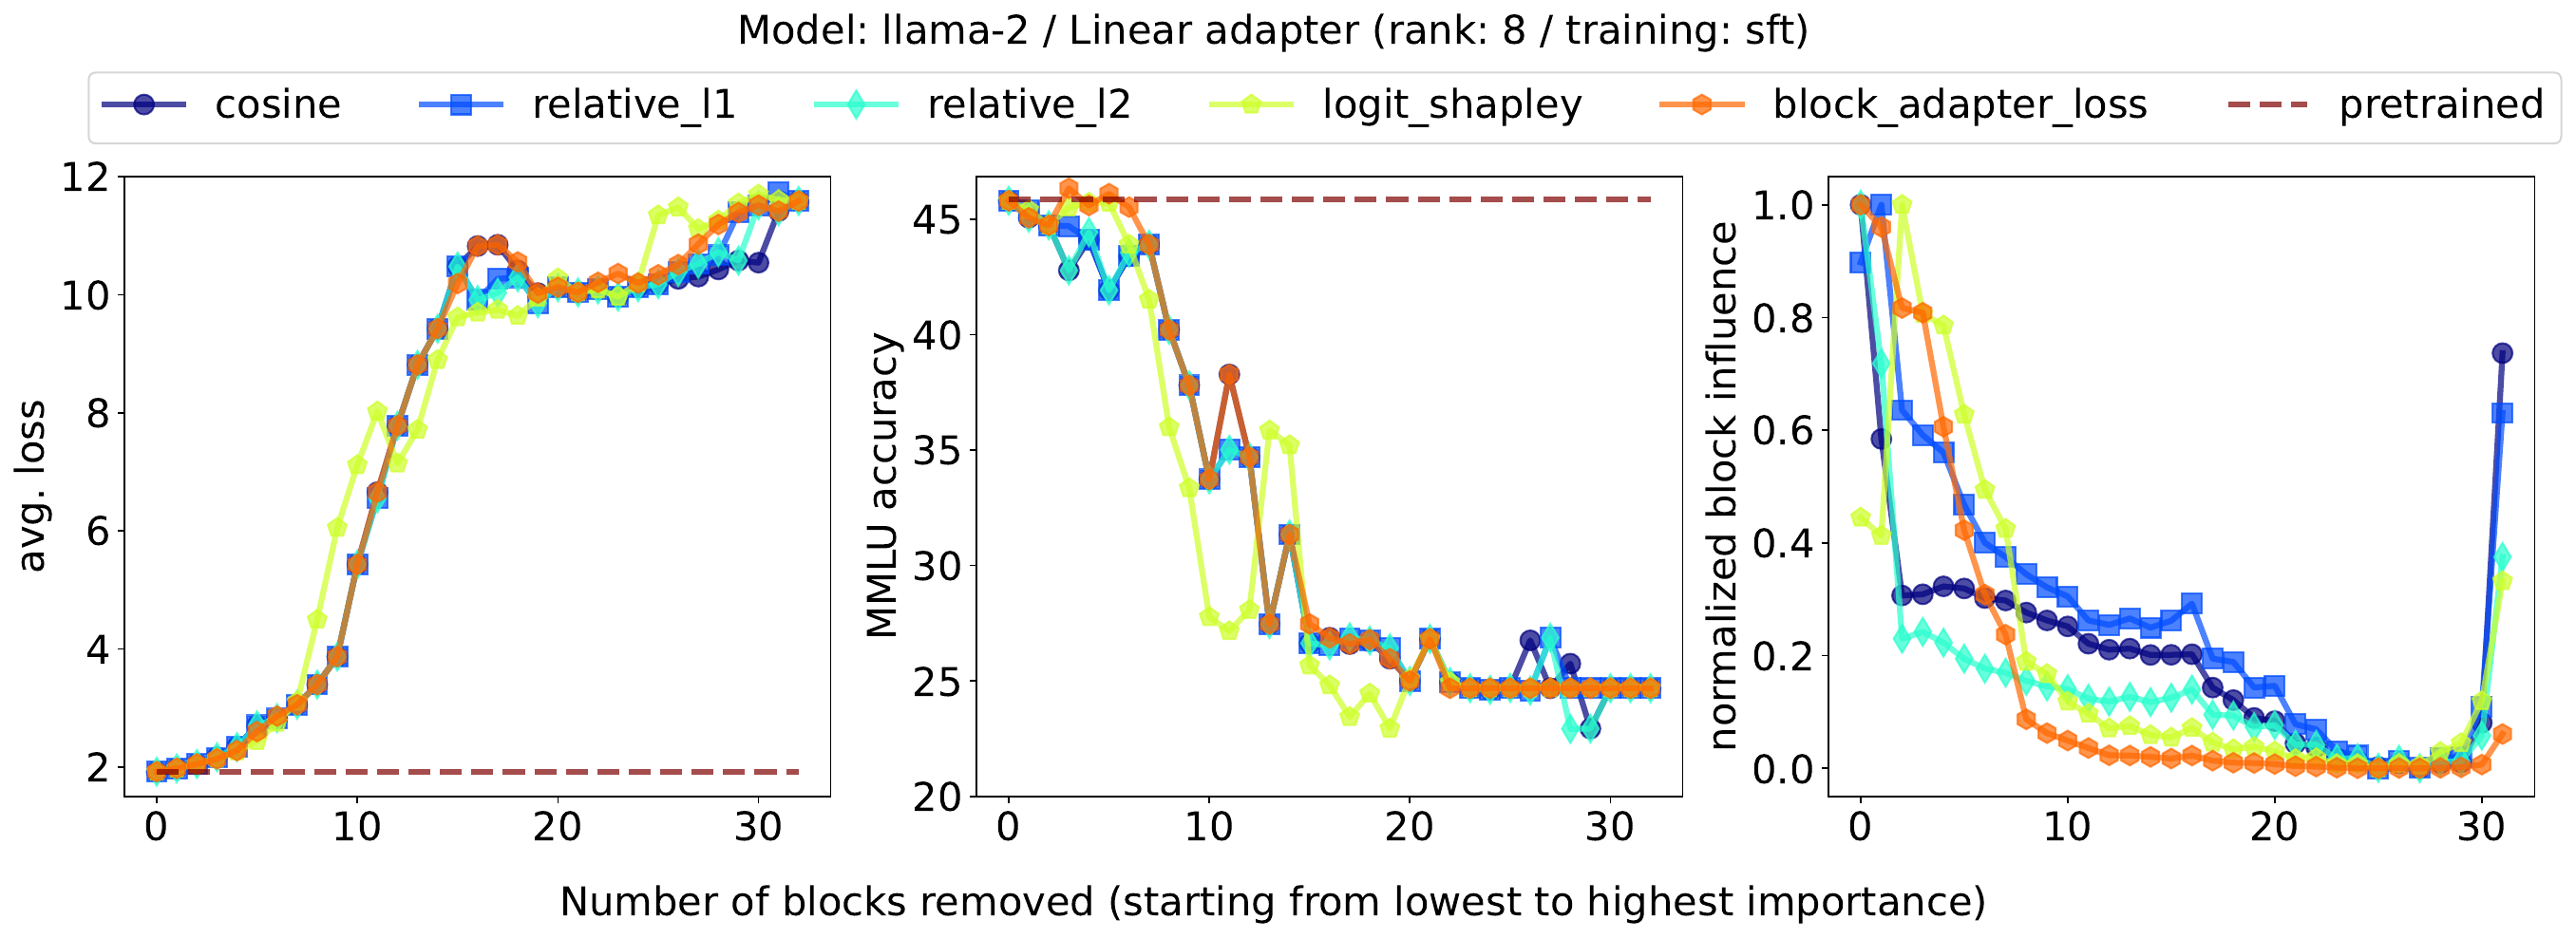}
    }

    \subfloat{
        \includegraphics[width=\textwidth]{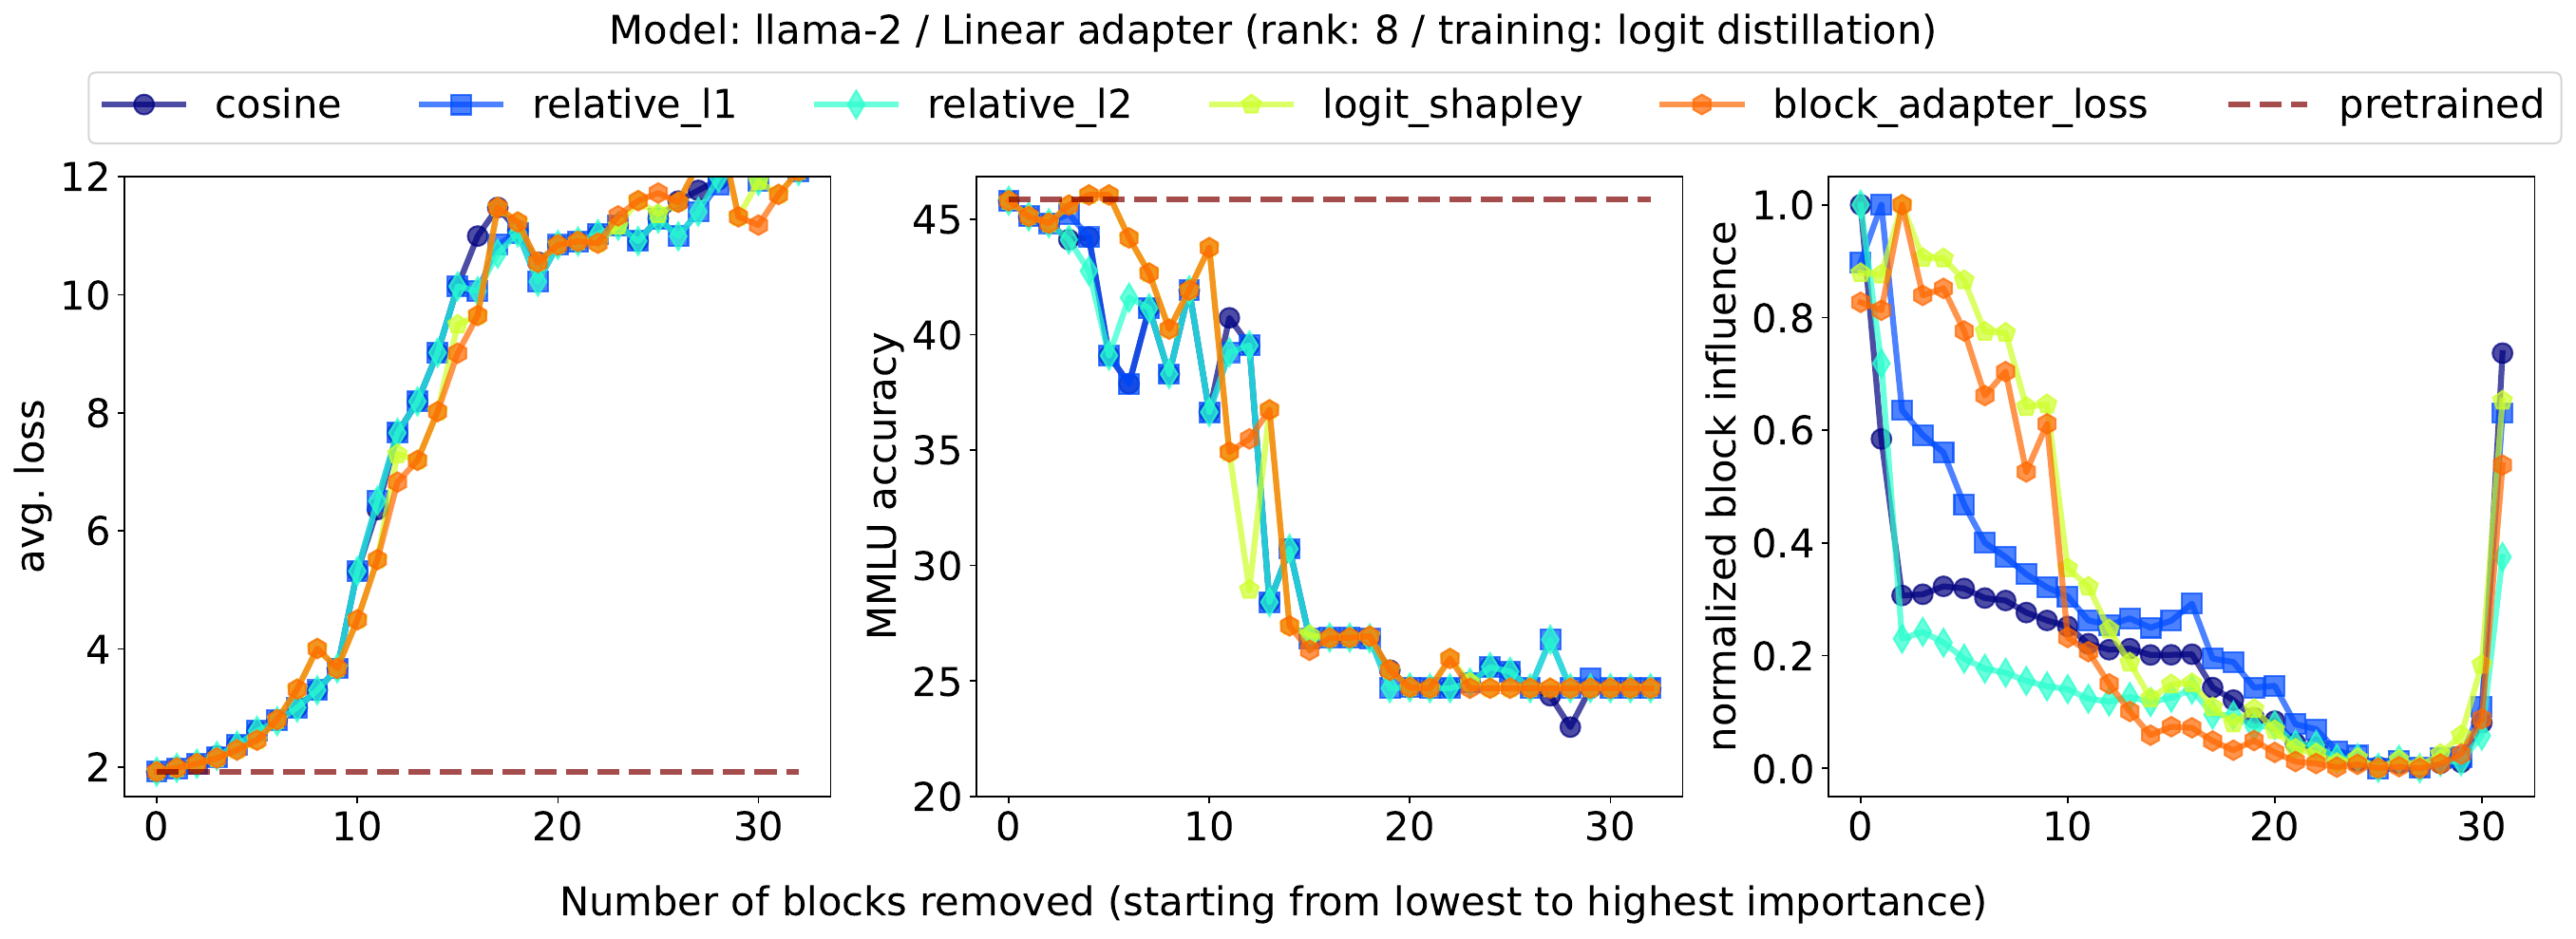}
    }
    \caption{\textbf{Evaluating the impact of linear adapters for LLaMa-2 7b with a rank of 8} trained using three different metrics including (a) MSE loss defined on the representation, (b) supervised fine-tuning (SFT), and (c) logit distillation where logits are distilled from the full model.}
    \label{fig:linear_adapters_rank_8_llama2}
\end{figure}

\begin{figure}
    \centering
    \subfloat{
        \includegraphics[width=\textwidth]{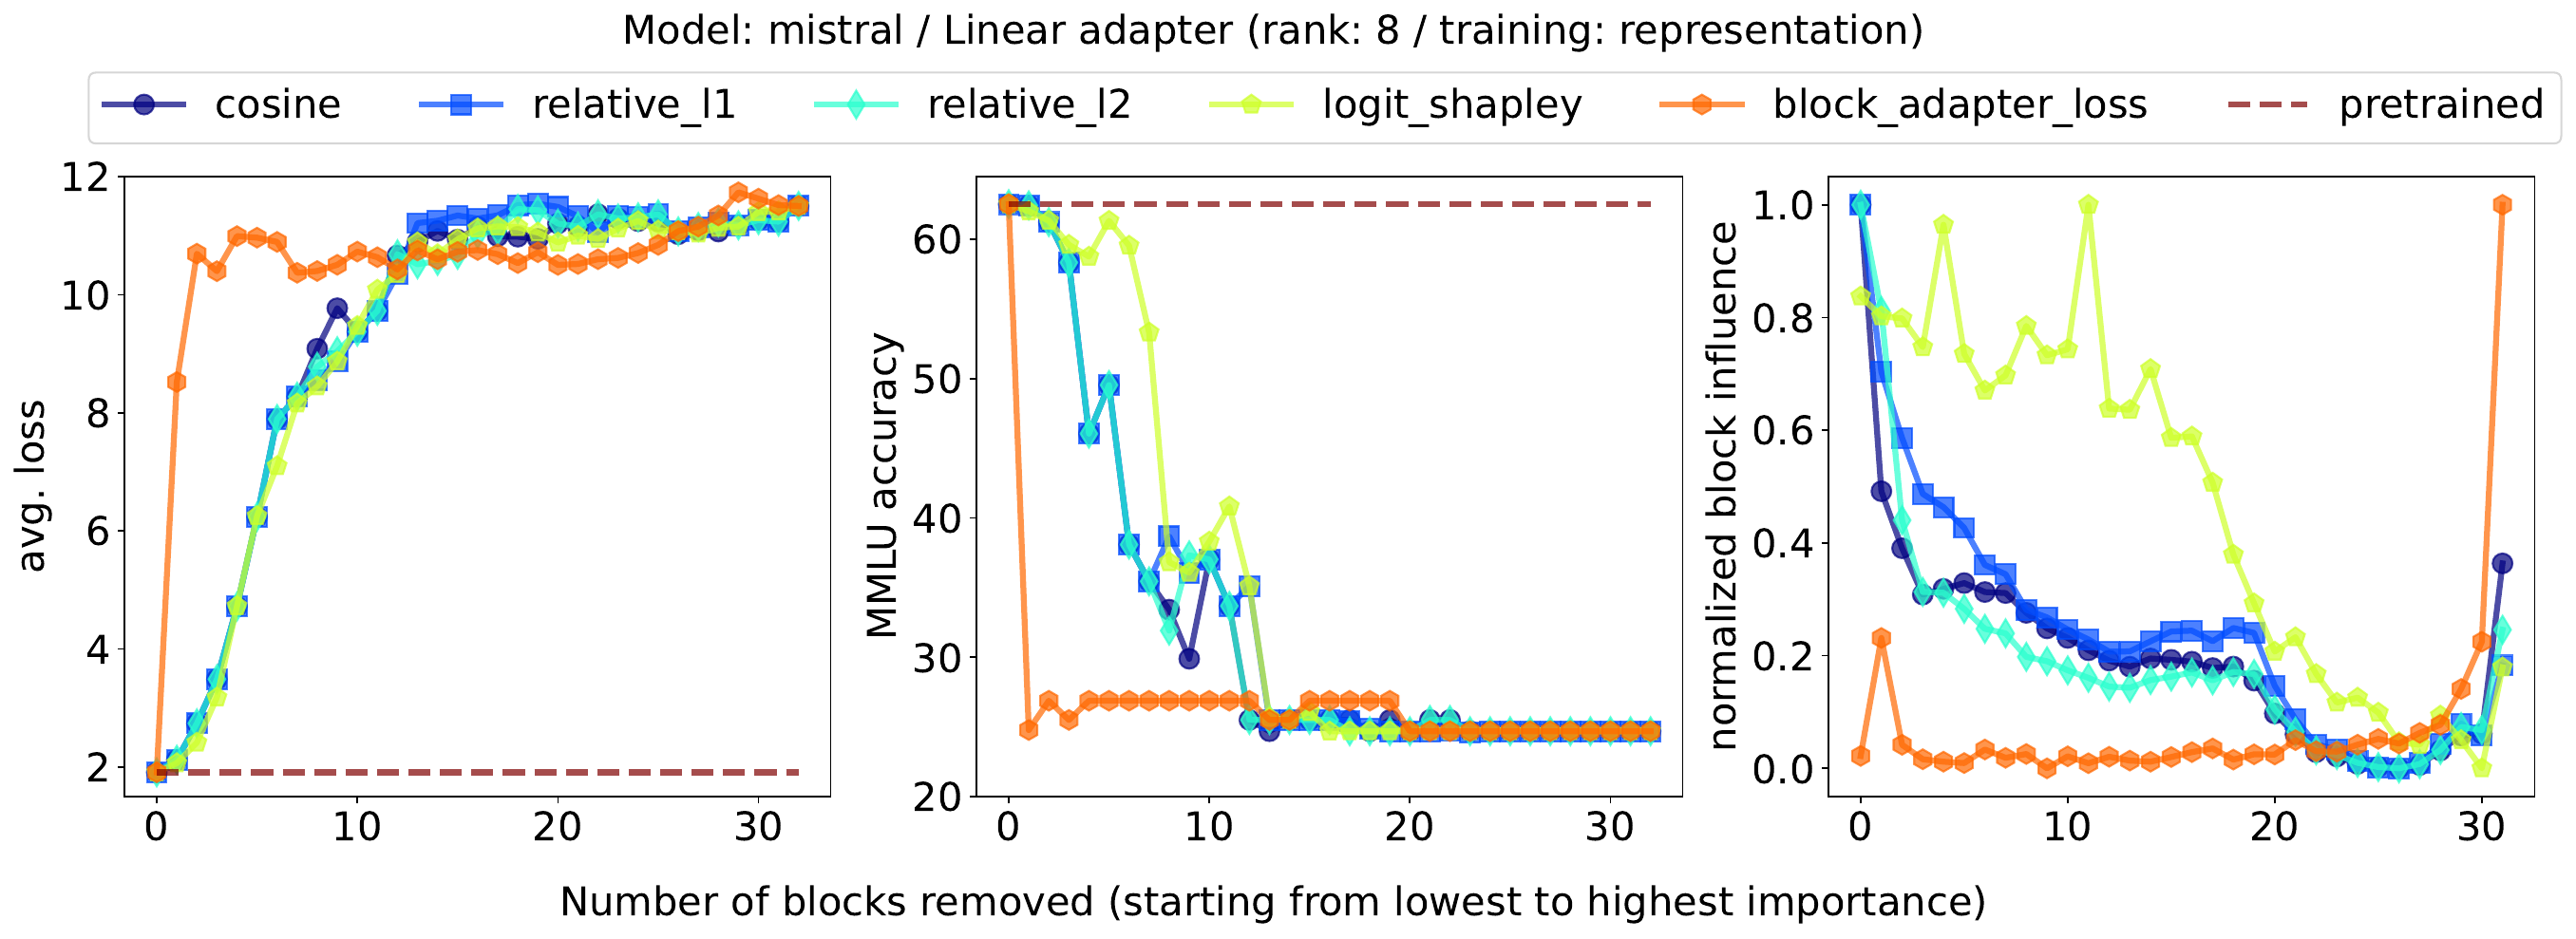}
    }

    \subfloat{
        \includegraphics[width=\textwidth]{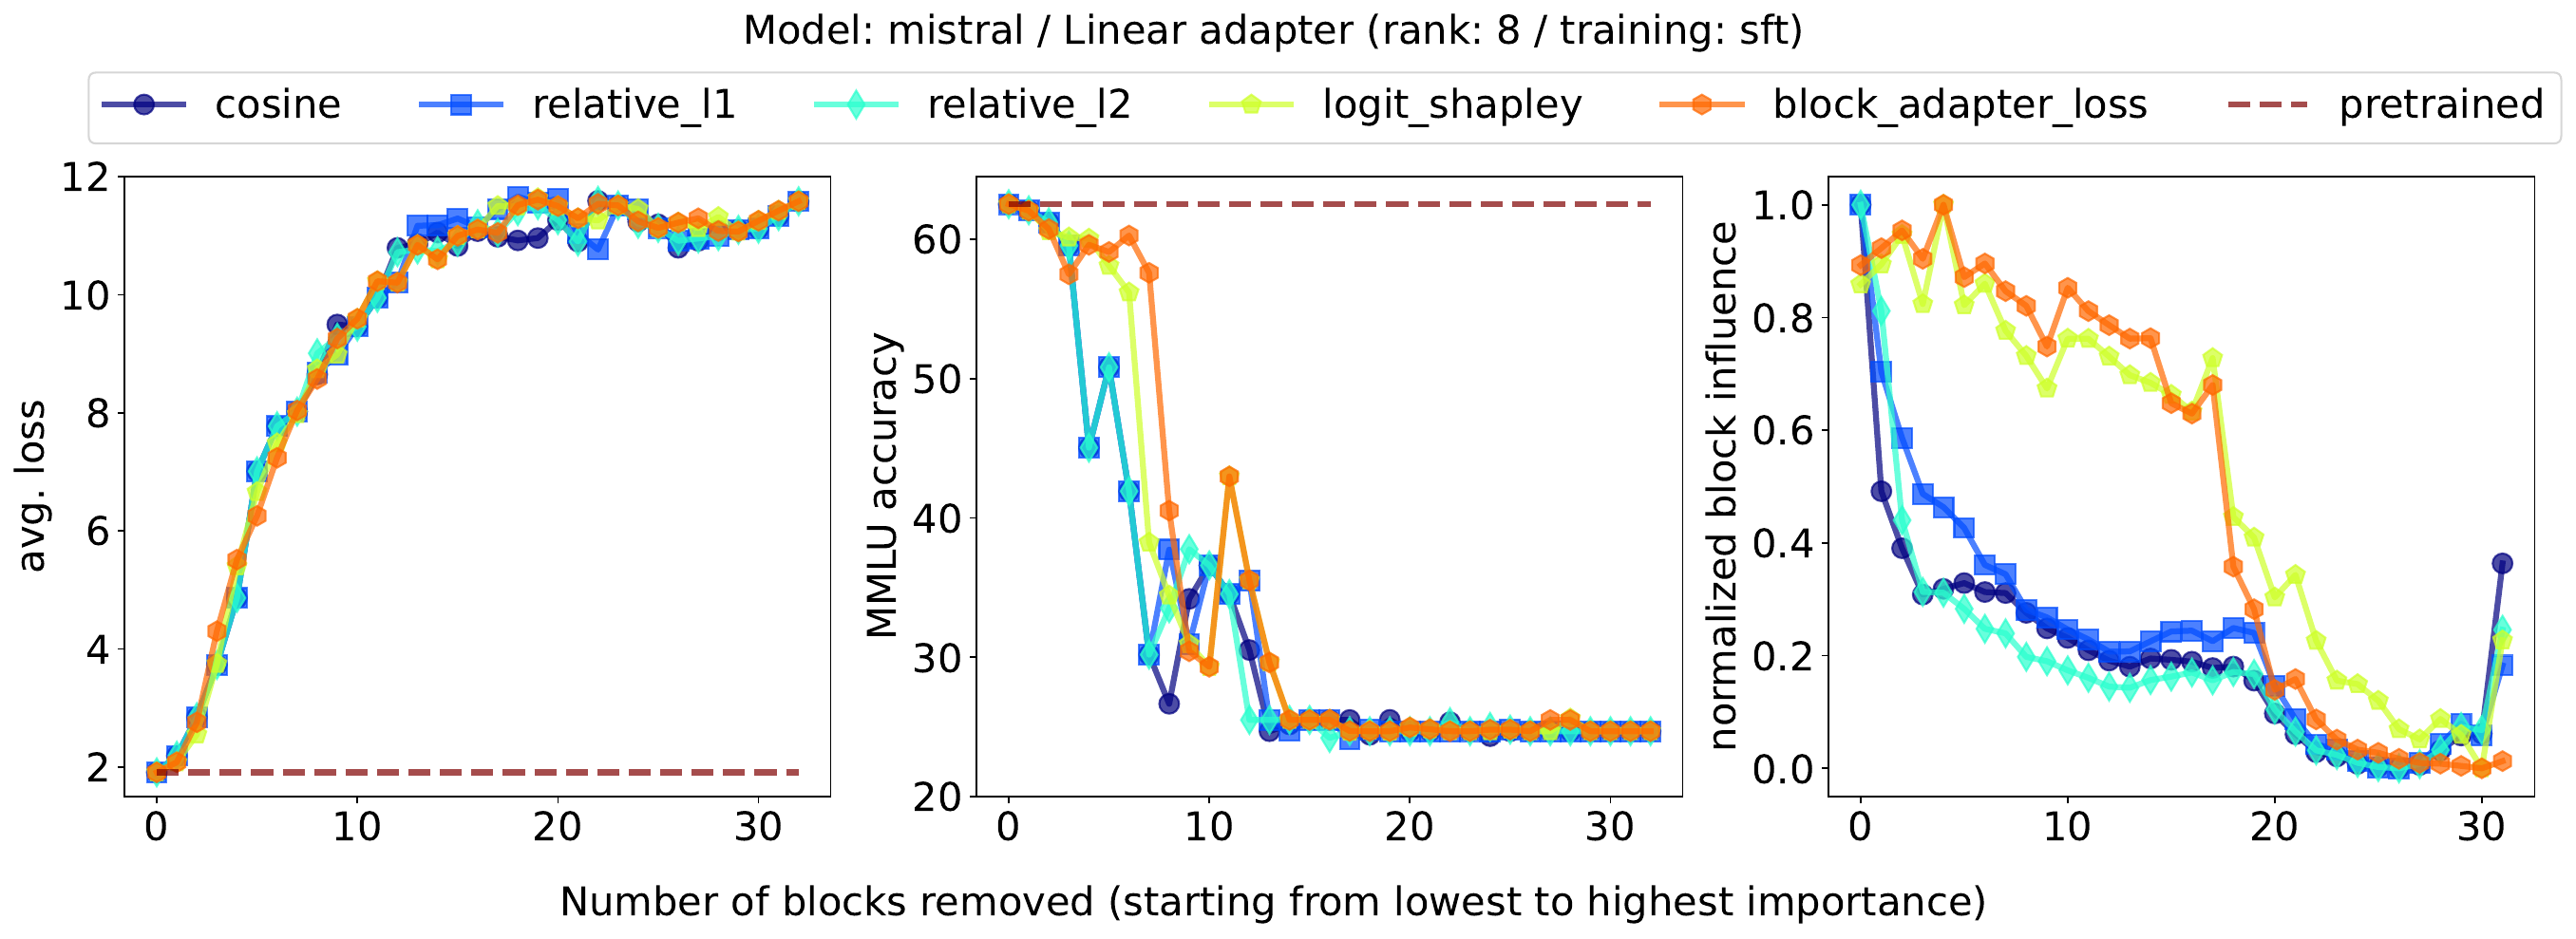}
    }

    \subfloat{
        \includegraphics[width=\textwidth]{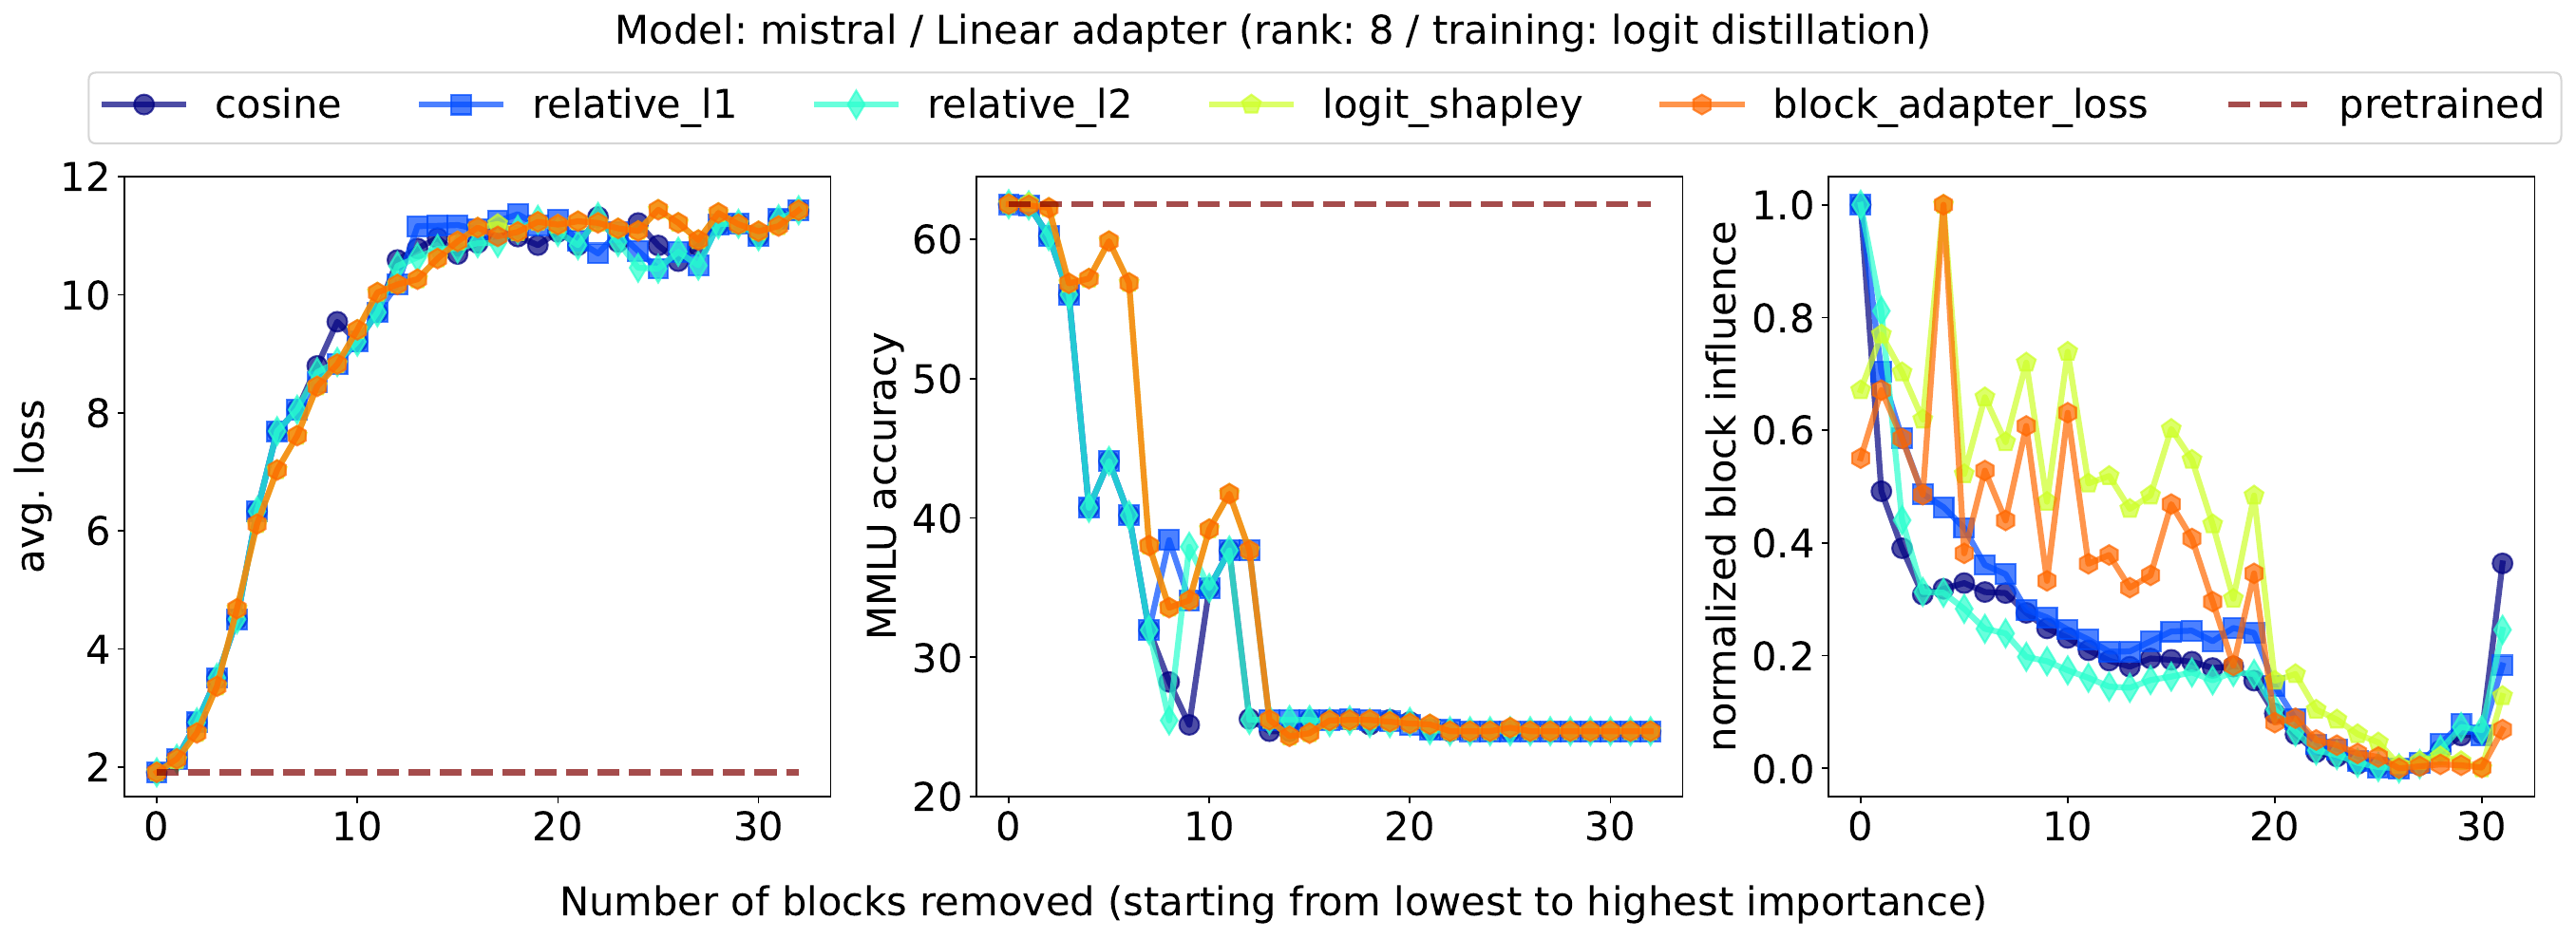}
    }
    \caption{\textbf{Evaluating the impact of linear adapters for Mistral 7b with a rank of 8} trained using three different metrics including (a) MSE loss defined on the representation, (b) supervised fine-tuning (SFT), and (c) logit distillation where logits are distilled from the full model.}
    \label{fig:linear_adapters_rank_8_mistral}
\end{figure}

Results for LLaMa-2 7b and Mistral 7b with an adapter rank of 8 on the original scale are visualized in 
Fig.~\ref{fig:linear_adapters_rank_8_llama2} and
Fig.~\ref{fig:linear_adapters_rank_8_mistral} respectively.

\begin{figure}
    \centering
    \subfloat{
        \includegraphics[width=\textwidth]{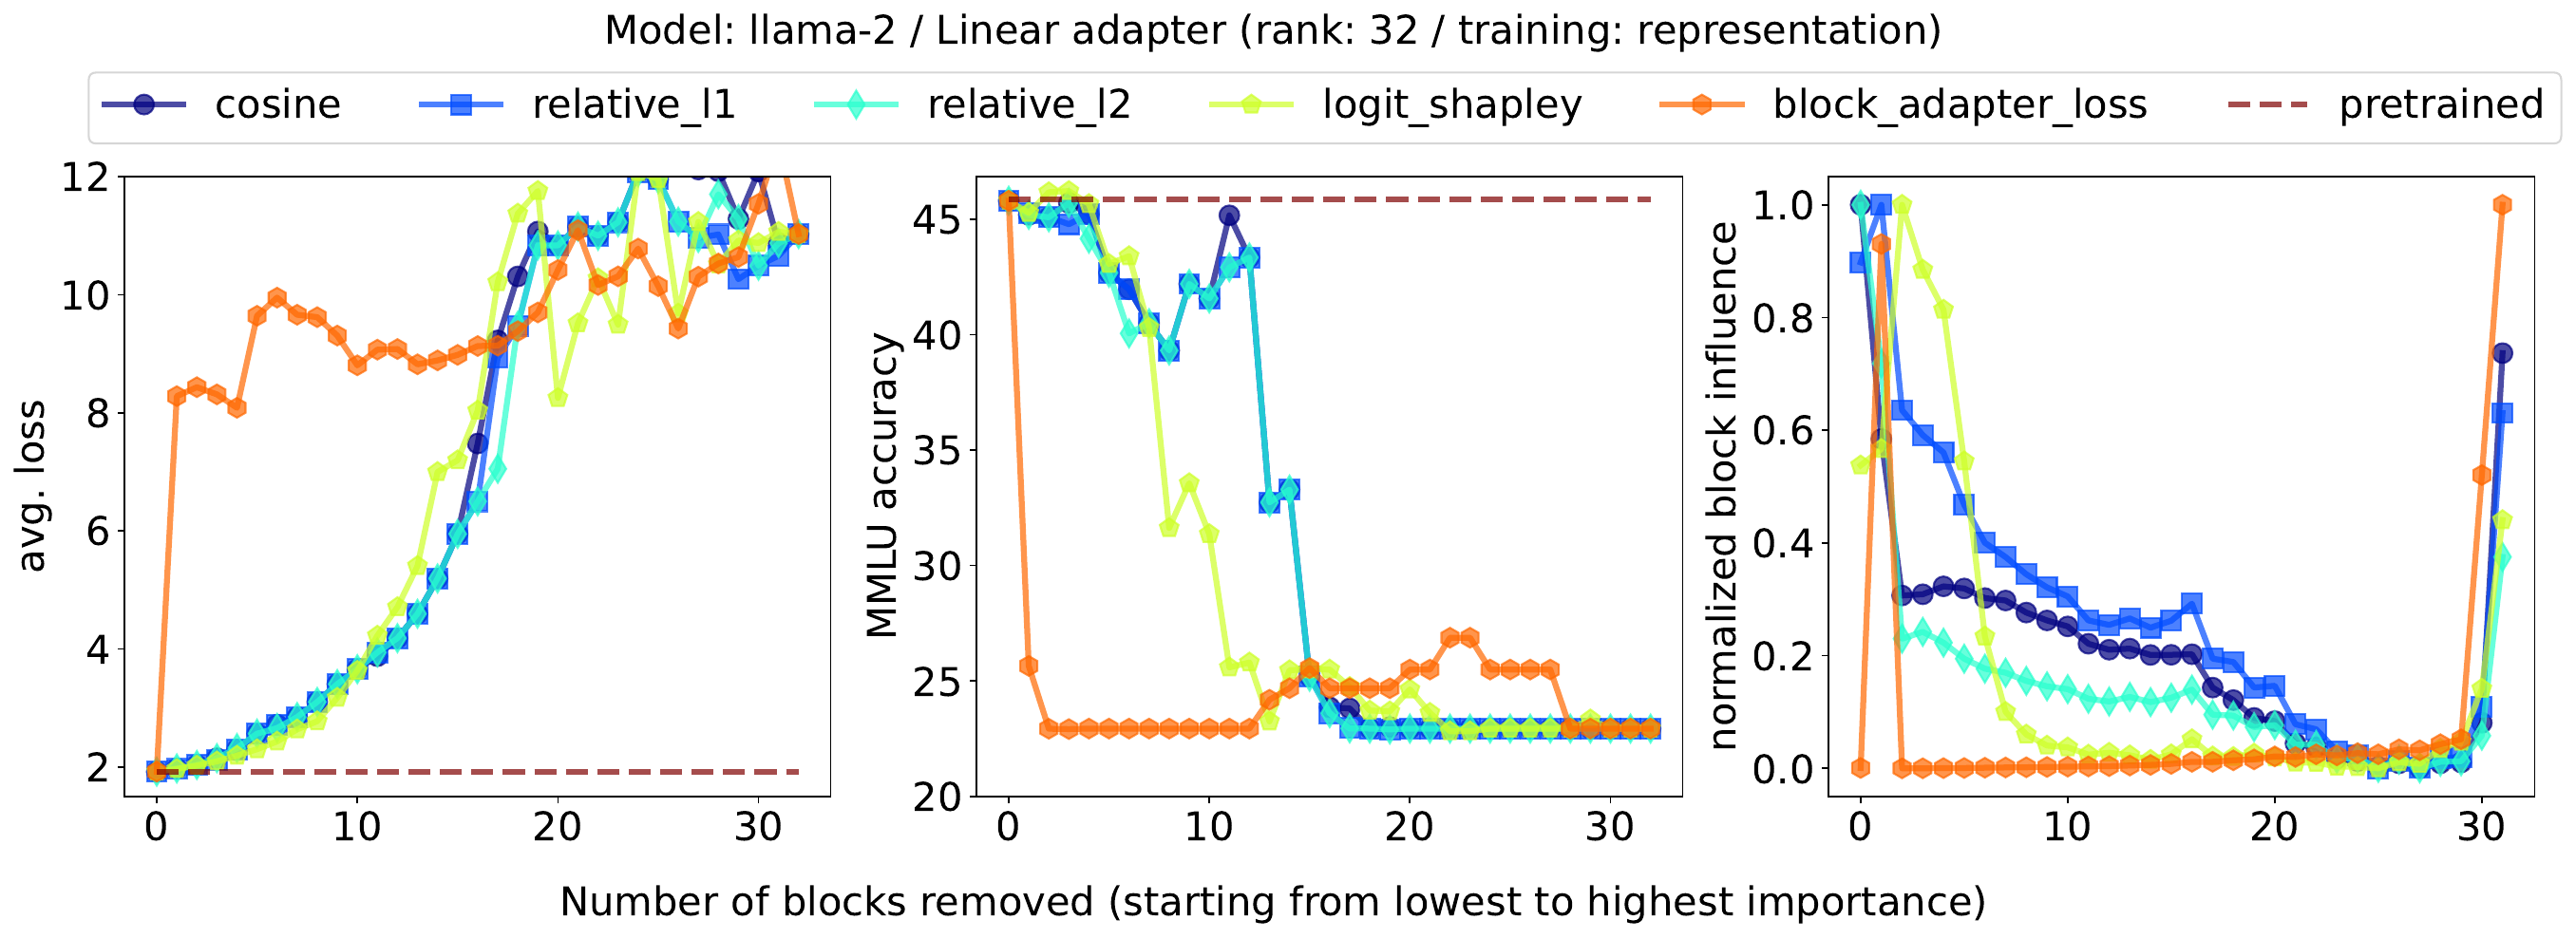}
    }

    \subfloat{
        \includegraphics[width=\textwidth]{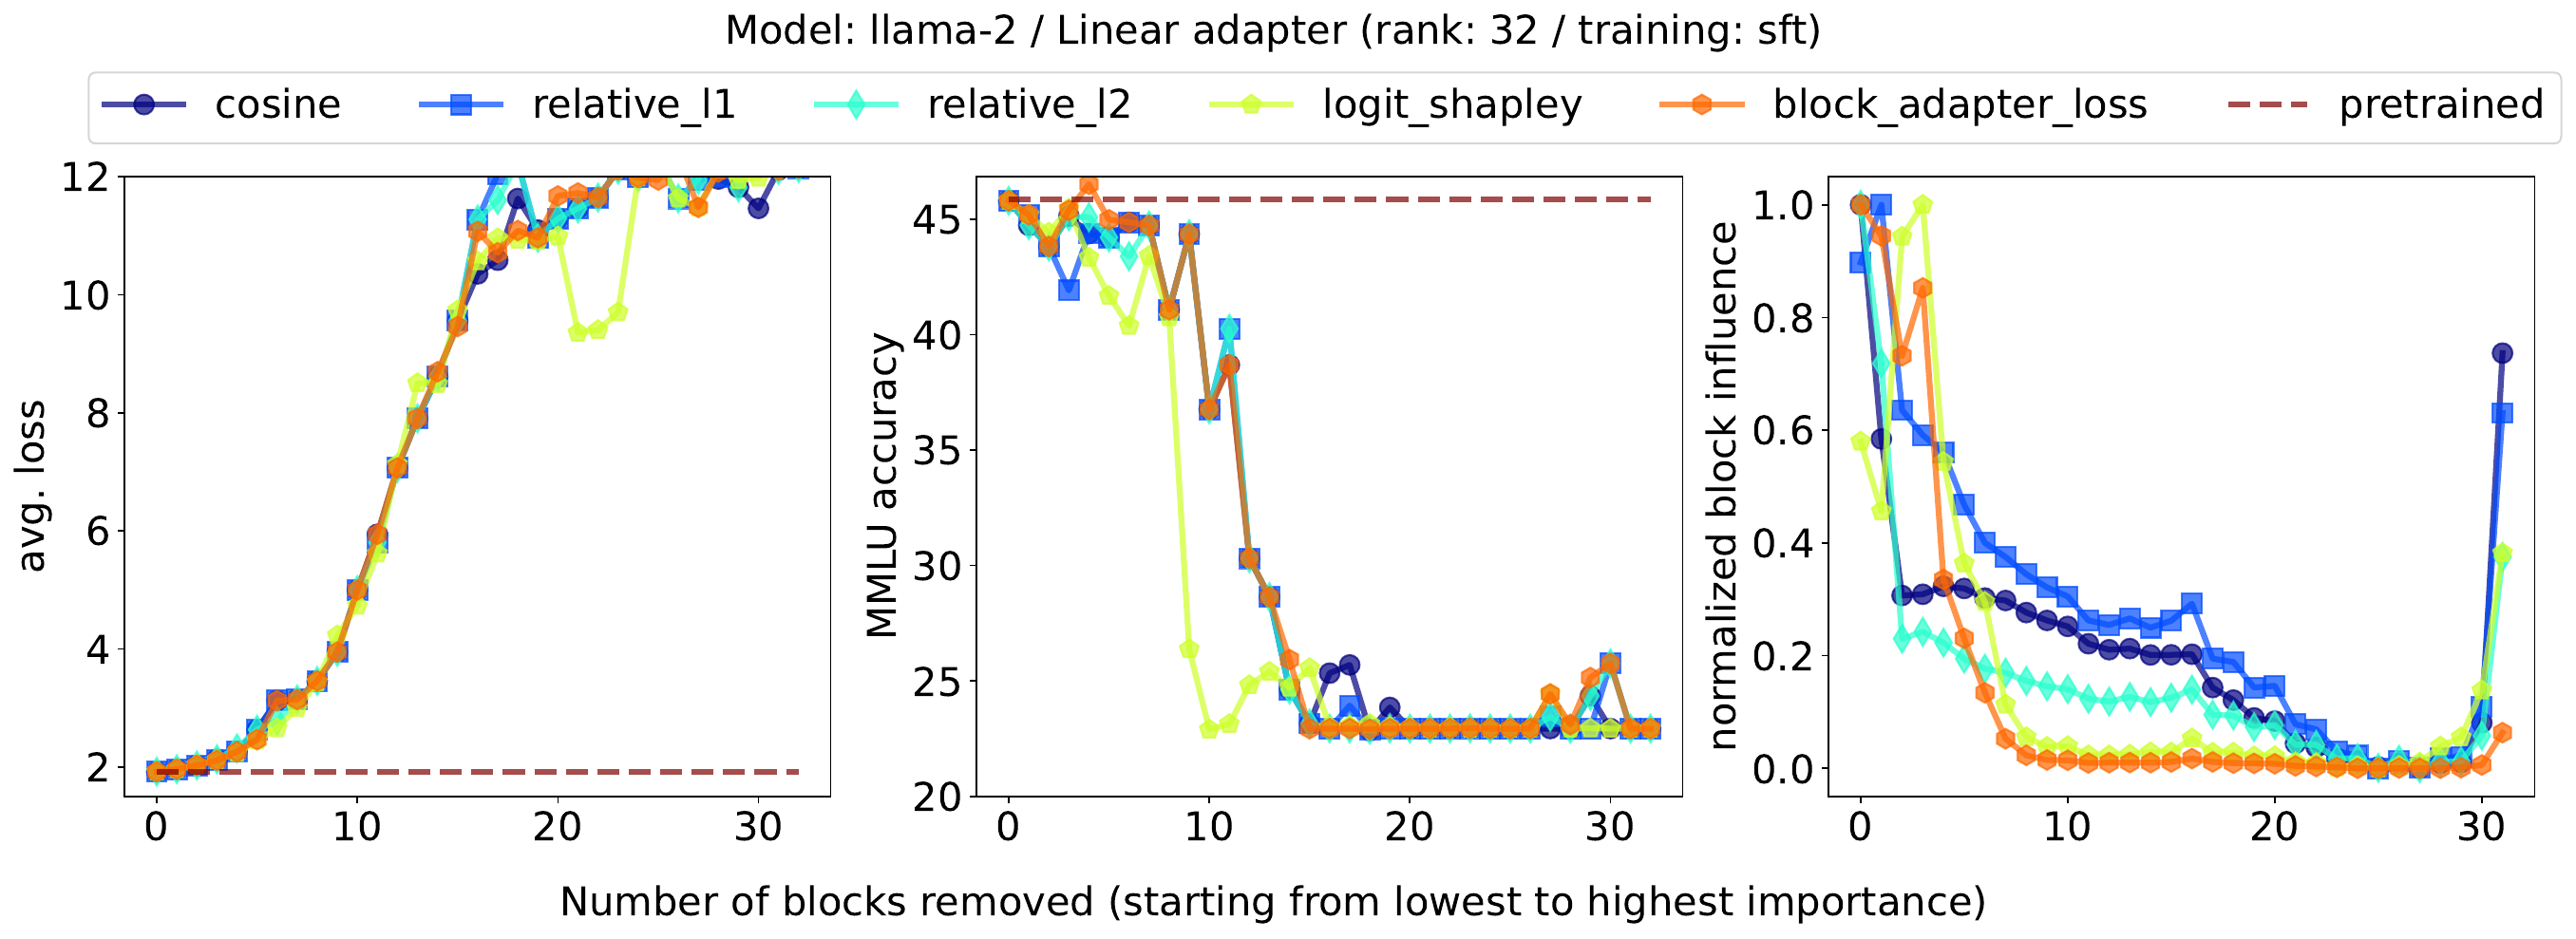}
    }

    \subfloat{
        \includegraphics[width=\textwidth]{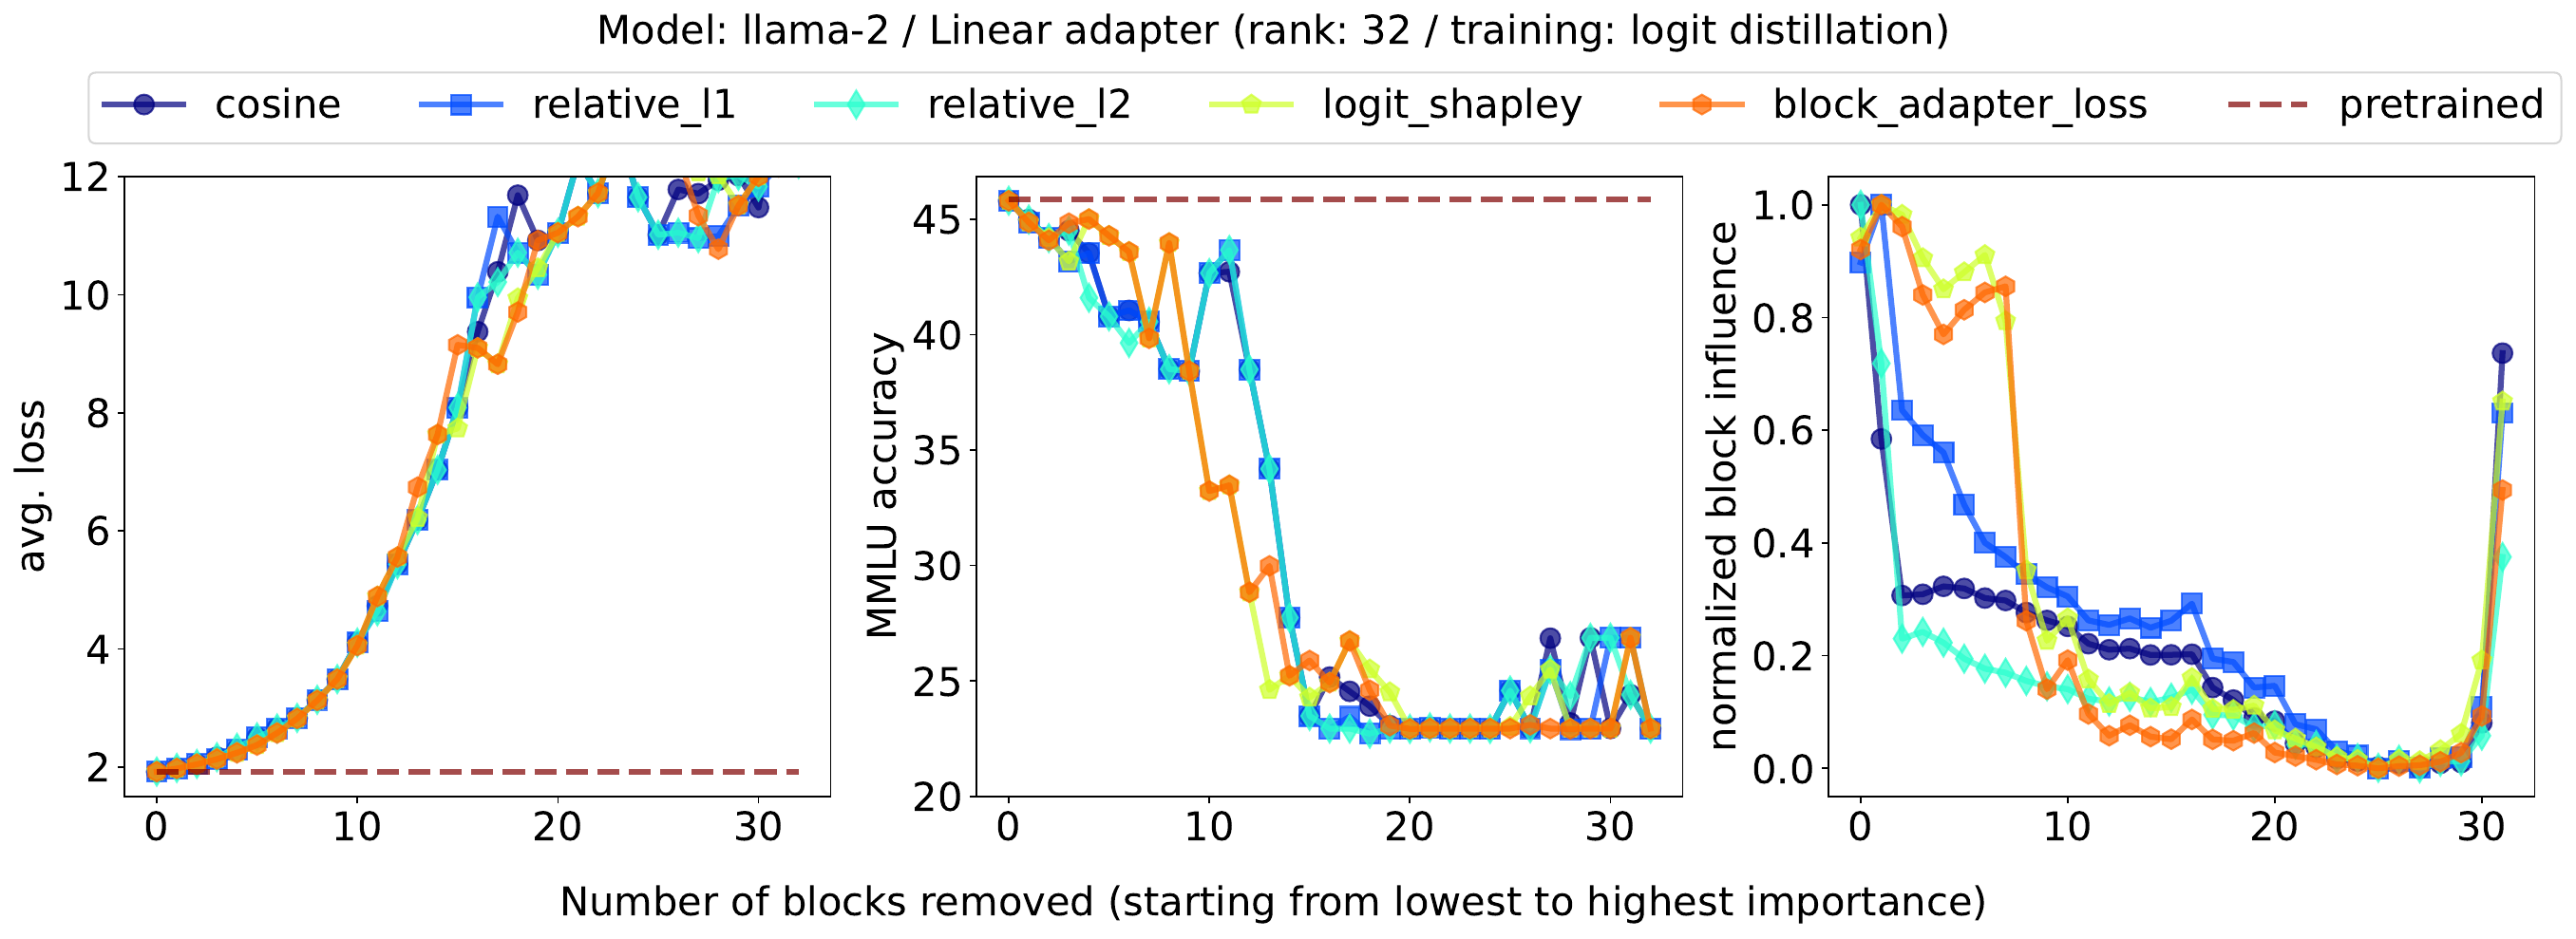}
    }
    \caption{\textbf{Evaluating the impact of linear adapters for LLaMa-2 7b with a rank of 32} trained using three different metrics including (a) MSE loss defined on the representation, (b) supervised fine-tuning (SFT), and (c) logit distillation where logits are distilled from the full model.}
    \label{fig:linear_adapters_rank_32_llama2}
\end{figure}

\begin{figure}
    \centering
    \subfloat{
        \includegraphics[width=\textwidth]{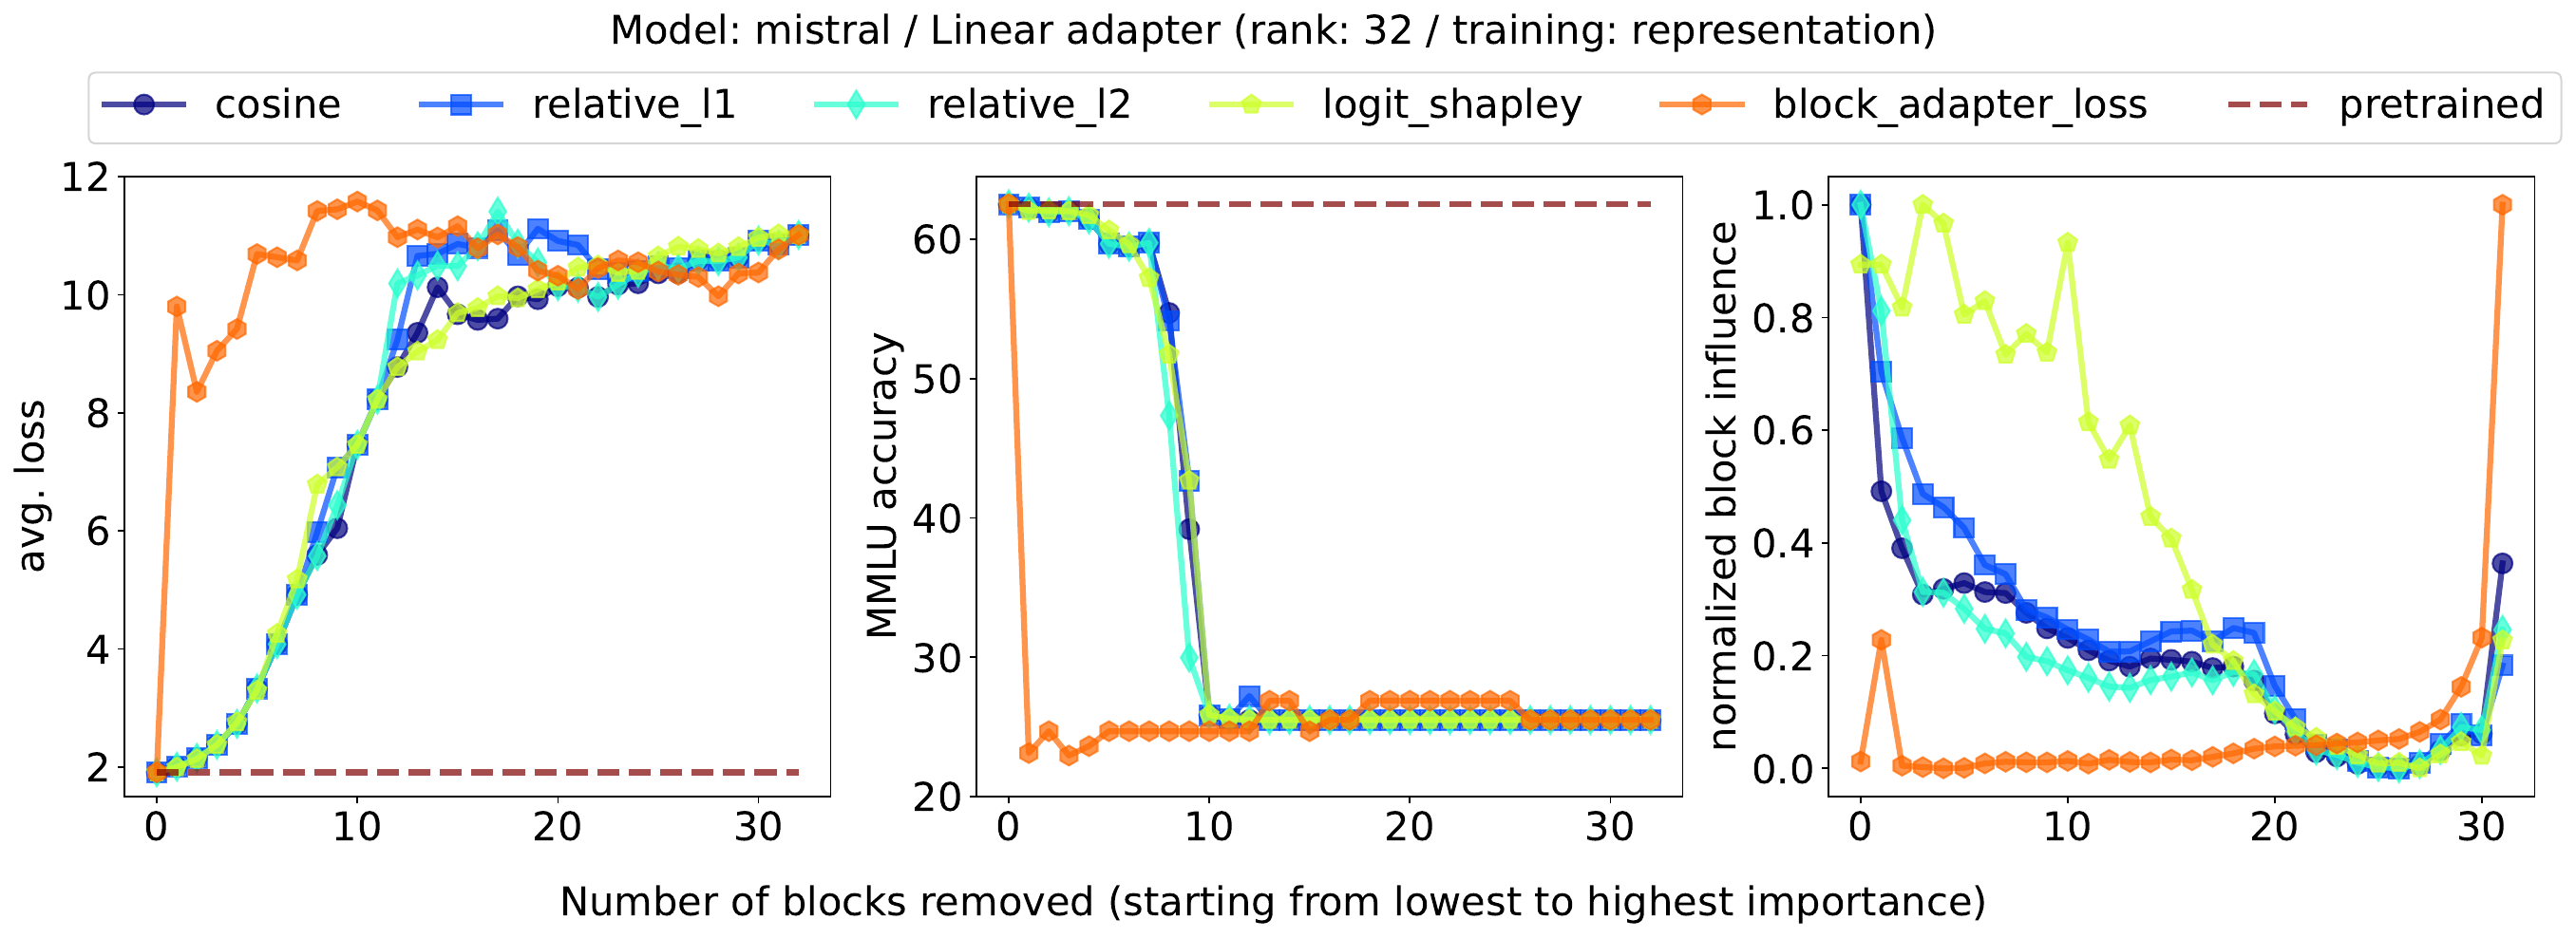}
    }

    \subfloat{
        \includegraphics[width=\textwidth]{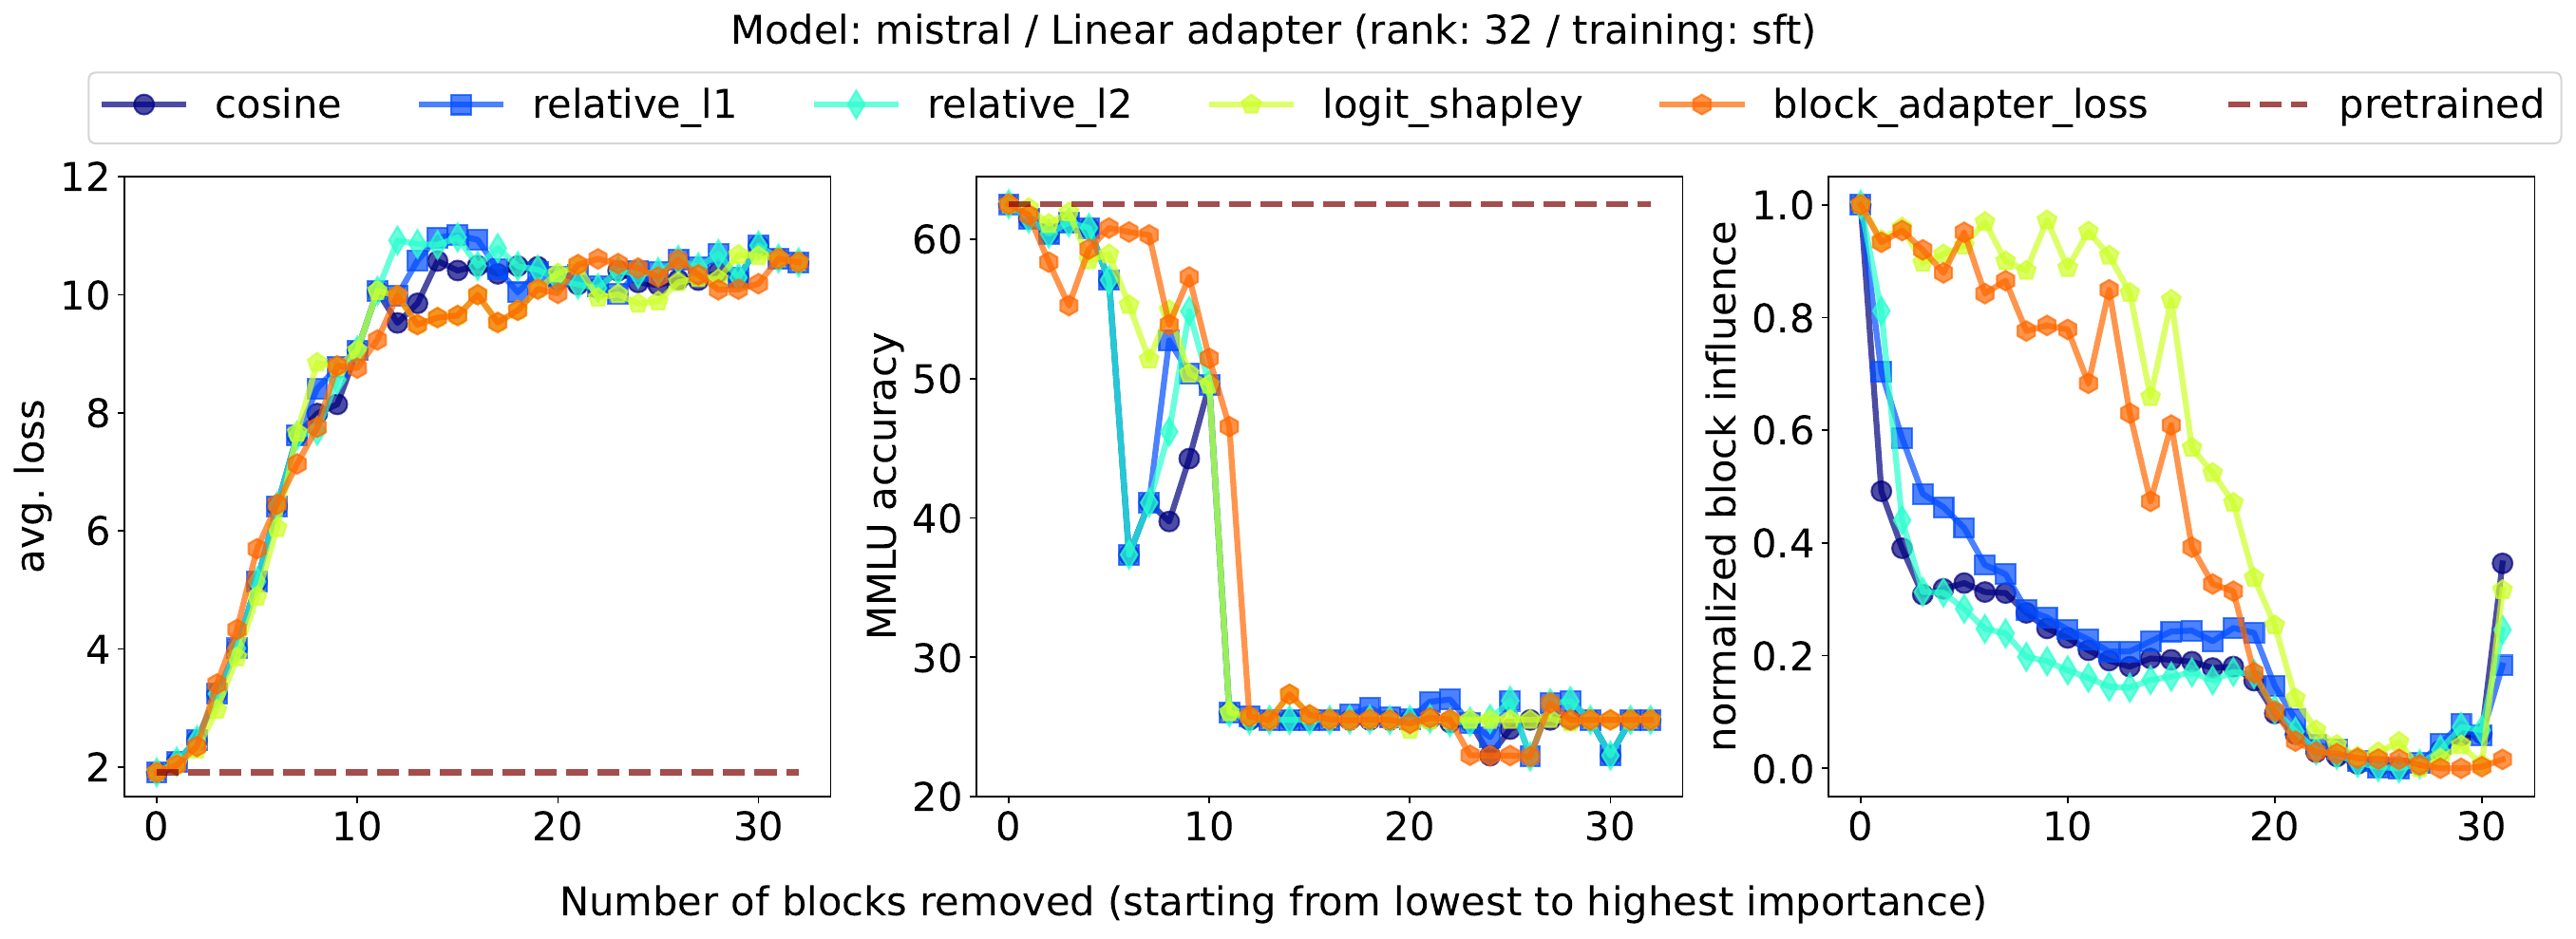}
    }

    \subfloat{
        \includegraphics[width=\textwidth]{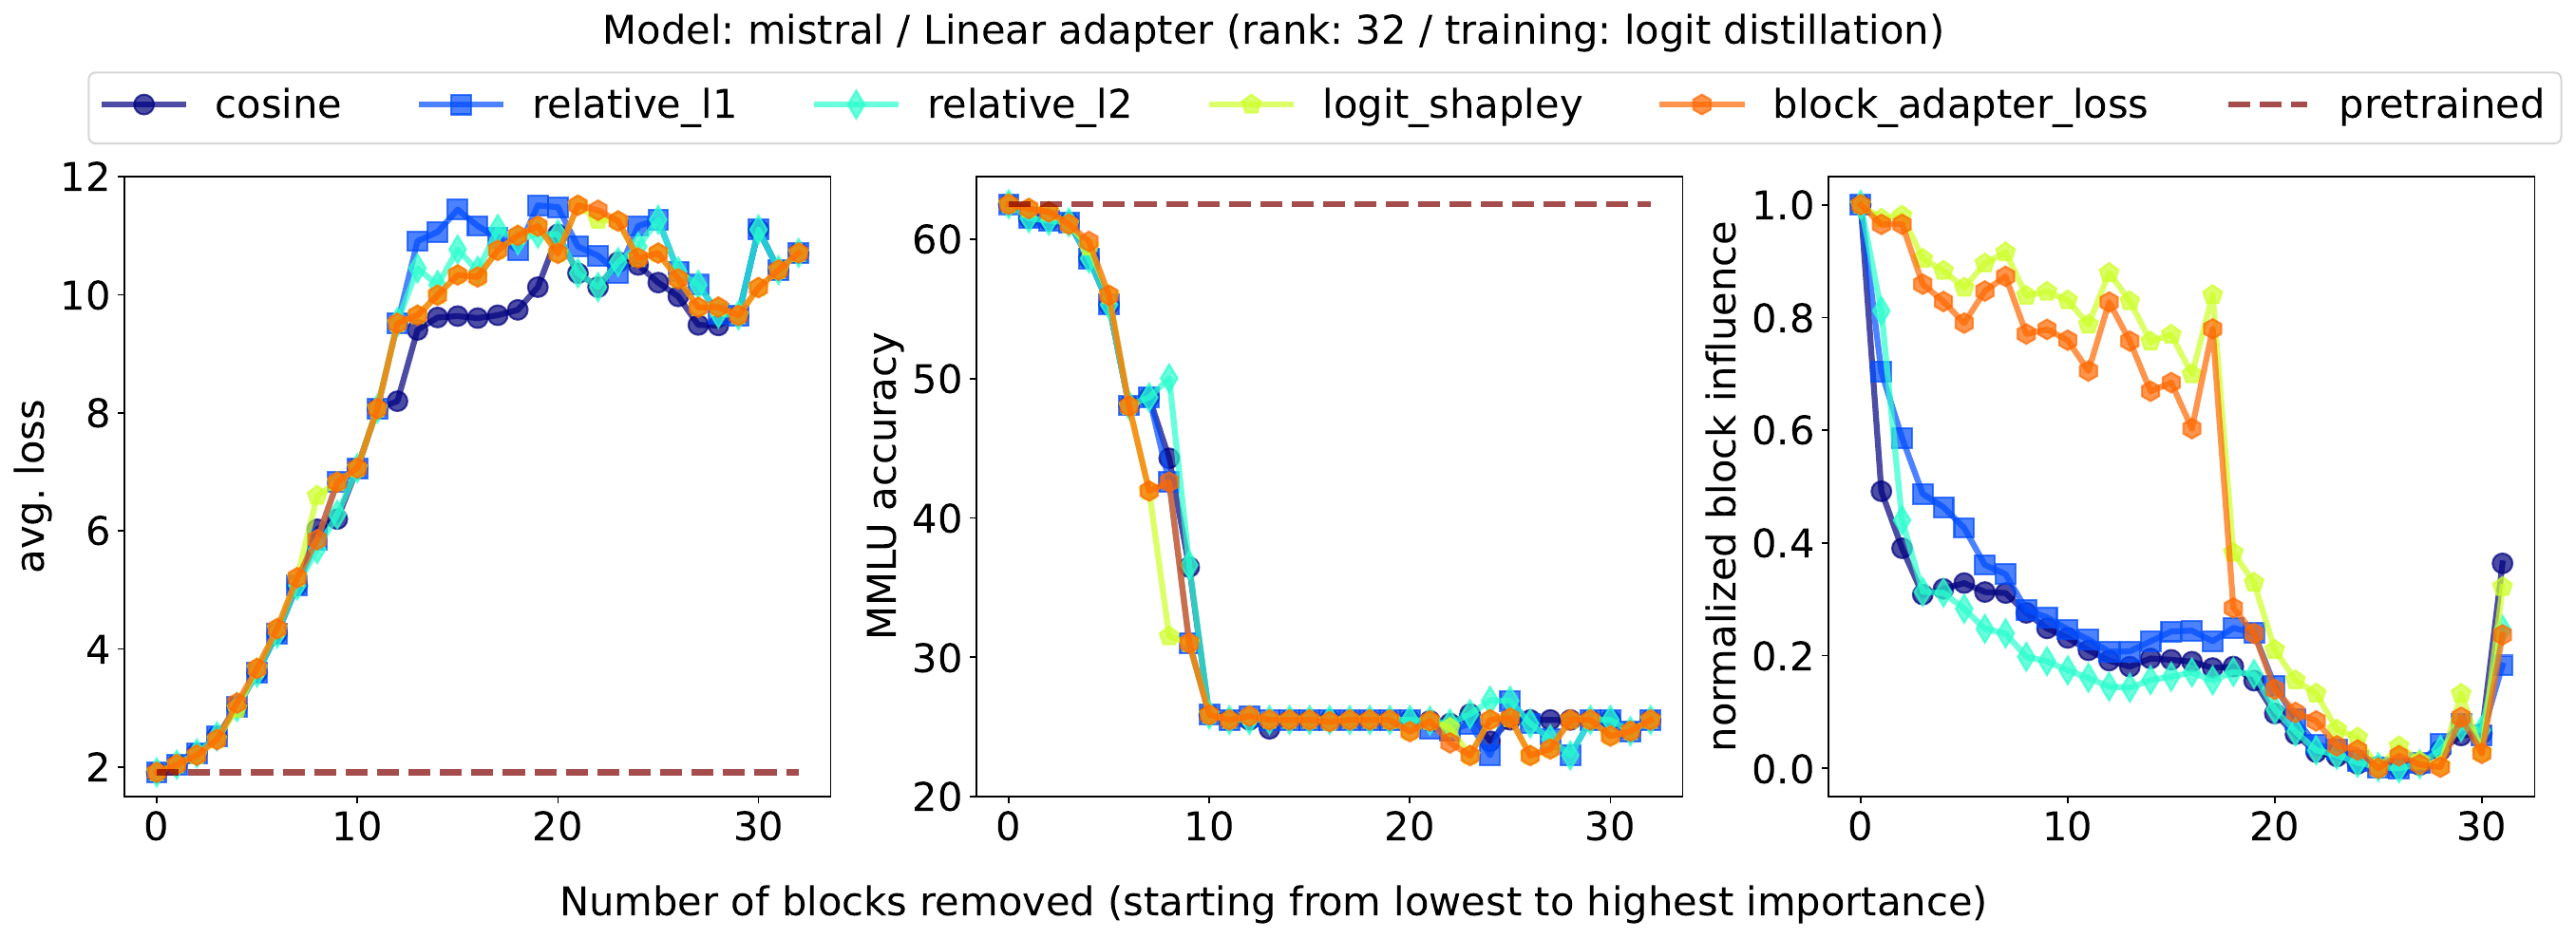}
    }
    \caption{\textbf{Evaluating the impact of linear adapters for Mistral 7b with a rank of 32} trained using three different metrics including (a) MSE loss defined on the representation, (b) supervised fine-tuning (SFT), and (c) logit distillation where logits are distilled from the full model.}
    \label{fig:linear_adapters_rank_32_mistral}
\end{figure}

Results for LLaMa-2 7b and Mistral 7b with an adapter rank of 32 on the original scale are visualized in Fig.~\ref{fig:linear_adapters_rank_32_llama2} and Fig.~\ref{fig:linear_adapters_rank_32_mistral} respectively.

\begin{figure}
    \centering
    \subfloat{
        \includegraphics[width=\textwidth]{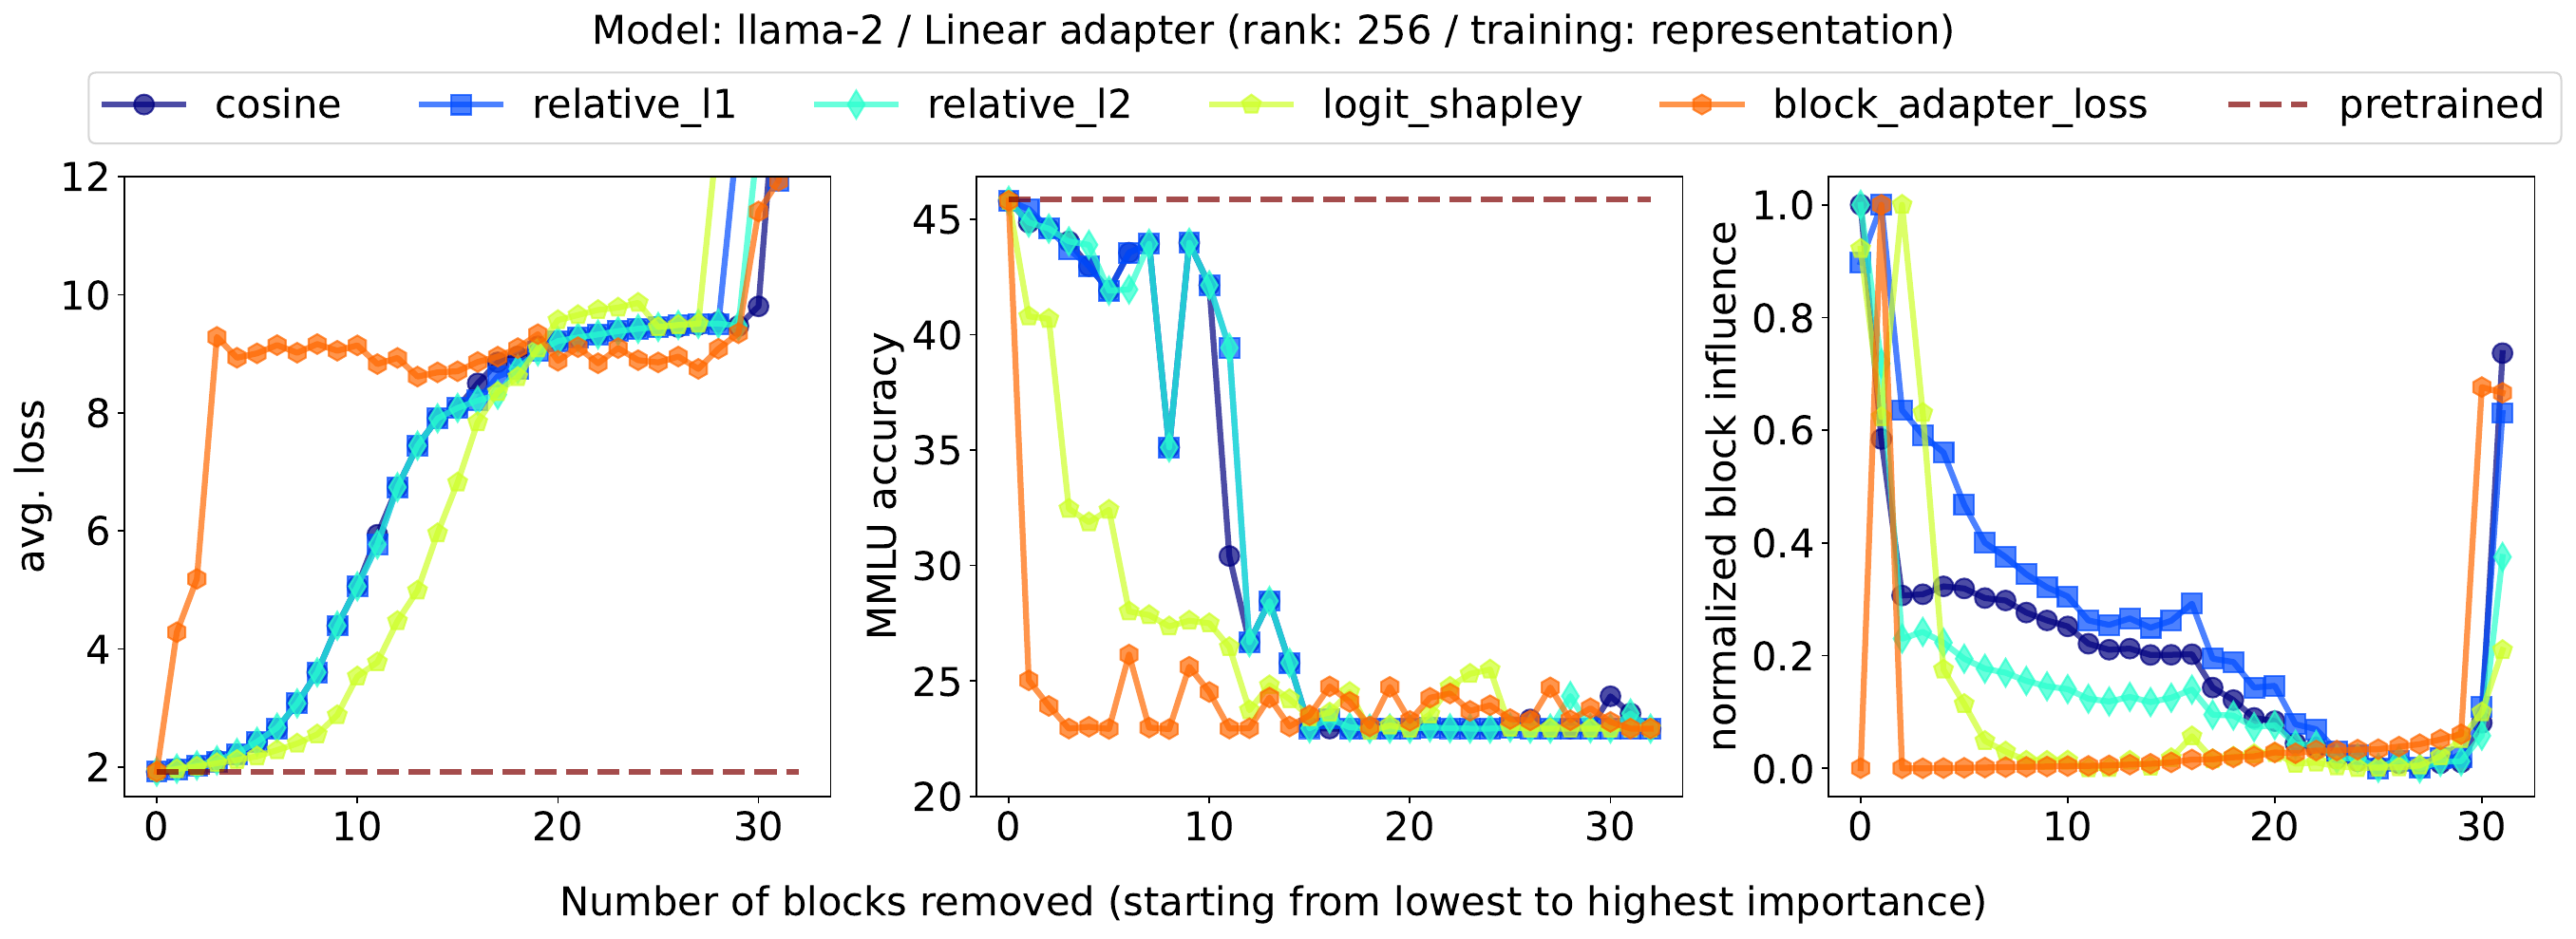}
    }

    \subfloat{
        \includegraphics[width=\textwidth]{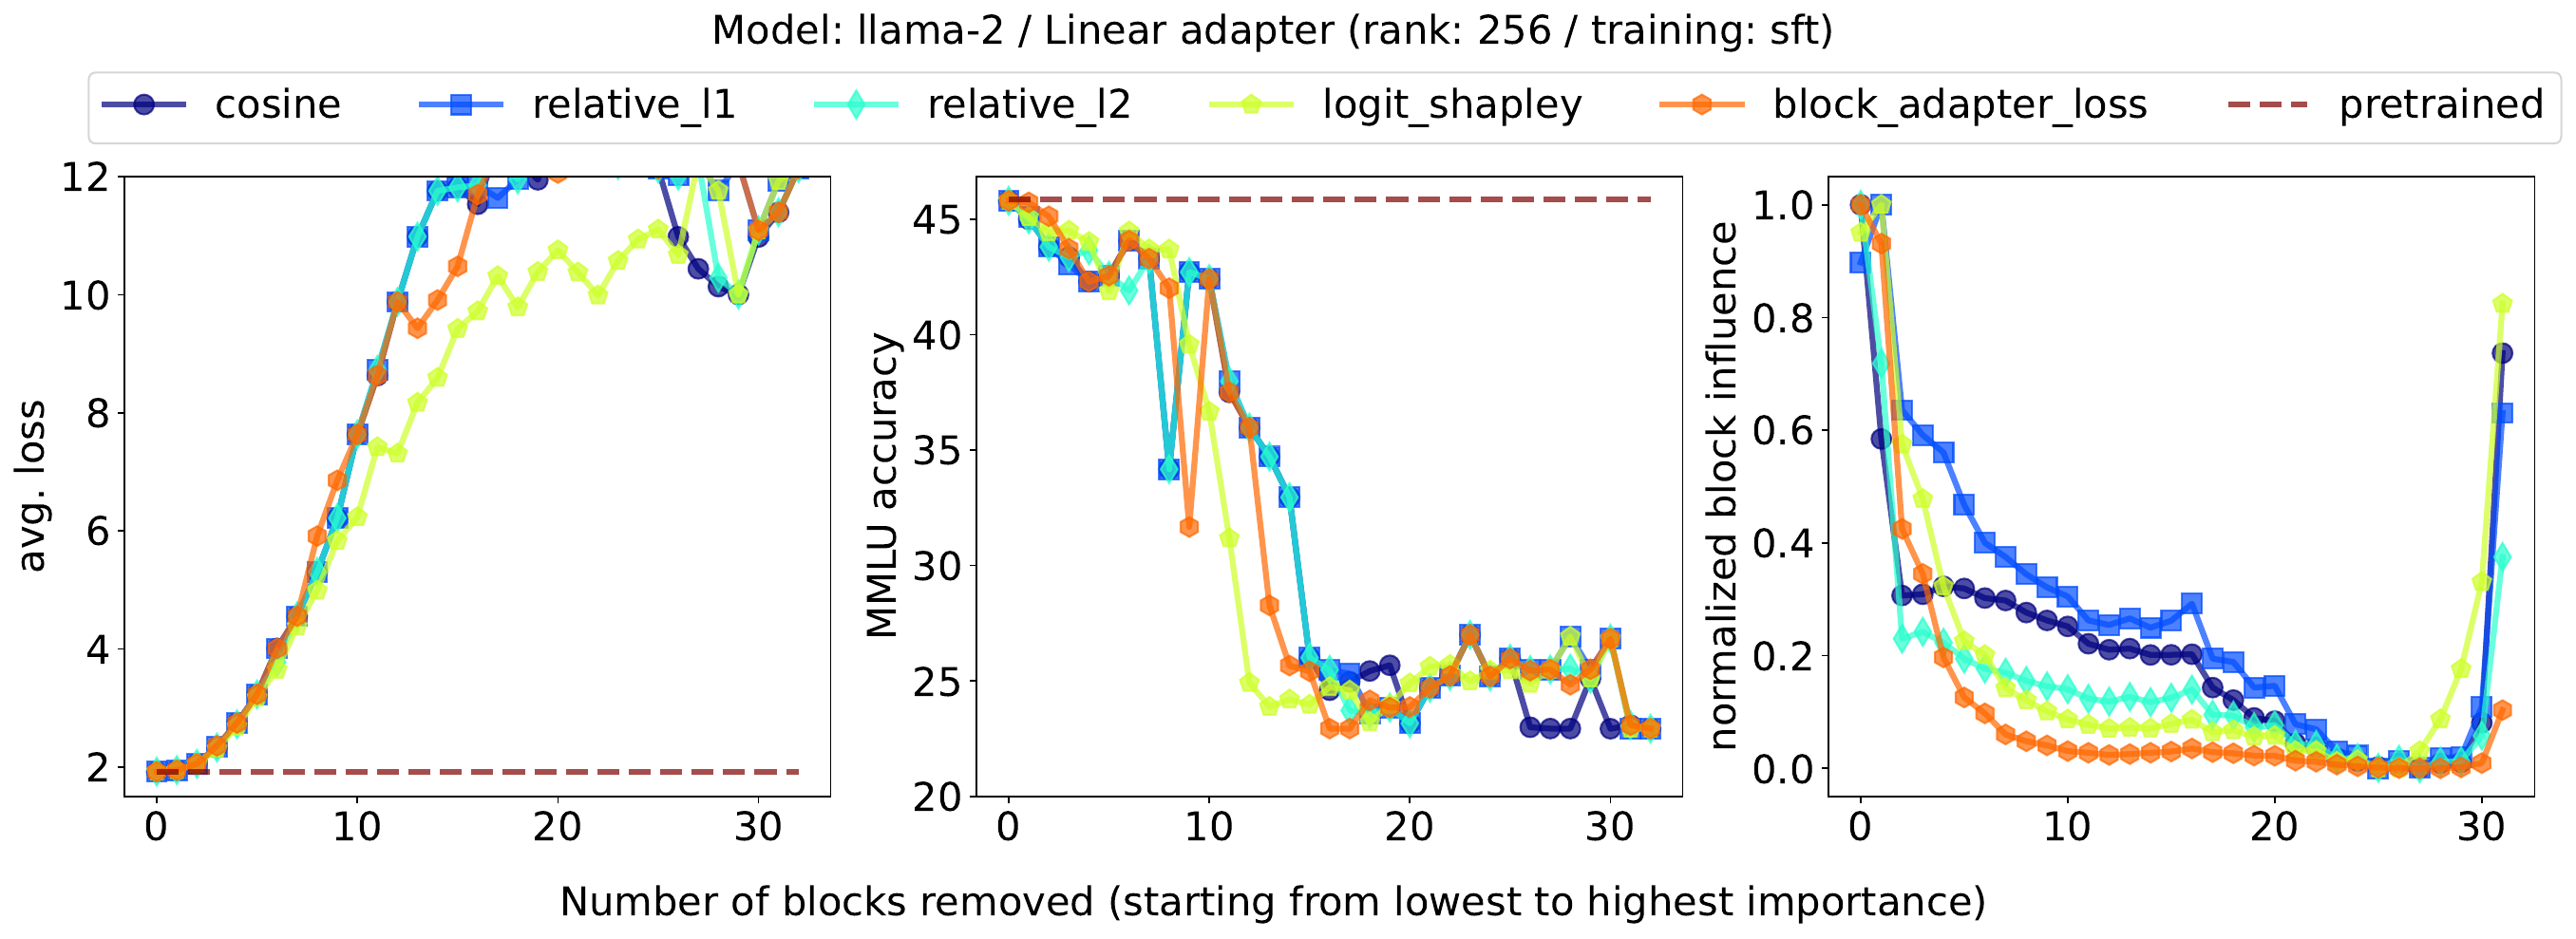}
    }

    \subfloat{
        \includegraphics[width=\textwidth]{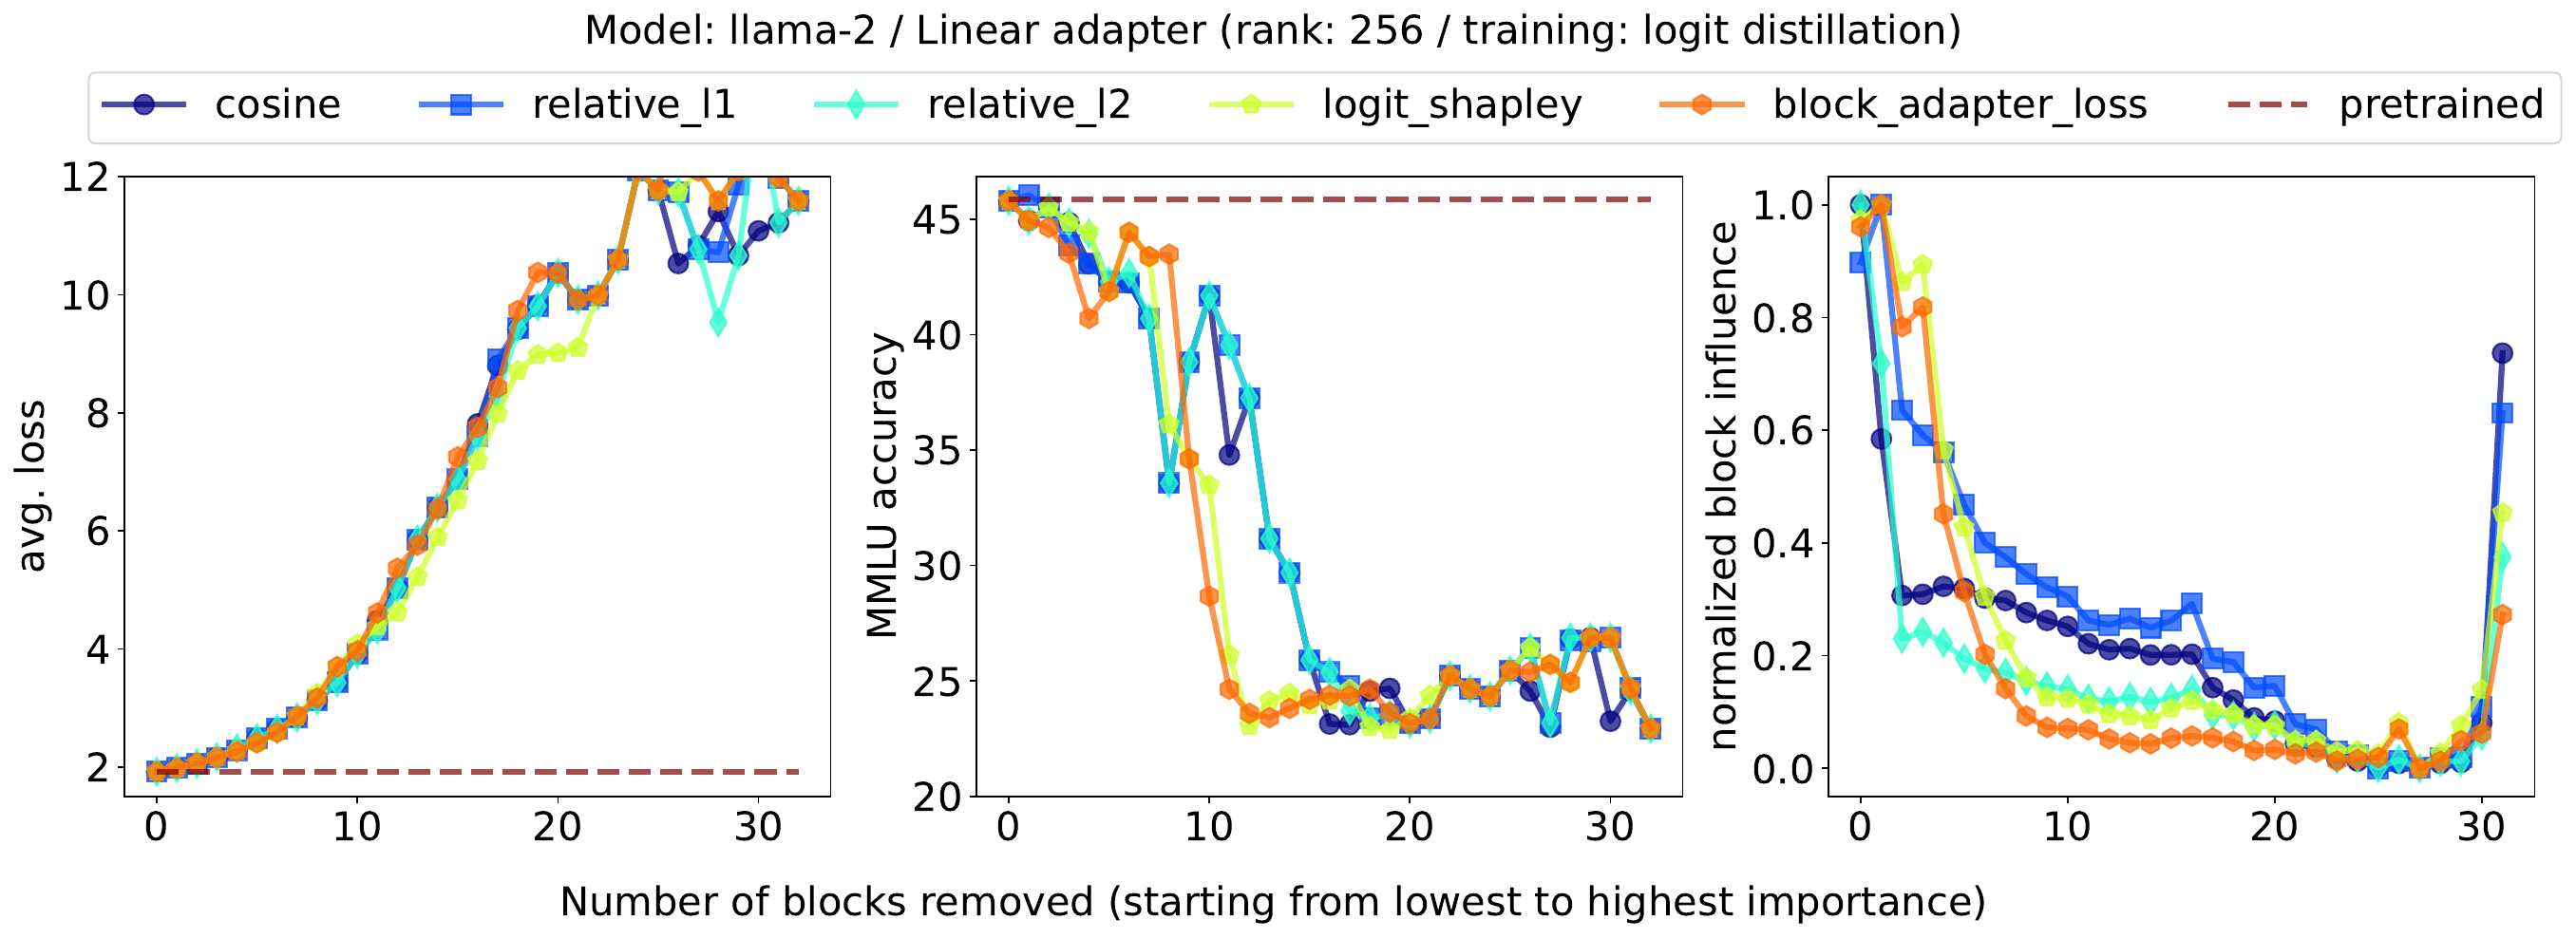}
    }
    \caption{\textbf{Evaluating the impact of linear adapters for LLaMa-2 7b with a rank of 256} trained using three different metrics including (a) MSE loss defined on the representation, (b) supervised fine-tuning (SFT), and (c) logit distillation where logits are distilled from the full model.}
    \label{fig:linear_adapters_rank_256_llama2}
\end{figure}

\begin{figure}
    \centering
    \subfloat{
        \includegraphics[width=\textwidth]{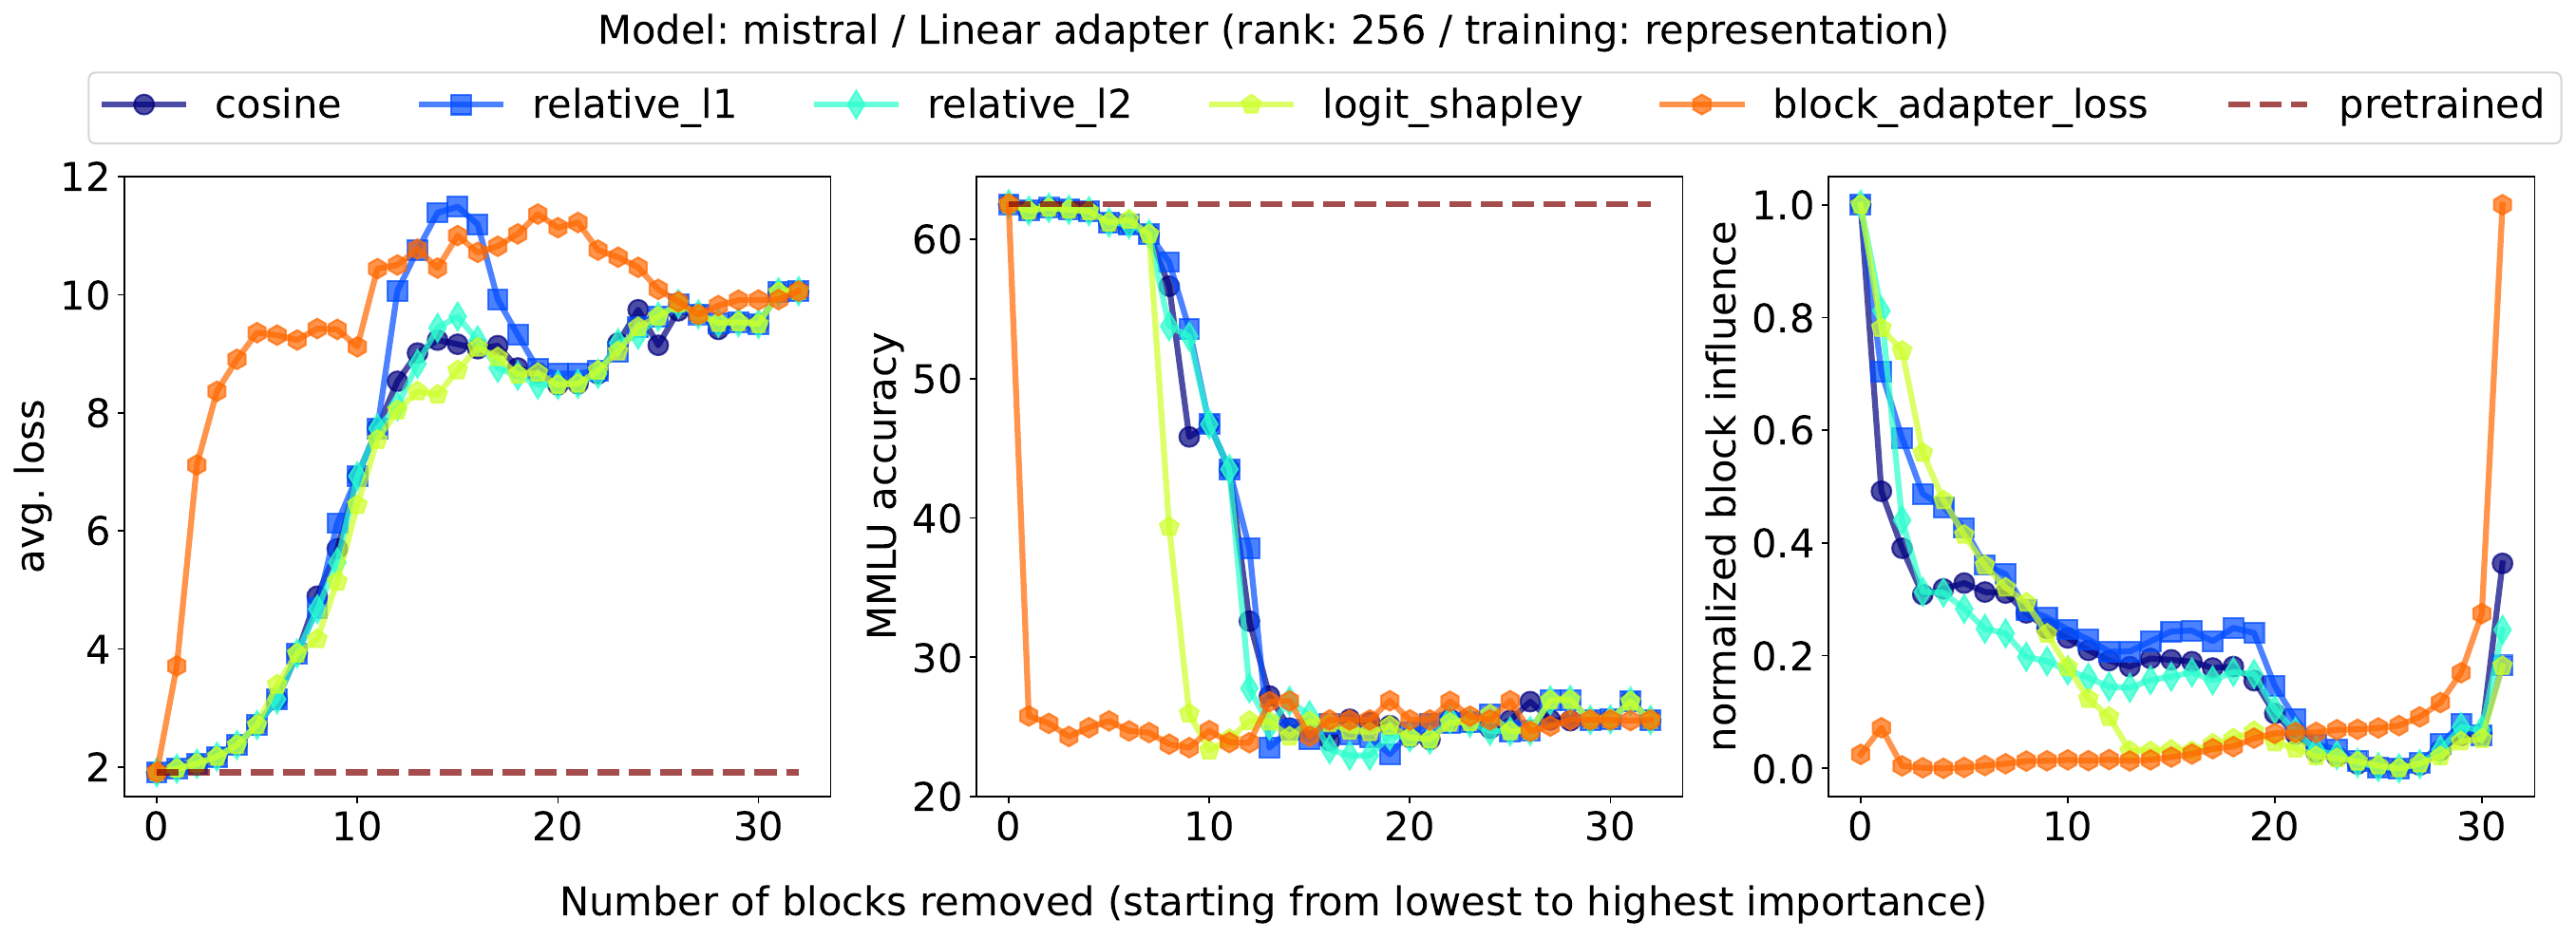}
    }

    \subfloat{
        \includegraphics[width=\textwidth]{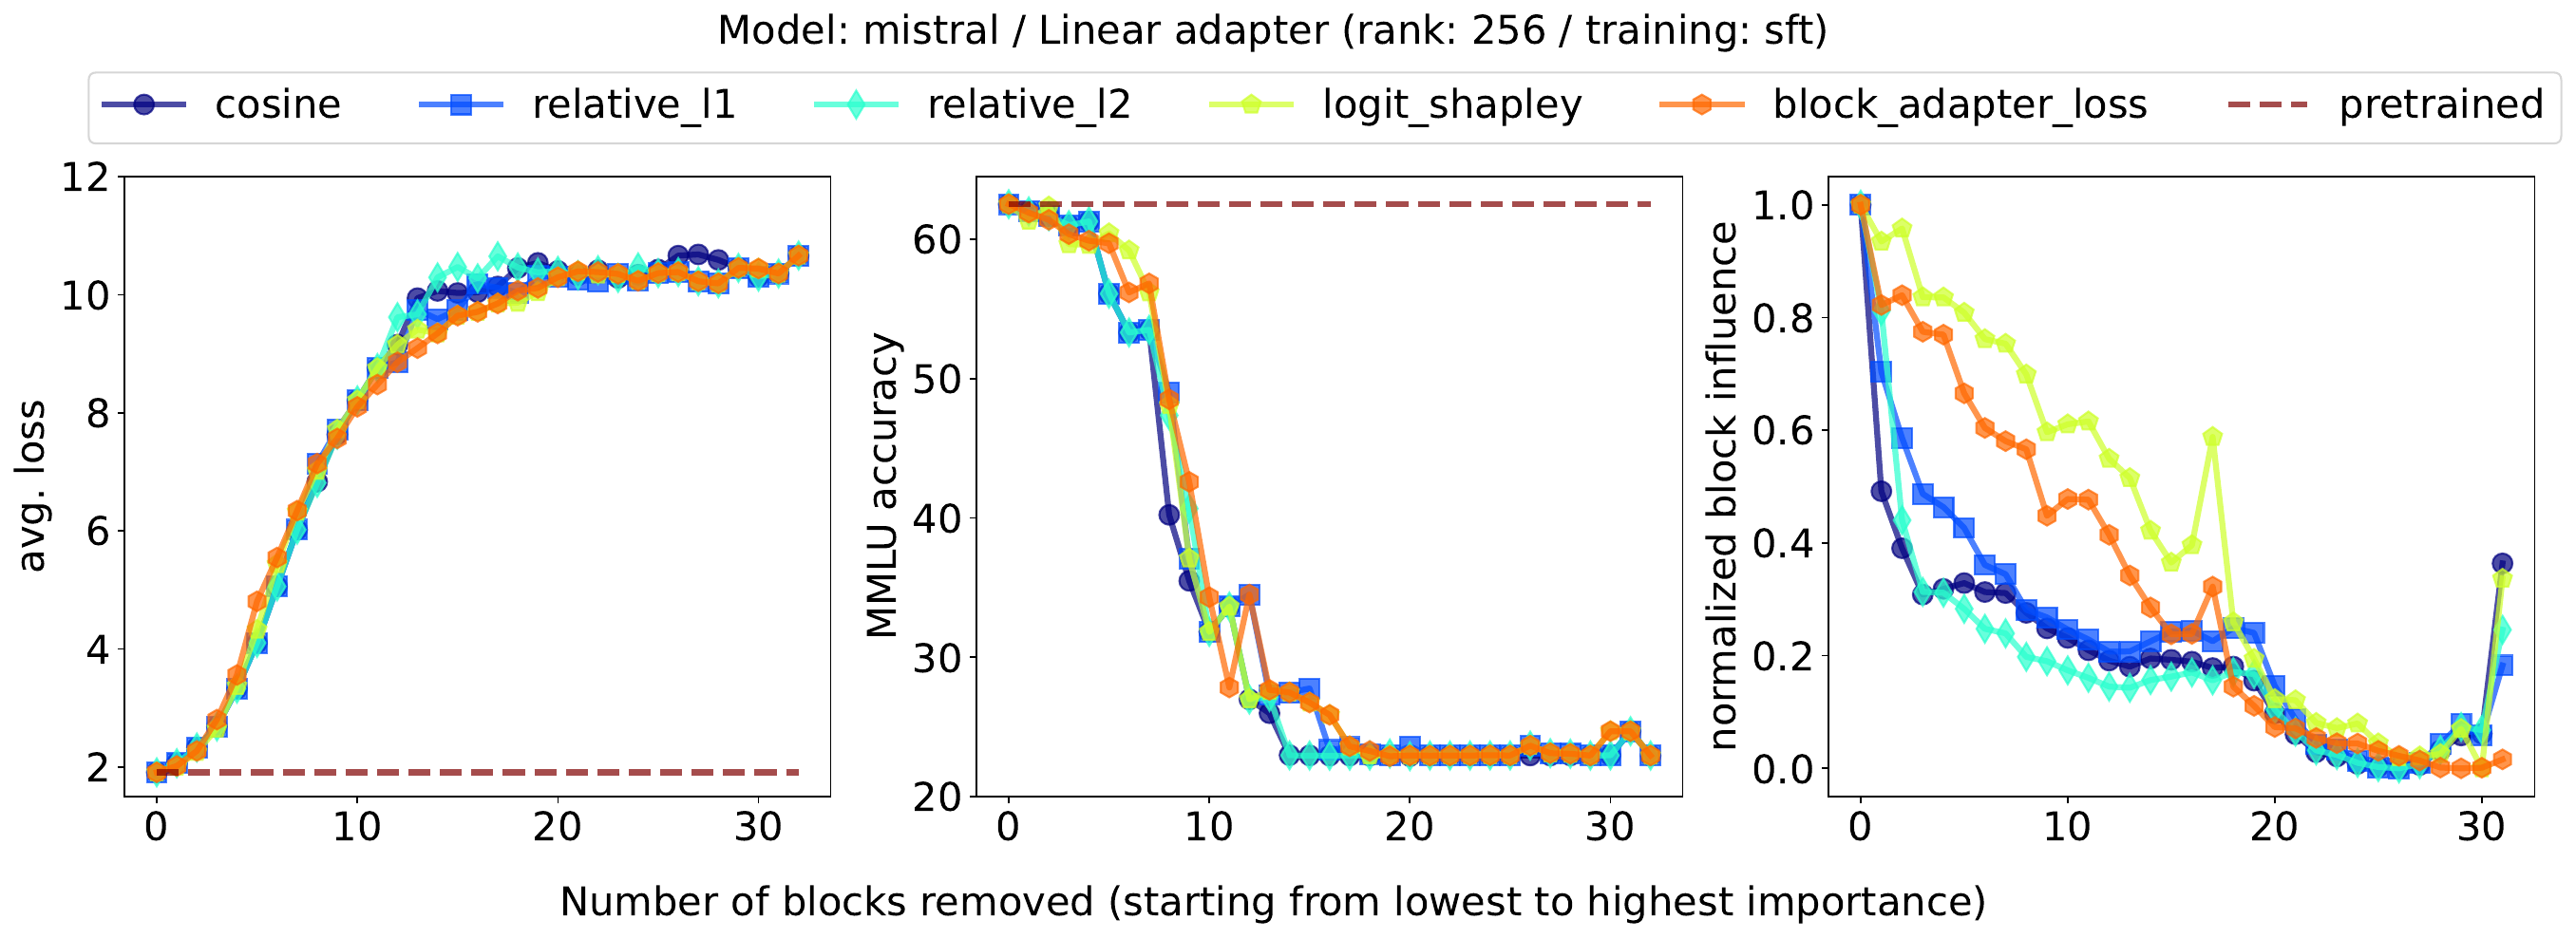}
    }

    \subfloat{
        \includegraphics[width=\textwidth]{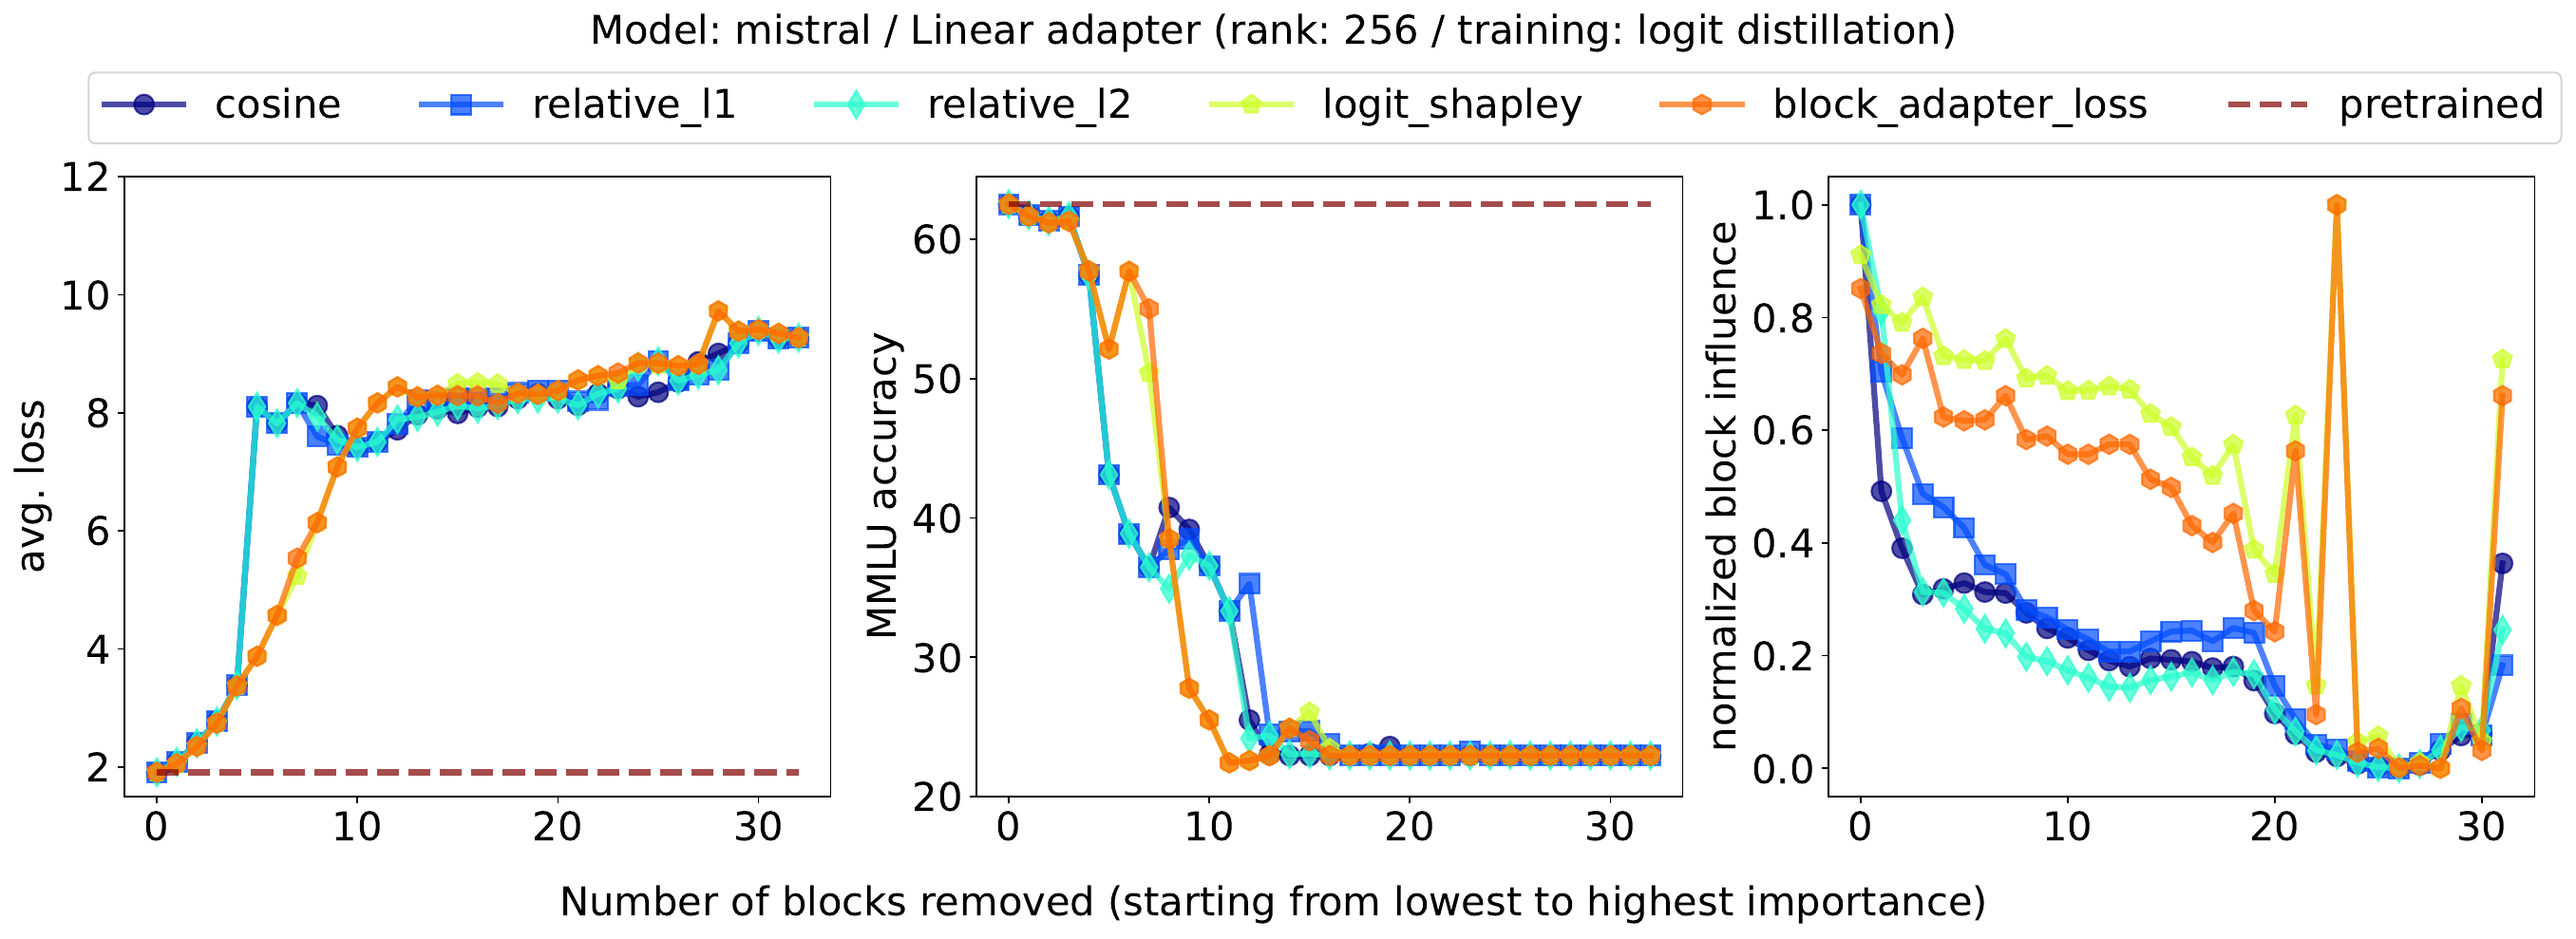}
    }
    \caption{\textbf{Evaluating the impact of linear adapters for Mistral 7b with a rank of 256} trained using three different metrics including (a) MSE loss defined on the representation, (b) supervised fine-tuning (SFT), and (c) logit distillation where logits are distilled from the full model.}
    \label{fig:linear_adapters_rank_256_mistral}
\end{figure}

Results for LLaMa-2 7b and Mistral 7b with an adapter rank of 256 on the original scale are visualized in
Fig.~\ref{fig:linear_adapters_rank_256_llama2} and Fig.~\ref{fig:linear_adapters_rank_256_mistral} respectively.

\section{Low-rank linear adapter loss curves}
\label{appendix:linear_adapter_loss_curves}

\begin{figure}[t]
    \centering
    \subfloat{
        \includegraphics[width=0.245\textwidth]{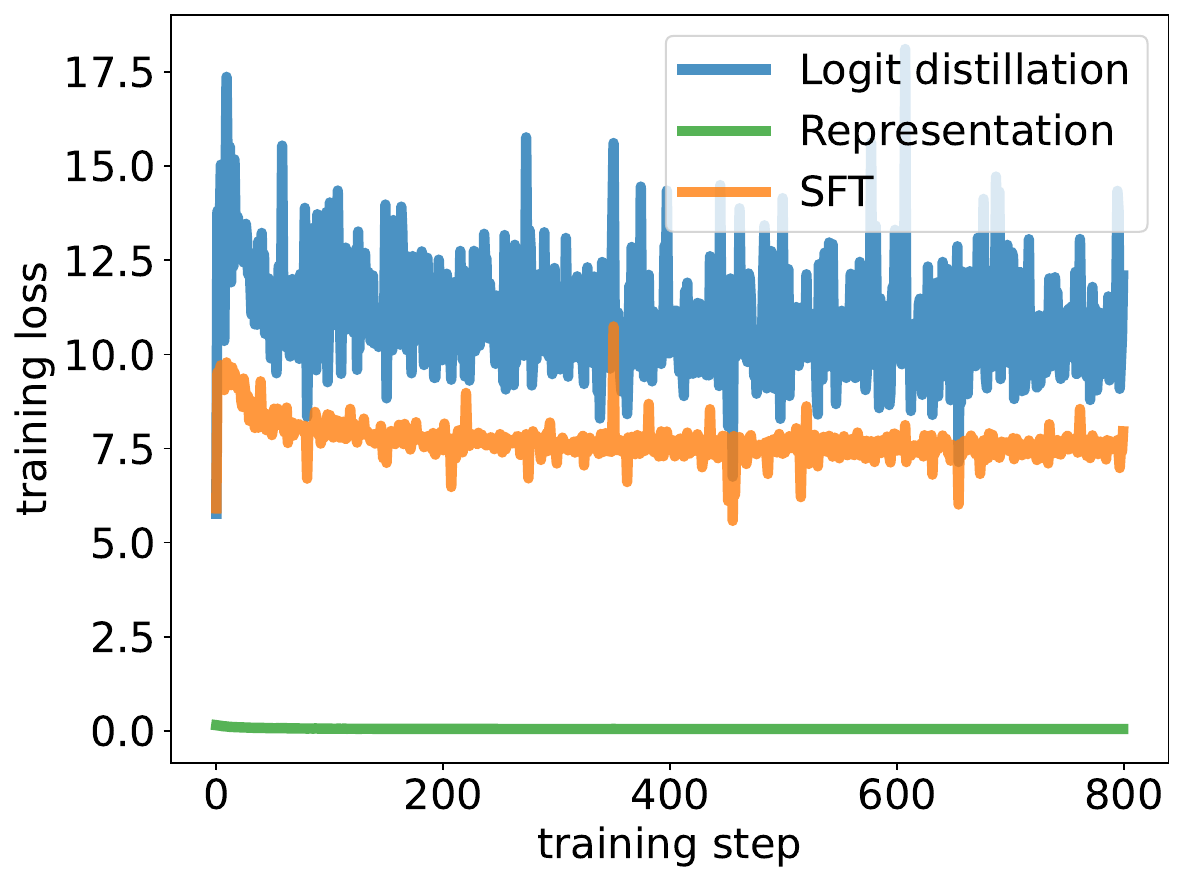}
    }
    \subfloat{
        \includegraphics[width=0.245\textwidth]{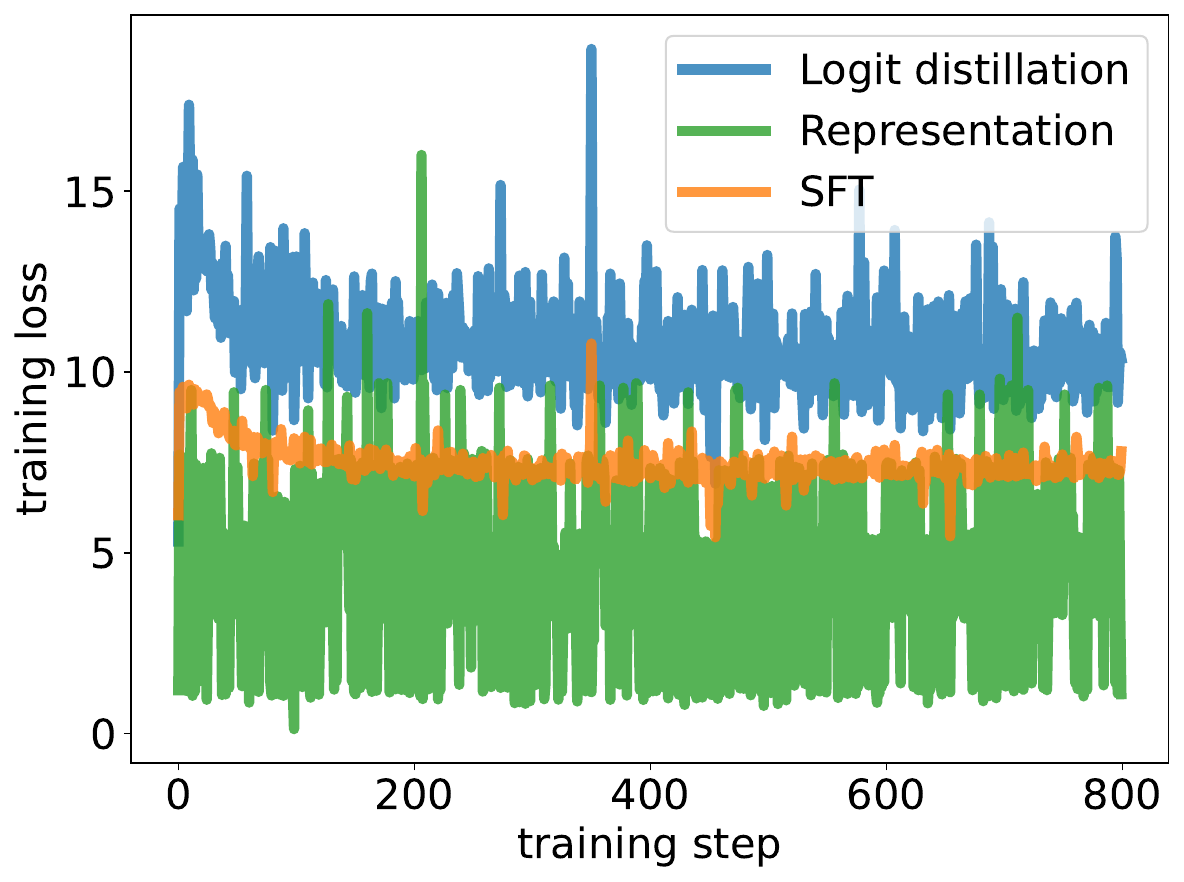}
    }
    \subfloat{
        \includegraphics[width=0.245\textwidth]{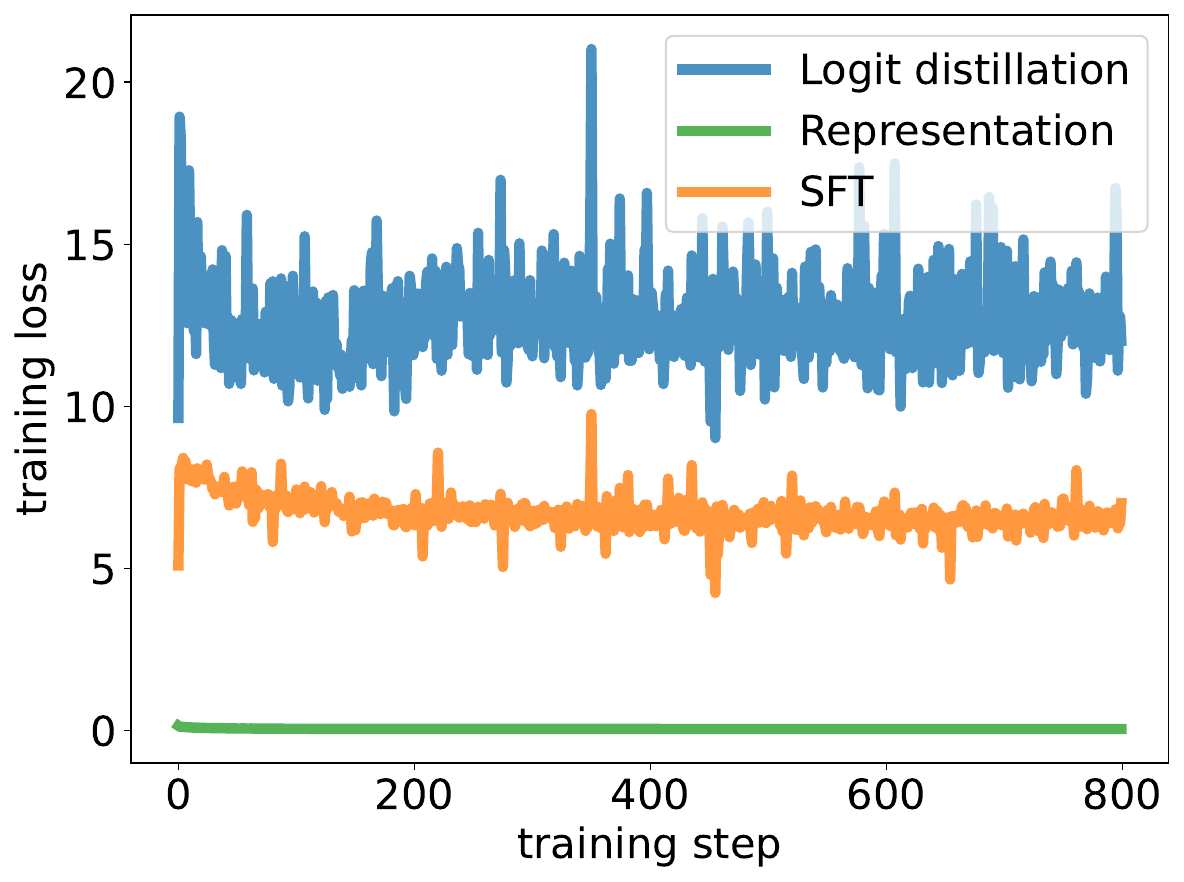}
    }
    \subfloat{
        \includegraphics[width=0.245\textwidth]{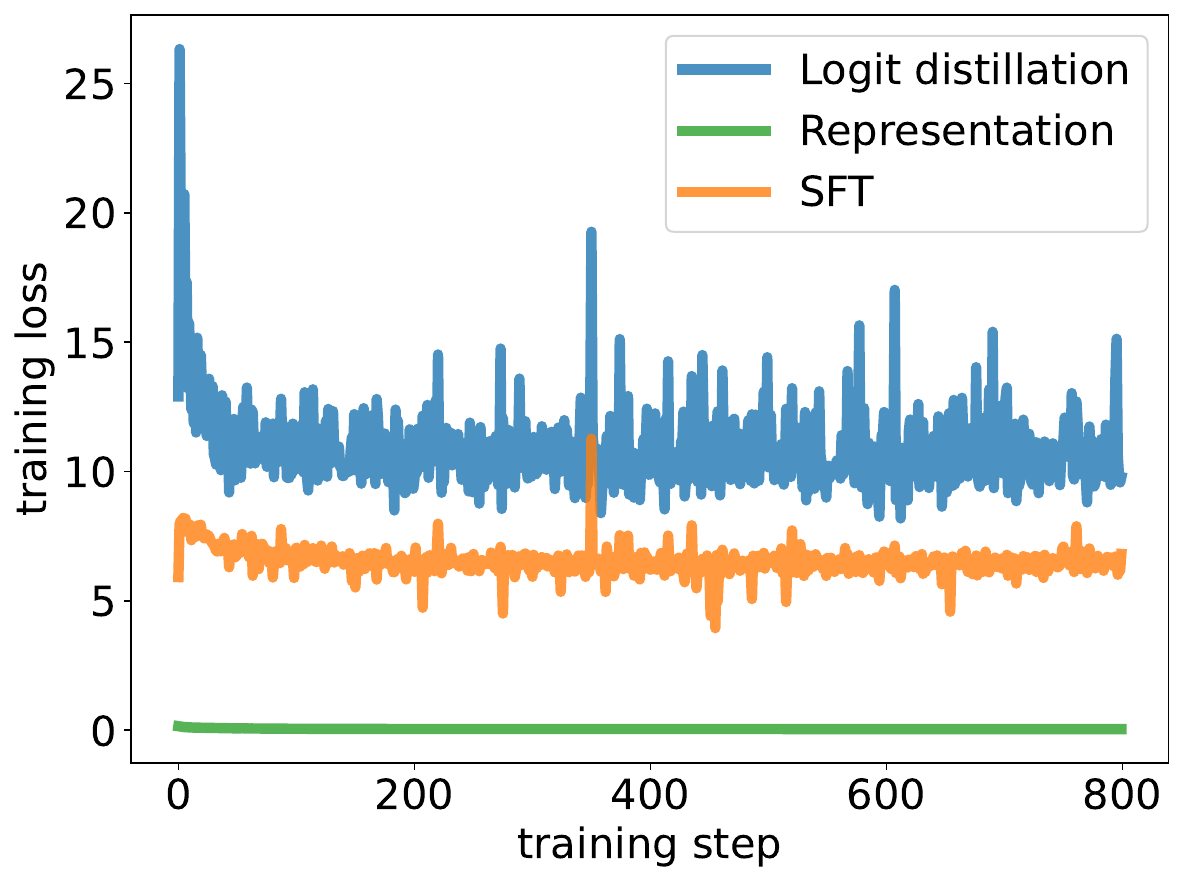}
    }

    \subfloat{
        \includegraphics[width=0.245\textwidth]{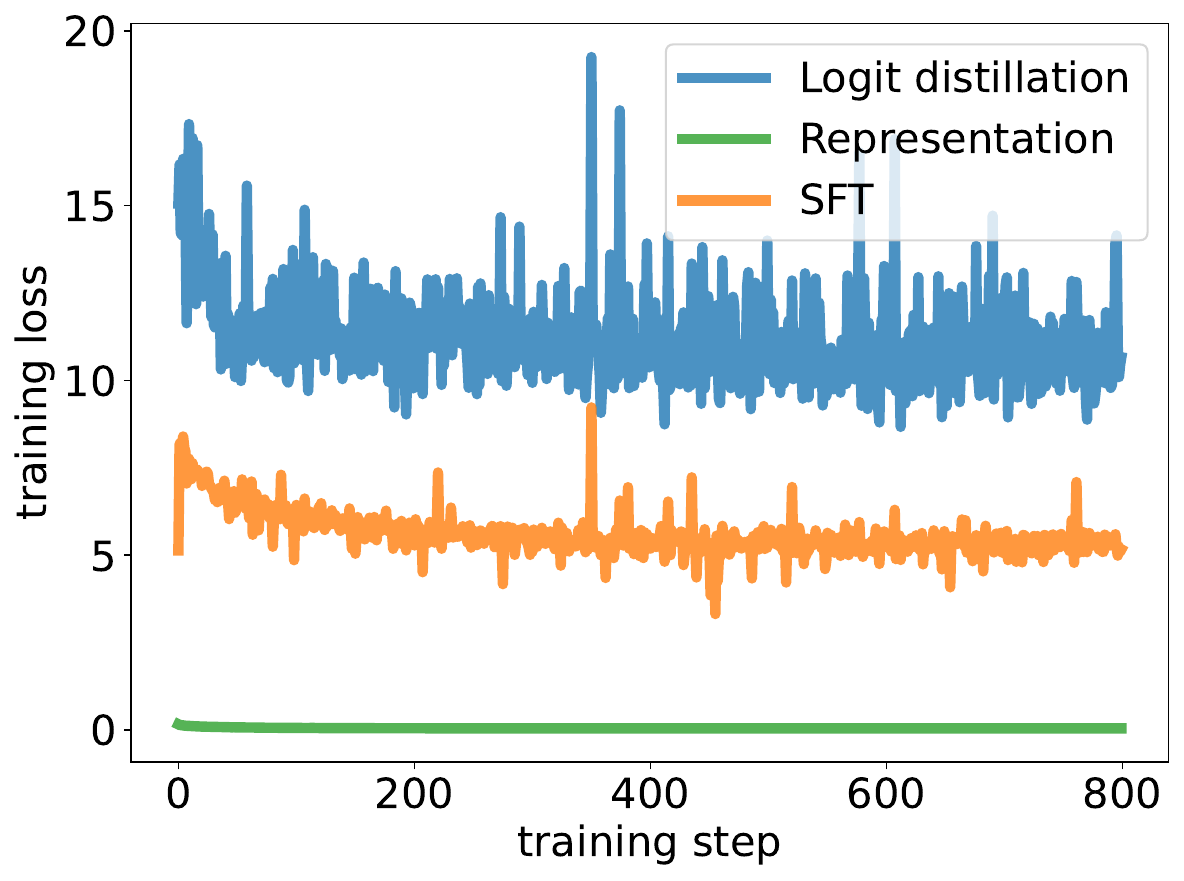}
    }
    \subfloat{
        \includegraphics[width=0.245\textwidth]{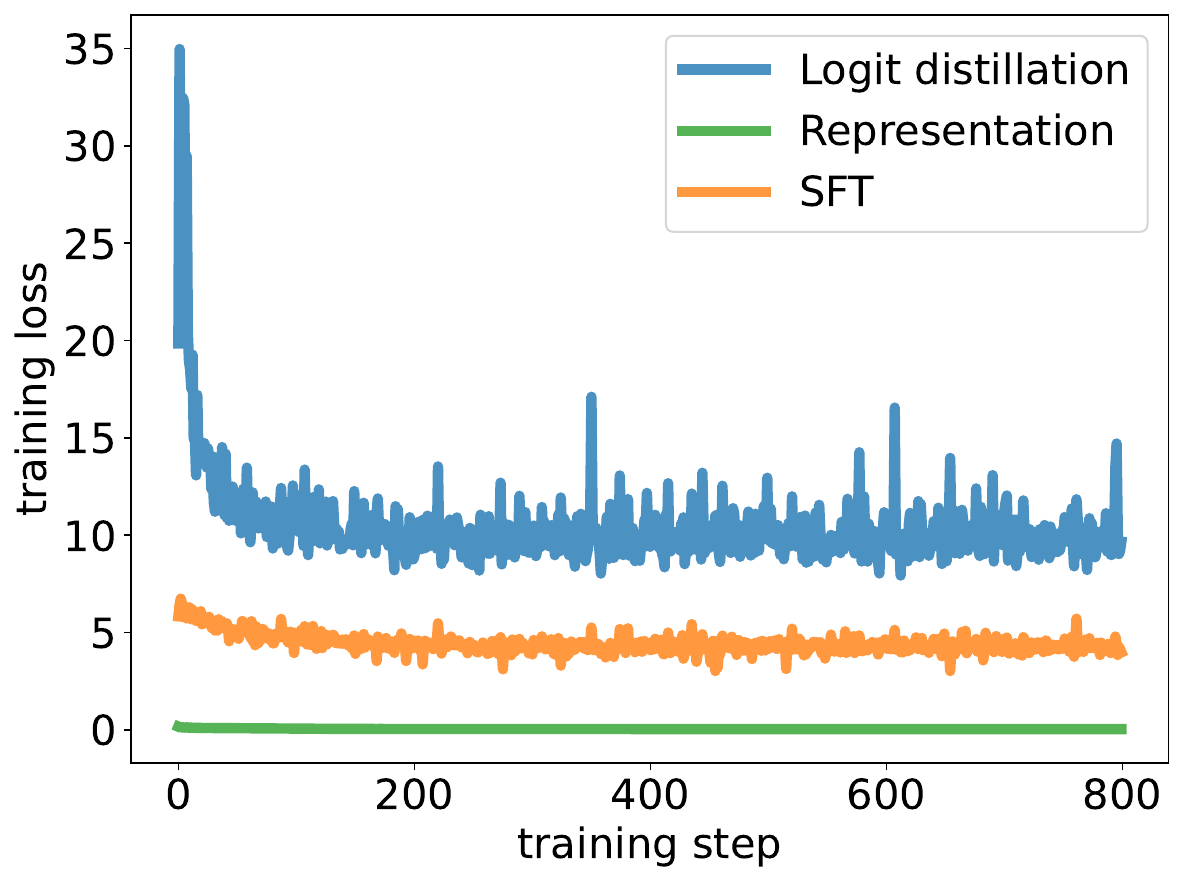}
    }
    \subfloat{
        \includegraphics[width=0.245\textwidth]{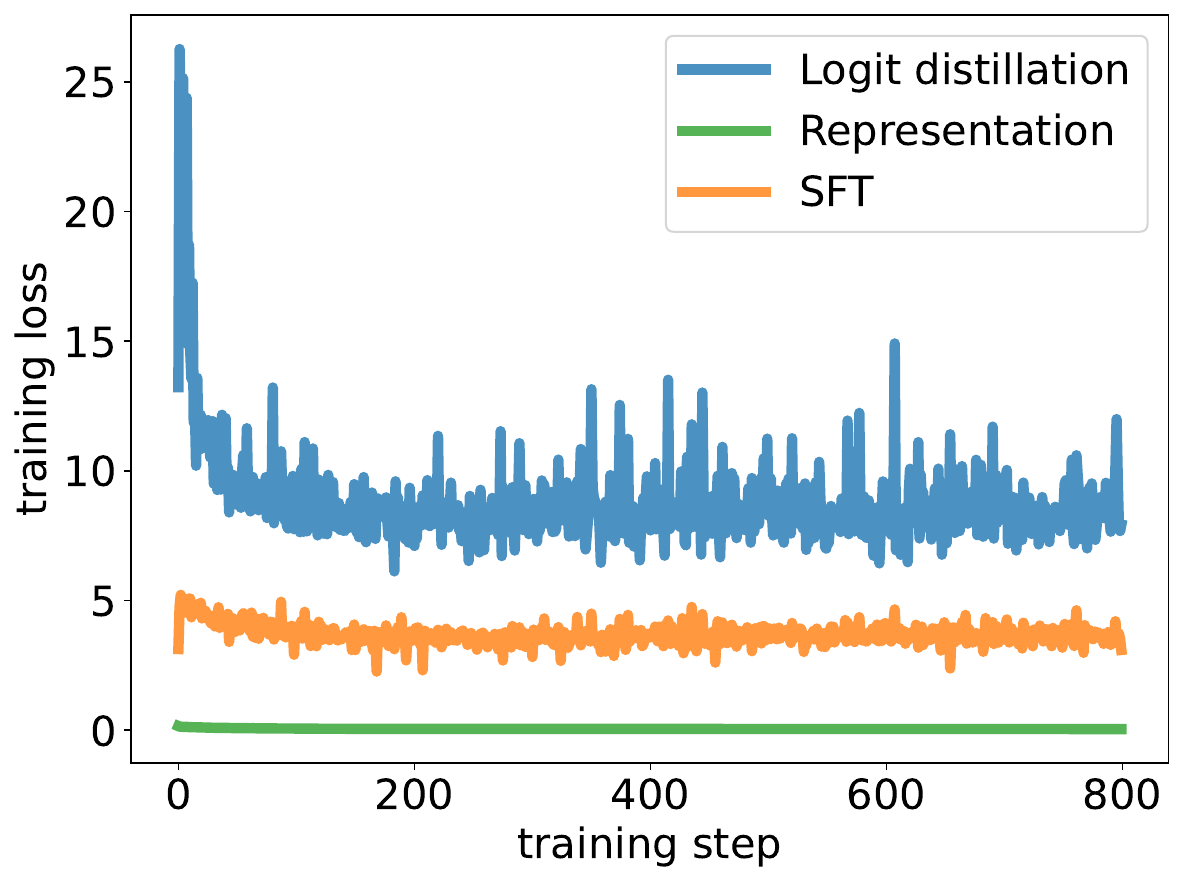}
    }
    \subfloat{
        \includegraphics[width=0.245\textwidth]{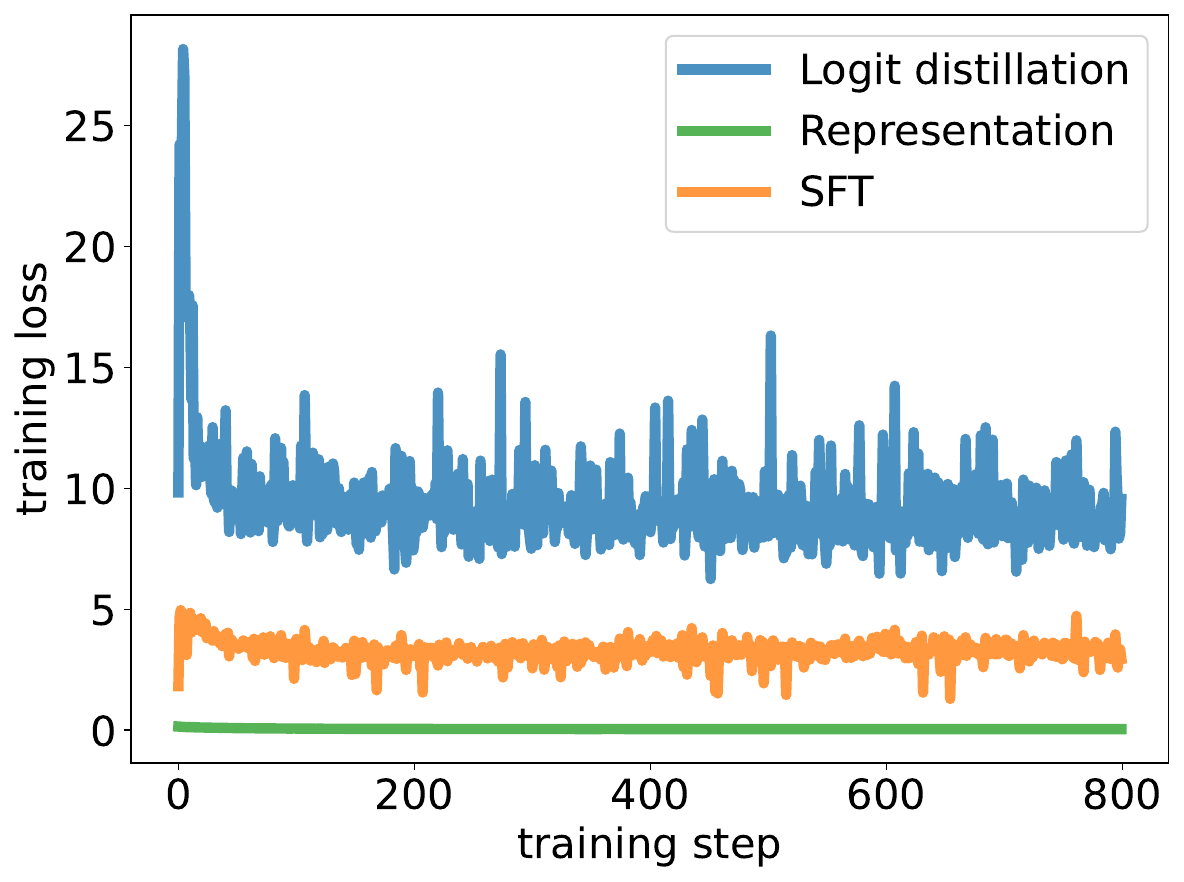}
    }

    \subfloat{
        \includegraphics[width=0.245\textwidth]{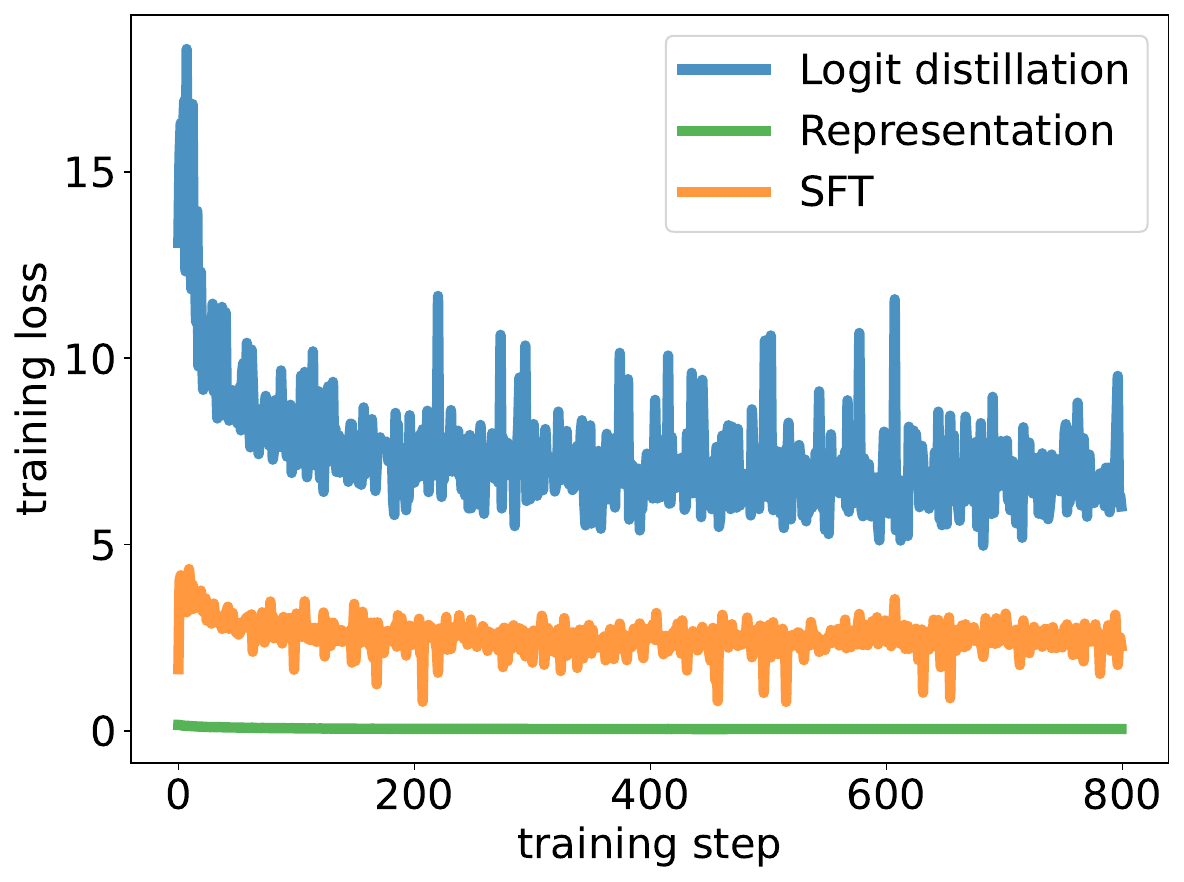}
    }
    \subfloat{
        \includegraphics[width=0.245\textwidth]{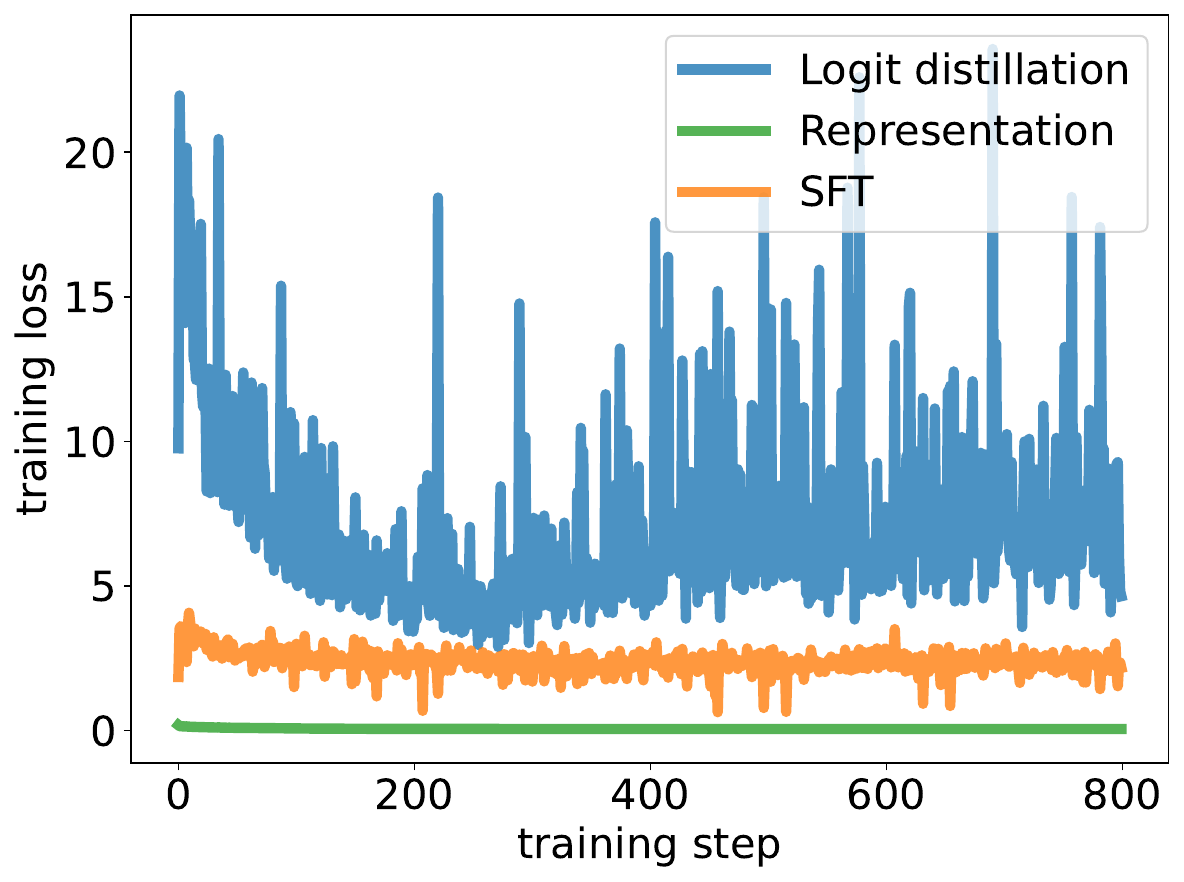}
    }
    \subfloat{
        \includegraphics[width=0.245\textwidth]{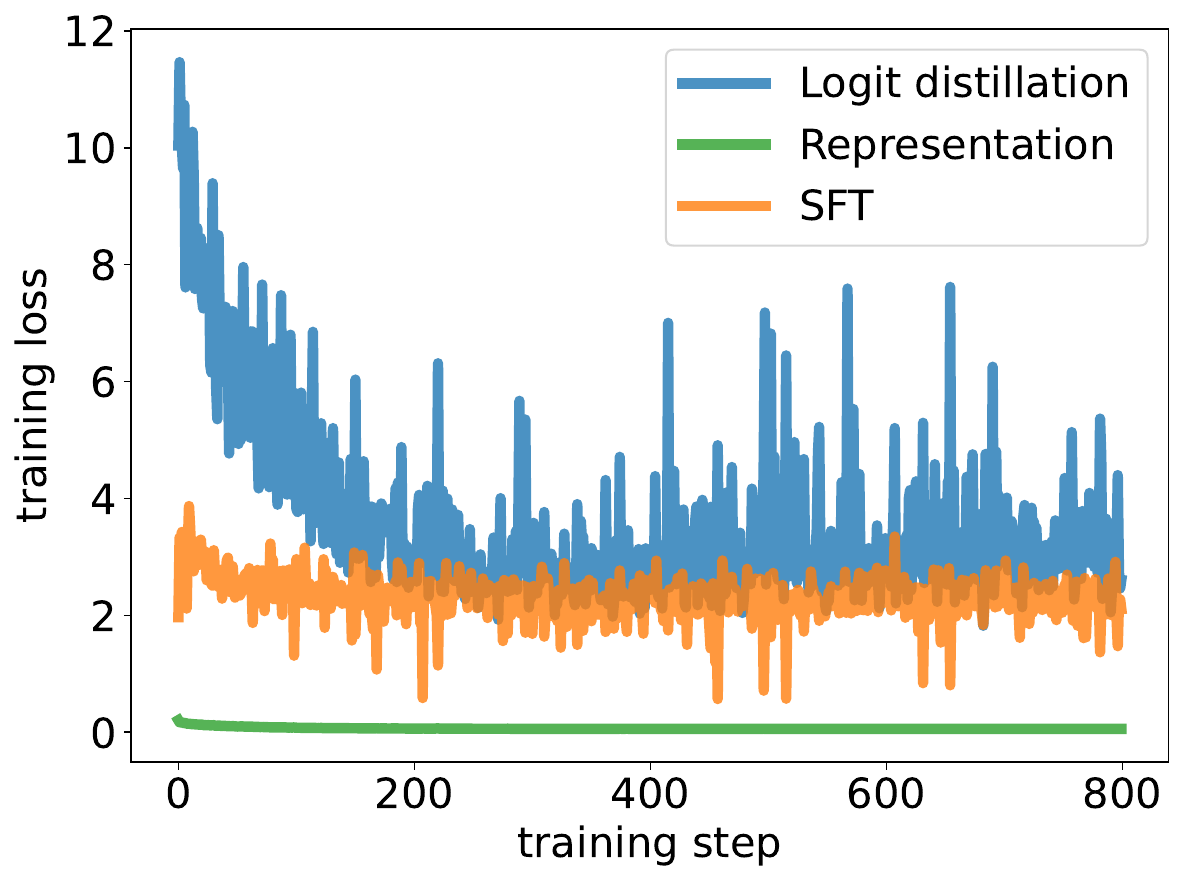}
    }
    \subfloat{
        \includegraphics[width=0.245\textwidth]{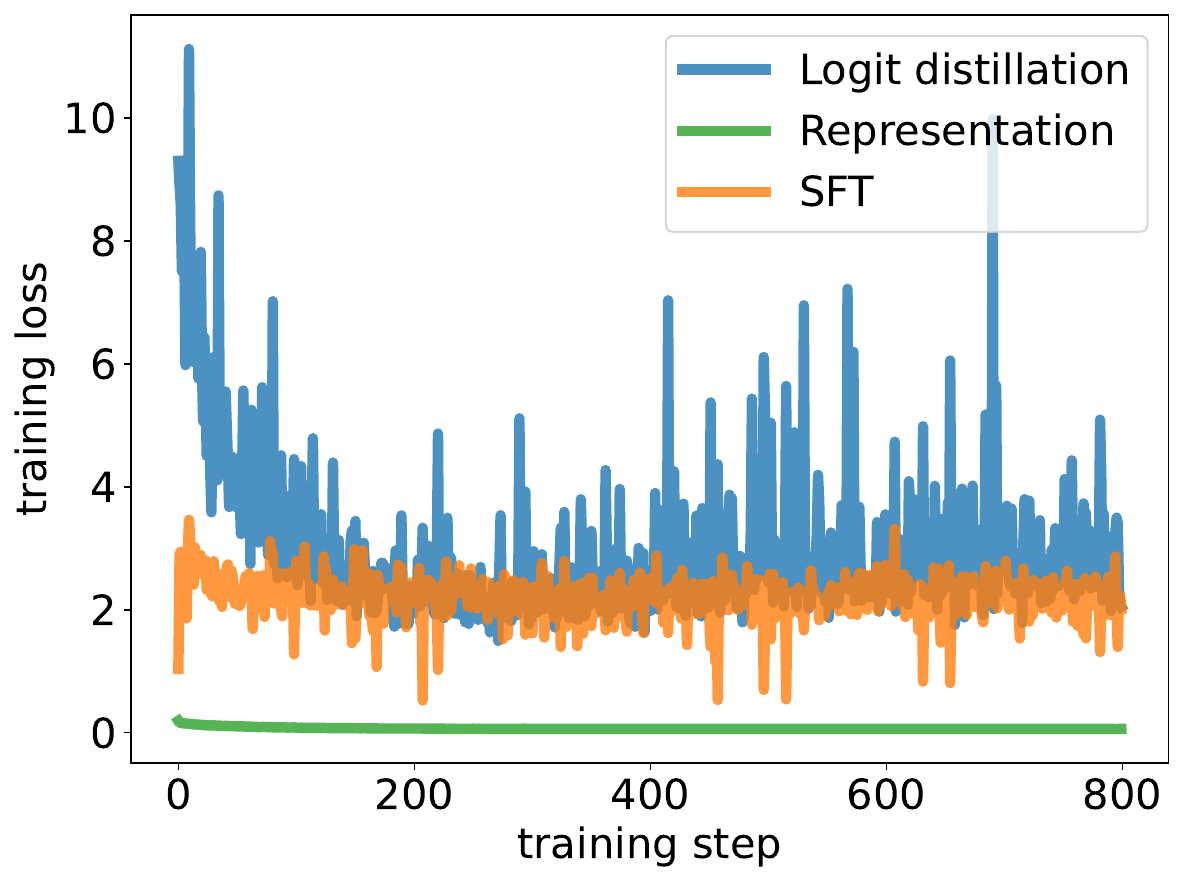}
    }

    \subfloat{
        \includegraphics[width=0.245\textwidth]{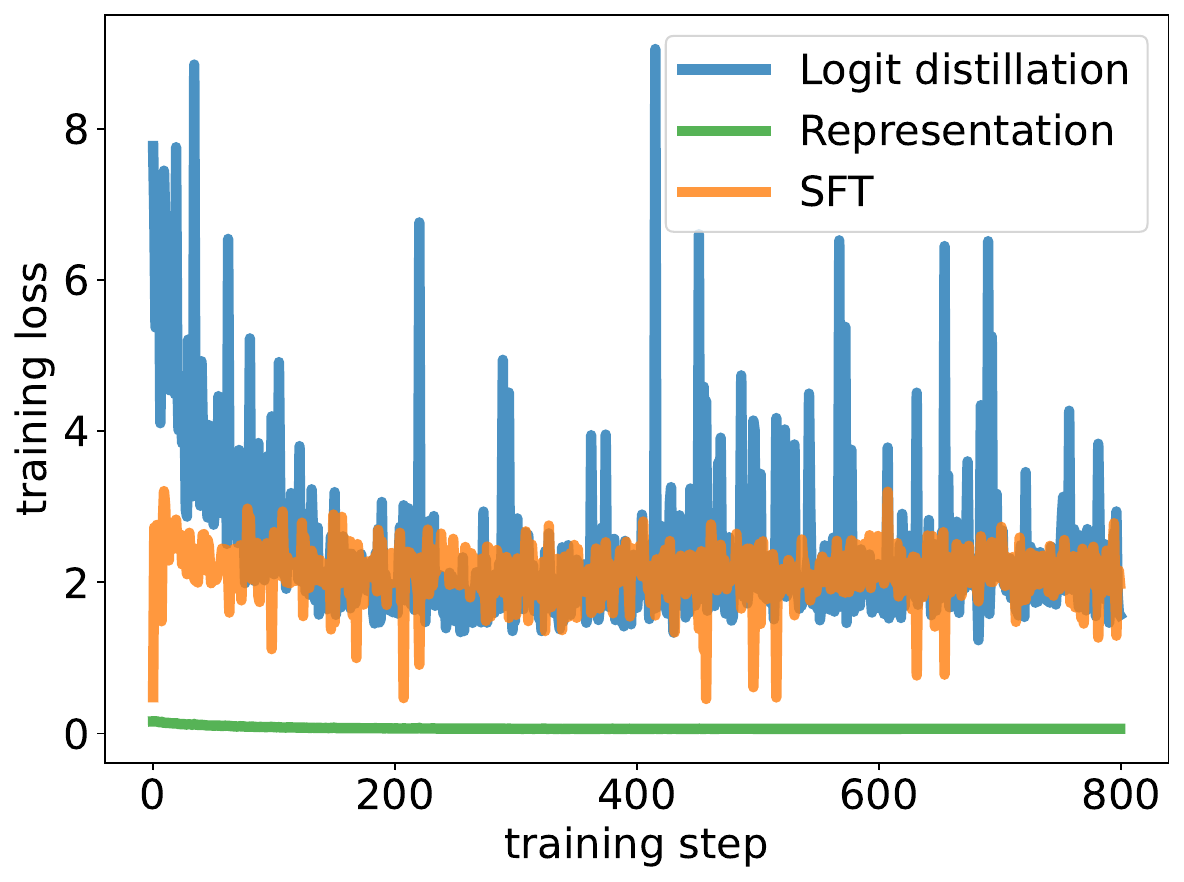}
    }
    \subfloat{
        \includegraphics[width=0.245\textwidth]{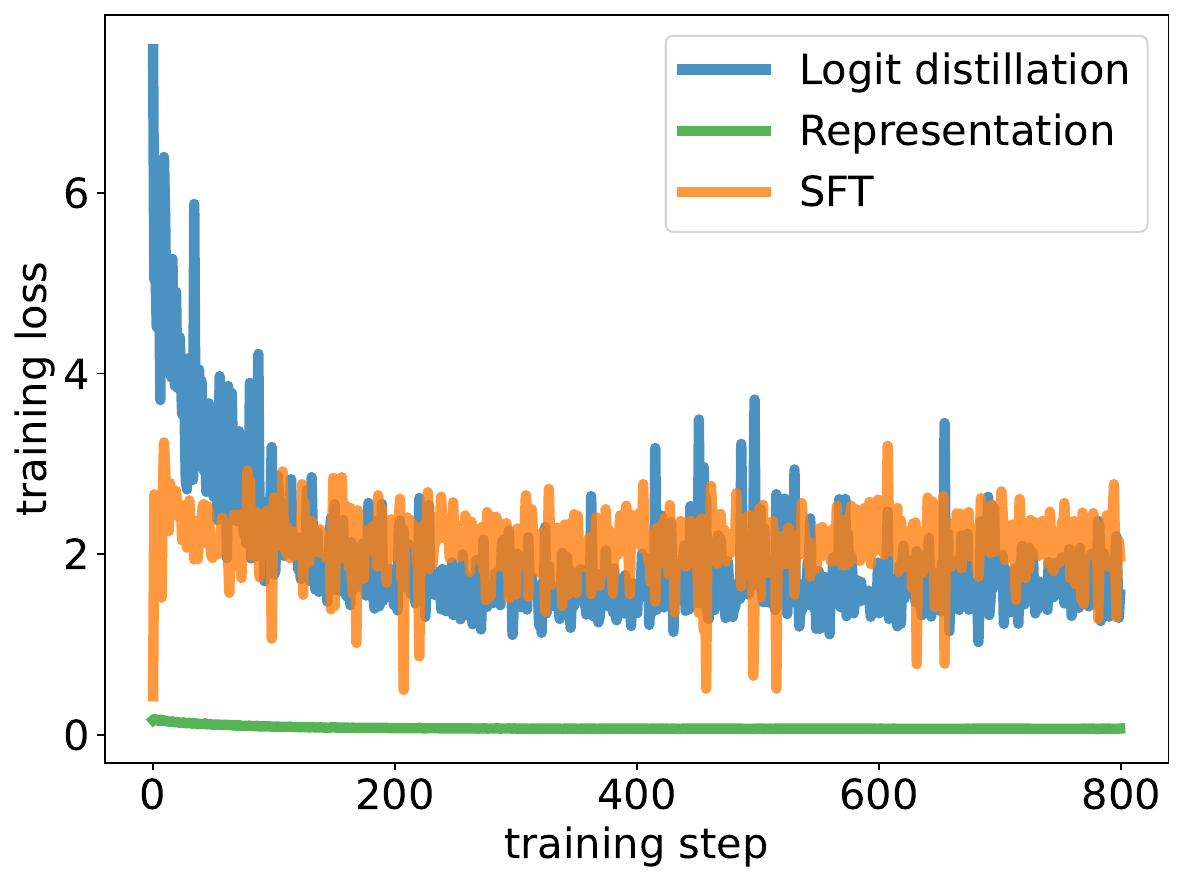}
    }
    \subfloat{
        \includegraphics[width=0.245\textwidth]{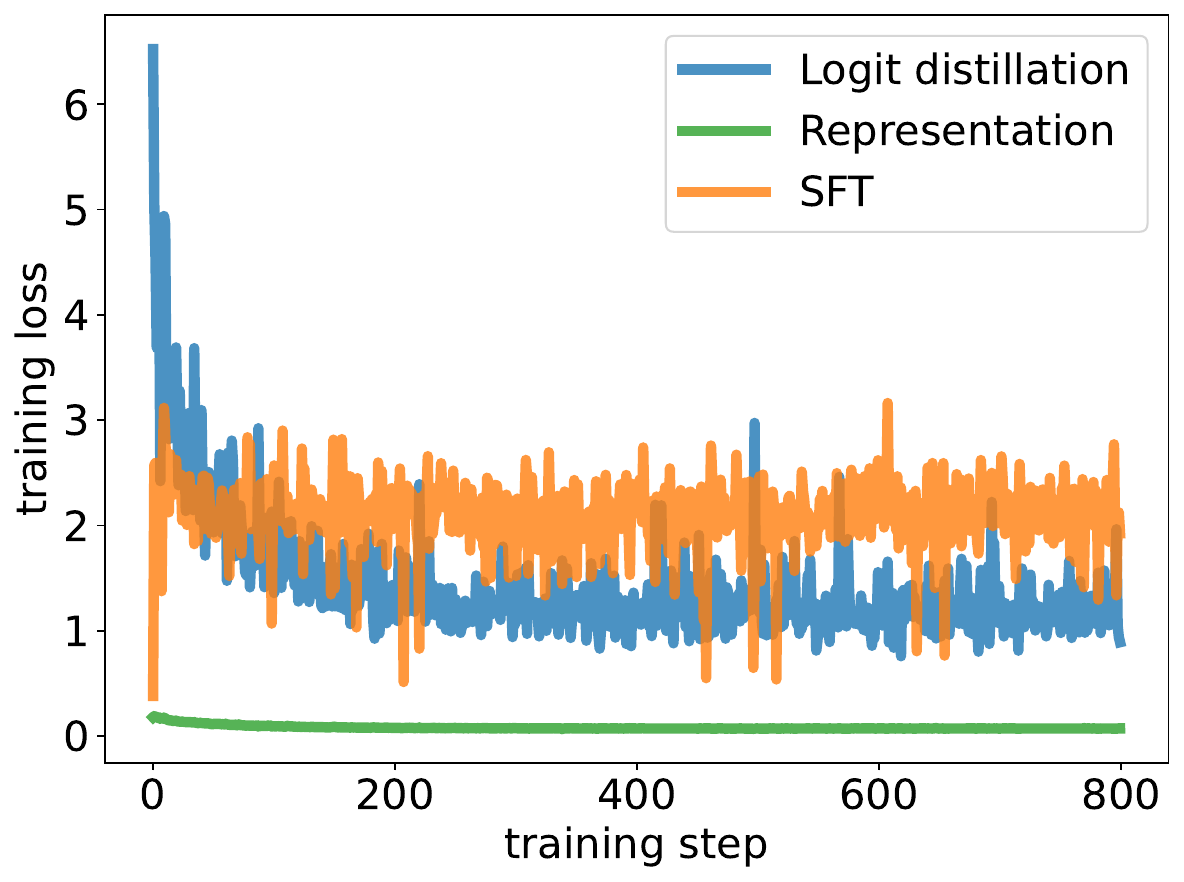}
    }
    \subfloat{
        \includegraphics[width=0.245\textwidth]{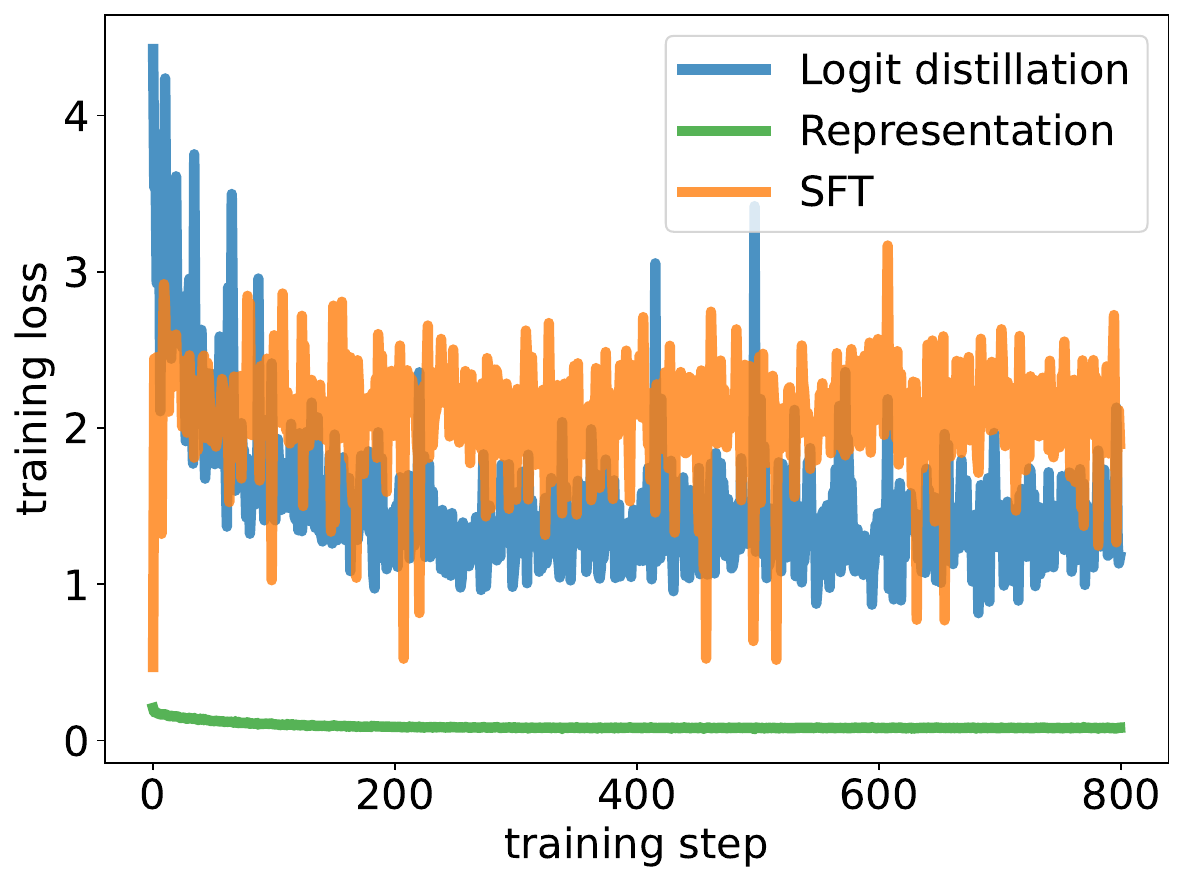}
    }

    \subfloat{
        \includegraphics[width=0.245\textwidth]{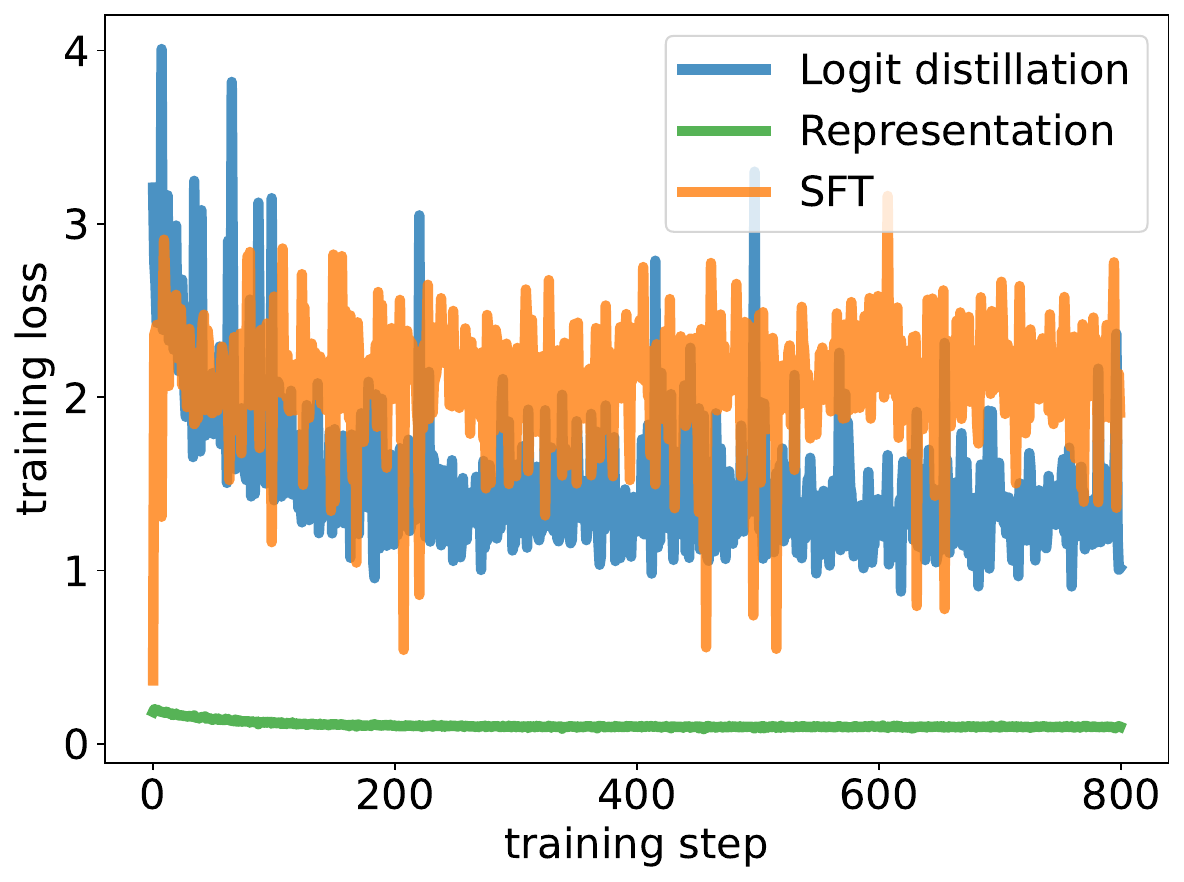}
    }
    \subfloat{
        \includegraphics[width=0.245\textwidth]{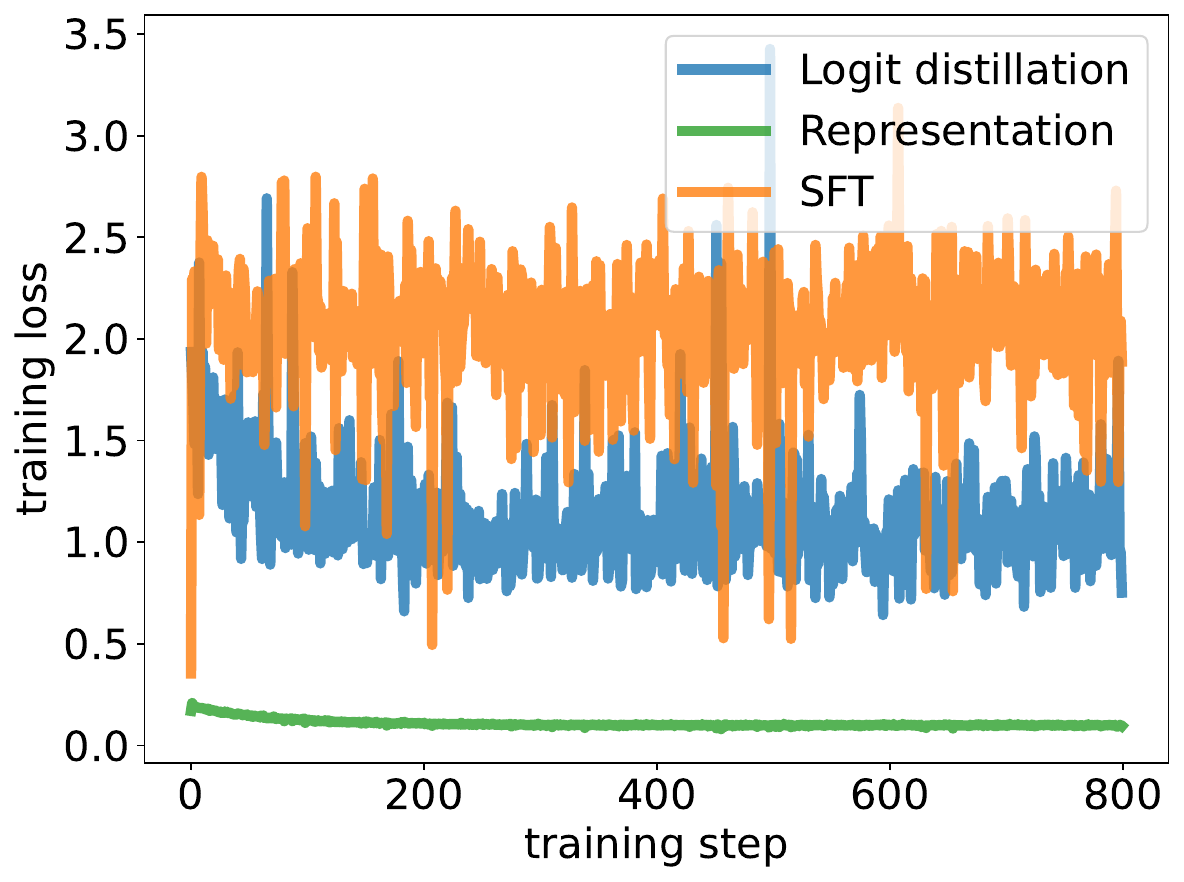}
    }
    \subfloat{
        \includegraphics[width=0.245\textwidth]{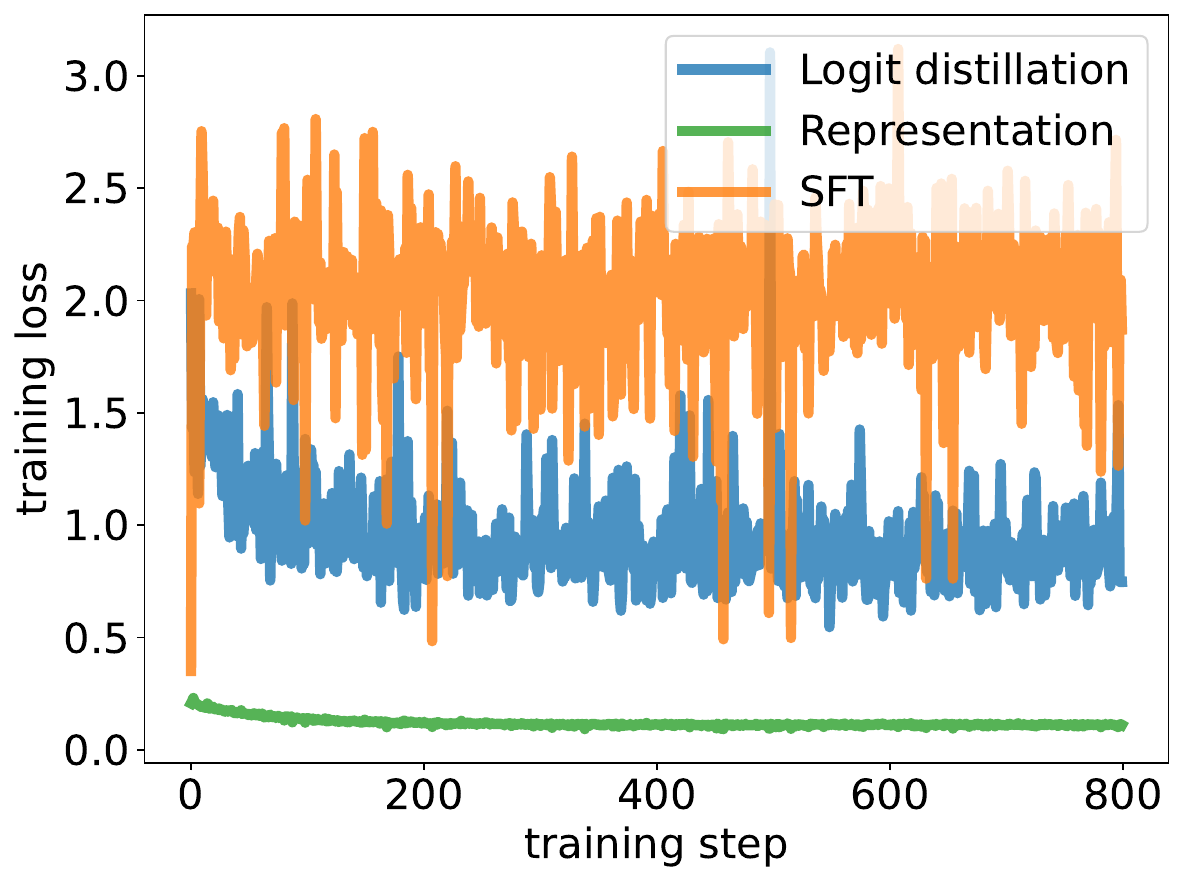}
    }
    \subfloat{
        \includegraphics[width=0.245\textwidth]{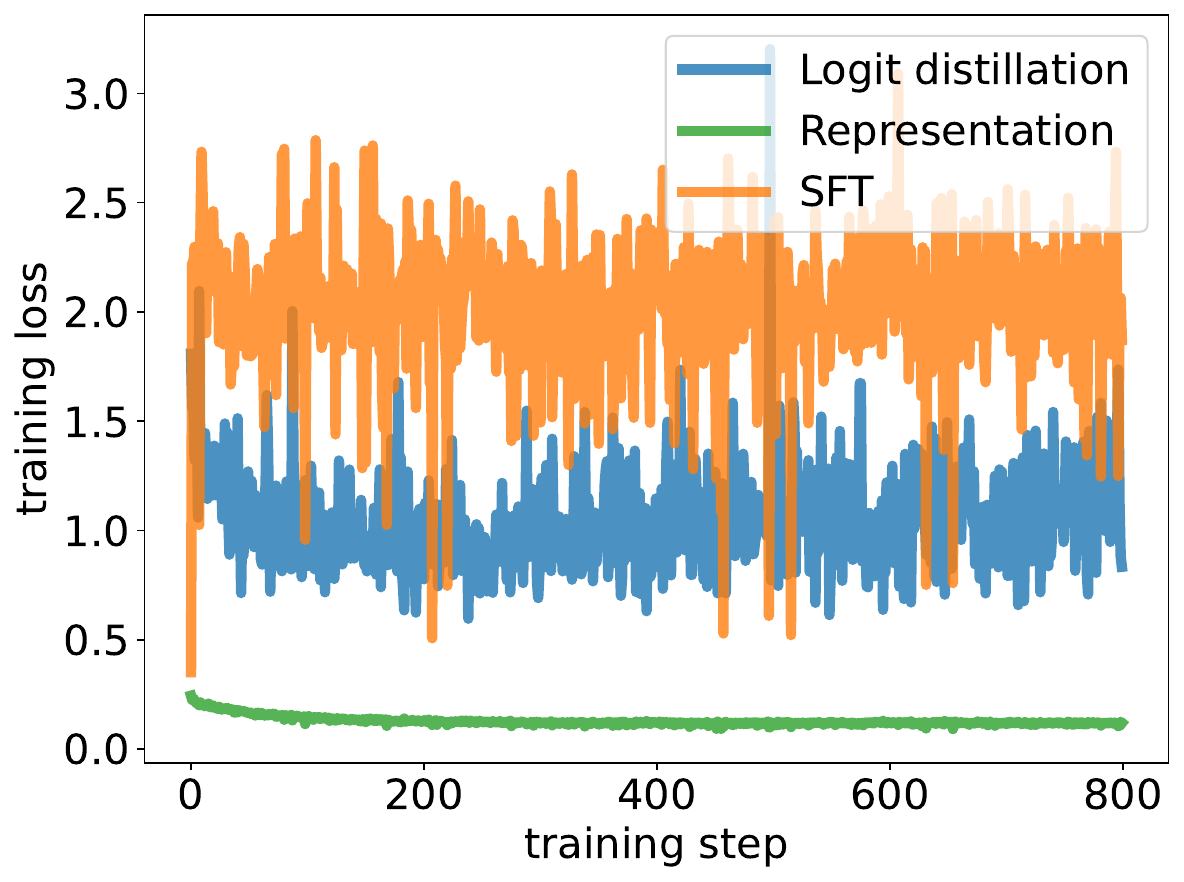}
    }

    \subfloat{
        \includegraphics[width=0.245\textwidth]{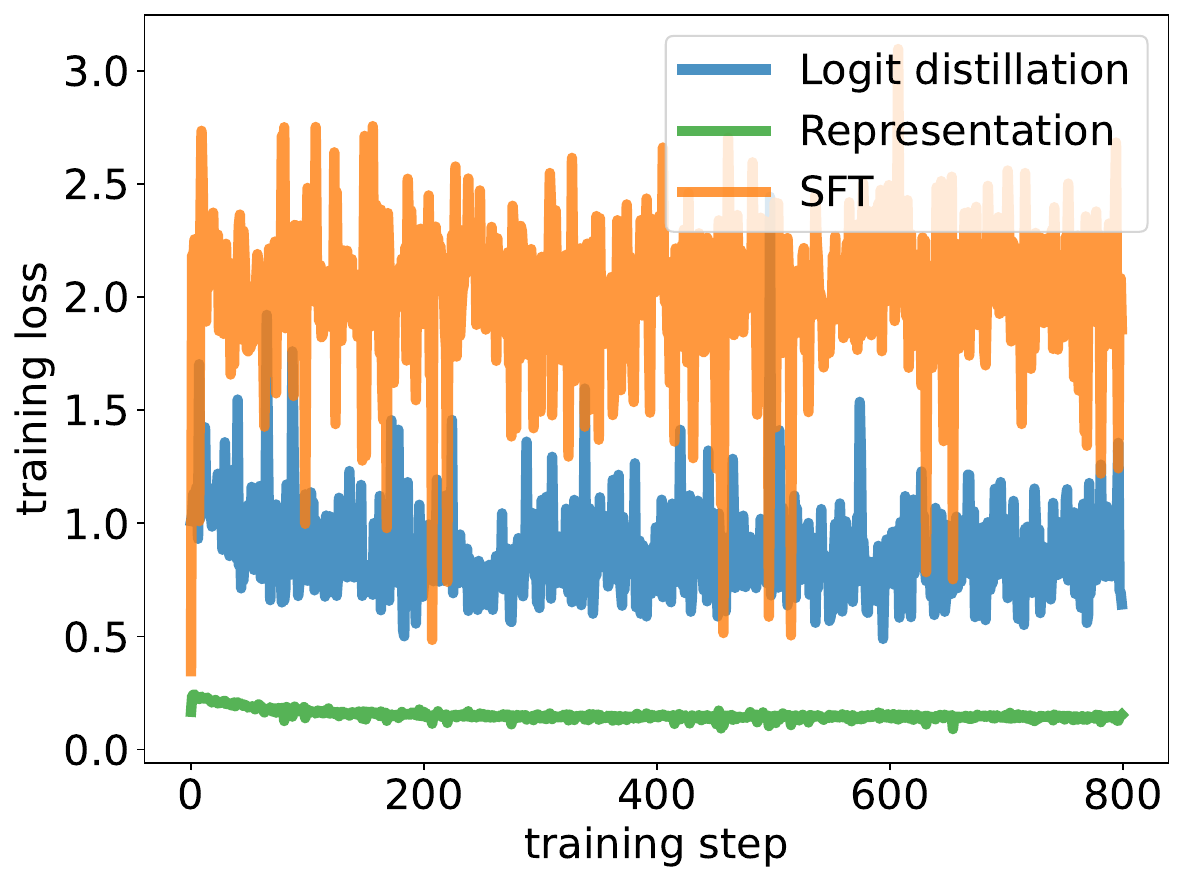}
    }
    \subfloat{
        \includegraphics[width=0.245\textwidth]{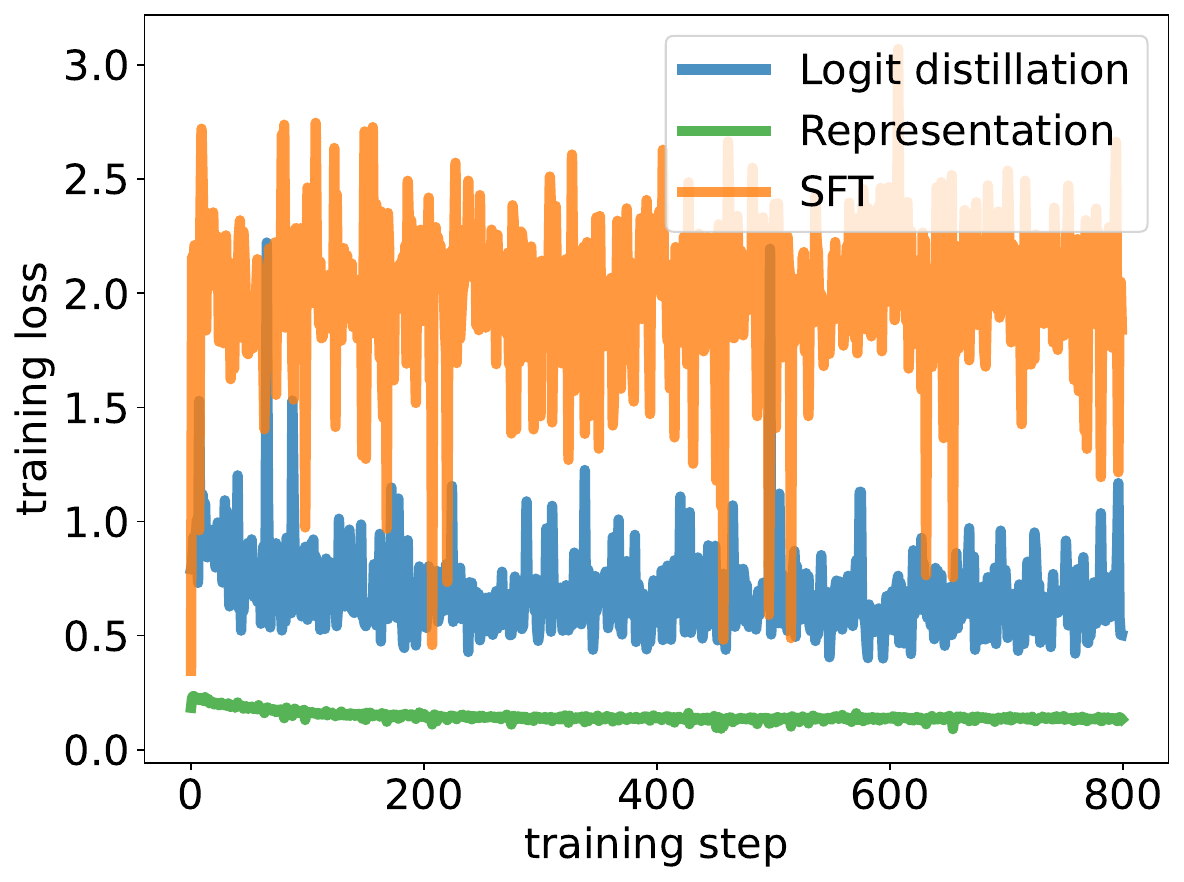}
    }
    \subfloat{
        \includegraphics[width=0.245\textwidth]{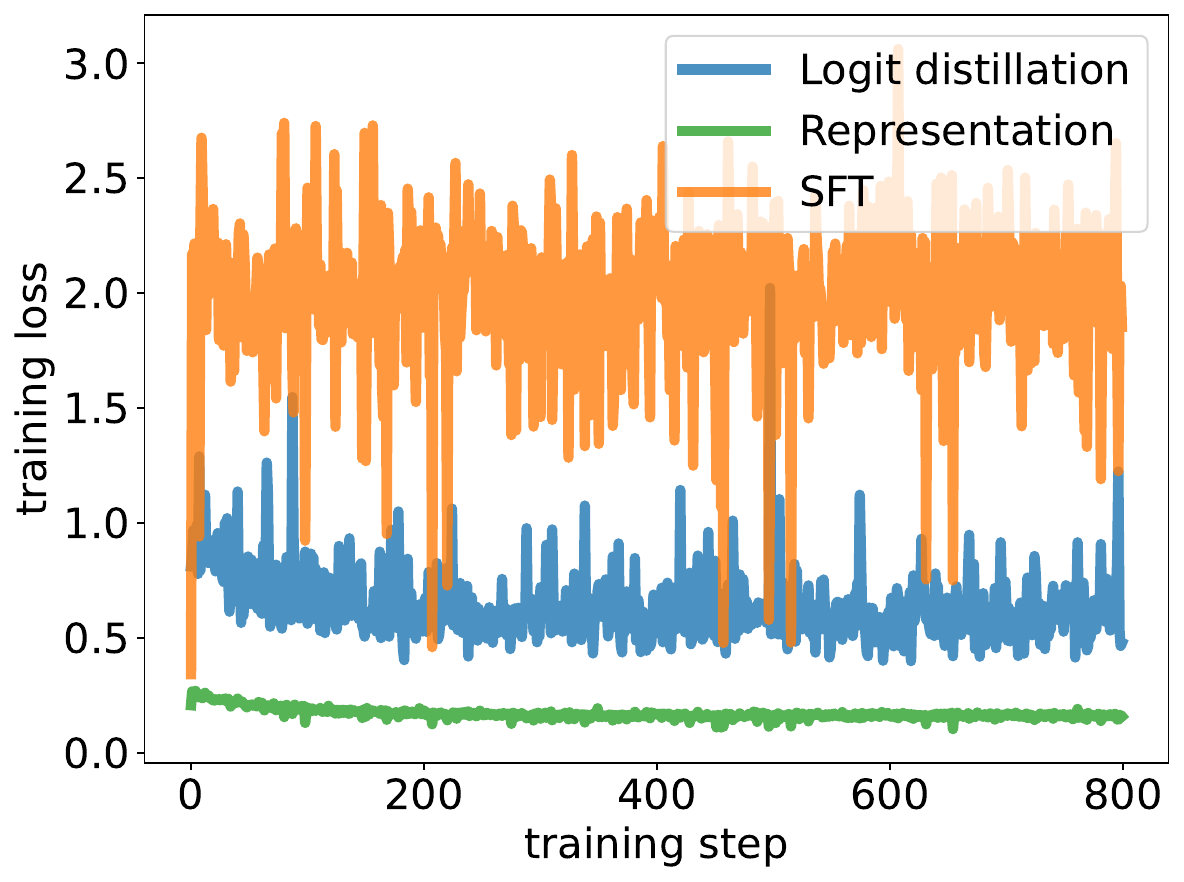}
    }
    \subfloat{
        \includegraphics[width=0.245\textwidth]{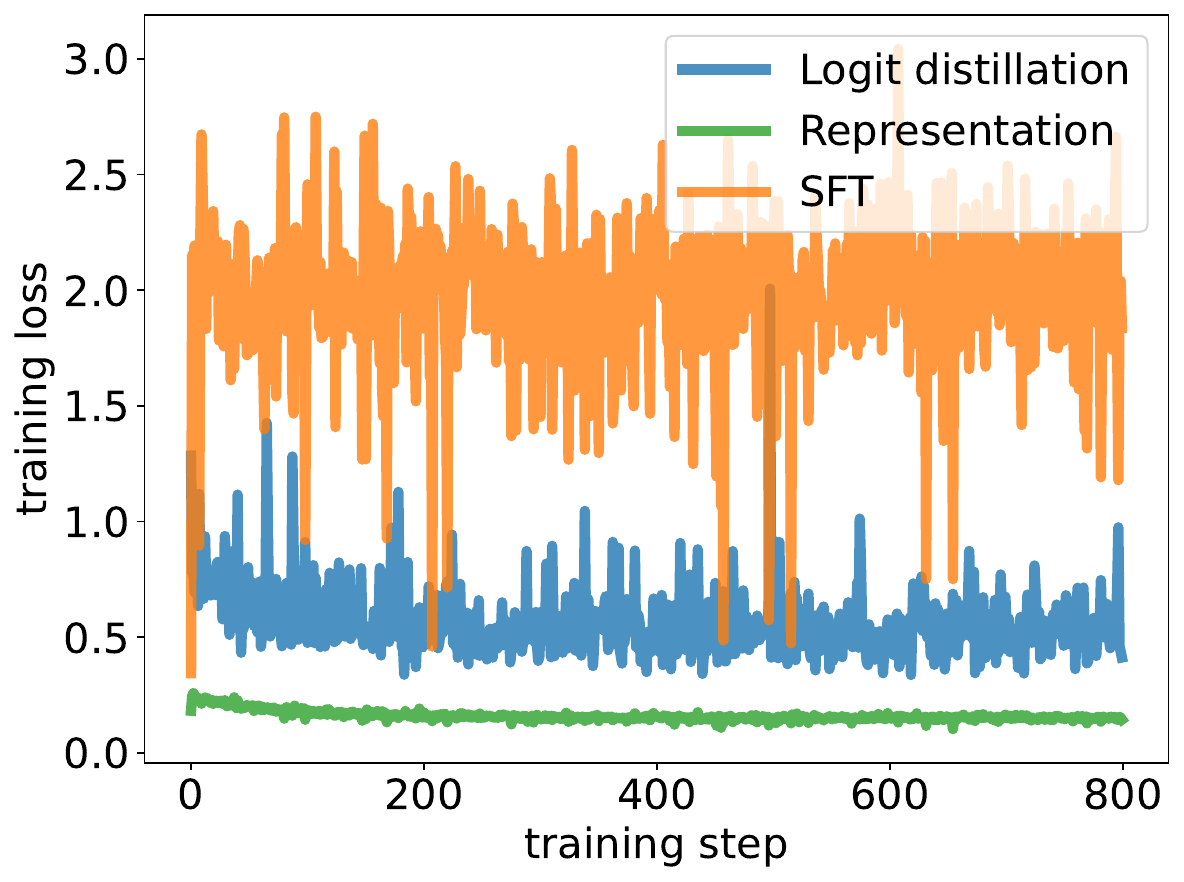}
    }

    \caption{\textbf{Low-rank linear adapter training curves for the first 24 LLaMa-2 7b blocks with a rank of 8} trained using three different objectives including (a) MSE loss defined on the representation, (b) supervised fine-tuning (SFT), and (c) logit distillation where logits are distilled from the full model. Rest of the blocks are visualized in Fig.~\ref{fig:linear_adapters_rank_8_llama2_train_loss_b}.}
    \label{fig:linear_adapters_rank_8_llama2_train_loss_a}
\end{figure}

\begin{figure}[t]
    \centering
    \subfloat{
        \includegraphics[width=0.245\textwidth]{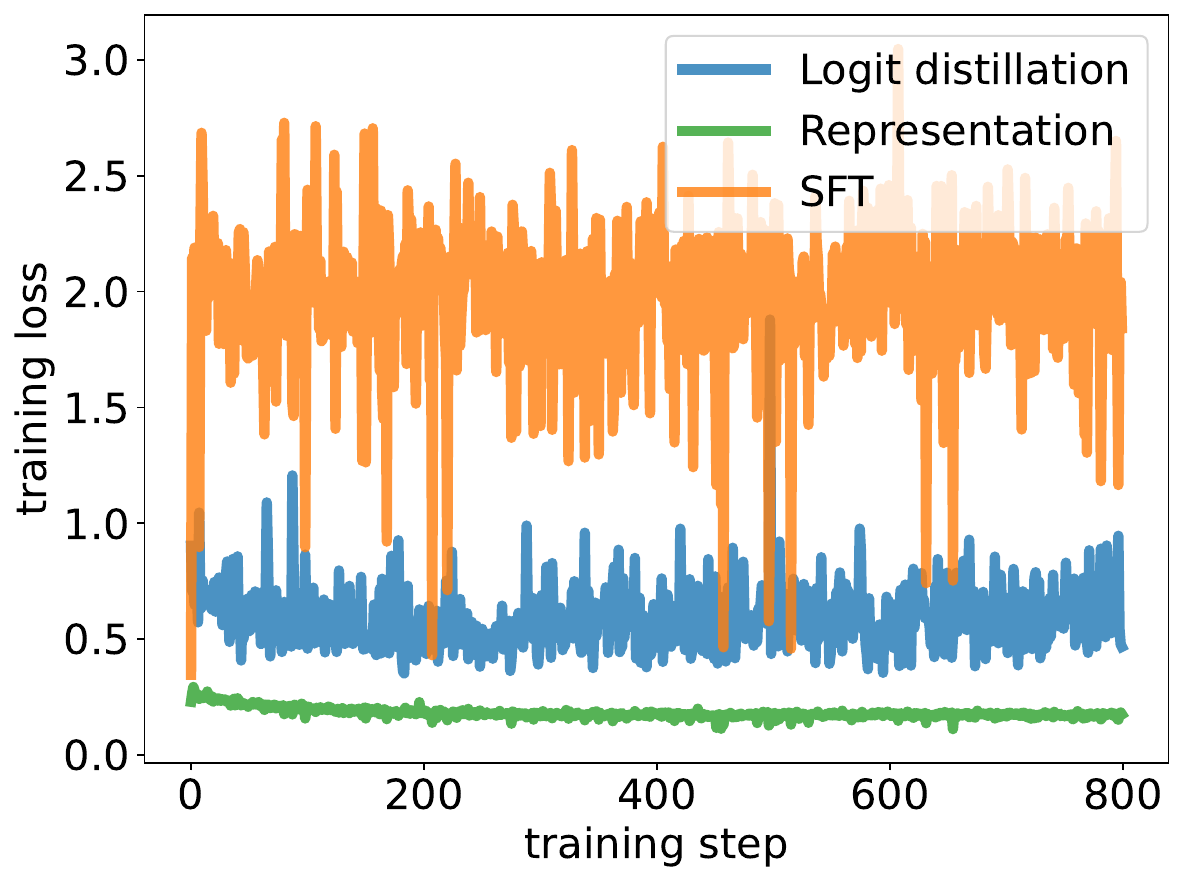}
    }
    \subfloat{
        \includegraphics[width=0.245\textwidth]{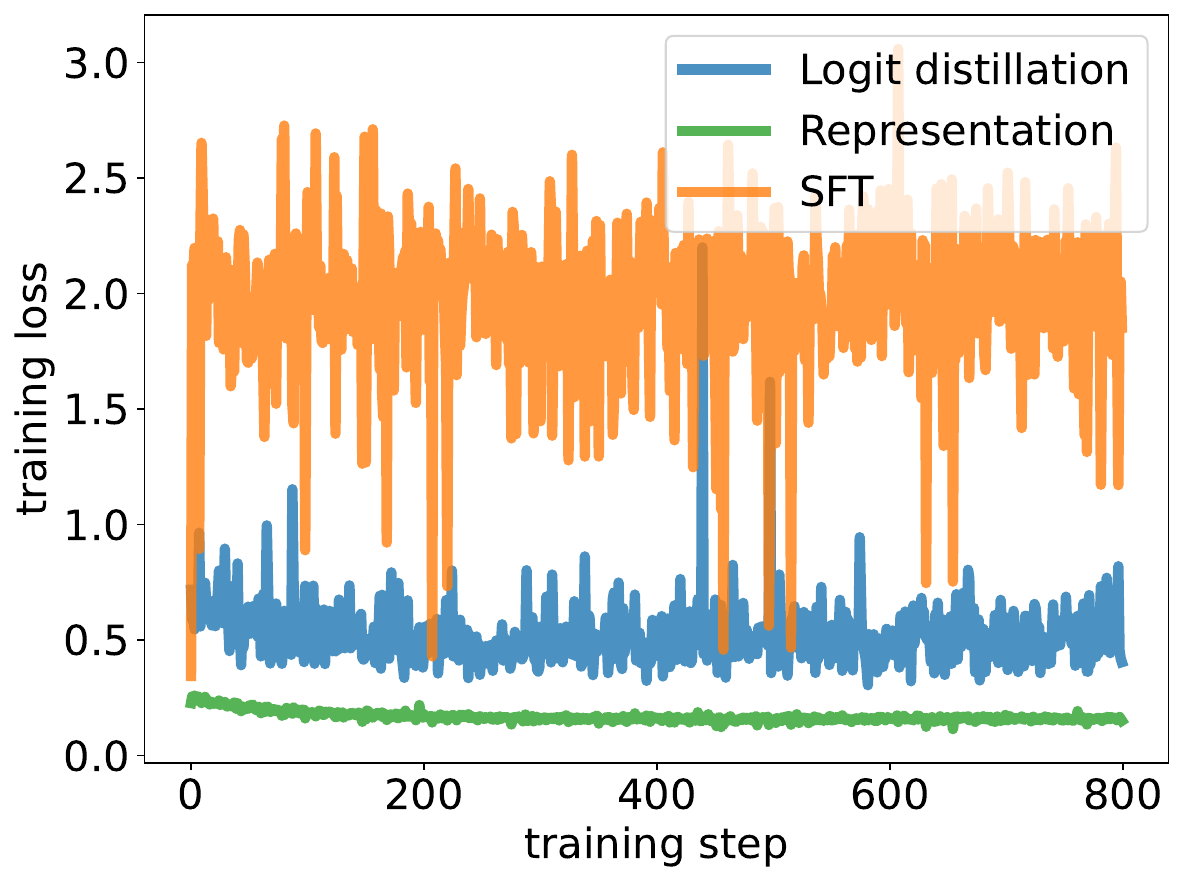}
    }
    \subfloat{
        \includegraphics[width=0.245\textwidth]{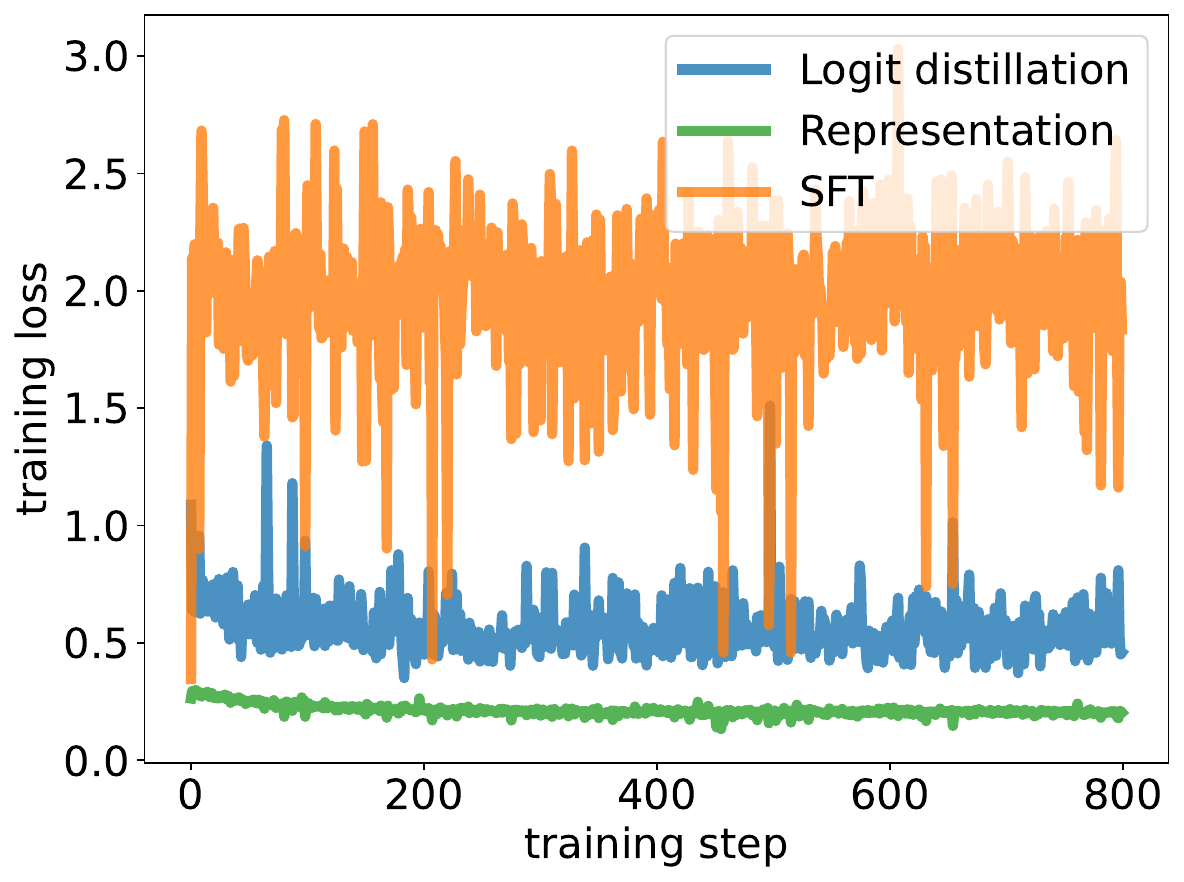}
    }
    \subfloat{
        \includegraphics[width=0.245\textwidth]{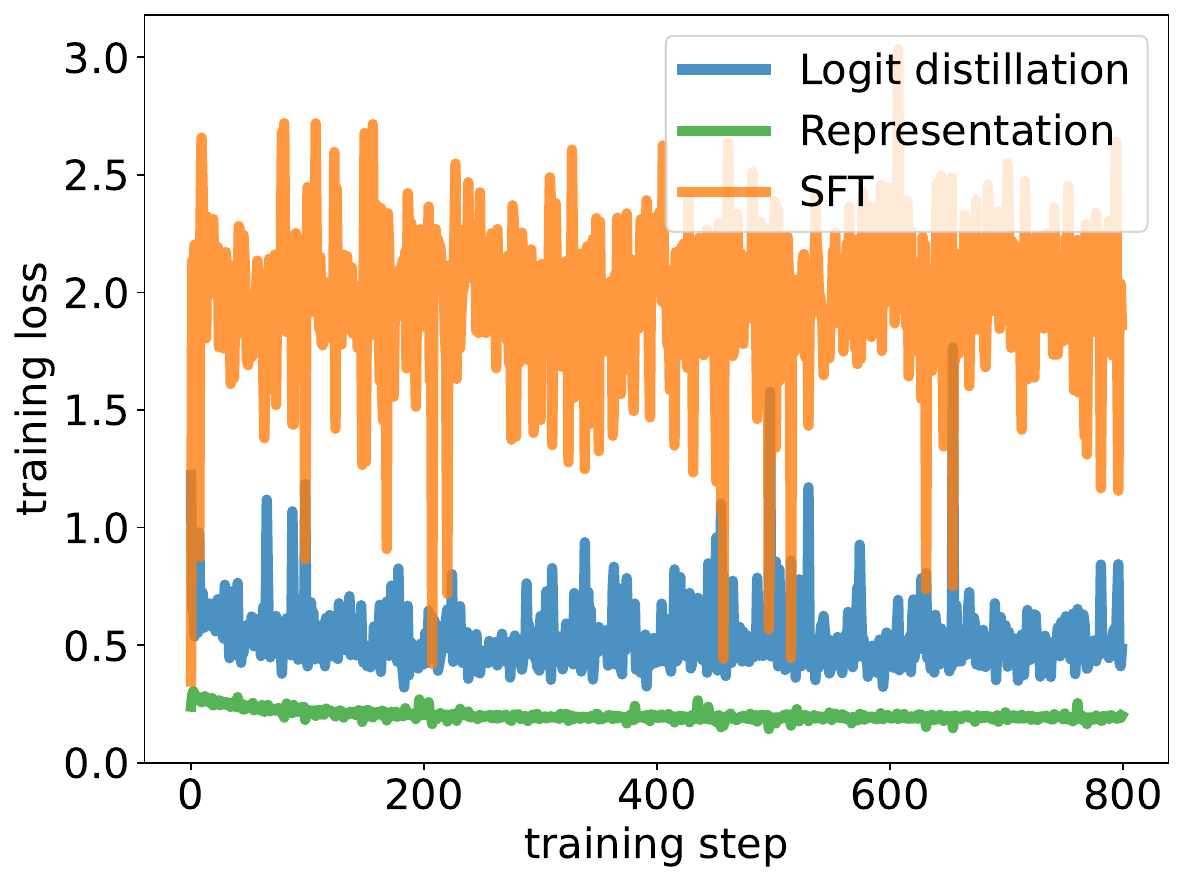}
    }

    \subfloat{
        \includegraphics[width=0.245\textwidth]{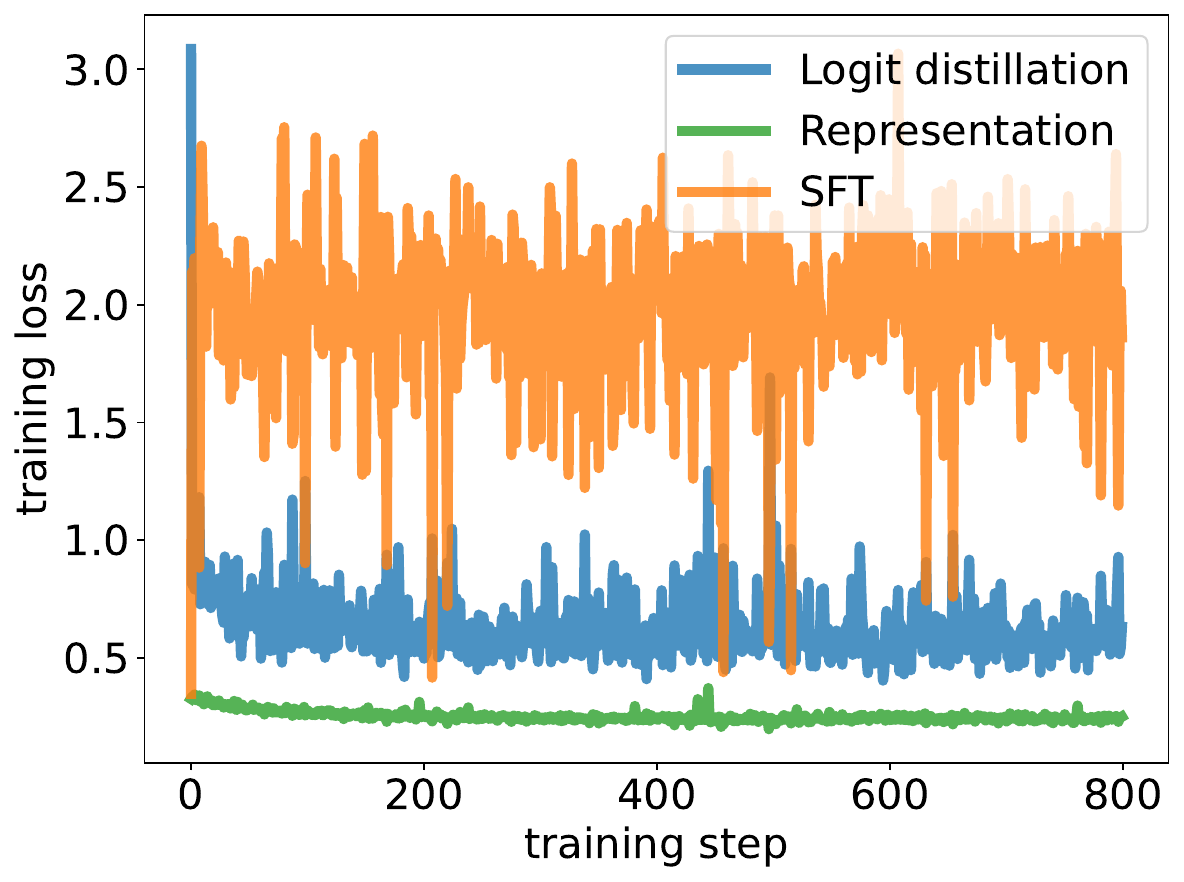}
    }
    \subfloat{
        \includegraphics[width=0.245\textwidth]{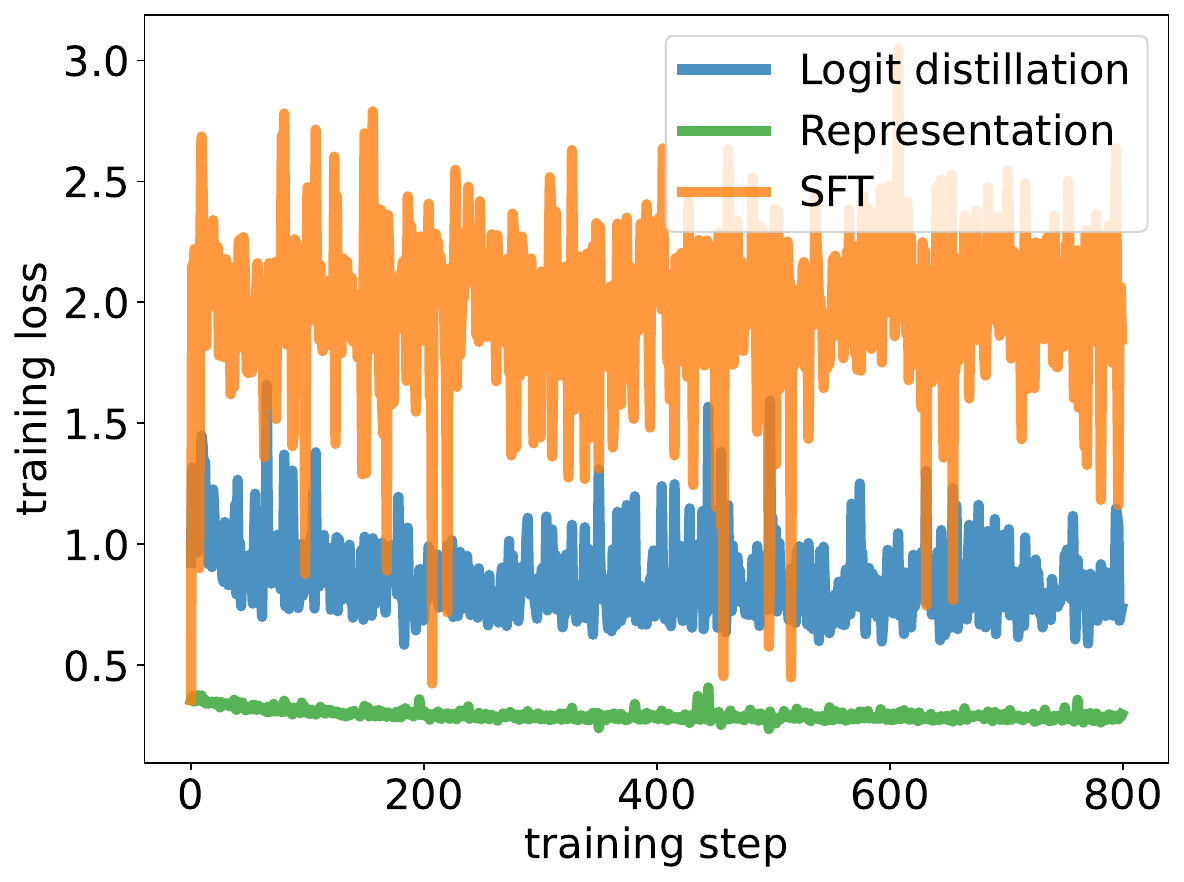}
    }
    \subfloat{
        \includegraphics[width=0.245\textwidth]{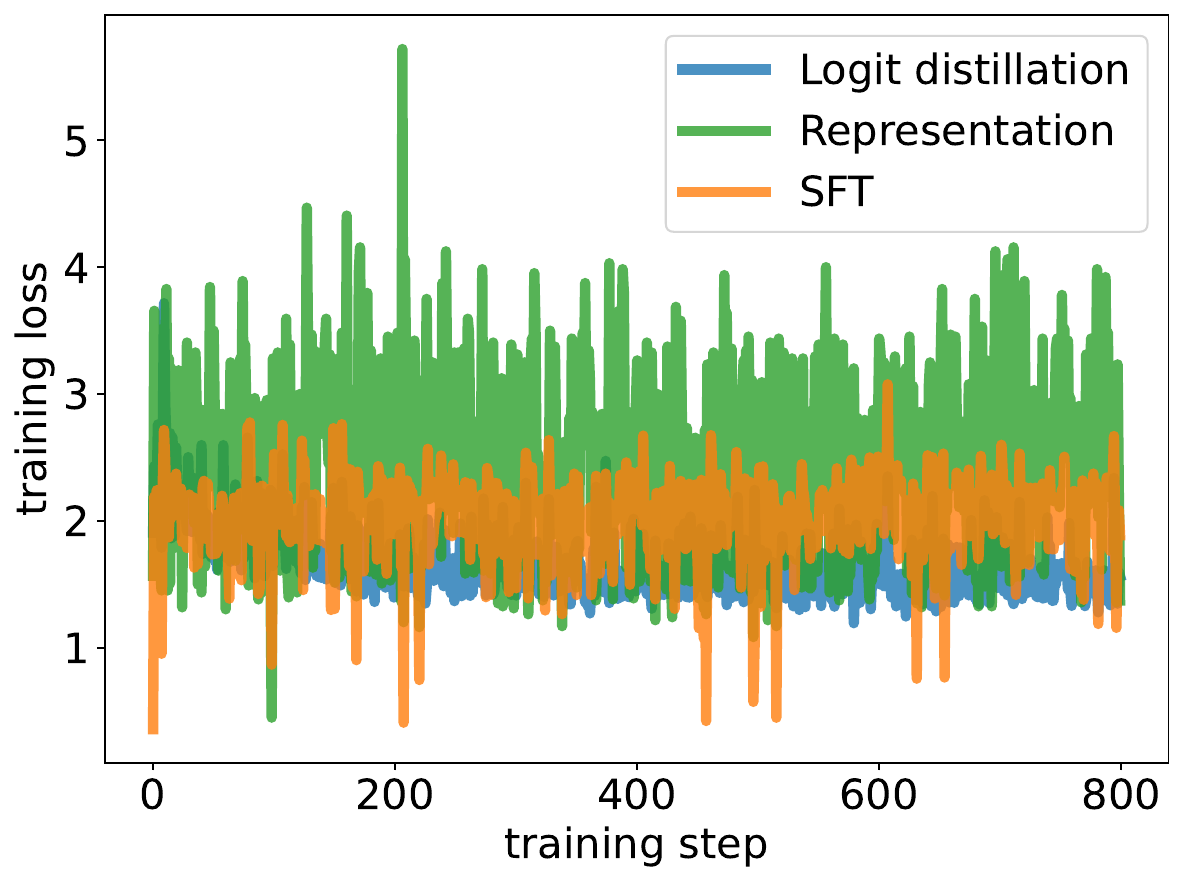}
    }
    \subfloat{
        \includegraphics[width=0.245\textwidth]{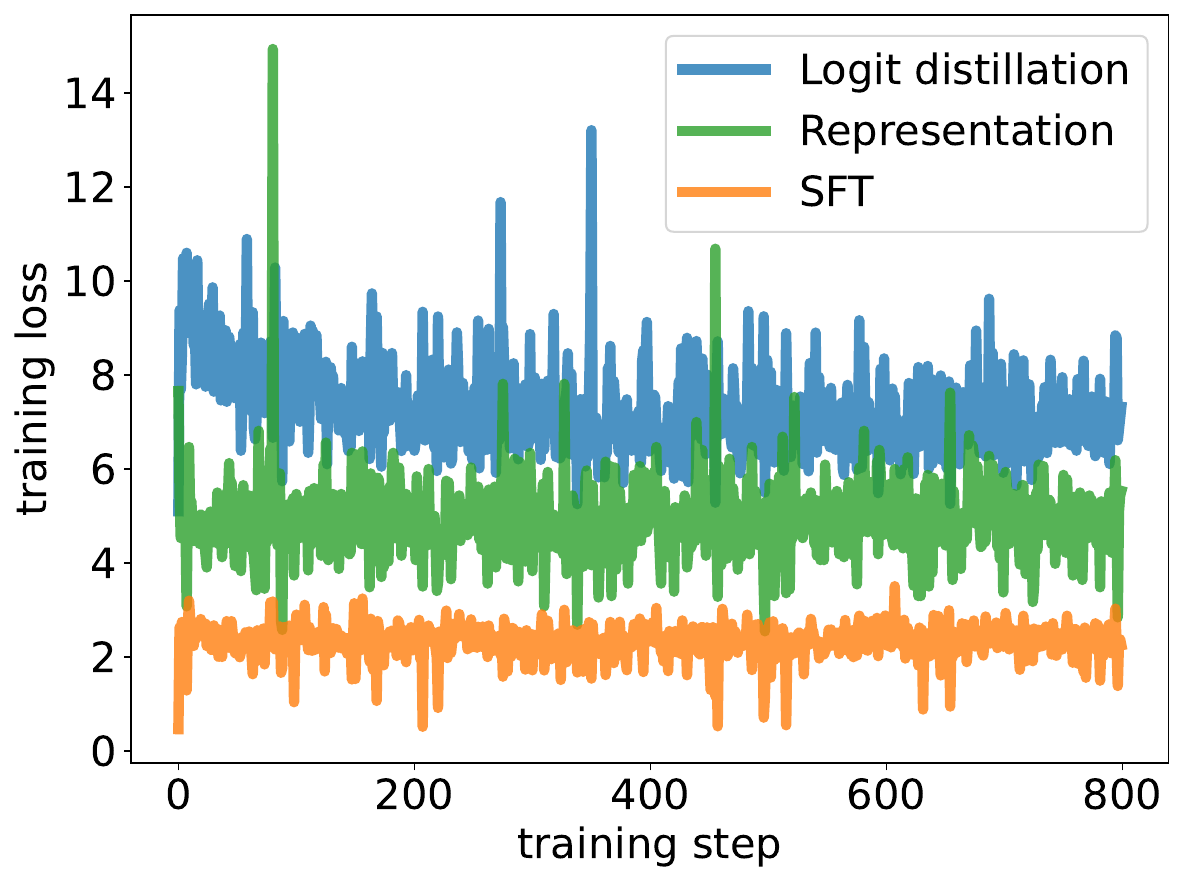}
    }

    \caption{\textbf{Low-rank linear adapter training loss curves for the last 8 LLaMa-2 7b blocks with a rank of 8} trained using three different objectives including (a) MSE loss defined on the representation, (b) supervised fine-tuning (SFT), and (c) logit distillation where logits are distilled from the full model. The first set of blocks are visualized in Fig.~\ref{fig:linear_adapters_rank_8_llama2_train_loss_a}.}
    \label{fig:linear_adapters_rank_8_llama2_train_loss_b}
\end{figure}

The loss curves for the training of the low-rank adapter with a rank of 8 on LLaMa-2 are visualized in Fig.~\ref{fig:linear_adapters_rank_8_llama2_train_loss_a} and Fig.~\ref{fig:linear_adapters_rank_8_llama2_train_loss_b}respectively.

\begin{figure}[t]
    \centering
    \subfloat{
        \includegraphics[width=0.245\textwidth]{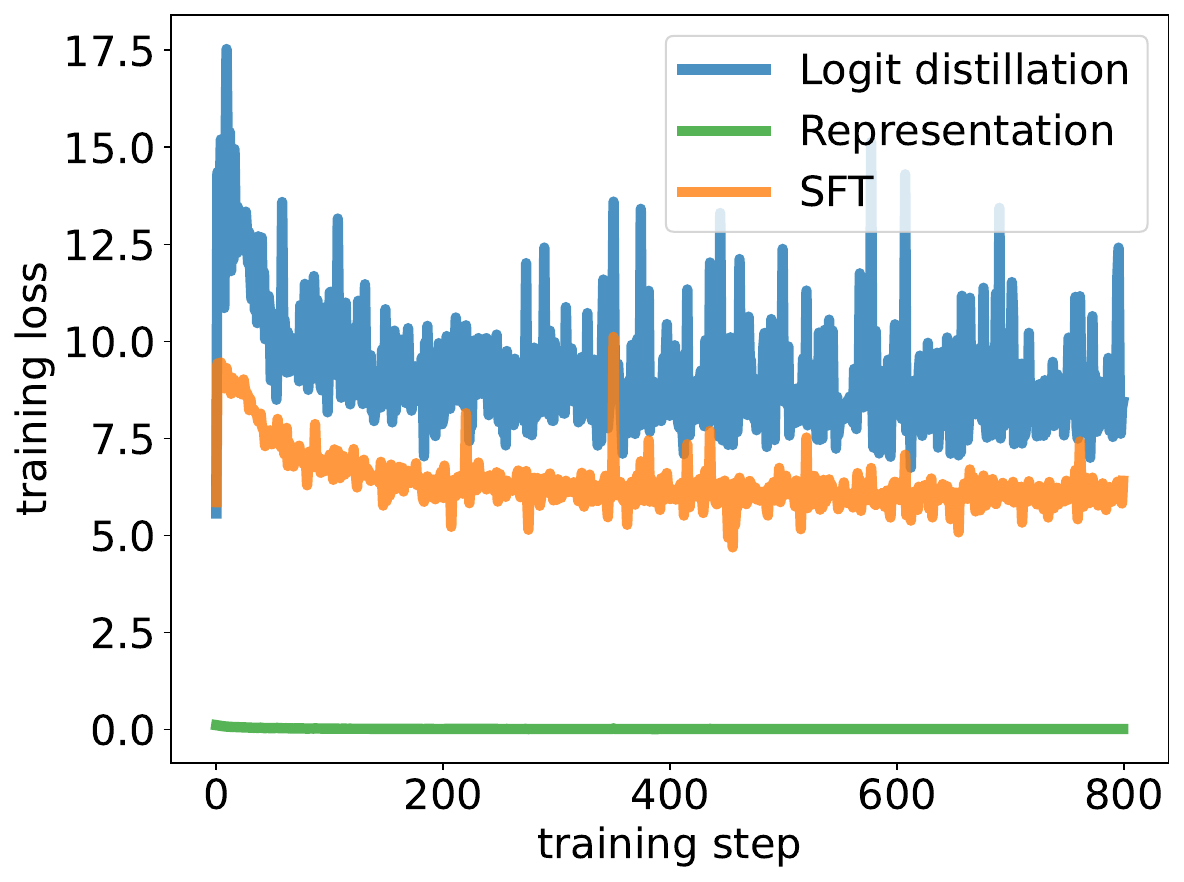}
    }
    \subfloat{
        \includegraphics[width=0.245\textwidth]{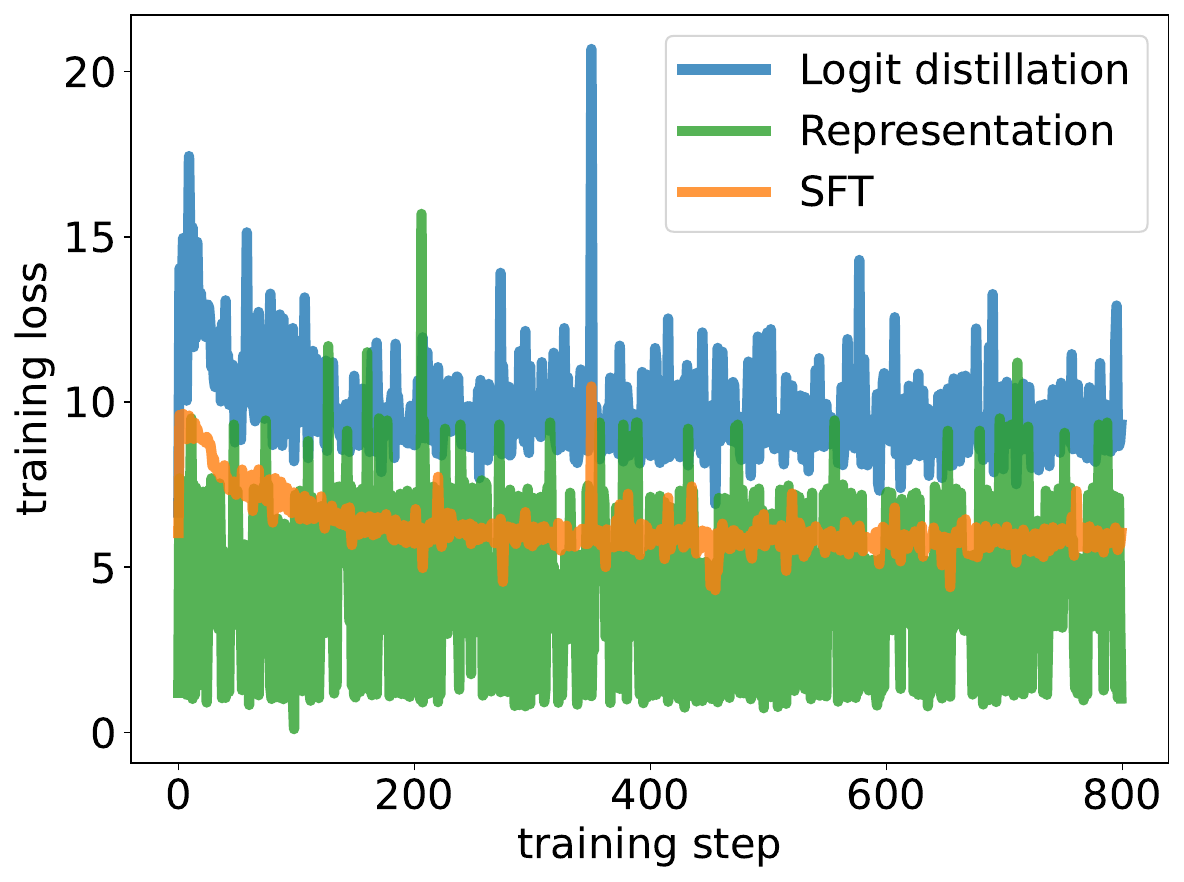}
    }
    \subfloat{
        \includegraphics[width=0.245\textwidth]{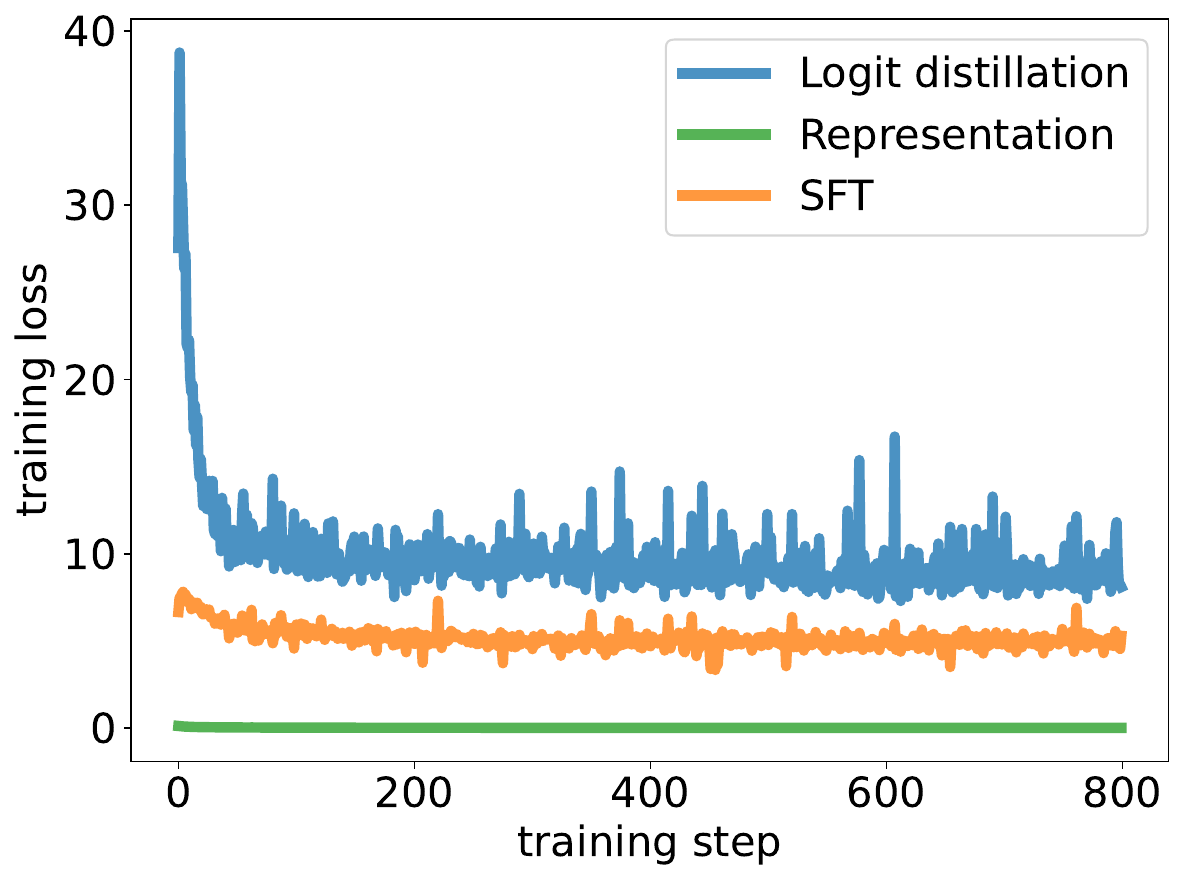}
    }
    \subfloat{
        \includegraphics[width=0.245\textwidth]{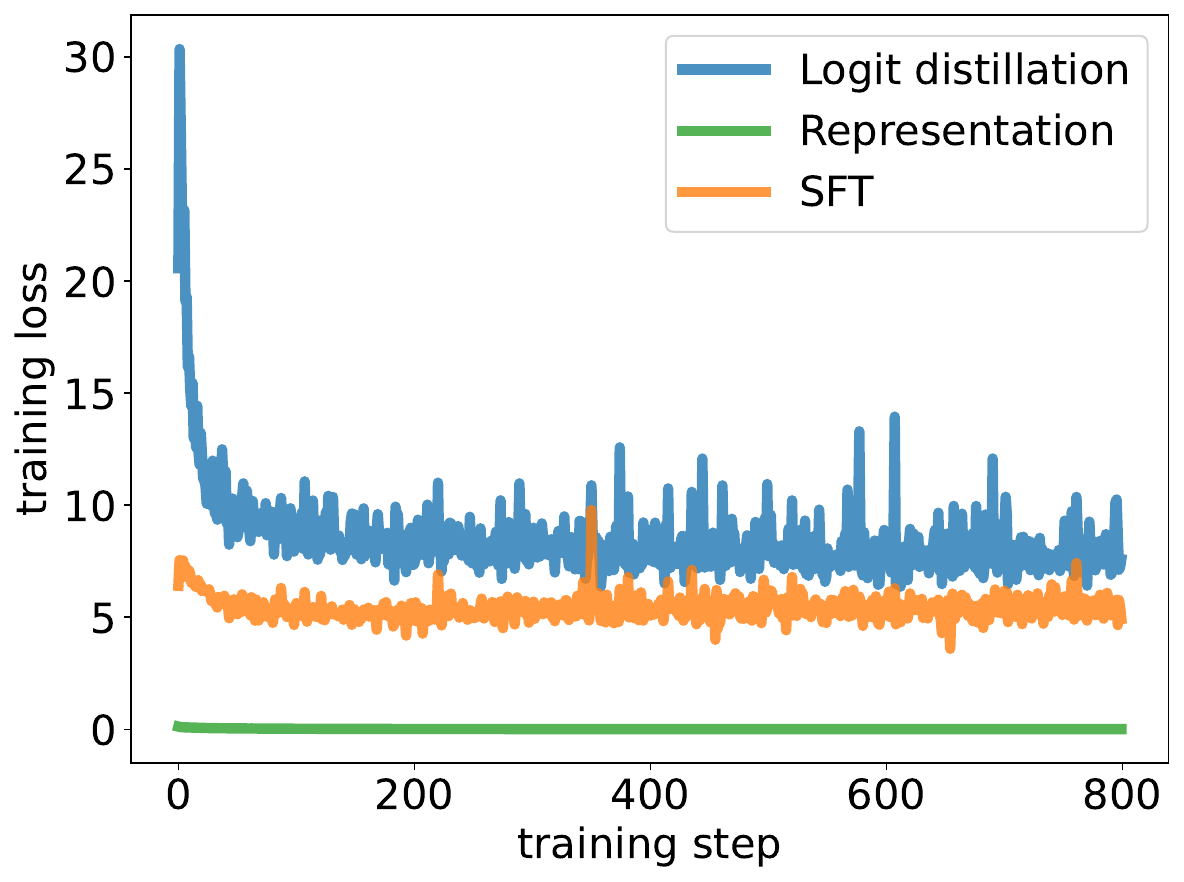}
    }

    \subfloat{
        \includegraphics[width=0.245\textwidth]{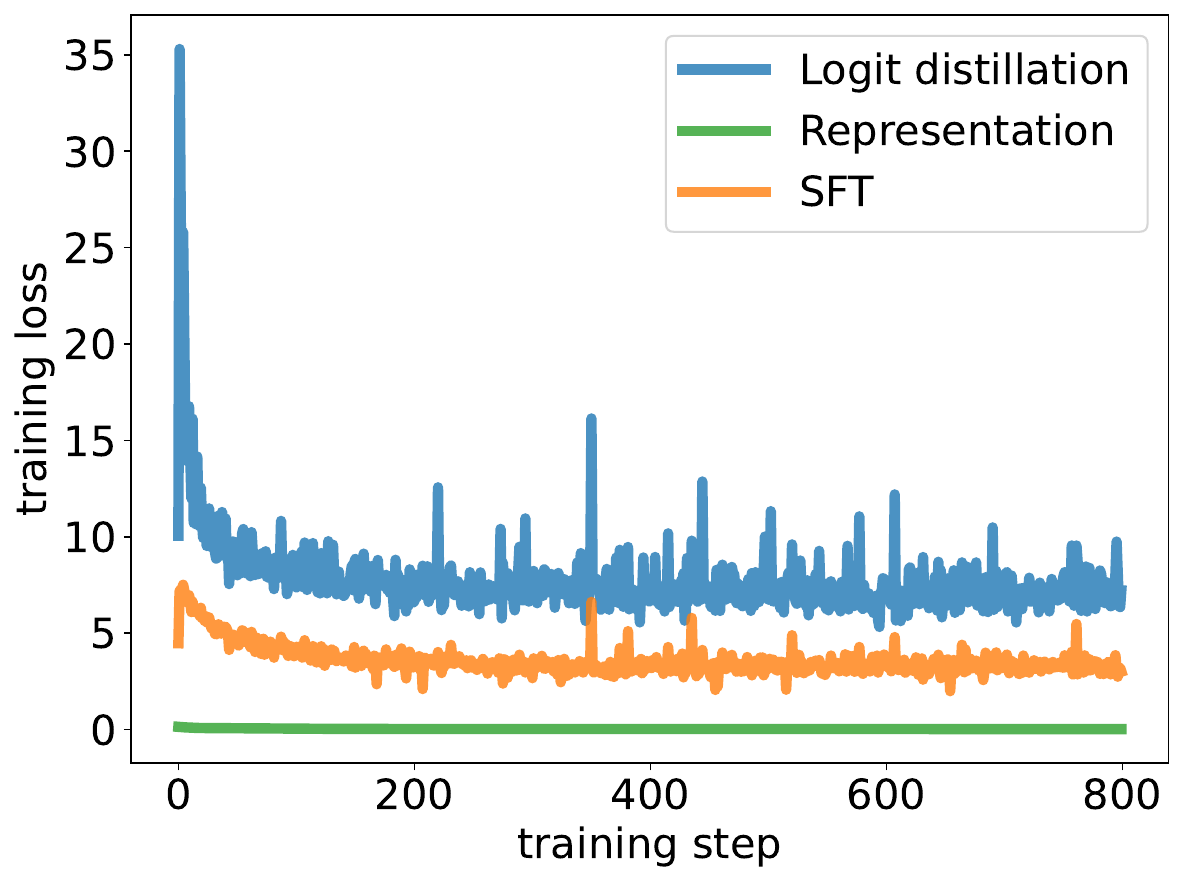}
    }
    \subfloat{
        \includegraphics[width=0.245\textwidth]{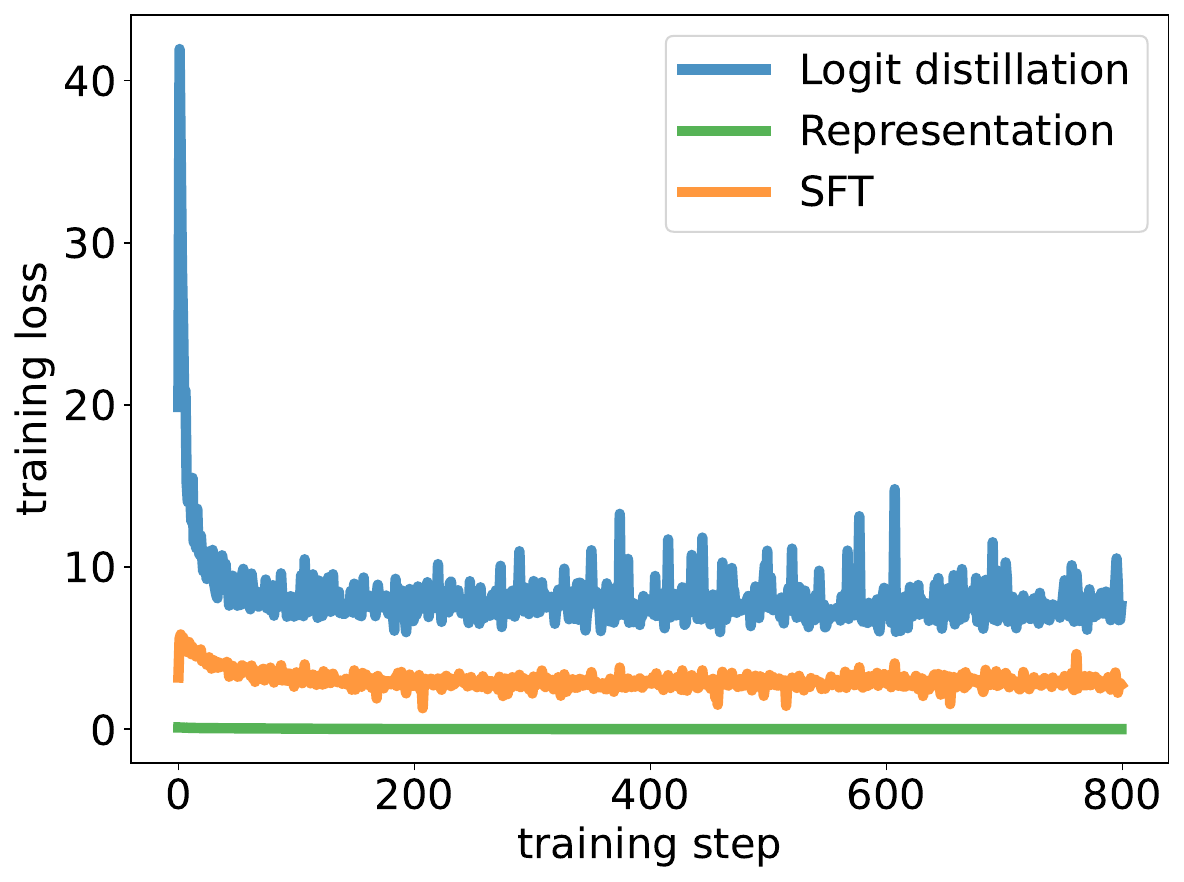}
    }
    \subfloat{
        \includegraphics[width=0.245\textwidth]{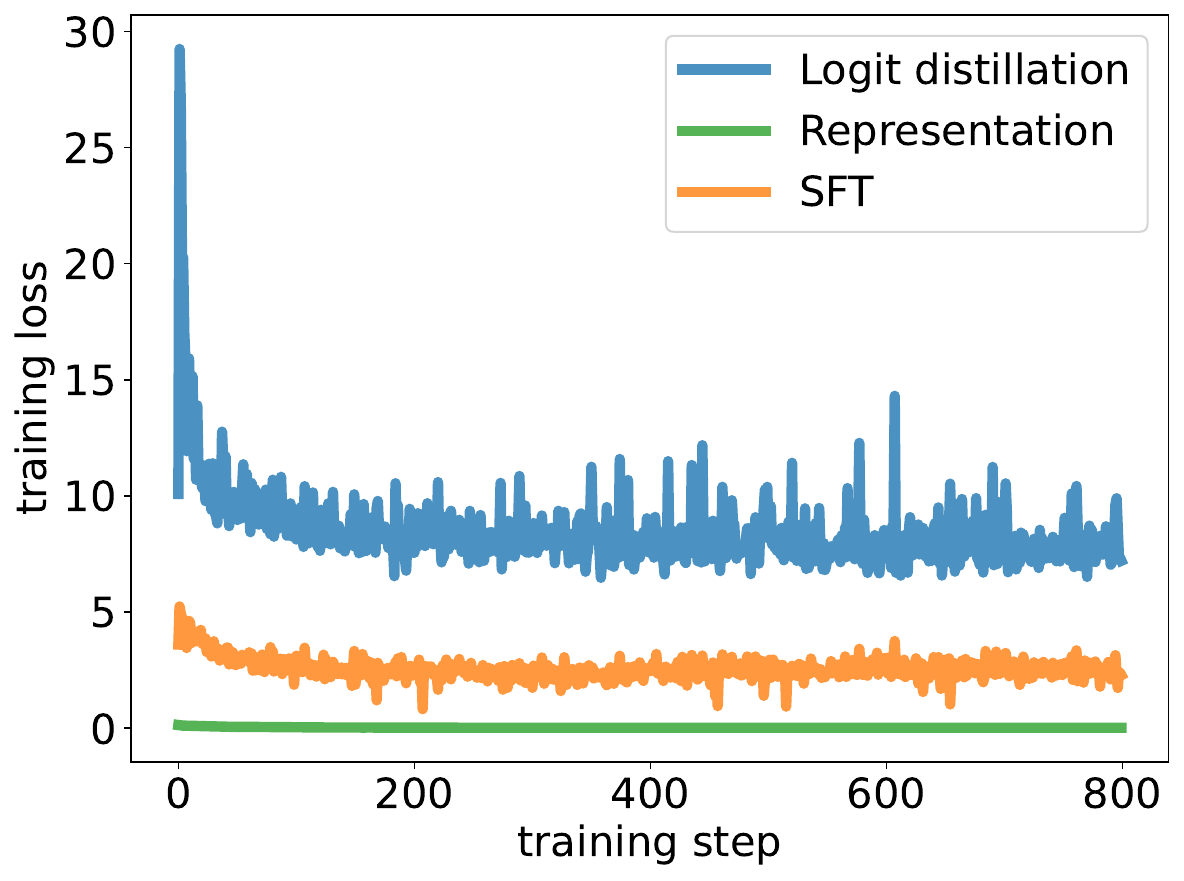}
    }
    \subfloat{
        \includegraphics[width=0.245\textwidth]{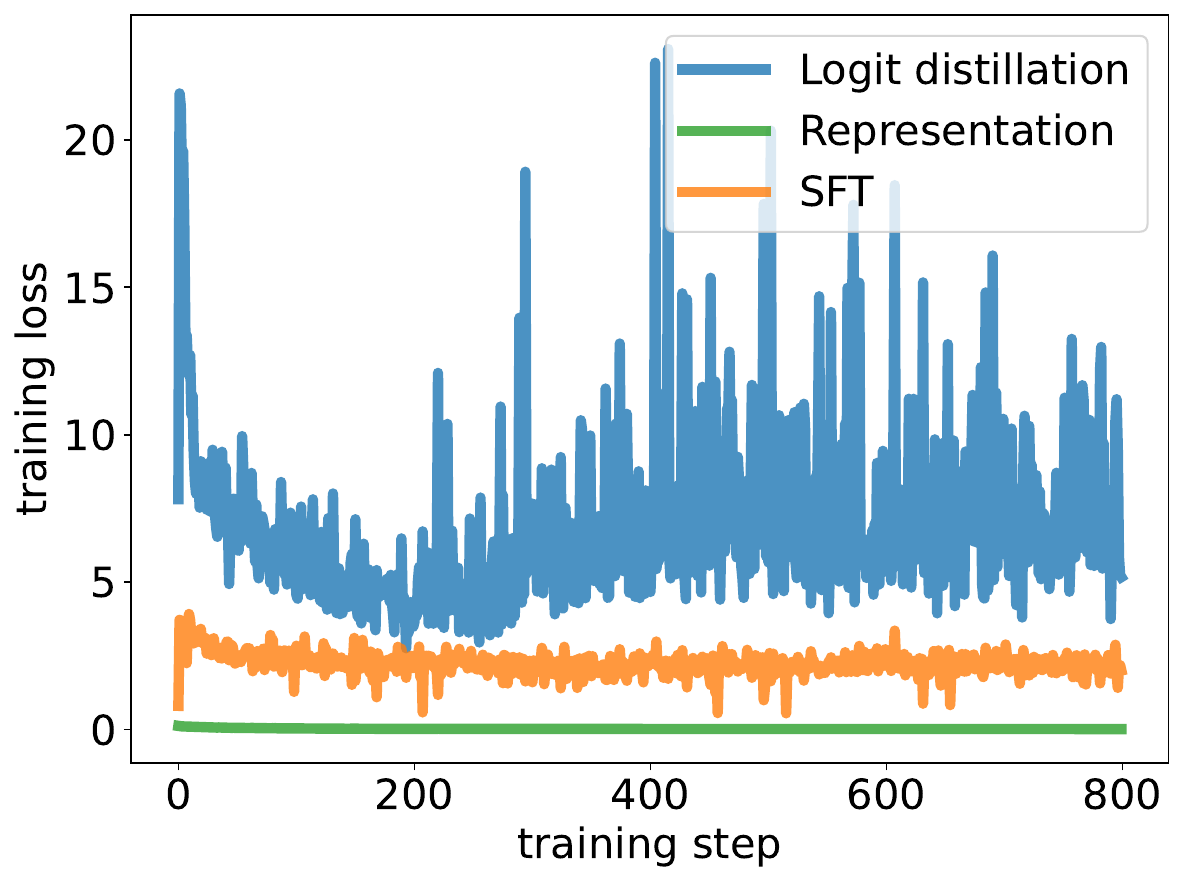}
    }

    \subfloat{
        \includegraphics[width=0.245\textwidth]{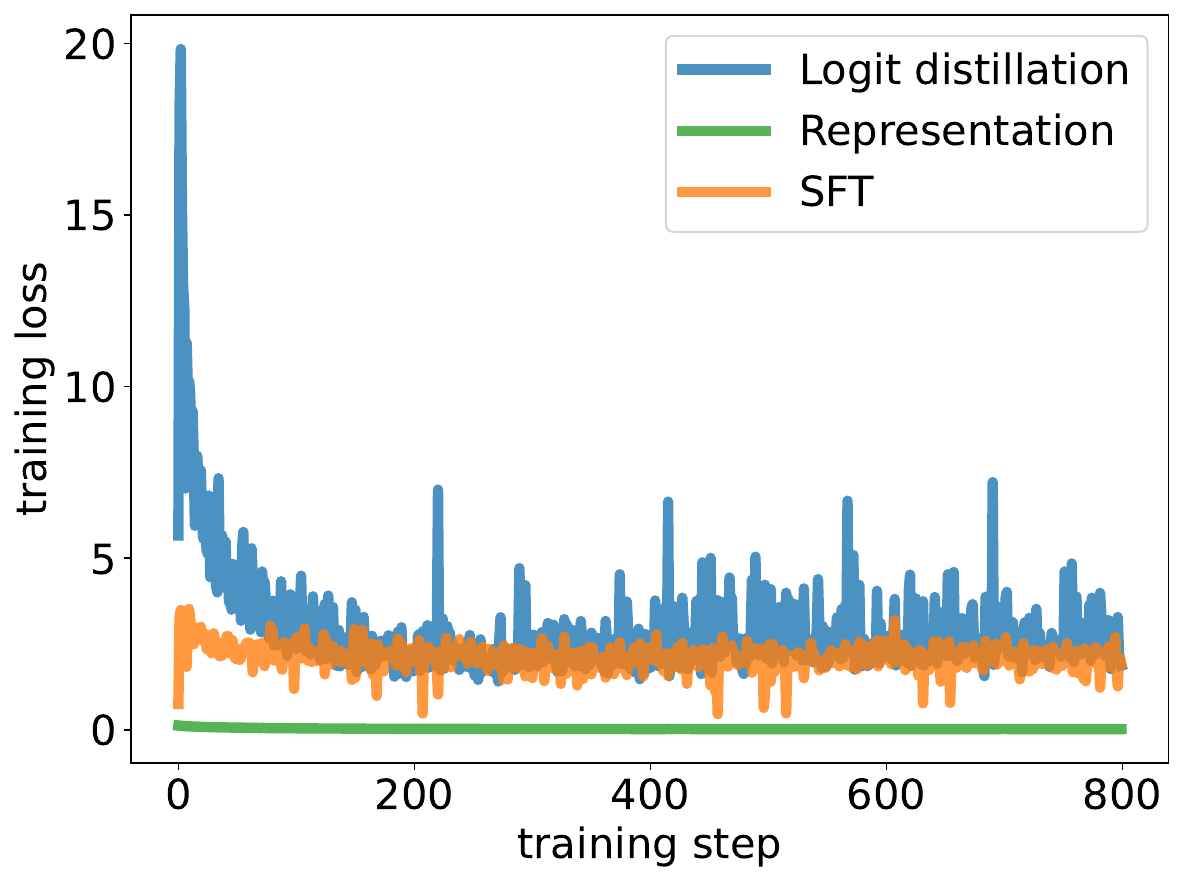}
    }
    \subfloat{
        \includegraphics[width=0.245\textwidth]{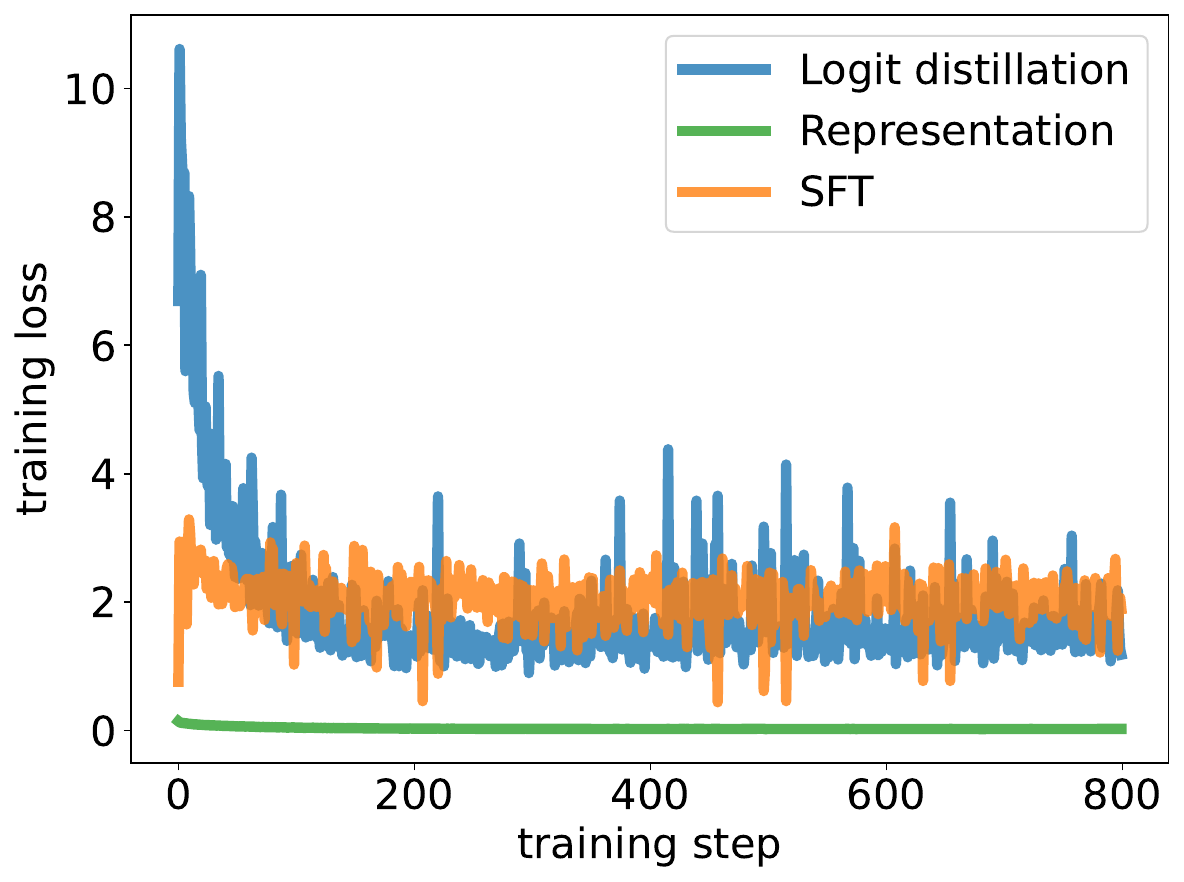}
    }
    \subfloat{
        \includegraphics[width=0.245\textwidth]{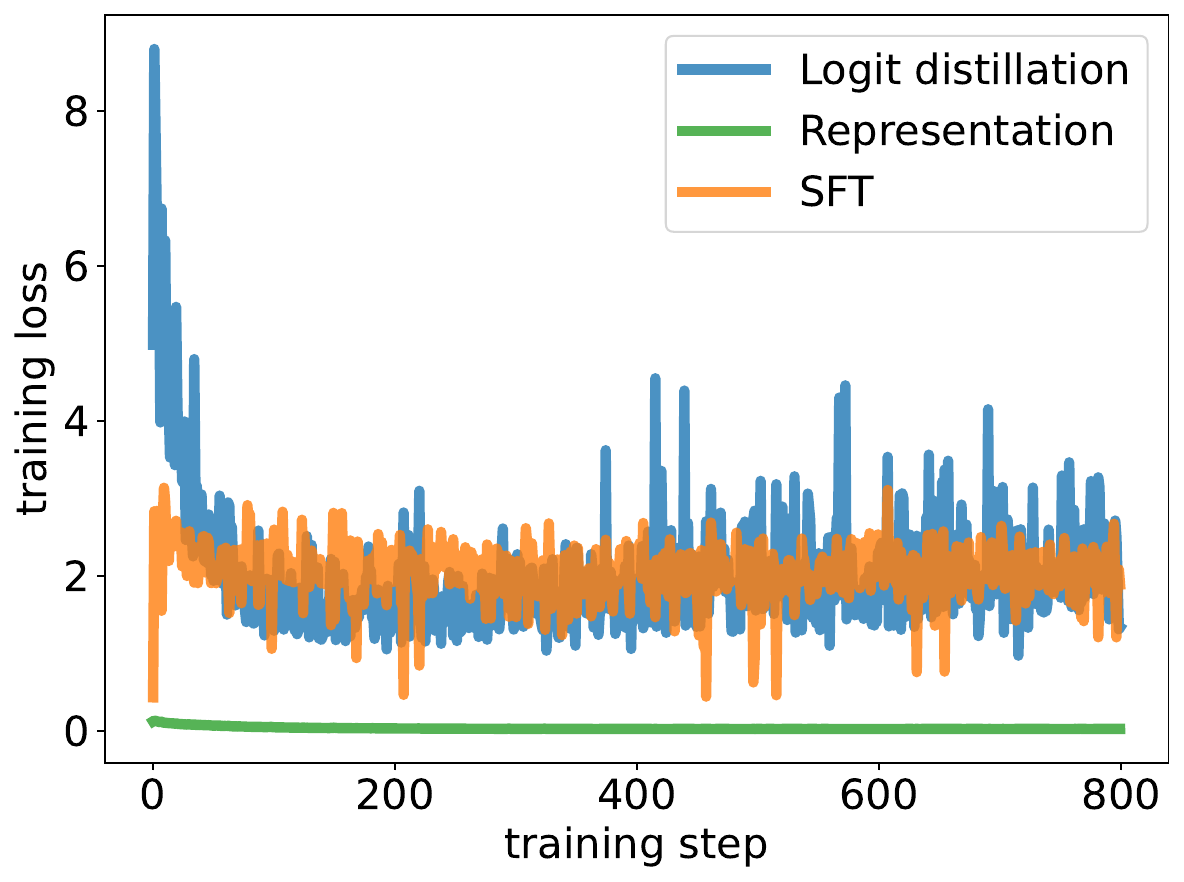}
    }
    \subfloat{
        \includegraphics[width=0.245\textwidth]{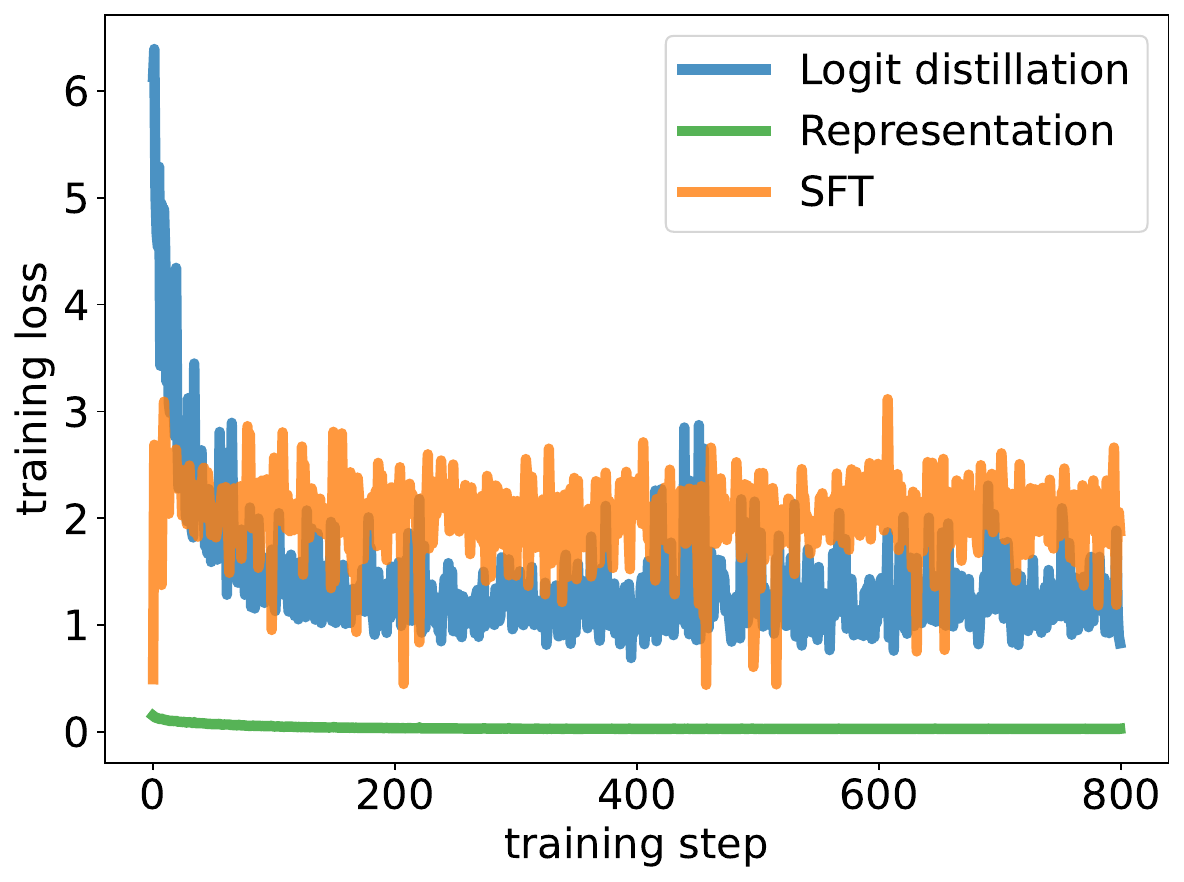}
    }

    \subfloat{
        \includegraphics[width=0.245\textwidth]{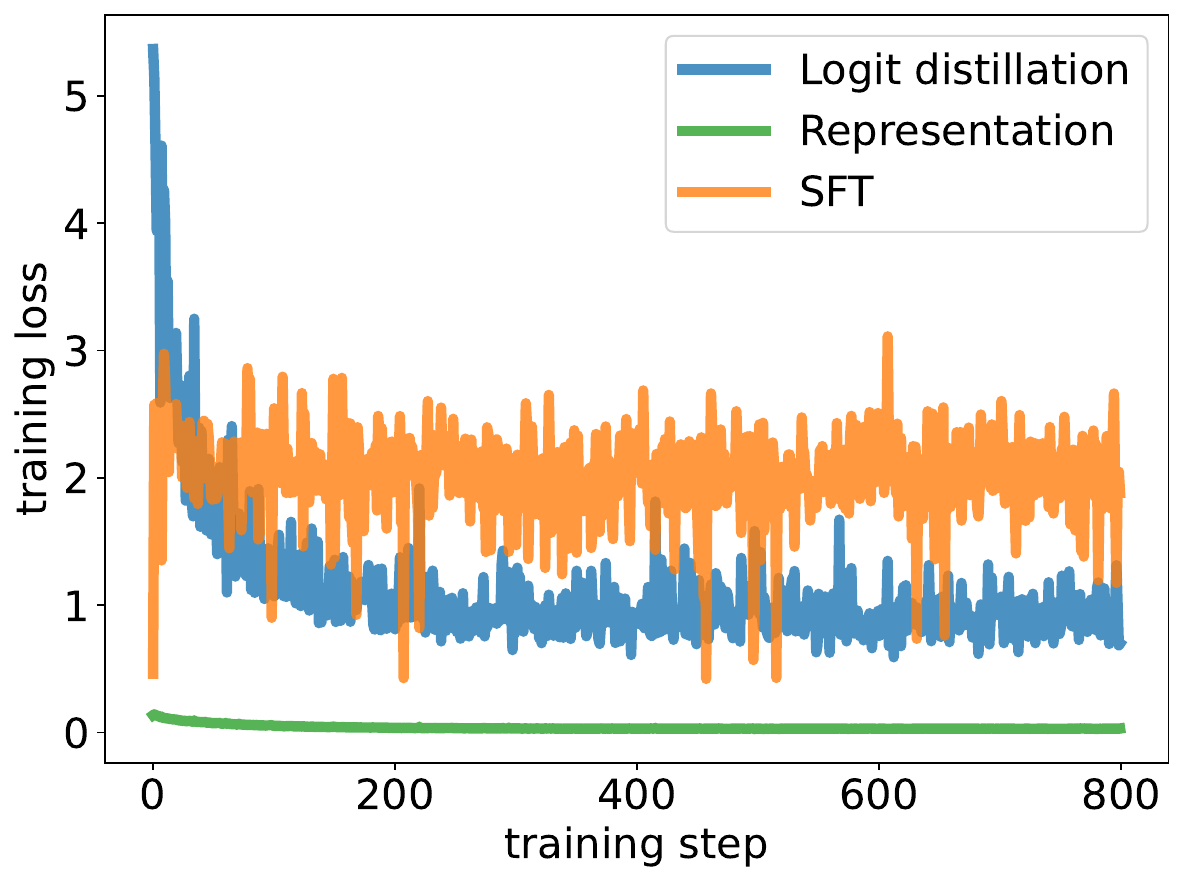}
    }
    \subfloat{
        \includegraphics[width=0.245\textwidth]{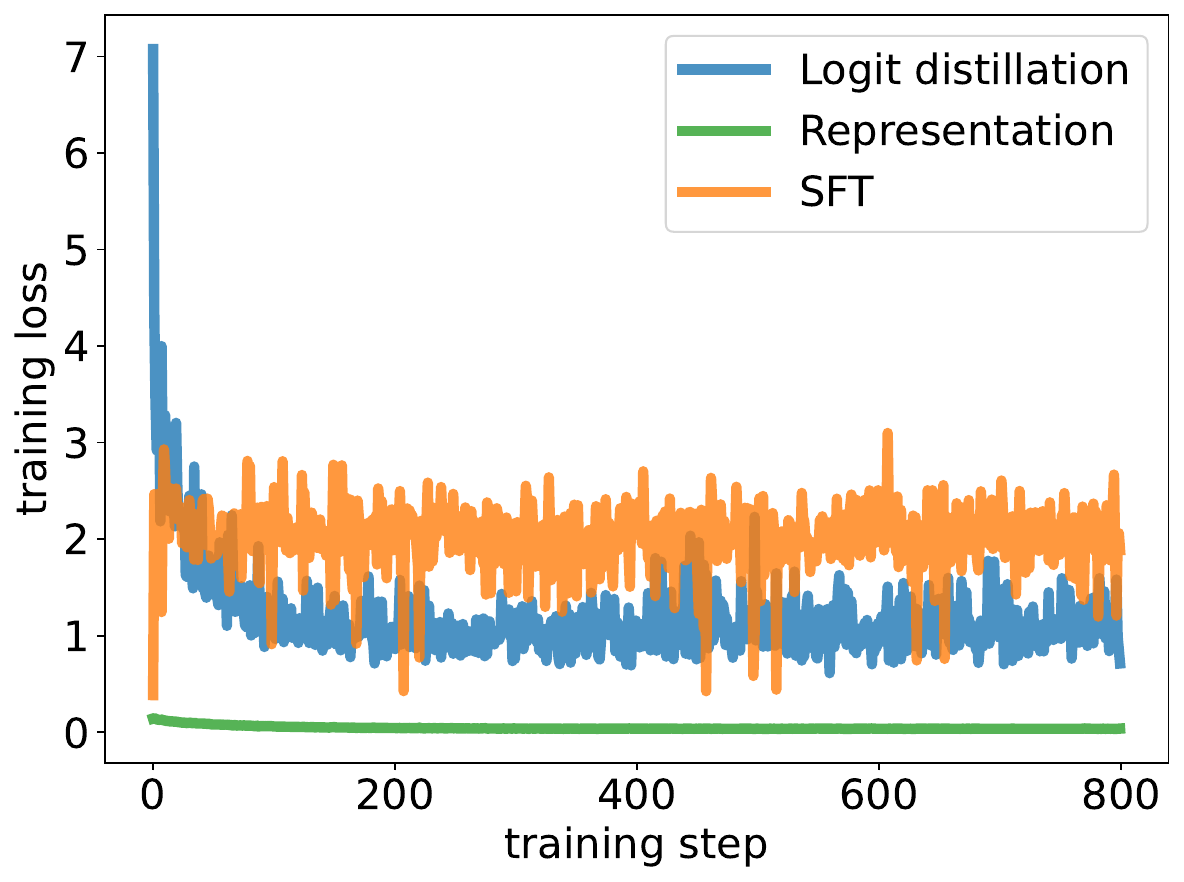}
    }
    \subfloat{
        \includegraphics[width=0.245\textwidth]{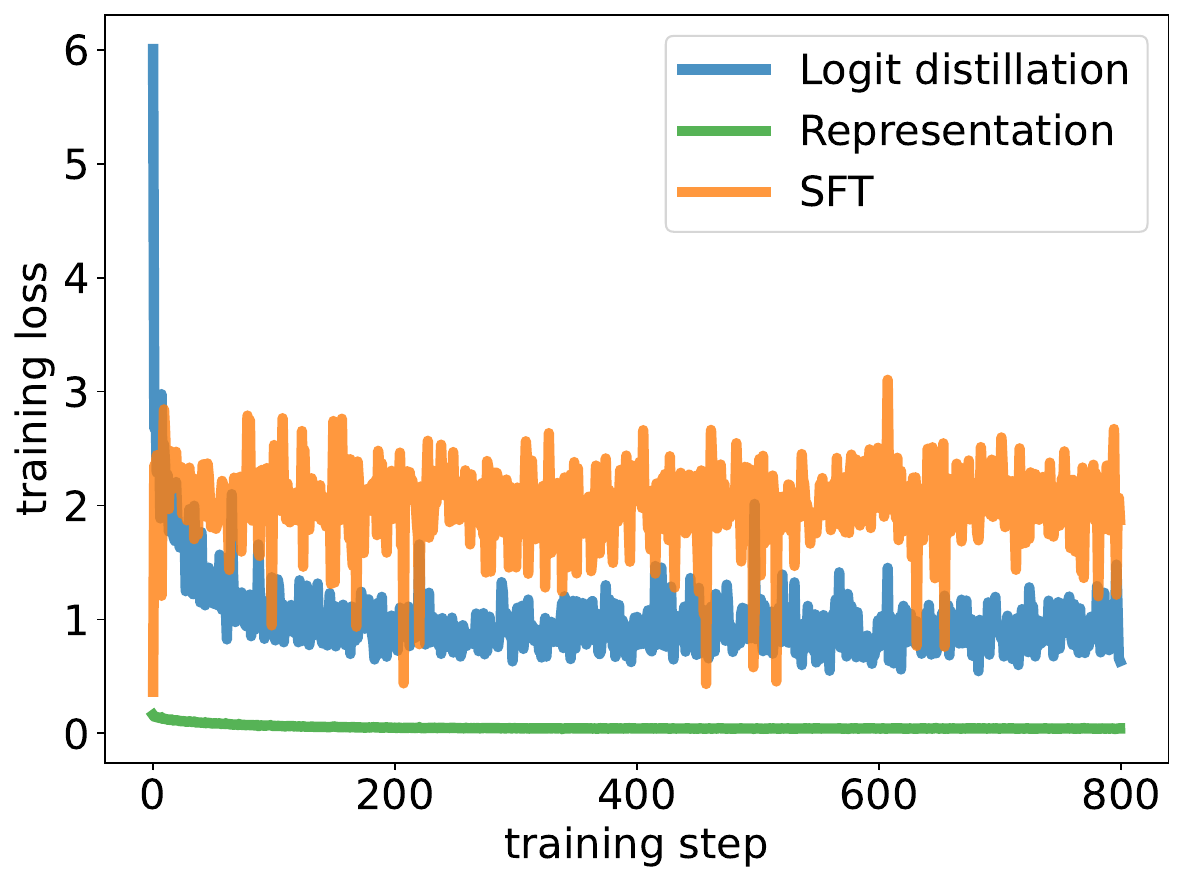}
    }
    \subfloat{
        \includegraphics[width=0.245\textwidth]{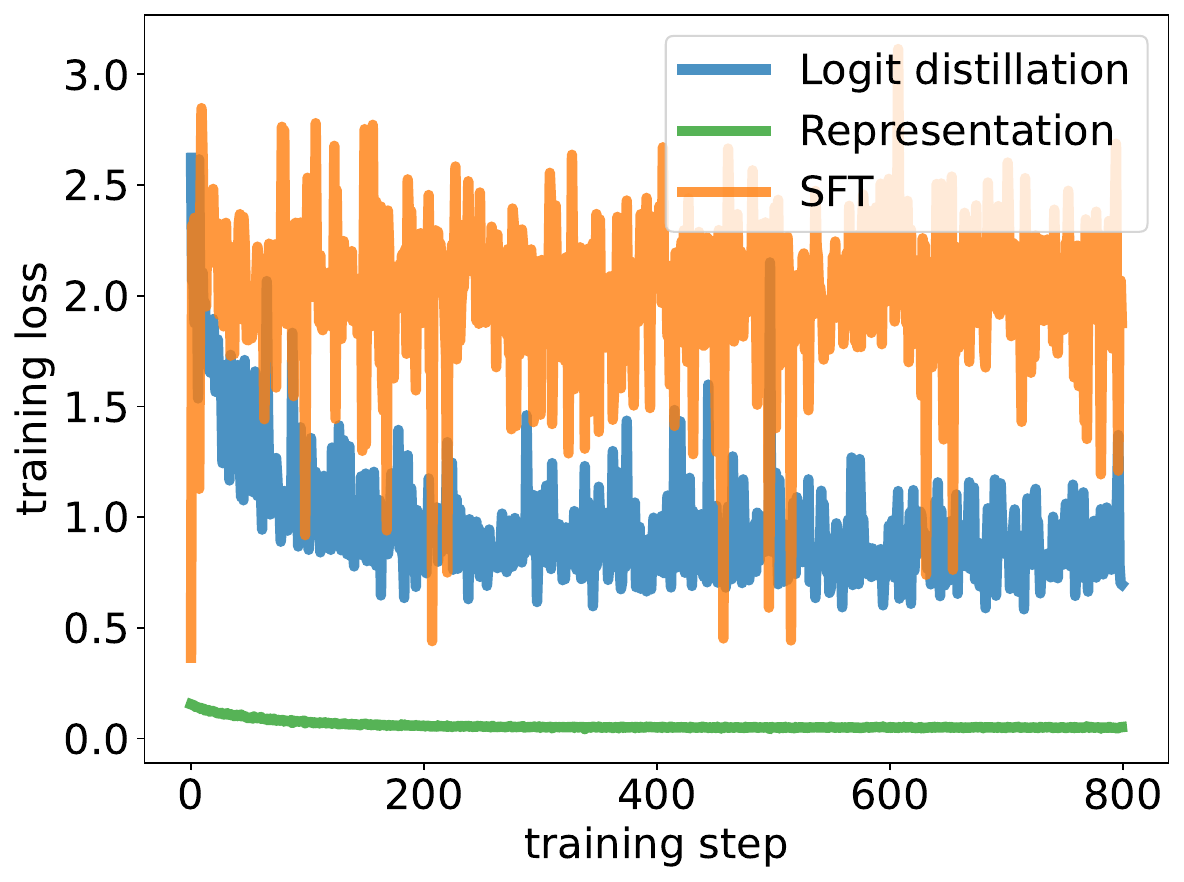}
    }

    \subfloat{
        \includegraphics[width=0.245\textwidth]{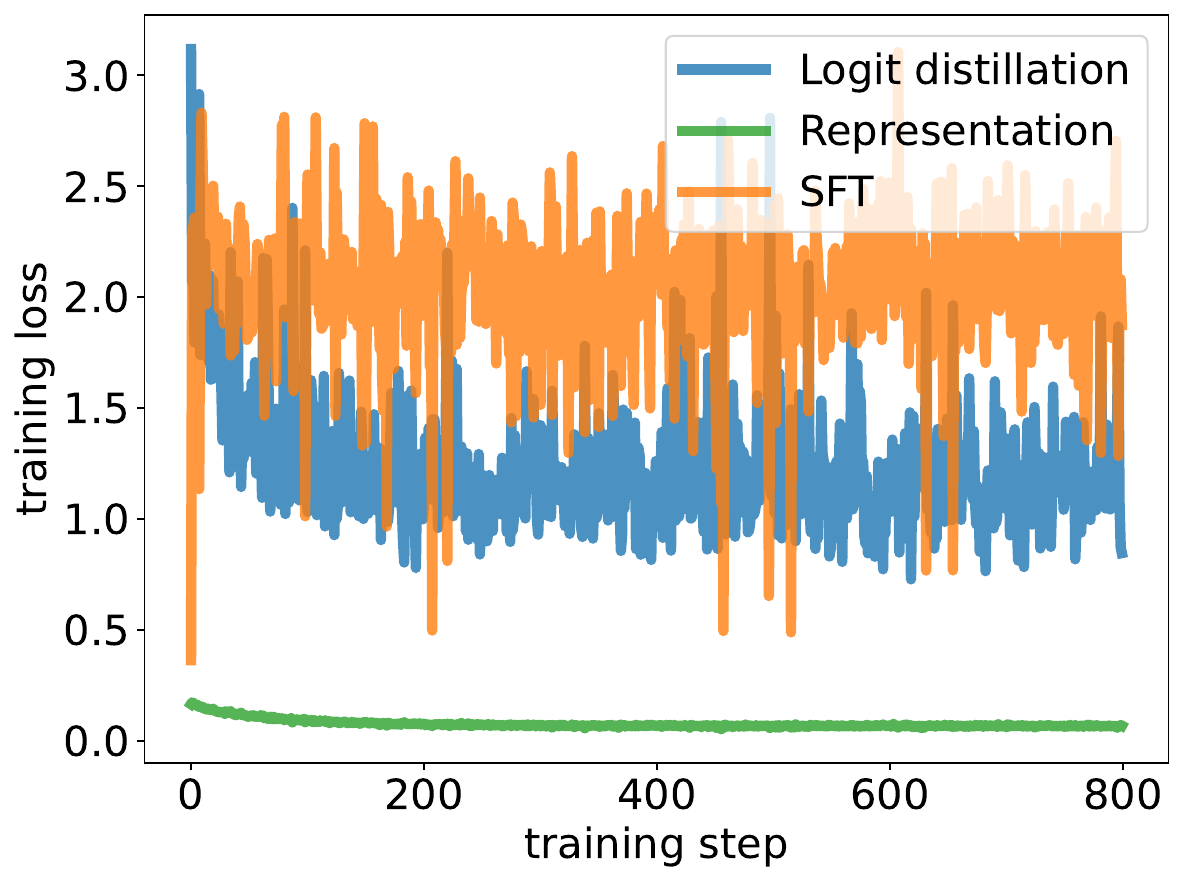}
    }
    \subfloat{
        \includegraphics[width=0.245\textwidth]{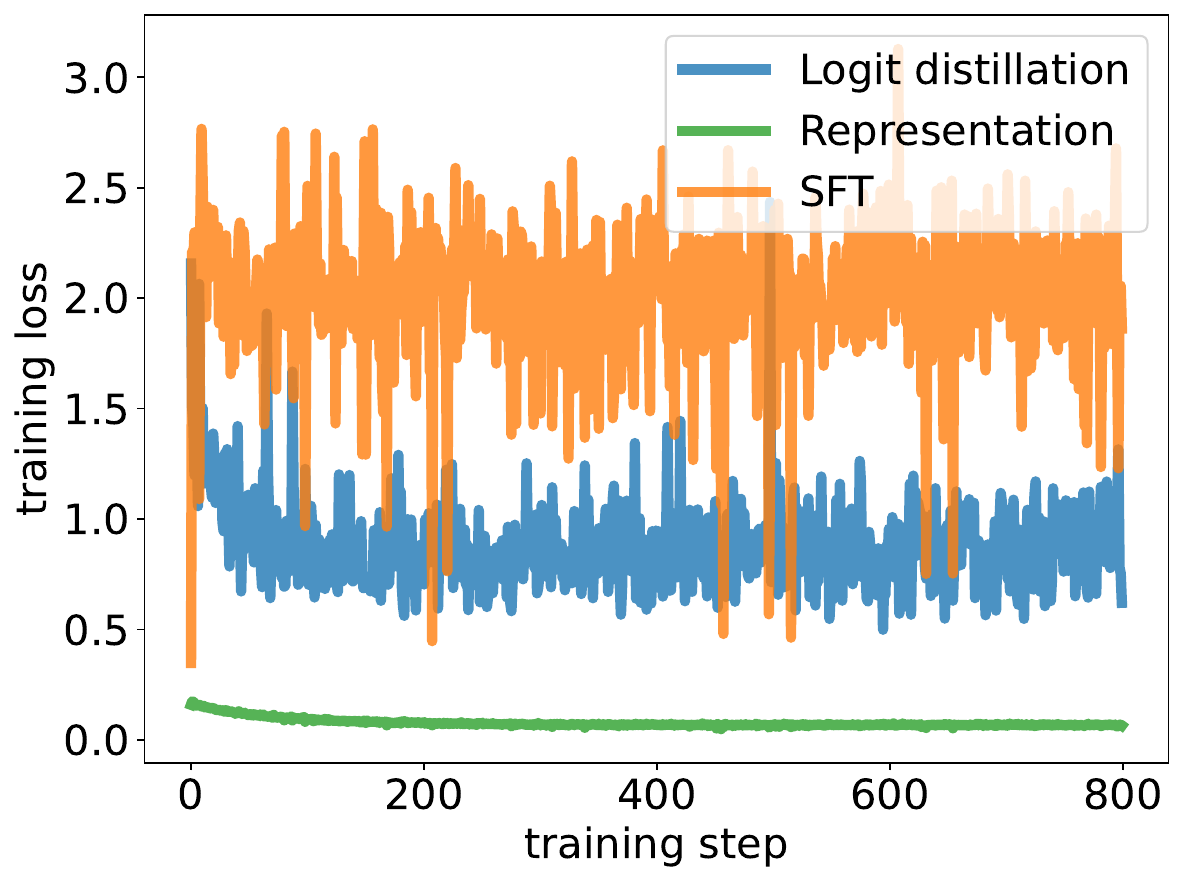}
    }
    \subfloat{
        \includegraphics[width=0.245\textwidth]{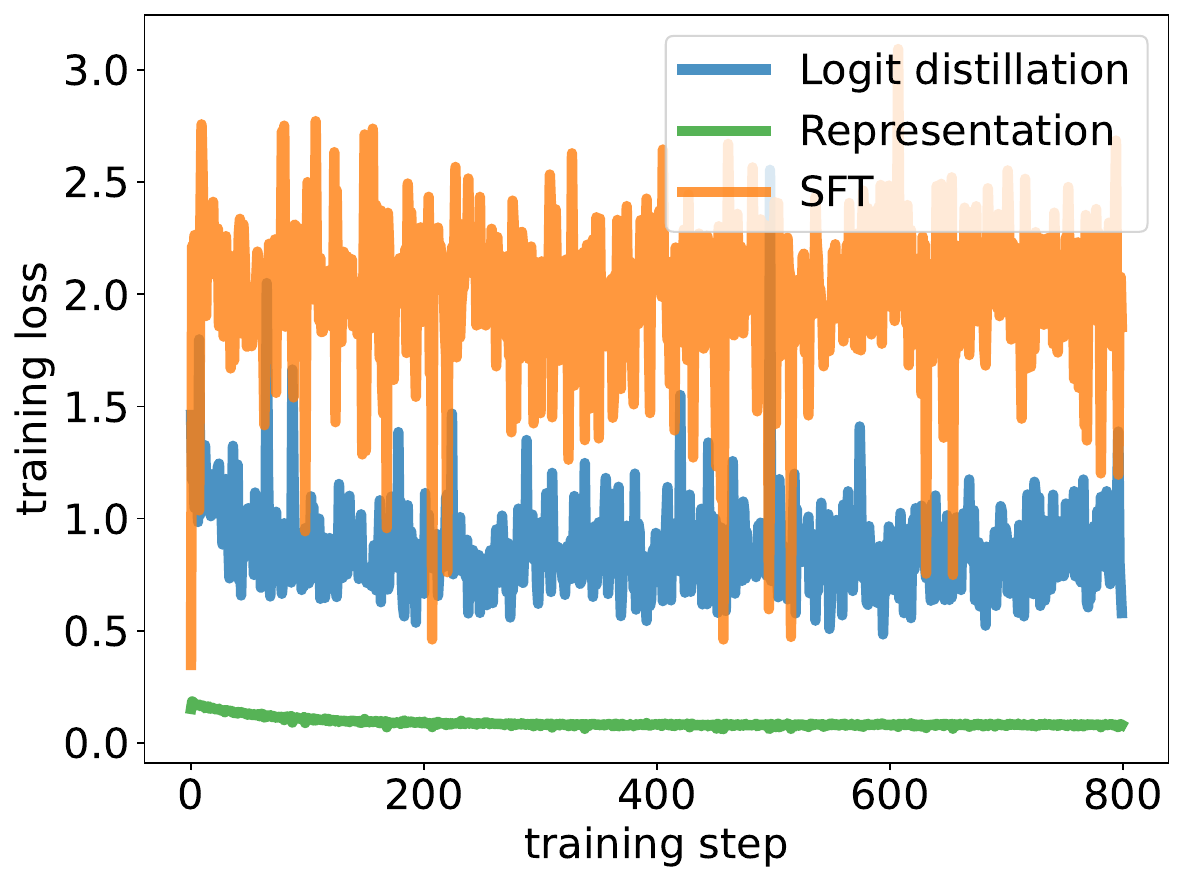}
    }
    \subfloat{
        \includegraphics[width=0.245\textwidth]{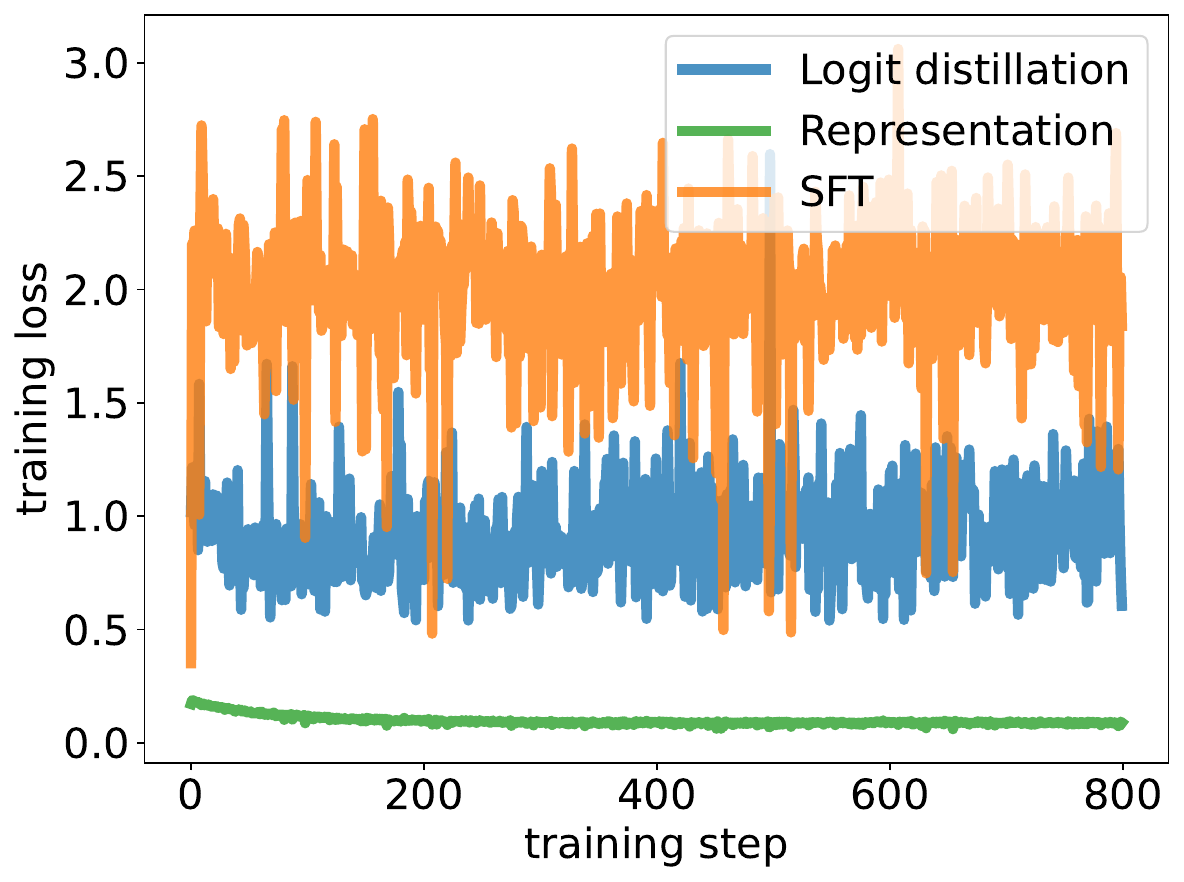}
    }

    \subfloat{
        \includegraphics[width=0.245\textwidth]{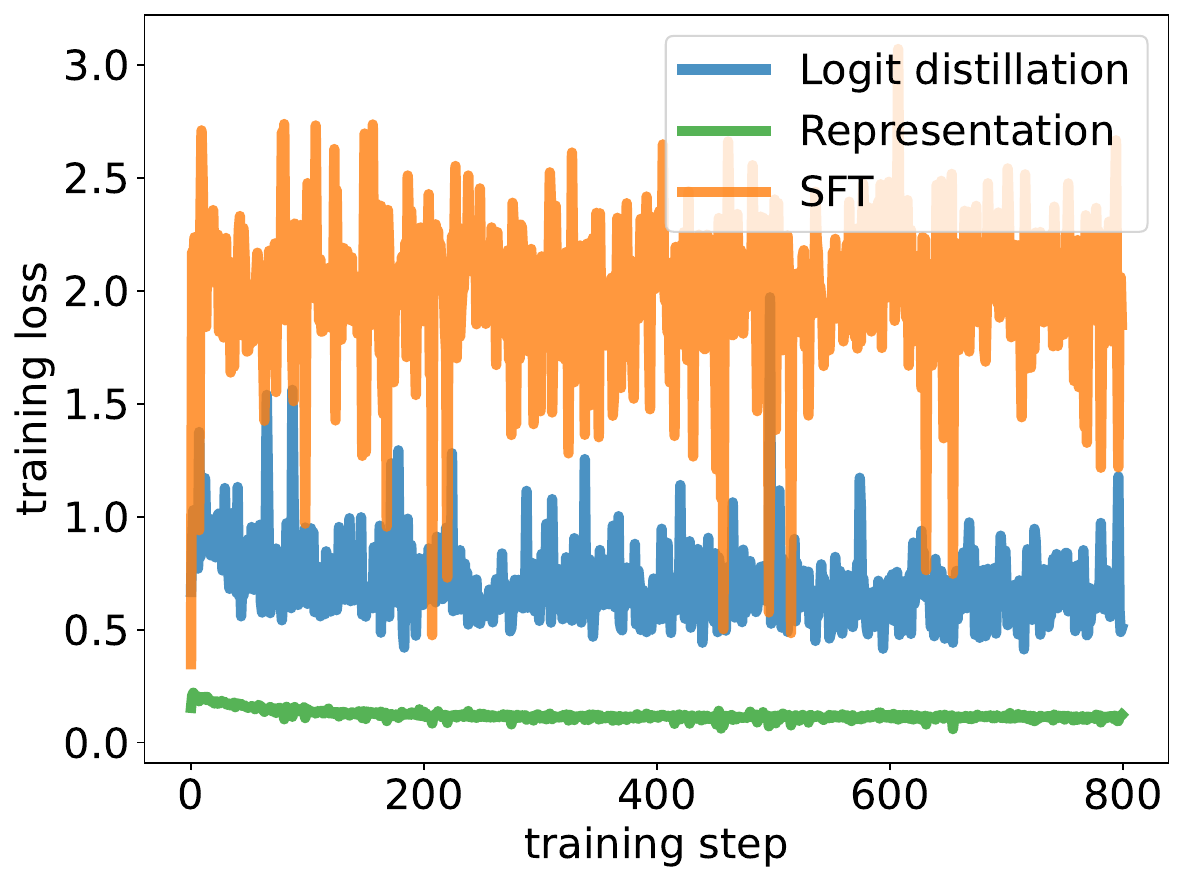}
    }
    \subfloat{
        \includegraphics[width=0.245\textwidth]{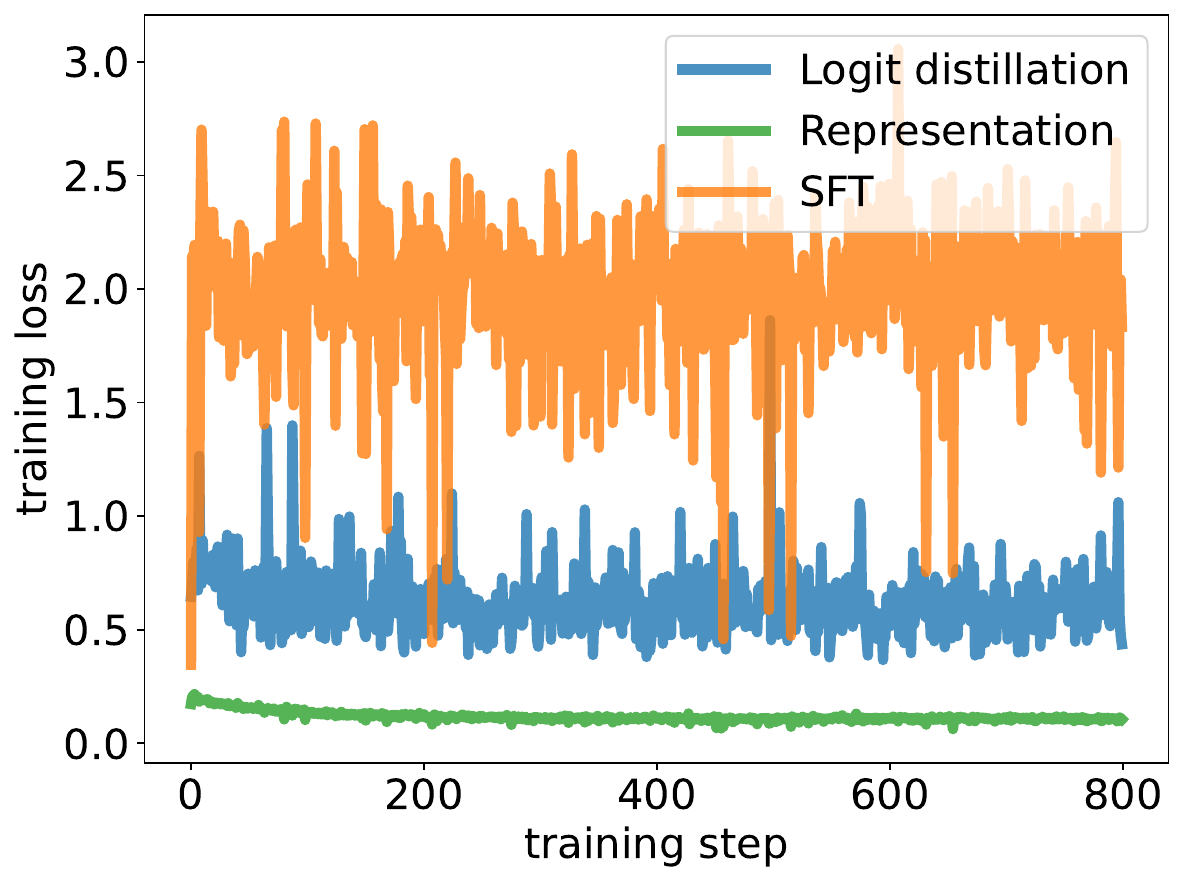}
    }
    \subfloat{
        \includegraphics[width=0.245\textwidth]{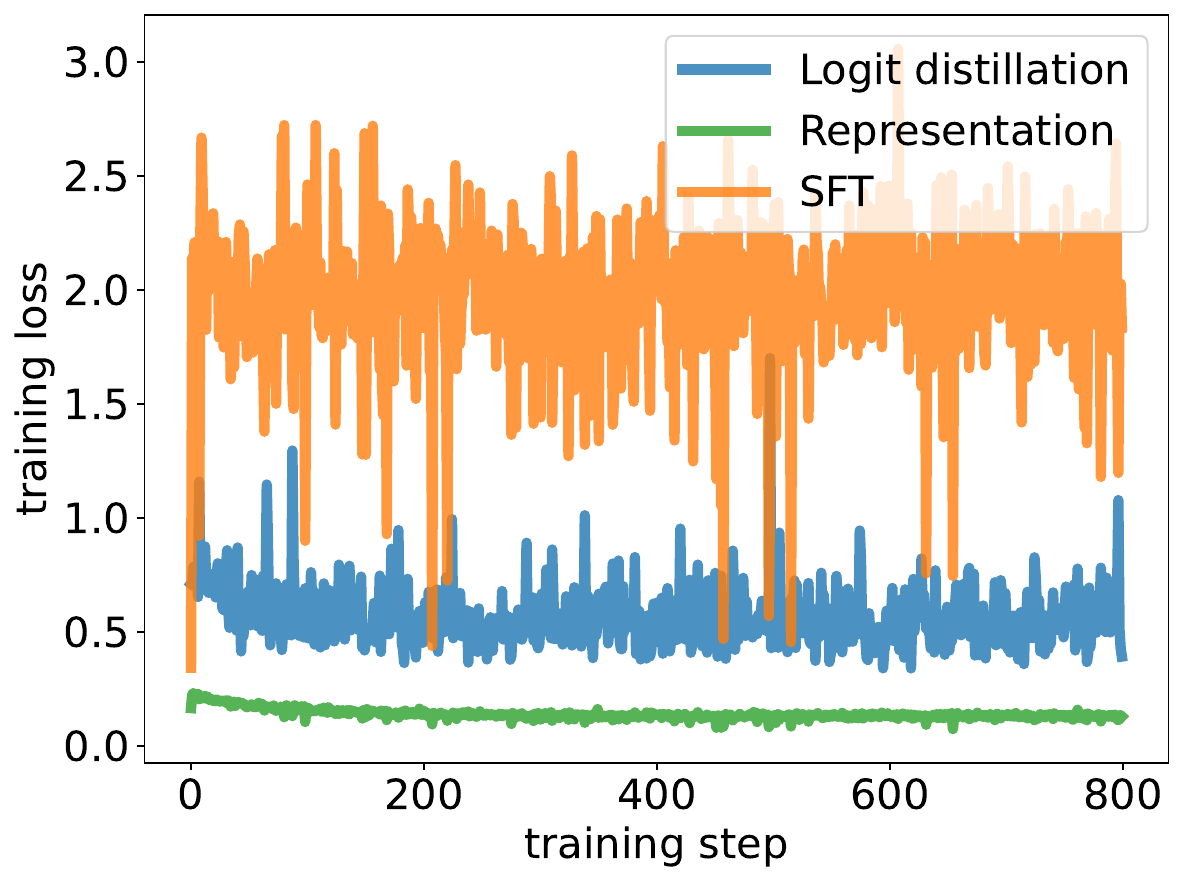}
    }
    \subfloat{
        \includegraphics[width=0.245\textwidth]{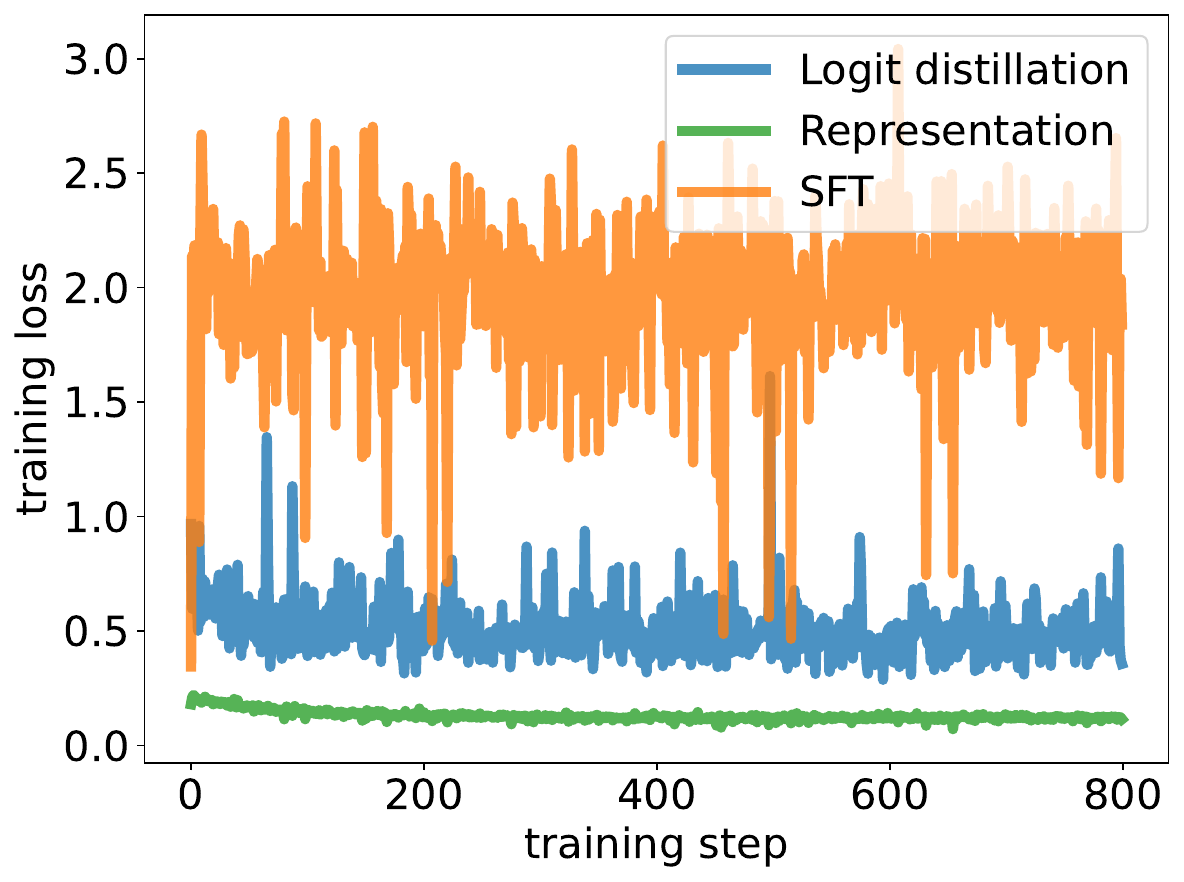}
    }

    \caption{\textbf{Low-rank linear adapter training curves for the first 24 LLaMa-2 7b blocks with a rank of 32} trained using three different objectives including (a) MSE loss defined on the representation, (b) supervised fine-tuning (SFT), and (c) logit distillation where logits are distilled from the full model. Rest of the blocks are visualized in Fig.~\ref{fig:linear_adapters_rank_32_llama2_train_loss_b}.}
    \label{fig:linear_adapters_rank_32_llama2_train_loss_a}
\end{figure}

\begin{figure}[t]
    \centering
    \subfloat{
        \includegraphics[width=0.245\textwidth]{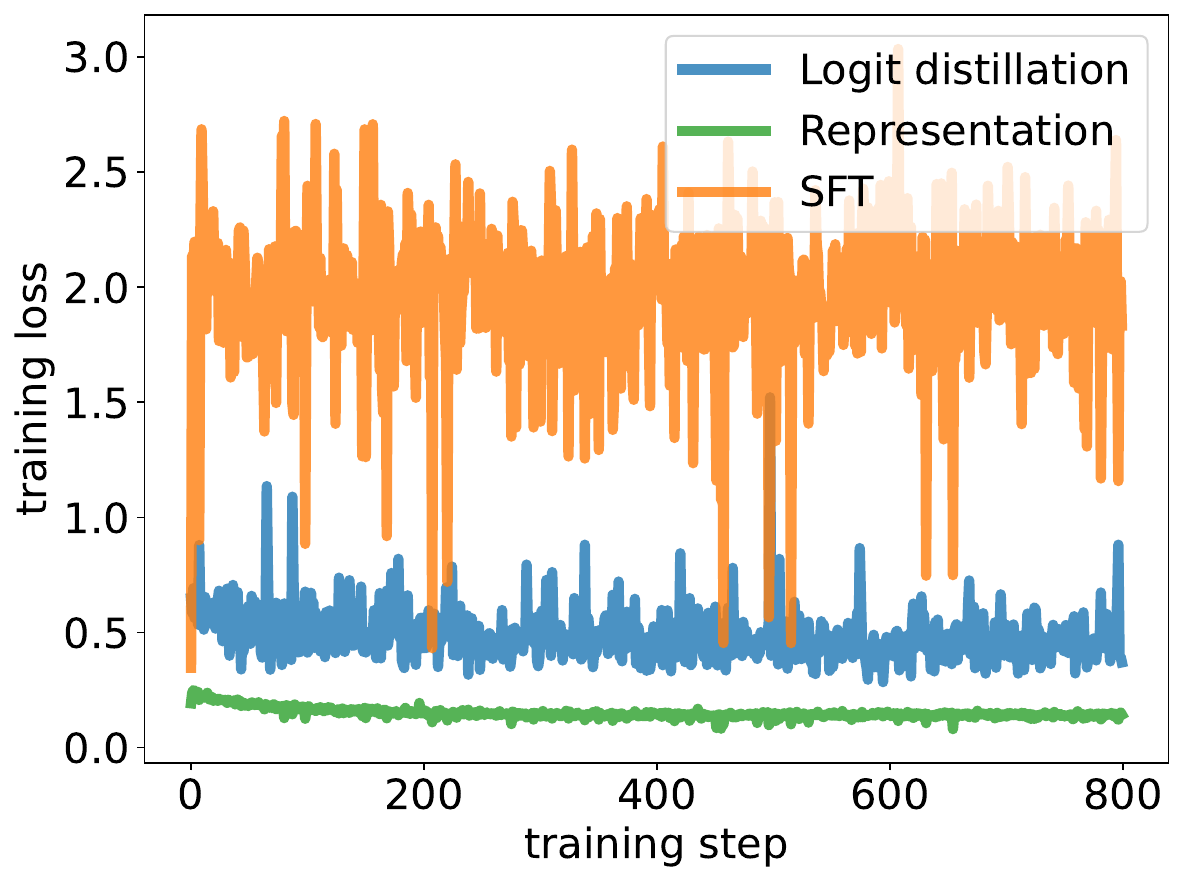}
    }
    \subfloat{
        \includegraphics[width=0.245\textwidth]{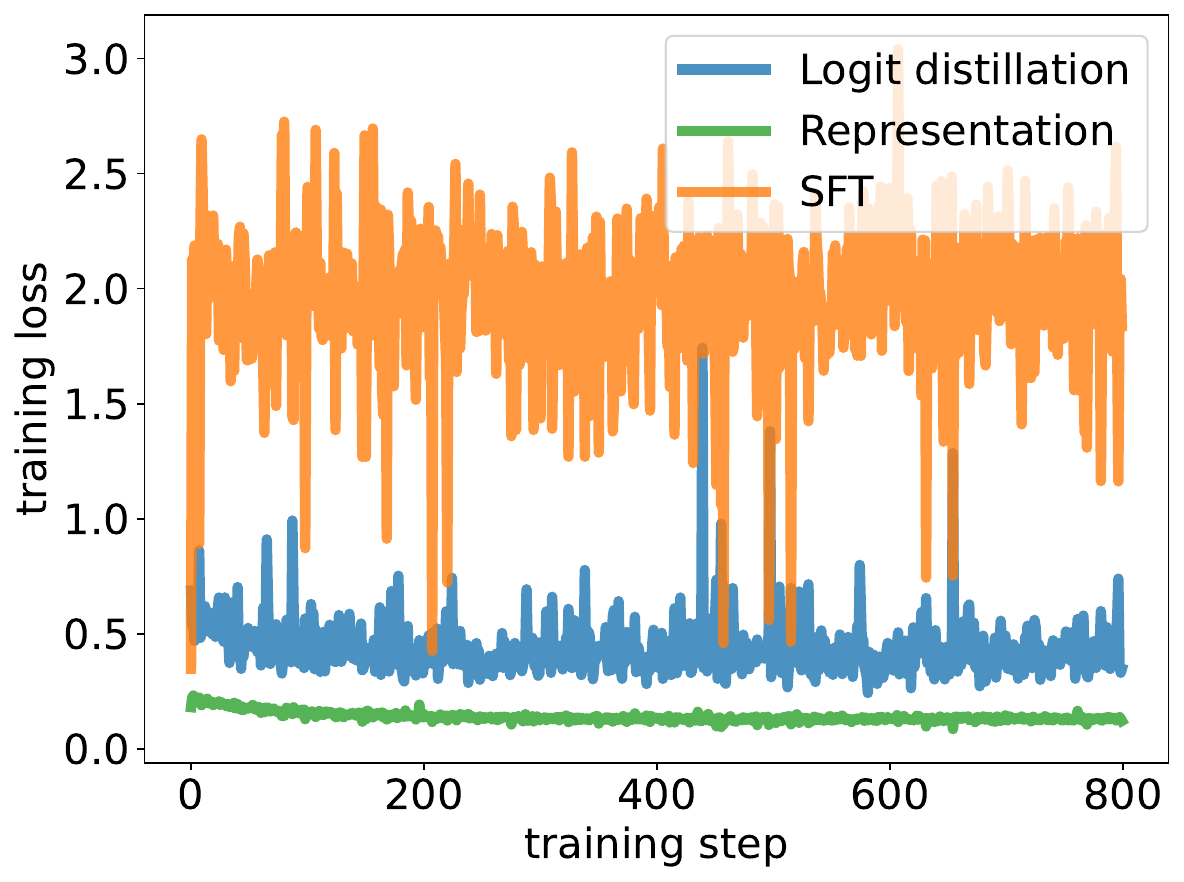}
    }
    \subfloat{
        \includegraphics[width=0.245\textwidth]{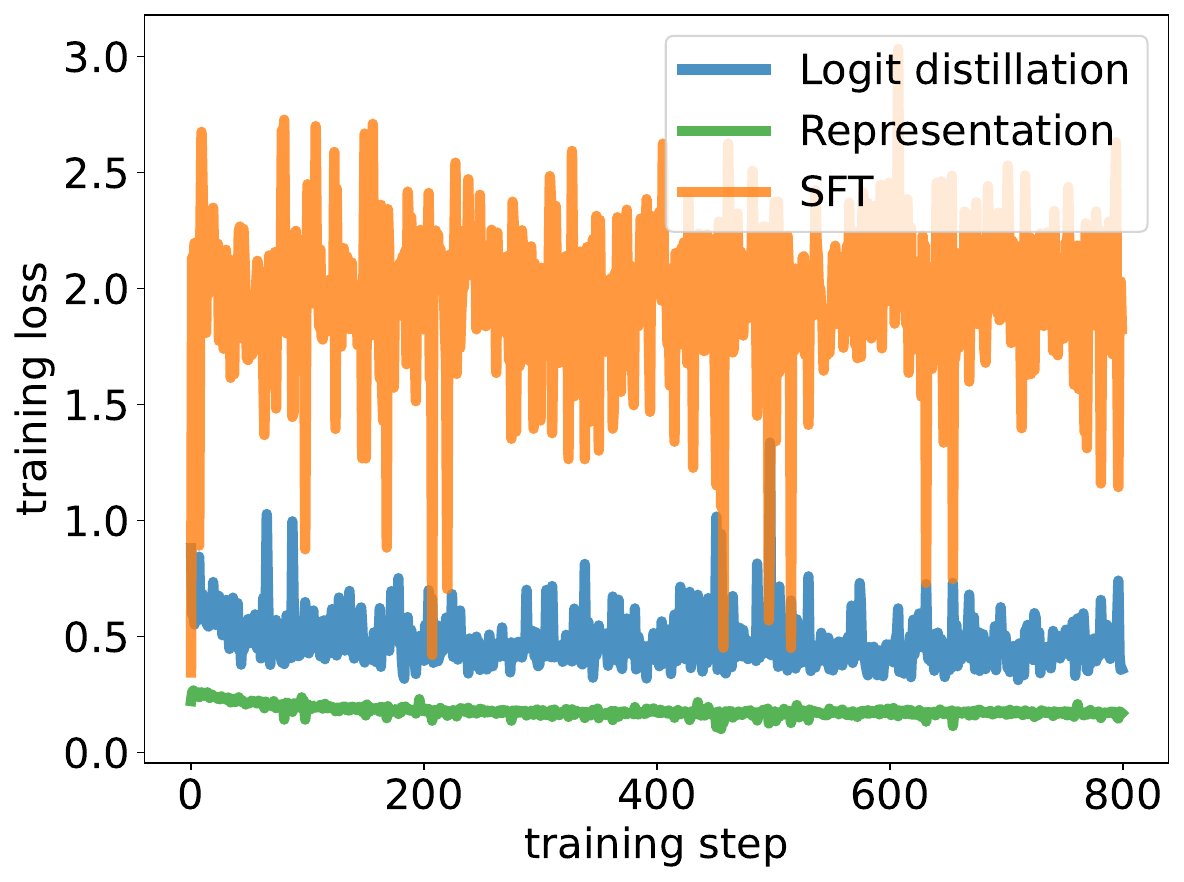}
    }
    \subfloat{
        \includegraphics[width=0.245\textwidth]{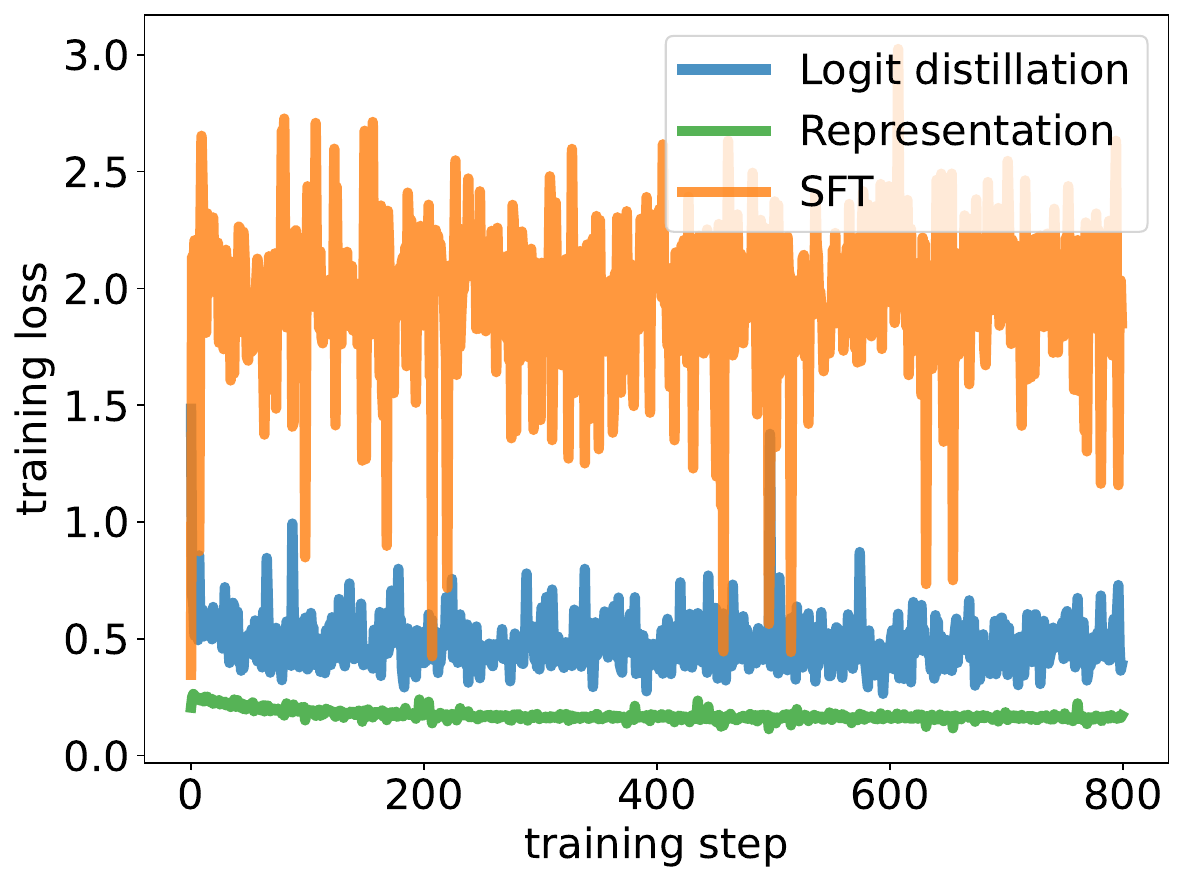}
    }

    \subfloat{
        \includegraphics[width=0.245\textwidth]{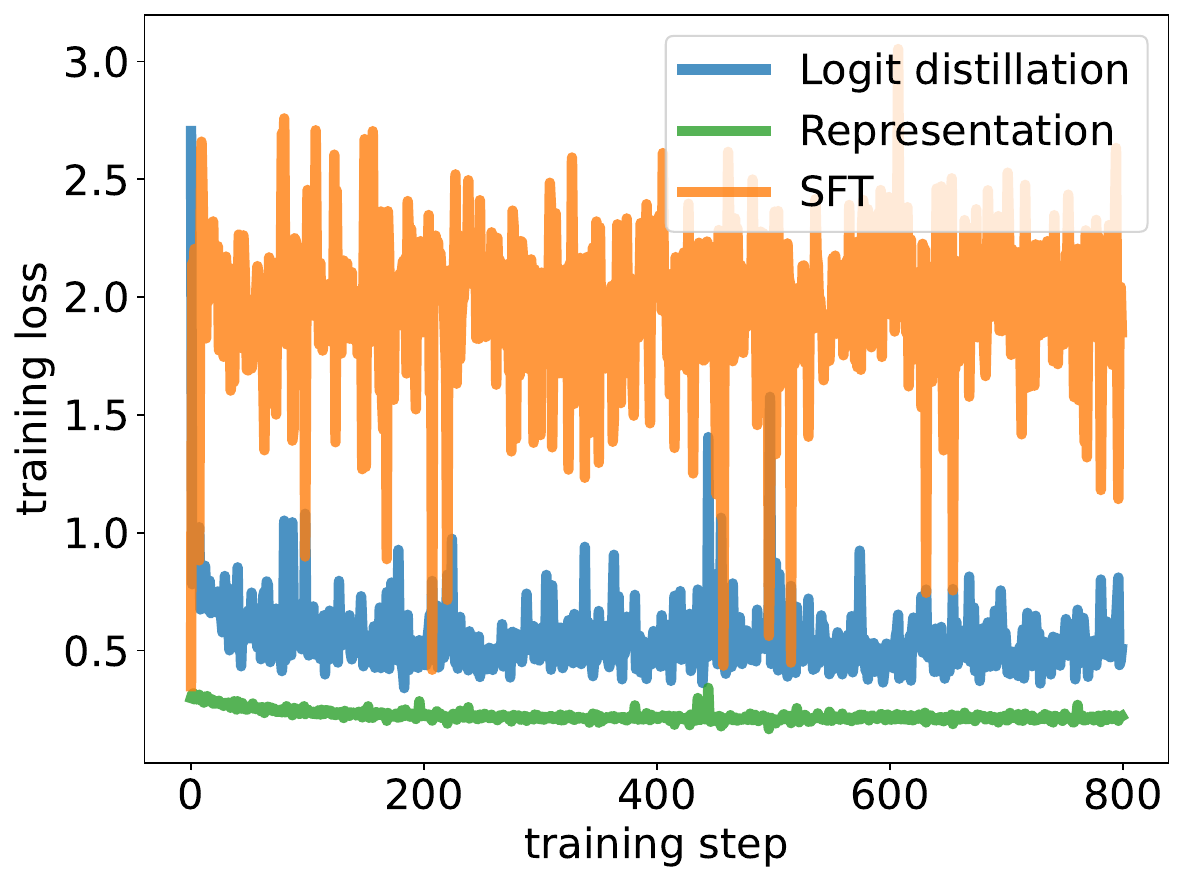}
    }
    \subfloat{
        \includegraphics[width=0.245\textwidth]{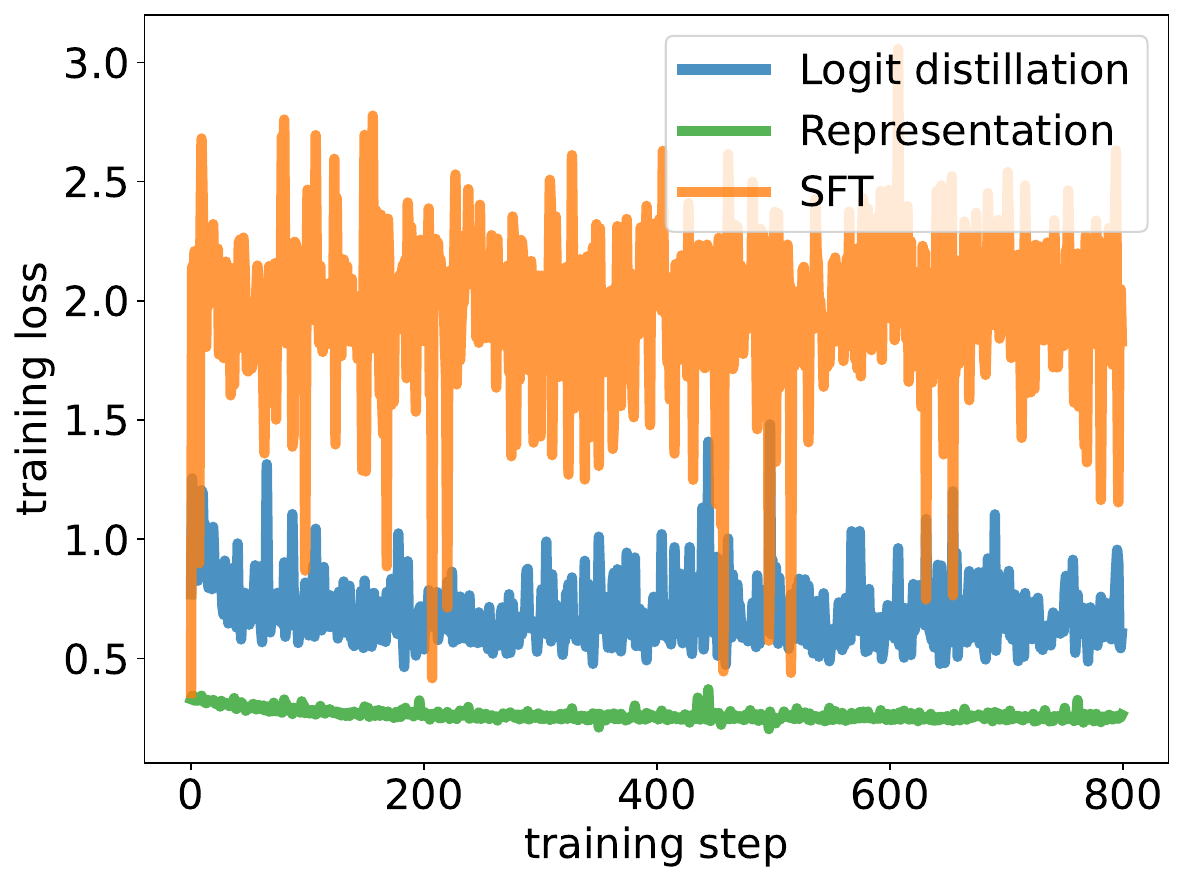}
    }
    \subfloat{
        \includegraphics[width=0.245\textwidth]{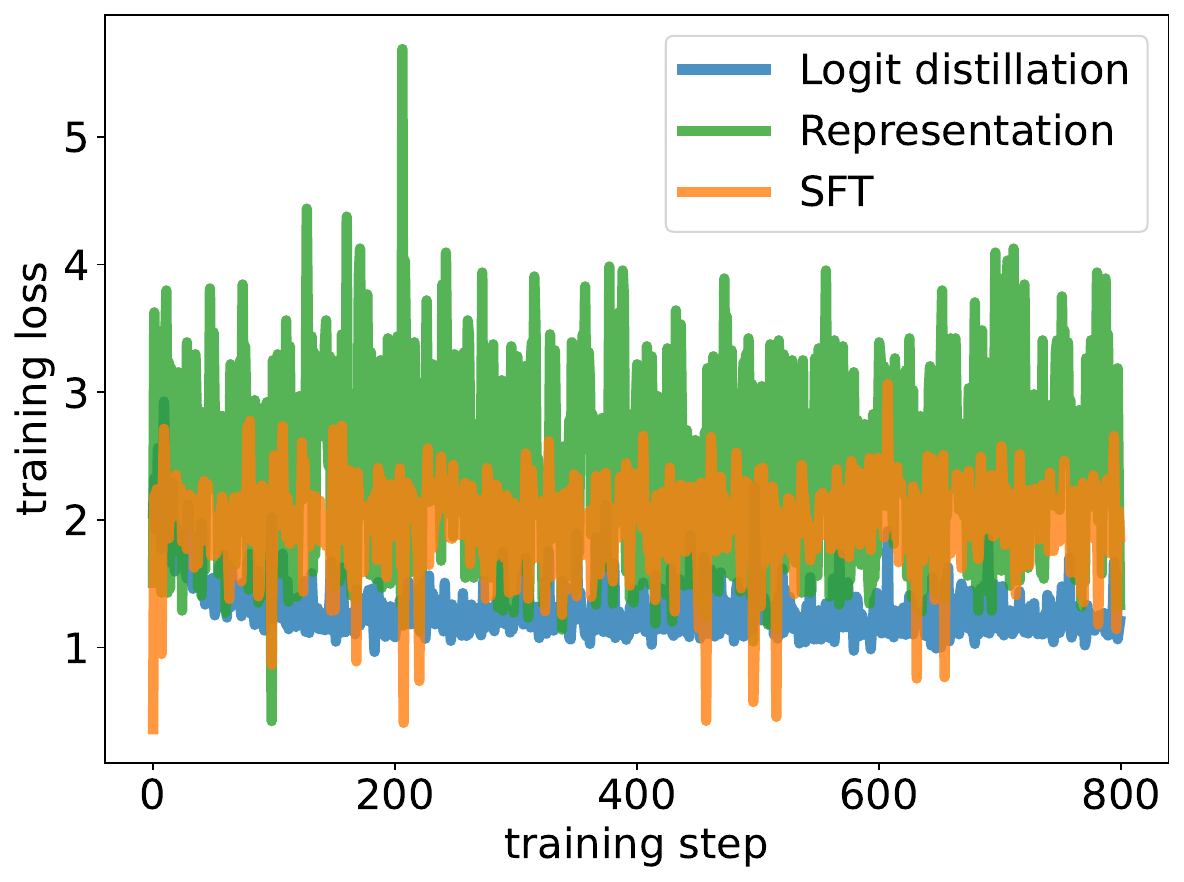}
    }
    \subfloat{
        \includegraphics[width=0.245\textwidth]{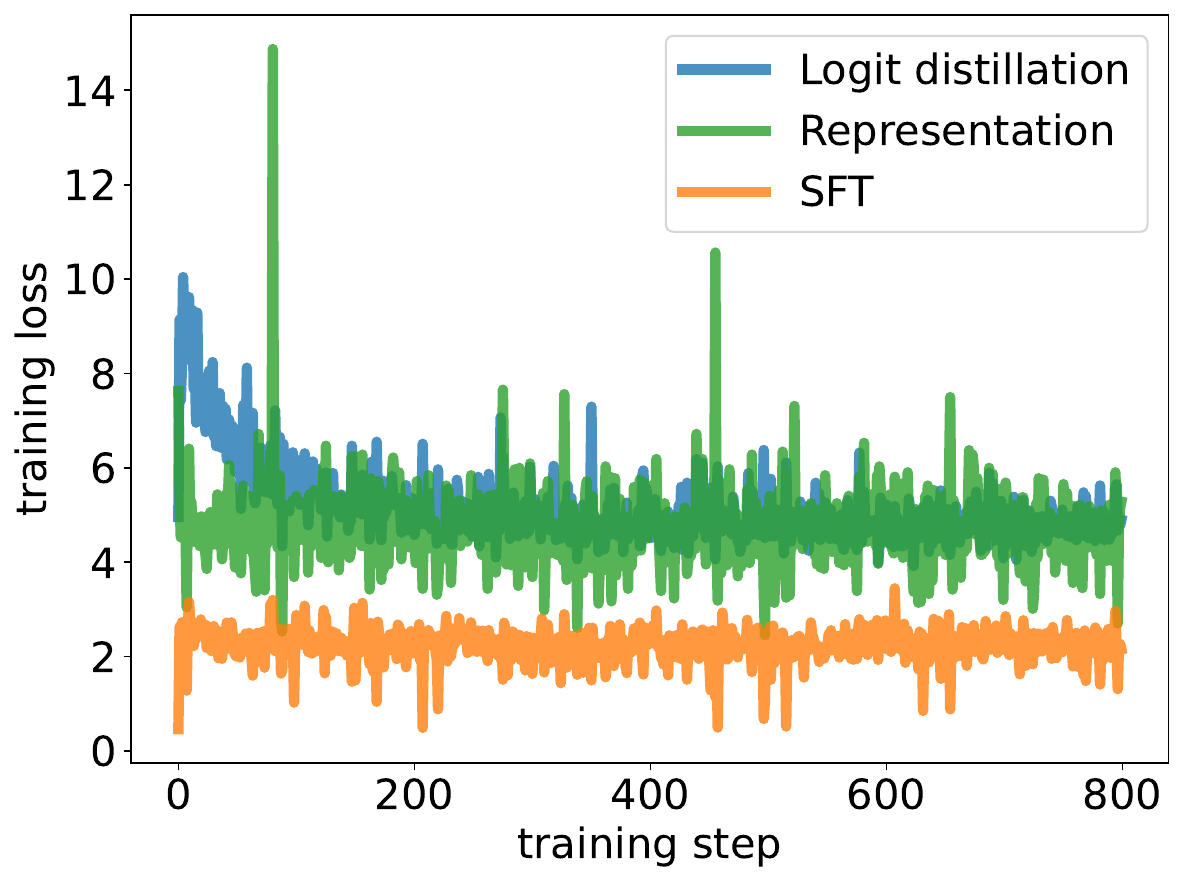}
    }

    \caption{\textbf{Low-rank linear adapter training curves for the last 8 LLaMa-2 7b blocks with a rank of 32} trained using three different objectives including (a) MSE loss defined on the representation, (b) supervised fine-tuning (SFT), and (c) logit distillation where logits are distilled from the full model. The first set of blocks are visualized in Fig.~\ref{fig:linear_adapters_rank_32_llama2_train_loss_a}.}
    \label{fig:linear_adapters_rank_32_llama2_train_loss_b}
\end{figure}

The loss curves for the training of the low-rank adapter with a rank of 32 on LLaMa-2 are visualized in Fig.~\ref{fig:linear_adapters_rank_32_llama2_train_loss_a} and Fig.~\ref{fig:linear_adapters_rank_32_llama2_train_loss_b} respectively.

\begin{figure}[t]
    \centering
    \subfloat{
        \includegraphics[width=0.245\textwidth]{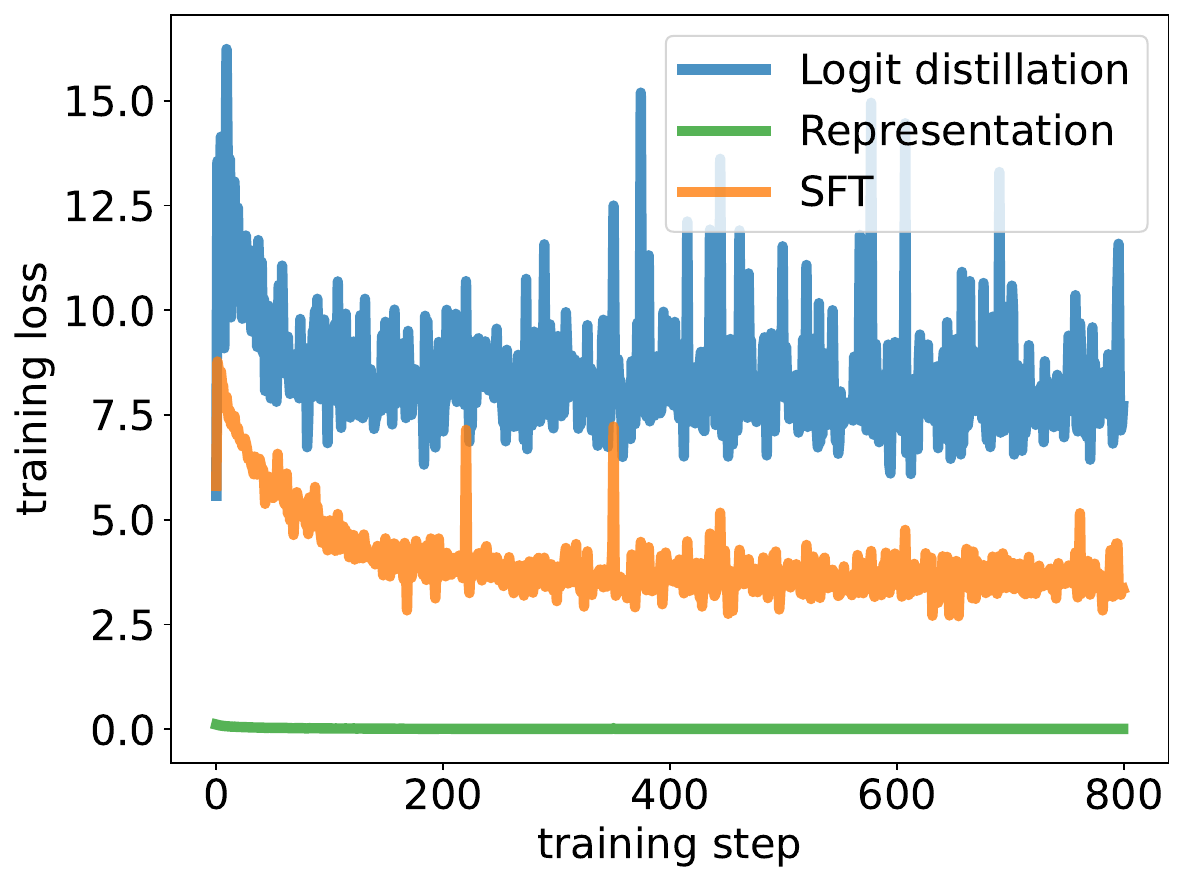}
    }
    \subfloat{
        \includegraphics[width=0.245\textwidth]{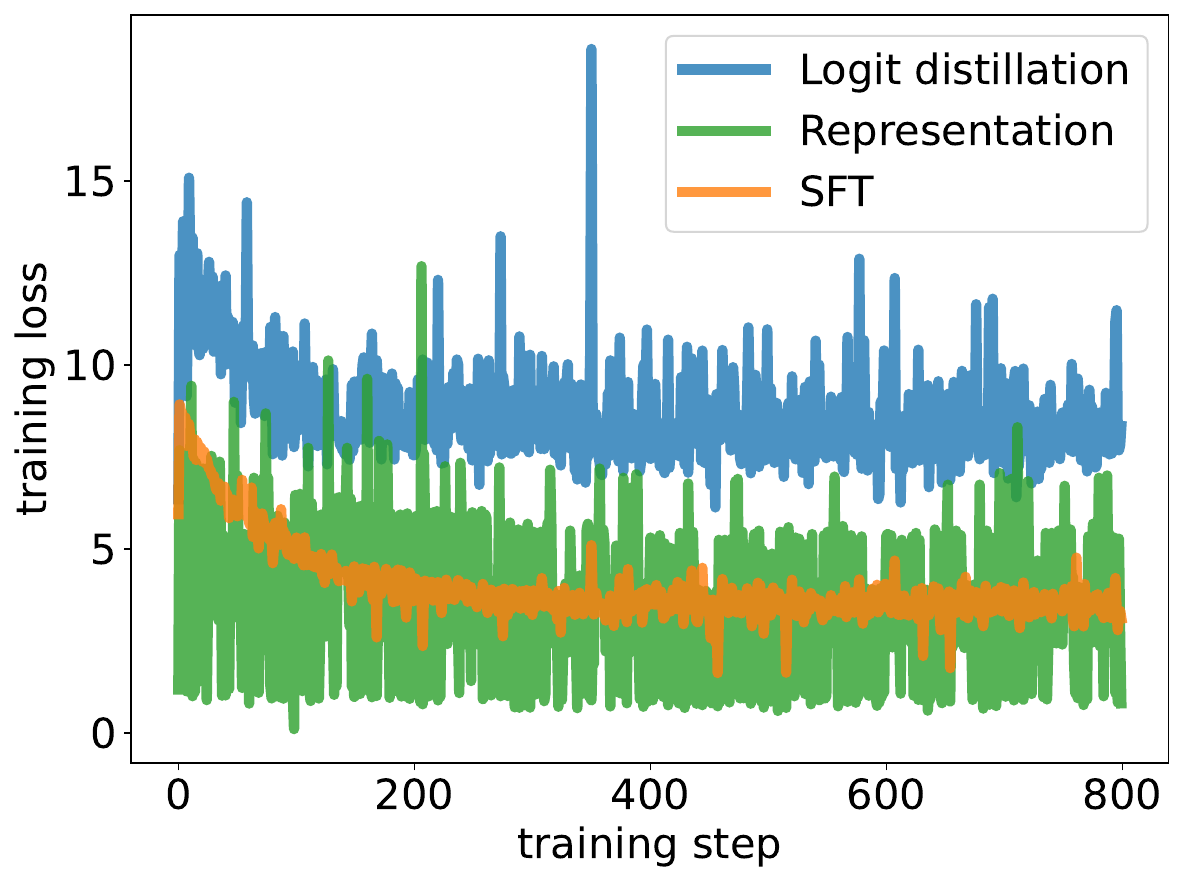}
    }
    \subfloat{
        \includegraphics[width=0.245\textwidth]{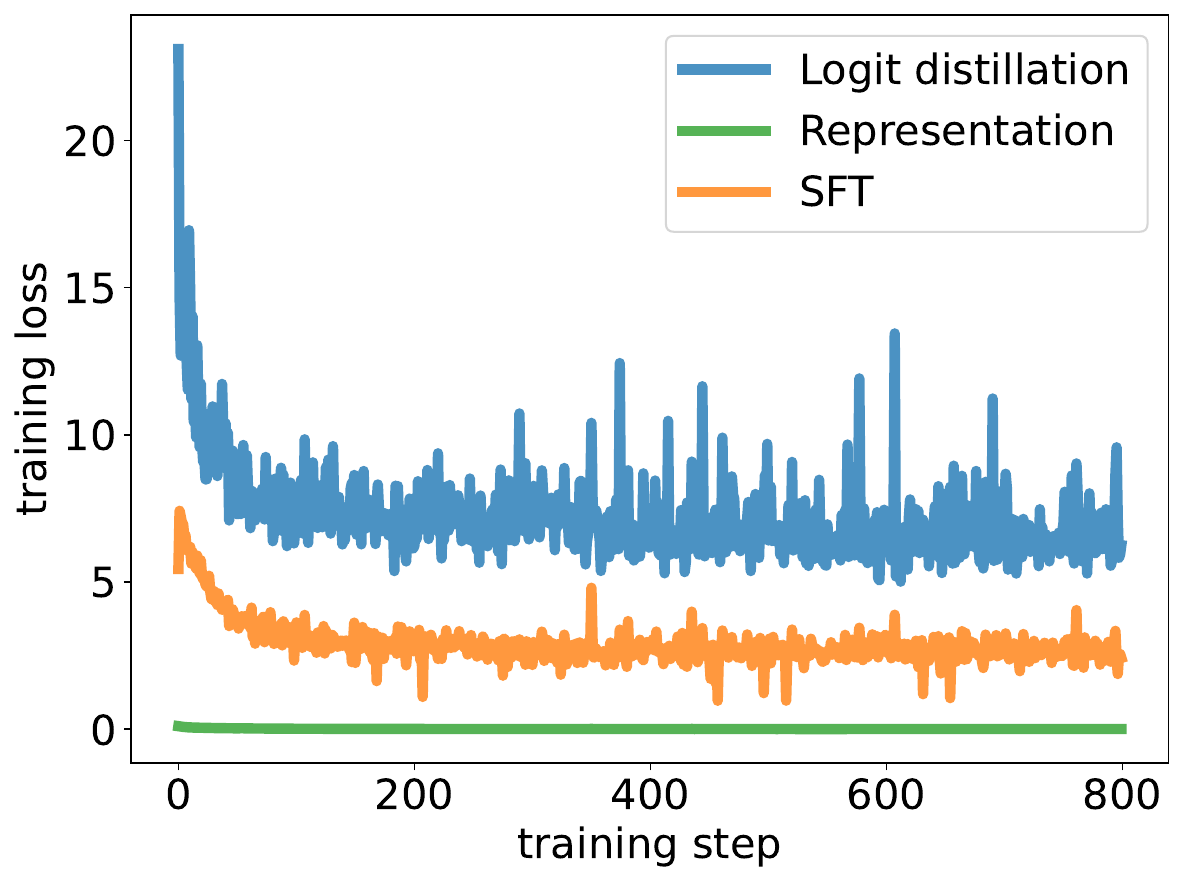}
    }
    \subfloat{
        \includegraphics[width=0.245\textwidth]{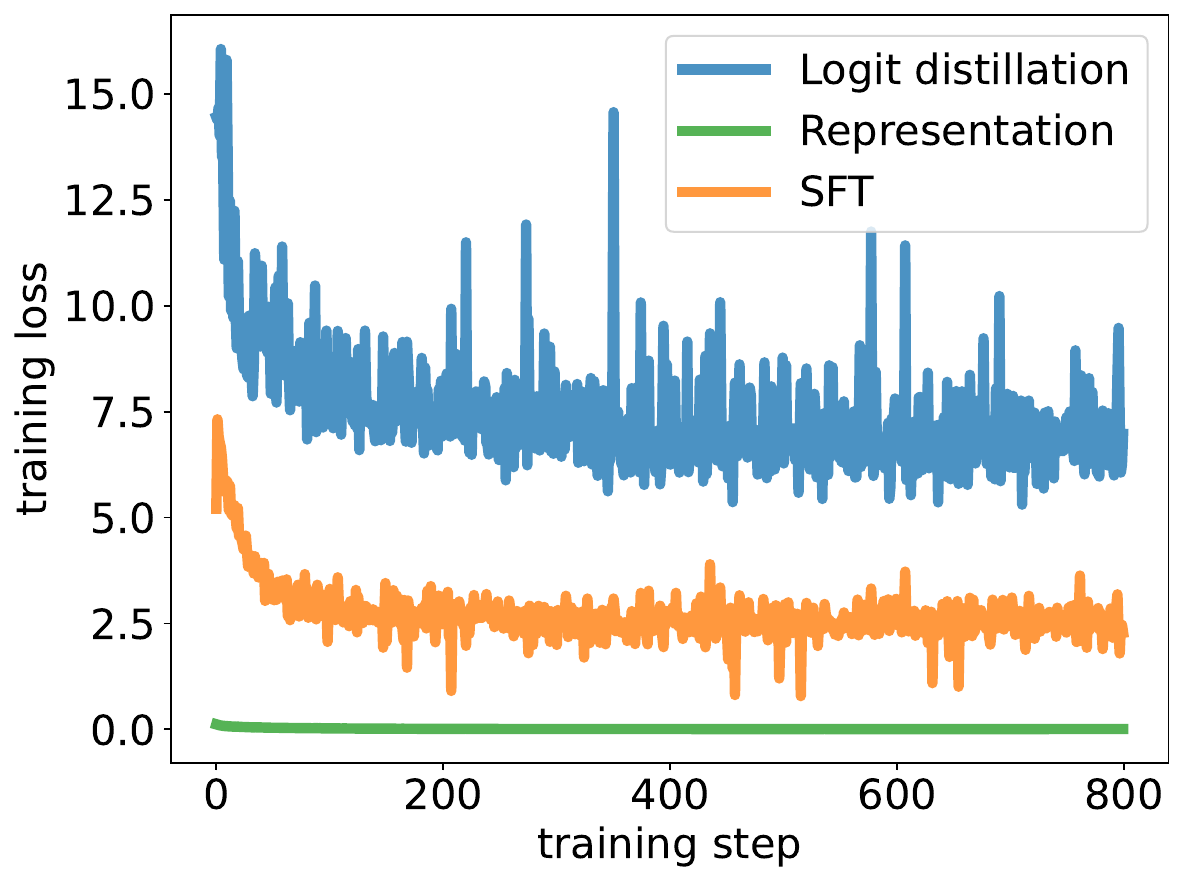}
    }

    \subfloat{
        \includegraphics[width=0.245\textwidth]{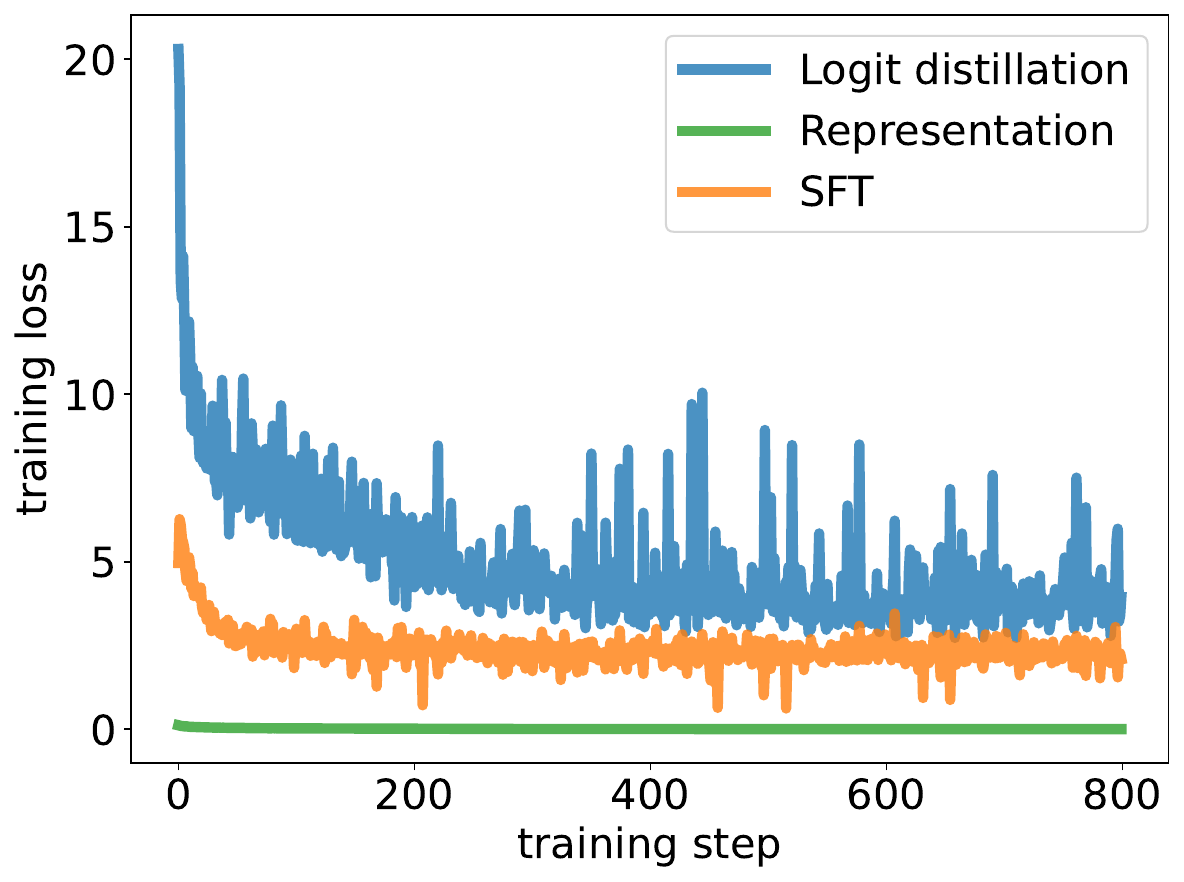}
    }
    \subfloat{
        \includegraphics[width=0.245\textwidth]{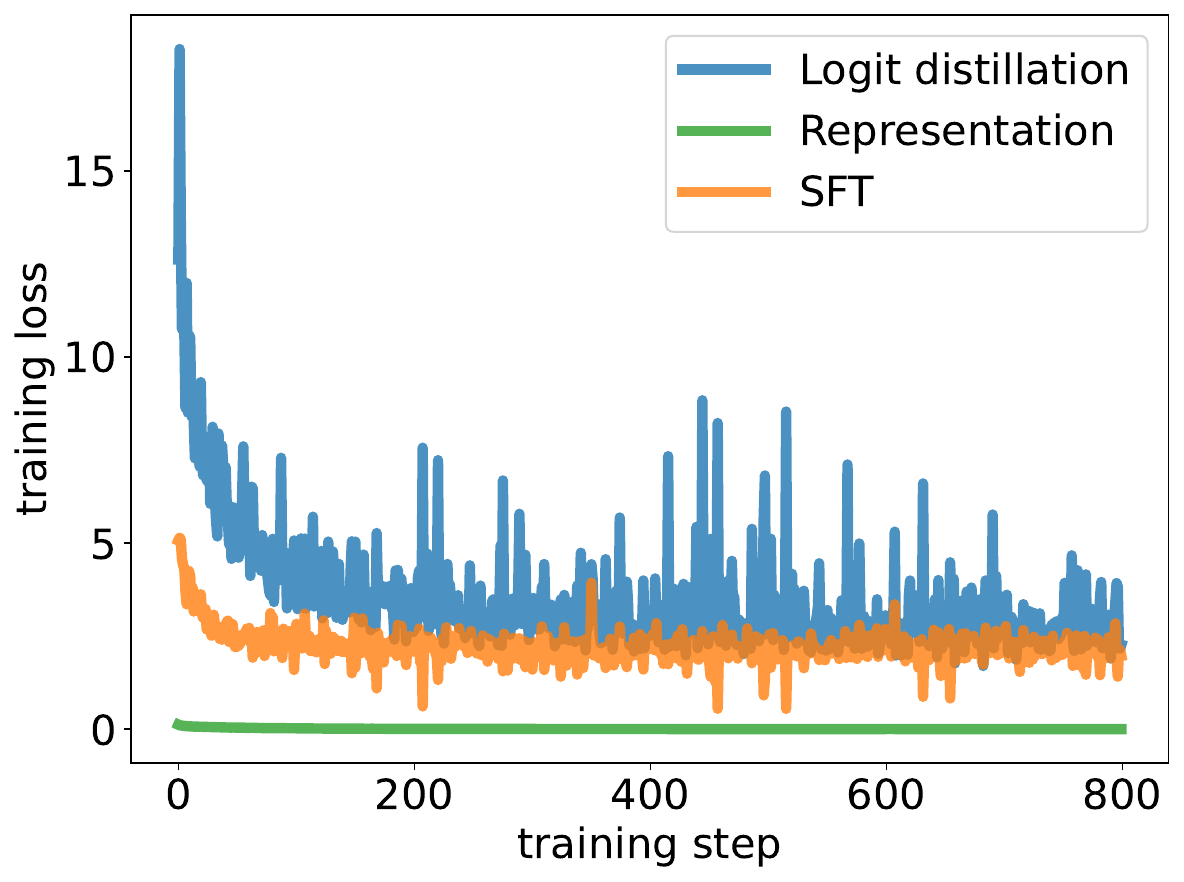}
    }
    \subfloat{
        \includegraphics[width=0.245\textwidth]{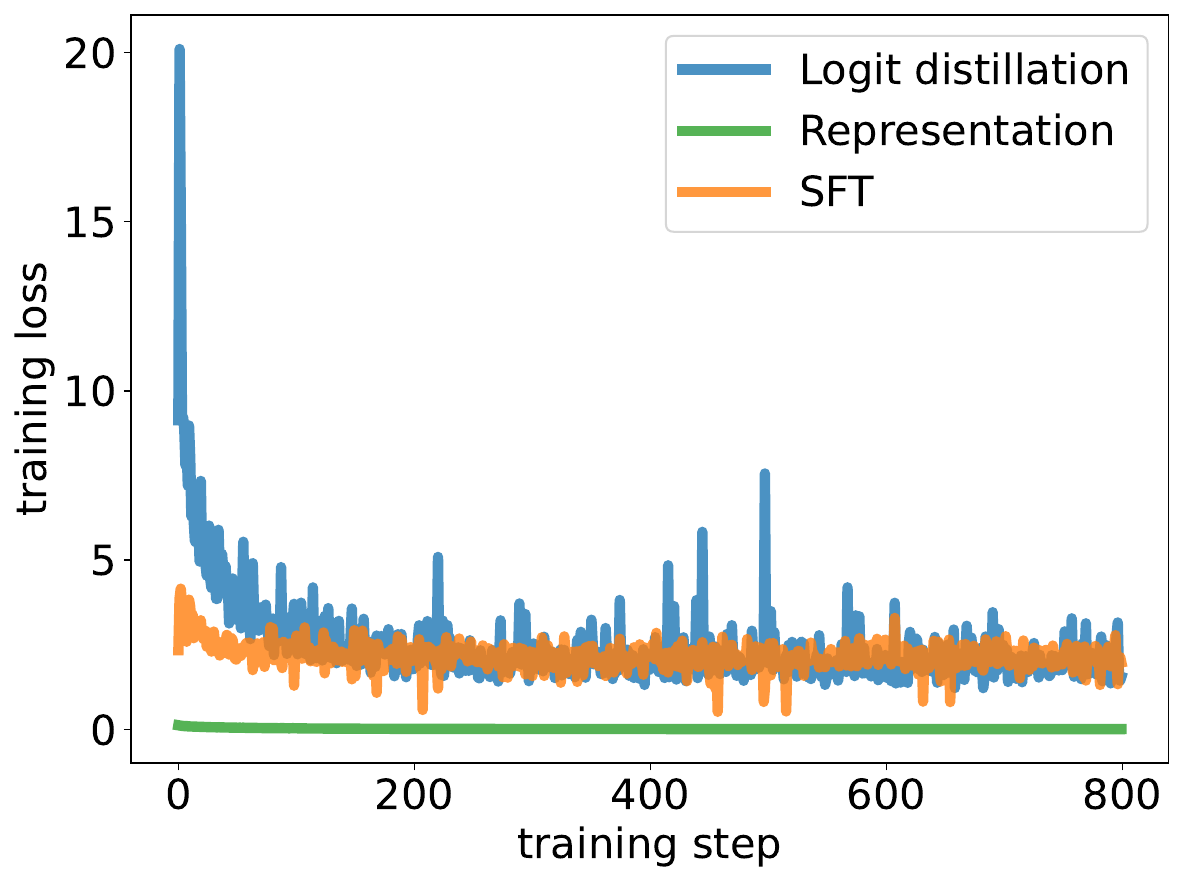}
    }
    \subfloat{
        \includegraphics[width=0.245\textwidth]{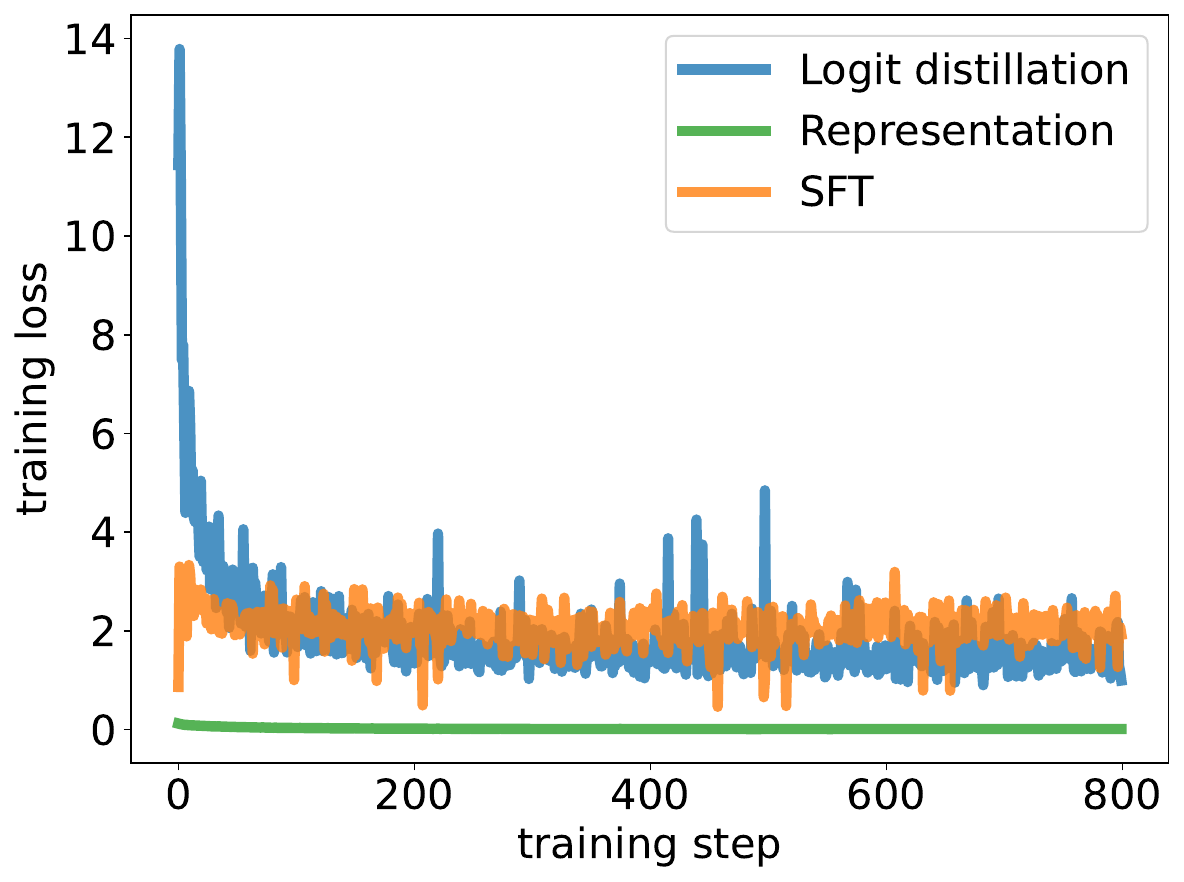}
    }

    \subfloat{
        \includegraphics[width=0.245\textwidth]{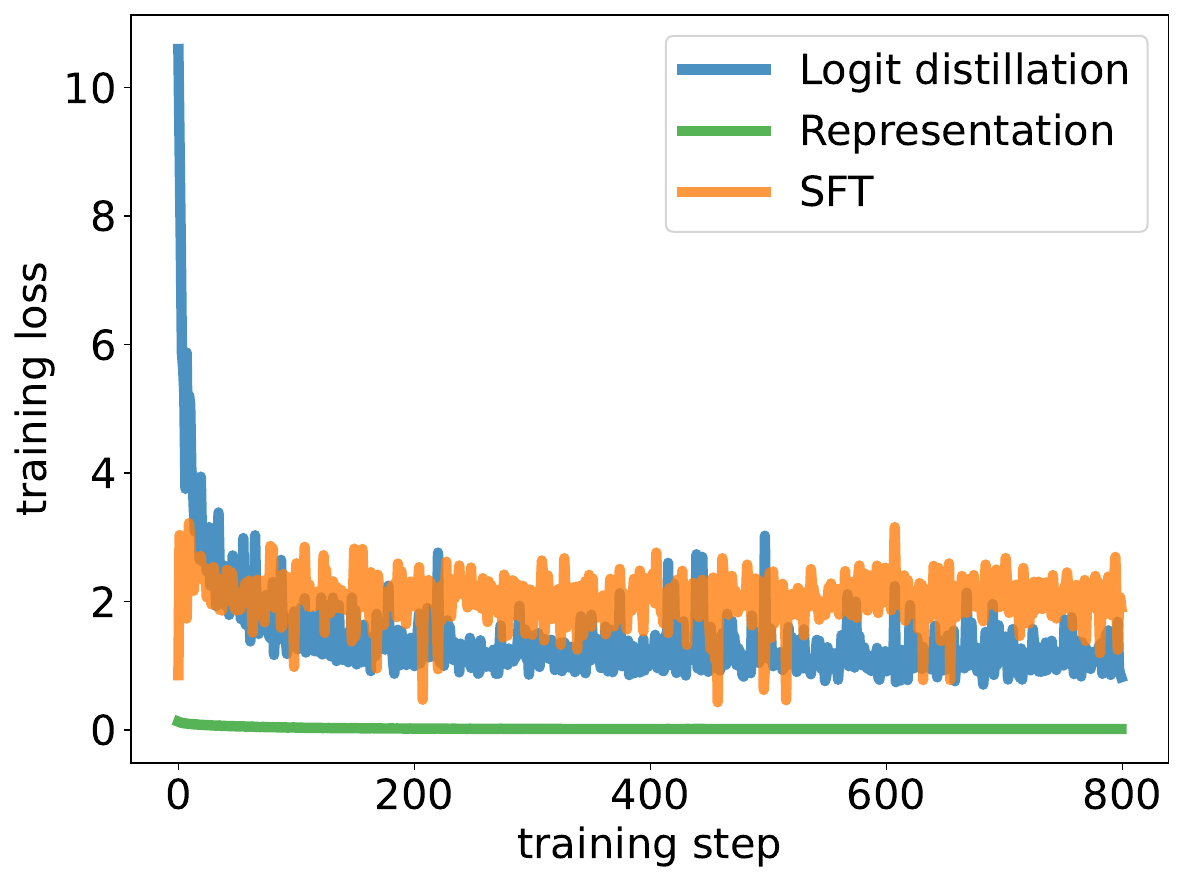}
    }
    \subfloat{
        \includegraphics[width=0.245\textwidth]{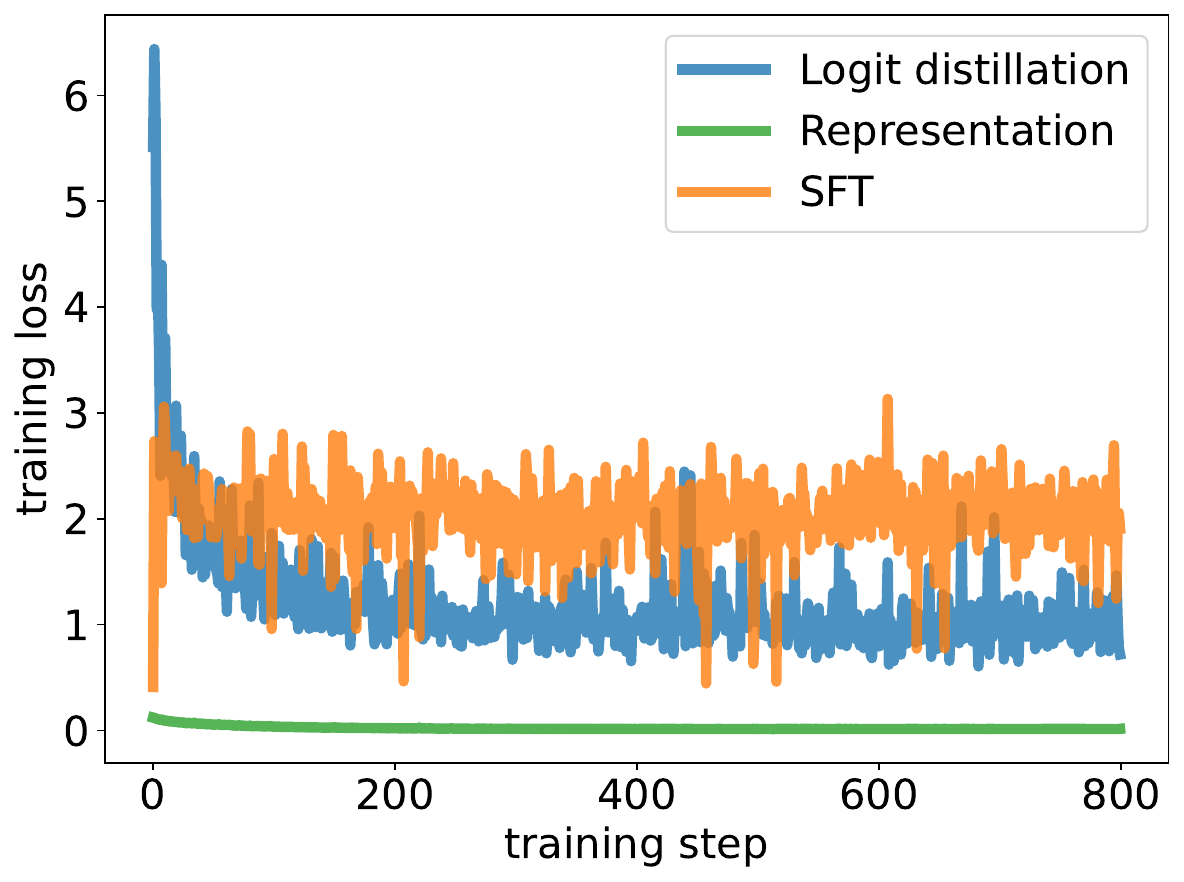}
    }
    \subfloat{
        \includegraphics[width=0.245\textwidth]{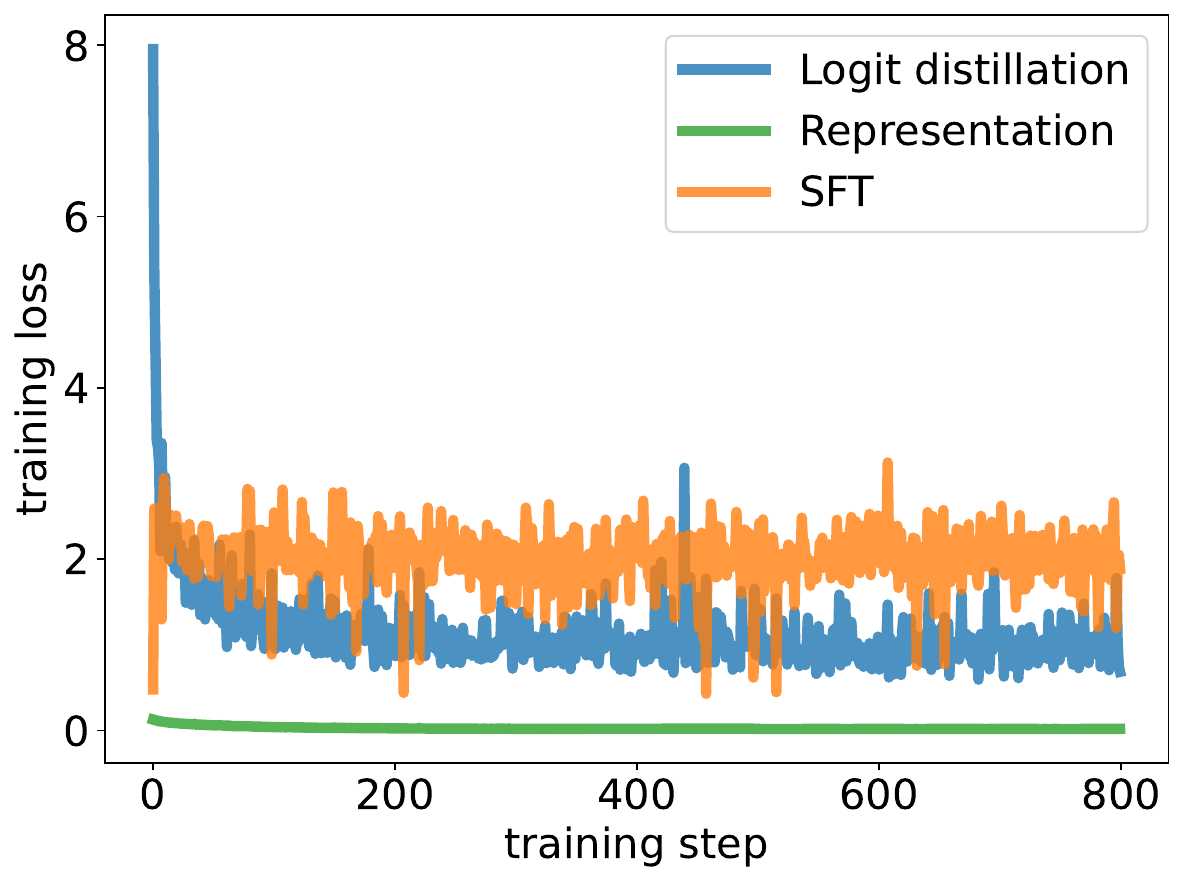}
    }
    \subfloat{
        \includegraphics[width=0.245\textwidth]{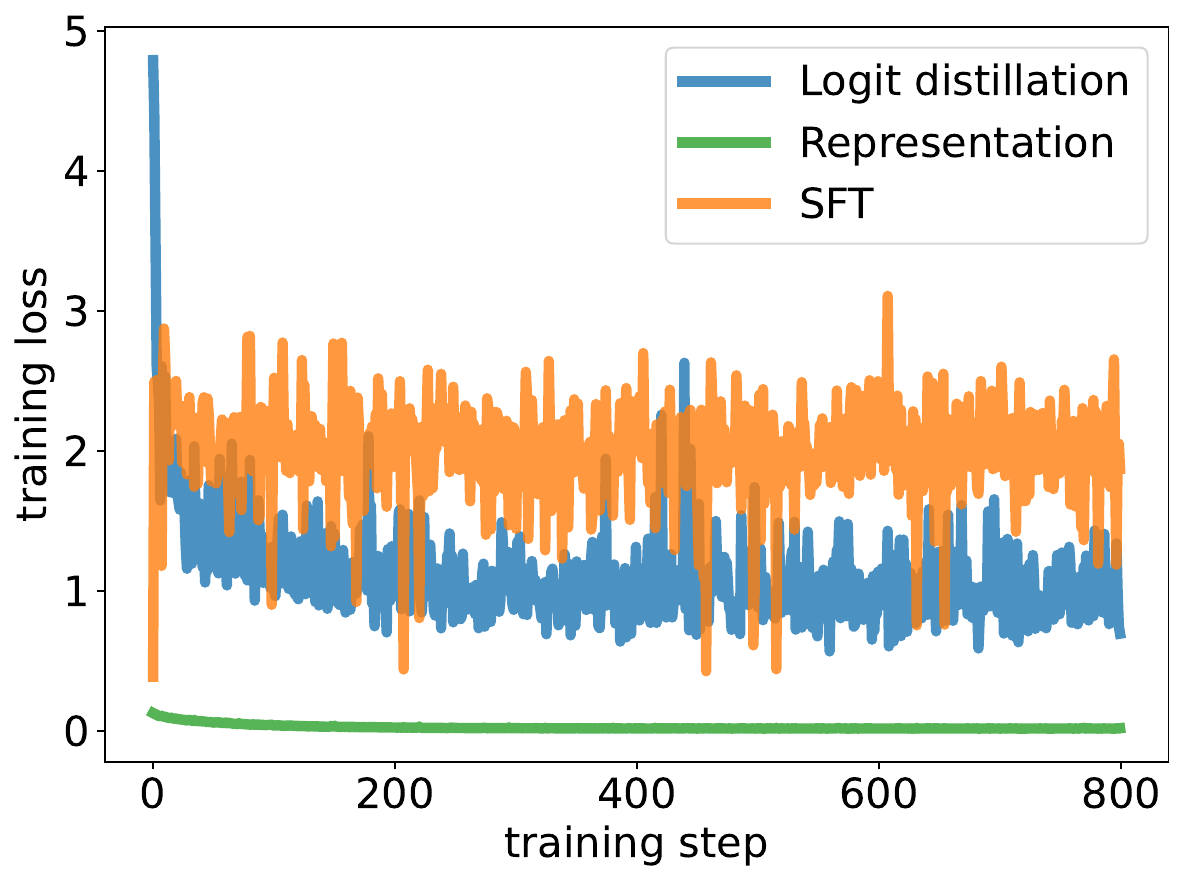}
    }

    \subfloat{
        \includegraphics[width=0.245\textwidth]{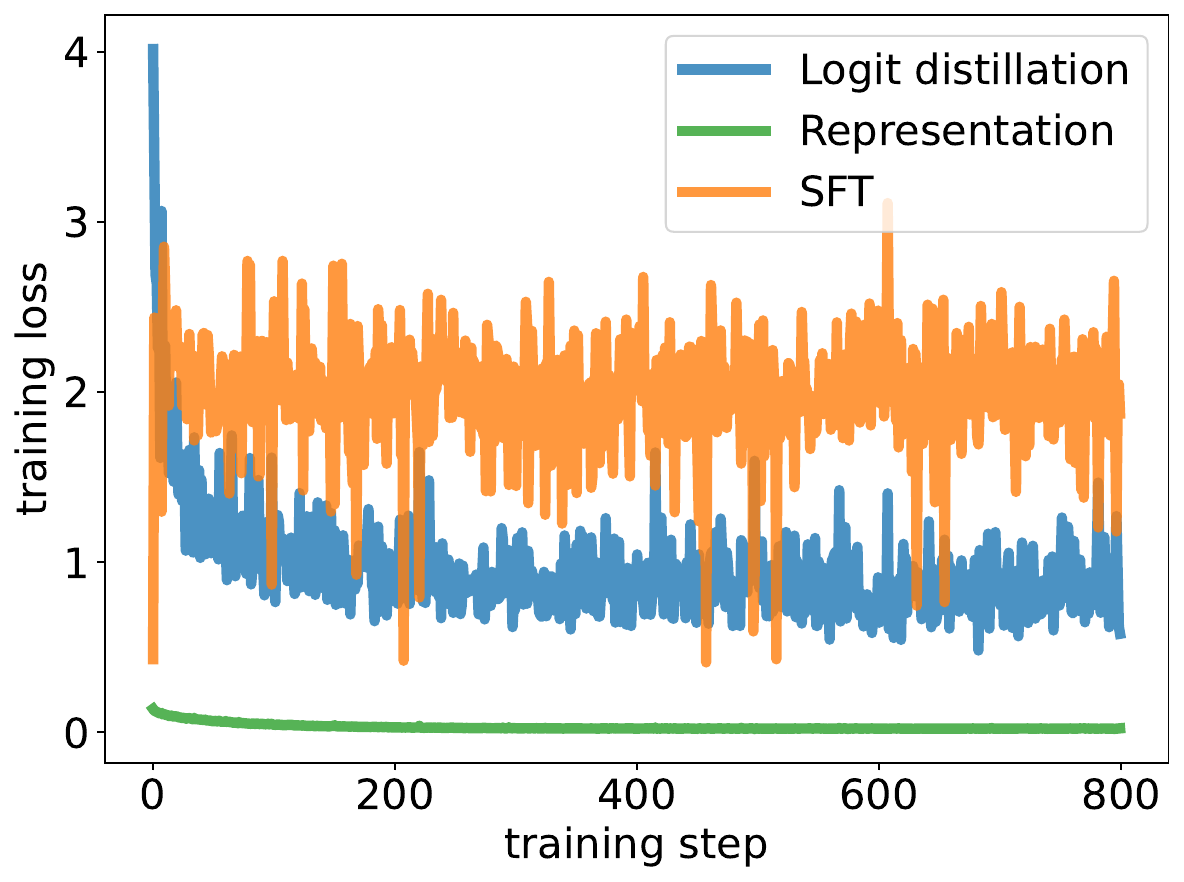}
    }
    \subfloat{
        \includegraphics[width=0.245\textwidth]{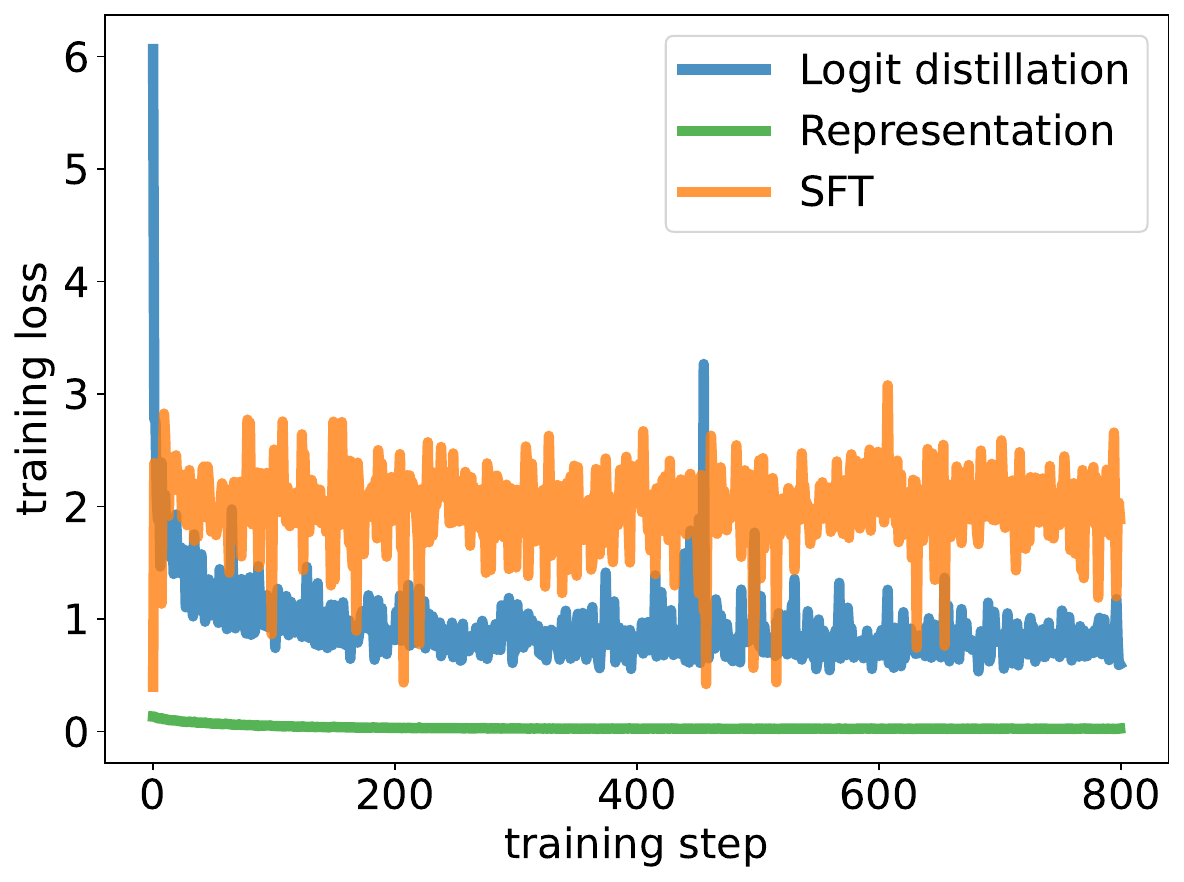}
    }
    \subfloat{
        \includegraphics[width=0.245\textwidth]{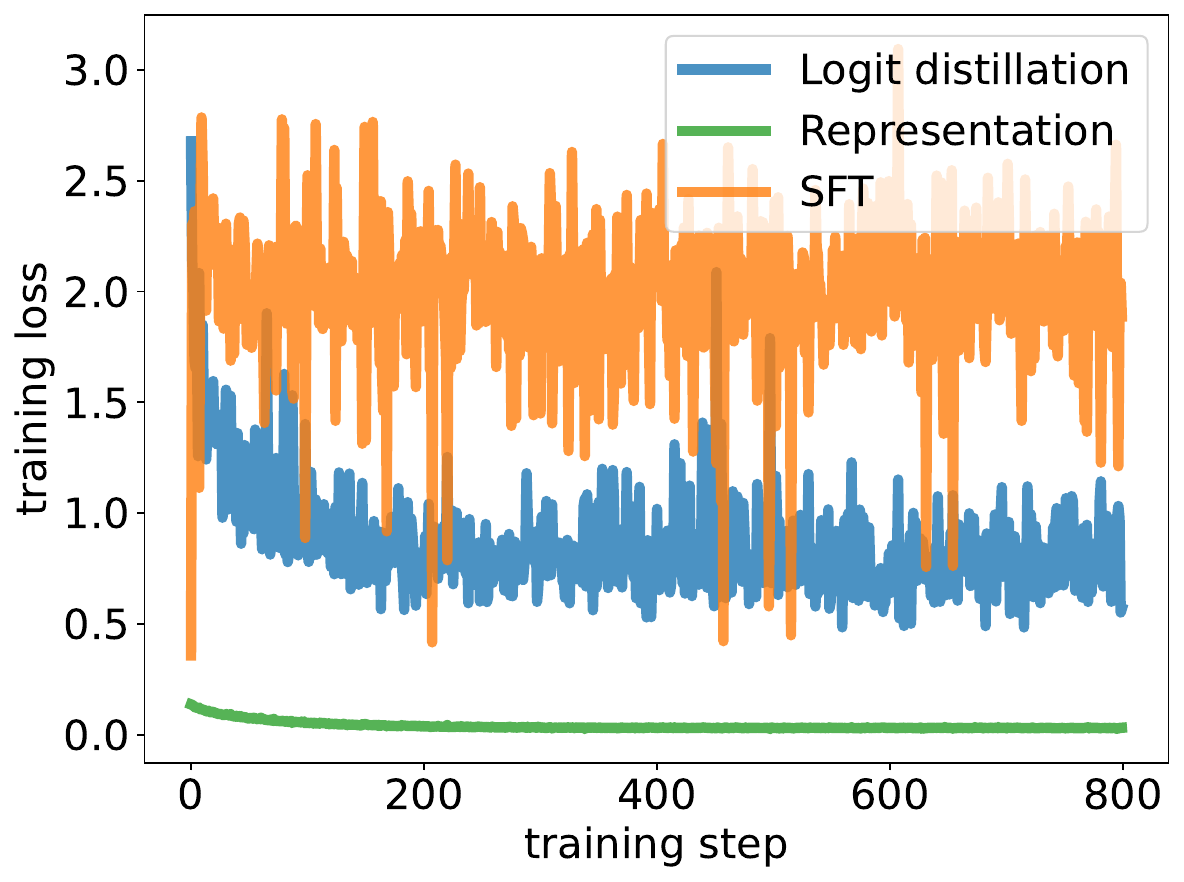}
    }
    \subfloat{
        \includegraphics[width=0.245\textwidth]{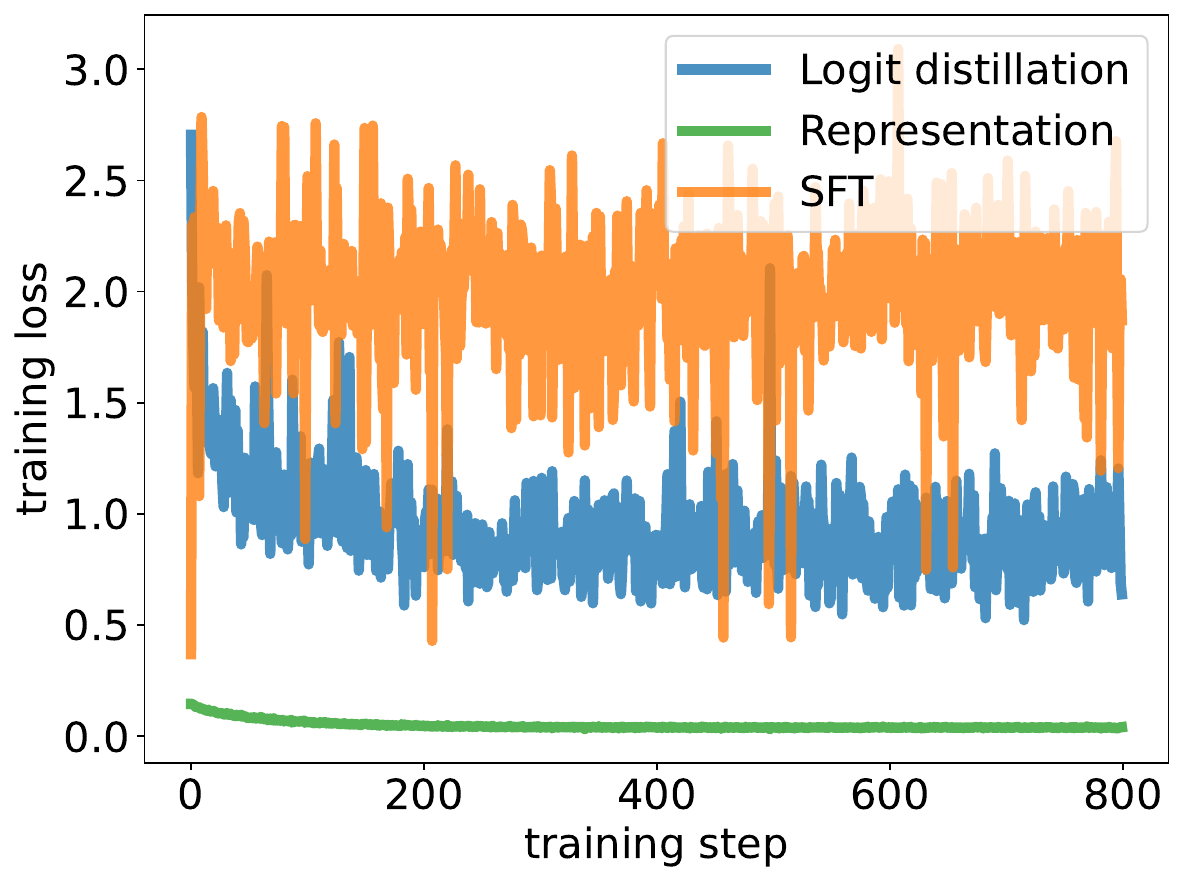}
    }

    \subfloat{
        \includegraphics[width=0.245\textwidth]{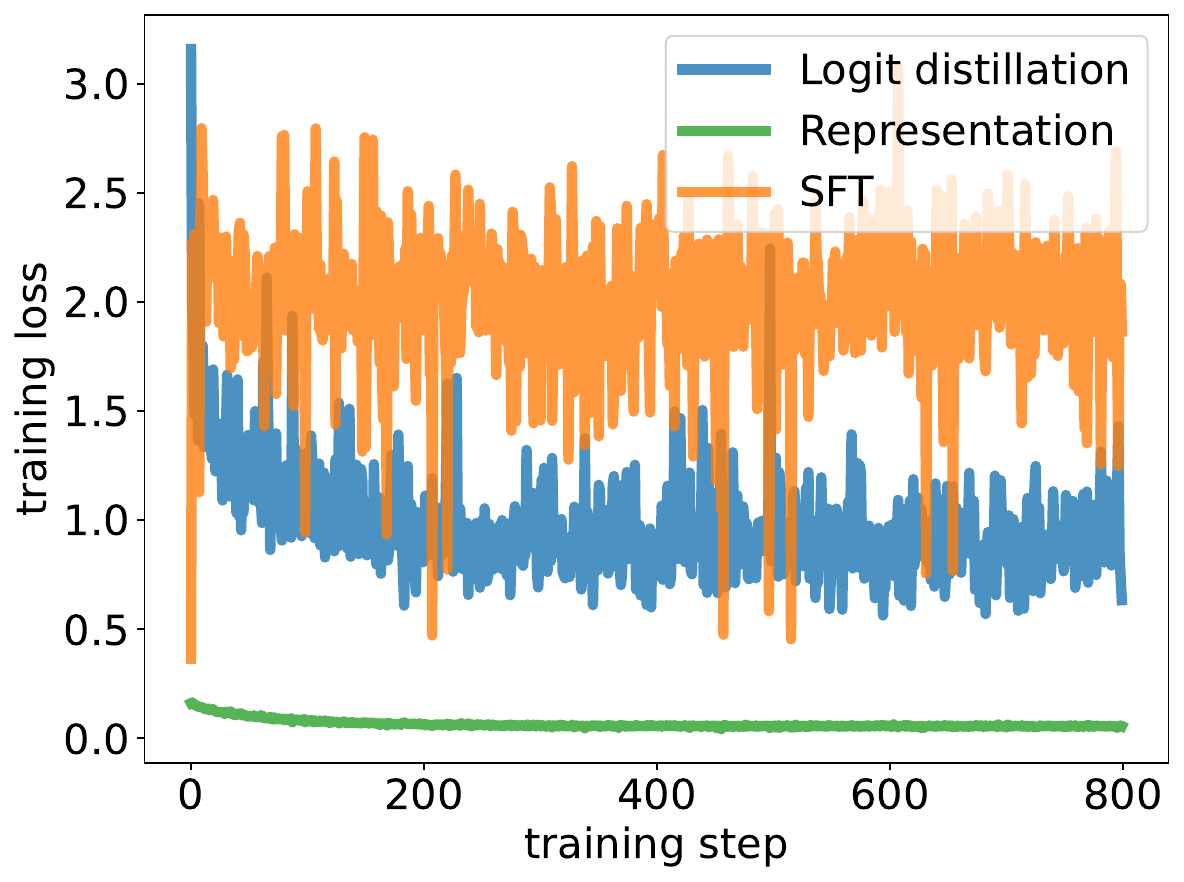}
    }
    \subfloat{
        \includegraphics[width=0.245\textwidth]{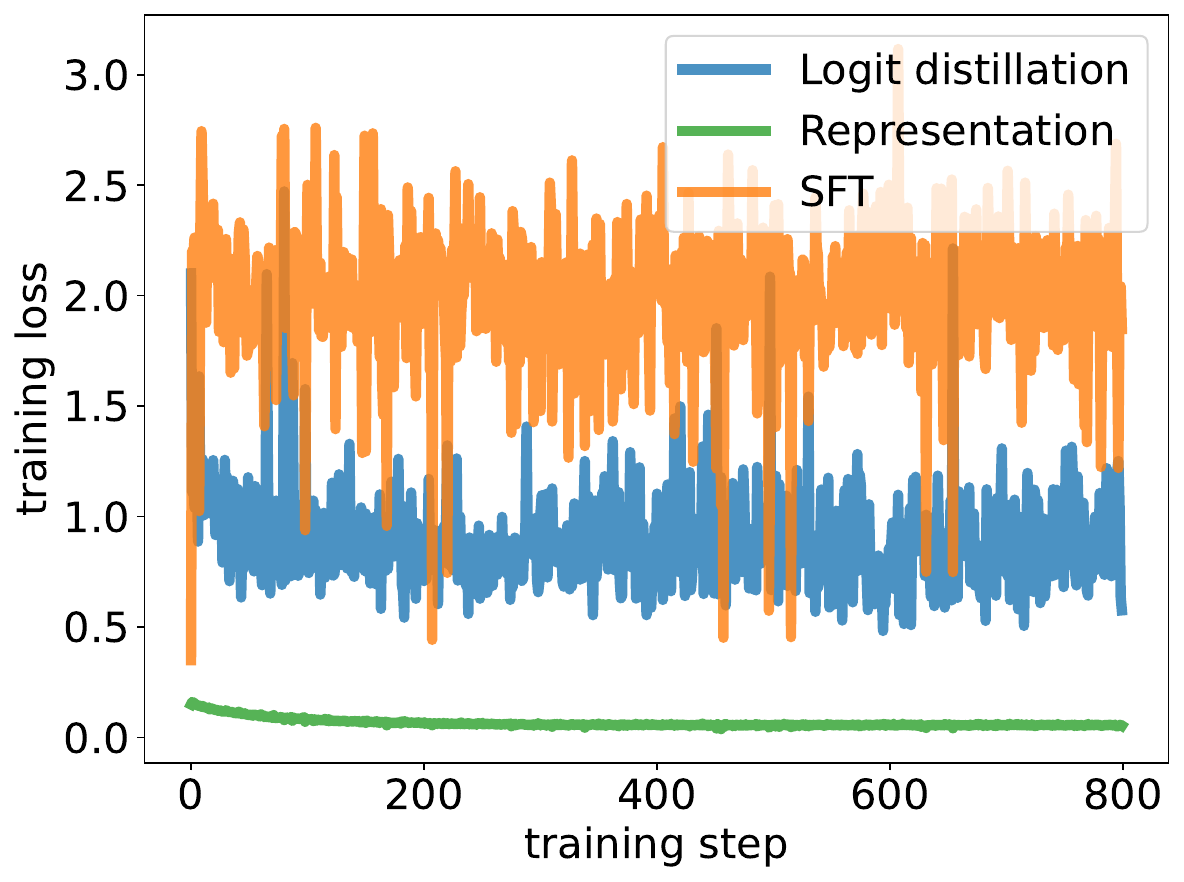}
    }
    \subfloat{
        \includegraphics[width=0.245\textwidth]{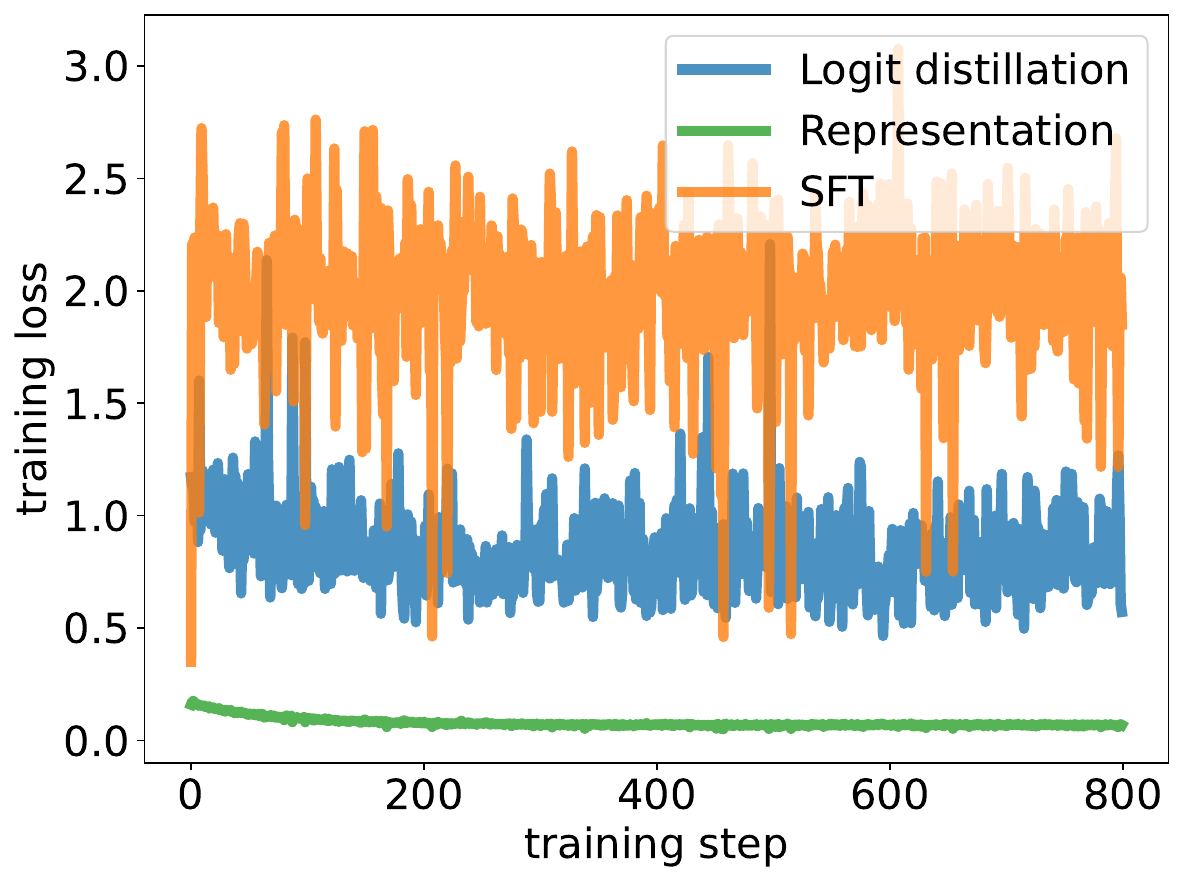}
    }
    \subfloat{
        \includegraphics[width=0.245\textwidth]{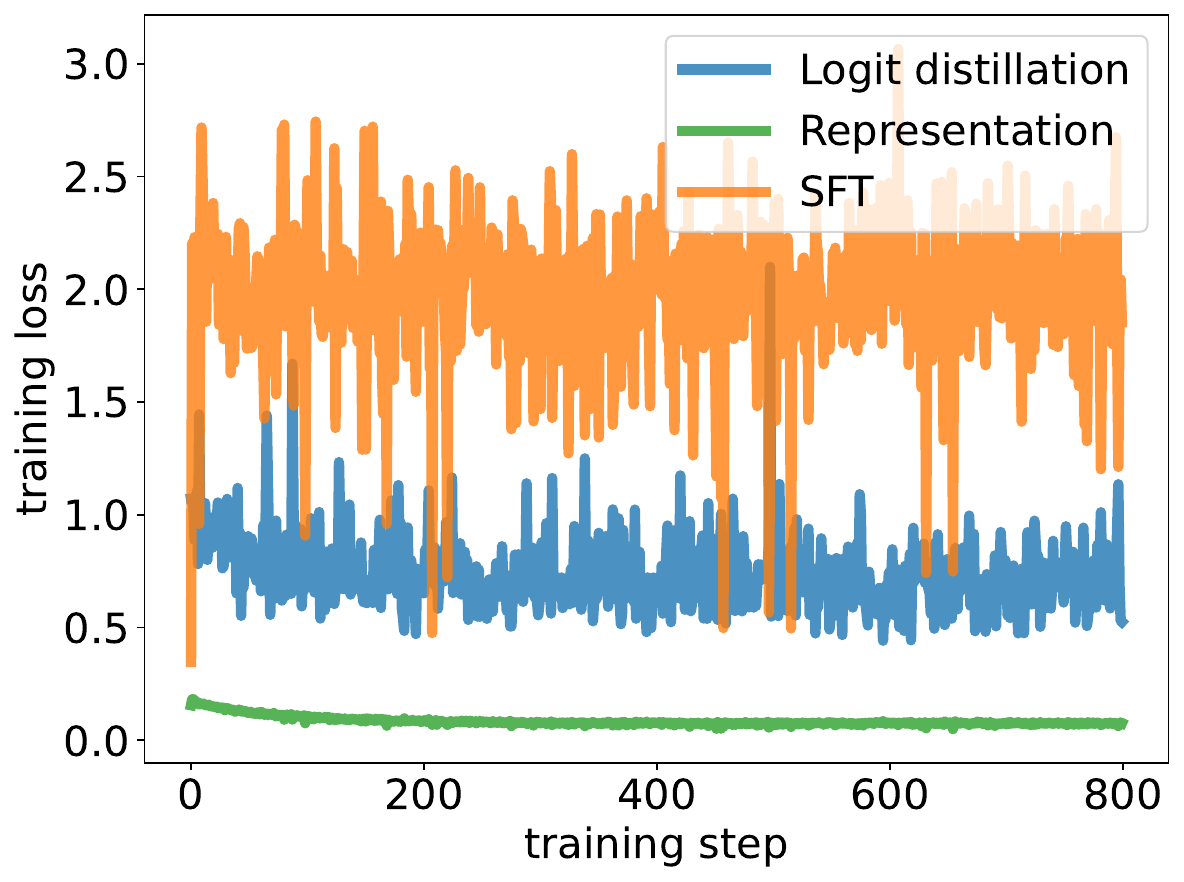}
    }

    \subfloat{
        \includegraphics[width=0.245\textwidth]{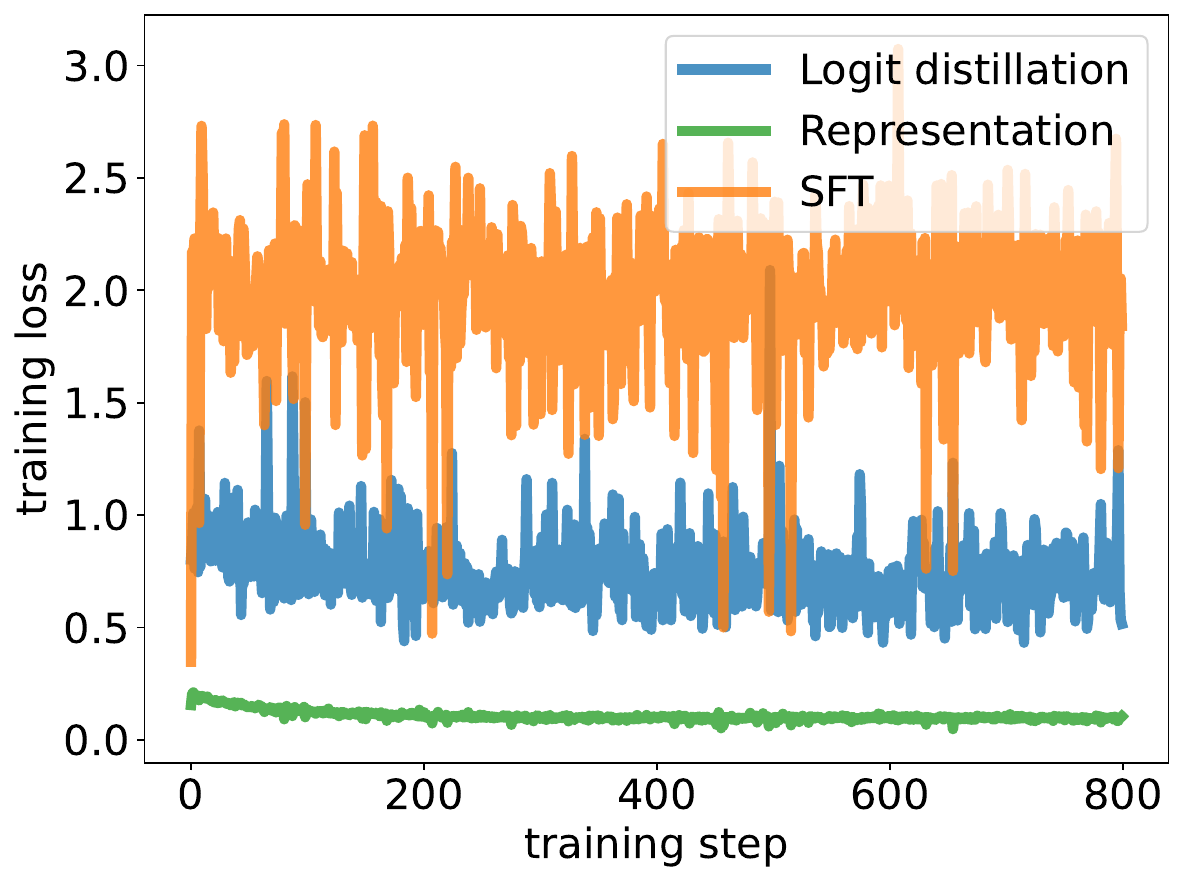}
    }
    \subfloat{
        \includegraphics[width=0.245\textwidth]{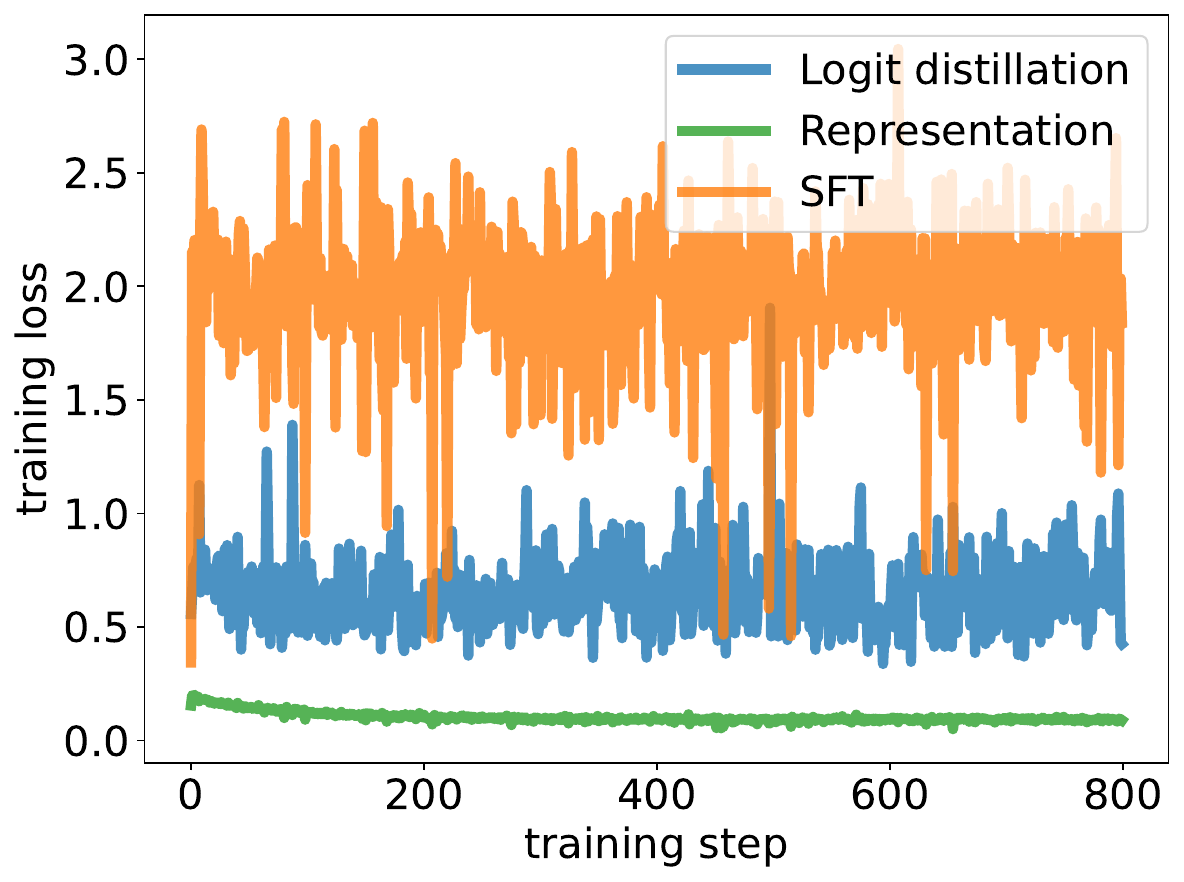}
    }
    \subfloat{
        \includegraphics[width=0.245\textwidth]{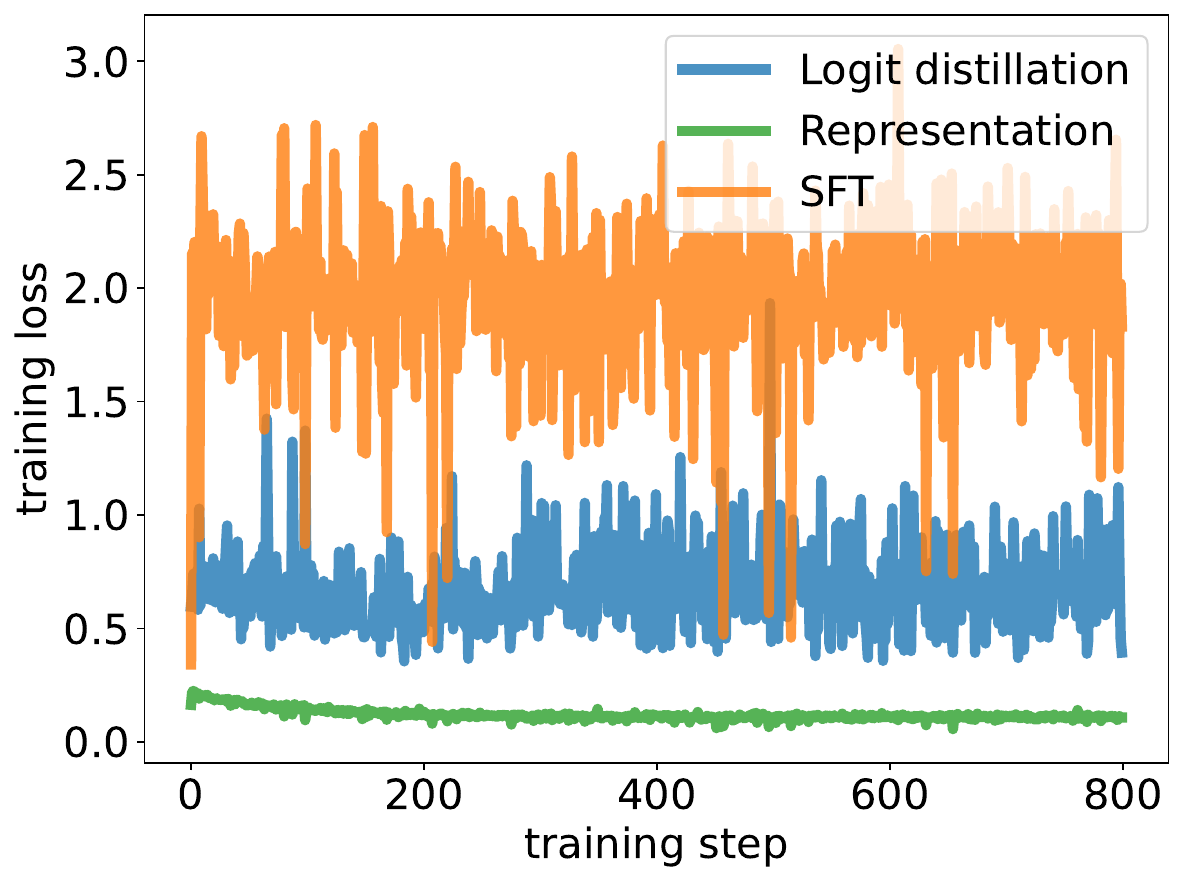}
    }
    \subfloat{
        \includegraphics[width=0.245\textwidth]{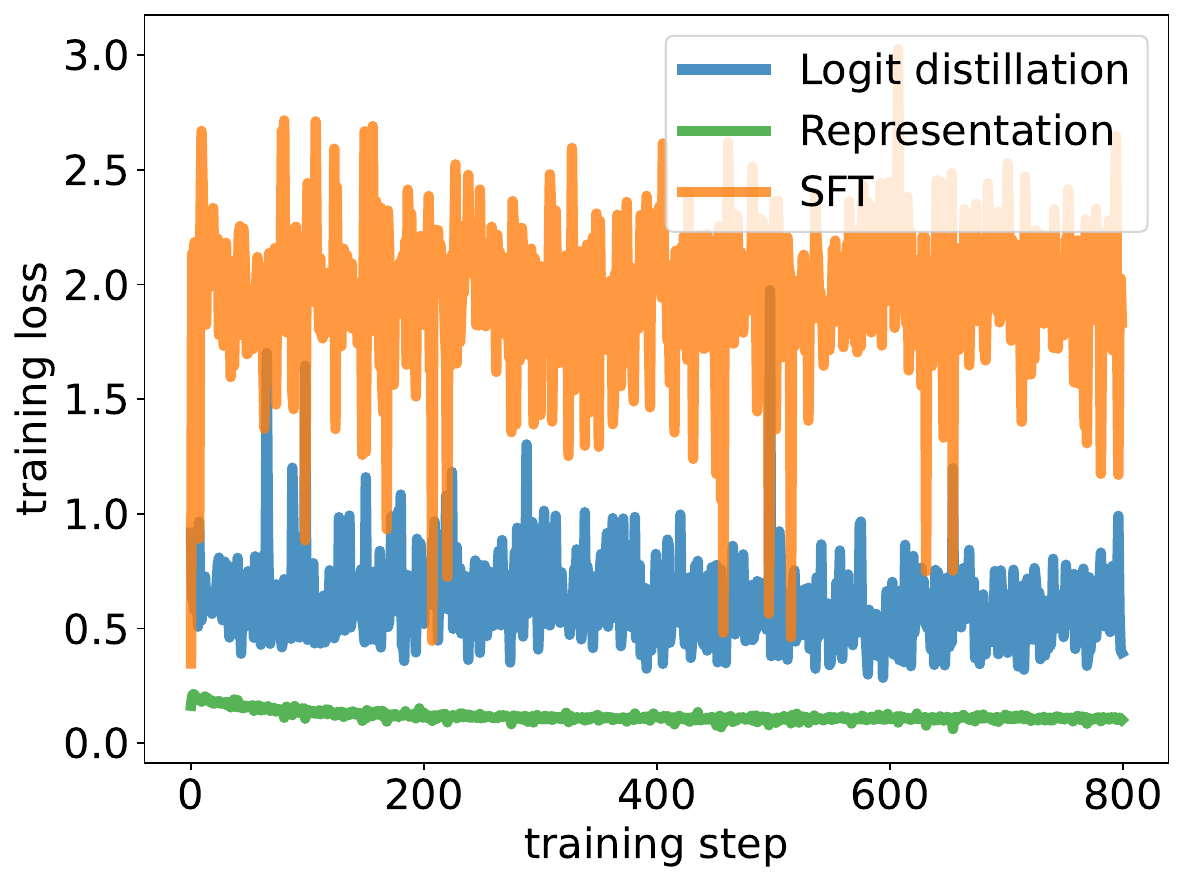}
    }

    \caption{\textbf{Low-rank linear adapter training curves for the first 24 LLaMa-2 7b blocks with a rank of 256} trained using three different objectives including (a) MSE loss defined on the representation, (b) supervised fine-tuning (SFT), and (c) logit distillation where logits are distilled from the full model. Rest of the blocks are visualized in Fig.~\ref{fig:linear_adapters_rank_256_llama2_train_loss_b}.}
    \label{fig:linear_adapters_rank_256_llama2_train_loss_a}
\end{figure}

\begin{figure}[t]
    \centering
    \subfloat{
        \includegraphics[width=0.245\textwidth]{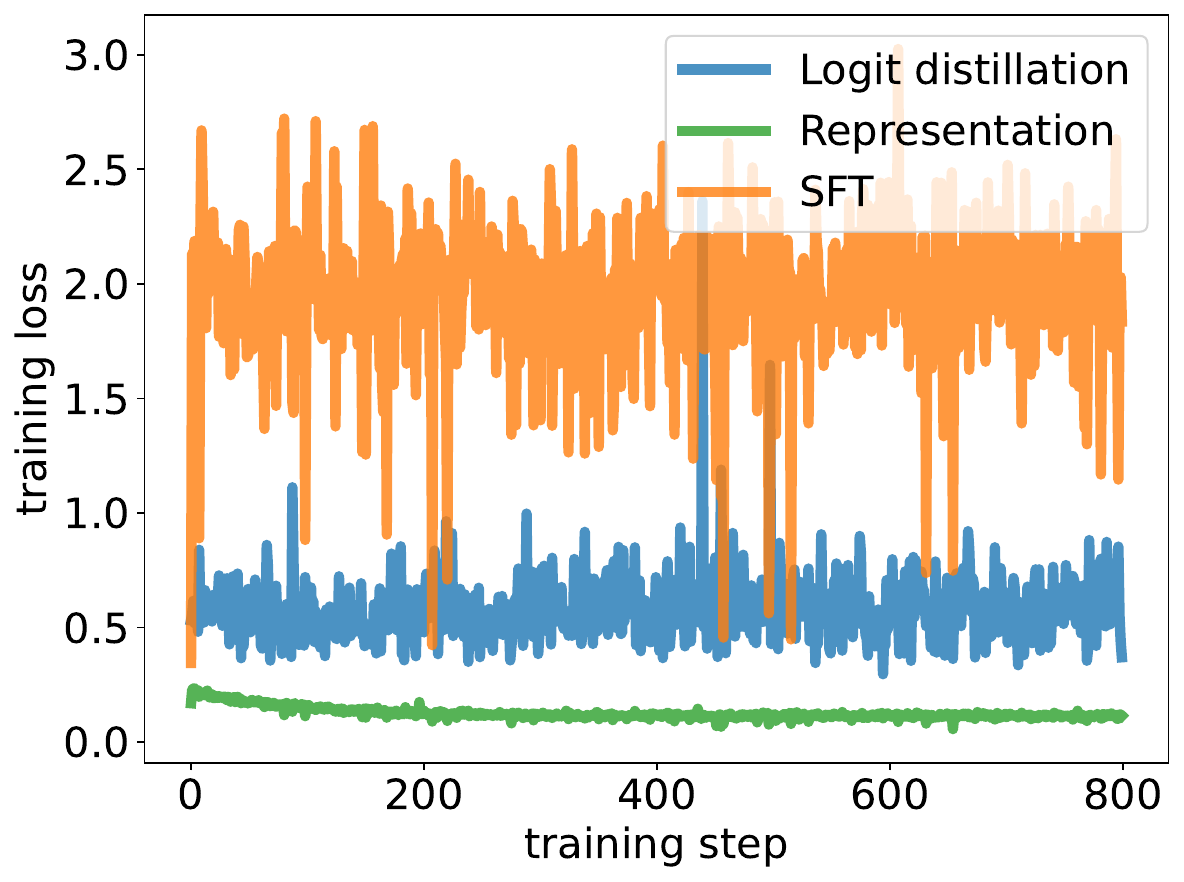}
    }
    \subfloat{
        \includegraphics[width=0.245\textwidth]{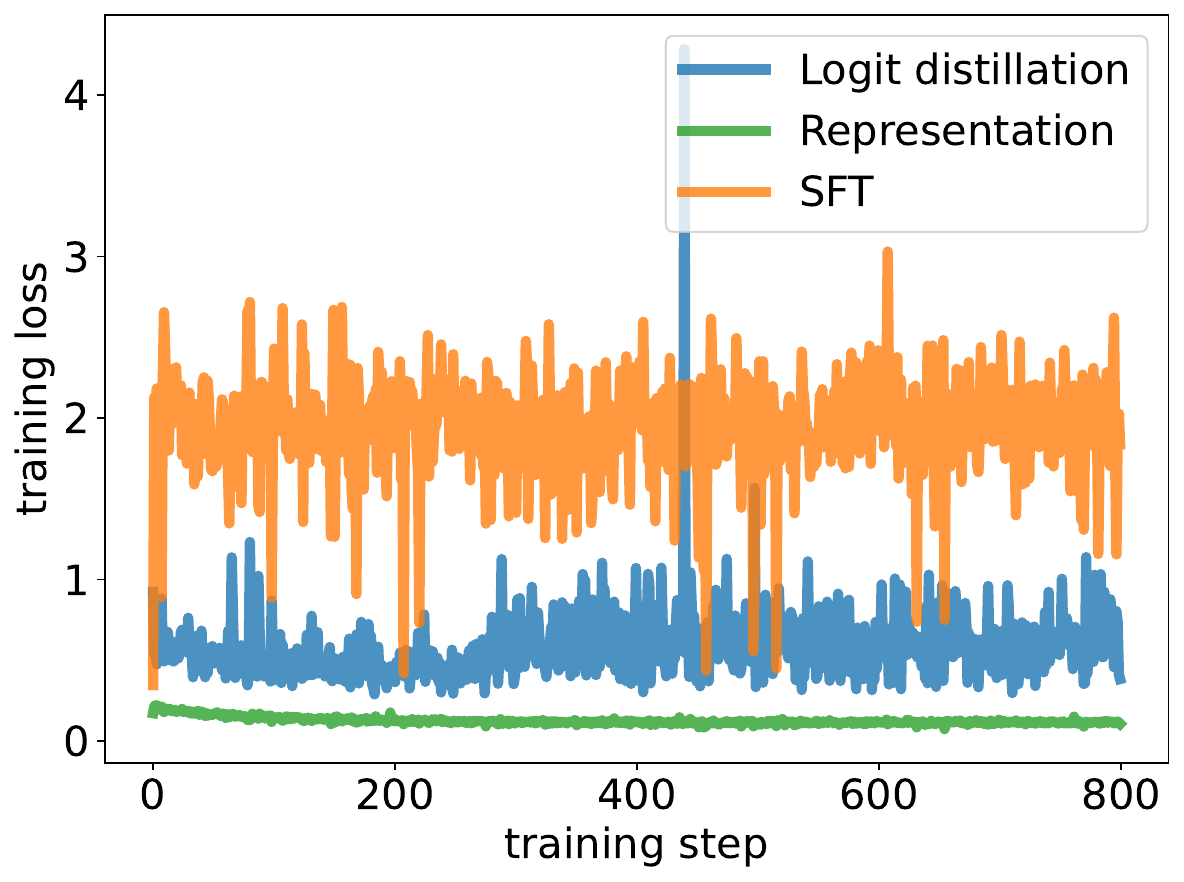}
    }
    \subfloat{
        \includegraphics[width=0.245\textwidth]{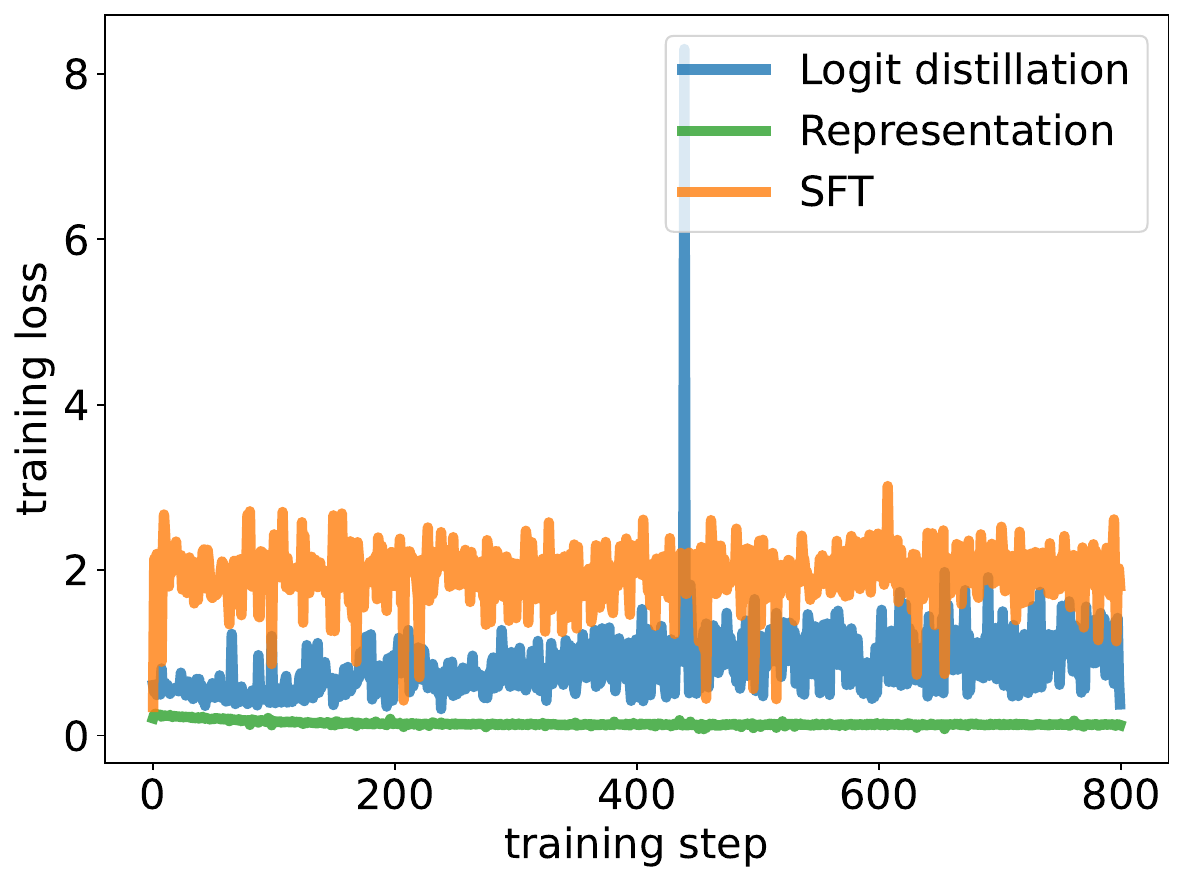}
    }
    \subfloat{
        \includegraphics[width=0.245\textwidth]{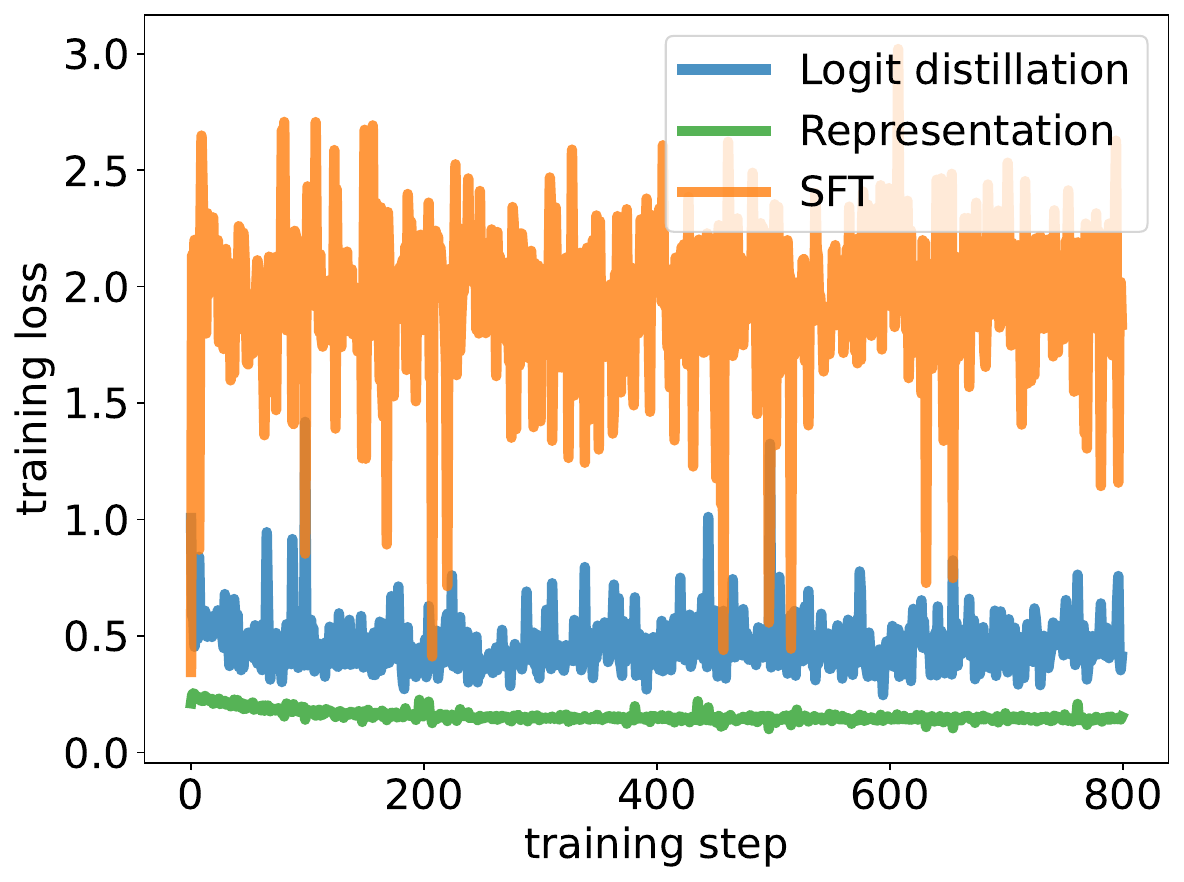}
    }

    \subfloat{
        \includegraphics[width=0.245\textwidth]{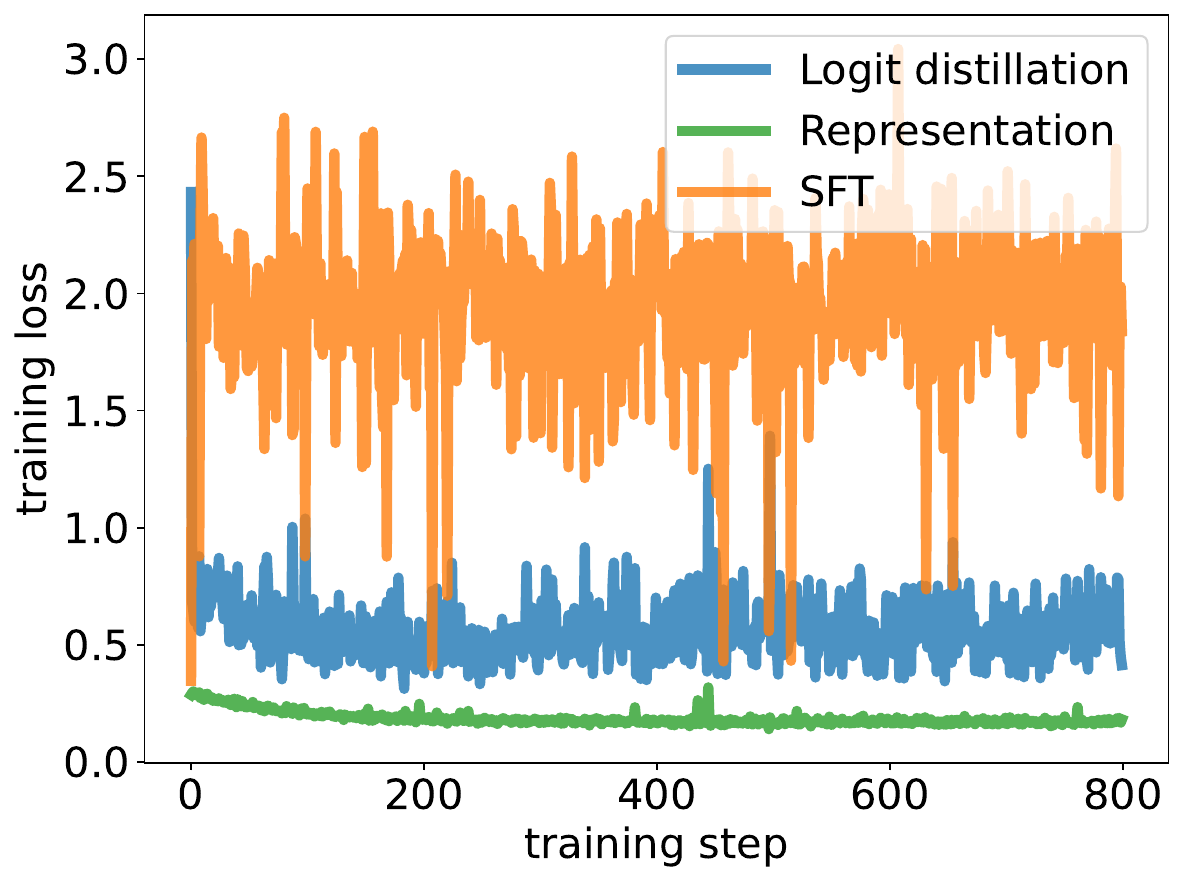}
    }
    \subfloat{
        \includegraphics[width=0.245\textwidth]{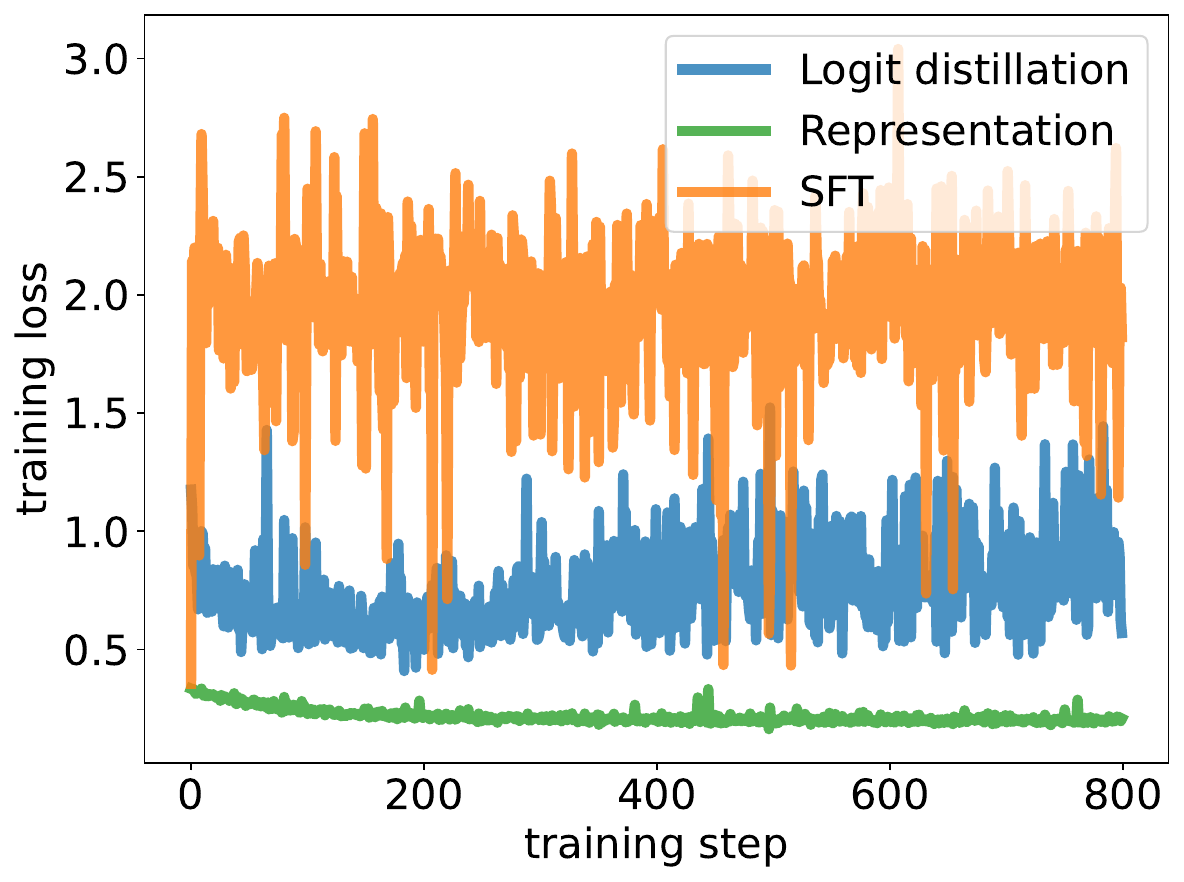}
    }
    \subfloat{
        \includegraphics[width=0.245\textwidth]{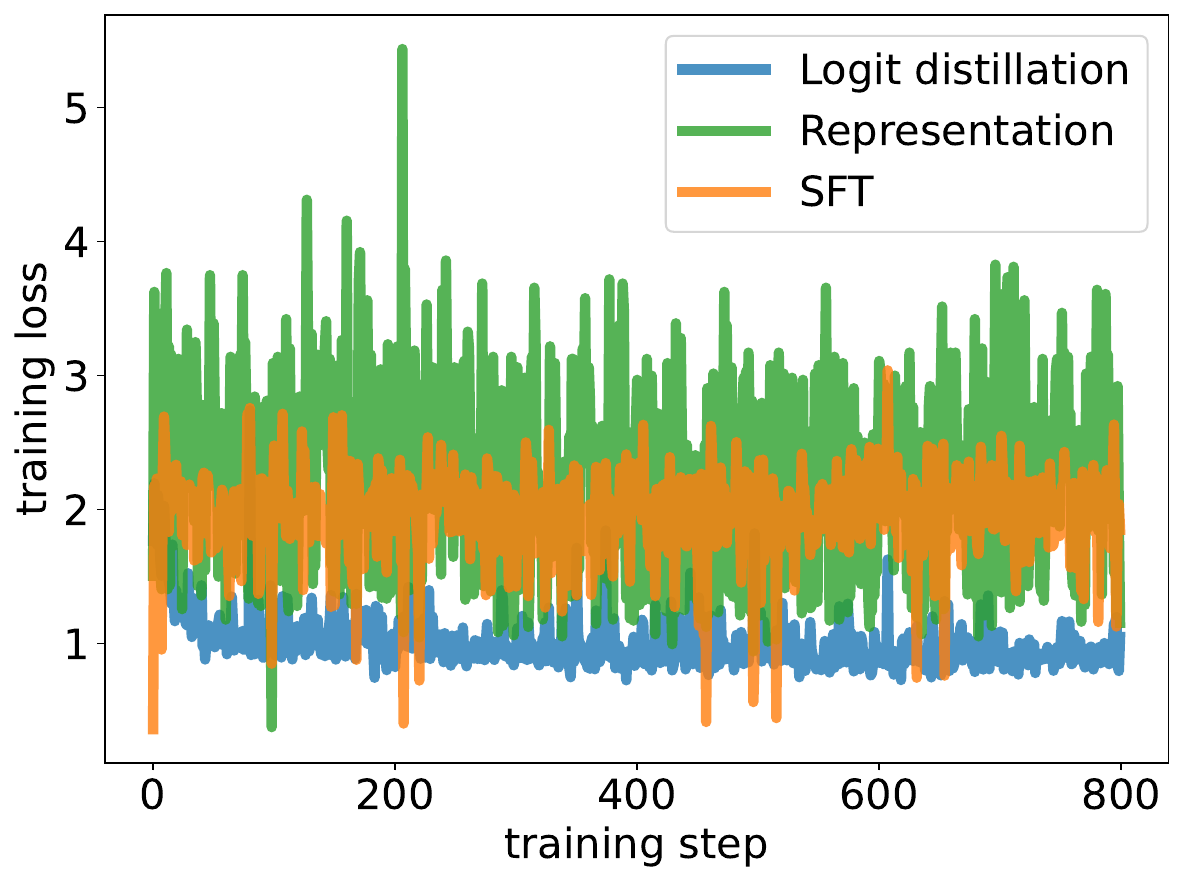}
    }
    \subfloat{
        \includegraphics[width=0.245\textwidth]{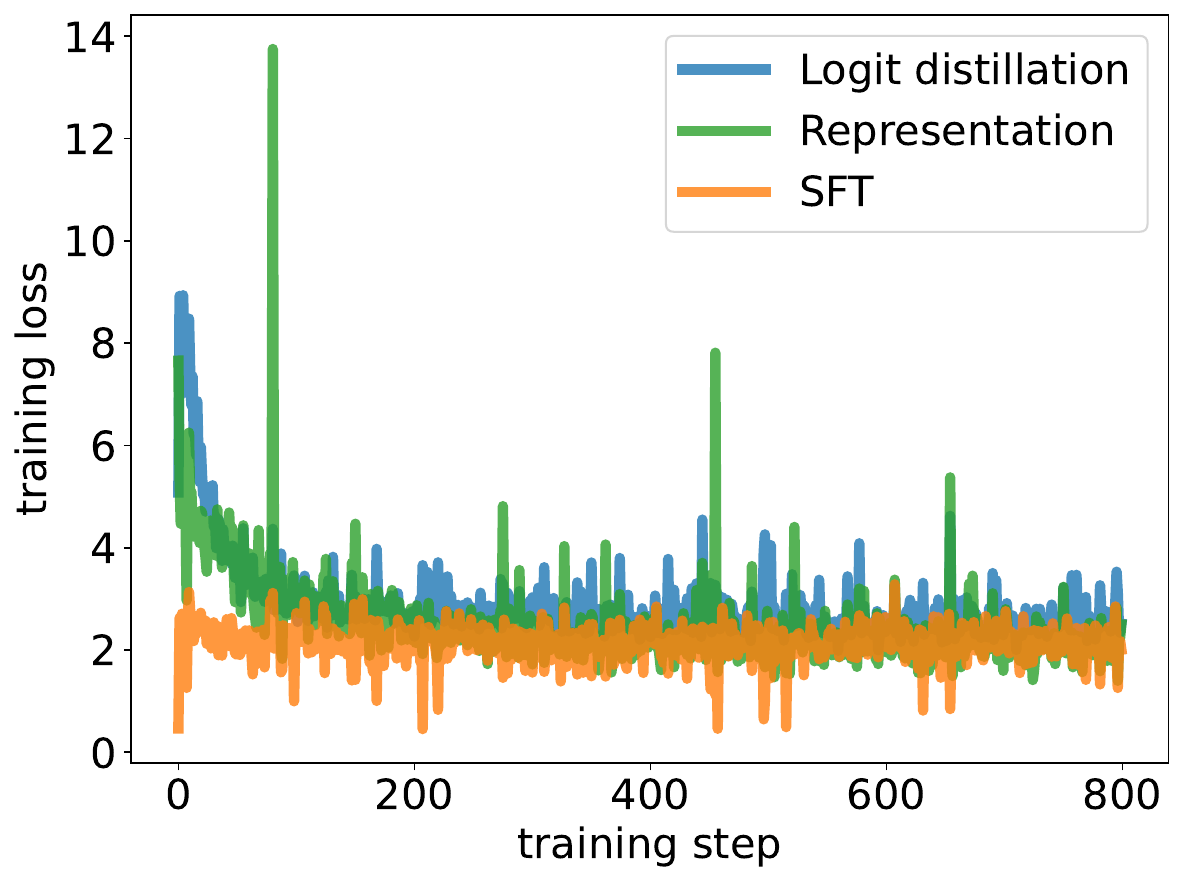}
    }

    \caption{\textbf{Low-rank linear adapter training curves for the last 8 LLaMa-2 7b blocks with a rank of 256} trained using three different objectives including (a) MSE loss defined on the representation, (b) supervised fine-tuning (SFT), and (c) logit distillation where logits are distilled from the full model. The first set of blocks are visualized in Fig.~\ref{fig:linear_adapters_rank_256_llama2_train_loss_a}.}
    \label{fig:linear_adapters_rank_256_llama2_train_loss_b}
\end{figure}

The loss curves for the training of the low-rank adapter with a rank of 256 on LLaMa-2 are visualized in Fig.~\ref{fig:linear_adapters_rank_256_llama2_train_loss_a} and Fig.~\ref{fig:linear_adapters_rank_256_llama2_train_loss_b}.

\begin{figure}[t]
    \centering
    \subfloat{
        \includegraphics[width=0.245\textwidth]{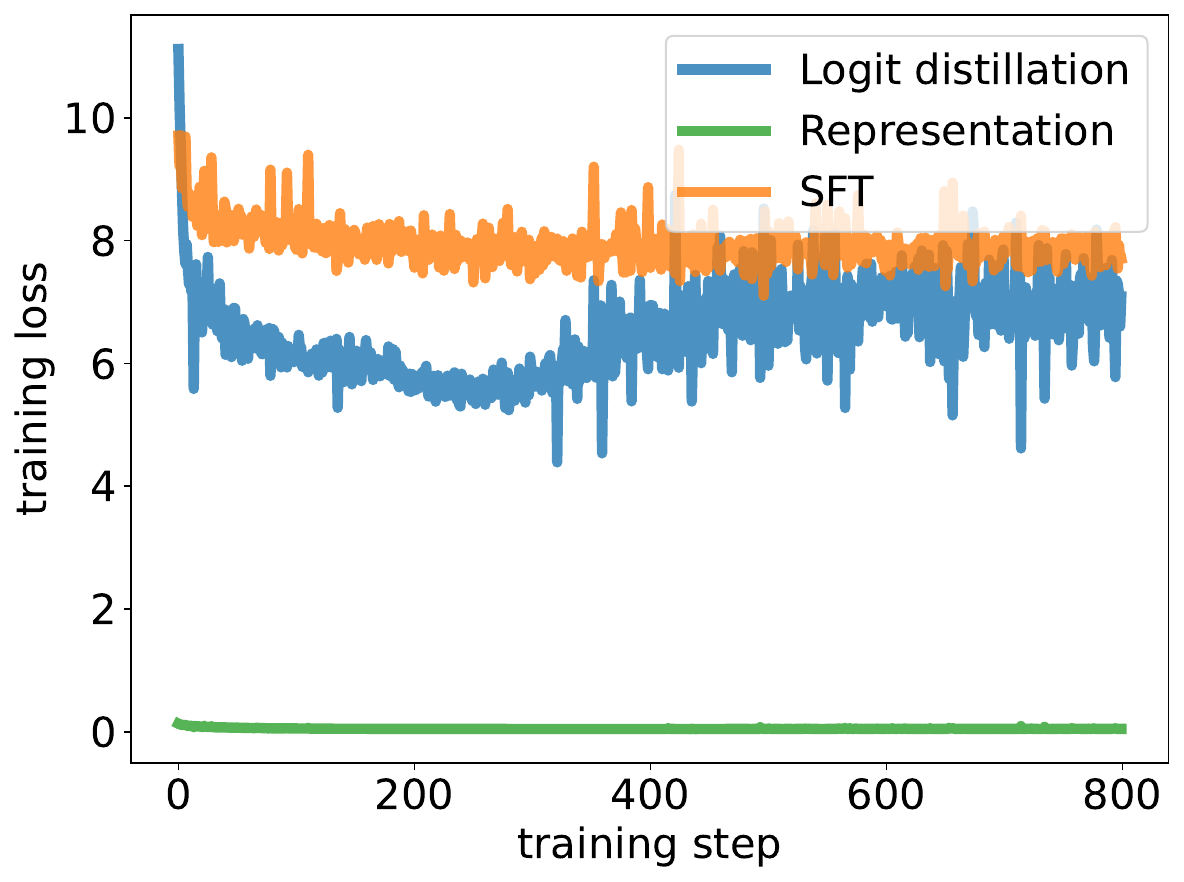}
    }
    \subfloat{
        \includegraphics[width=0.245\textwidth]{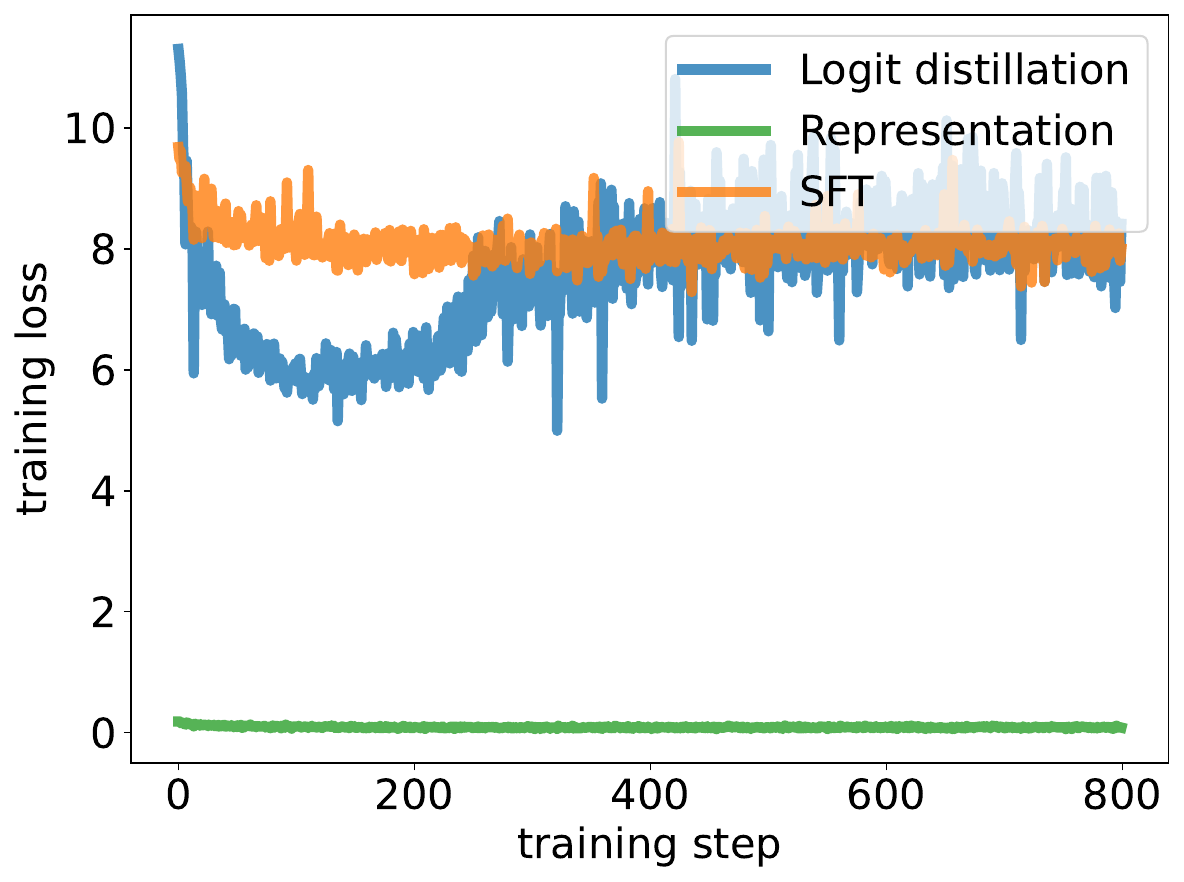}
    }
    \subfloat{
        \includegraphics[width=0.245\textwidth]{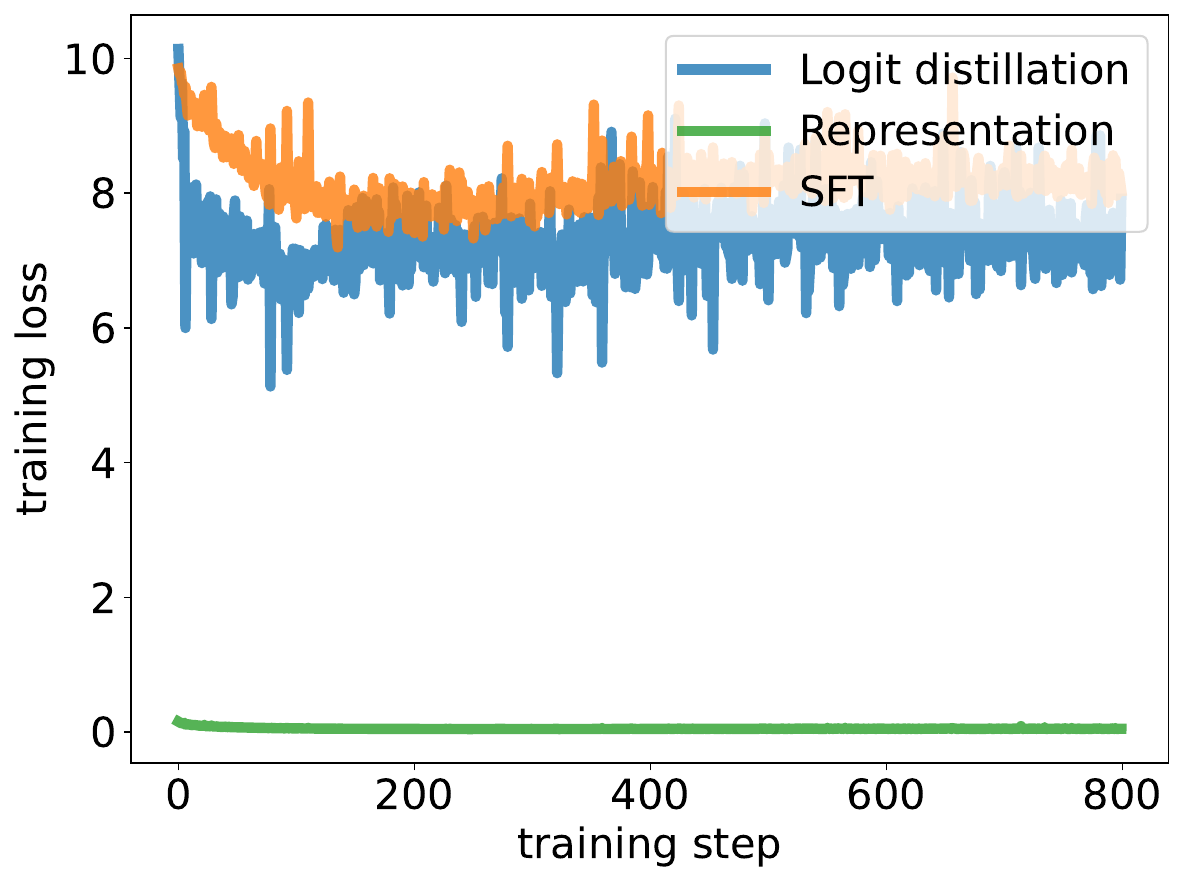}
    }
    \subfloat{
        \includegraphics[width=0.245\textwidth]{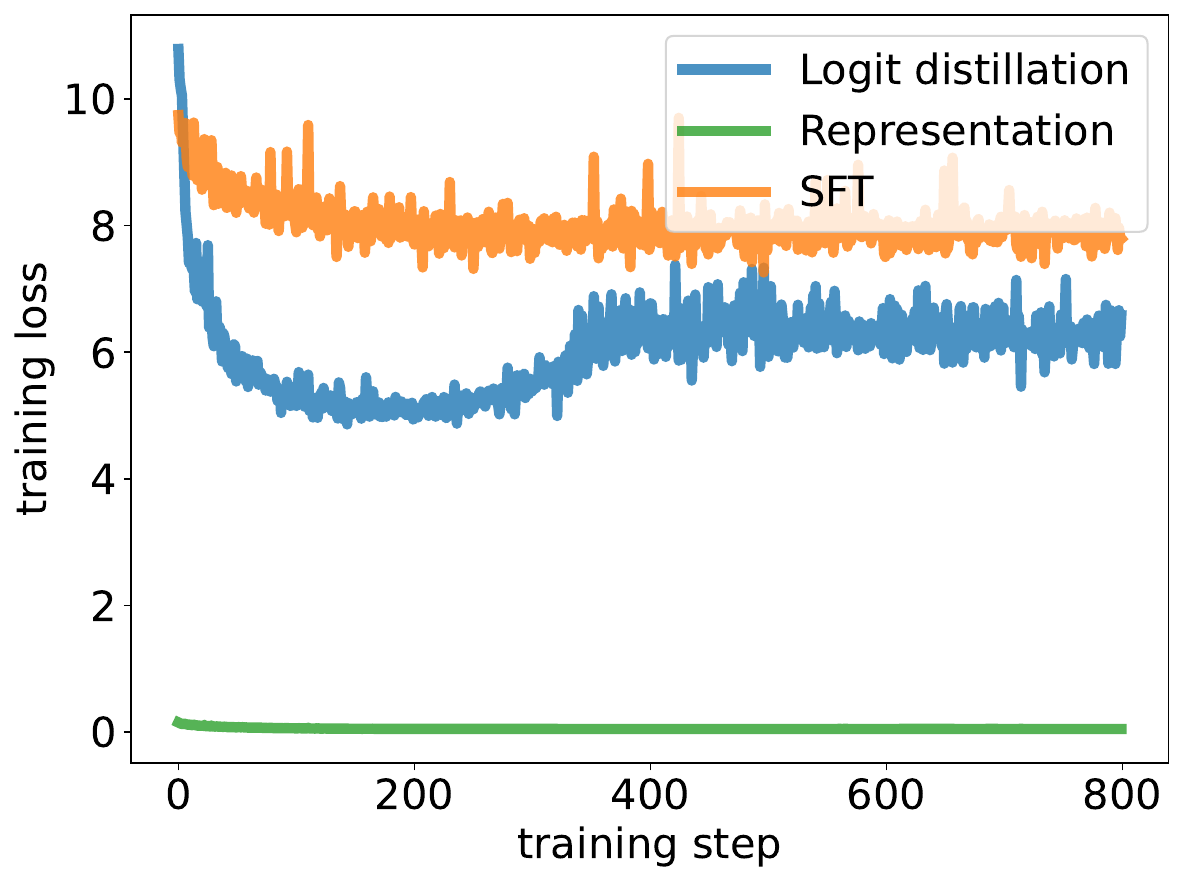}
    }

    \subfloat{
        \includegraphics[width=0.245\textwidth]{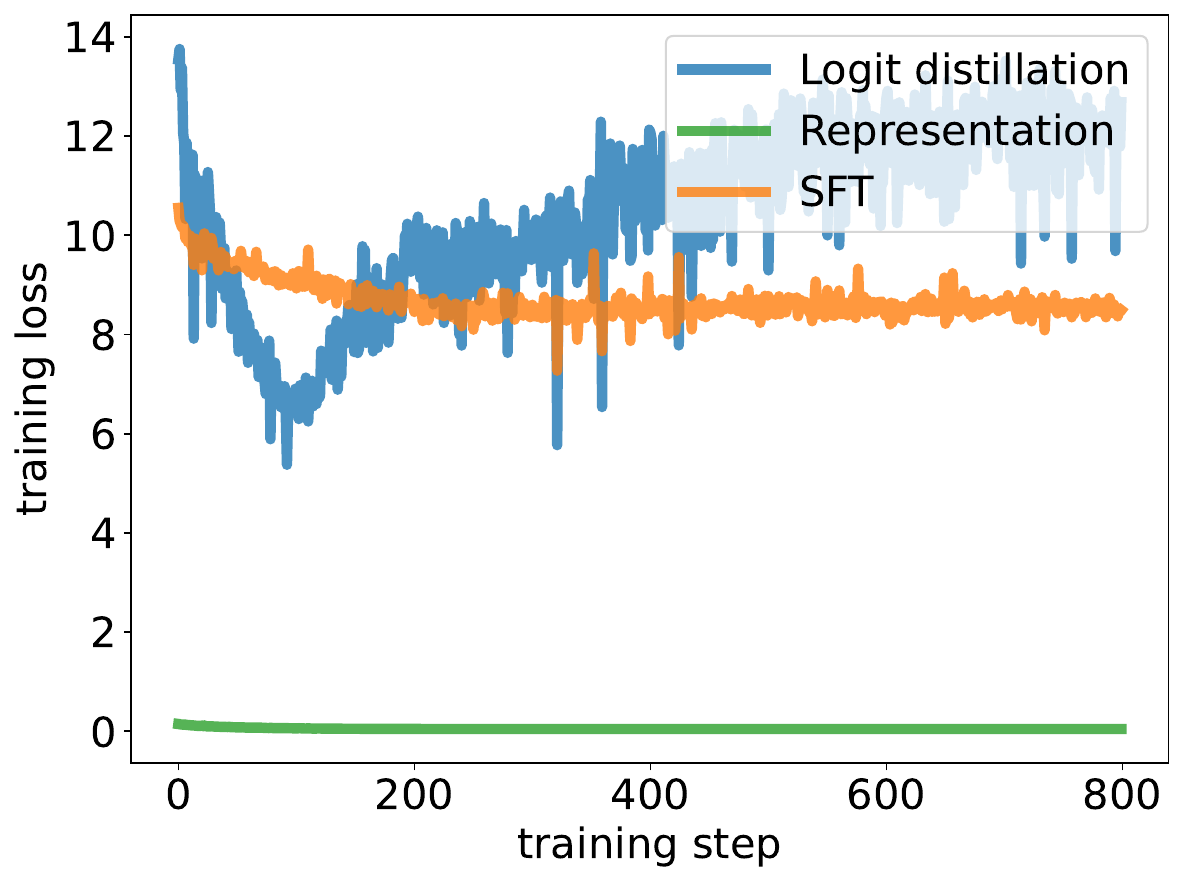}
    }
    \subfloat{
        \includegraphics[width=0.245\textwidth]{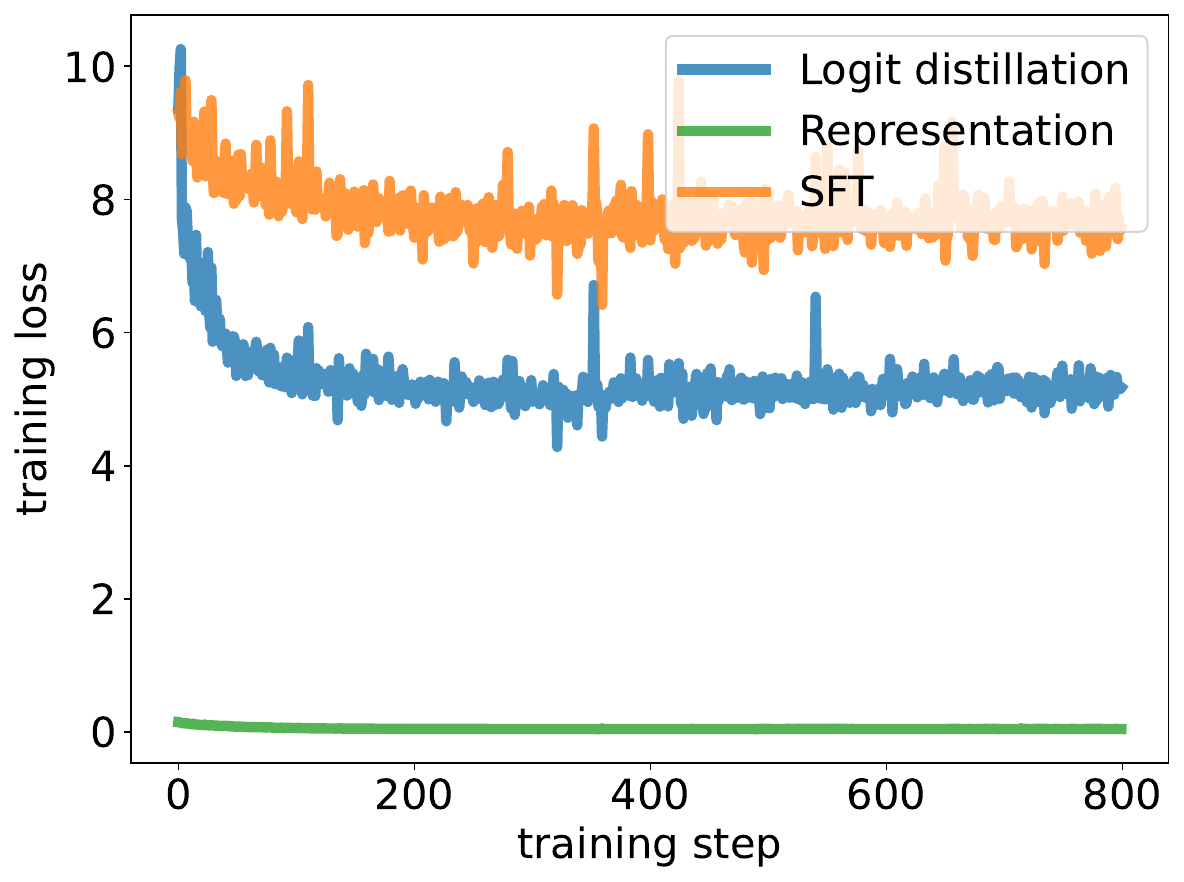}
    }
    \subfloat{
        \includegraphics[width=0.245\textwidth]{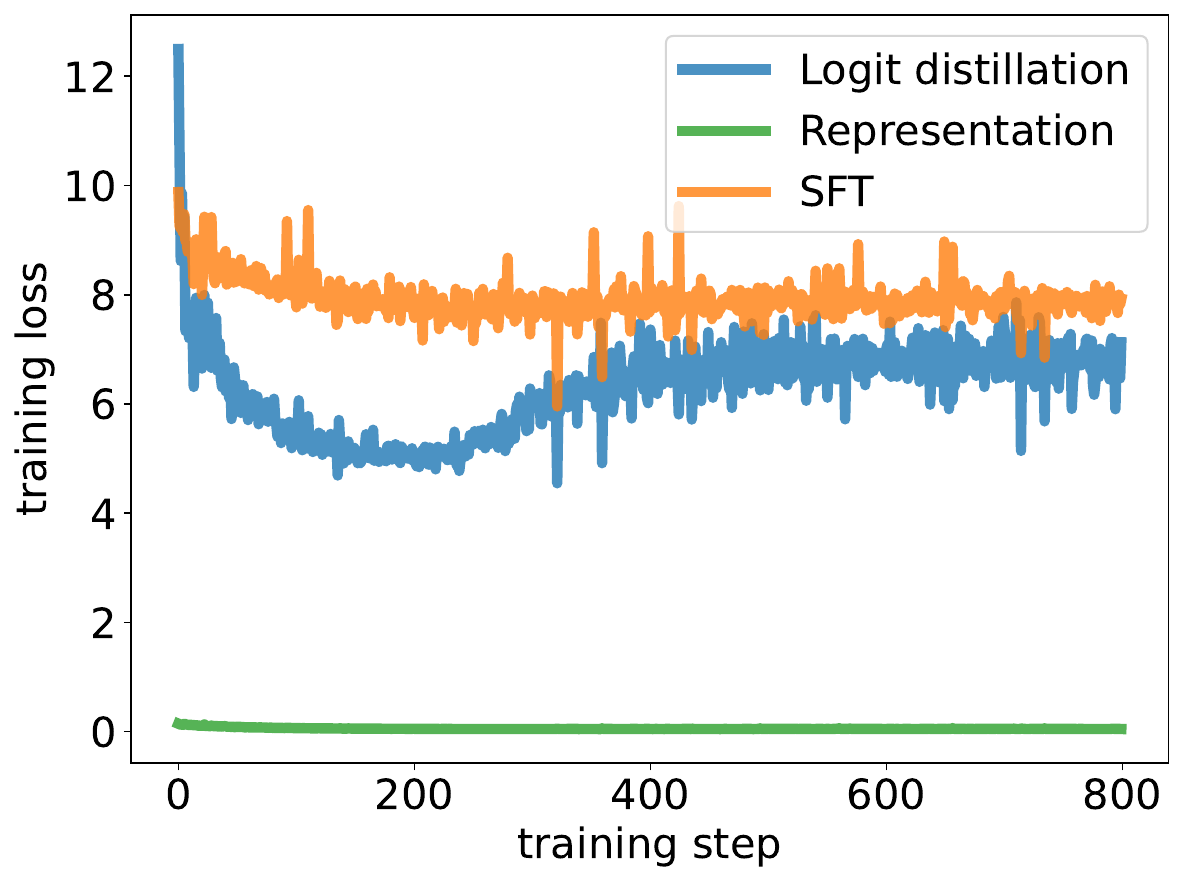}
    }
    \subfloat{
        \includegraphics[width=0.245\textwidth]{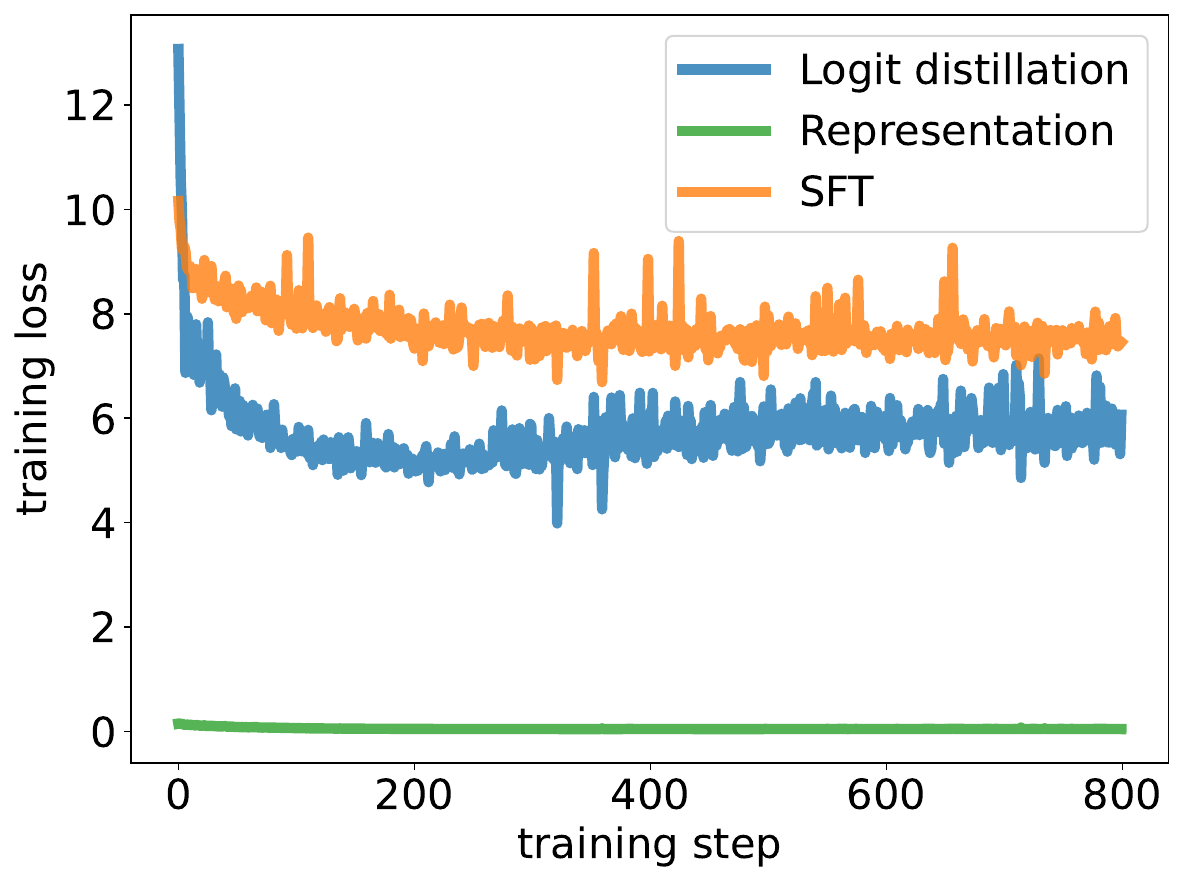}
    }

    \subfloat{
        \includegraphics[width=0.245\textwidth]{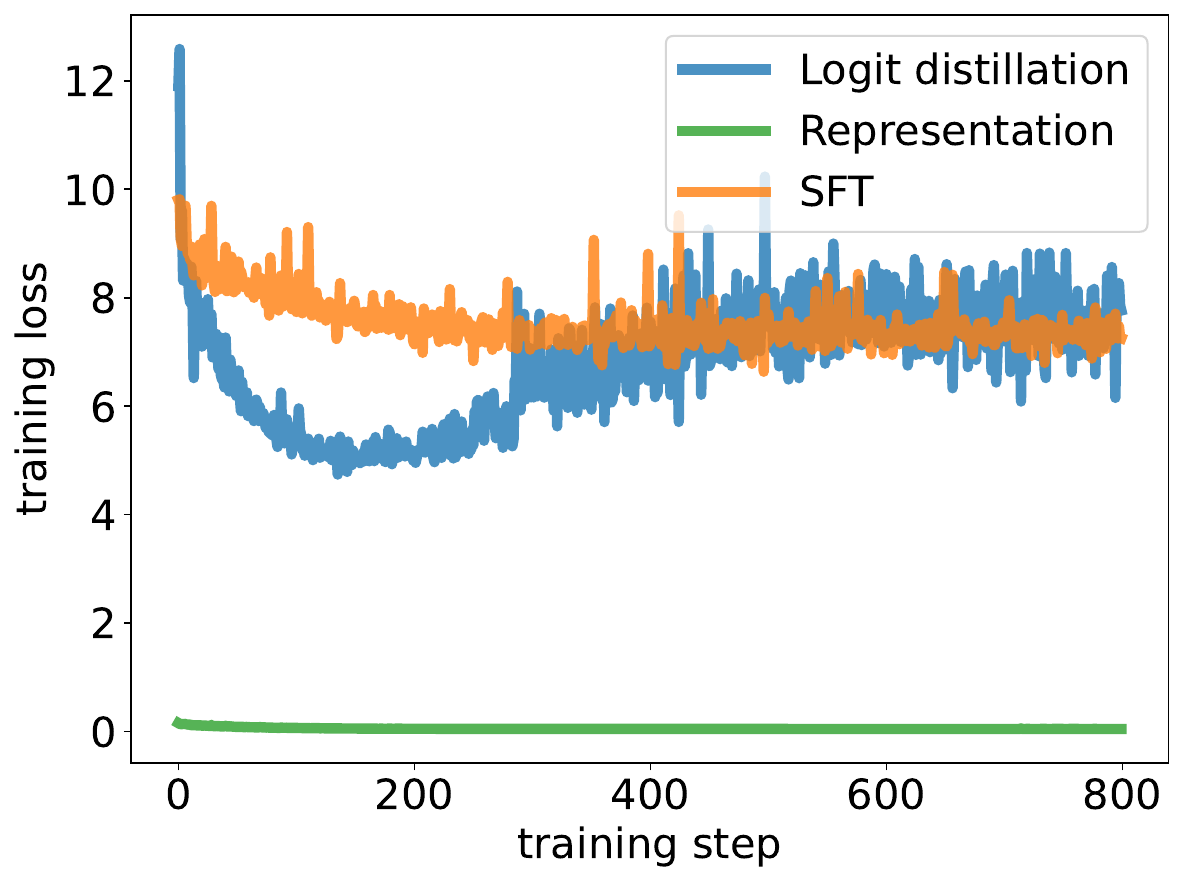}
    }
    \subfloat{
        \includegraphics[width=0.245\textwidth]{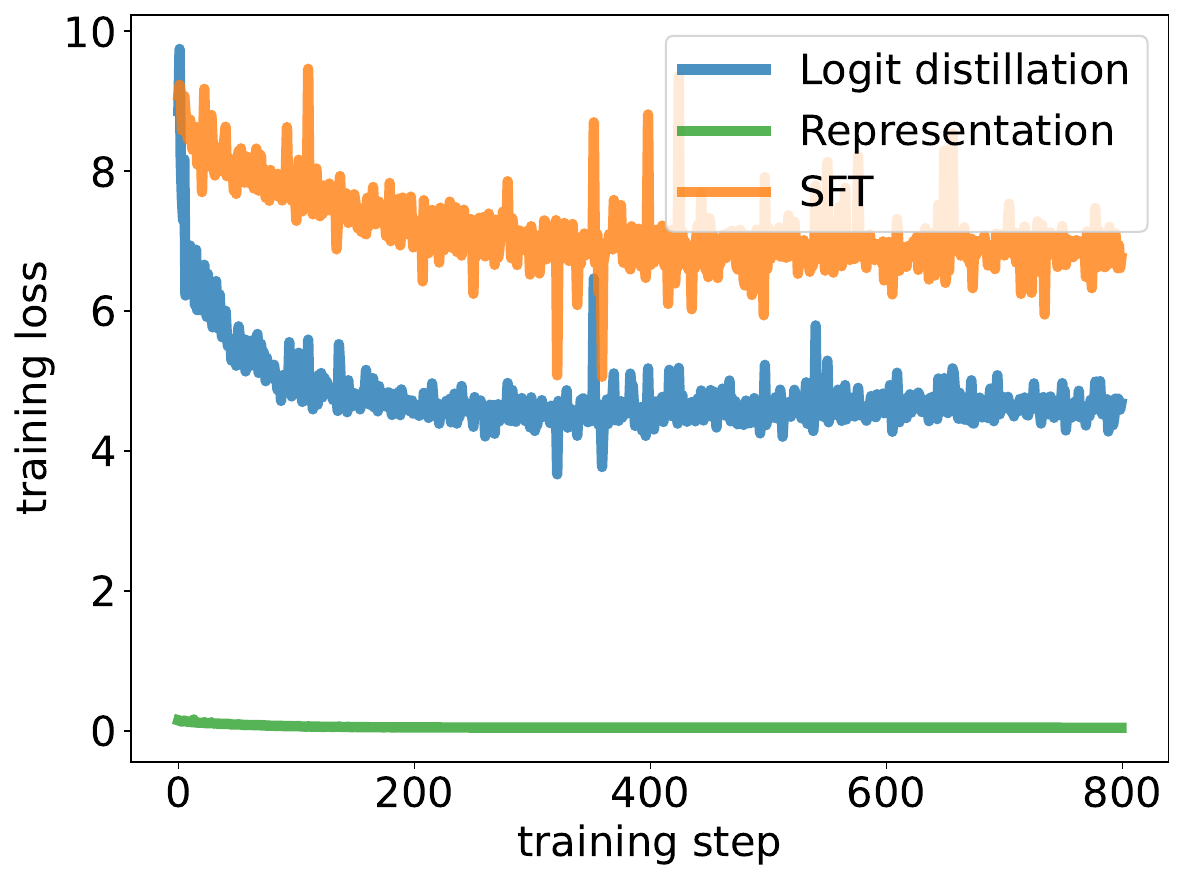}
    }
    \subfloat{
        \includegraphics[width=0.245\textwidth]{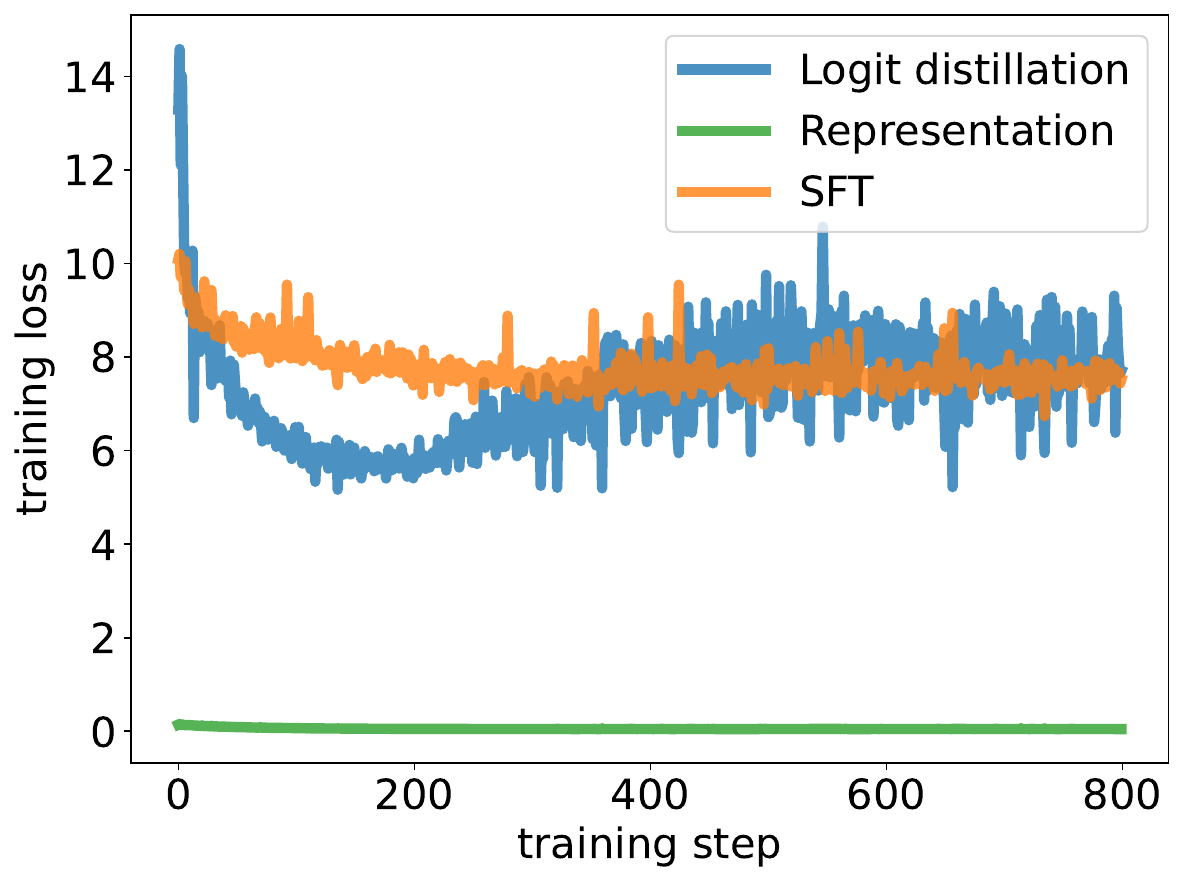}
    }
    \subfloat{
        \includegraphics[width=0.245\textwidth]{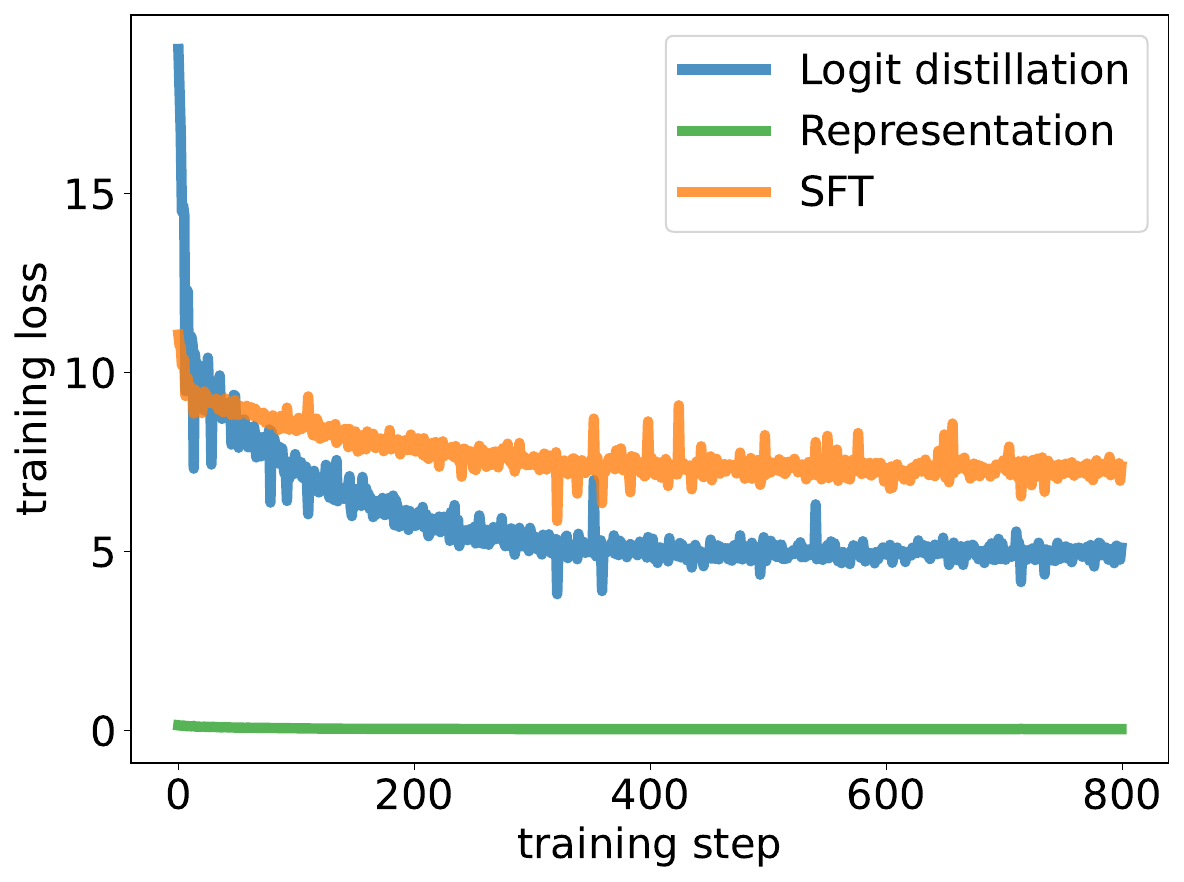}
    }

    \subfloat{
        \includegraphics[width=0.245\textwidth]{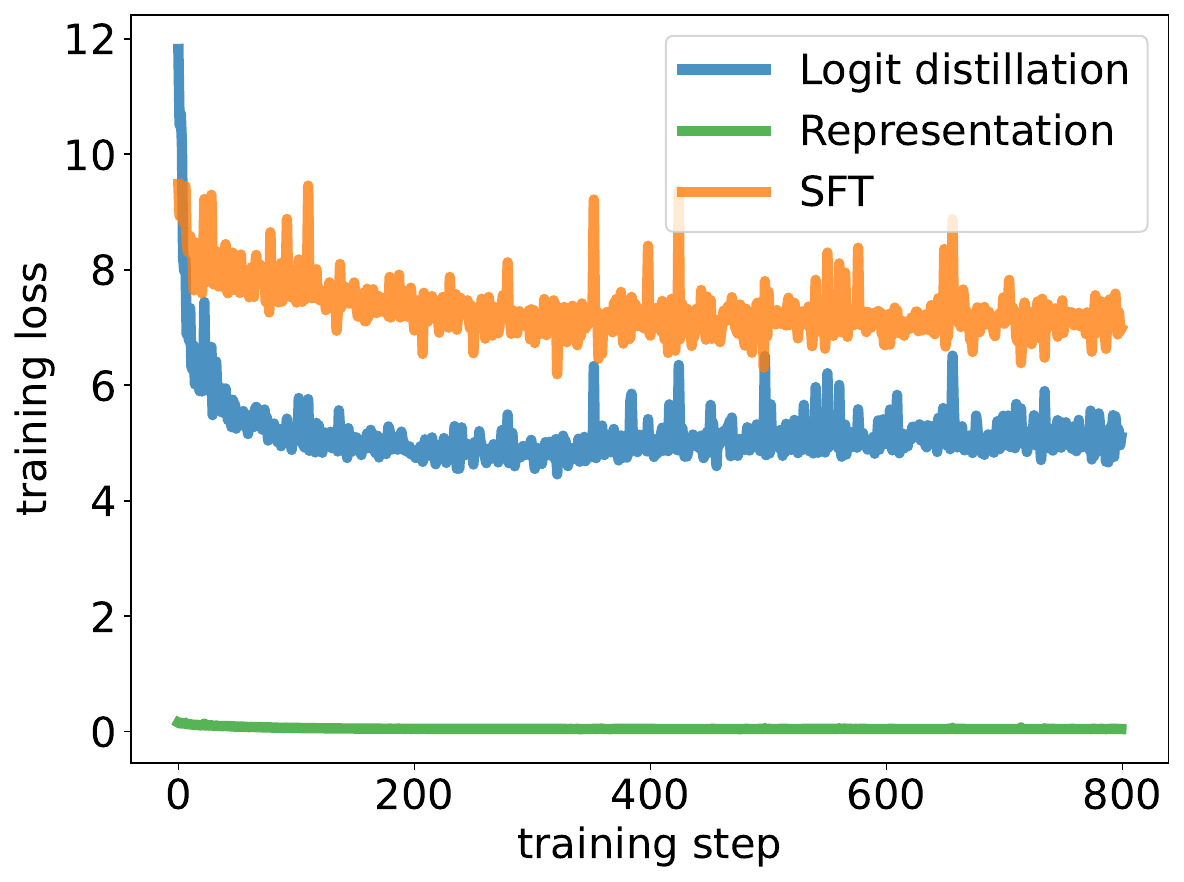}
    }
    \subfloat{
        \includegraphics[width=0.245\textwidth]{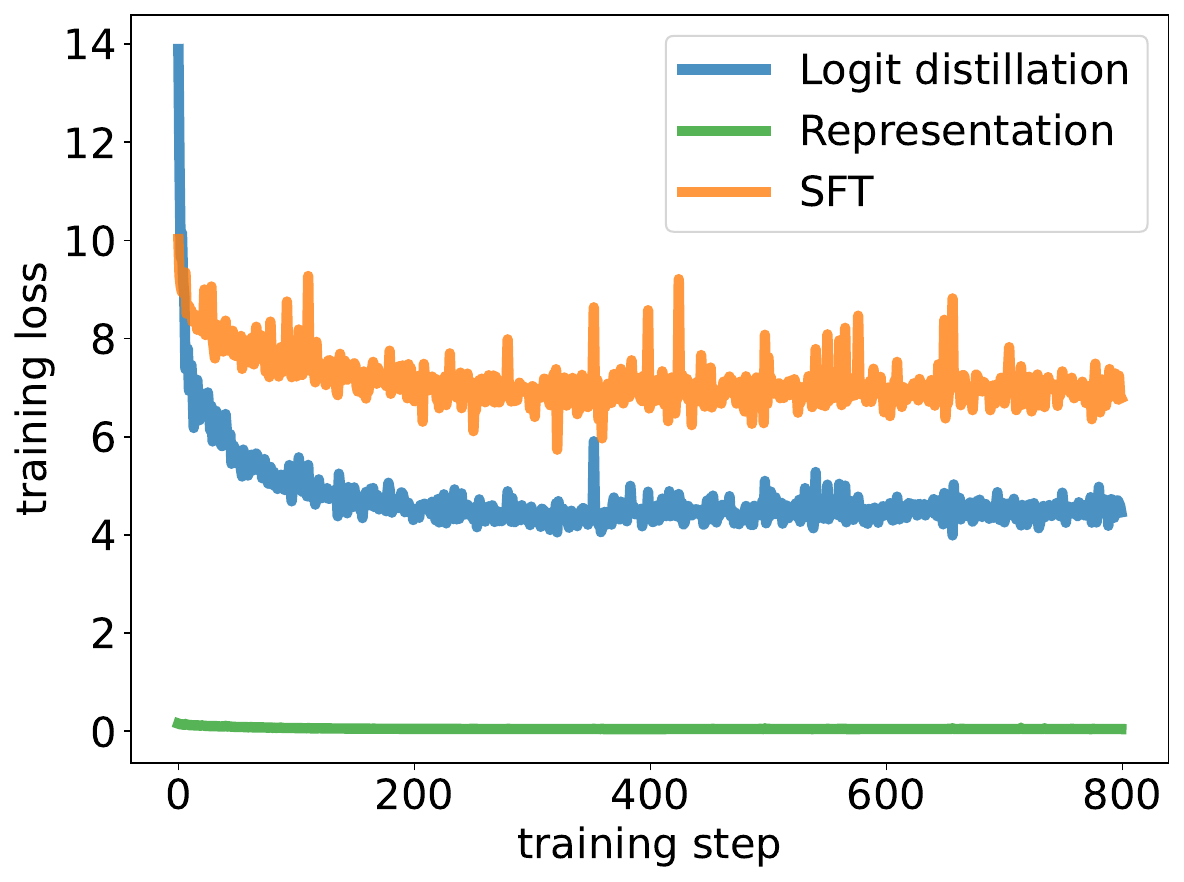}
    }
    \subfloat{
        \includegraphics[width=0.245\textwidth]{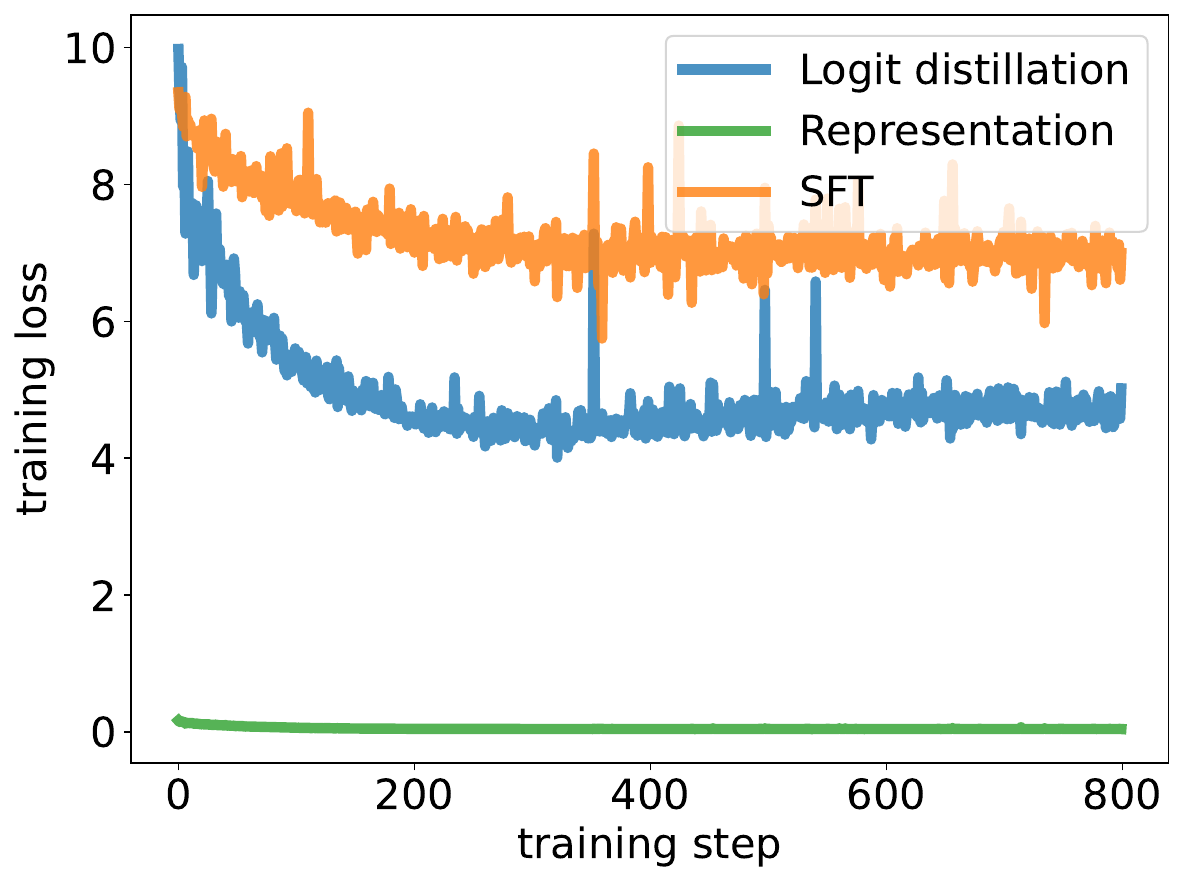}
    }
    \subfloat{
        \includegraphics[width=0.245\textwidth]{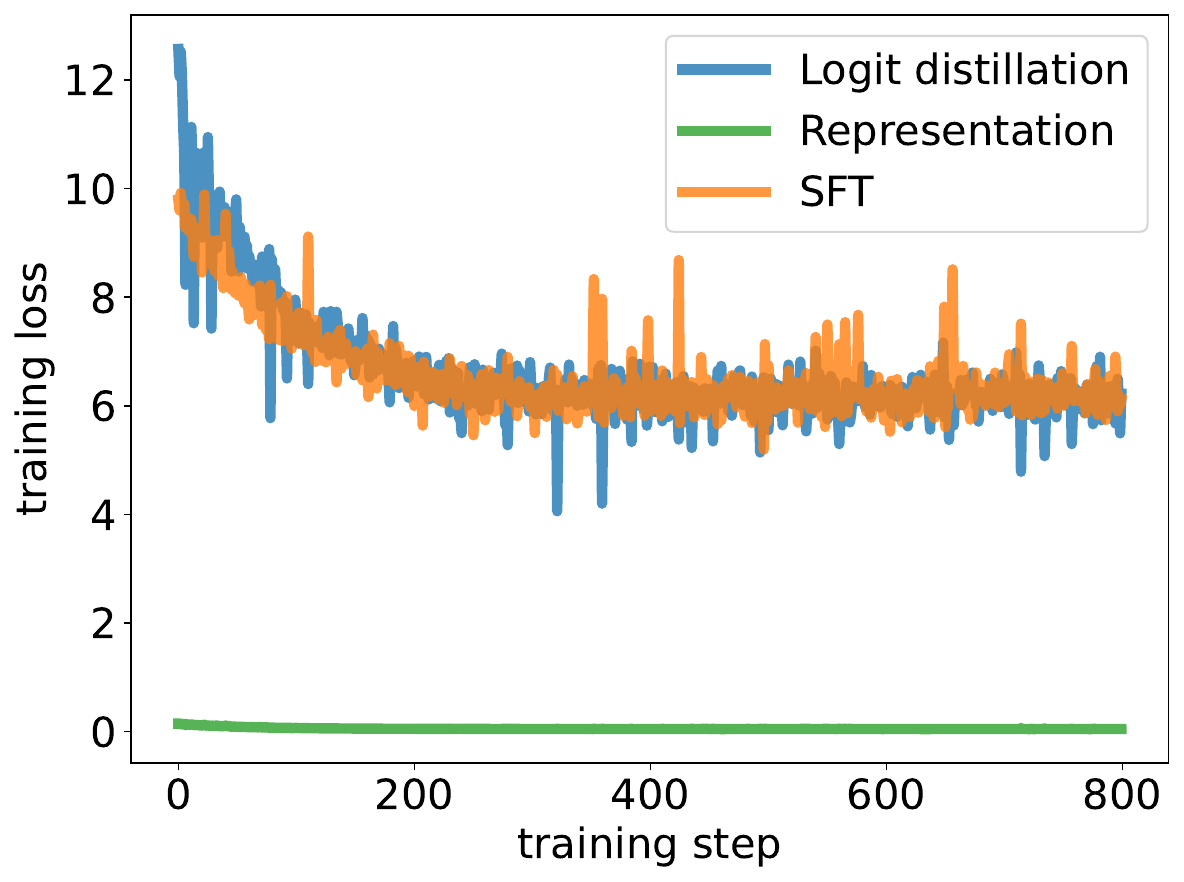}
    }

    \subfloat{
        \includegraphics[width=0.245\textwidth]{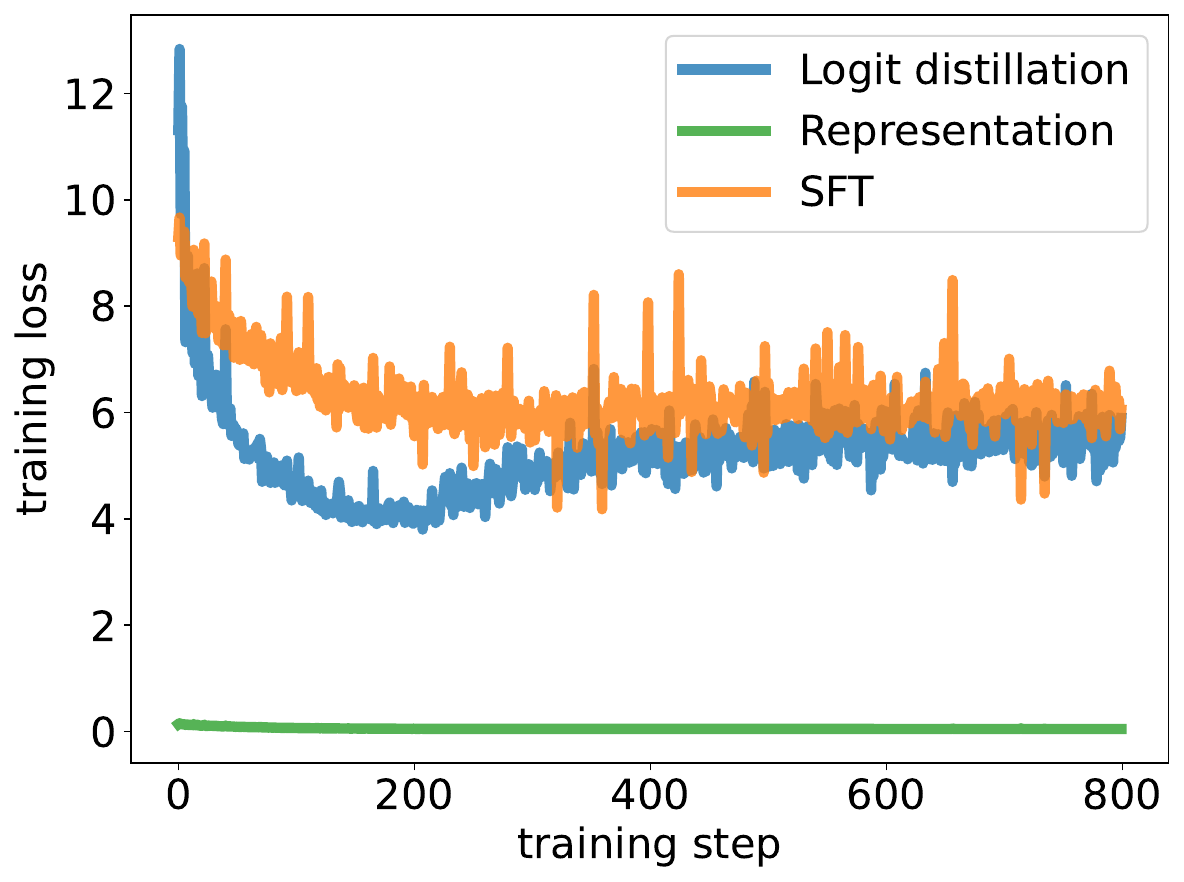}
    }
    \subfloat{
        \includegraphics[width=0.245\textwidth]{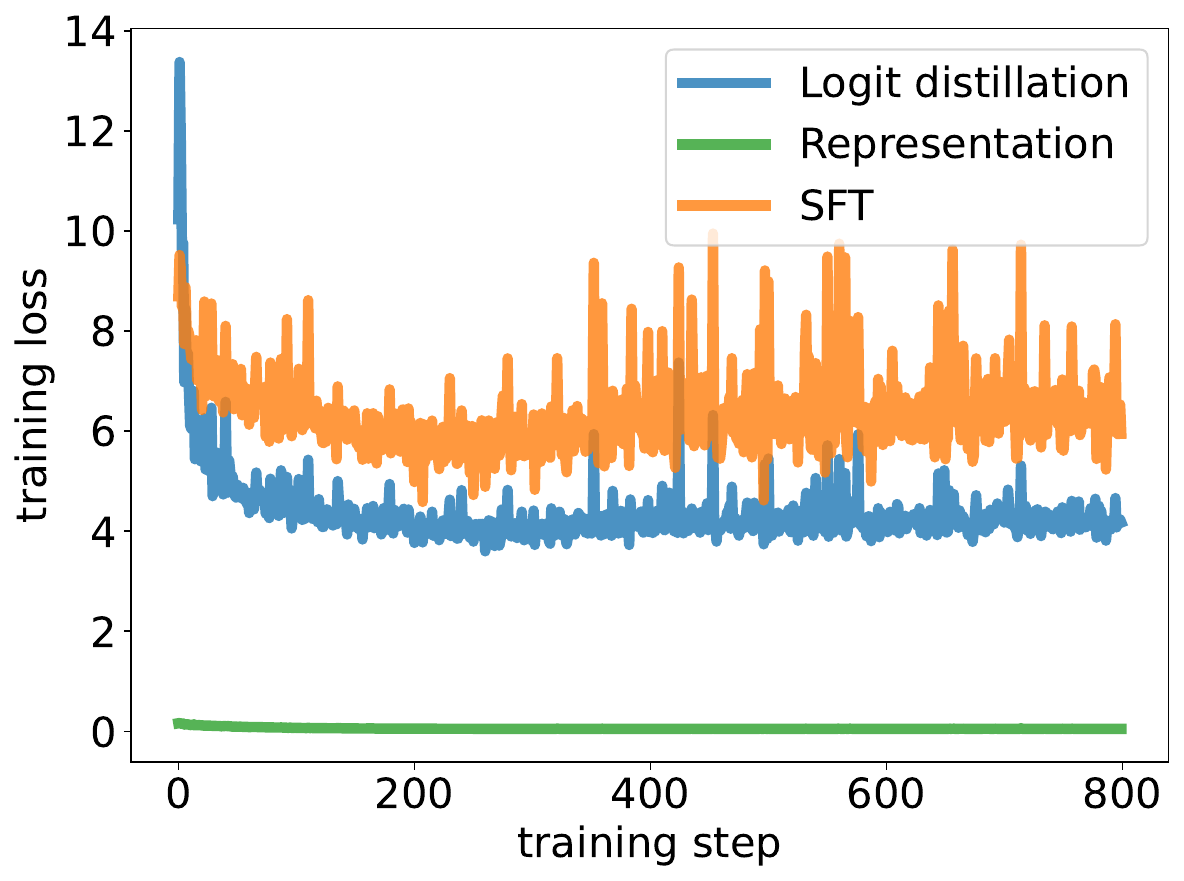}
    }
    \subfloat{
        \includegraphics[width=0.245\textwidth]{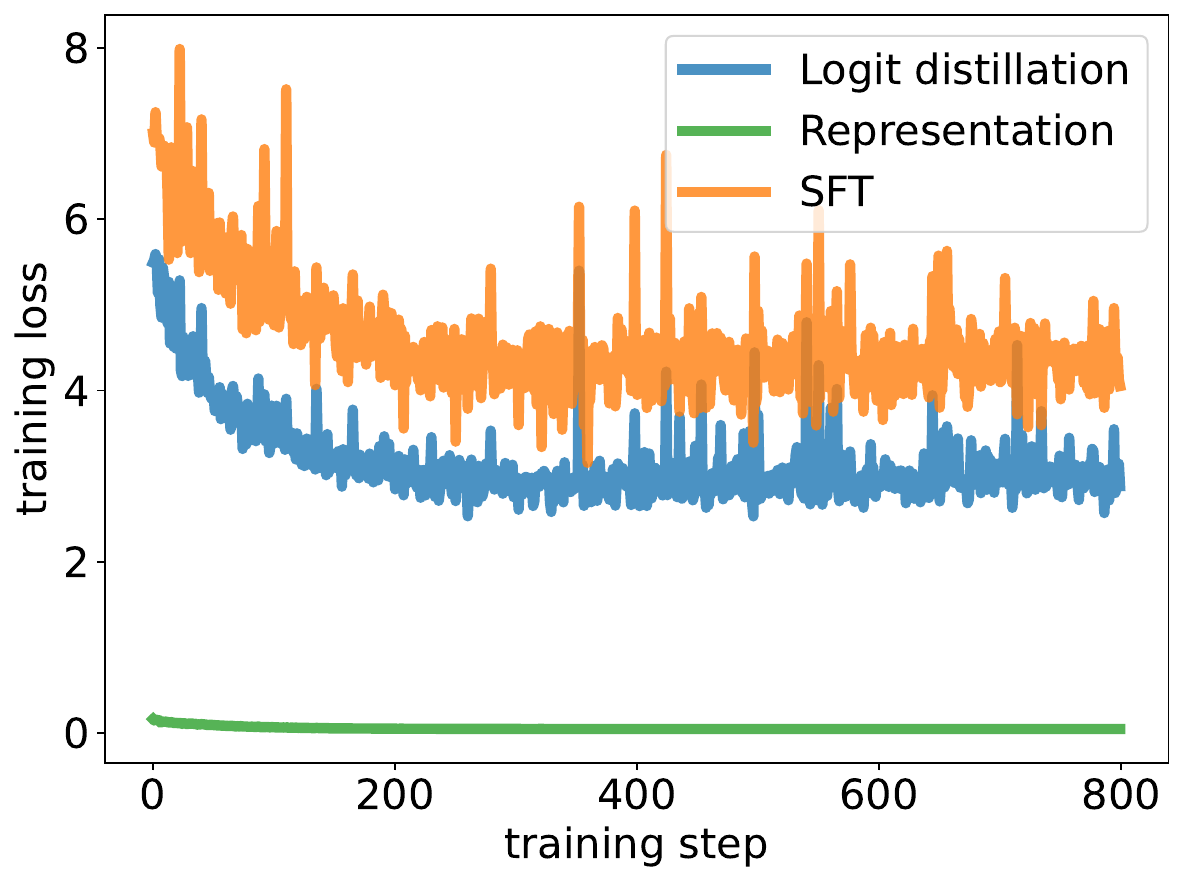}
    }
    \subfloat{
        \includegraphics[width=0.245\textwidth]{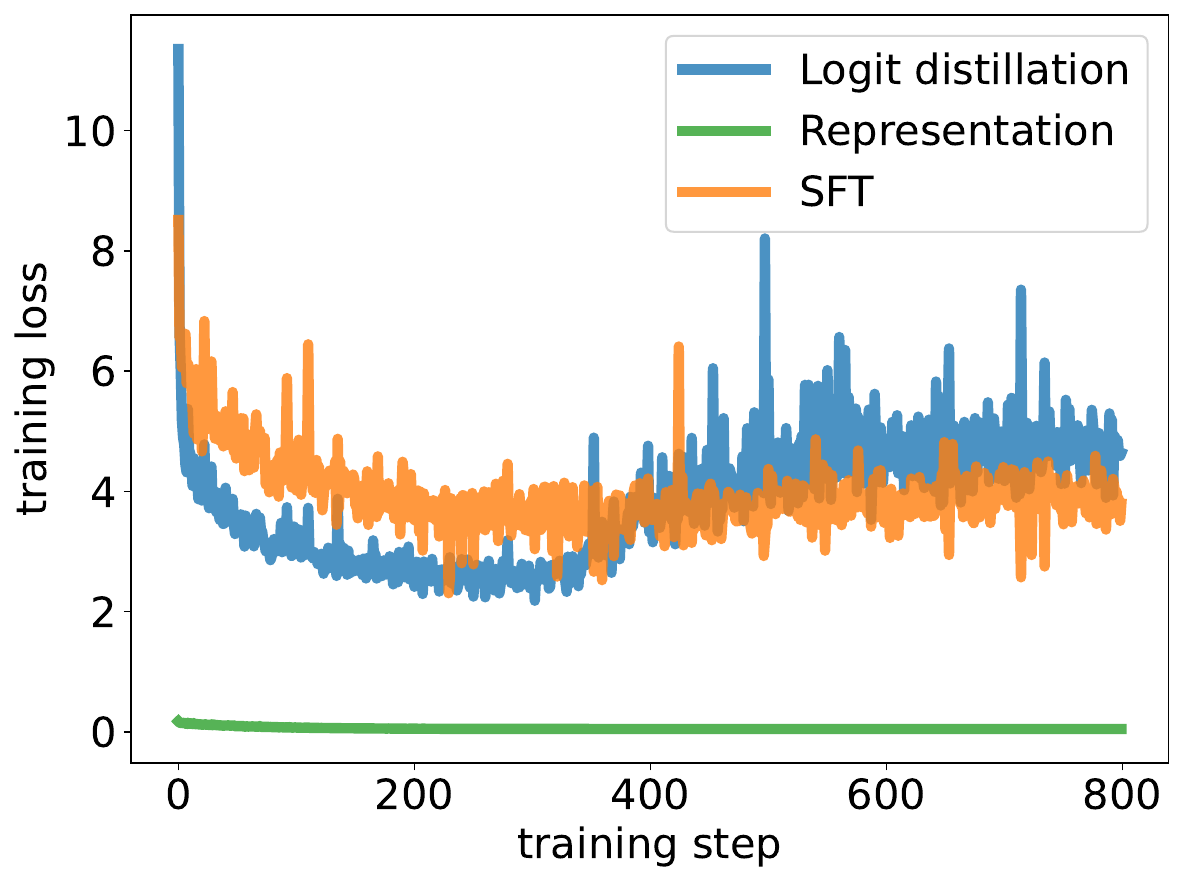}
    }

    \subfloat{
        \includegraphics[width=0.245\textwidth]{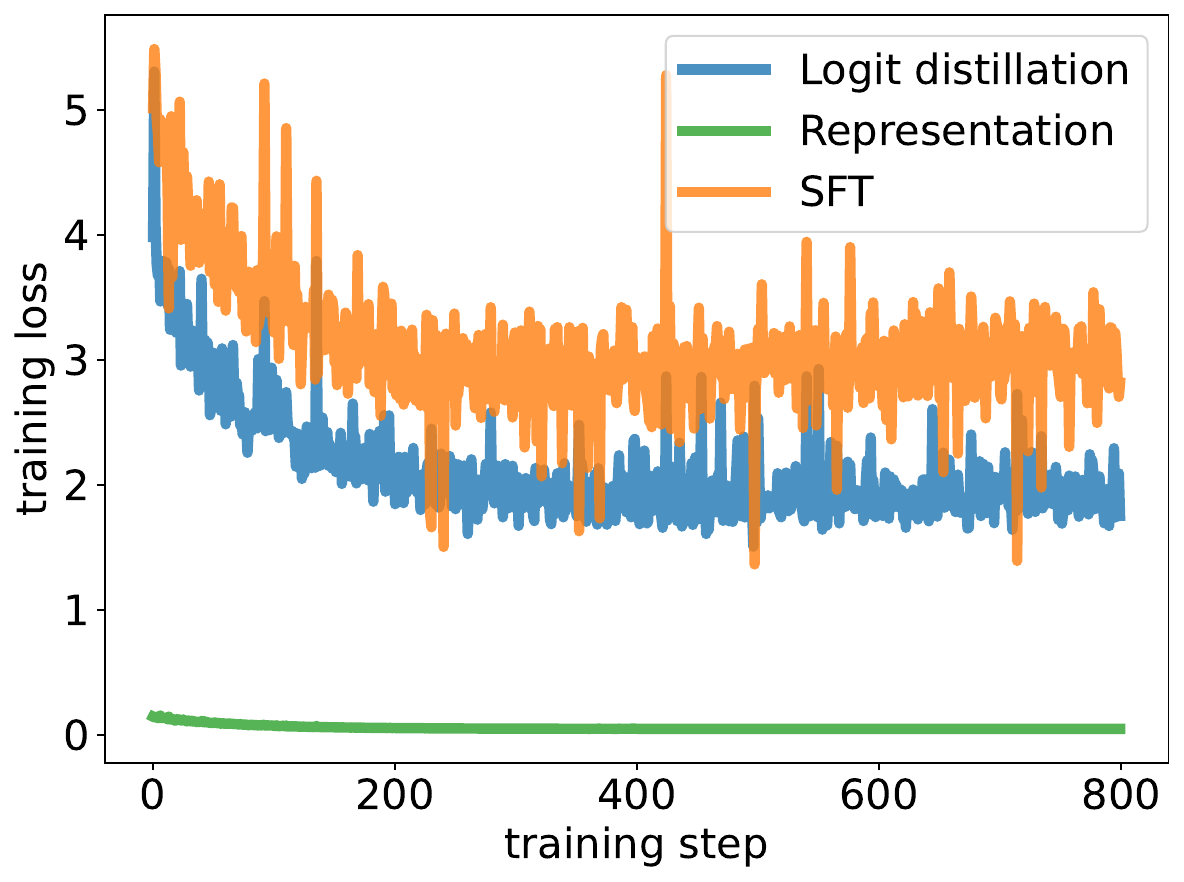}
    }
    \subfloat{
        \includegraphics[width=0.245\textwidth]{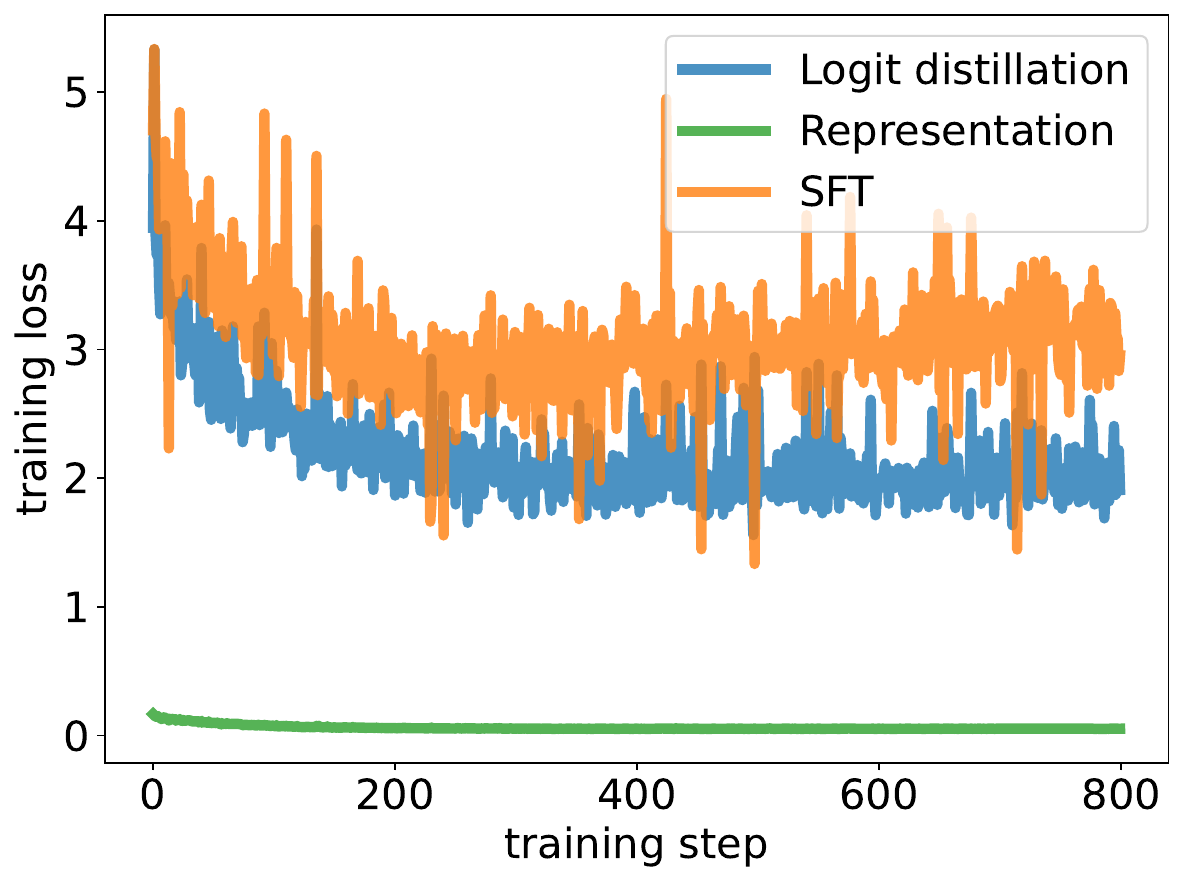}
    }
    \subfloat{
        \includegraphics[width=0.245\textwidth]{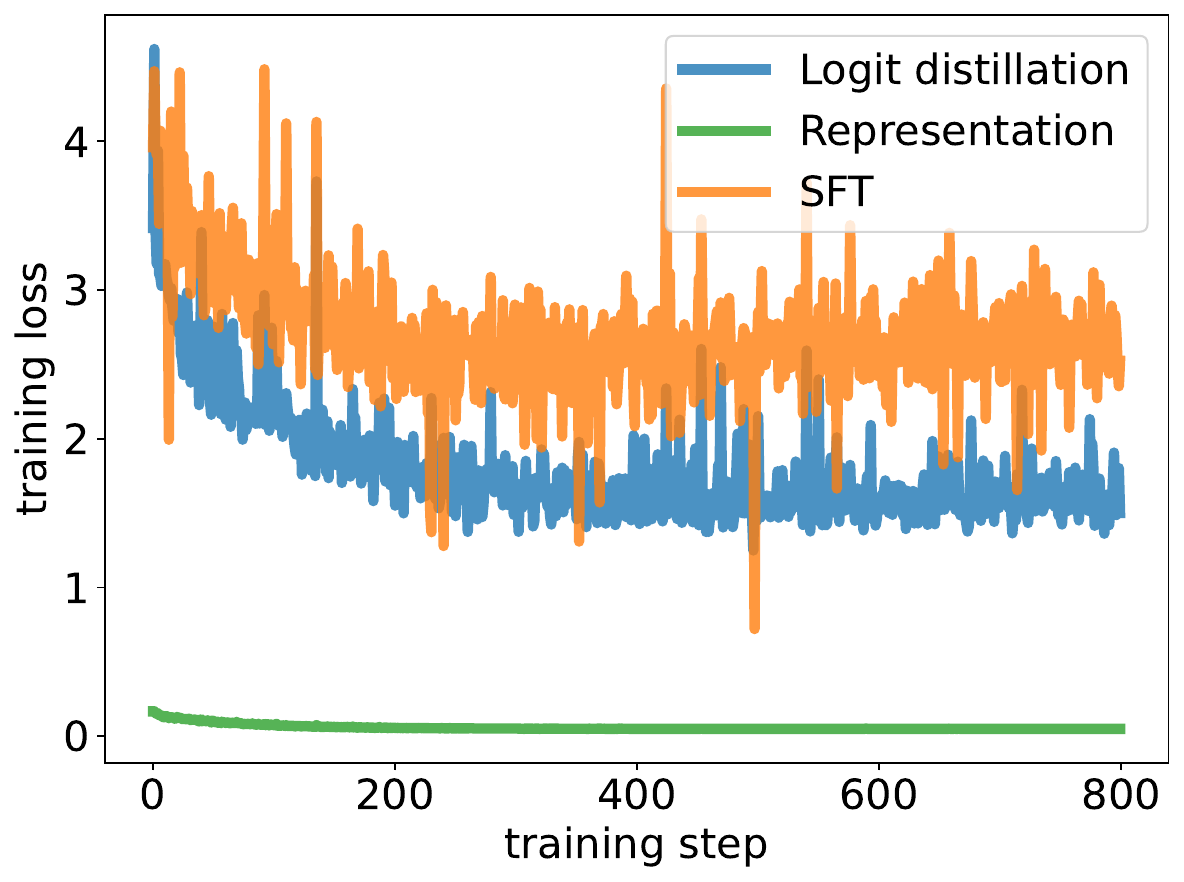}
    }
    \subfloat{
        \includegraphics[width=0.245\textwidth]{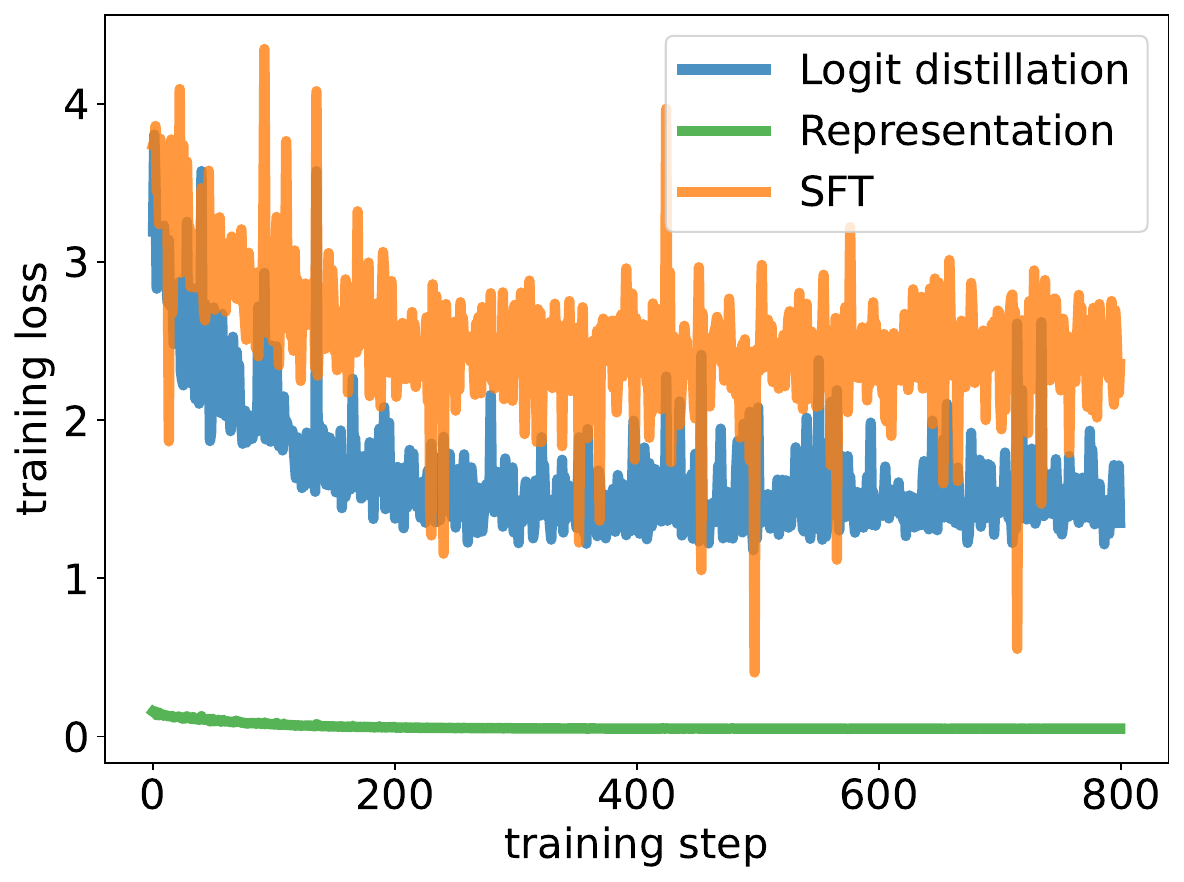}
    }

    \caption{\textbf{Low-rank linear adapter training curves for the first 24 Mistral 7b blocks with a rank of 8} trained using three different objectives including (a) MSE loss defined on the representation, (b) supervised fine-tuning (SFT), and (c) logit distillation where logits are distilled from the full model. Rest of the blocks are visualized in Fig.~\ref{fig:linear_adapters_rank_8_llama2_train_loss_b}.}
    \label{fig:linear_adapters_rank_8_mistral_train_loss_a}
\end{figure}

\begin{figure}[t]
    \centering
    \subfloat{
        \includegraphics[width=0.245\textwidth]{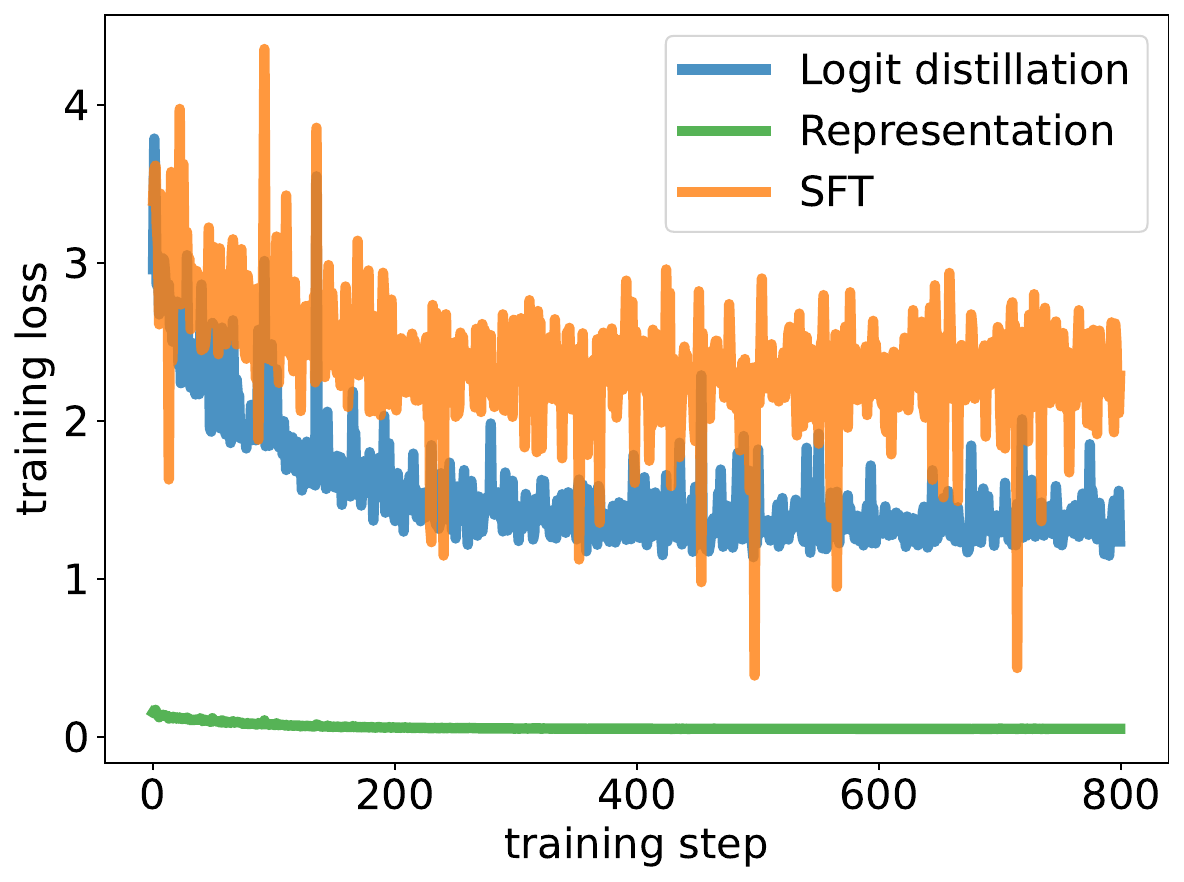}
    }
    \subfloat{
        \includegraphics[width=0.245\textwidth]{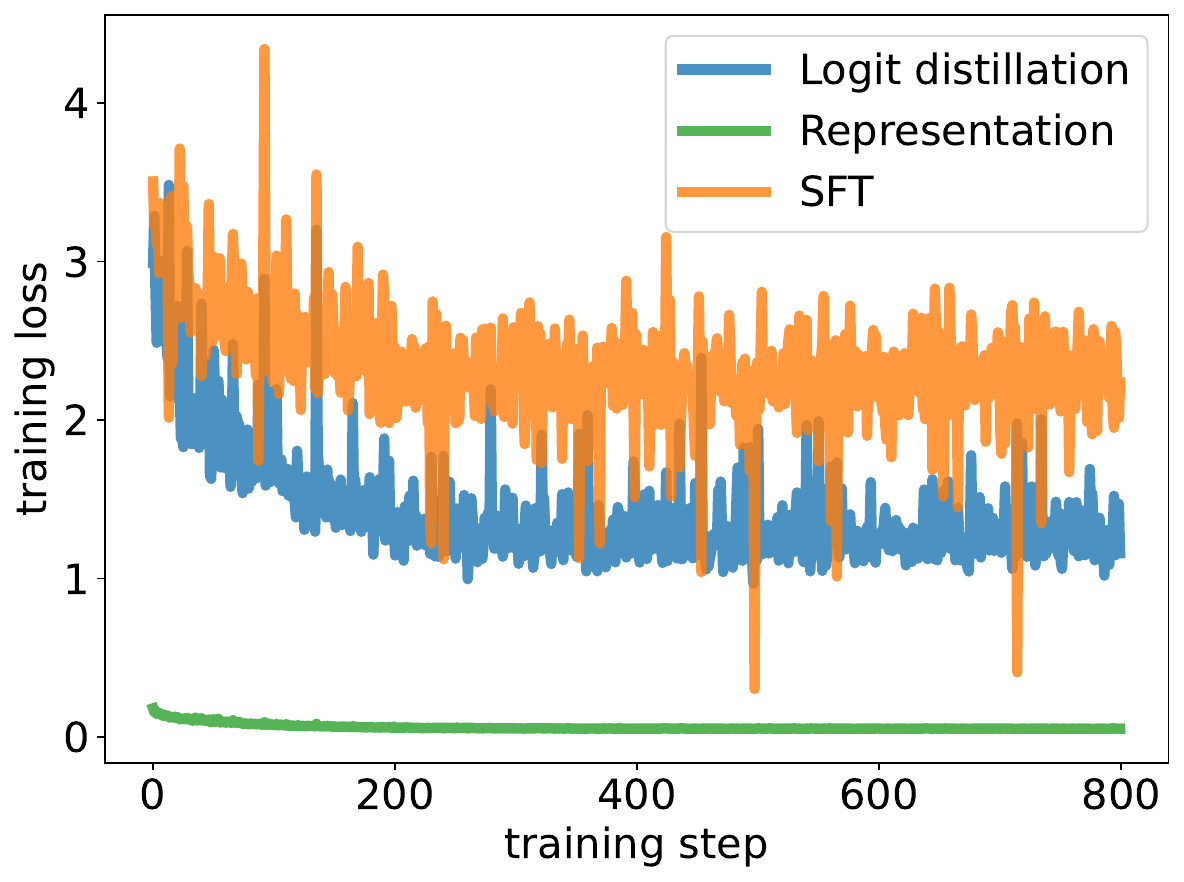}
    }
    \subfloat{
        \includegraphics[width=0.245\textwidth]{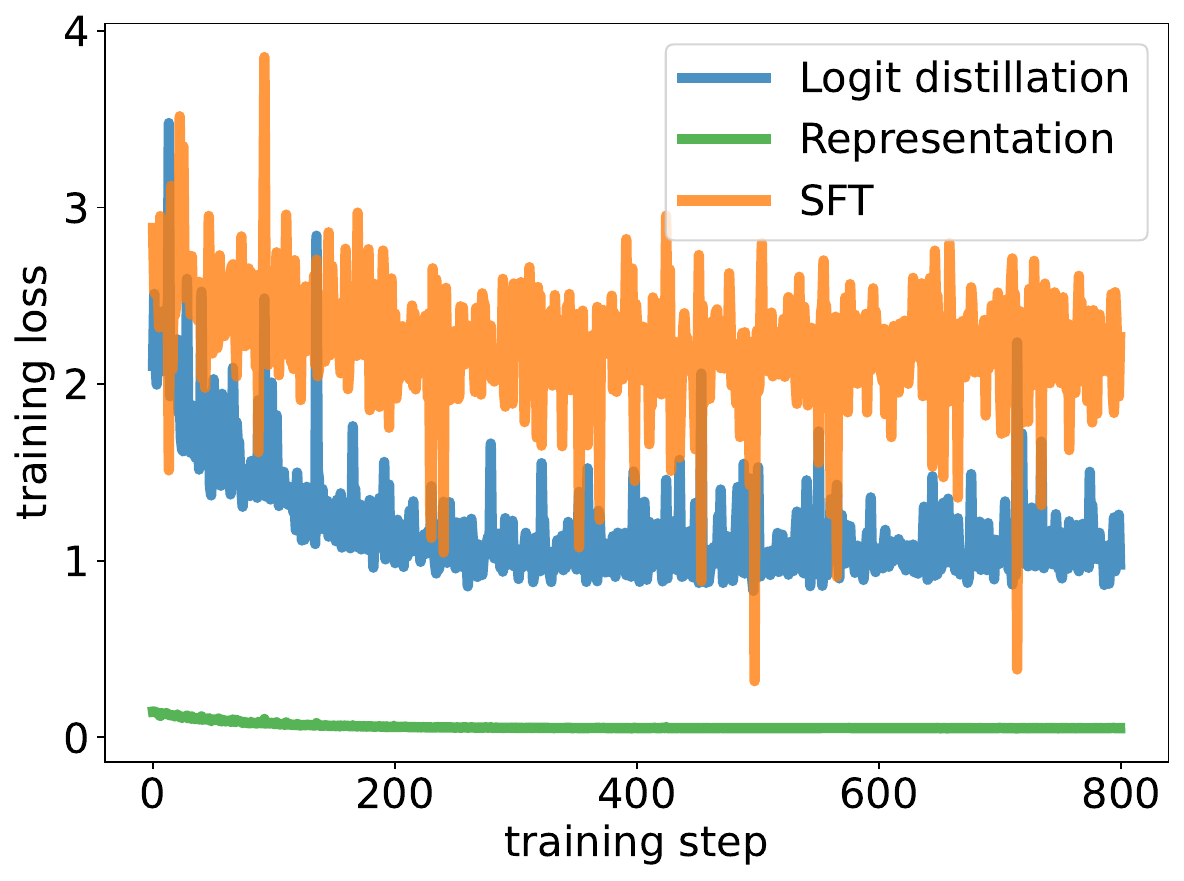}
    }
    \subfloat{
        \includegraphics[width=0.245\textwidth]{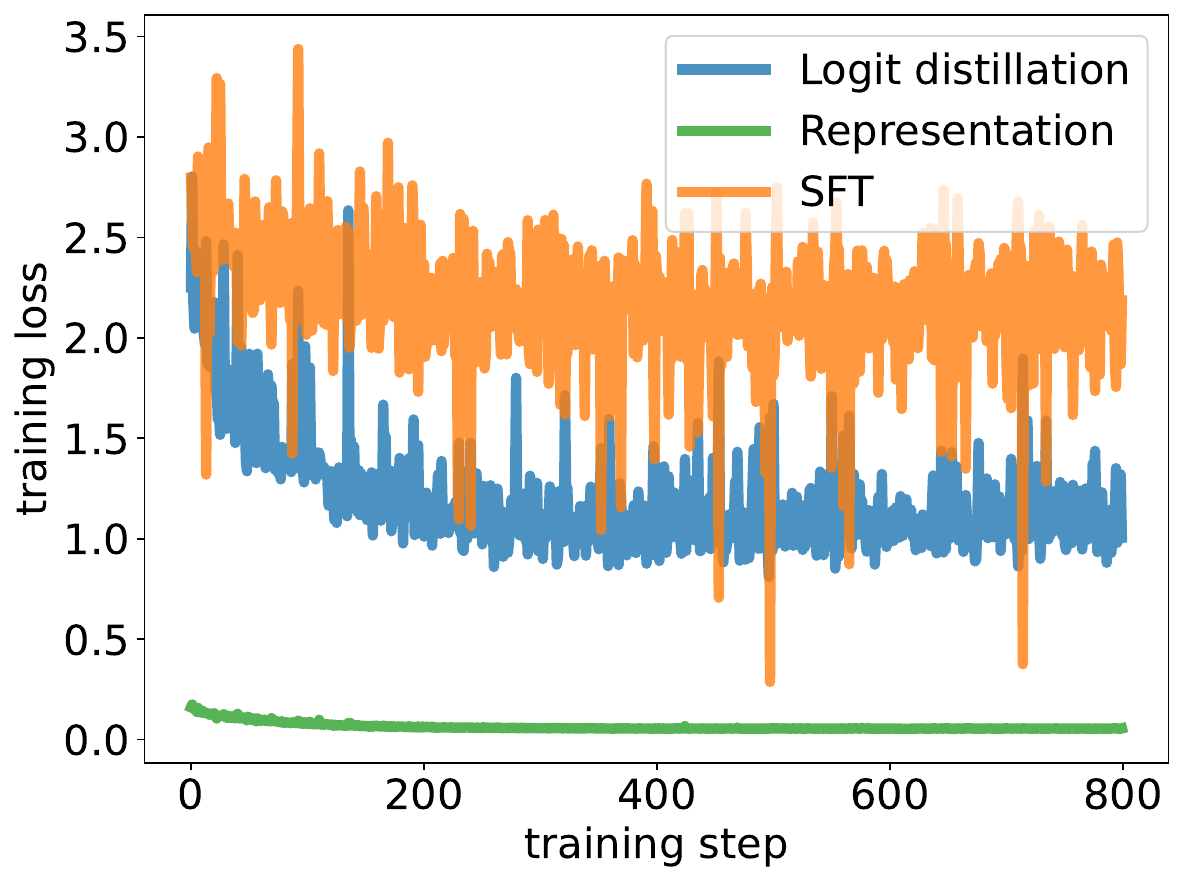}
    }

    \subfloat{
        \includegraphics[width=0.245\textwidth]{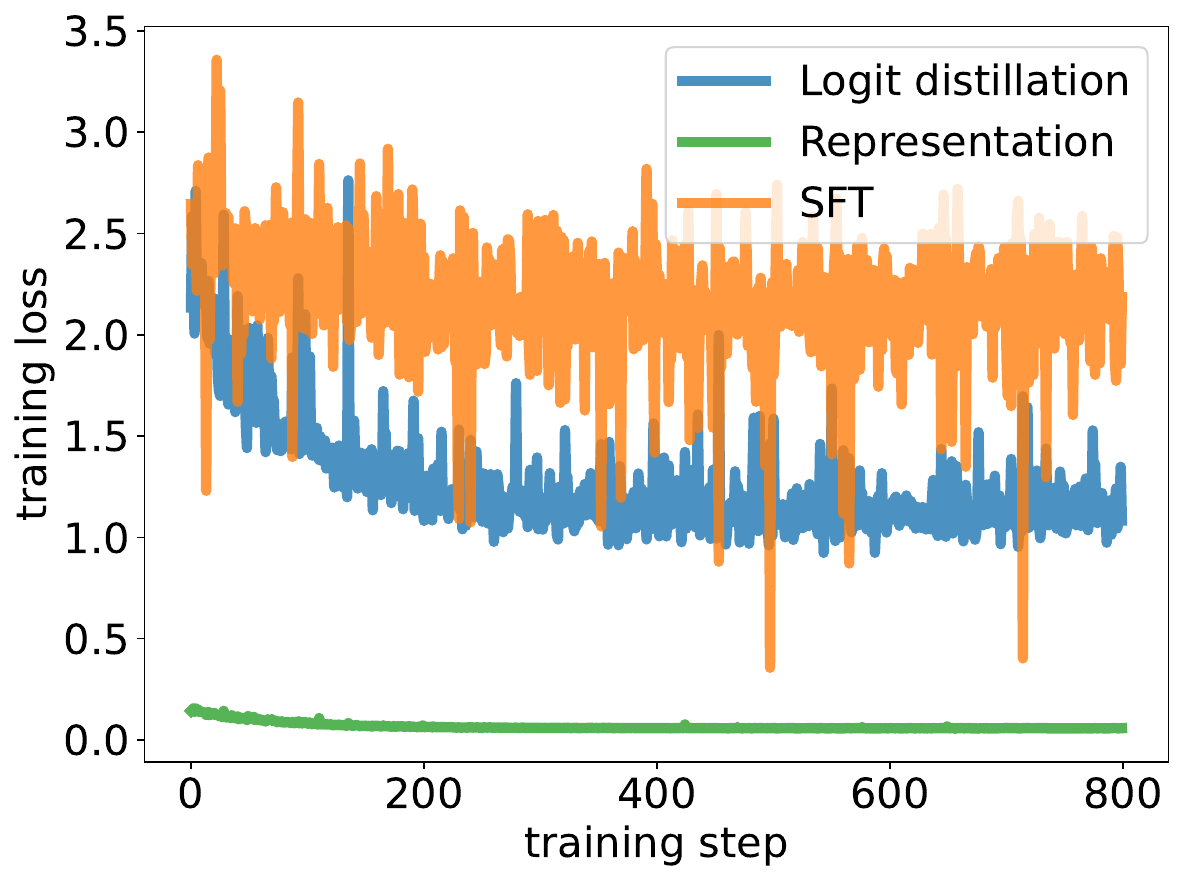}
    }
    \subfloat{
        \includegraphics[width=0.245\textwidth]{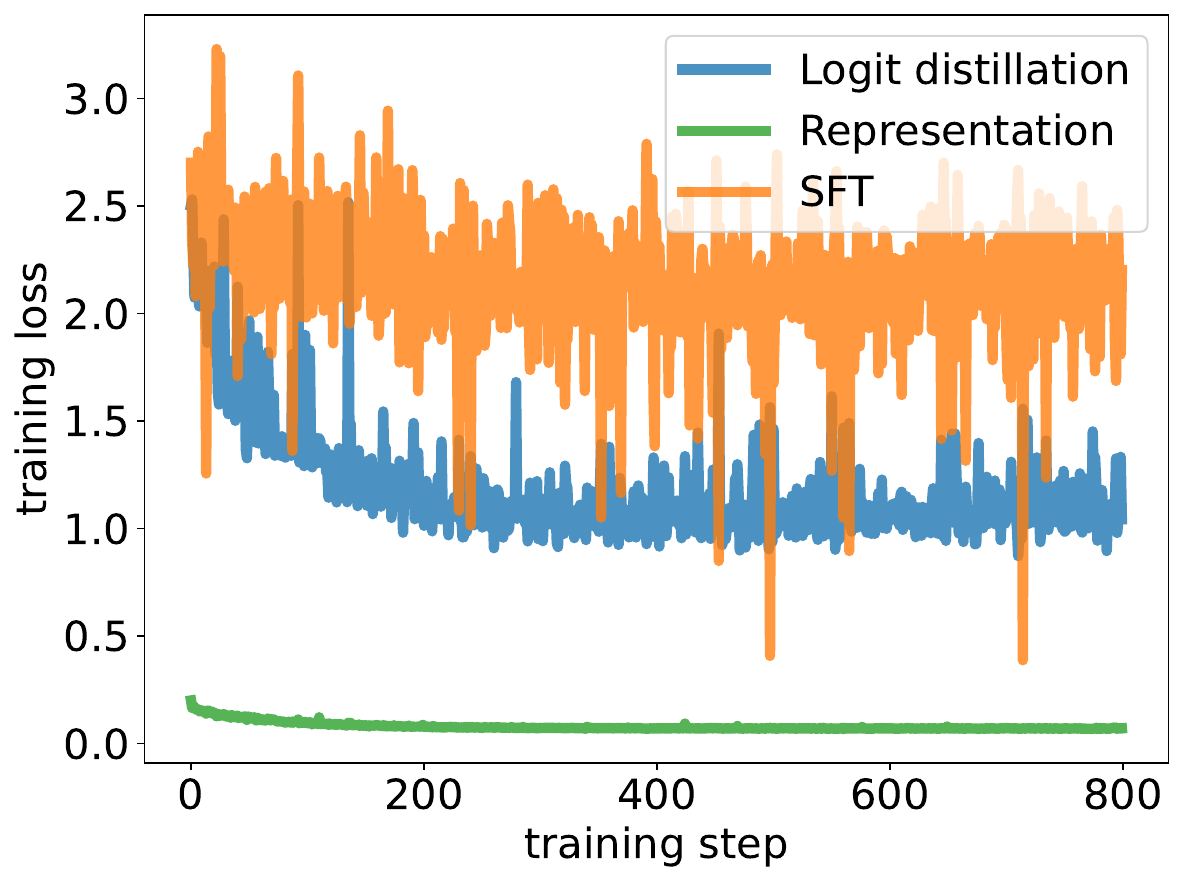}
    }
    \subfloat{
        \includegraphics[width=0.245\textwidth]{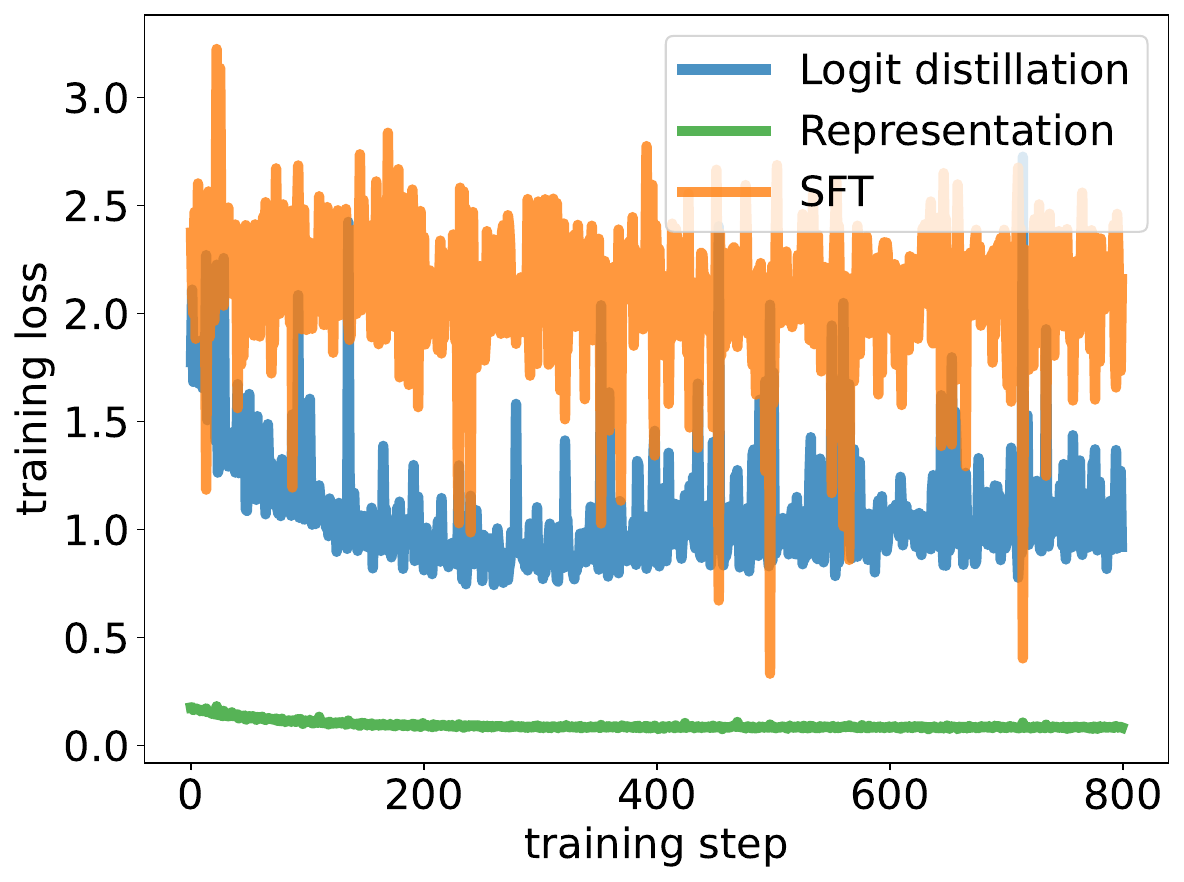}
    }
    \subfloat{
        \includegraphics[width=0.245\textwidth]{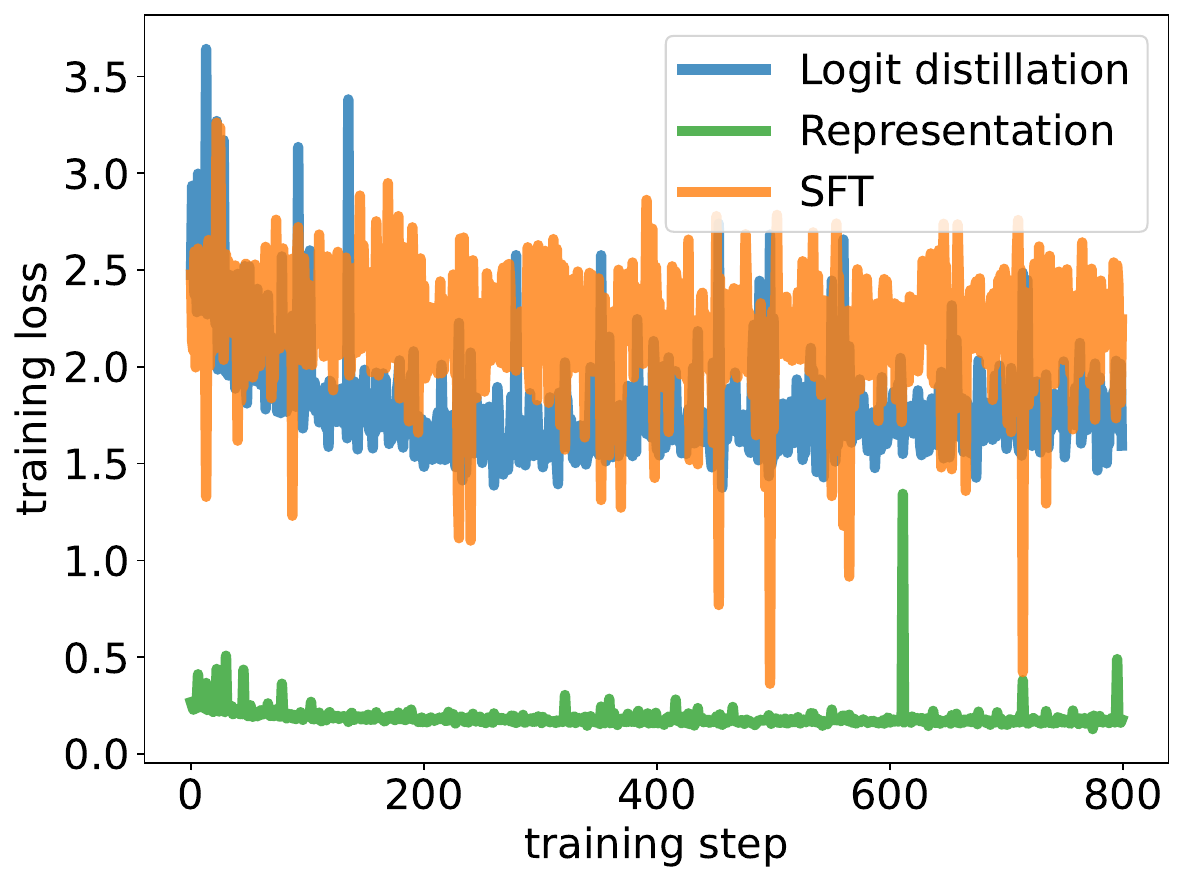}
    }

    \caption{\textbf{Low-rank linear adapter training curves for the last 8 Mistral 7b blocks with a rank of 8} trained using three different objectives including (a) MSE loss defined on the representation, (b) supervised fine-tuning (SFT), and (c) logit distillation where logits are distilled from the full model. The first set of blocks are visualized in Fig.~\ref{fig:linear_adapters_rank_8_llama2_train_loss_a}.}
    \label{fig:linear_adapters_rank_8_mistral_train_loss_b}
\end{figure}

The loss curves for the training of the low-rank adapter with a rank of 8 on Mistral are visualized in Fig.~\ref{fig:linear_adapters_rank_8_mistral_train_loss_a} and Fig.~\ref{fig:linear_adapters_rank_8_mistral_train_loss_b}.

\begin{figure}[t]
    \centering
    \subfloat{
        \includegraphics[width=0.245\textwidth]{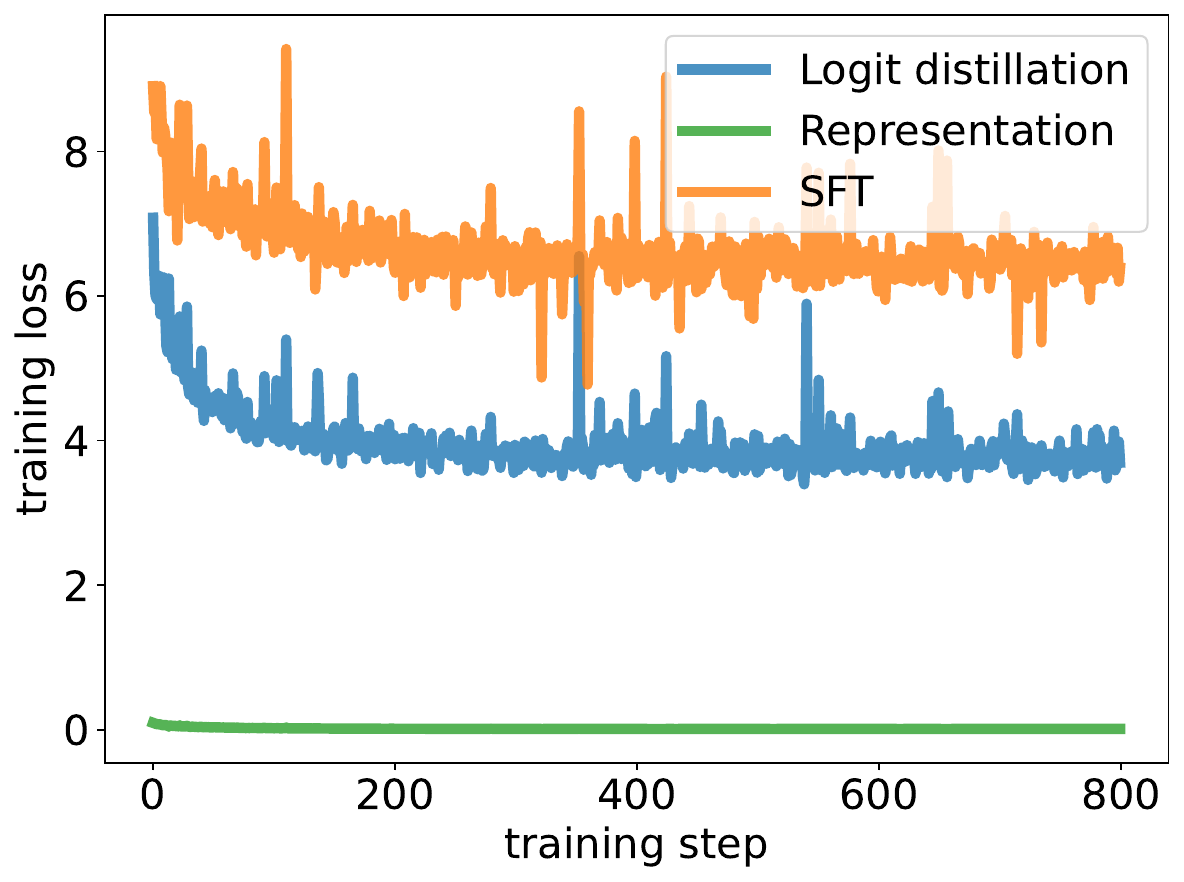}
    }
    \subfloat{
        \includegraphics[width=0.245\textwidth]{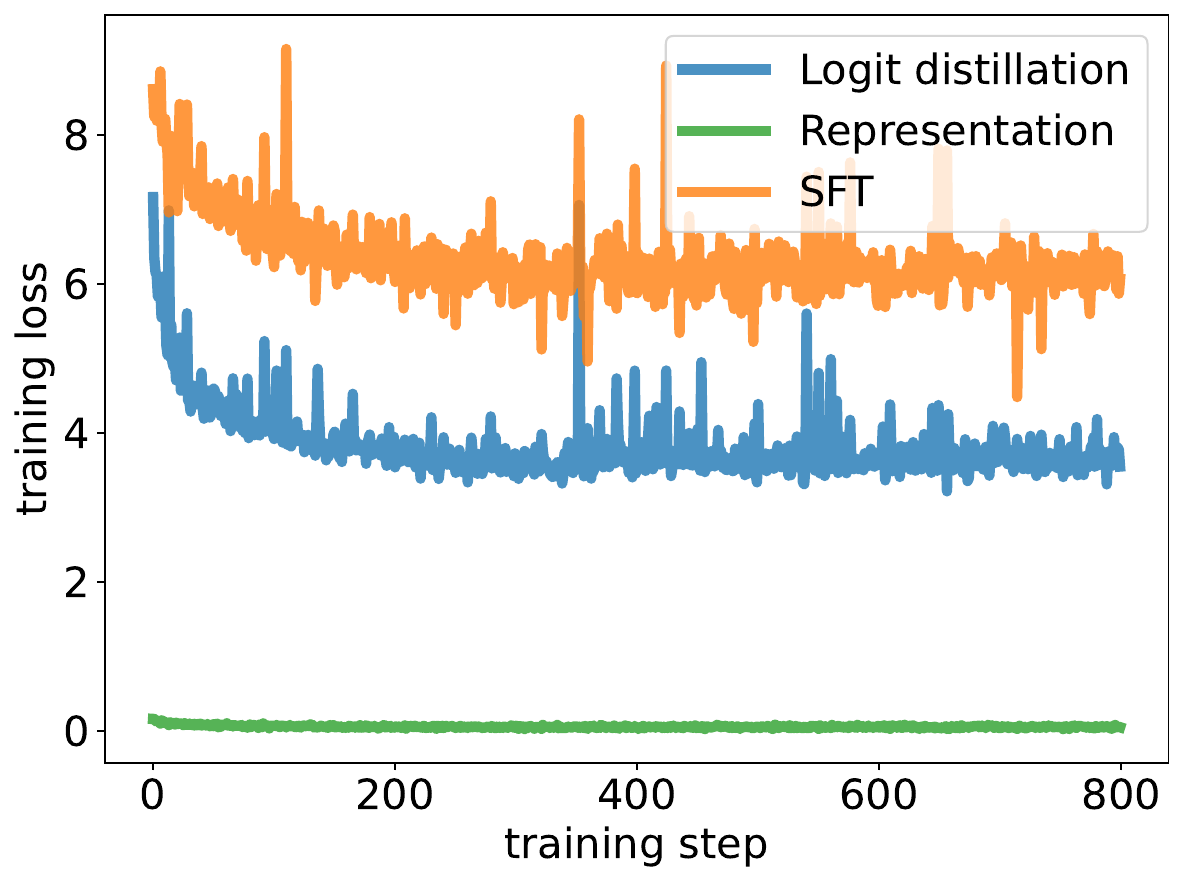}
    }
    \subfloat{
        \includegraphics[width=0.245\textwidth]{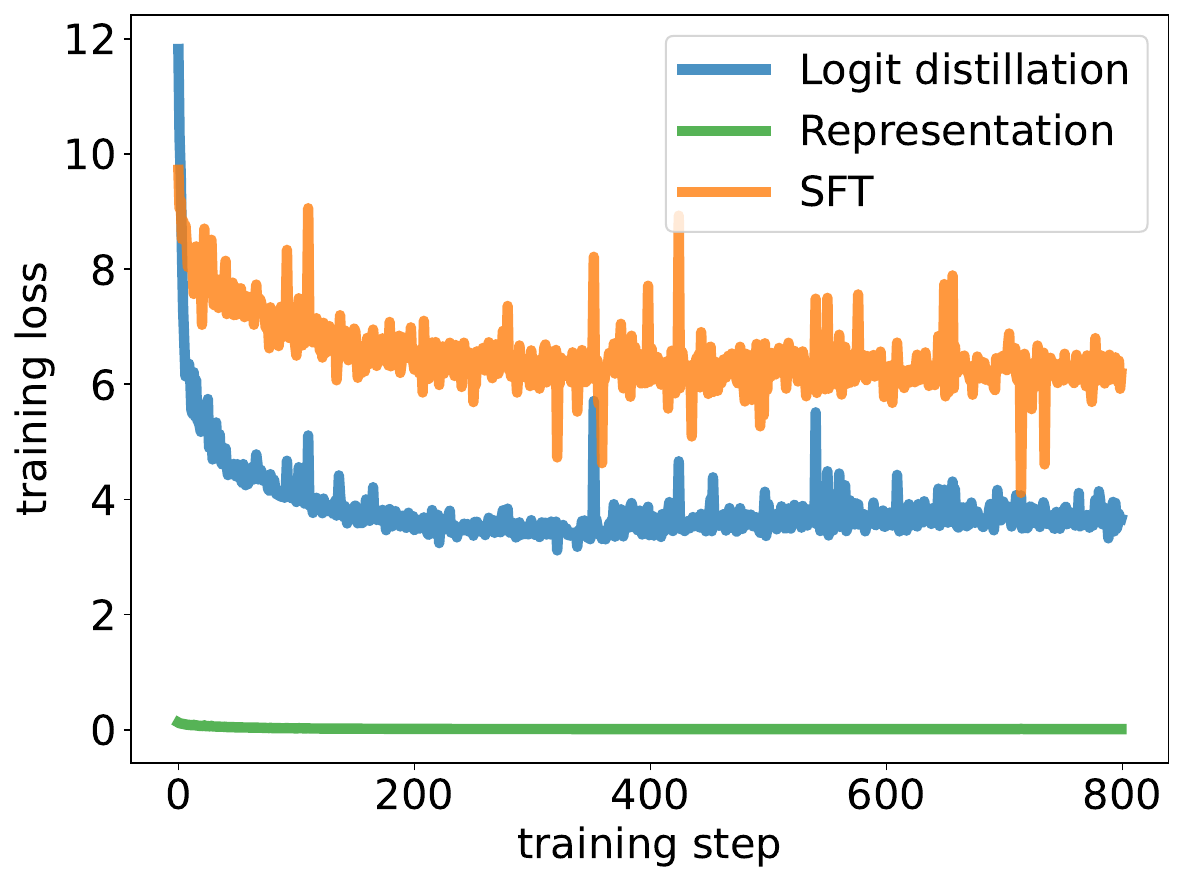}
    }
    \subfloat{
        \includegraphics[width=0.245\textwidth]{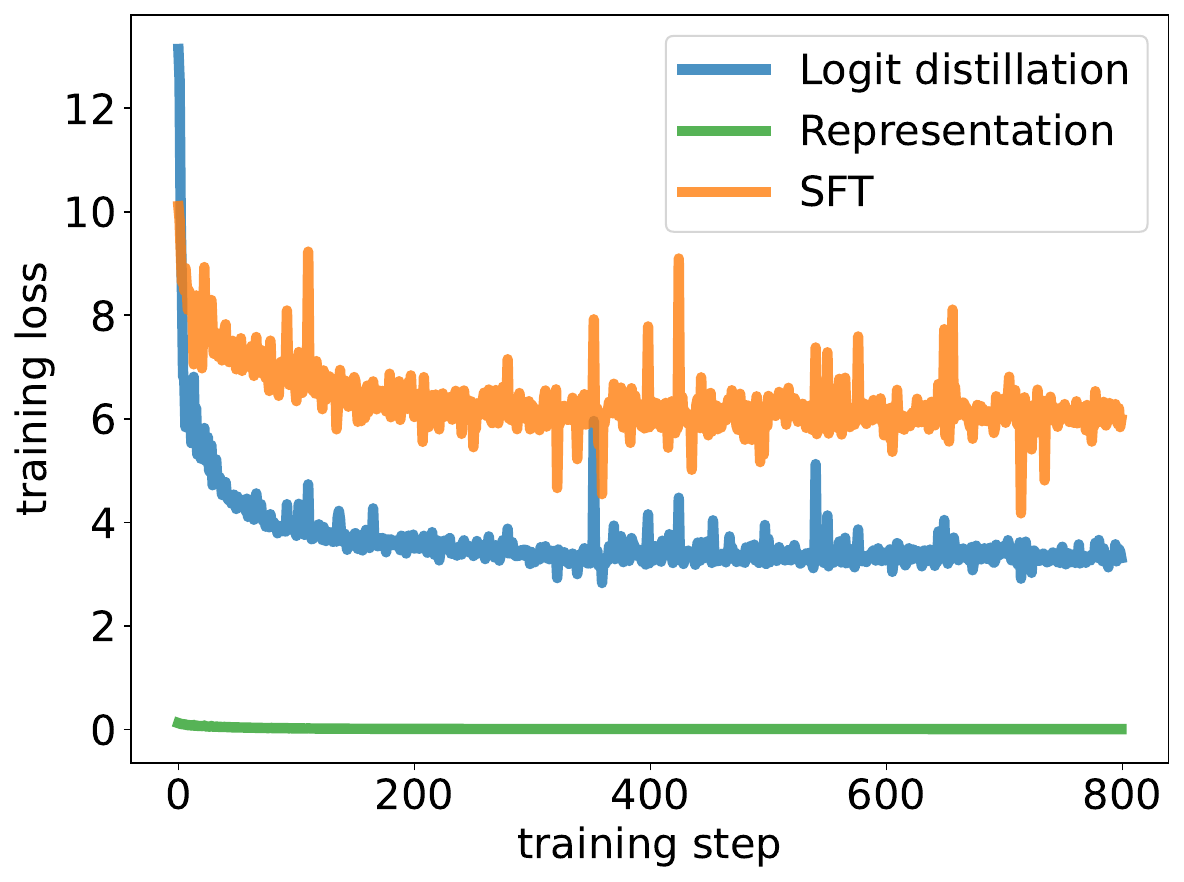}
    }

    \subfloat{
        \includegraphics[width=0.245\textwidth]{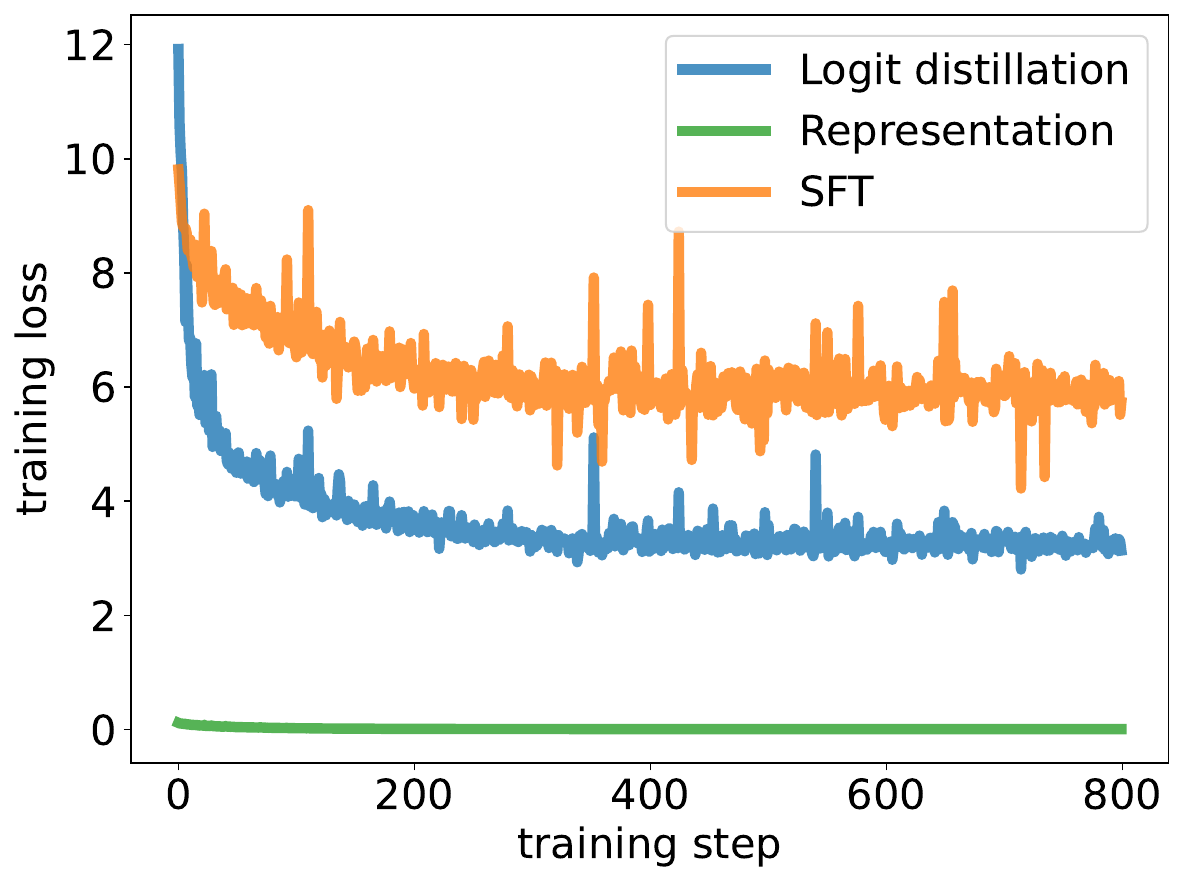}
    }
    \subfloat{
        \includegraphics[width=0.245\textwidth]{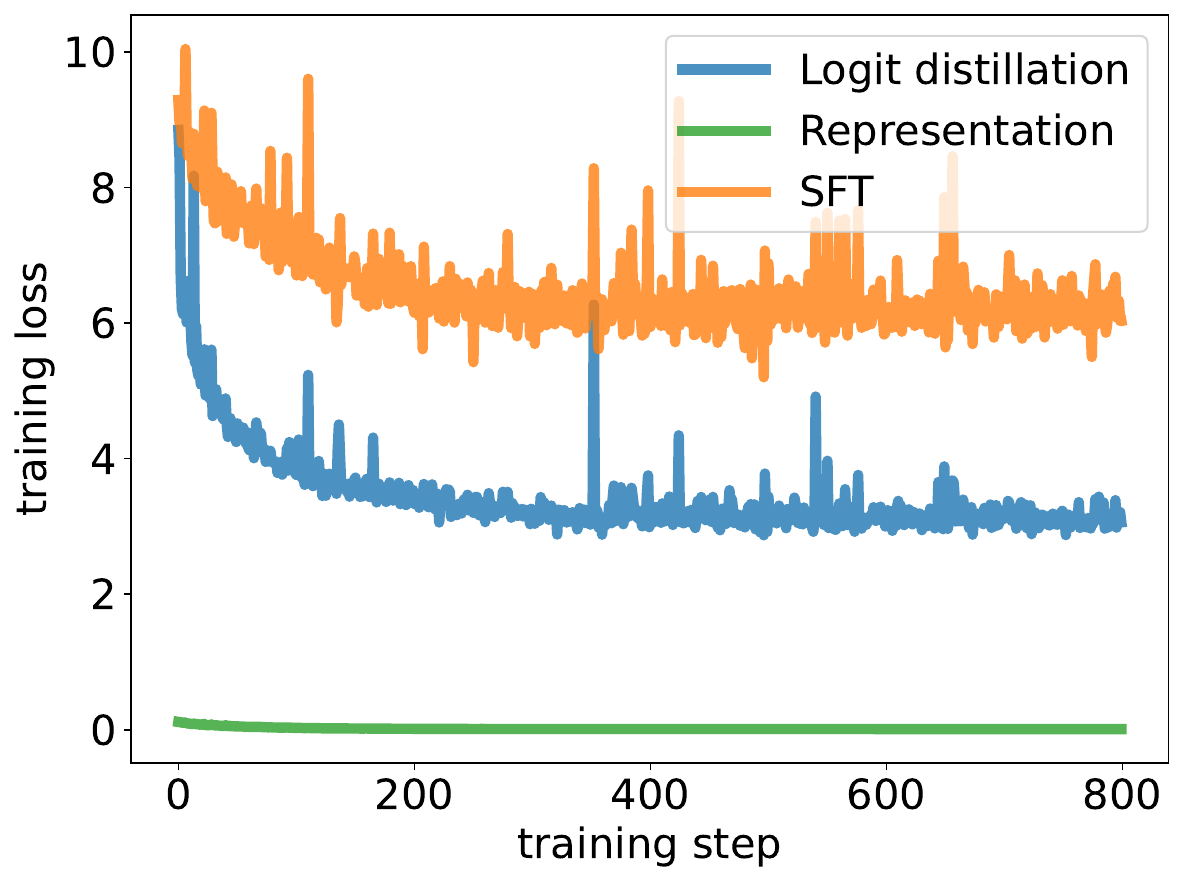}
    }
    \subfloat{
        \includegraphics[width=0.245\textwidth]{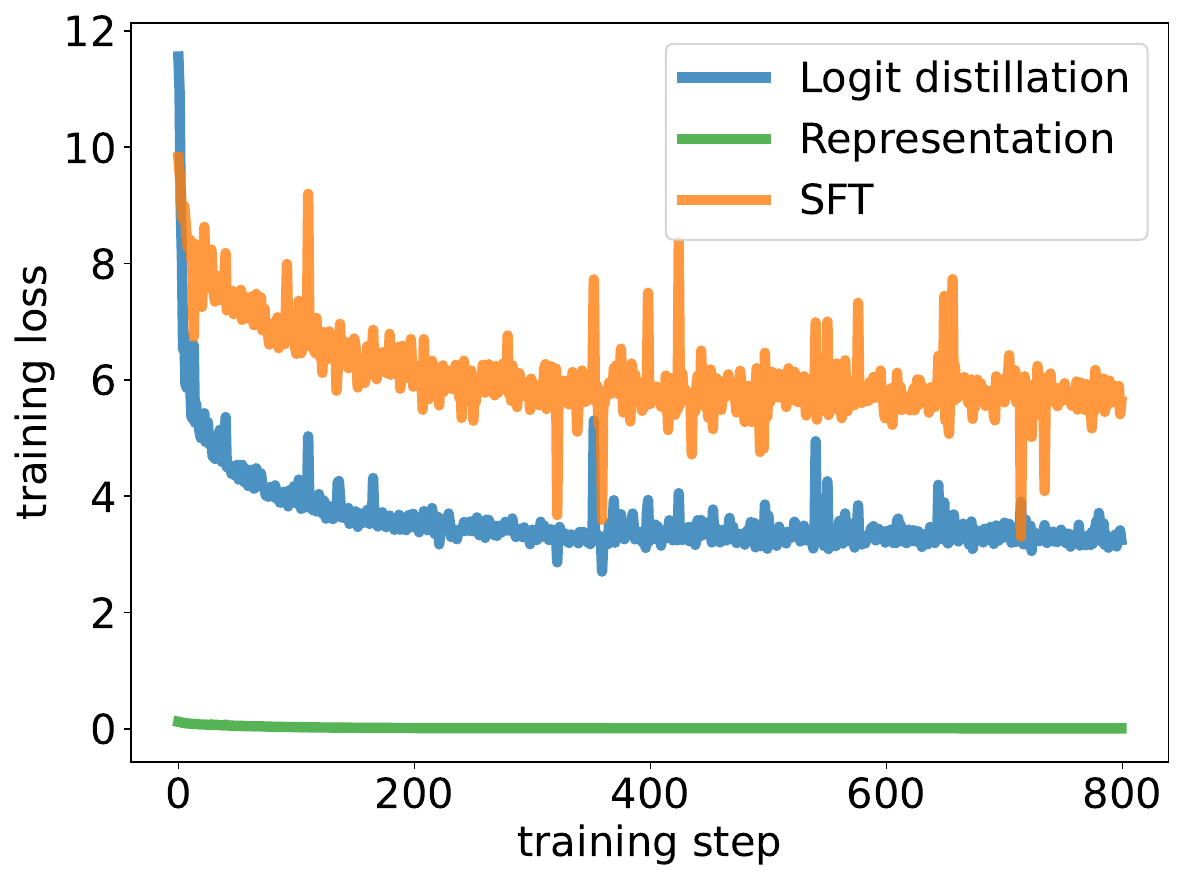}
    }
    \subfloat{
        \includegraphics[width=0.245\textwidth]{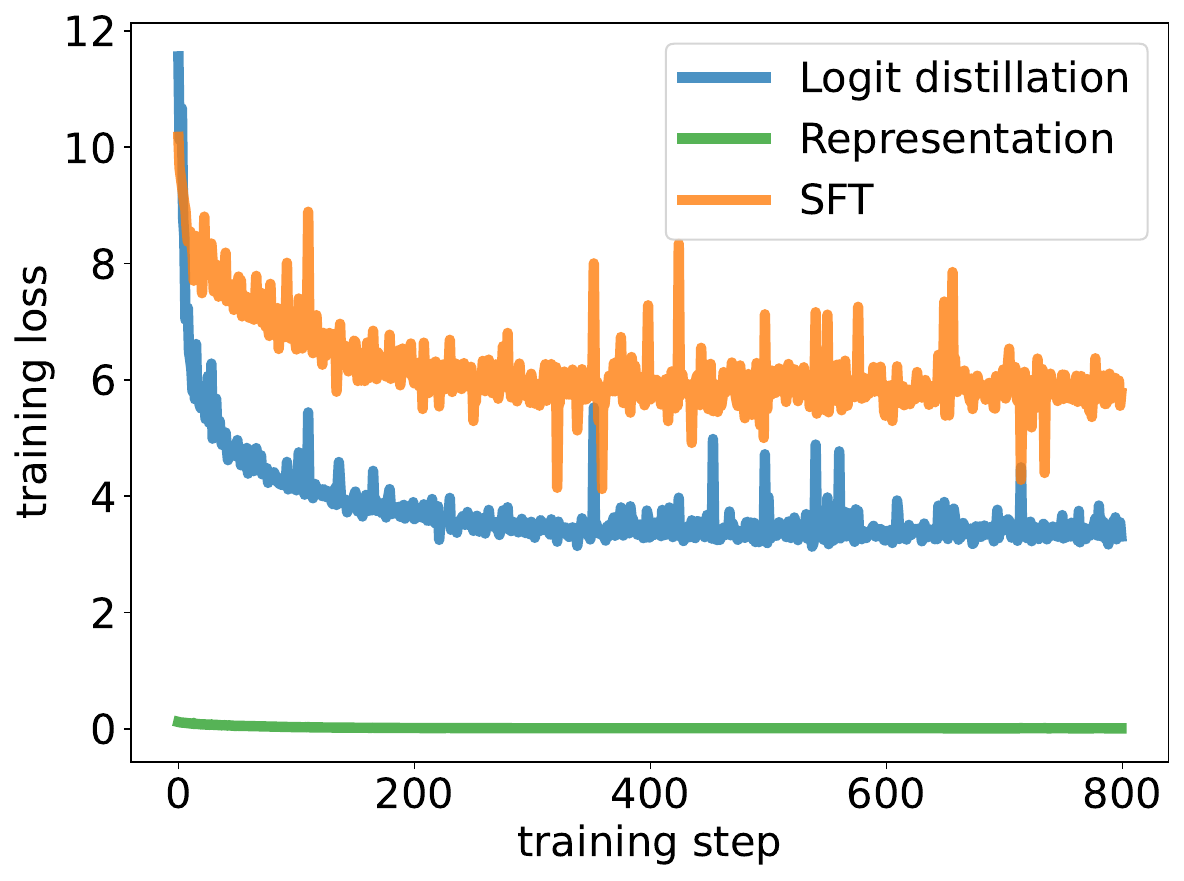}
    }

    \subfloat{
        \includegraphics[width=0.245\textwidth]{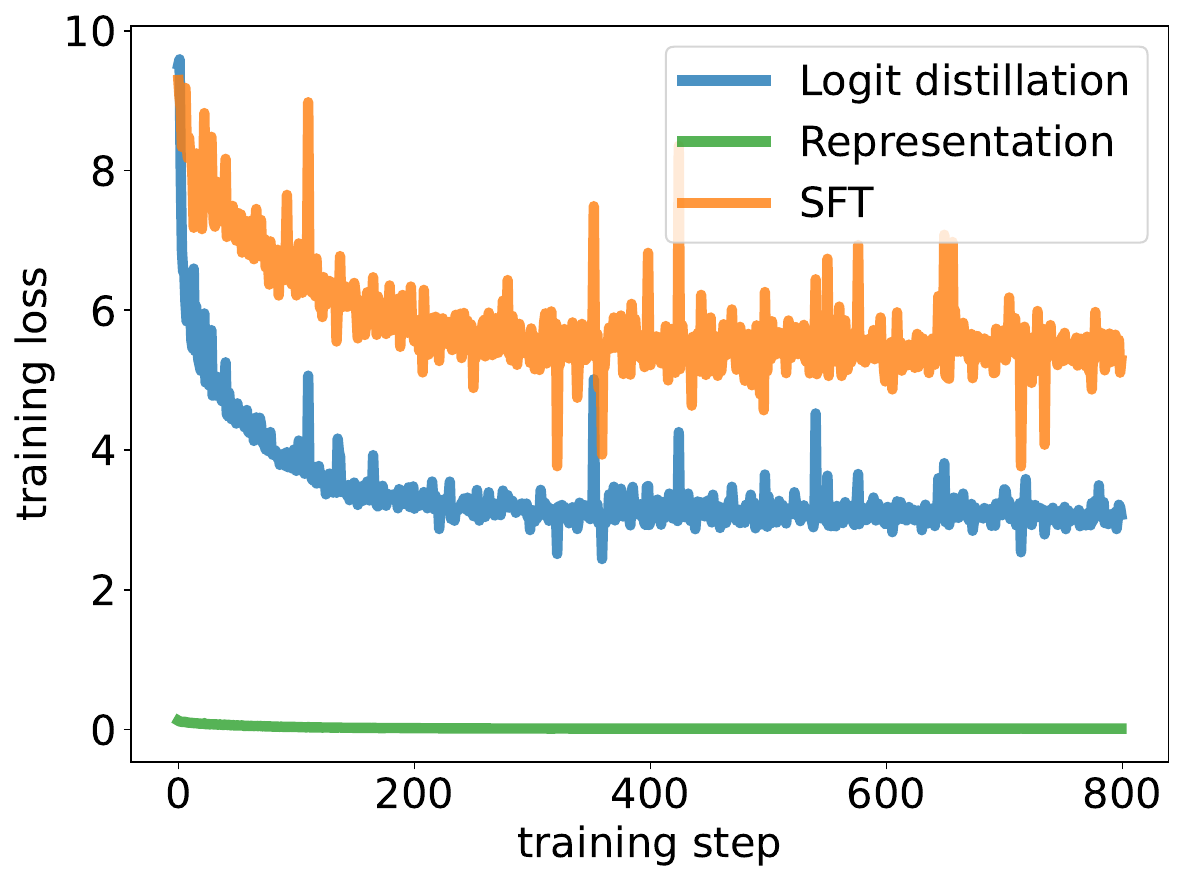}
    }
    \subfloat{
        \includegraphics[width=0.245\textwidth]{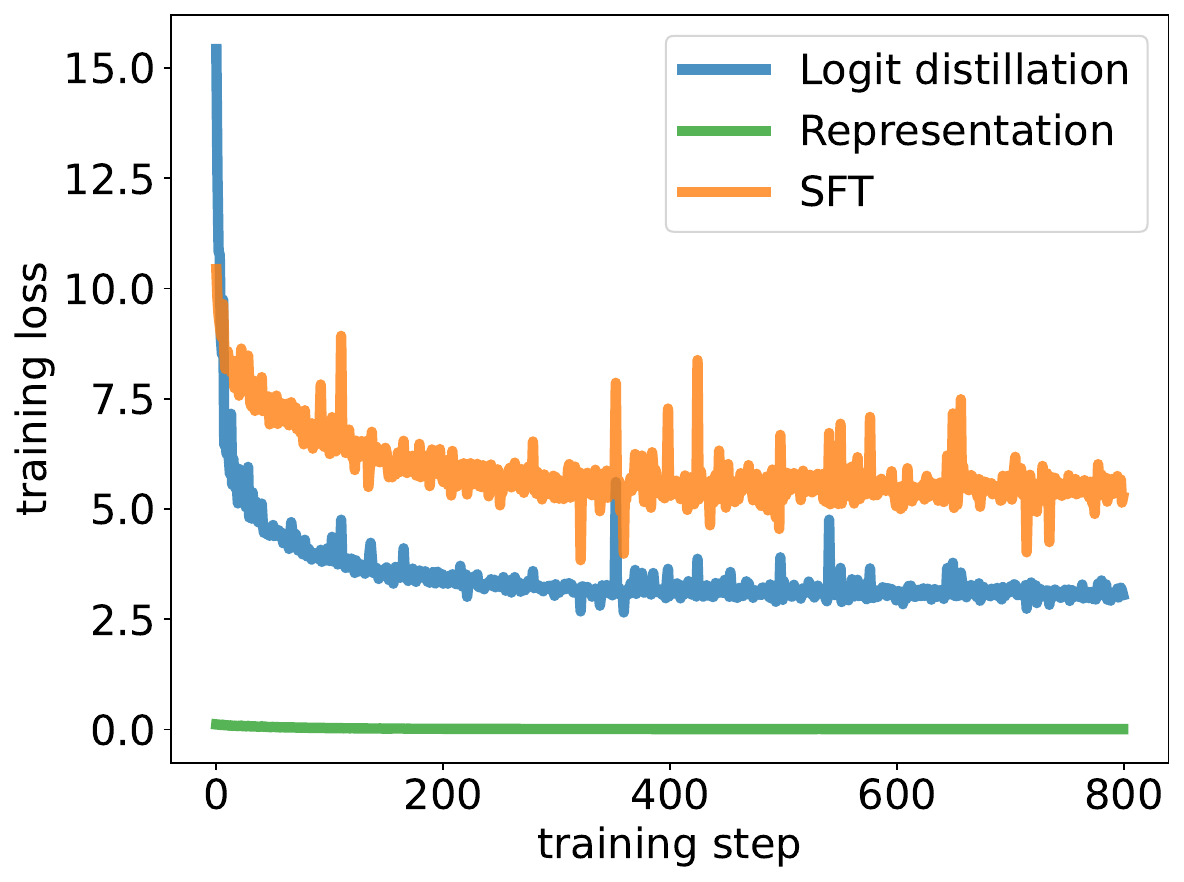}
    }
    \subfloat{
        \includegraphics[width=0.245\textwidth]{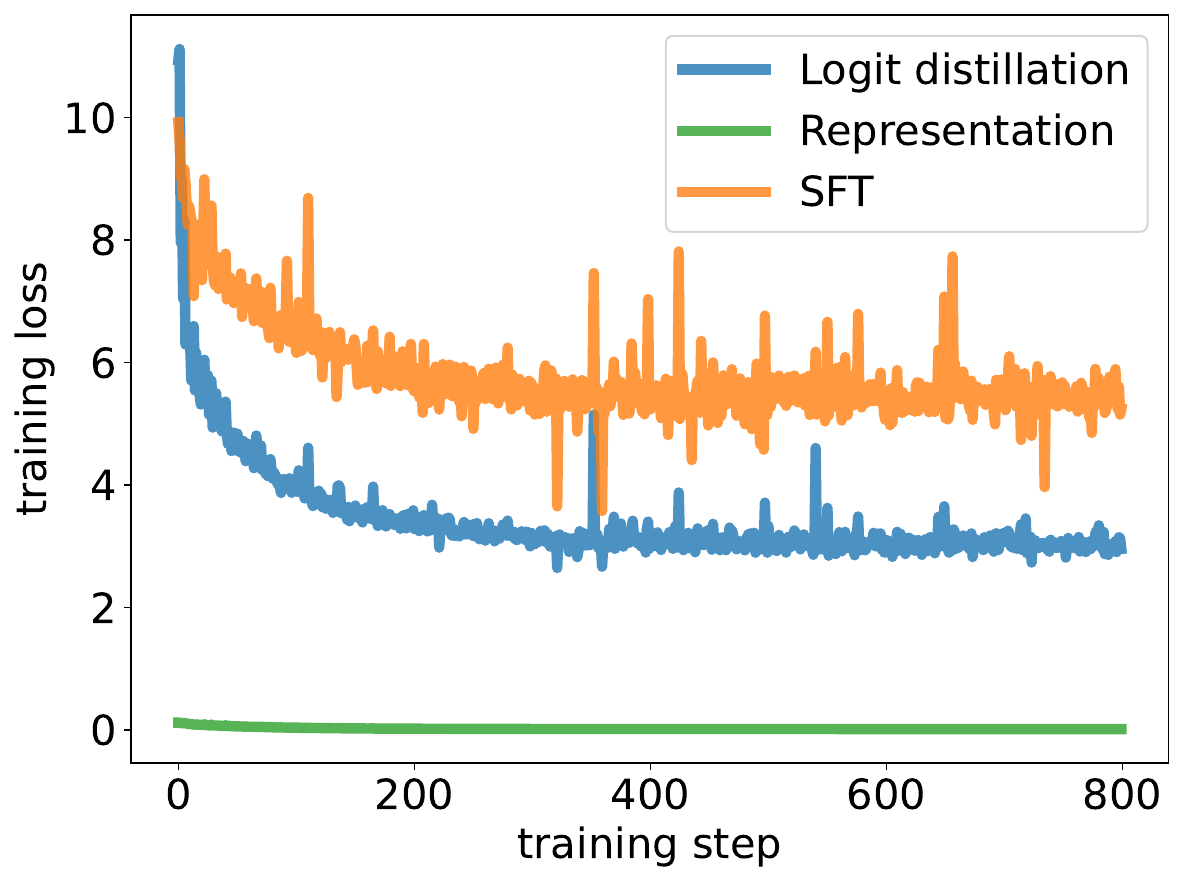}
    }
    \subfloat{
        \includegraphics[width=0.245\textwidth]{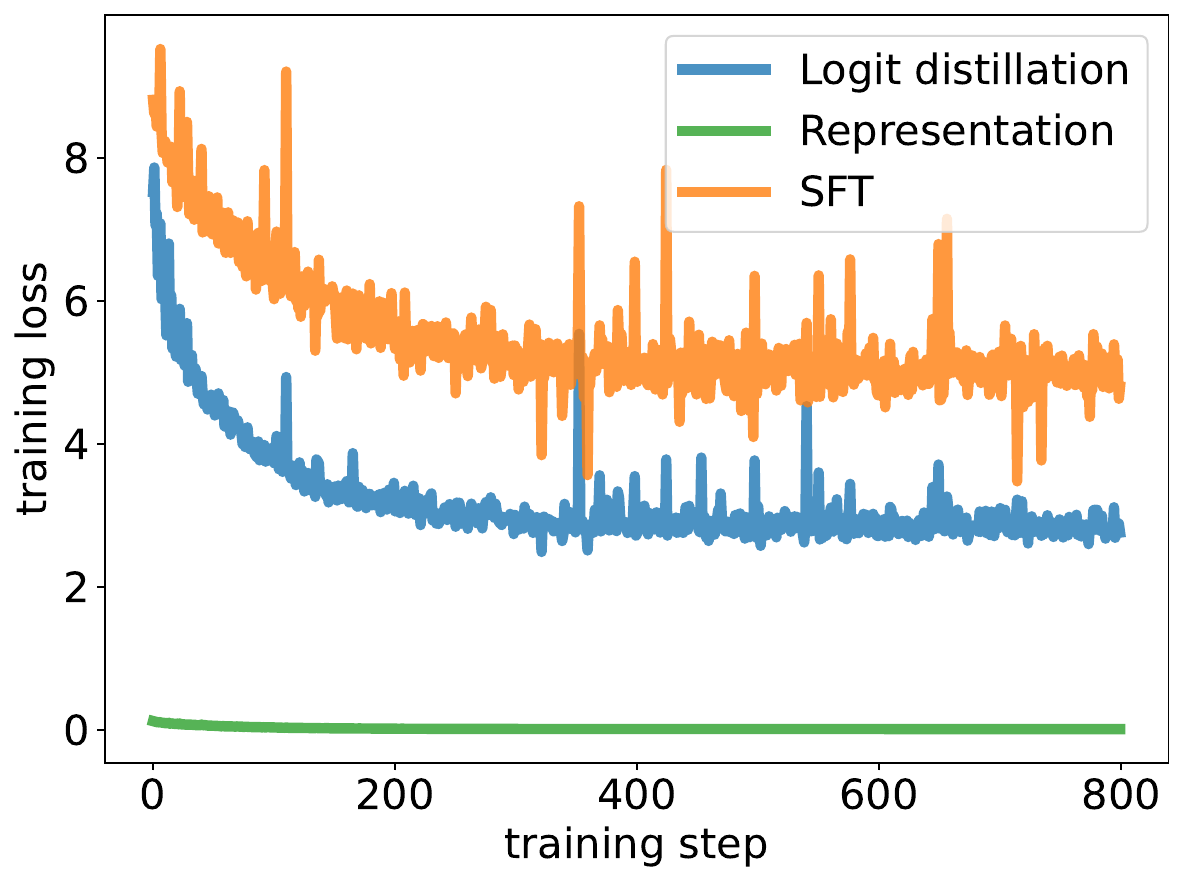}
    }

    \subfloat{
        \includegraphics[width=0.245\textwidth]{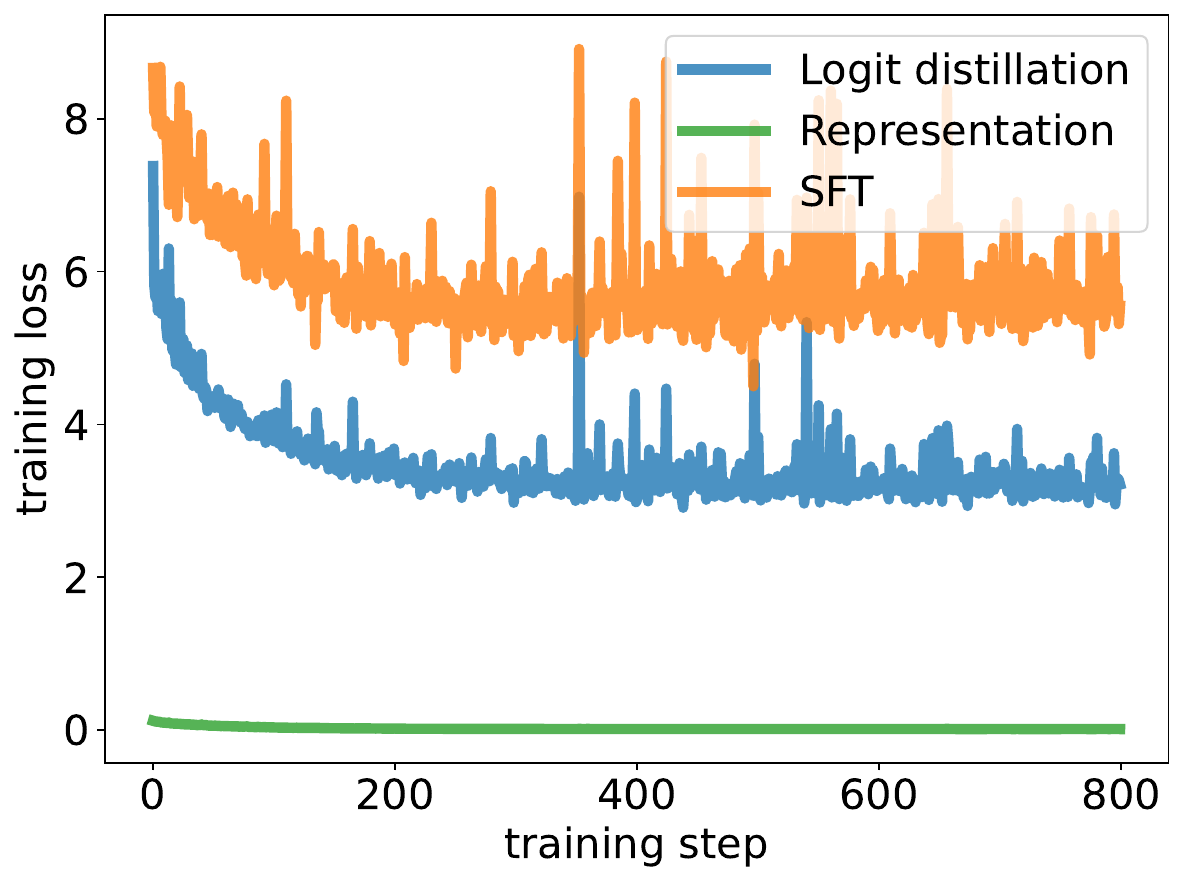}
    }
    \subfloat{
        \includegraphics[width=0.245\textwidth]{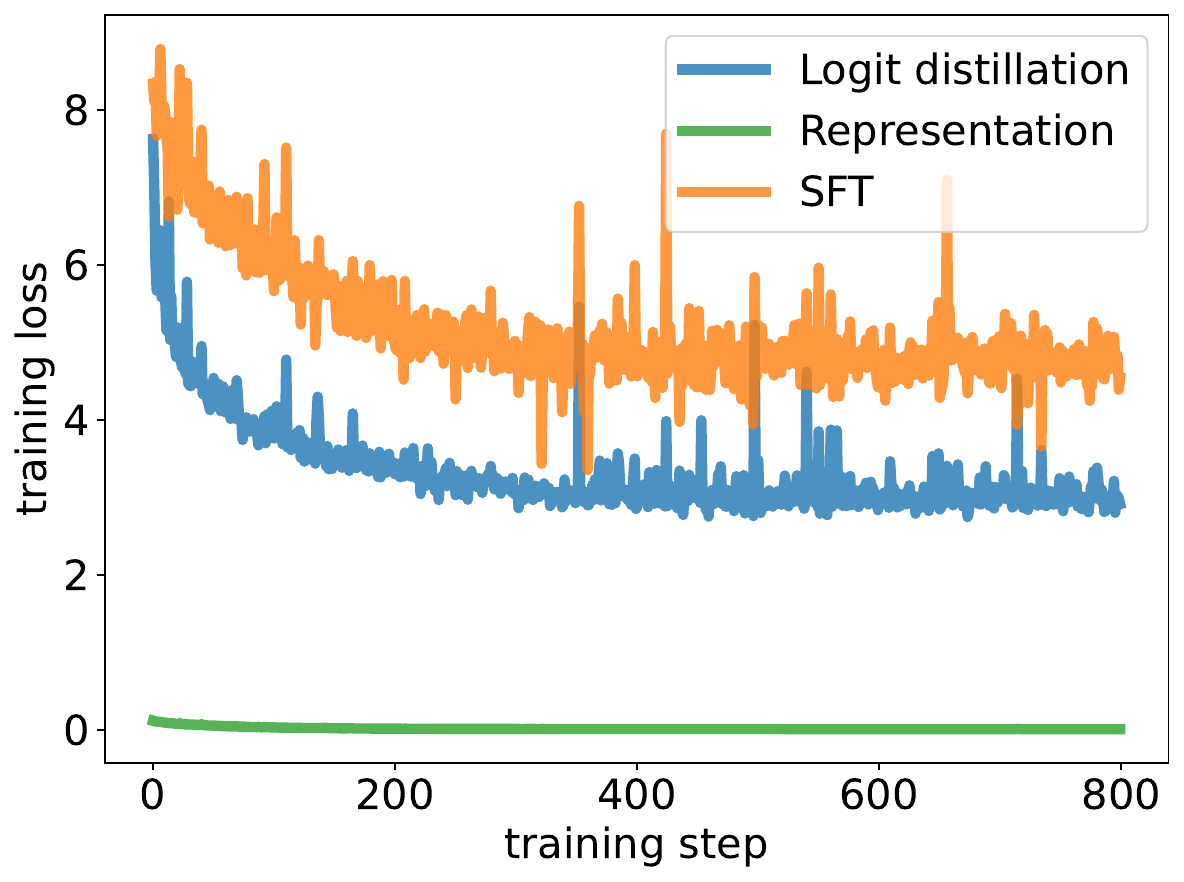}
    }
    \subfloat{
        \includegraphics[width=0.245\textwidth]{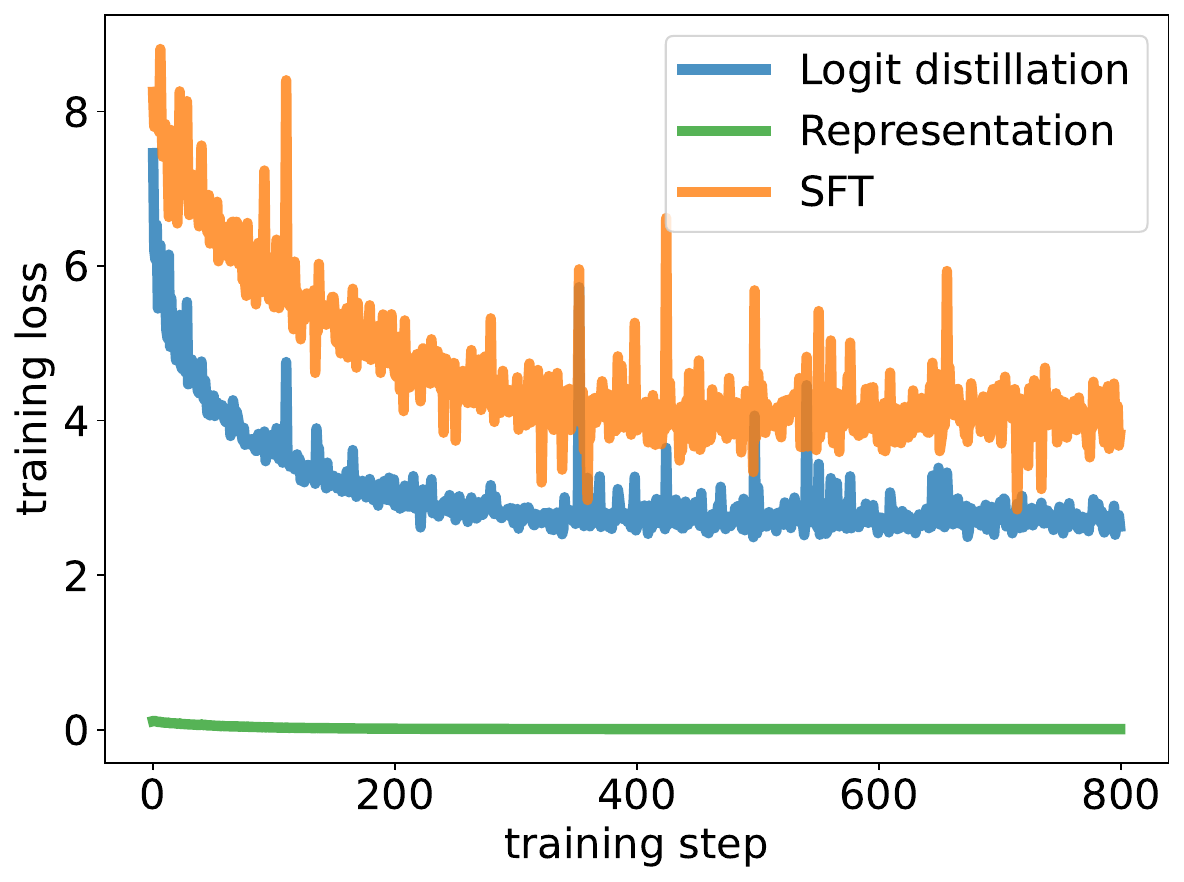}
    }
    \subfloat{
        \includegraphics[width=0.245\textwidth]{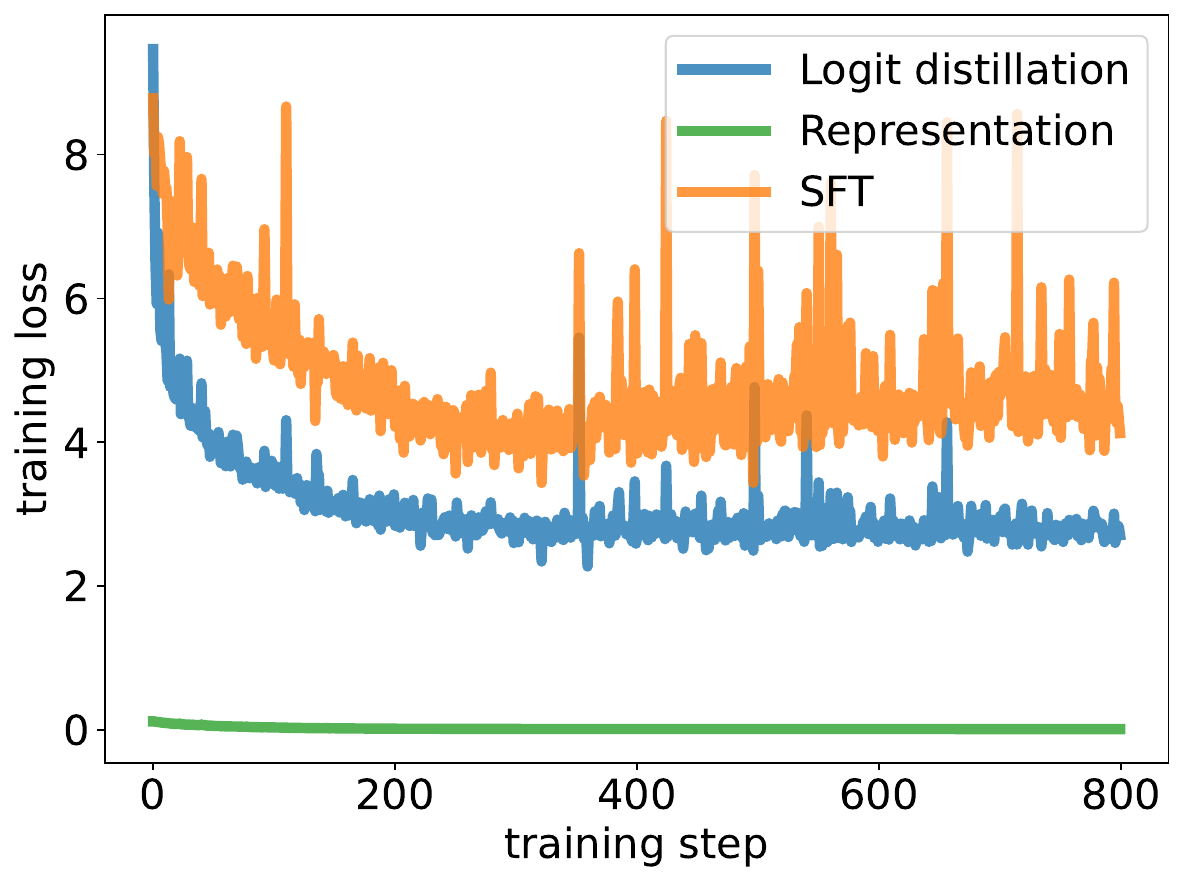}
    }

    \subfloat{
        \includegraphics[width=0.245\textwidth]{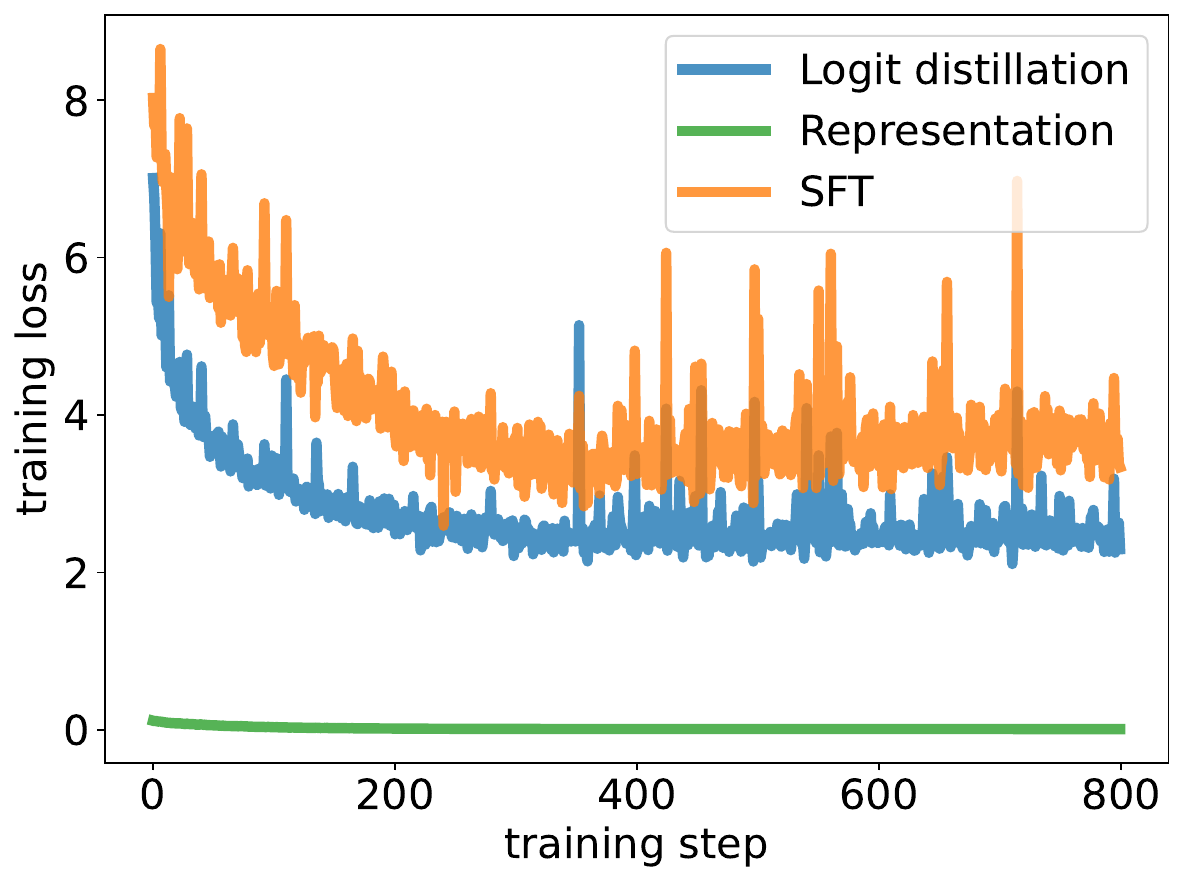}
    }
    \subfloat{
        \includegraphics[width=0.245\textwidth]{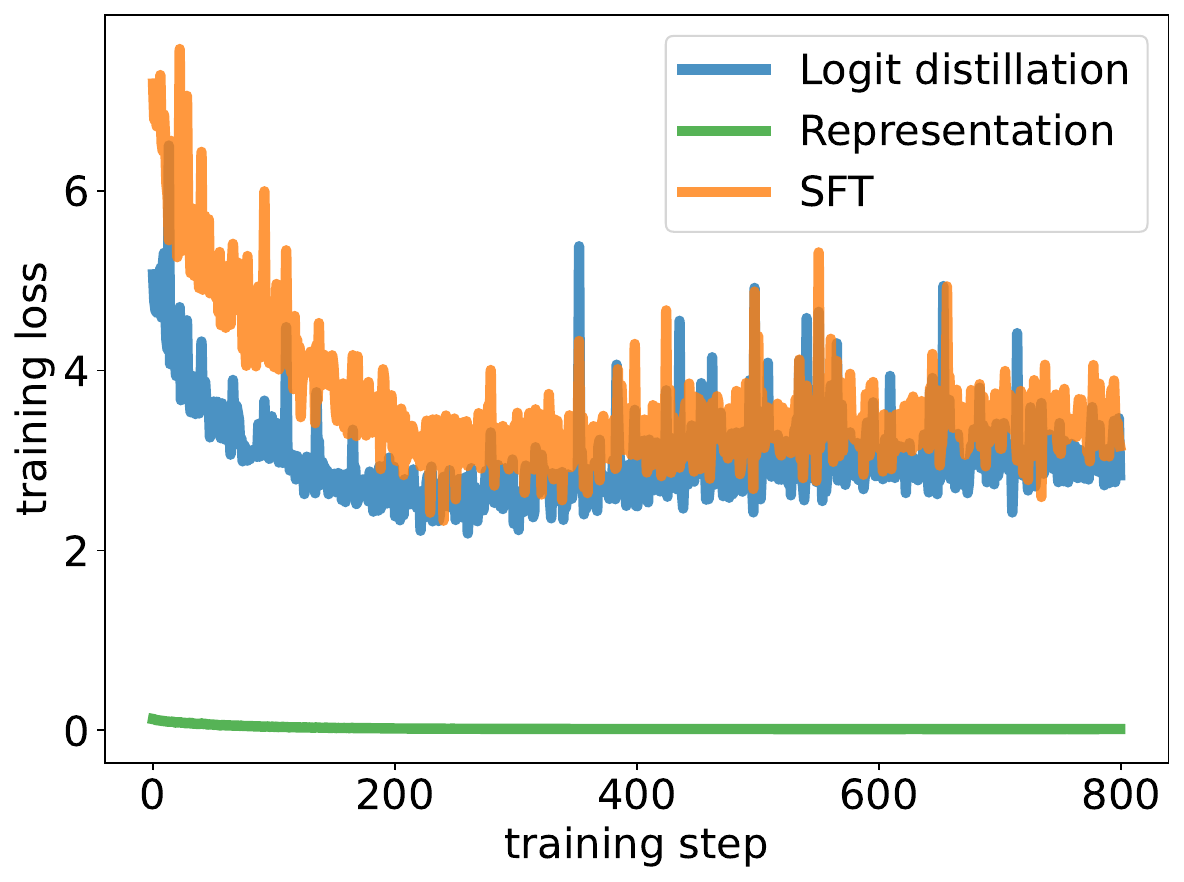}
    }
    \subfloat{
        \includegraphics[width=0.245\textwidth]{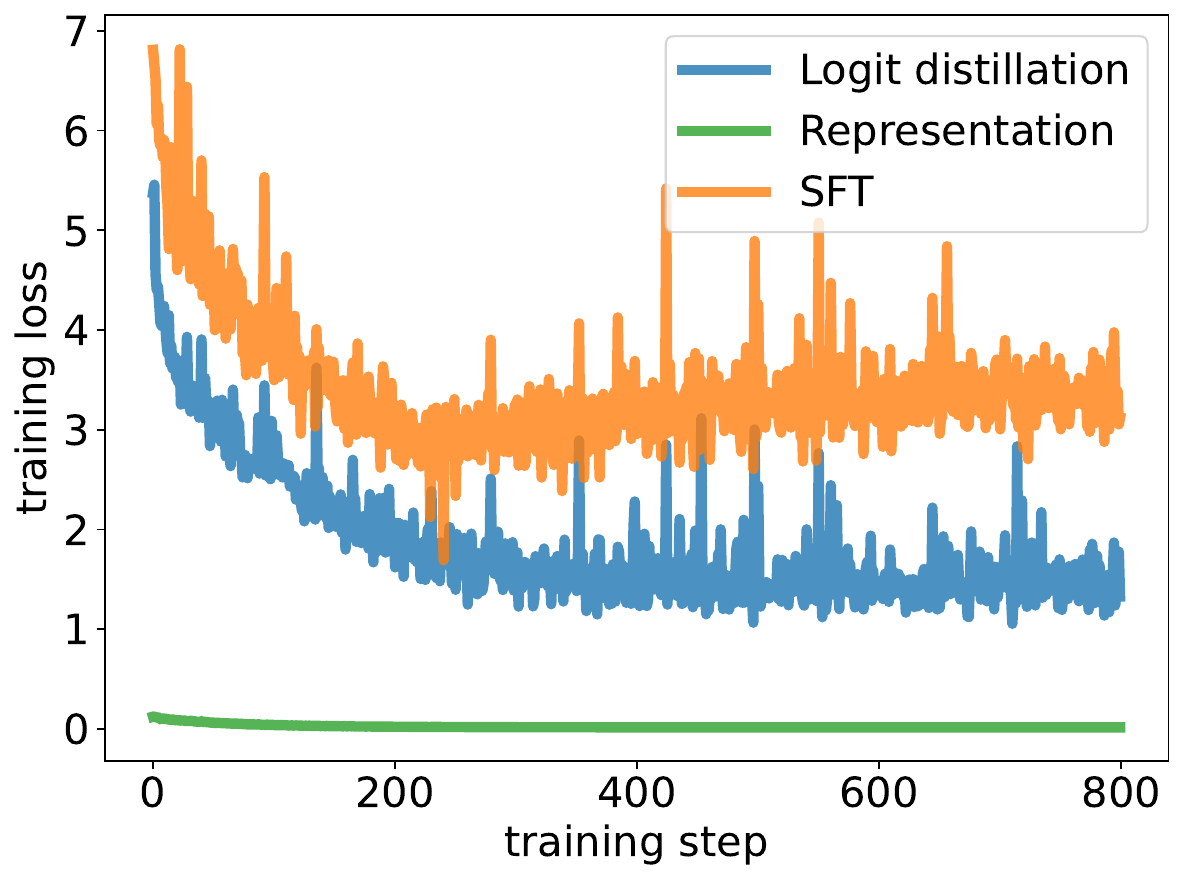}
    }
    \subfloat{
        \includegraphics[width=0.245\textwidth]{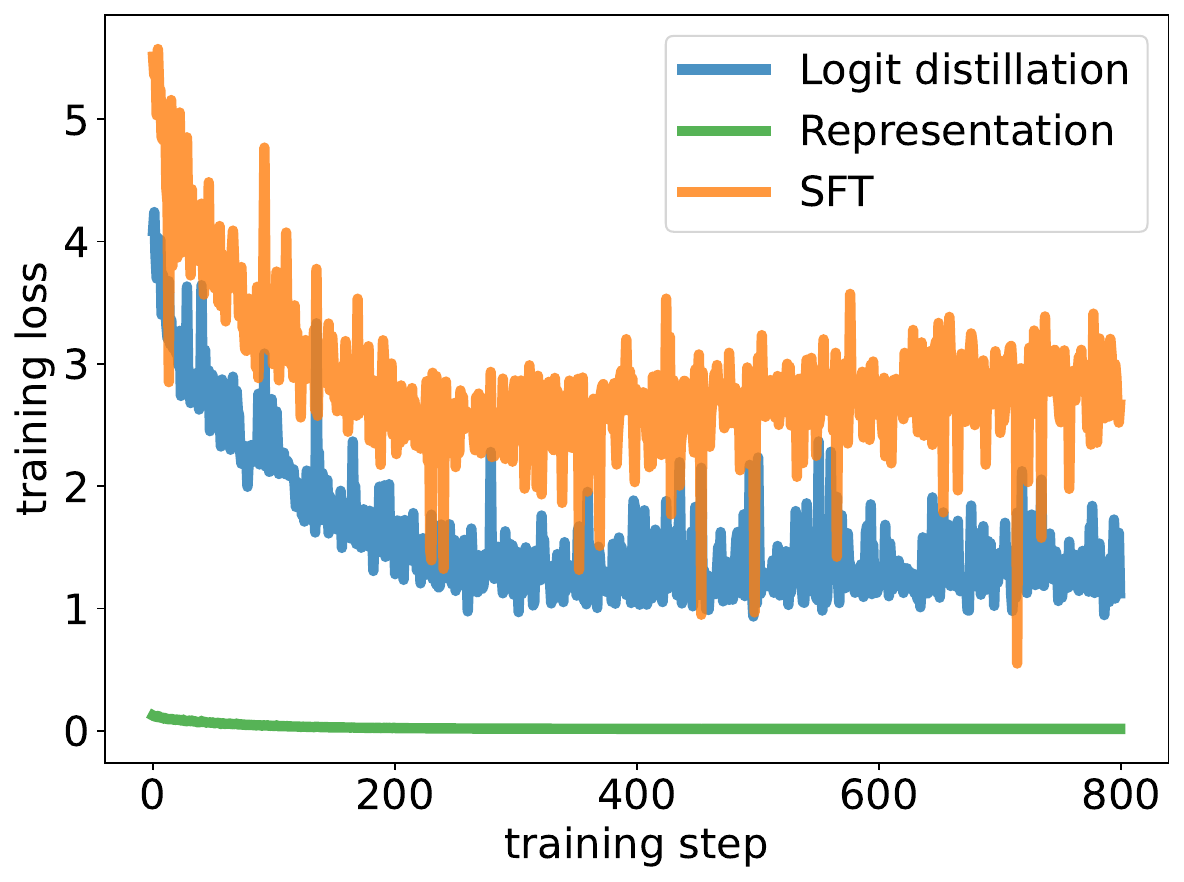}
    }

    \subfloat{
        \includegraphics[width=0.245\textwidth]{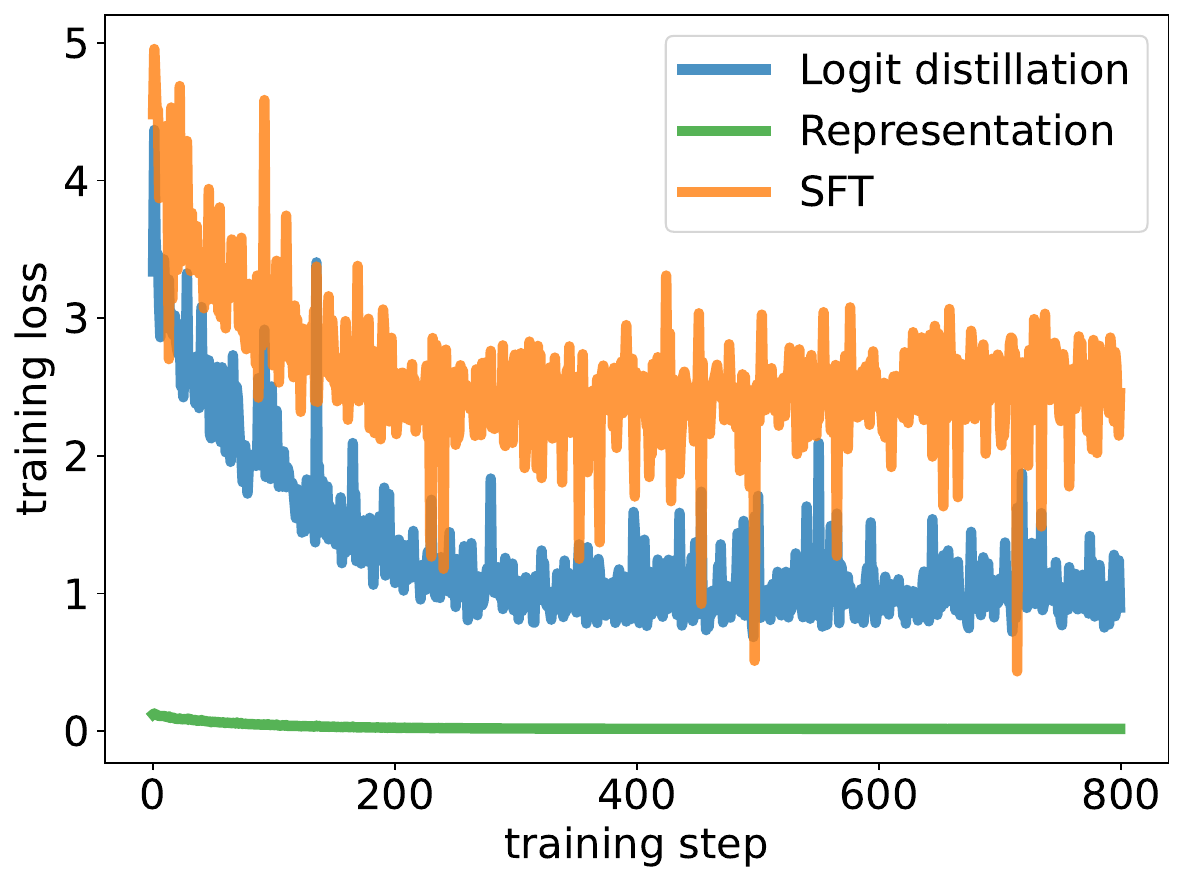}
    }
    \subfloat{
        \includegraphics[width=0.245\textwidth]{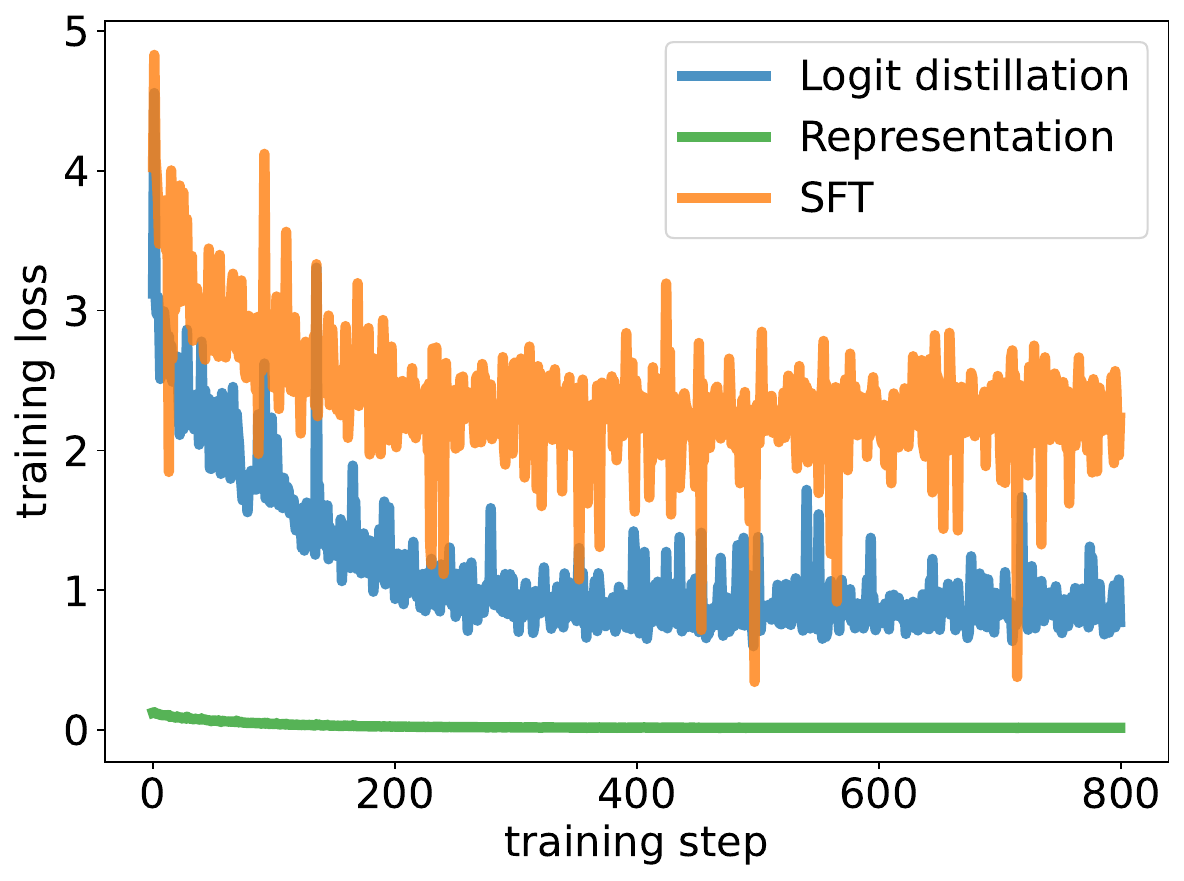}
    }
    \subfloat{
        \includegraphics[width=0.245\textwidth]{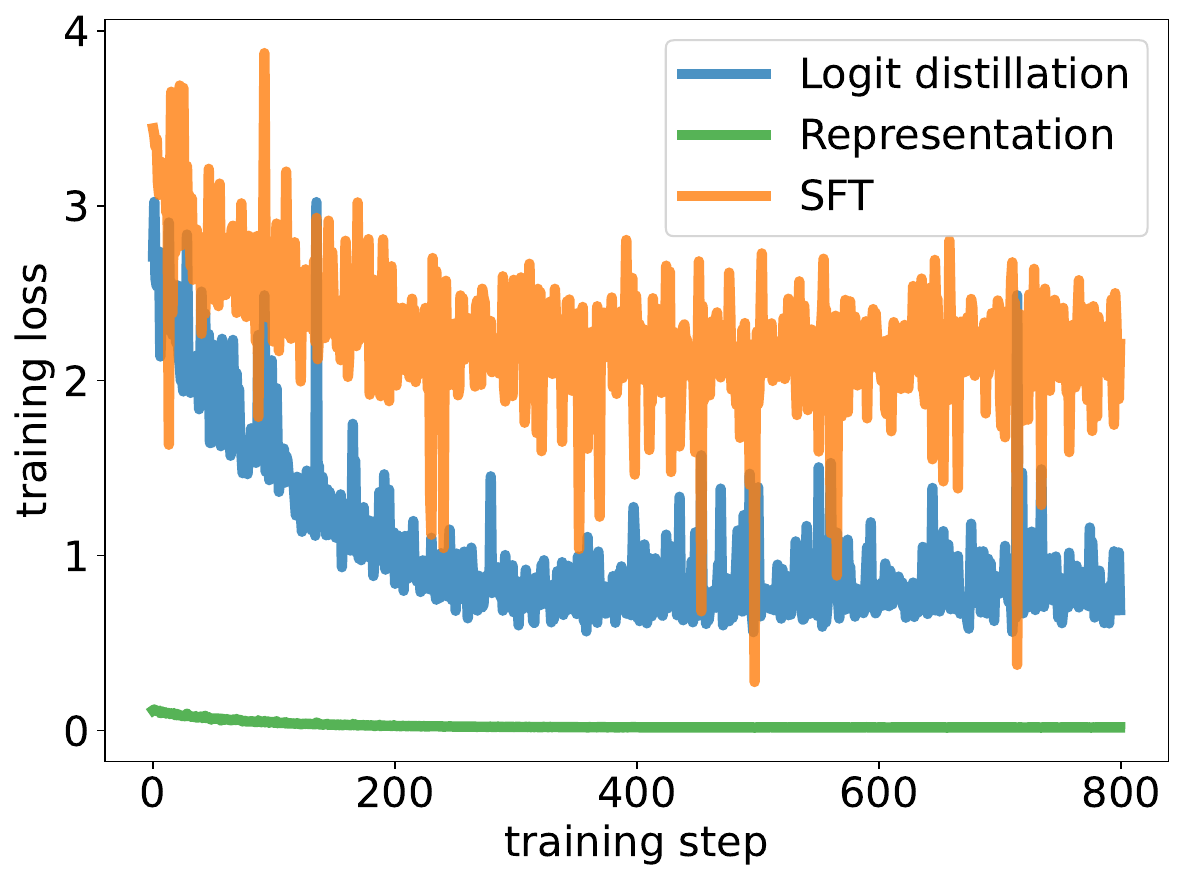}
    }
    \subfloat{
        \includegraphics[width=0.245\textwidth]{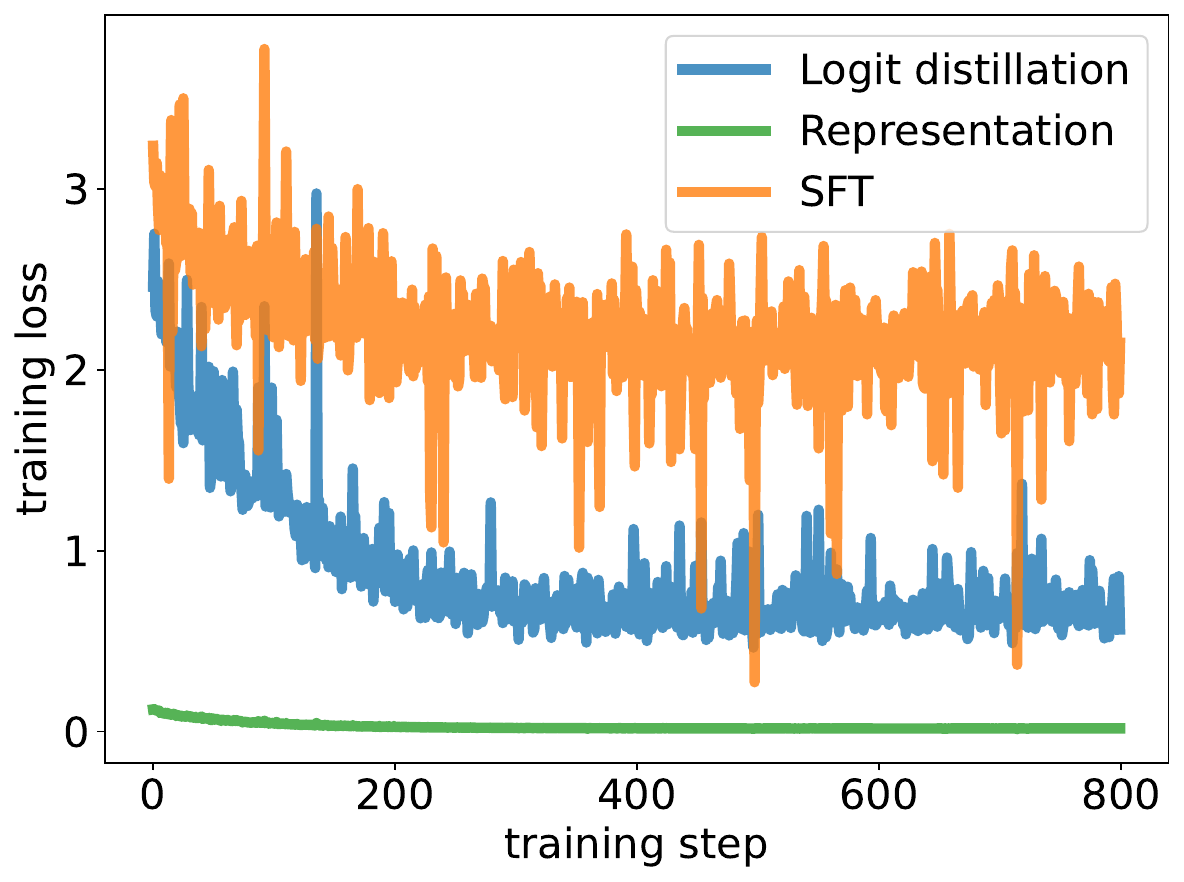}
    }

    \caption{\textbf{Low-rank linear adapter training curves for the first 24 Mistral 7b blocks with a rank of 32} trained using three different objectives including (a) MSE loss defined on the representation, (b) supervised fine-tuning (SFT), and (c) logit distillation where logits are distilled from the full model. Rest of the blocks are visualized in Fig.~\ref{fig:linear_adapters_rank_32_llama2_train_loss_b}.}
    \label{fig:linear_adapters_rank_32_mistral_train_loss_a}
\end{figure}

\begin{figure}[t]
    \centering
    \subfloat{
        \includegraphics[width=0.245\textwidth]{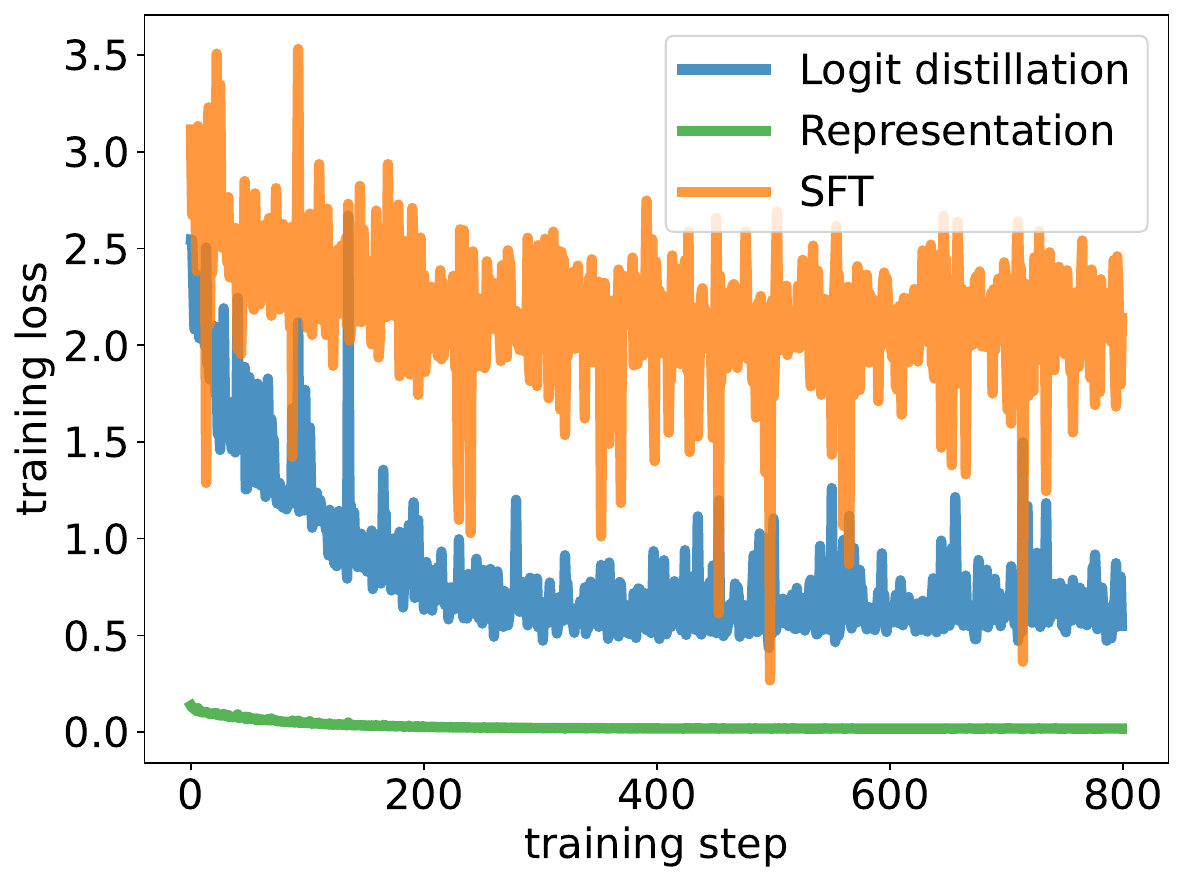}
    }
    \subfloat{
        \includegraphics[width=0.245\textwidth]{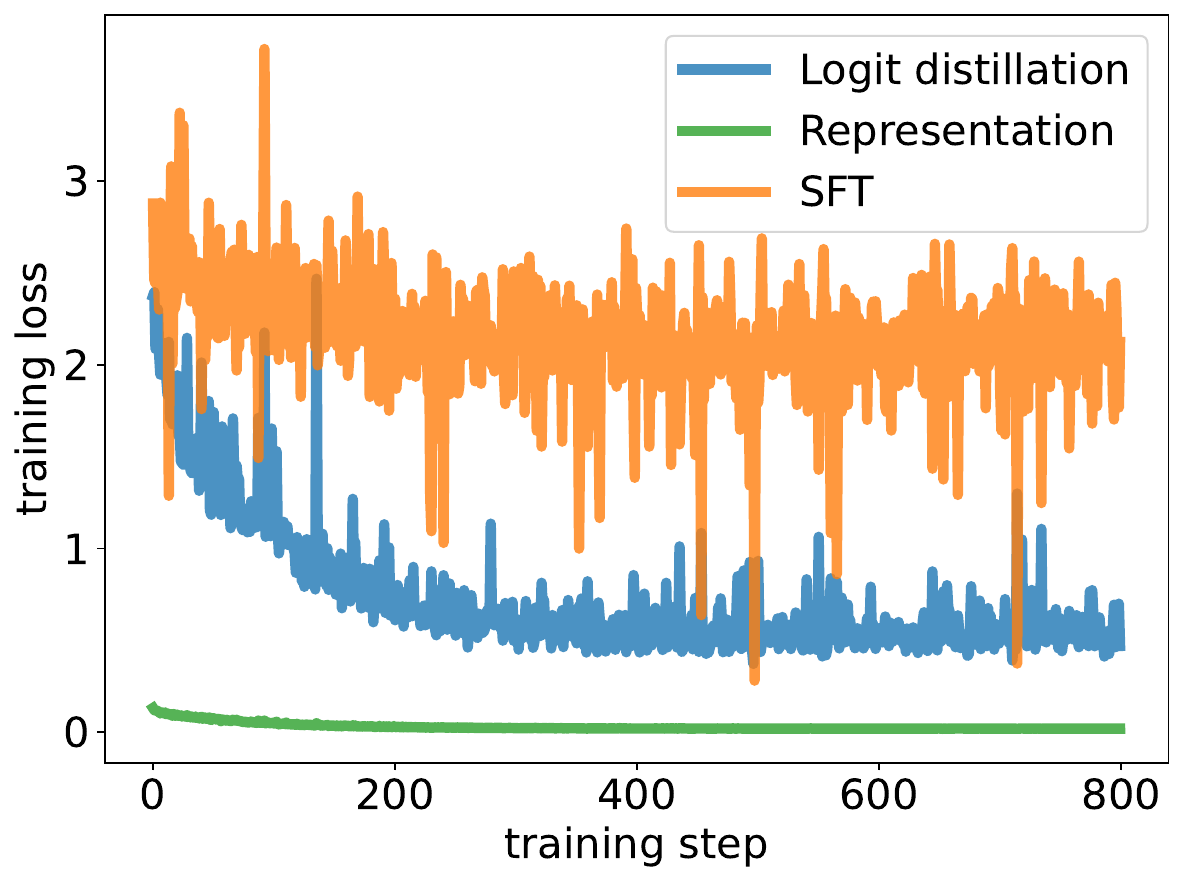}
    }
    \subfloat{
        \includegraphics[width=0.245\textwidth]{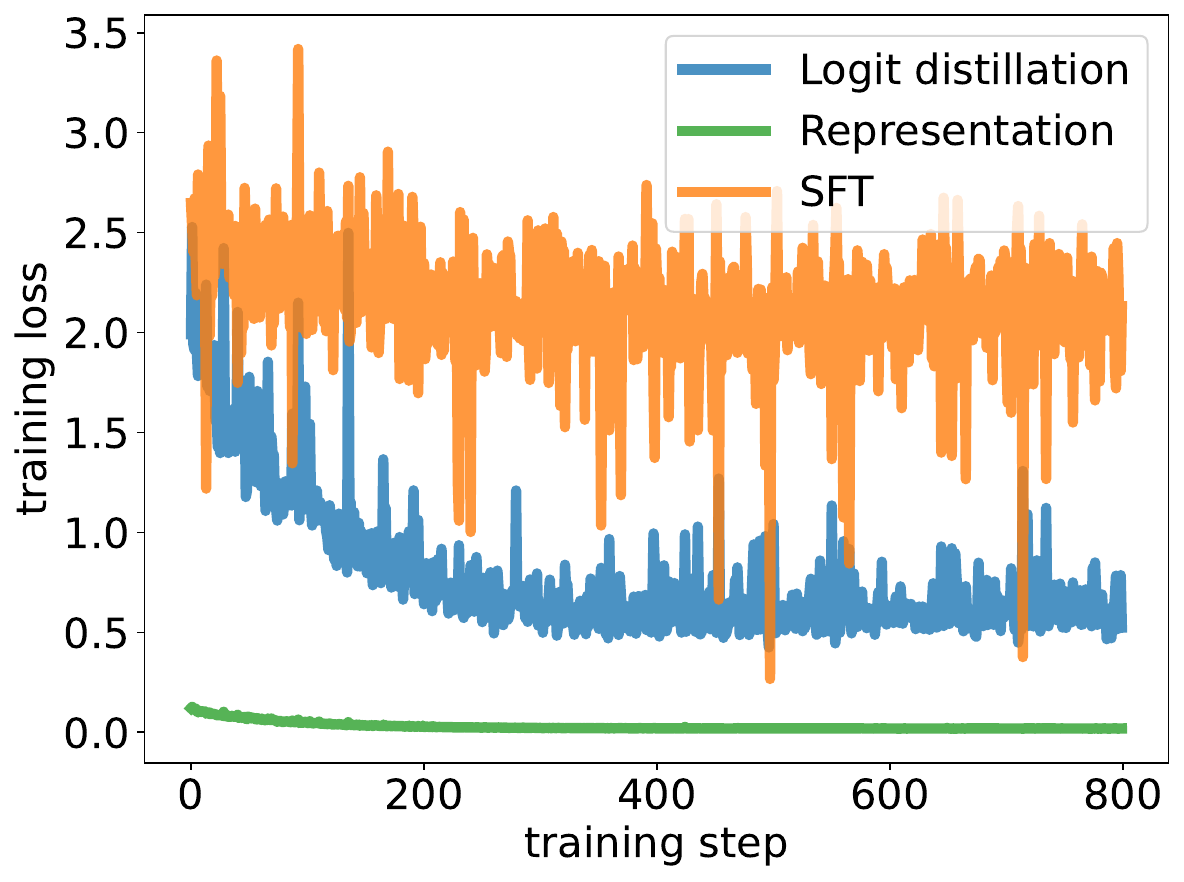}
    }
    \subfloat{
        \includegraphics[width=0.245\textwidth]{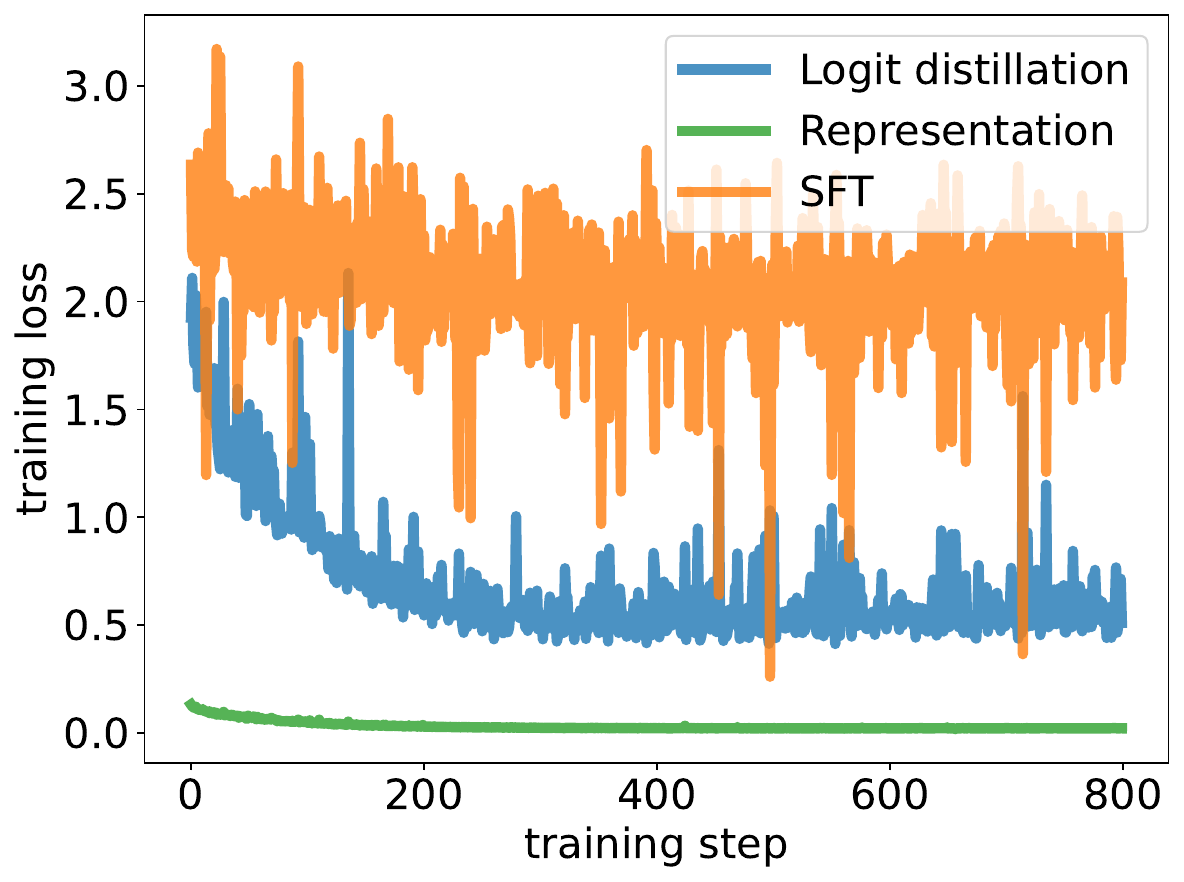}
    }

    \subfloat{
        \includegraphics[width=0.245\textwidth]{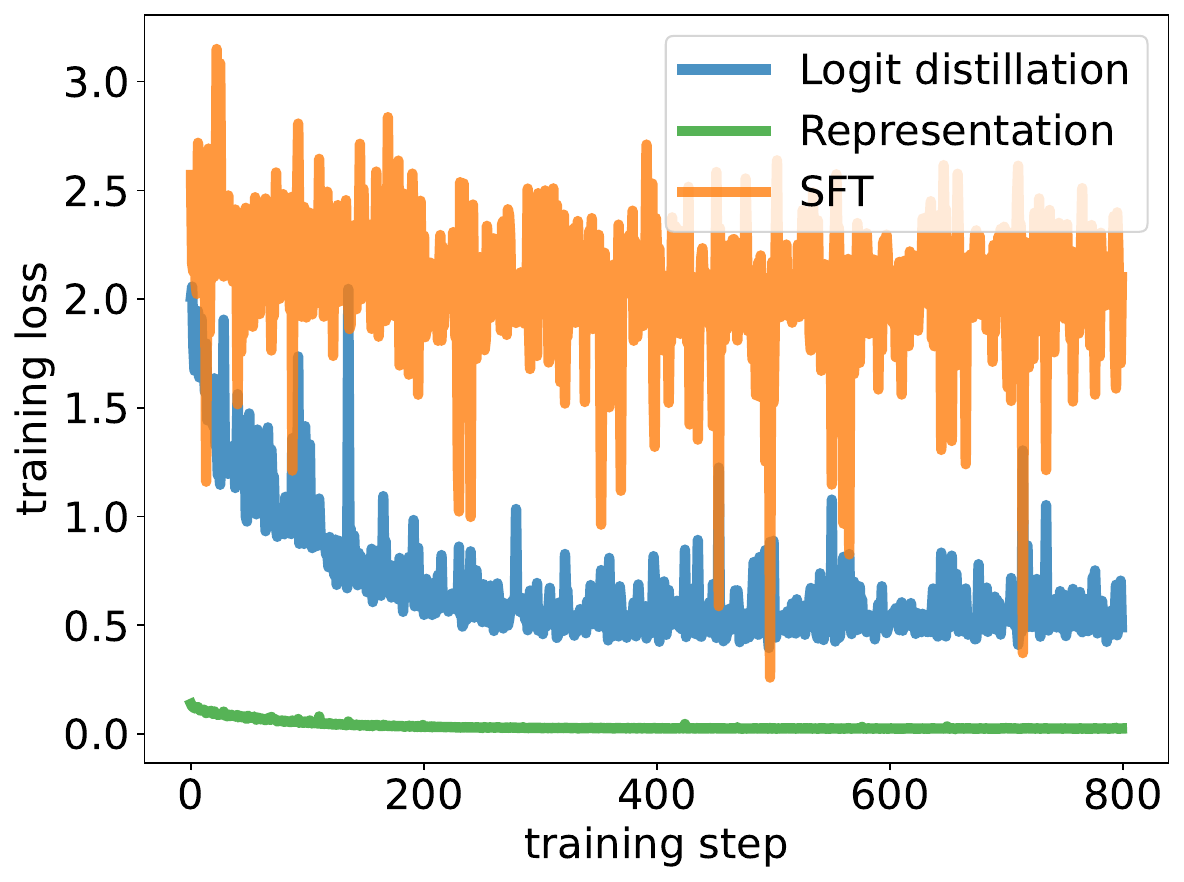}
    }
    \subfloat{
        \includegraphics[width=0.245\textwidth]{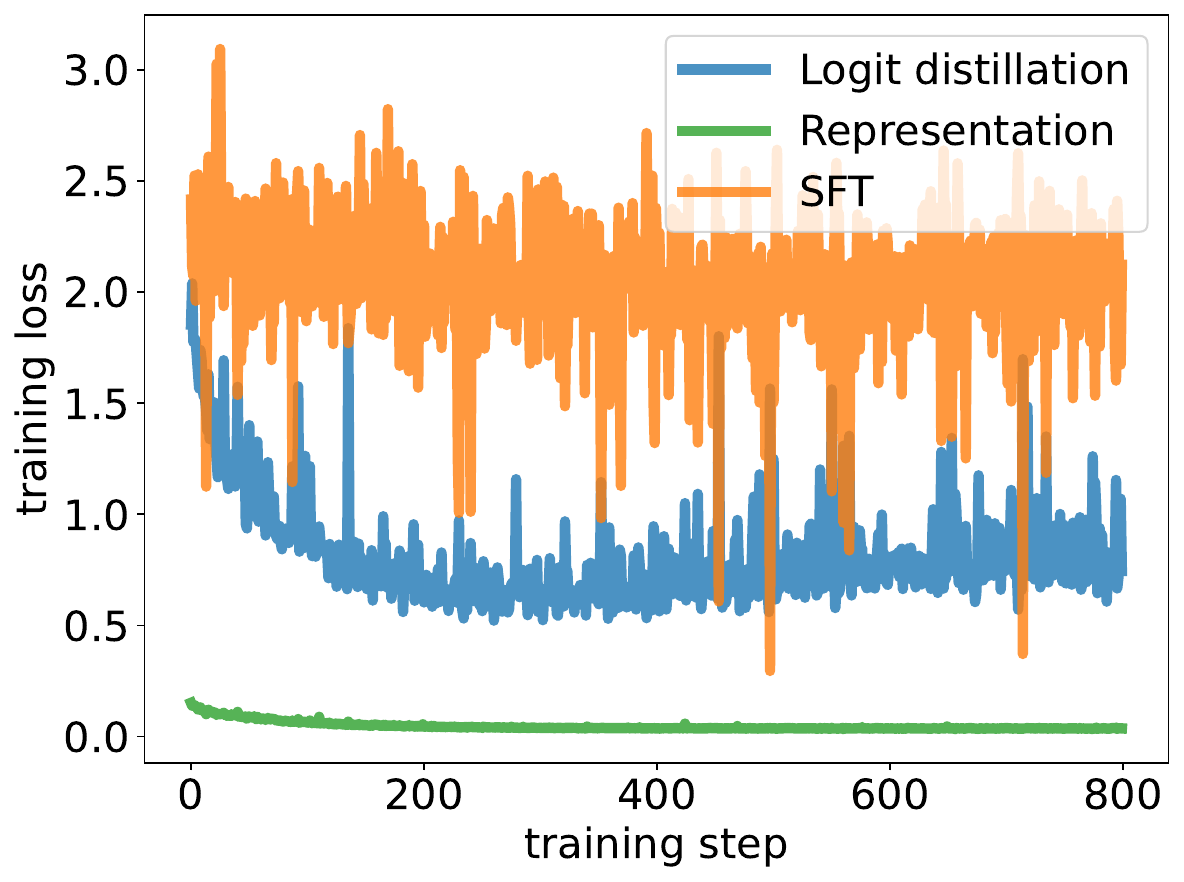}
    }
    \subfloat{
        \includegraphics[width=0.245\textwidth]{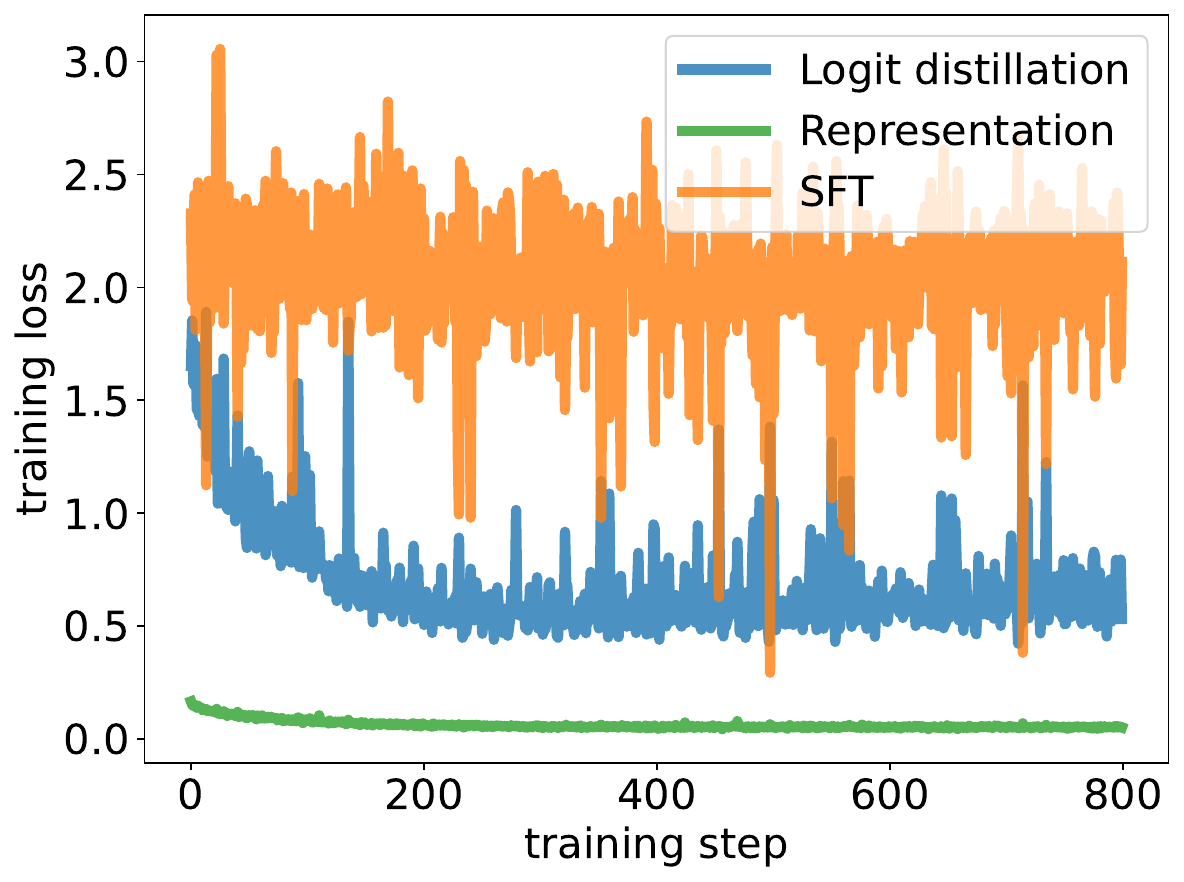}
    }
    \subfloat{
        \includegraphics[width=0.245\textwidth]{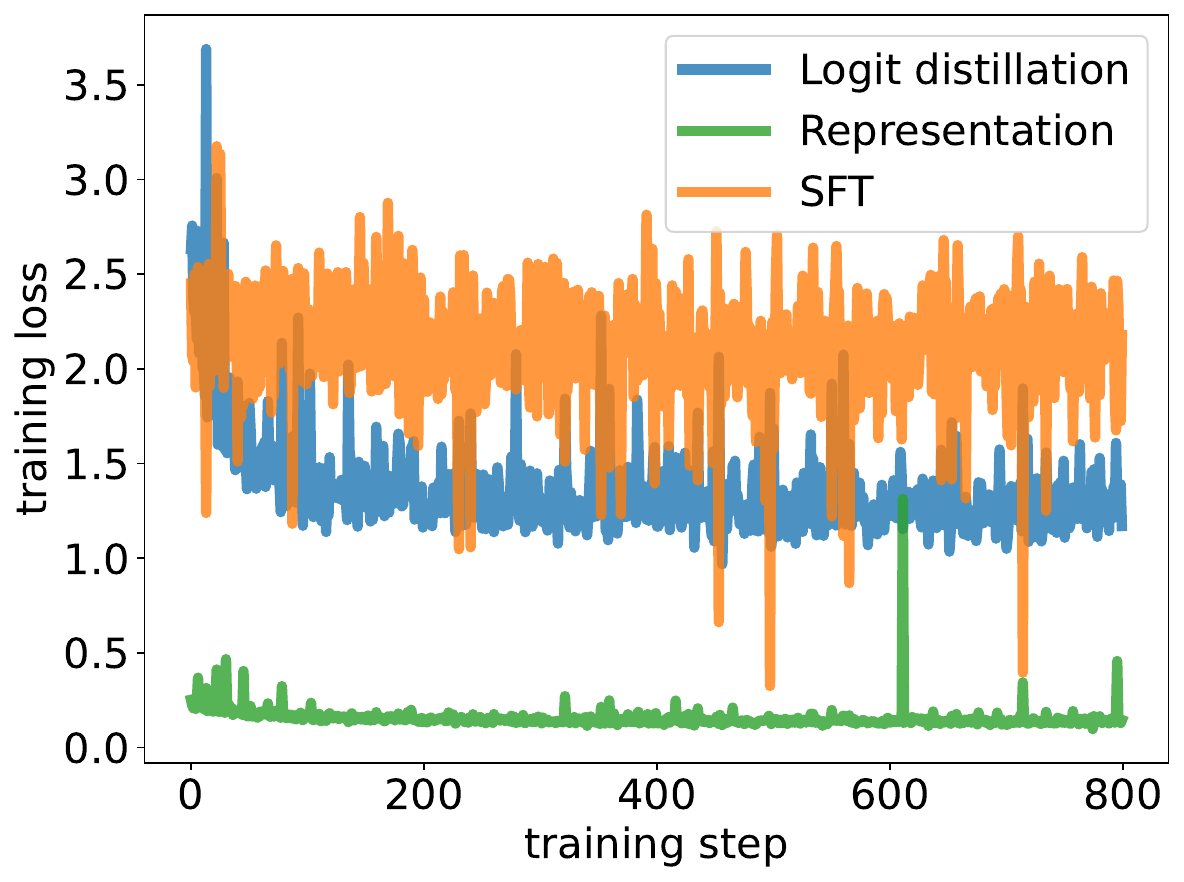}
    }

    \caption{\textbf{Low-rank linear adapter training curves for the last 8 Mistral 7b blocks with a rank of 32} trained using three different objectives including (a) MSE loss defined on the representation, (b) supervised fine-tuning (SFT), and (c) logit distillation where logits are distilled from the full model. The first set of blocks are visualized in Fig.~\ref{fig:linear_adapters_rank_32_llama2_train_loss_a}.}
    \label{fig:linear_adapters_rank_32_mistral_train_loss_b}
\end{figure}

The loss curves for the training of the low-rank adapter with a rank of 32 on Mistral are visualized in Fig.~\ref{fig:linear_adapters_rank_32_mistral_train_loss_a} and Fig.~\ref{fig:linear_adapters_rank_32_mistral_train_loss_b}.

\begin{figure}[t]
    \centering
    \subfloat{
        \includegraphics[width=0.245\textwidth]{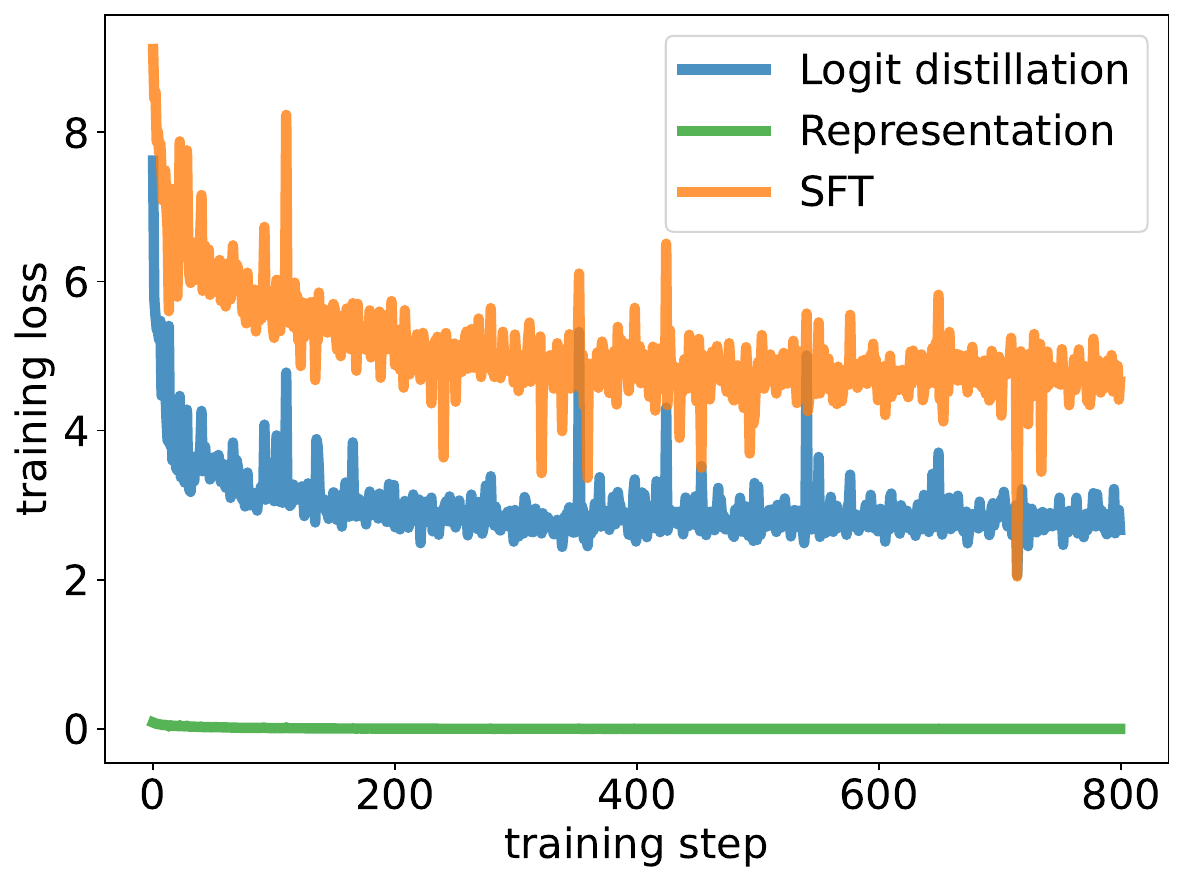}
    }
    \subfloat{
        \includegraphics[width=0.245\textwidth]{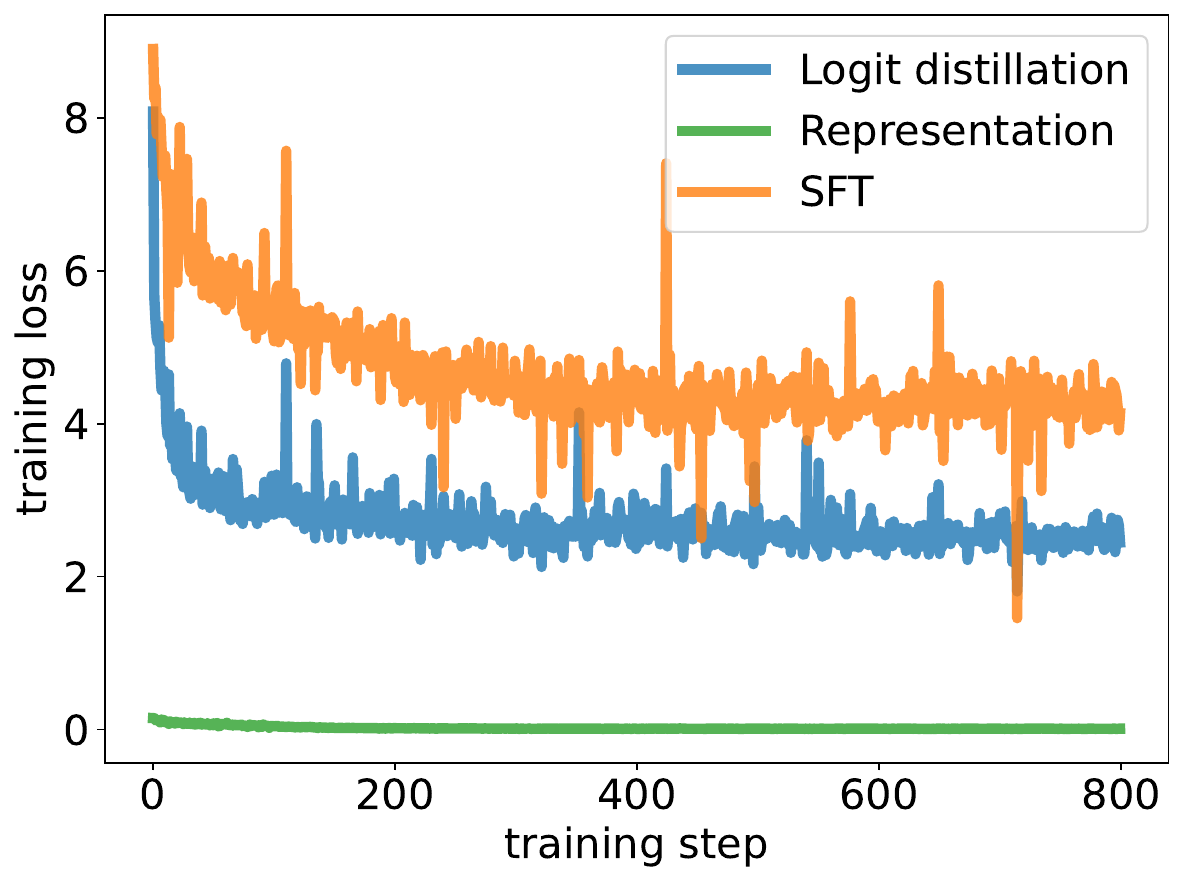}
    }
    \subfloat{
        \includegraphics[width=0.245\textwidth]{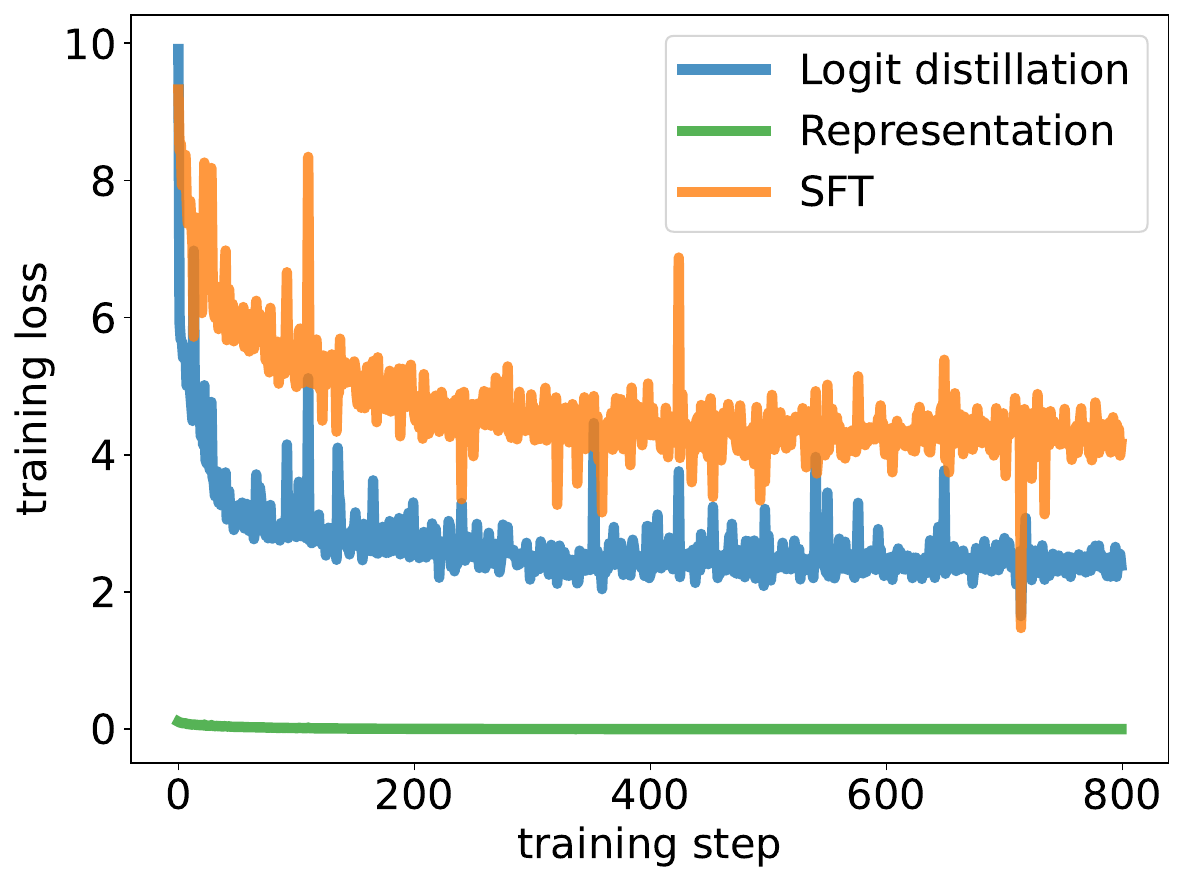}
    }
    \subfloat{
        \includegraphics[width=0.245\textwidth]{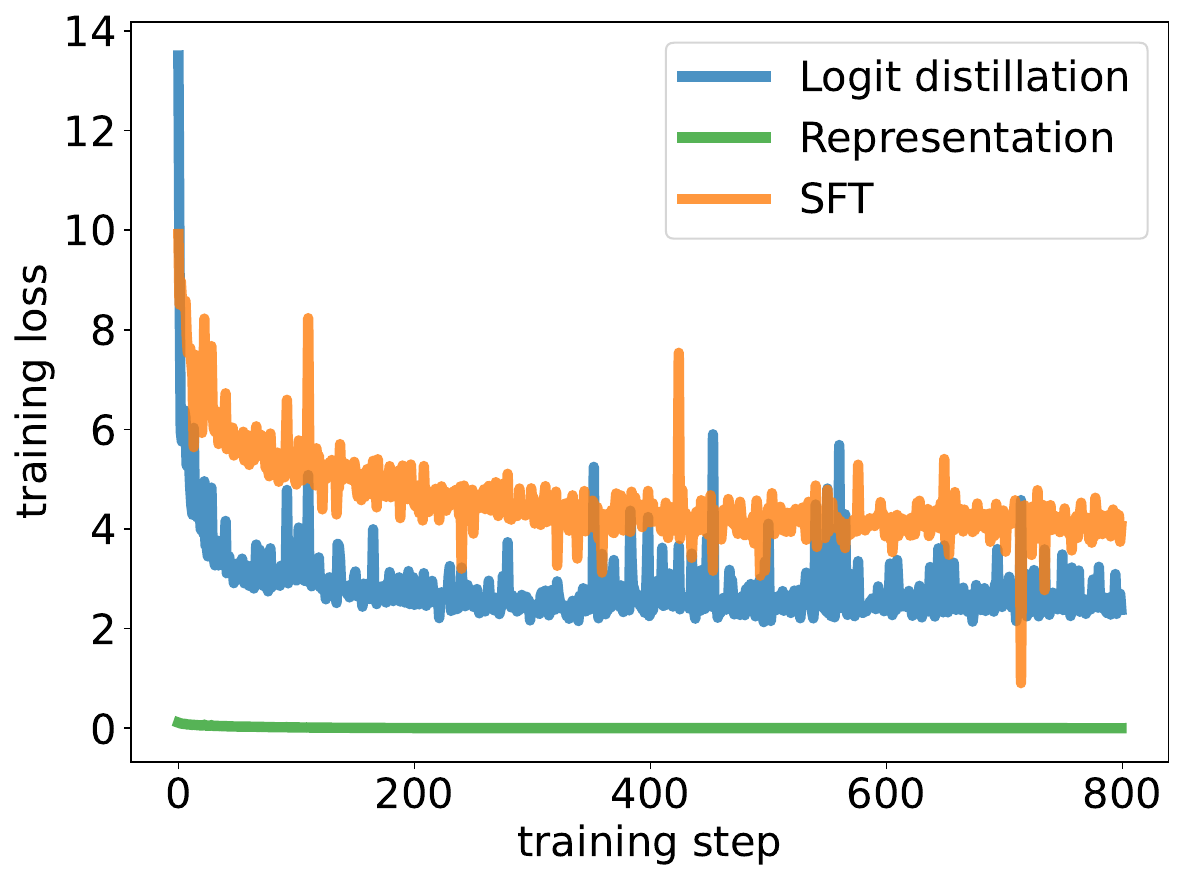}
    }

    \subfloat{
        \includegraphics[width=0.245\textwidth]{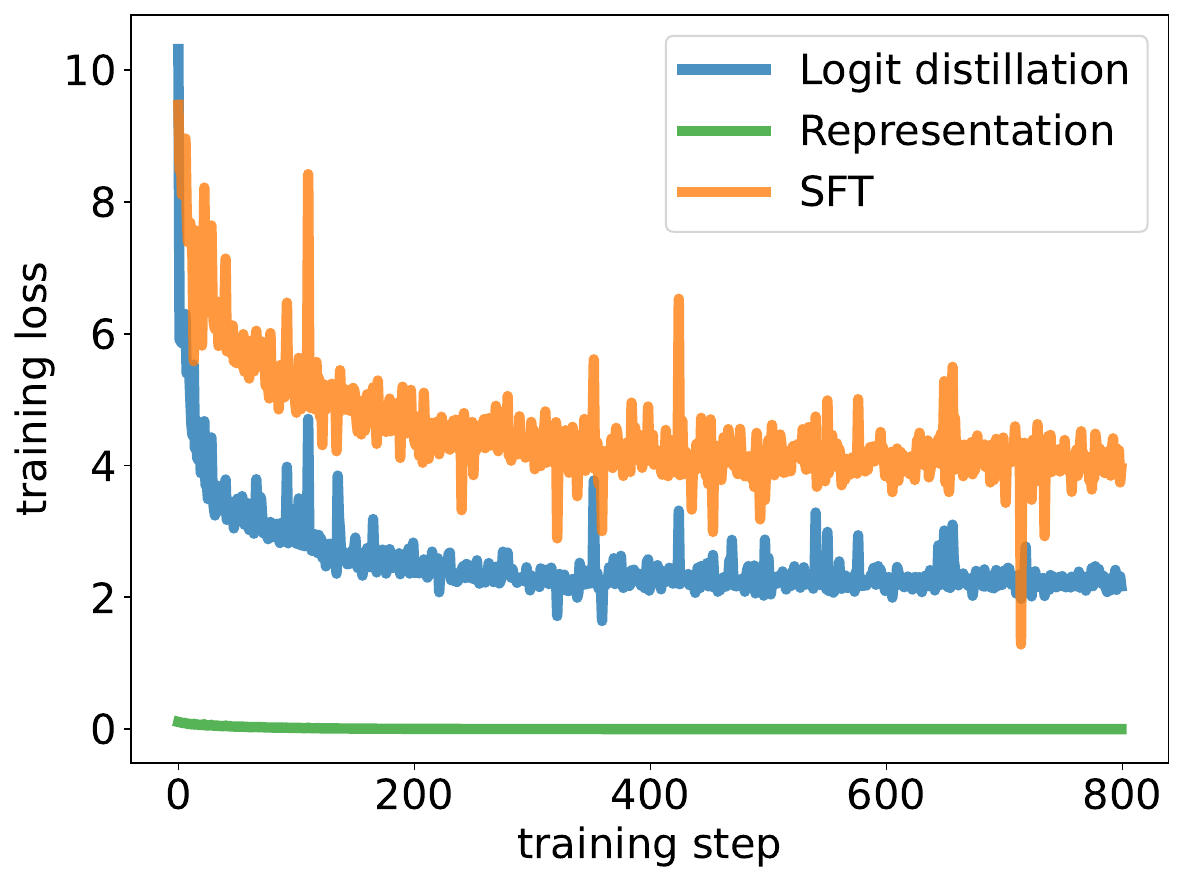}
    }
    \subfloat{
        \includegraphics[width=0.245\textwidth]{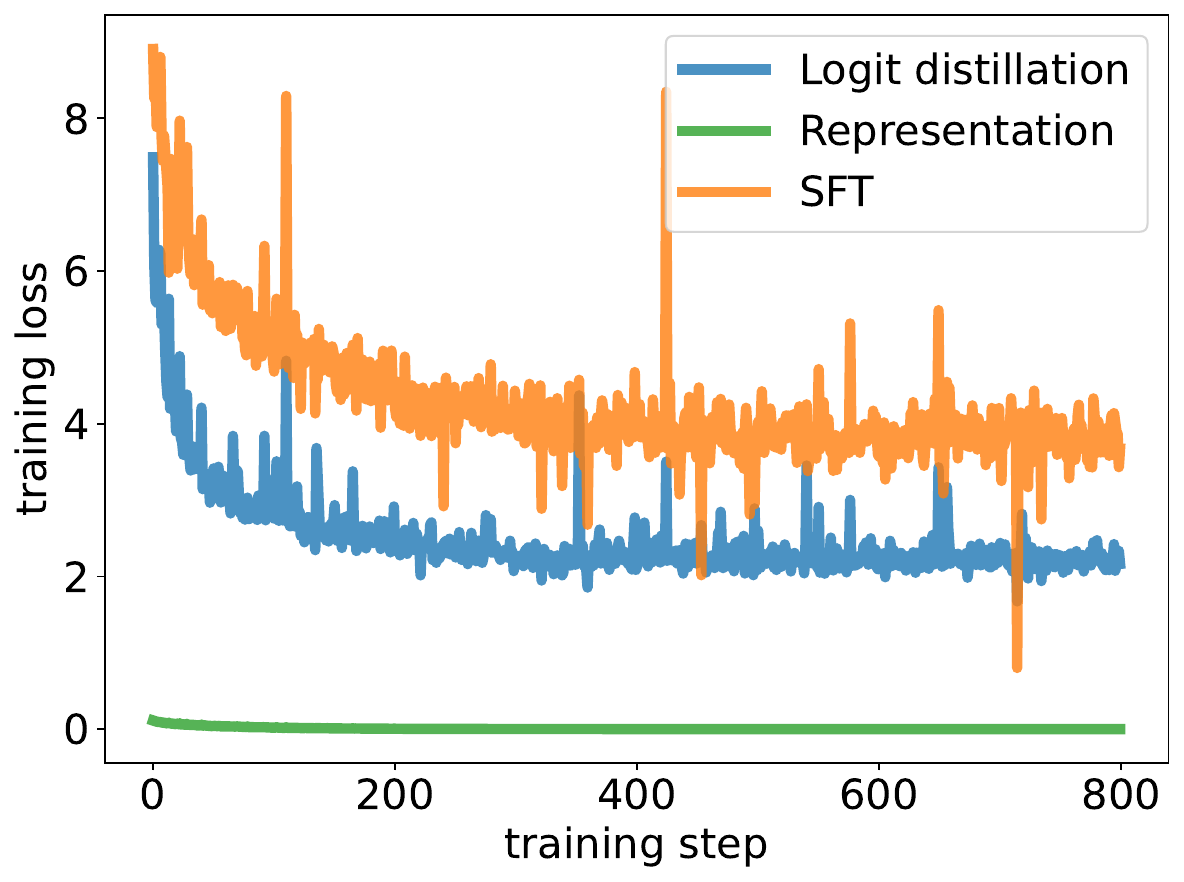}
    }
    \subfloat{
        \includegraphics[width=0.245\textwidth]{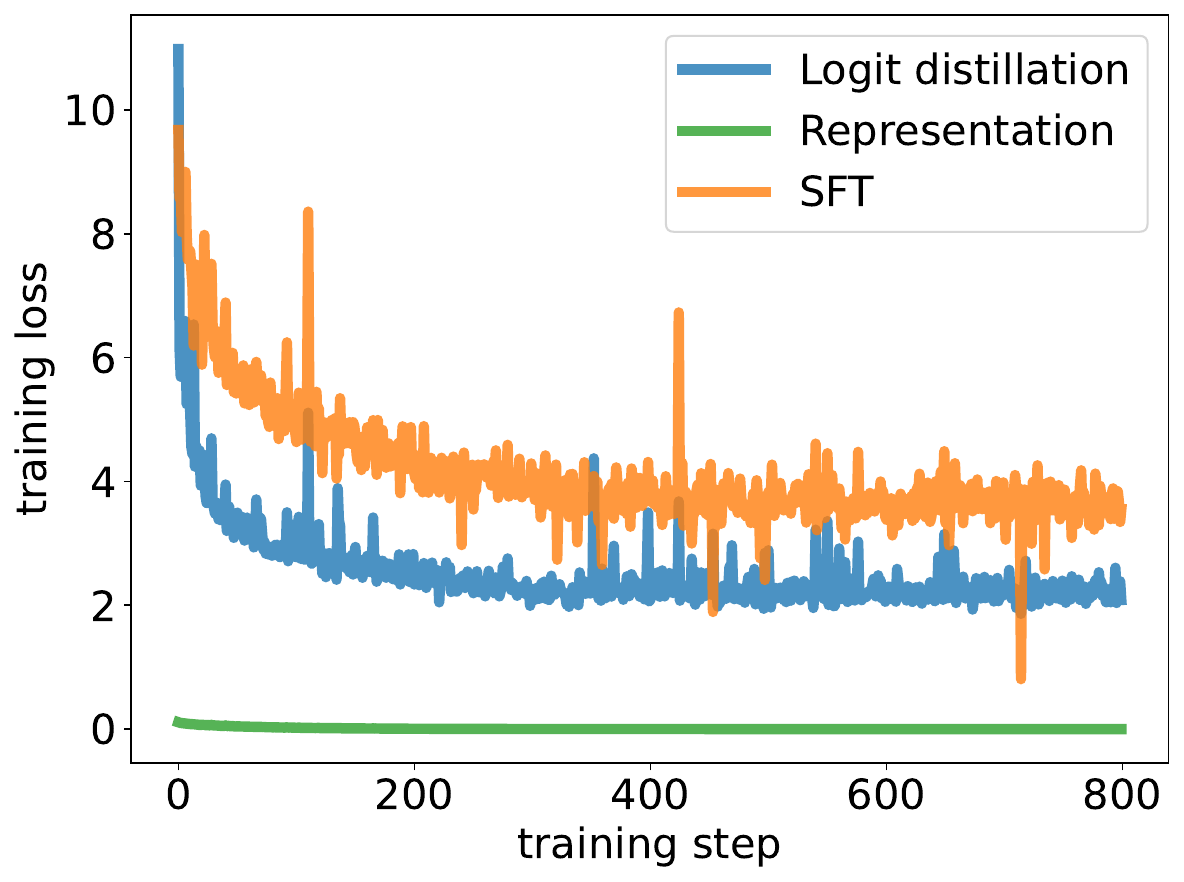}
    }
    \subfloat{
        \includegraphics[width=0.245\textwidth]{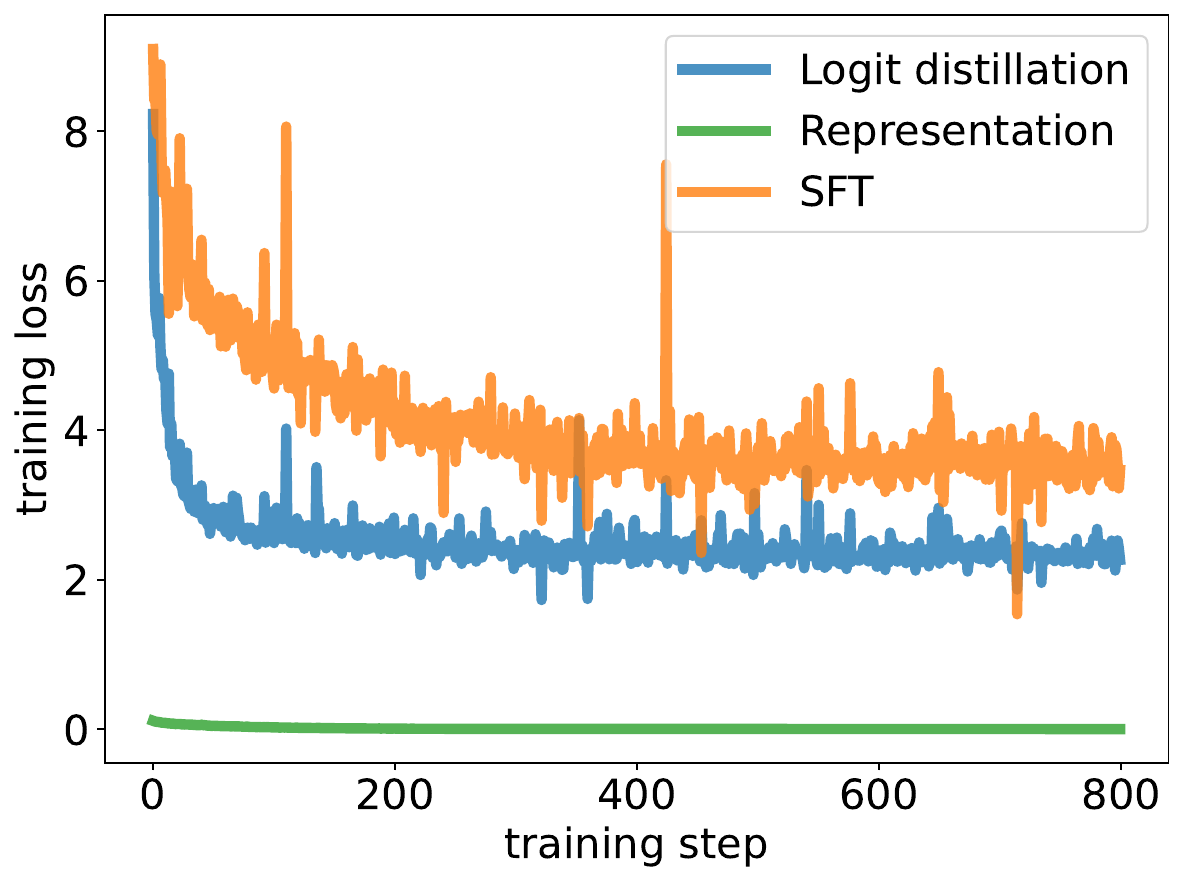}
    }

    \subfloat{
        \includegraphics[width=0.245\textwidth]{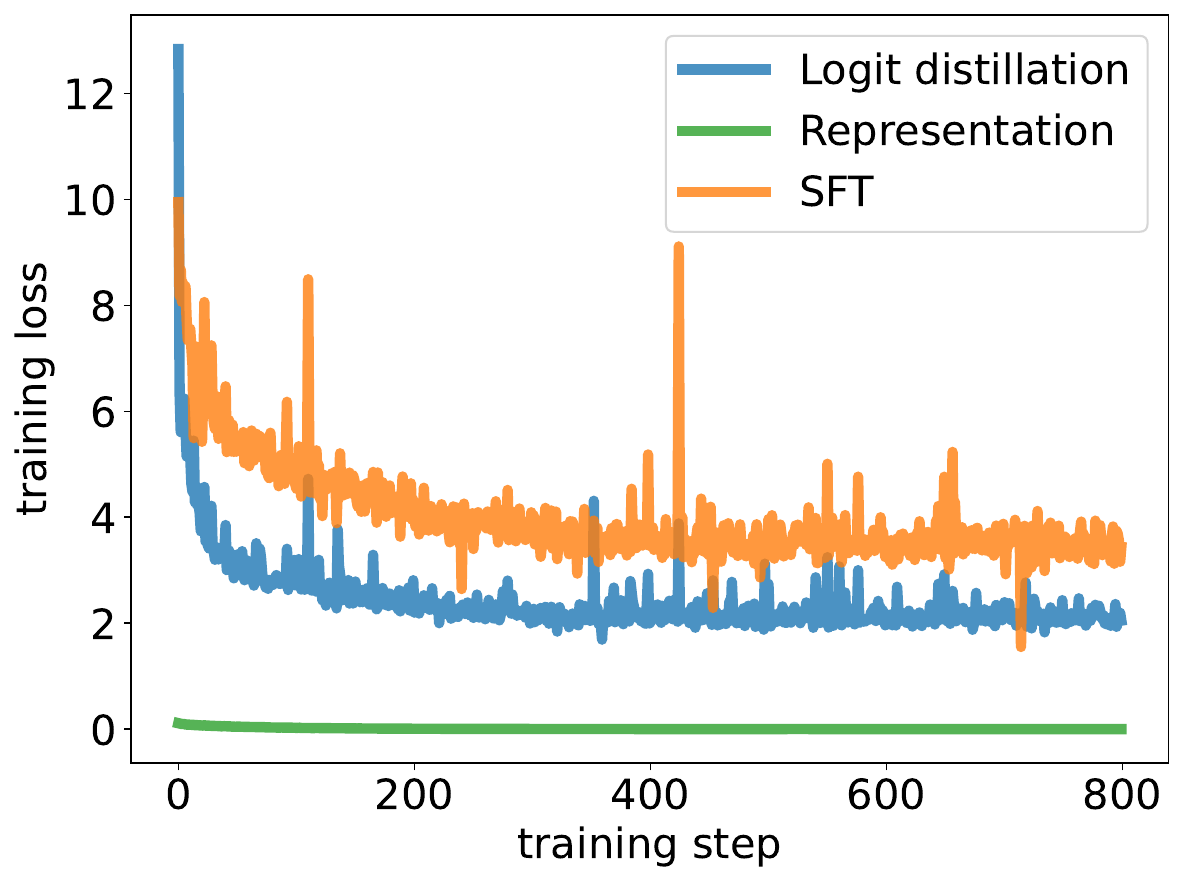}
    }
    \subfloat{
        \includegraphics[width=0.245\textwidth]{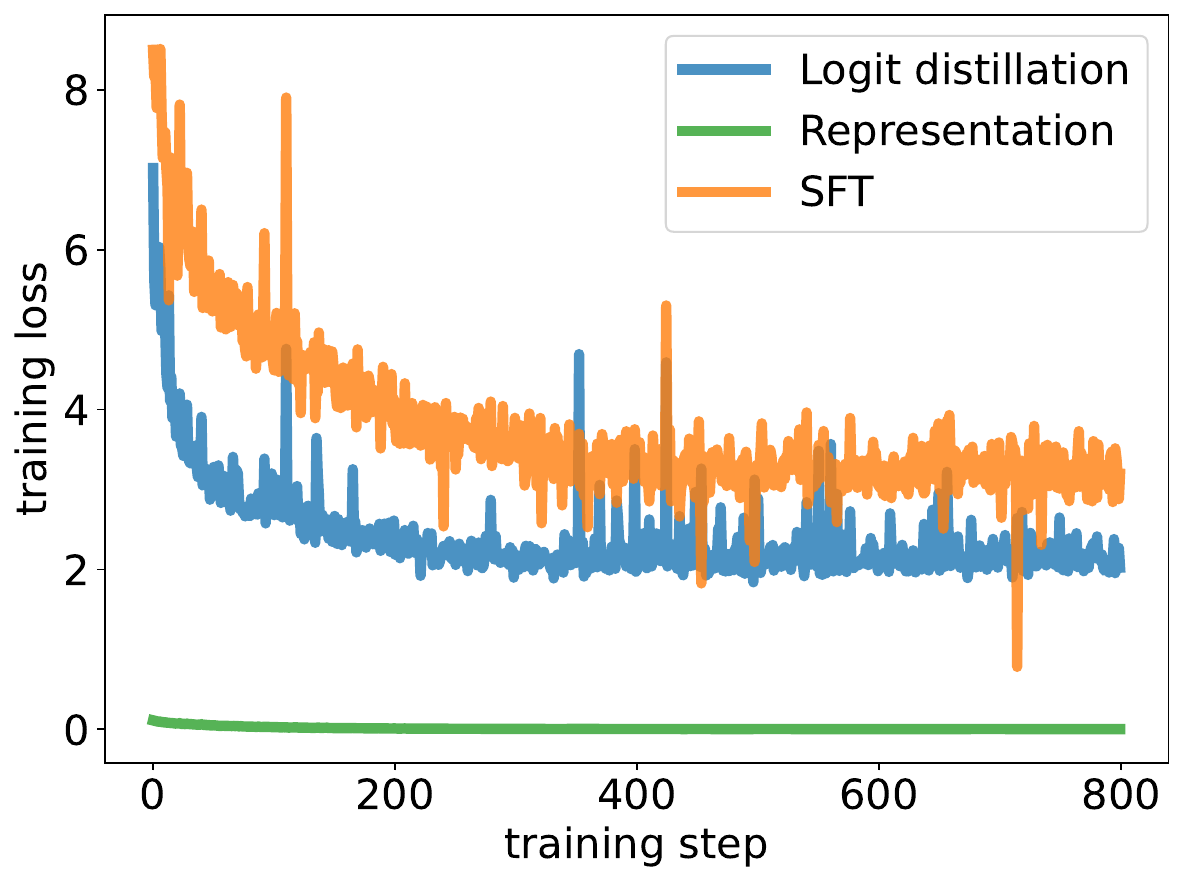}
    }
    \subfloat{
        \includegraphics[width=0.245\textwidth]{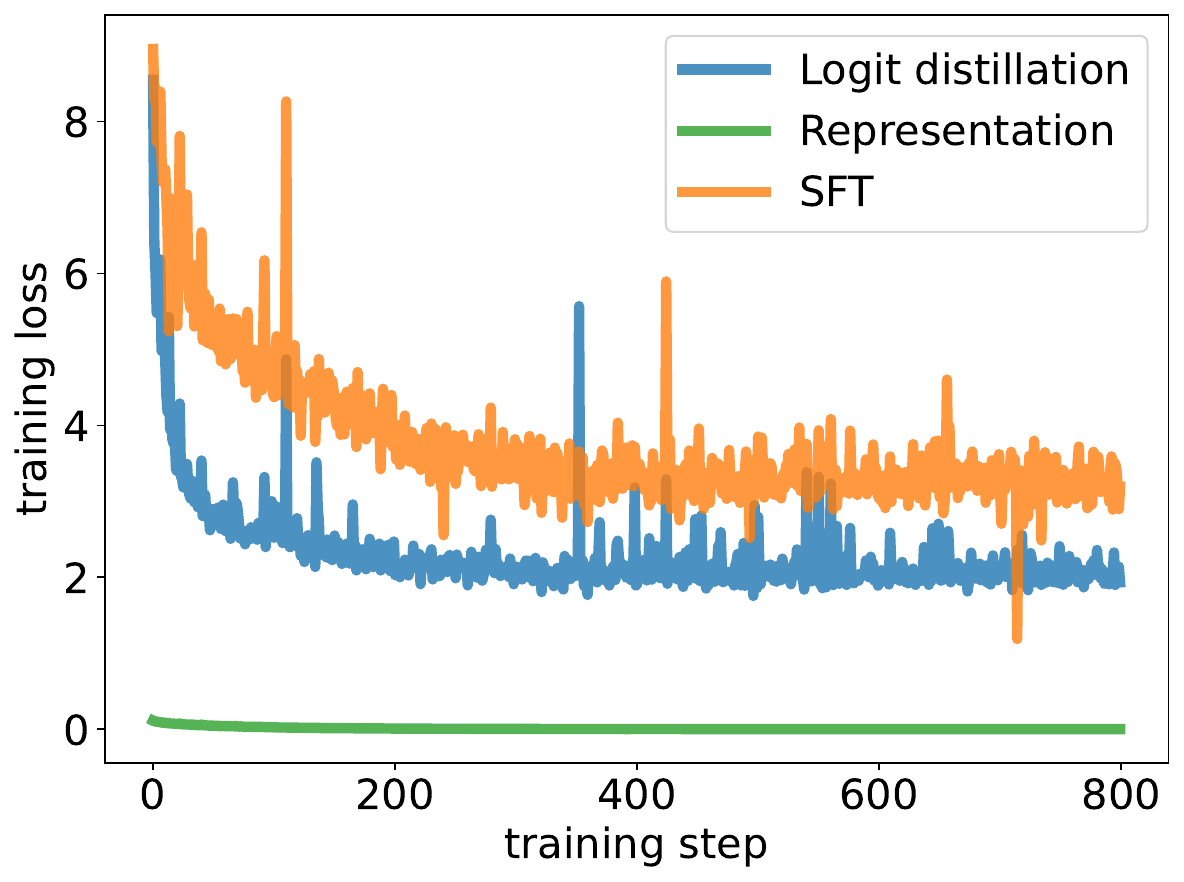}
    }
    \subfloat{
        \includegraphics[width=0.245\textwidth]{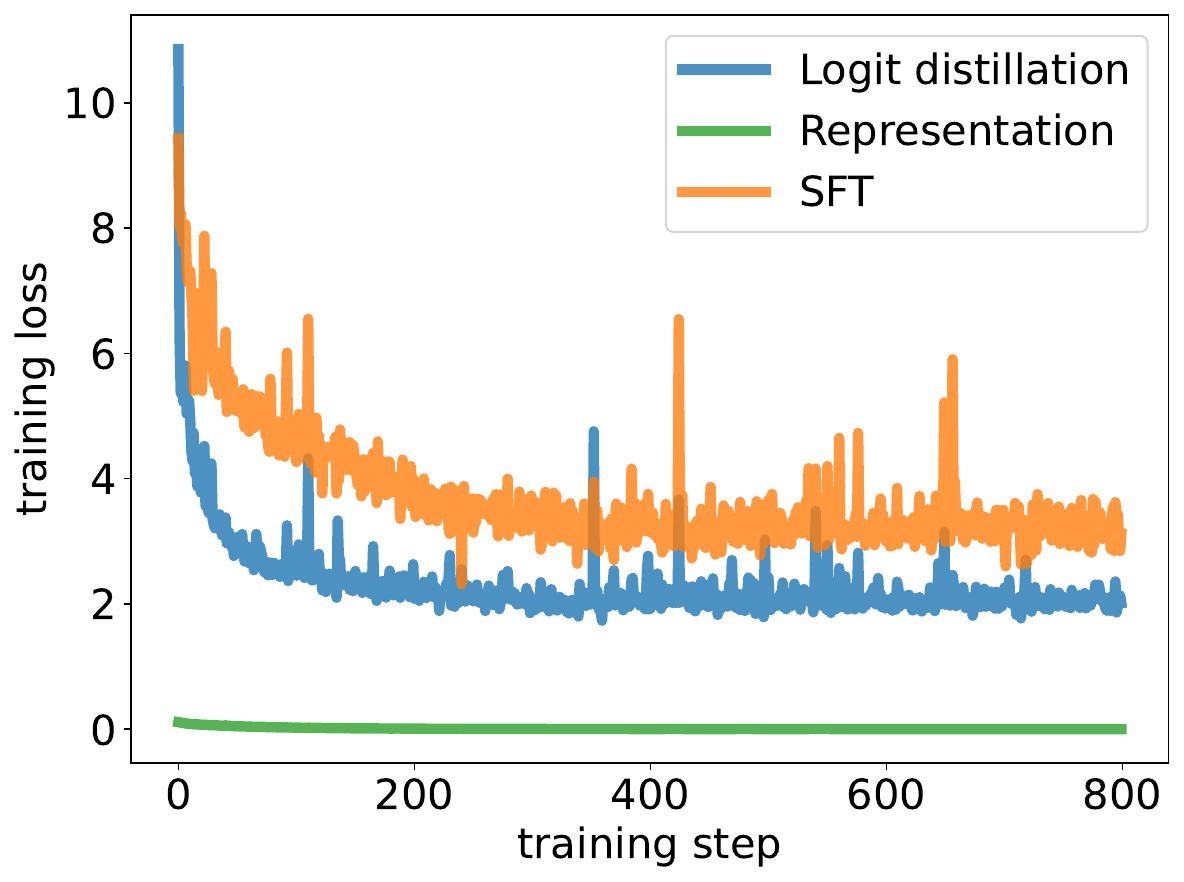}
    }

    \subfloat{
        \includegraphics[width=0.245\textwidth]{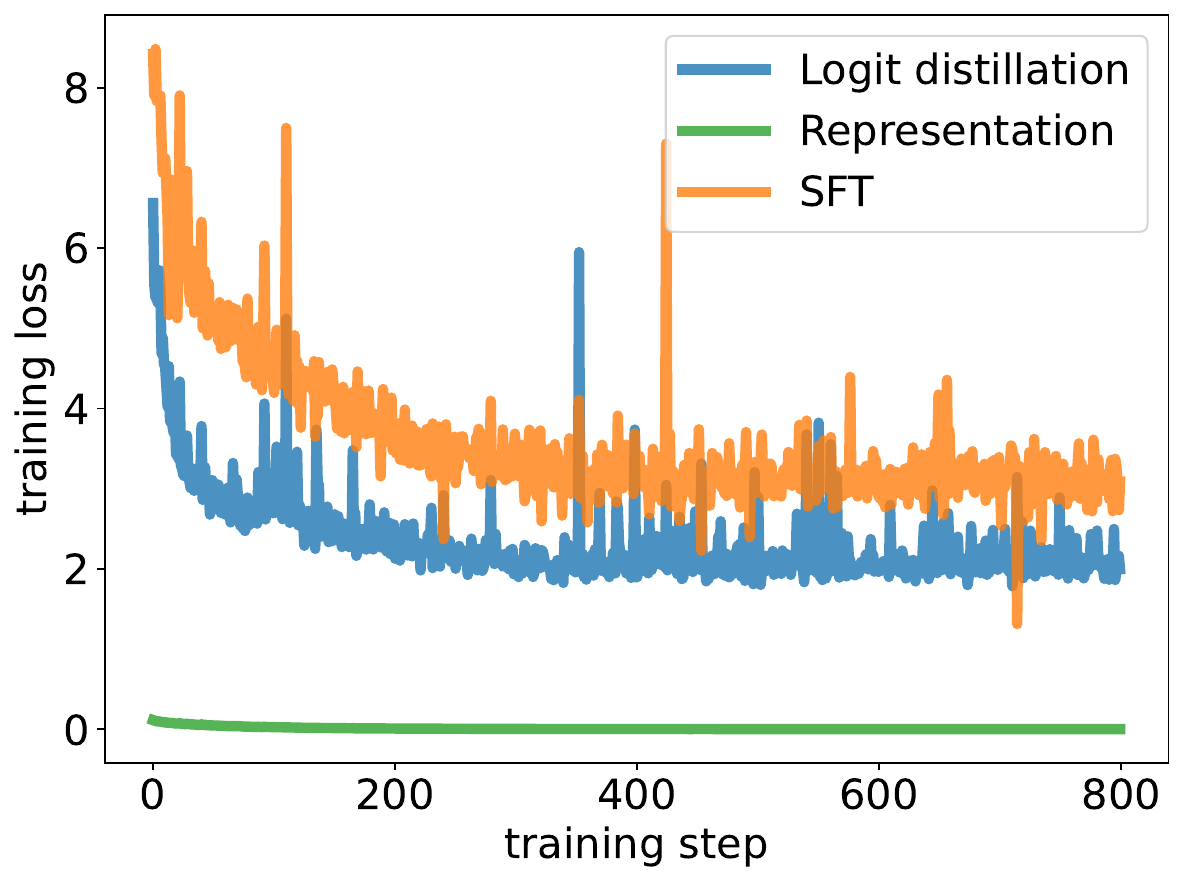}
    }
    \subfloat{
        \includegraphics[width=0.245\textwidth]{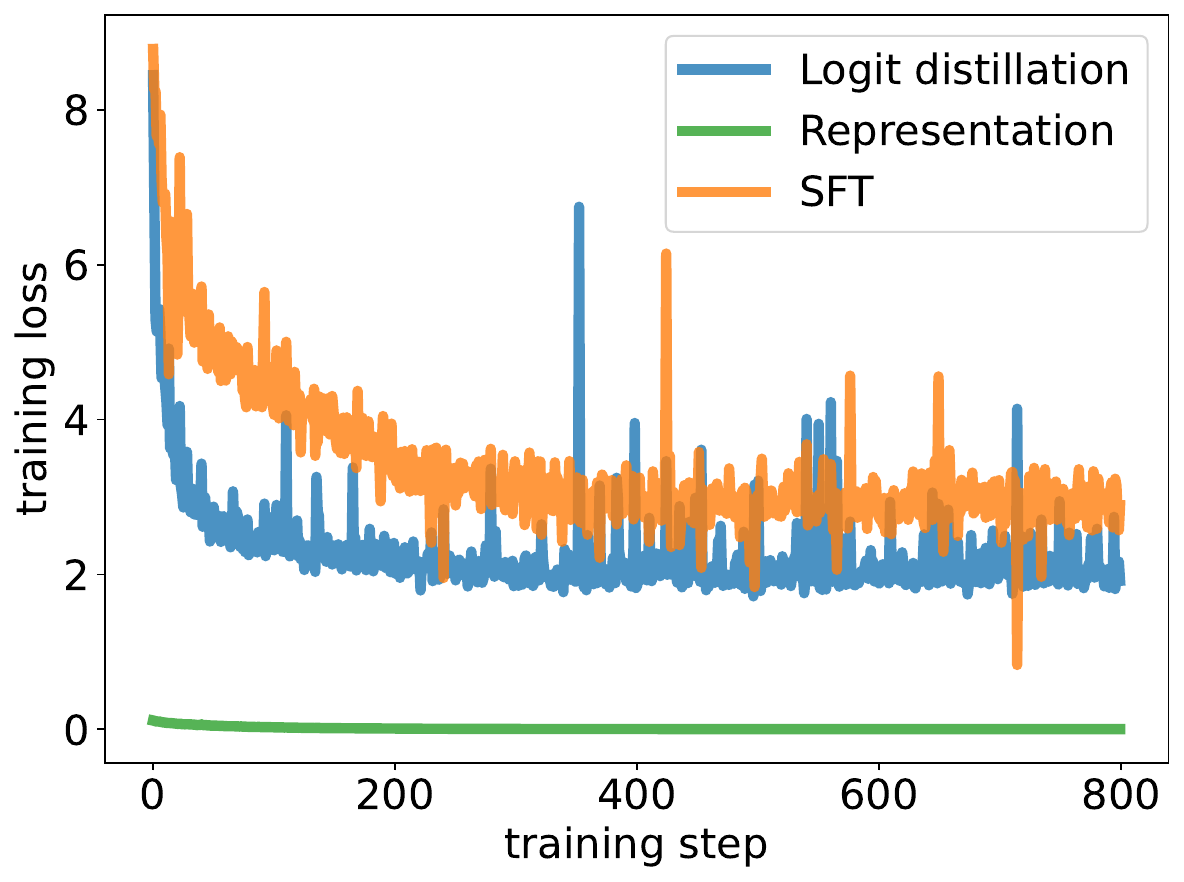}
    }
    \subfloat{
        \includegraphics[width=0.245\textwidth]{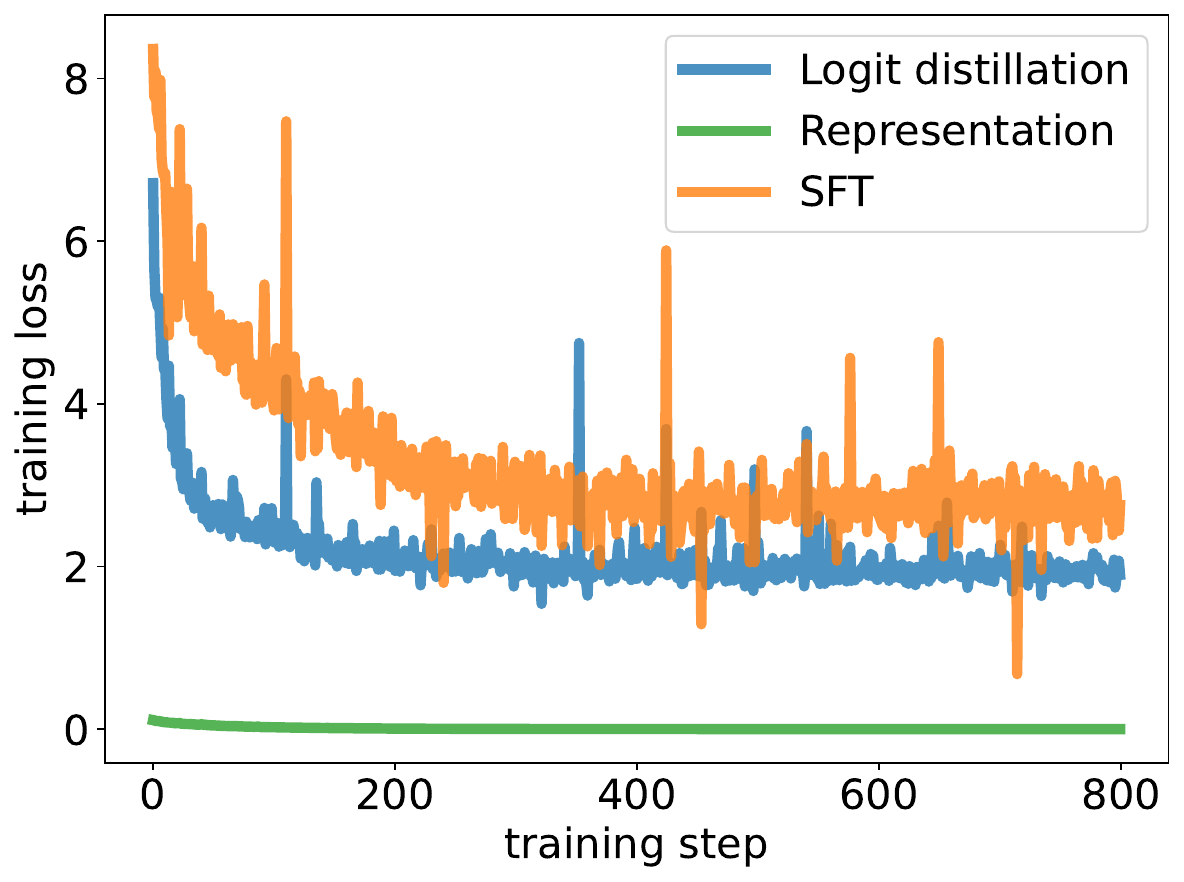}
    }
    \subfloat{
        \includegraphics[width=0.245\textwidth]{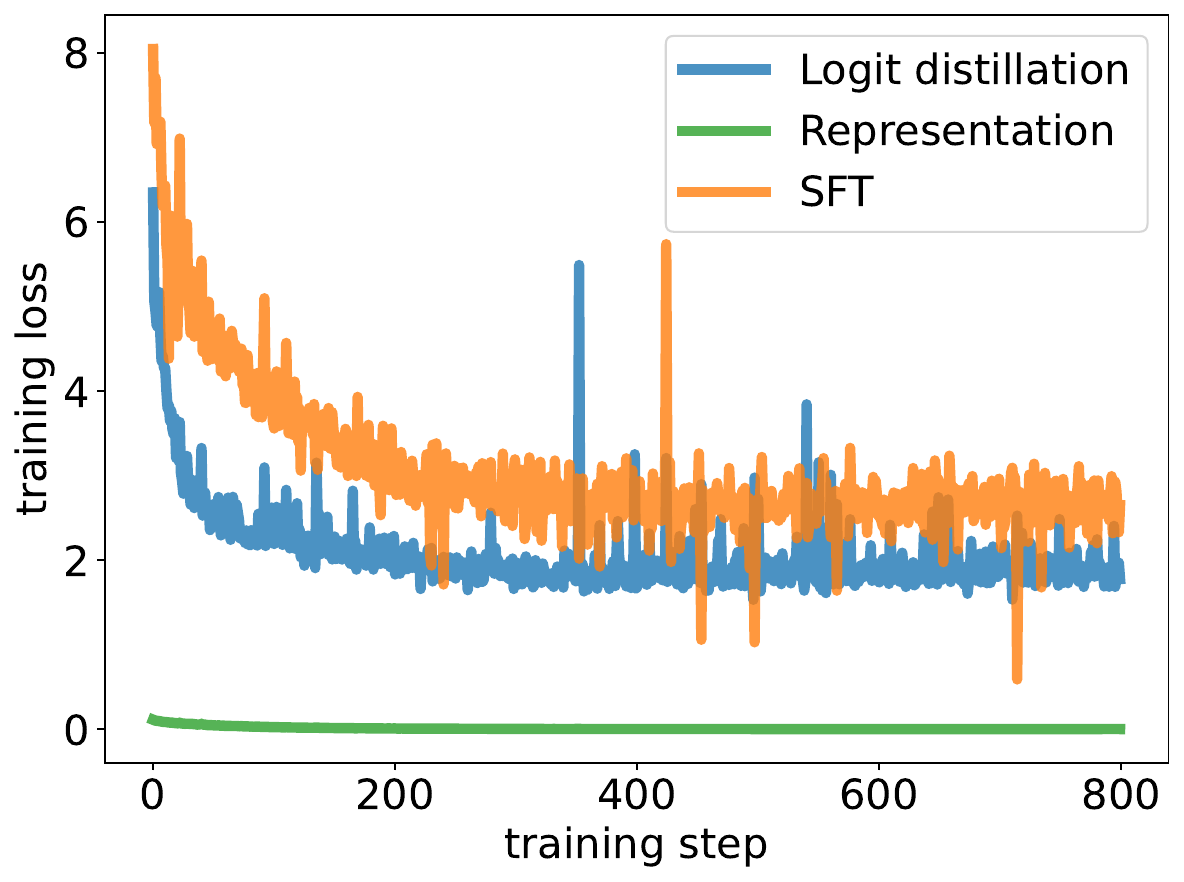}
    }

    \subfloat{
        \includegraphics[width=0.245\textwidth]{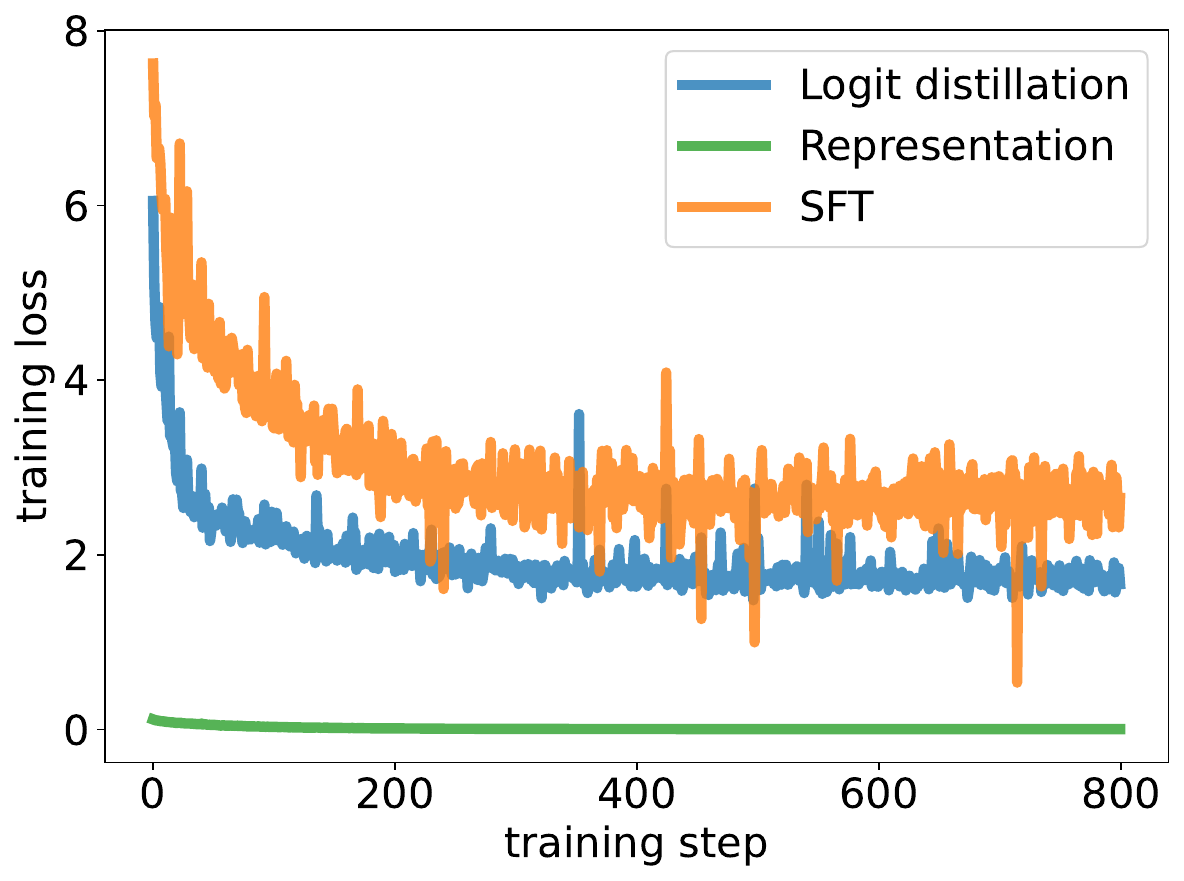}
    }
    \subfloat{
        \includegraphics[width=0.245\textwidth]{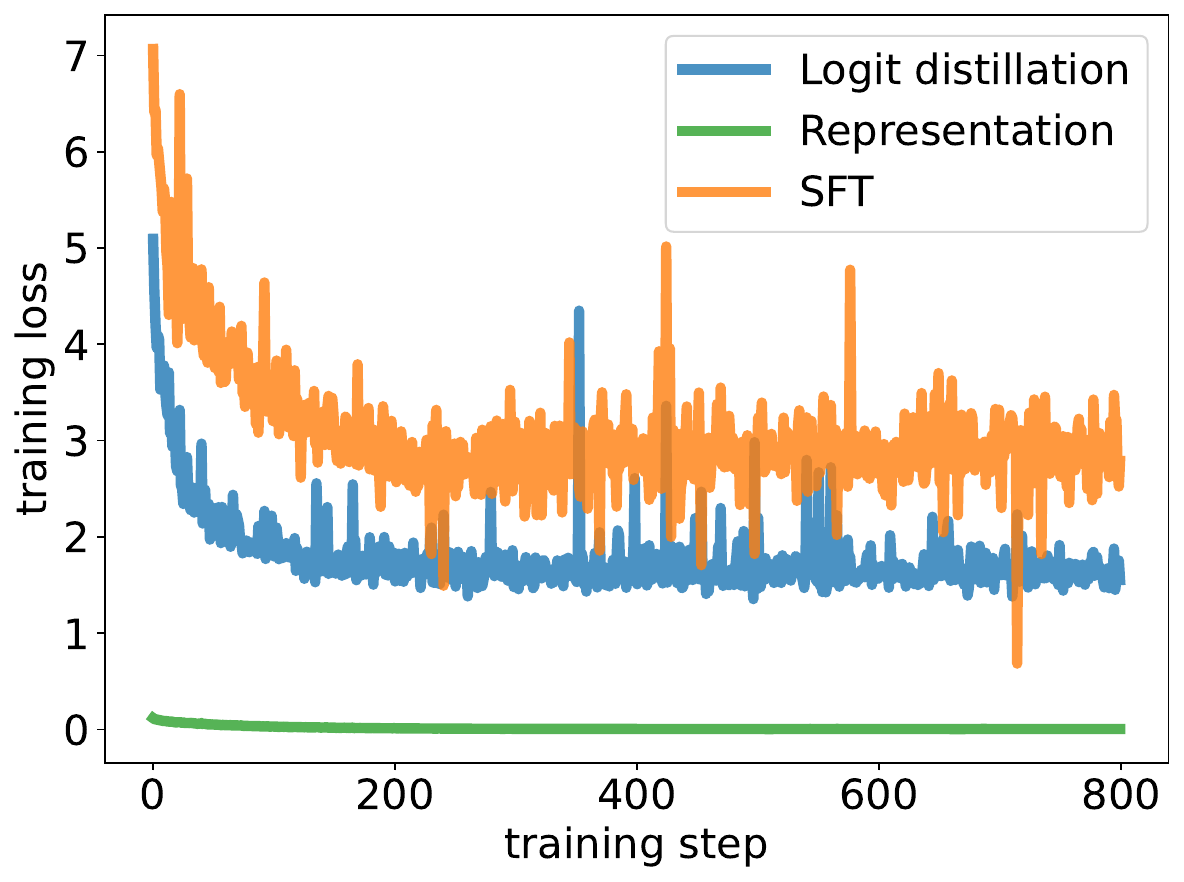}
    }
    \subfloat{
        \includegraphics[width=0.245\textwidth]{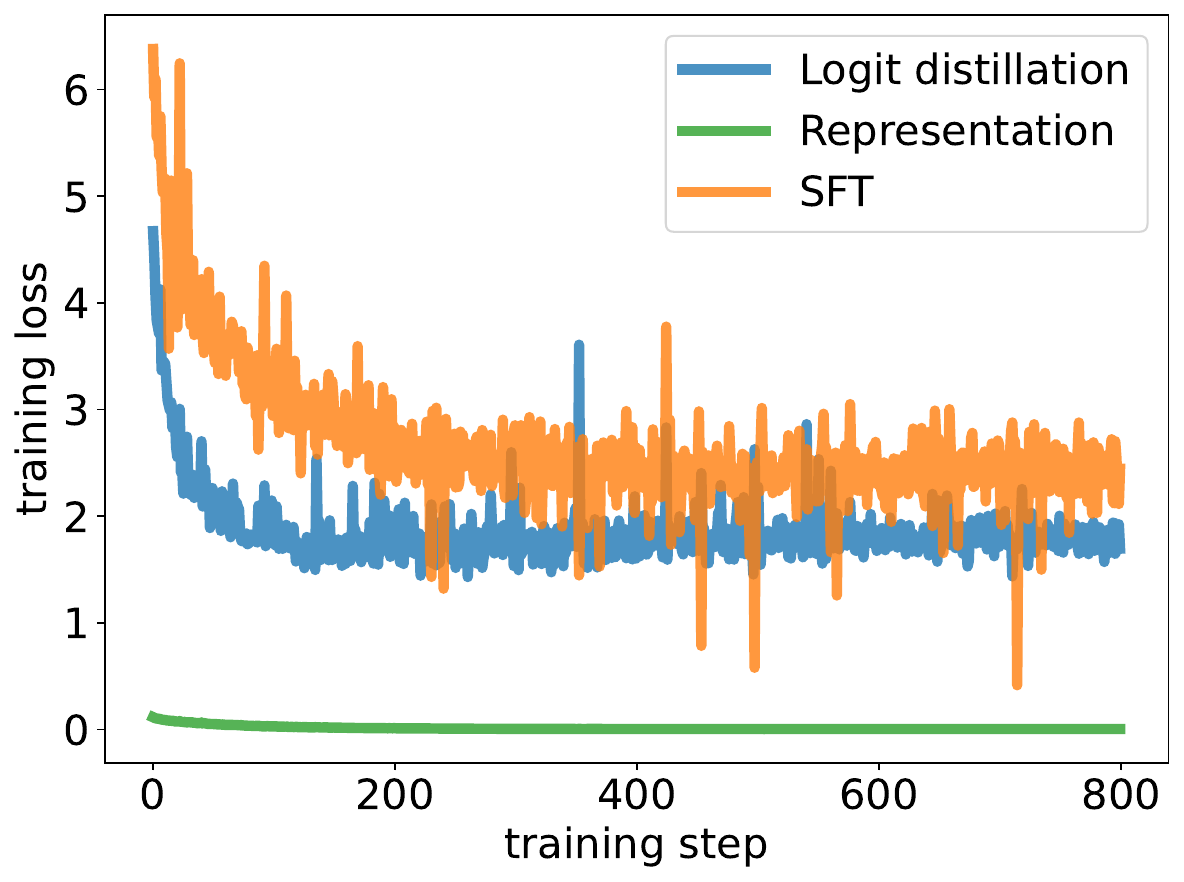}
    }
    \subfloat{
        \includegraphics[width=0.245\textwidth]{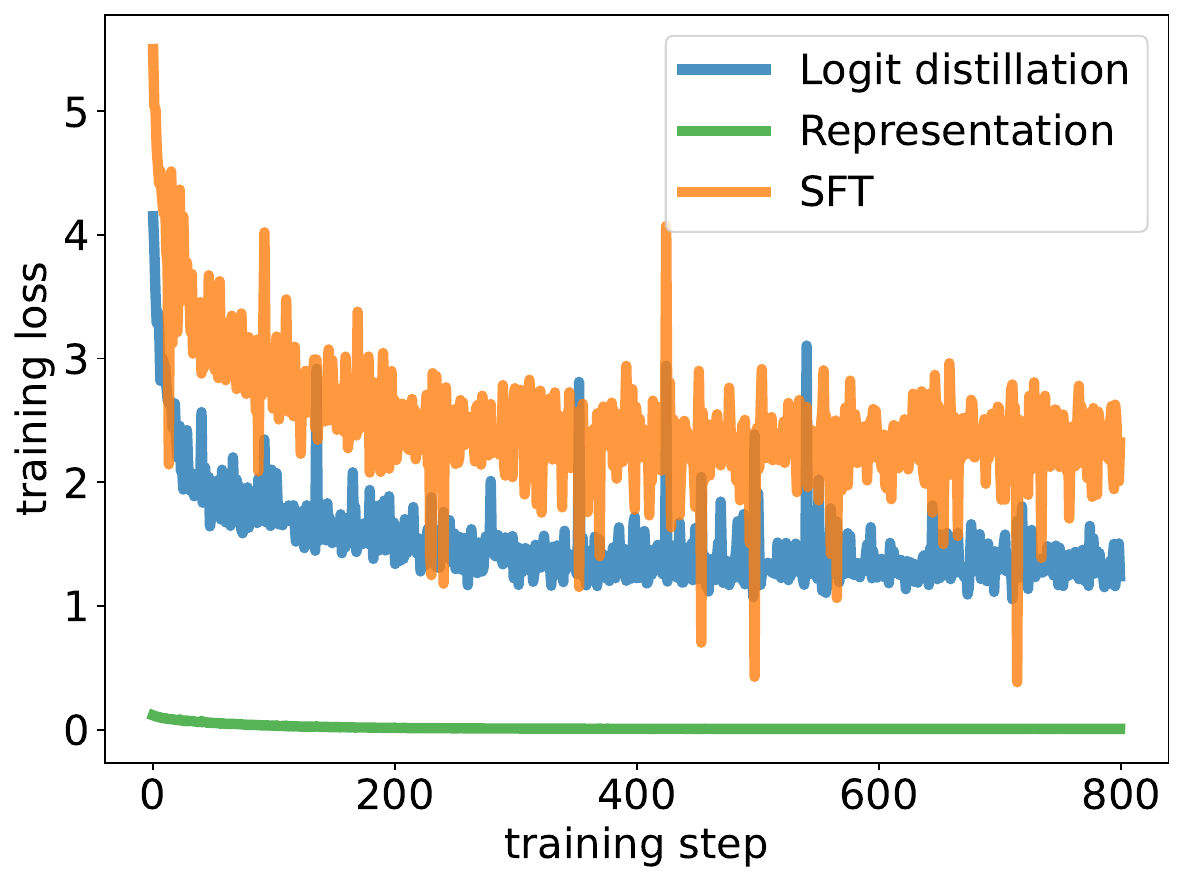}
    }

    \subfloat{
        \includegraphics[width=0.245\textwidth]{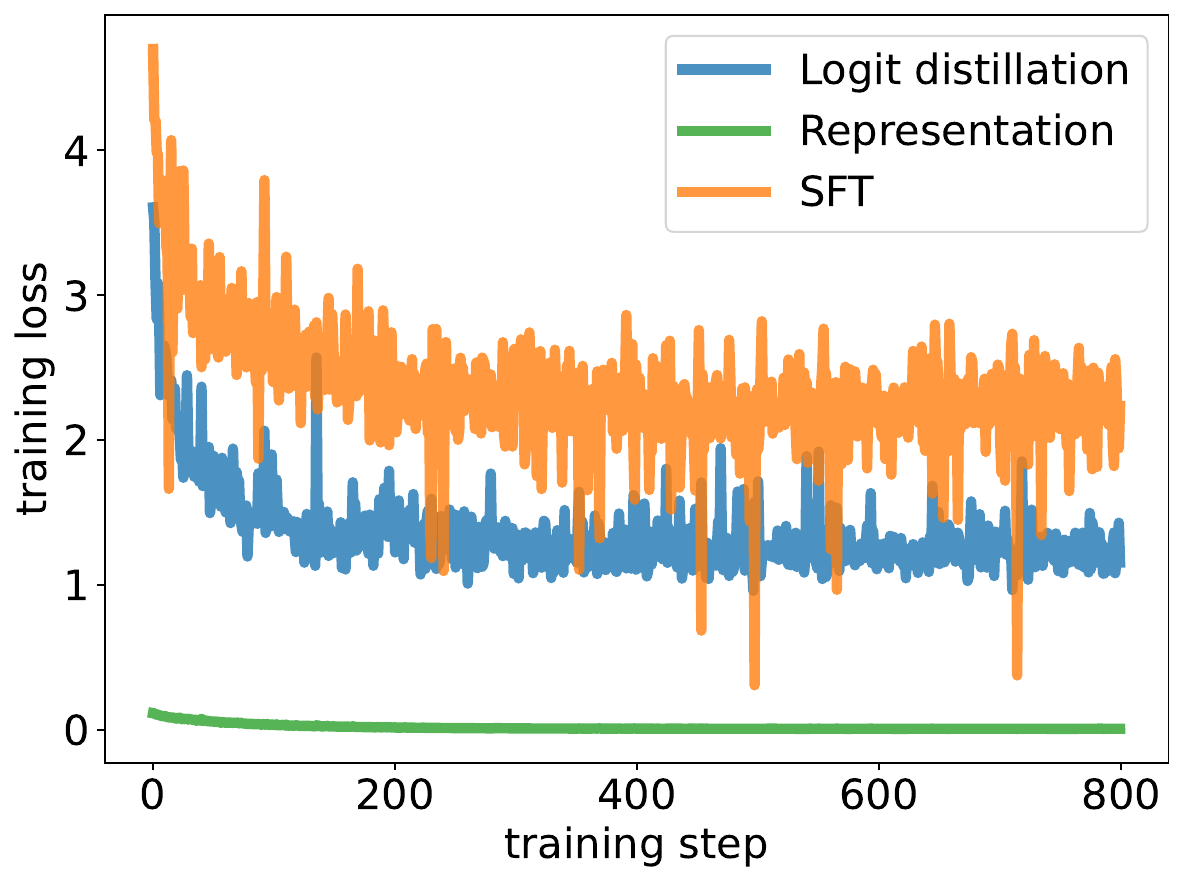}
    }
    \subfloat{
        \includegraphics[width=0.245\textwidth]{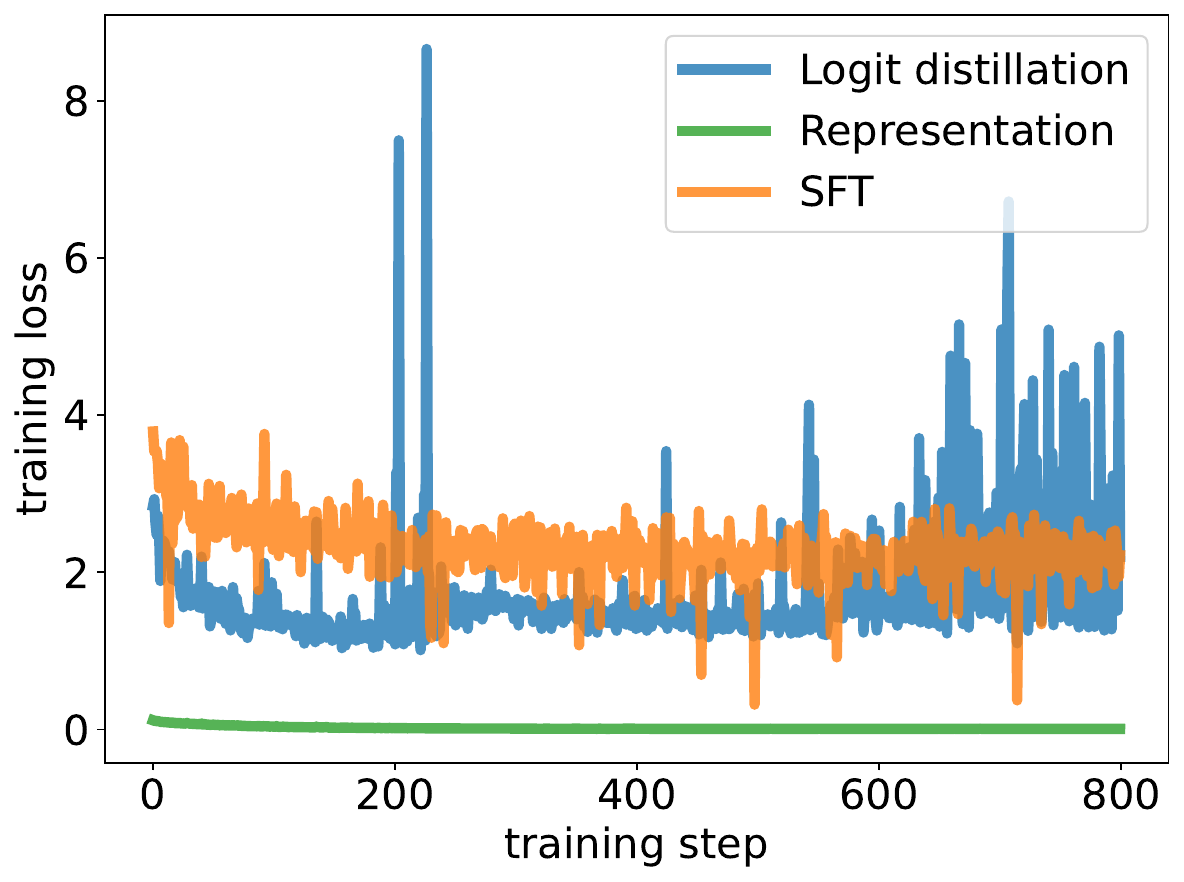}
    }
    \subfloat{
        \includegraphics[width=0.245\textwidth]{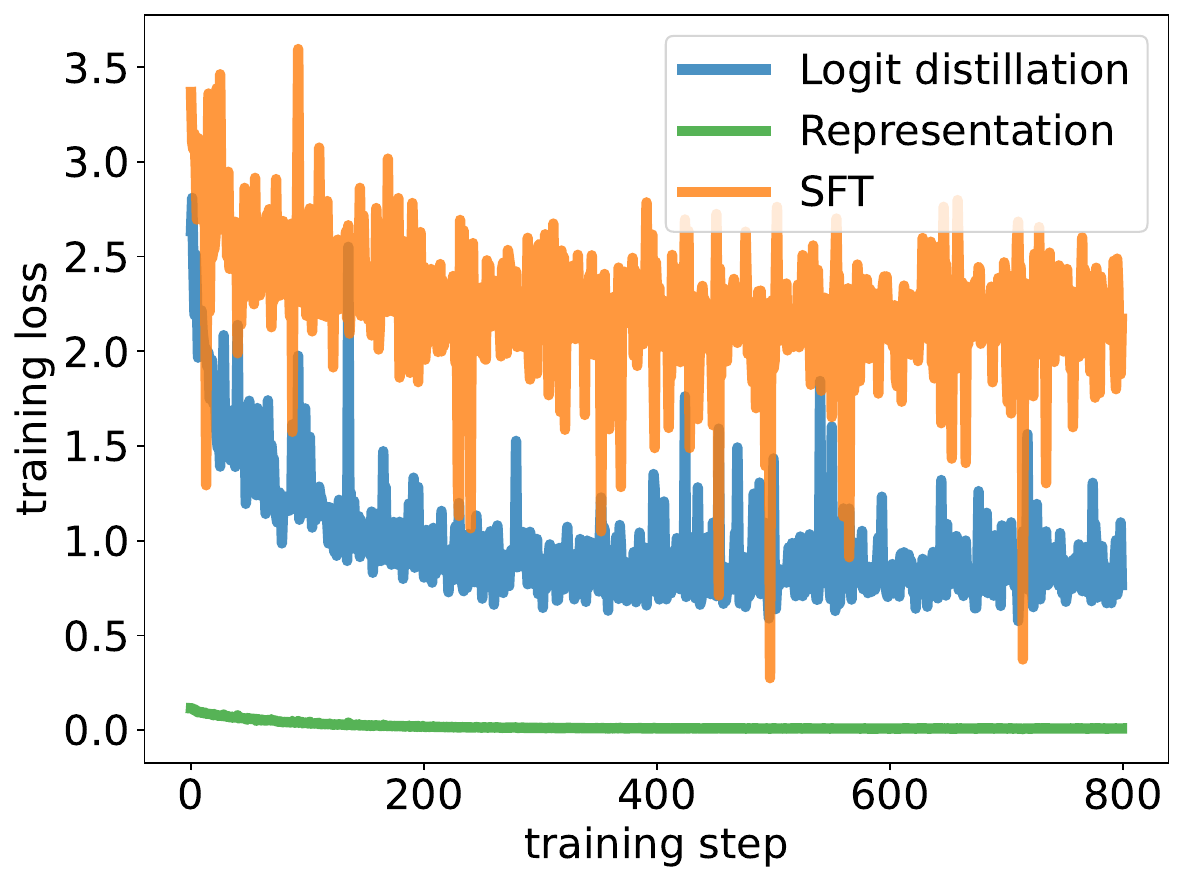}
    }
    \subfloat{
        \includegraphics[width=0.245\textwidth]{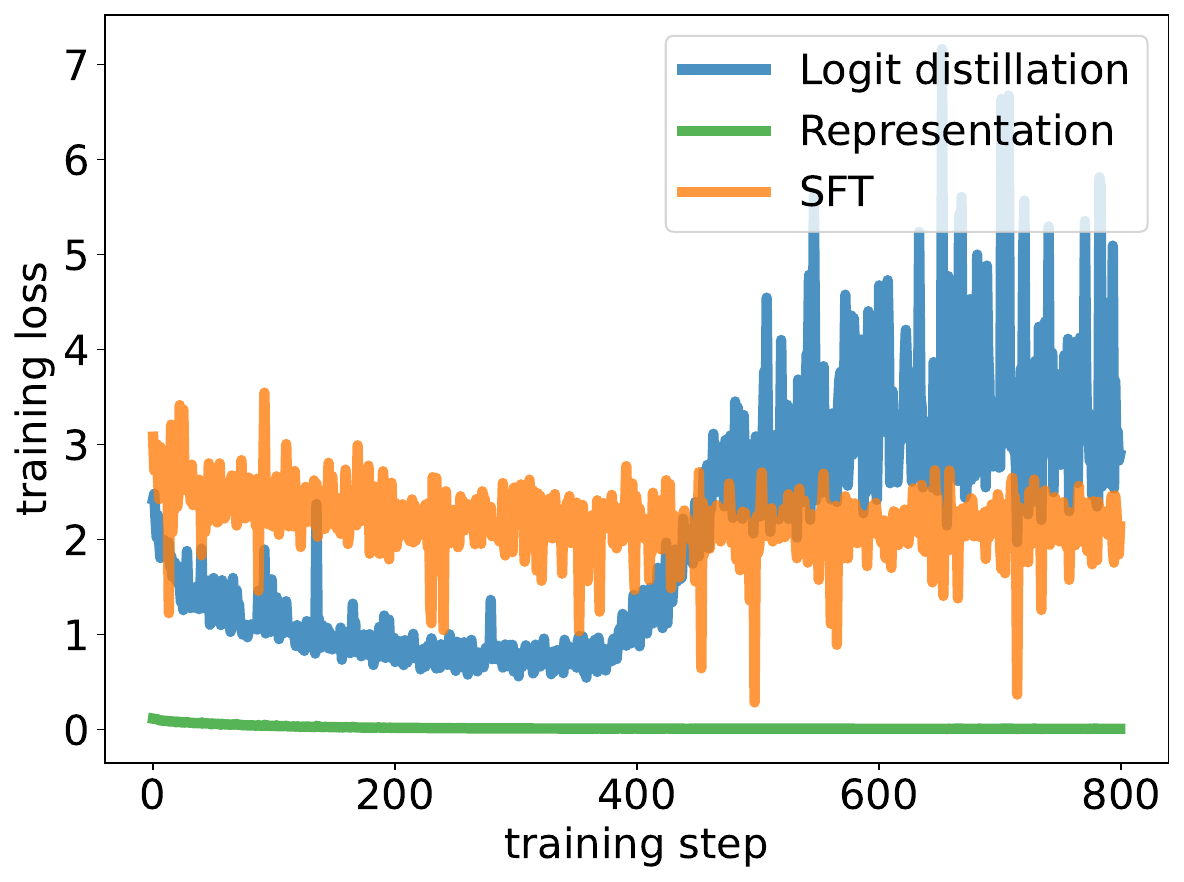}
    }

    \caption{\textbf{Low-rank linear adapter training curves for the first 24 Mistral 7b blocks with a rank of 256} trained using three different objectives including (a) MSE loss defined on the representation, (b) supervised fine-tuning (SFT), and (c) logit distillation where logits are distilled from the full model. Rest of the blocks are visualized in Fig.~\ref{fig:linear_adapters_rank_256_llama2_train_loss_b}.}
    \label{fig:linear_adapters_rank_256_mistral_train_loss_a}
\end{figure}

\begin{figure}[t]
    \centering
    \subfloat{
        \includegraphics[width=0.245\textwidth]{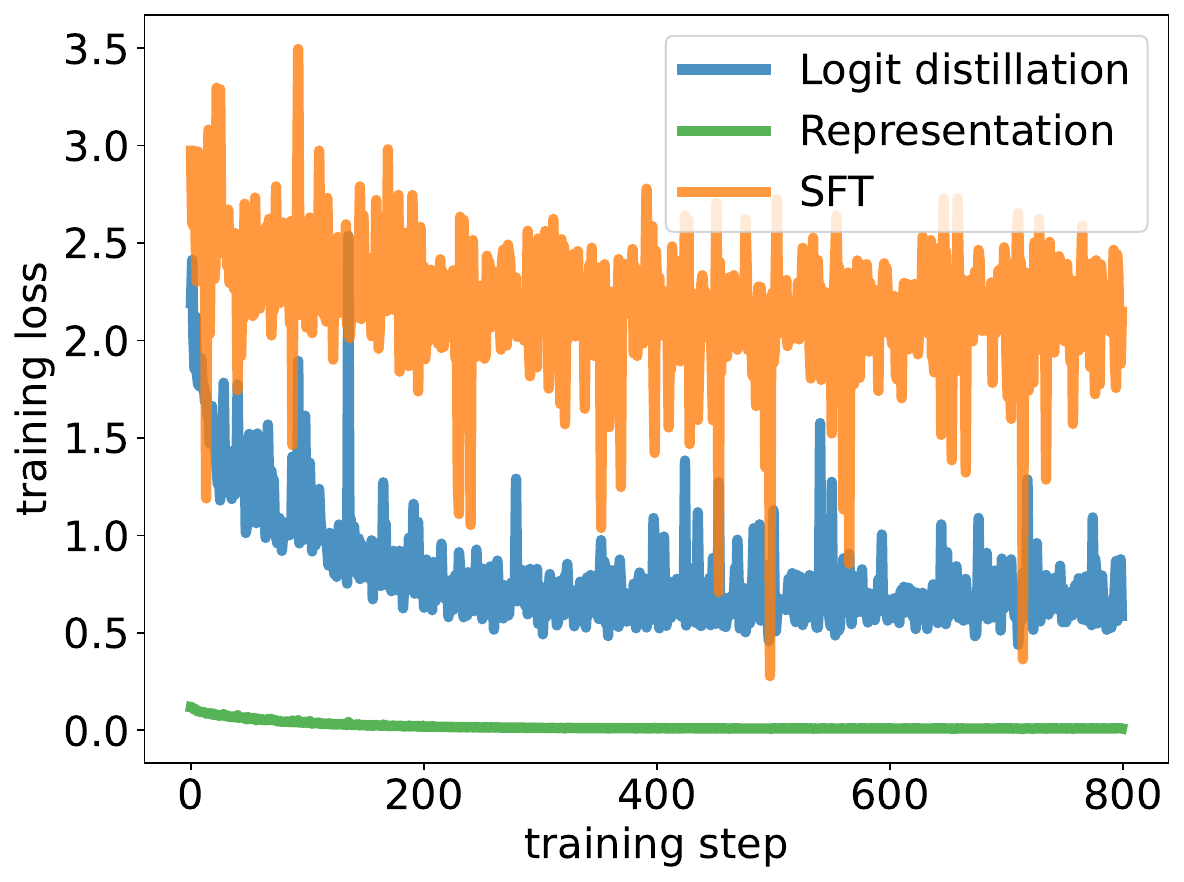}
    }
    \subfloat{
        \includegraphics[width=0.245\textwidth]{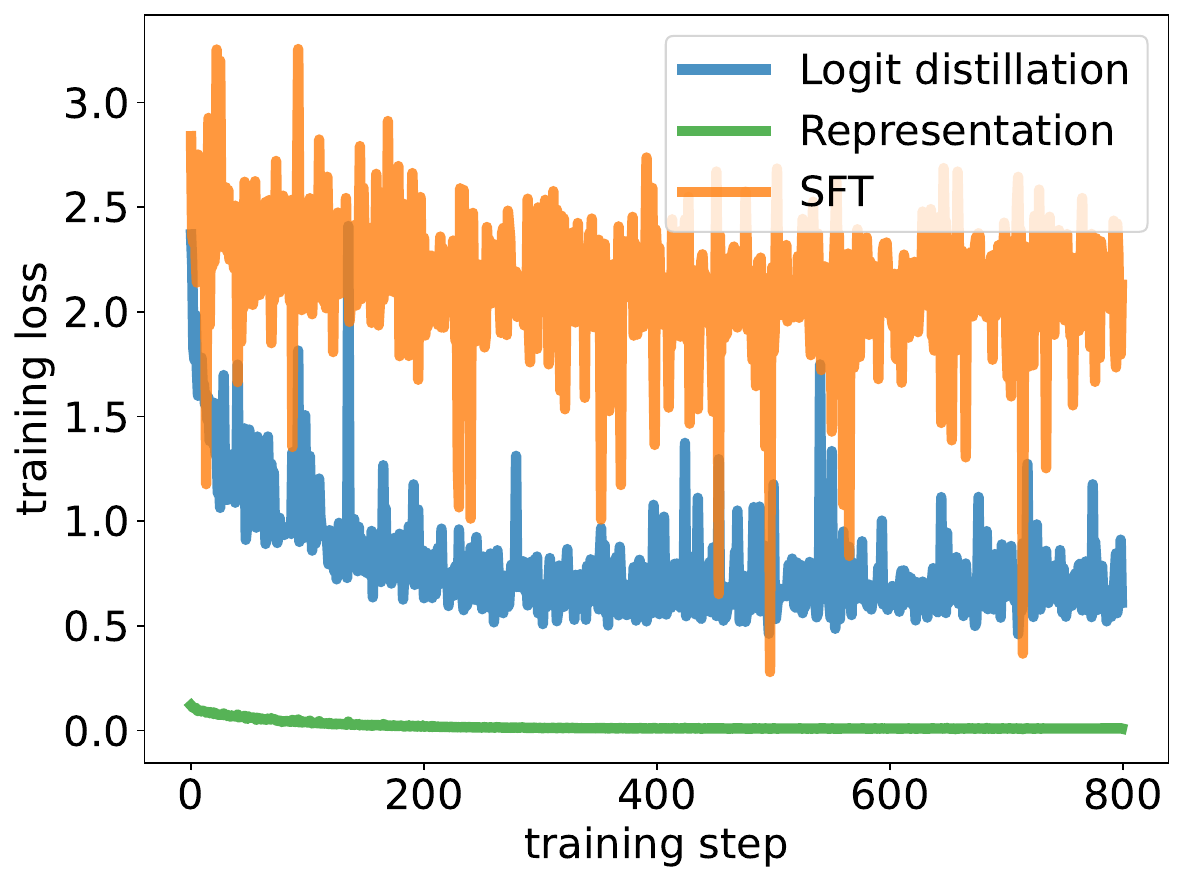}
    }
    \subfloat{
        \includegraphics[width=0.245\textwidth]{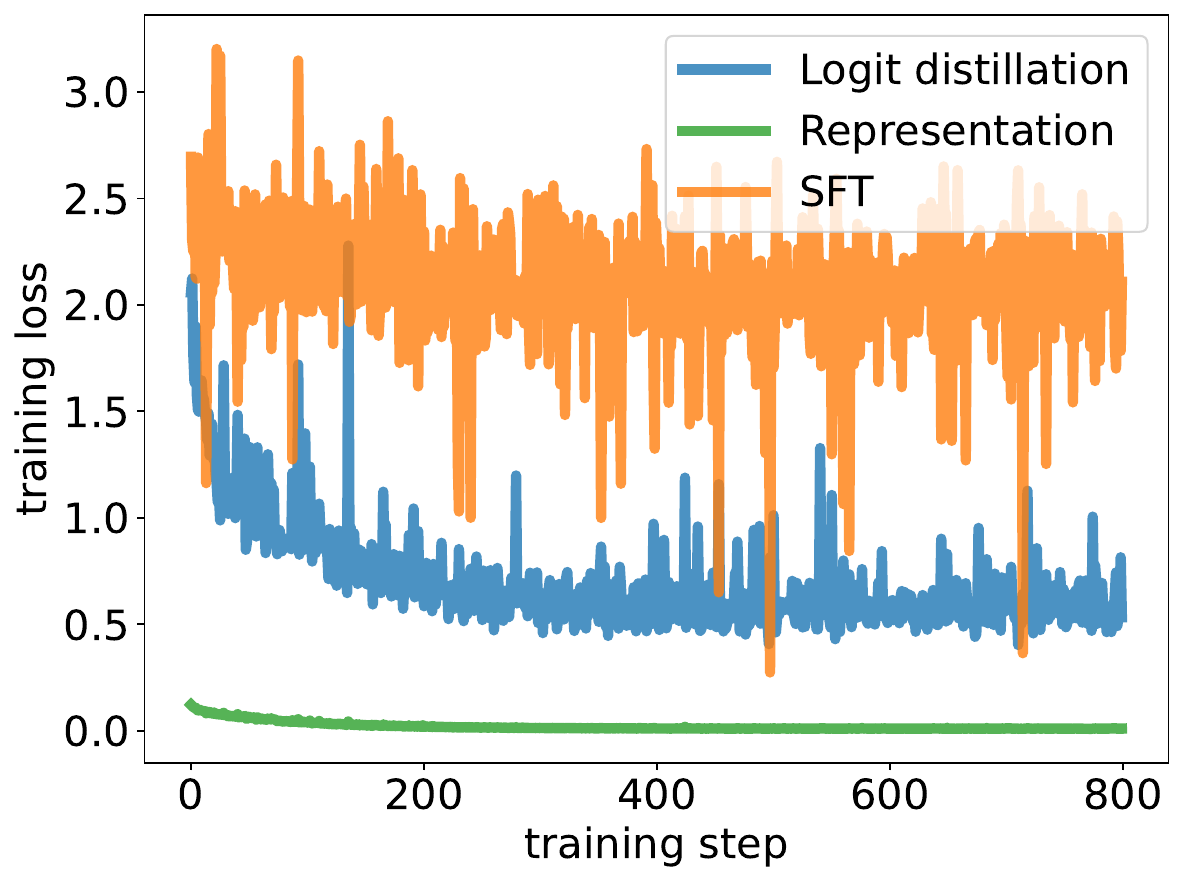}
    }
    \subfloat{
        \includegraphics[width=0.245\textwidth]{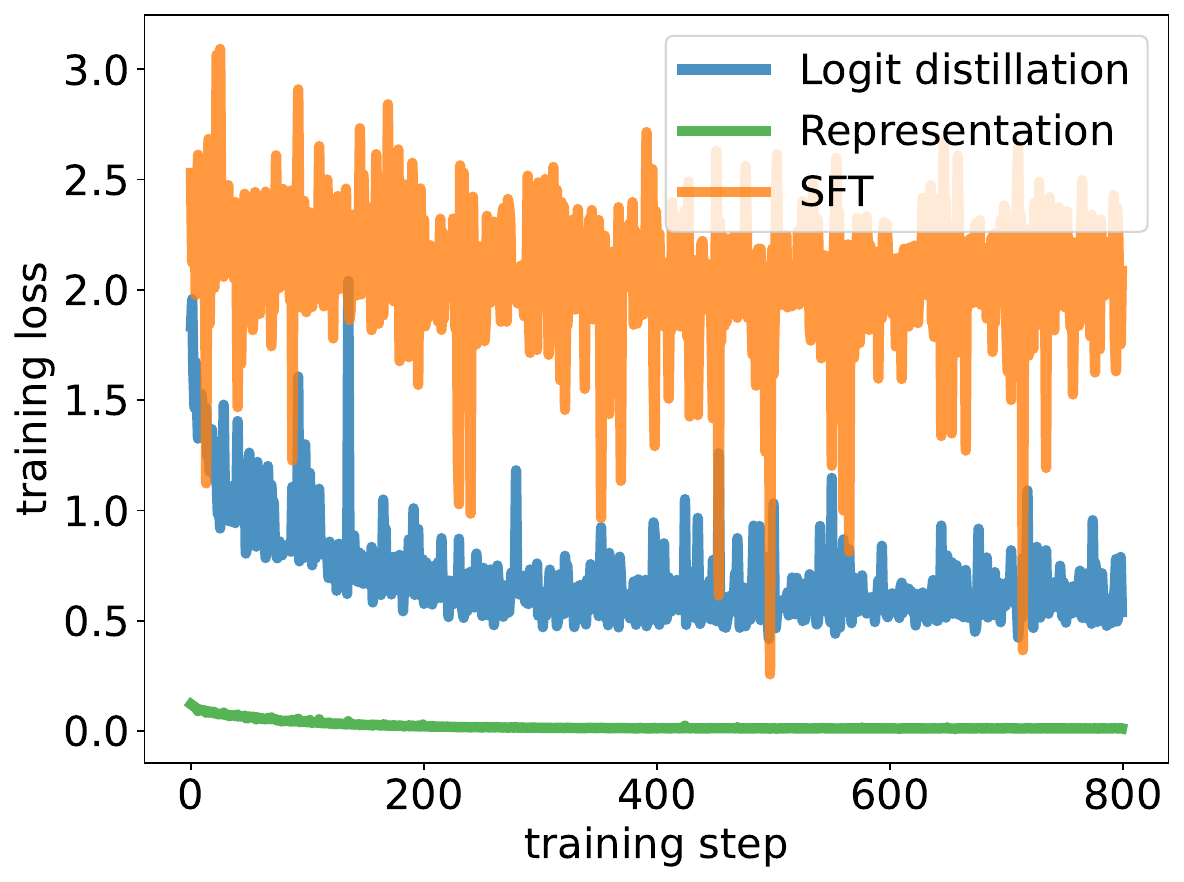}
    }

    \subfloat{
        \includegraphics[width=0.245\textwidth]{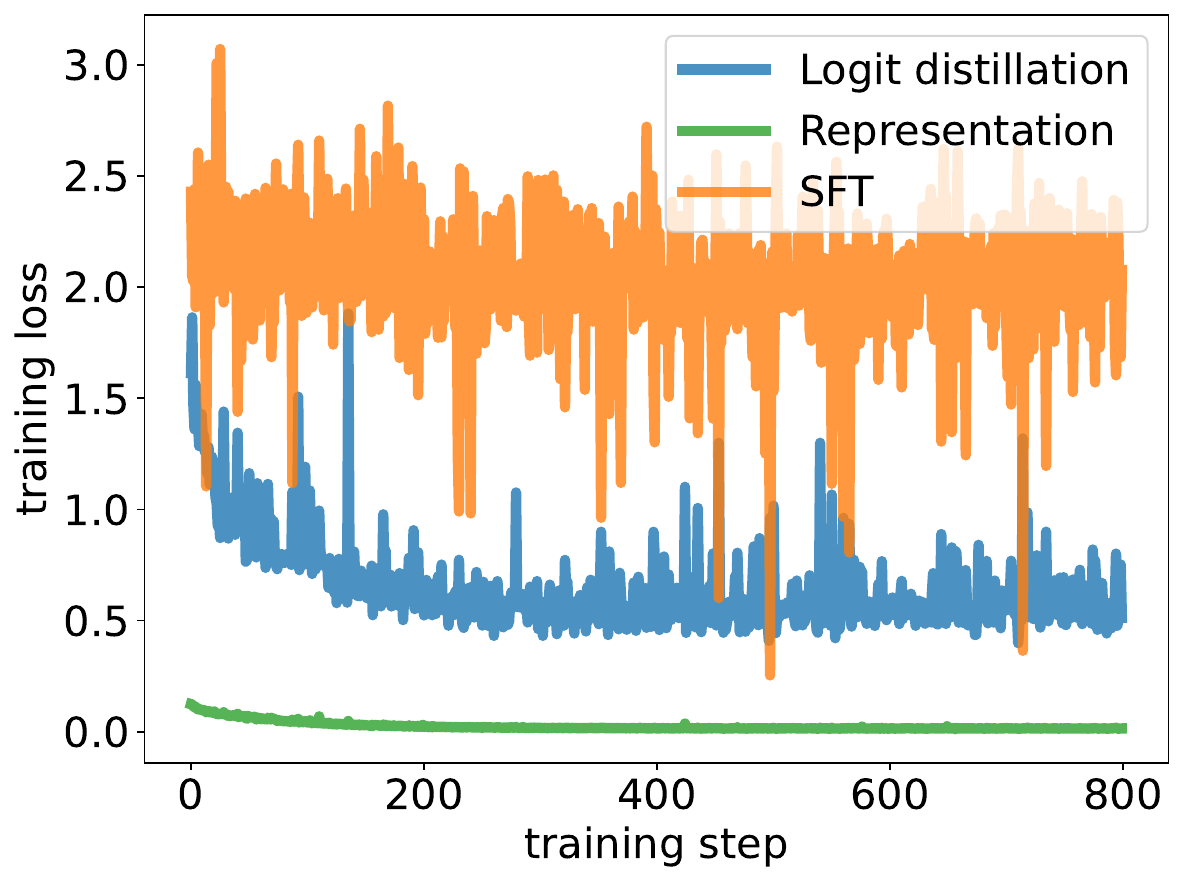}
    }
    \subfloat{
        \includegraphics[width=0.245\textwidth]{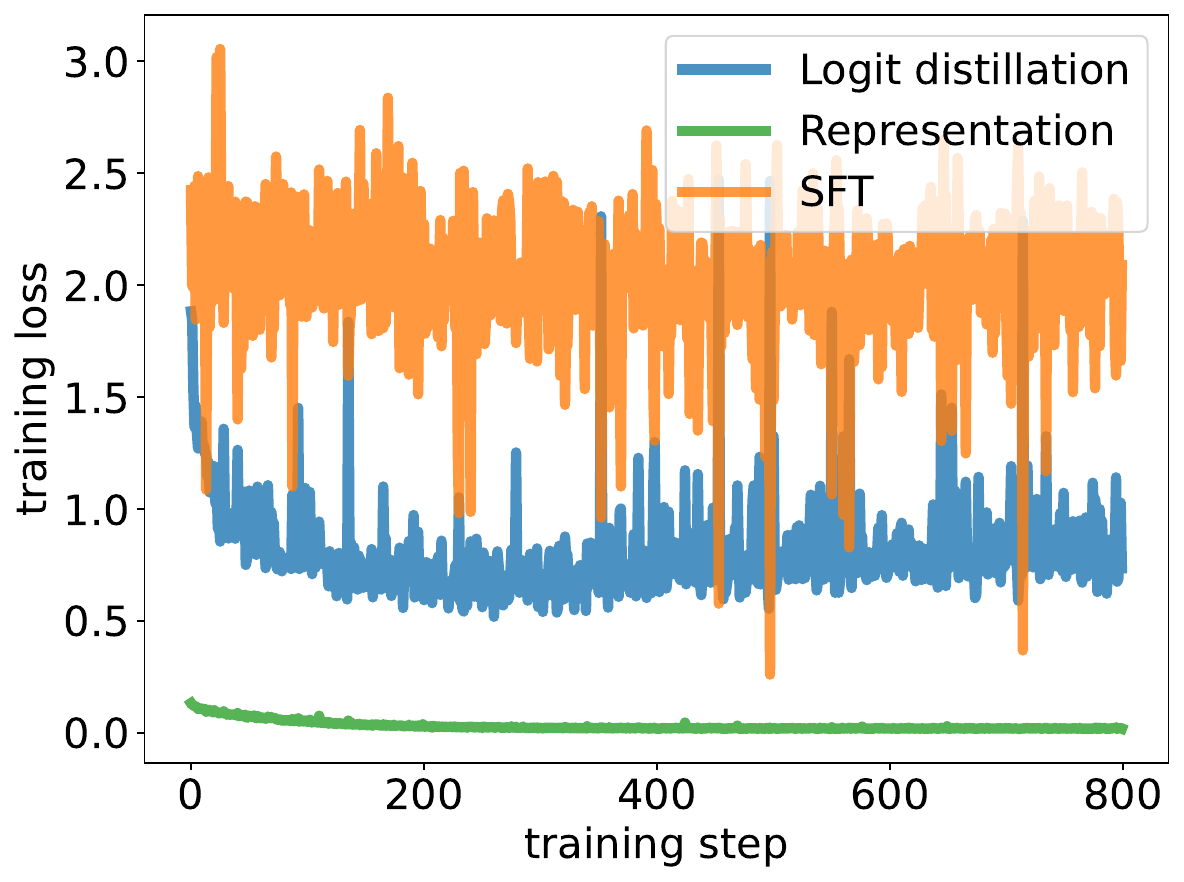}
    }
    \subfloat{
        \includegraphics[width=0.245\textwidth]{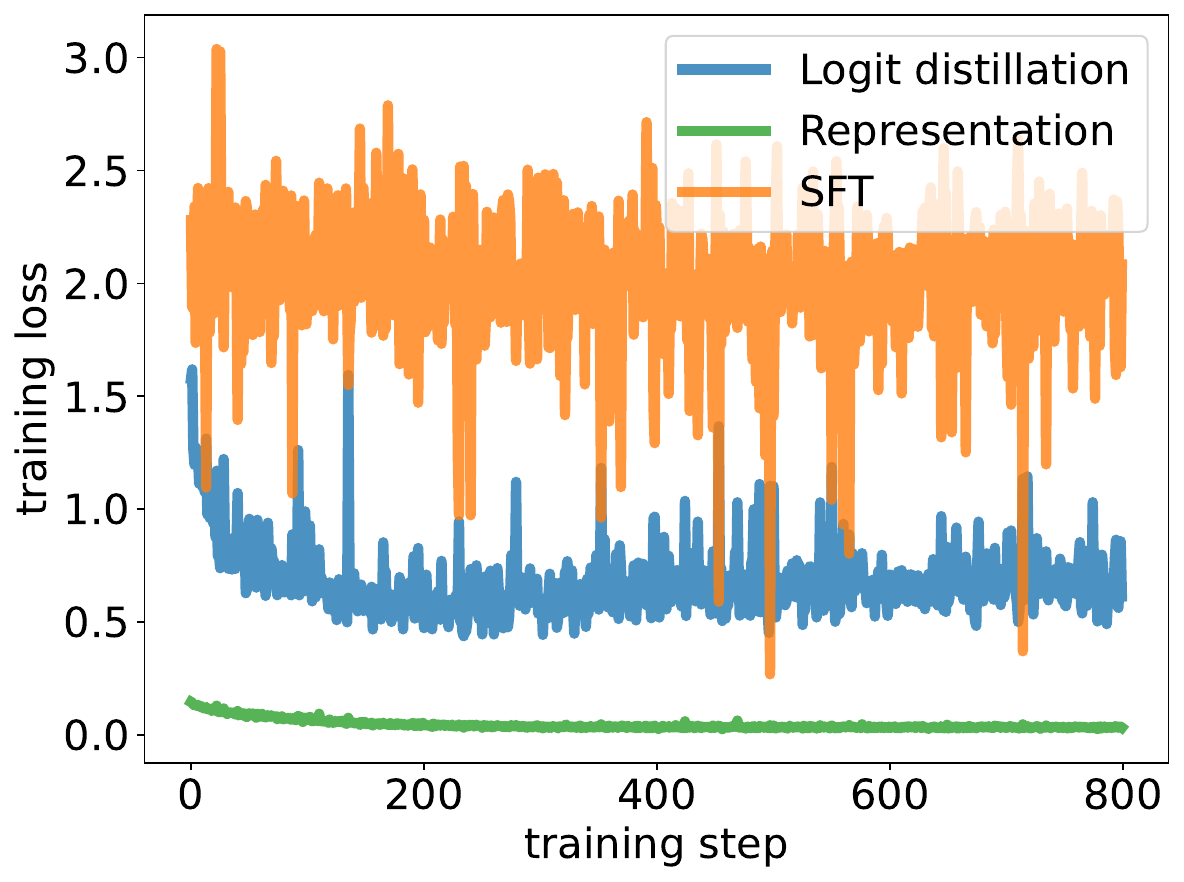}
    }
    \subfloat{
        \includegraphics[width=0.245\textwidth]{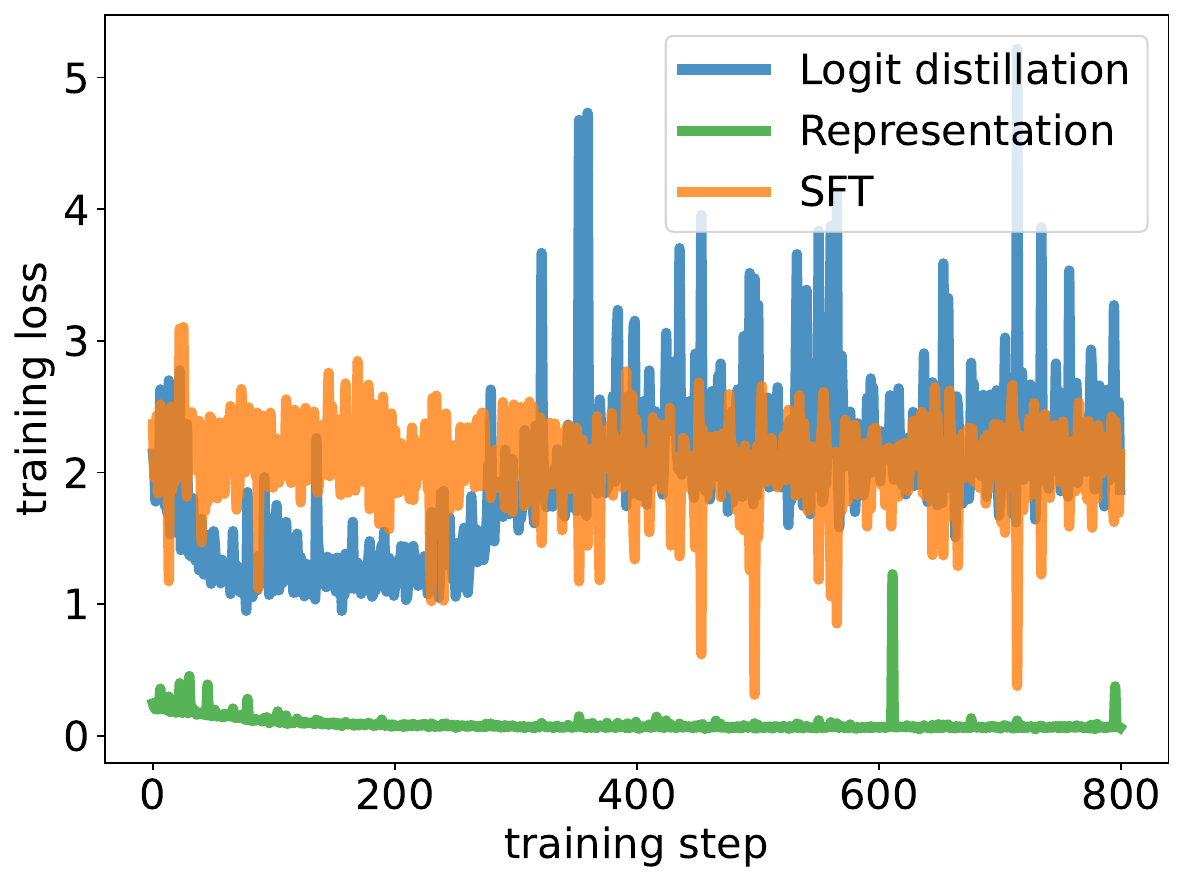}
    }

    \caption{\textbf{Low-rank linear adapter training curves for the last 8 Mistral 7b blocks with a rank of 256} trained using three different objectives including (a) MSE loss defined on the representation, (b) supervised fine-tuning (SFT), and (c) logit distillation where logits are distilled from the full model. The first set of blocks are visualized in Fig.~\ref{fig:linear_adapters_rank_256_llama2_train_loss_a}.}
    \label{fig:linear_adapters_rank_256_mistral_train_loss_b}
\end{figure}

The loss curves for the training of the low-rank adapter with a rank of 32 on Mistral are visualized in Fig.~\ref{fig:linear_adapters_rank_256_mistral_train_loss_a} and Fig.~\ref{fig:linear_adapters_rank_256_mistral_train_loss_b}.

\section{Evolution of cosine block influence during training}
\label{appendix:pythia_cosine_over_time}

\begin{figure}
    \centering
    \includegraphics[width=0.6\textwidth]{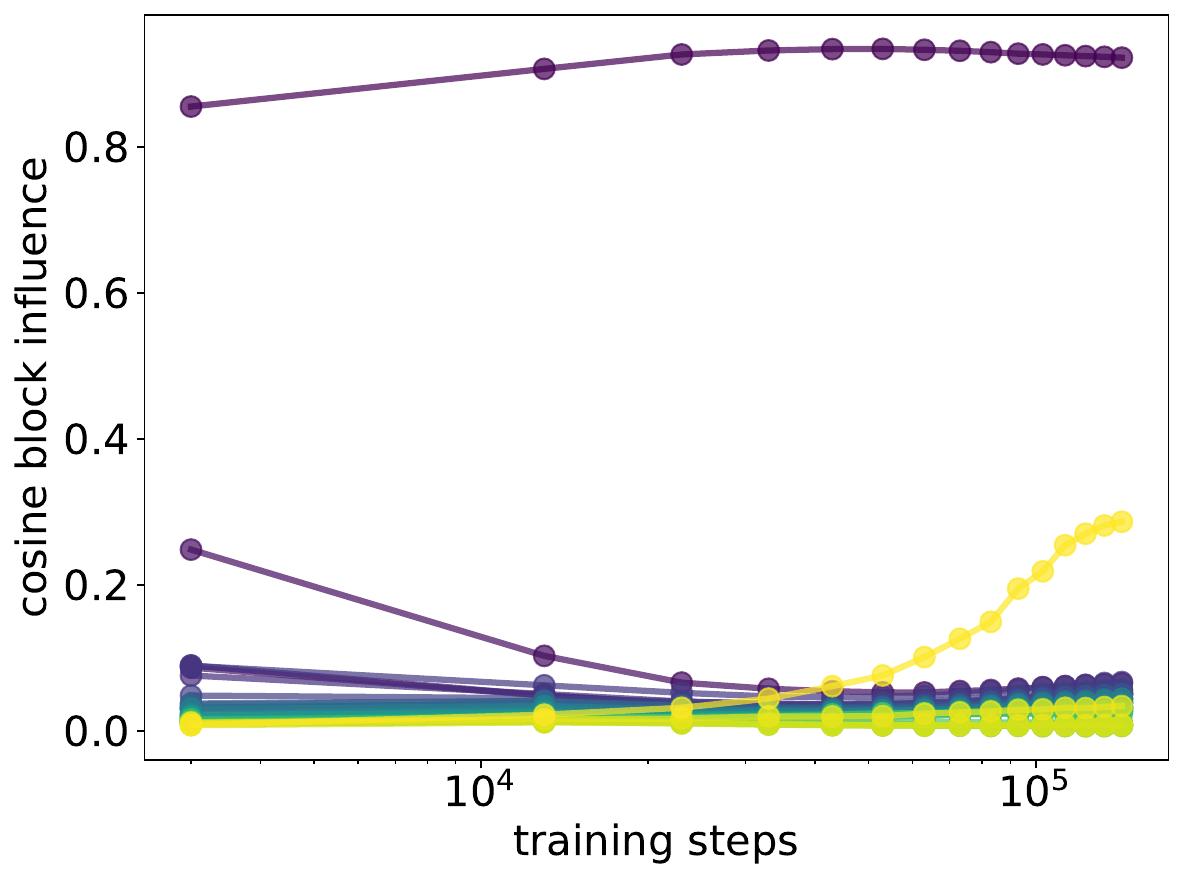}
    \caption{\textbf{Evolution of the cosine block influence metric during training} computed over Pythia-2.8b~\citep{biderman2023pythia} model. Darker colors represent lower blocks while lighter colors represent higher blocks.}
    \label{fig:pythia_cosine_block_influence}
\end{figure}

The evolution of the cosine block influence metric on the Pythia 2.8B model~\citep{biderman2023pythia} is visualized in Fig.~\ref{fig:pythia_cosine_block_influence}.
It is clear from the figure that the first block of the model has been assigned a high cosine influence right from the start.
On the other hand, the influence of the second block starts high but goes down during training.
Finally, the last block starts with a small influence but gains a significant influence at the end.
These rankings are aligned with the results on LLaMa-2 and Mistral where we see that the first and the last blocks are particularly important when considering the cosine influence.
